# Supplementary material for: Nice pseudo-Riemannian nilsolitons
Source: arXiv:2107.07767 ancillary file (2021-07-16)
Supplement: Supplementary file 1 [file ancillaryNiceNilsoliton.pdf]

# Nice pseudo-Riemannian nilsolitons - ancillary file

Diego Conti and Federico A. Rossi

July 16, 2021

## A Tables

### A.1 Nice nilpotent Lie algebras of dimension 8 with $\dim \text{coker } M_\Delta \leq 1$

Table A.1: Irreducible nice nilpotent Lie algebras of dimension 8 with  $\dim \text{coker } M_\Delta \leq 1$  that admit a diagonal nilsoliton metric of type Nil4

| Name      | $\mathfrak{g}$                                                                | $N$                                            | Signatures $\mathbf{S}$               |
|-----------|-------------------------------------------------------------------------------|------------------------------------------------|---------------------------------------|
| 8654321:1 | $0, 0, e^{12}, e^{13}, e^{14}, e^{15}, e^{16}, e^{17}$                        | $1/29(1, 26, 27, 28, 29, 30, 31, 32)$          | $\{\emptyset, 12468, 1357, 2345678\}$ |
| 8654321:2 | $0, 0, e^{12}, e^{13}, e^{14}, e^{15}, e^{16}, e^{17} + e^{23}$               | $19/159(1, 5, 6, 7, 8, 9, 10, 11)$             | $\{\emptyset, 12468\}$                |
| 8654321:3 | $0, 0, e^{12}, e^{13}, e^{14}, e^{15}, e^{16} + e^{23}, e^{24} + e^{17}$      | $25/186(1, 4, 5, 6, 7, 8, 9, 10)$              | $\{\emptyset, 1357\}$                 |
| 8654321:4 | $0, 0, -e^{12}, e^{13}, e^{14}, e^{15}, e^{16}, e^{25} + e^{34} + e^{17}$     | $43/281(1, 3, 4, 5, 6, 7, 8, 9)$               | $\{13578, 234567\}$                   |
| 865431:1  | $0, 0, -e^{12}, e^{13}, e^{14}, e^{15}, e^{25} + e^{34}, e^{16}$              | $1/19(2, 11, 13, 15, 17, 19, 28, 21)$          | $\{\emptyset, 12467, 13578, 234568\}$ |
| 865431:2  | $0, 0, -e^{12}, e^{13}, e^{14}, e^{15}, e^{25} + e^{34}, e^{16} + e^{23}$     | $17/131(1, 4, 5, 6, 7, 8, 11, 9)$              | $\{\emptyset, 13578\}$                |
| 865321:1  | $0, 0, e^{12}, e^{13}, e^{23}, e^{14}, e^{16}, e^{17}$                        | $1/281(34, 167, 201, 235, 368, 269, 303, 337)$ | $\{\emptyset, 12457, 13568, 234678\}$ |
| 86532:1   | $0, 0, -e^{12}, e^{13}, e^{23}, e^{14}, e^{16}, e^{26} + e^{34}$              | $3/19(1, 3, 4, 5, 7, 6, 7, 9)$                 | $\{\emptyset, 124578, 13568, 23467\}$ |
| 86532:2   | $0, 0, -e^{12}, e^{13}, e^{23}, e^{14}, e^{26} + e^{34}, e^{25} + e^{16}$     | $57/497(2, 3, 5, 7, 8, 9, 12, 11)$             | $\{\emptyset, 23468\}$                |
| 86531:1   | $0, 0, e^{12}, e^{13}, e^{23}, e^{14}, e^{25}, e^{16}$                        | $1/123(28, 45, 73, 101, 118, 129, 163, 157)$   | $\{\emptyset, 12458, 13567, 234678\}$ |
| 86531:2   | $0, 0, e^{12}, e^{13}, e^{23}, e^{14}, e^{24} + e^{15}, e^{16}$               | $1/106(19, 50, 69, 88, 119, 107, 138, 126)$    | $\{\emptyset, 12458, 1356, 23468\}$   |
| 86531:3   | $0, 0, -e^{12}, e^{13}, e^{23}, e^{14}, e^{25}, e^{26} + e^{34}$              | $1/257(65, 82, 147, 212, 229, 277, 311, 359)$  | $\{\emptyset, 12458, 135678, 23467\}$ |
| 86531:4   | $0, 0, e^{12}, e^{13}, e^{23}, e^{14}, e^{24} + e^{15}, e^{25} + e^{16}$      | $55/453(2, 3, 5, 7, 8, 9, 10, 11)$             | $\{\emptyset, 23468\}$                |
| 86531:11  | $0, 0, e^{12}, e^{13}, e^{23}, e^{14}, e^{25}, e^{27} + e^{16}$               | $23/81(1, 1, 2, 3, 3, 4, 4, 5)$                | $\{12367, 345678\}$                   |
| 854321:2  | $0, 0, 0, e^{12}, e^{14}, e^{15}, e^{16}, e^{17} + e^{23}$                    | $1/29(4, 19, 20, 23, 27, 31, 35, 39)$          | $\{\emptyset, 12357, 13468, 245678\}$ |
| 854321:4  | $0, 0, 0, -e^{12}, e^{14}, e^{15}, e^{16} + e^{23}, e^{34} + e^{17}$          | $2/69(5, 22, 20, 27, 32, 37, 42, 47)$          | $\{\emptyset, 1257, 1468, 245678\}$   |
| 85432:2   | $0, 0, 0, -e^{12}, e^{14}, e^{15}, e^{16}, e^{45} + e^{13} + e^{26}$          | $1/43(7, 19, 52, 26, 33, 40, 47, 59)$          | $\{123578, 13468, 234567, 3\}$        |
| 85432:3   | $0, 0, 0, -e^{12}, e^{14}, e^{15}, e^{16} + e^{23}, e^{26} + e^{45}$          | $1/124(25, 52, 100, 77, 102, 127, 152, 179)$   | $\{\emptyset, 12578, 1468, 24567\}$   |
| 85432:7   | $0, 0, 0, -e^{12}, e^{14}, e^{15}, e^{24} + e^{16}, e^{45} + e^{13} + e^{26}$ | $43/281(1, 3, 8, 4, 5, 6, 7, 9)$               | $\{13468, 234567\}$                   |
| 85421:2   | $0, 0, 0, e^{12}, e^{14}, e^{24} + e^{13}, e^{15}, e^{17}$                    | $3/17(1, 3, 6, 4, 5, 7, 6, 7)$                 | $\{123568, 13467, 234578, 3\}$        |
| 85421:3   | $0, 0, 0, e^{12}, e^{14}, e^{24}, e^{15}, e^{17} + e^{23}$                    | $1/24(5, 12, 20, 17, 22, 29, 27, 32)$          | $\{\emptyset, 12568, 1467, 24578\}$   |
| 85421:7   | $0, 0, 0, -e^{12}, e^{14}, e^{24}, e^{15} + e^{23}, e^{34} + e^{17}$          | $1/225(51, 107, 153, 158, 209, 265, 260, 311)$ | $\{\emptyset, 123568, 13467, 24578\}$ |
| 85421:8   | $0, 0, 0, -e^{12}, e^{14}, e^{24} + e^{13}, e^{15}, e^{45} + e^{27}$          | $1/17(3, 8, 16, 11, 14, 19, 17, 25)$           | $\{\emptyset, 12568, 14678, 2457\}$   |
| 85421:9   | $0, 0, 0, -e^{12}, e^{14}, e^{24} + e^{13}, e^{15} + e^{23}, e^{34} + e^{17}$ | $51/389(2, 3, 6, 5, 7, 8, 9, 11)$              | $\{123568, 13467\}$                   |
| 85421:10  | $0, 0, 0, -e^{12}, e^{14}, e^{24}, e^{15} + e^{23}, e^{45} + e^{27}$          | $1/53(14, 19, 42, 33, 47, 52, 61, 80)$         | $\{12358, 13478, 24567, 6\}$          |

Table A.1 – Continued to next page

Table A.1 – Continued from previous page

| Name      | $g$                                                                            | $N$                                            | Signatures $S$                                                |
|-----------|--------------------------------------------------------------------------------|------------------------------------------------|---------------------------------------------------------------|
| 85421:12  | $0, 0, 0, -e^{12}, e^{14}, e^{24} + e^{13}, e^{15} + e^{23}, e^{45} + e^{27}$  | $13/103(2, 3, 6, 5, 7, 8, 9, 12)$              | $\{12358, 13478\}$                                            |
| 85421:13  | $0, 0, 0, e^{12}, e^{14}, e^{24} + e^{13}, e^{15} + e^{23}, e^{26} + e^{17}$   | $51/389(2, 3, 6, 5, 7, 8, 9, 11)$              | $\{\emptyset, 24578\}$                                        |
| 85421:14  | $0, 0, 0, -e^{12}, e^{14}, e^{24}, e^{15} + e^{23}, e^{45} + e^{13} + e^{27}$  | $3/17(2, 1, 6, 3, 5, 4, 7, 8)$                 | $\{12358, 13478\}$                                            |
| 85421:15  | $0, 0, 0, e^{12}, e^{14}, e^{24} + e^{13}, e^{15}, e^{26} + e^{34} + e^{17}$   | $51/389(2, 3, 6, 5, 7, 8, 9, 11)$              | $\{\emptyset, 24578\}$                                        |
| 85421:16  | $0, 0, 0, -e^{12}, e^{14}, e^{24}, e^{15} + e^{23}, e^{26} + e^{34} + e^{17}$  | $51/389(2, 3, 6, 5, 7, 8, 9, 11)$              | $\{\emptyset, 24578\}$                                        |
| 85421:28a | $0, 0, 0, -e^{12}, e^{14}, e^{24}, e^{26} + e^{15}, e^{13} + e^{27} + e^{45}$  | $23/81(1, 1, 4, 2, 3, 3, 4, 5)$                | $\{123568, 134678, 23457, 3\}$                                |
| 85421:28b | $0, 0, 0, -e^{12}, -e^{14}, e^{24}, e^{26} + e^{15}, e^{45} + e^{13} + e^{27}$ | $23/81(1, 1, 4, 2, 3, 3, 4, 5)$                | $\{123568, 134678, 23457, 3\}$                                |
| 85321:1   | $0, 0, 0, e^{12}, e^{13}, e^{14}, e^{16}, e^{17}$                              | $1/23(2, 19, 22, 21, 24, 23, 25, 27)$          | $\{\emptyset, 12368, 12568, 1347, 1457, 2345678, 24678, 35\}$ |
| 85321:2   | $0, 0, 0, e^{12}, e^{13}, e^{24}, e^{26}, e^{27}$                              | $1/47(30, 7, 32, 37, 62, 44, 51, 58)$          | $\{\emptyset, 12368, 12568, 134678, 145678, 23457, 247, 35\}$ |
| 85321:3   | $0, 0, 0, e^{12}, e^{13}, e^{14}, e^{16}, e^{35} + e^{17}$                     | $3/293(14, 76, 59, 90, 73, 104, 118, 132)$     | $\{\emptyset, 12368, 12568, 35\}$                             |
| 85321:4a  | $0, 0, 0, e^{12}, e^{13}, e^{24}, e^{26}, e^{27} + e^{35}$                     | $1/5(3, 1, 2, 4, 5, 5, 6, 7)$                  | $\{\emptyset, 12368, 12568, 134678, 145678, 23457, 247, 35\}$ |
| 85321:4b  | $0, 0, 0, -e^{12}, e^{13}, e^{24}, e^{26}, e^{27} + e^{35}$                    | $1/5(3, 1, 2, 4, 5, 5, 6, 7)$                  | $\{\emptyset, 12368, 12568, 134678, 145678, 23457, 247, 35\}$ |
| 85321:5   | $0, 0, 0, e^{12}, e^{13}, e^{14}, e^{16}, e^{17} + e^{23}$                     | $1/26(5, 16, 20, 21, 25, 26, 31, 36)$          | $\{1268, 147, 245678, 5\}$                                    |
| 85321:6   | $0, 0, 0, e^{12}, e^{13}, e^{24}, e^{26}, e^{27} + e^{15}$                     | $1/57(23, 15, 37, 38, 60, 53, 68, 83)$         | $\{12457, 15, 23568, 345678\}$                                |
| 85321:7   | $0, 0, 0, e^{12}, e^{13}, e^{14}, e^{16}, e^{24} + e^{17}$                     | $1/21(4, 12, 19, 16, 23, 20, 24, 28)$          | $\{\emptyset, 12368, 12568, 35\}$                             |
| 85321:8   | $0, 0, 0, e^{12}, e^{13}, e^{24}, e^{26}, e^{27} + e^{14}$                     | $1/281(156, 52, 203, 208, 359, 260, 312, 364)$ | $\{\emptyset, 12368, 12568, 35\}$                             |
| 85321:9   | $0, 0, 0, -e^{12}, e^{13}, e^{14}, e^{16}, e^{46} + e^{27}$                    | $1/52(8, 27, 48, 35, 56, 43, 51, 78)$          | $\{\emptyset, 12368, 12568, 13478, 14578, 234567, 2467, 35\}$ |
| 85321:10  | $0, 0, 0, e^{12}, e^{13}, e^{24}, e^{26}, e^{17} + e^{46}$                     | $1/60(24, 13, 48, 37, 72, 50, 63, 87)$         | $\{\emptyset, 12368, 12568, 13467, 14567, 234578, 2478, 35\}$ |
| 85321:11  | $0, 0, 0, -e^{12}, e^{13}, e^{14}, e^{16} + e^{23}, e^{34} + e^{17}$           | $1/9(2, 5, 6, 7, 8, 9, 11, 13)$                | $\{123568, 13457, 245678, 5\}$                                |
| 85321:13a | $0, 0, 0, e^{12}, e^{13}, e^{14}, e^{16}, e^{24} + e^{35} + e^{17}$            | $33/161(1, 3, 3, 4, 4, 5, 6, 7)$               | $\{13478, 14578, 234567, 2467\}$                              |
| 85321:13b | $0, 0, 0, -e^{12}, e^{13}, e^{14}, e^{16}, e^{24} + e^{35} + e^{17}$           | $33/161(1, 3, 3, 4, 4, 5, 6, 7)$               | $\{13478, 14578, 234567, 2467\}$                              |
| 85321:16  | $0, 0, 0, -e^{12}, e^{13}, e^{14}, e^{16} + e^{23}, e^{27} + e^{46}$           | $1/124(32, 45, 96, 77, 128, 109, 141, 186)$    | $\{\emptyset, 12368, 13478, 2467\}$                           |
| 85321:17a | $0, 0, 0, -e^{12}, e^{13}, e^{14}, e^{16}, e^{46} + e^{27} + e^{35}$           | $1/65(10, 37, 47, 47, 57, 57, 67, 104)$        | $\{\emptyset, 12368, 12568, 13478, 14578, 234567, 2467, 35\}$ |
| 85321:17b | $0, 0, 0, -e^{12}, -e^{13}, e^{14}, e^{16}, e^{27} + e^{35} + e^{46}$          | $1/65(10, 37, 47, 47, 57, 57, 67, 104)$        | $\{\emptyset, 12368, 12568, 13478, 14578, 234567, 2467, 35\}$ |
| 85321:18  | $0, 0, 0, e^{12}, e^{13}, e^{24}, e^{26}, e^{46} + e^{35} + e^{17}$            | $1/9(4, 2, 5, 6, 9, 8, 10, 14)$                | $\{\emptyset, 12368, 12568, 35\}$                             |
| 85321:19  | $0, 0, 0, e^{12}, e^{13}, e^{24}, e^{26}, e^{17} + e^{23} + e^{46}$            | $1/47(11, 13, 48, 24, 59, 37, 50, 61)$         | $\{12368, 13467, 234578, 35\}$                                |
| 85321:20  | $0, 0, 0, e^{12}, e^{13}, e^{14}, e^{24} + e^{16}, e^{26} + e^{17}$            | $2/61(7, 14, 27, 21, 34, 28, 35, 42)$          | $\{\emptyset, 1347, 1457, 35\}$                               |
| 85321:21  | $0, 0, 0, e^{12}, e^{13}, e^{24}, e^{26} + e^{14}, e^{27} + e^{16}$            | $1/31(14, 7, 24, 21, 38, 28, 35, 42)$          | $\{\emptyset, 23457, 247, 35\}$                               |
| 85321:24  | $0, 0, 0, -e^{12}, e^{13}, e^{14}, e^{24} + e^{16}, e^{27} + e^{46}$           | $1/19(4, 8, 17, 12, 21, 16, 20, 28)$           | $\{\emptyset, 13478, 14578, 35\}$                             |
| 85321:25  | $0, 0, 0, e^{12}, e^{13}, e^{24}, e^{26} + e^{14}, e^{46} + e^{17}$            | $1/53(22, 11, 42, 33, 64, 44, 55, 77)$         | $\{12368, 12568, 13467, 14567\}$                              |
| 85321:26a | $0, 0, 0, -e^{12}, e^{13}, e^{14}, e^{16} + e^{23}, e^{27} + e^{35} + e^{46}$  | $29/129(1, 2, 3, 3, 4, 4, 5, 7)$               | $\{\emptyset, 12368, 13478, 2467\}$                           |
| 85321:26b | $0, 0, 0, -e^{12}, -e^{13}, e^{14}, e^{16} + e^{23}, e^{46} + e^{27} + e^{35}$ | $29/129(1, 2, 3, 3, 4, 4, 5, 7)$               | $\{\emptyset, 12368, 13478, 2467\}$                           |
| 85321:27a | $0, 0, 0, -e^{12}, e^{13}, e^{14}, e^{16} + e^{23}, e^{27} + e^{15} + e^{46}$  | $23/81(1, 1, 3, 2, 4, 3, 4, 5)$                | $\{123568, 134578, 24567, 5\}$                                |
| 85321:27b | $0, 0, 0, -e^{12}, -e^{13}, e^{14}, e^{16} + e^{23}, e^{46} + e^{27} + e^{15}$ | $23/81(1, 1, 3, 2, 4, 3, 4, 5)$                | $\{123568, 134578, 24567, 5\}$                                |
| 85321:28  | $0, 0, 0, e^{12}, e^{13}, e^{14}, e^{24} + e^{16}, e^{26} + e^{35} + e^{17}$   | $9/73(2, 4, 5, 6, 7, 8, 10, 12)$               | $\{\emptyset, 35\}$                                           |
| 85321:29a | $0, 0, 0, e^{12}, e^{13}, e^{24}, e^{26} + e^{14}, e^{27} + e^{35} + e^{16}$   | $9/37(2, 1, 2, 3, 4, 4, 5, 6)$                 | $\{\emptyset, 23457, 247, 35\}$                               |
| 85321:29b | $0, 0, 0, -e^{12}, e^{13}, e^{24}, e^{26} + e^{14}, e^{27} + e^{35} + e^{16}$  | $9/37(2, 1, 2, 3, 4, 4, 5, 6)$                 | $\{\emptyset, 23457, 247, 35\}$                               |
| 85321:30a | $0, 0, 0, -e^{12}, e^{13}, e^{14}, e^{24} + e^{16}, e^{46} + e^{27} + e^{35}$  | $29/129(1, 2, 3, 3, 4, 4, 5, 7)$               | $\{\emptyset, 13478, 14578, 35\}$                             |
| 85321:30b | $0, 0, 0, -e^{12}, -e^{13}, e^{14}, e^{24} + e^{16}, e^{27} + e^{35} + e^{46}$ | $29/129(1, 2, 3, 3, 4, 4, 5, 7)$               | $\{\emptyset, 13478, 14578, 35\}$                             |
| 85321:32  | $0, 0, 0, e^{12}, e^{13}, e^{24}, e^{26} + e^{14}, e^{17} + e^{23} + e^{46}$   | $3/17(2, 1, 6, 3, 8, 4, 5, 7)$                 | $\{12368, 13467\}$                                            |
| 85321:36  | $0, 0, 0, e^{12}, e^{13}, e^{24}, e^{26} + e^{15}, e^{17} + e^{46}$            | $1/9(2, 3, 7, 5, 9, 8, 11, 13)$                | $\{\emptyset, 12568, 13467, 234578\}$                         |
| 85321:39  | $0, 0, 0, e^{12}, e^{13}, e^{24}, e^{26} + e^{15}, e^{46} + e^{35} + e^{17}$   | $7/23(1, 1, 2, 2, 3, 3, 4, 5)$                 | $\{\emptyset, 12568\}$                                        |
| 85321:43  | $0, 0, 0, e^{12}, e^{13}, e^{24}, e^{26} + e^{15}, e^{17} + e^{23} + e^{46}$   | $53/441(1, 3, 8, 4, 9, 7, 10, 11)$             | $\{13467, 234578\}$                                           |
| 8653:1    | $0, 0, e^{12}, e^{13}, e^{23}, e^{14}, e^{25}, e^{24} + e^{15}$                | $11/36(1, 1, 2, 3, 3, 4, 4, 4)$                | $\{\emptyset, 1245, 13567, 23467\}$                           |
| 8542:2    | $0, 0, 0, e^{12}, e^{14}, e^{24}, e^{15}, e^{13} + e^{26}$                     | $1/107(34, 35, 105, 69, 103, 104, 137, 139)$   | $\{\emptyset, 12356, 14678, 234578\}$                         |
| 8542:4    | $0, 0, 0, e^{12}, e^{14}, e^{24}, e^{15} + e^{23}, e^{13} + e^{26}$            | $21/65(1, 1, 3, 2, 3, 3, 4, 4)$                | $\{\emptyset, 12356\}$                                        |
| 8542:5    | $0, 0, 0, e^{12}, e^{14}, e^{24}, e^{15} + e^{23}, e^{25} + e^{16}$            | $1/51(15, 19, 45, 34, 49, 53, 64, 68)$         | $\{\emptyset, 12356, 13467, 2457\}$                           |

Table A.1 – Continued to next page

Table A.1 – Continued from previous page

| Name     | $g$                                                                          | $N$                                             | Signatures $S$                                                |
|----------|------------------------------------------------------------------------------|-------------------------------------------------|---------------------------------------------------------------|
| 8542:6   | $0, 0, 0, e^{12}, e^{14}, e^{24} + e^{13}, e^{15}, e^{26} + e^{34}$          | $1/59(17, 22, 44, 39, 56, 61, 73, 83)$          | $\{\emptyset, 1256, 14678, 24578\}$                           |
| 8542:8   | $0, 0, 0, e^{12}, e^{14}, e^{24} + e^{13}, e^{15}, e^{25} + e^{16}$          | $5/22(1, 2, 4, 3, 4, 5, 5, 6)$                  | $\{\emptyset, 1256, 1467, 2457\}$                             |
| 8542:9   | $0, 0, 0, e^{12}, e^{14}, e^{24} + e^{13}, e^{15} + e^{23}, e^{26} + e^{34}$ | $51/389(2, 3, 6, 5, 7, 8, 9, 11)$               | $\{1256, 14678\}$                                             |
| 8542:10  | $0, 0, 0, e^{12}, e^{14}, e^{24} + e^{13}, e^{15} + e^{23}, e^{25} + e^{16}$ | $25/184(2, 3, 6, 5, 7, 8, 9, 10)$               | $\{\emptyset, 2457\}$                                         |
| 8531:1   | $0, 0, 0, e^{12}, e^{13}, e^{14}, e^{24}, e^{16}$                            | $1/68(16, 35, 60, 51, 76, 67, 86, 83)$          | $\{\emptyset, 12367, 12567, 13478, 14578, 234568, 2468, 35\}$ |
| 8531:2   | $0, 0, 0, e^{12}, e^{13}, e^{24}, e^{14}, e^{26}$                            | $1/18(8, 5, 14, 13, 22, 18, 21, 23)$            | $\{\emptyset, 12367, 12567, 13468, 14568, 234578, 2478, 35\}$ |
| 8531:3   | $0, 0, 0, e^{12}, e^{13}, e^{14}, e^{35}, e^{16}$                            | $1/39(6, 30, 23, 36, 29, 42, 52, 48)$           | $\{\emptyset, 12367, 12567, 13478, 14578, 234568, 2468, 35\}$ |
| 8531:4   | $0, 0, 0, e^{12}, e^{13}, e^{24}, e^{35}, e^{26}$                            | $1/21(12, 5, 8, 17, 20, 22, 28, 27)$            | $\{\emptyset, 12367, 12567, 134678, 145678, 23458, 248, 35\}$ |
| 8531:5   | $0, 0, 0, e^{12}, e^{13}, e^{24}, e^{14} + e^{23}, e^{26}$                   | $1/17(7, 5, 14, 12, 21, 17, 19, 22)$            | $\{12367, 13468, 234578, 35\}$                                |
| 8531:6   | $0, 0, 0, e^{12}, e^{13}, e^{14}, e^{15}, e^{16}$                            | $1/16(2, 13, 14, 15, 16, 17, 18, 19)$           | $\{\emptyset, 12367, 1256, 13478, 1458, 2345678, 2468, 357\}$ |
| 8531:8   | $0, 0, 0, e^{12}, e^{13}, e^{14}, e^{24}, e^{16} + e^{23}$                   | $3/44(4, 7, 12, 11, 16, 15, 18, 19)$            | $\{\emptyset, 12367, 13478, 2468\}$                           |
| 8531:9   | $0, 0, 0, e^{12}, e^{13}, e^{14}, e^{15} + e^{23}, e^{16}$                   | $1/19(5, 10, 14, 15, 19, 20, 24, 25)$           | $\{134578, 148, 37, 5\}$                                      |
| 8531:11  | $0, 0, 0, e^{12}, e^{13}, e^{14}, e^{35}, e^{16} + e^{23}$                   | $1/32(6, 23, 18, 29, 24, 35, 42, 41)$           | $\{\emptyset, 12367, 13478, 2468\}$                           |
| 8531:12a | $0, 0, 0, e^{12}, e^{13}, e^{14}, e^{24} + e^{35}, e^{16}$                   | $1/89(18, 55, 55, 73, 73, 91, 128, 109)$        | $\{\emptyset, 12367, 12567, 13478, 14578, 234568, 2468, 35\}$ |
| 8531:12b | $0, 0, 0, -e^{12}, e^{13}, e^{14}, e^{24} + e^{35}, e^{16}$                  | $1/89(18, 55, 55, 73, 73, 91, 128, 109)$        | $\{\emptyset, 12367, 12567, 13478, 14578, 234568, 2468, 35\}$ |
| 8531:13  | $0, 0, 0, e^{12}, e^{13}, e^{14}, e^{25} + e^{34}, e^{16}$                   | $1/9(2, 5, 6, 7, 8, 9, 13, 11)$                 | $\{\emptyset, 12367, 1256, 1348, 14578, 234568, 24678, 357\}$ |
| 8531:14  | $0, 0, 0, e^{12}, e^{13}, e^{24}, e^{35} + e^{14}, e^{26}$                   | $1/123(68, 30, 49, 98, 117, 128, 166, 158)$     | $\{\emptyset, 12367, 12567, 35\}$                             |
| 8531:15  | $0, 0, 0, e^{12}, e^{13}, e^{24}, e^{25} + e^{34}, e^{26}$                   | $1/9(5, 2, 5, 7, 10, 9, 12, 11)$                | $\{\emptyset, 12367, 1256, 13468, 145678, 23458, 2478, 357\}$ |
| 8531:16  | $0, 0, 0, e^{12}, e^{13}, e^{14}, e^{15}, e^{35} + e^{16}$                   | $1/227(49, 170, 134, 219, 183, 268, 232, 317)$  | $\{\emptyset, 13478, 1458, 357\}$                             |
| 8531:17  | $0, 0, 0, e^{12}, e^{13}, e^{24}, e^{15}, e^{26} + e^{35}$                   | $1/57(21, 20, 30, 41, 51, 61, 72, 81)$          | $\{\emptyset, 134678, 14568, 357\}$                           |
| 8531:18  | $0, 0, 0, e^{12}, e^{13}, e^{24}, e^{35}, e^{26} + e^{15}$                   | $1/27(13, 8, 11, 21, 24, 29, 35, 37)$           | $\{\emptyset, 12567, 134678, 23458\}$                         |
| 8531:19  | $0, 0, 0, e^{12}, e^{13}, e^{14}, e^{15}, e^{16} + e^{23}$                   | $1/112(26, 73, 78, 99, 104, 125, 130, 151)$     | $\{\emptyset, 12367, 13478, 2468\}$                           |
| 8531:20  | $0, 0, 0, e^{12}, e^{13}, e^{14}, e^{24} + e^{15}, e^{16}$                   | $1/59(13, 32, 51, 45, 64, 58, 77, 71)$          | $\{\emptyset, 12367, 13478, 2468\}$                           |
| 8531:21  | $0, 0, 0, e^{12}, e^{13}, e^{14}, e^{24}, e^{35} + e^{16}$                   | $1/353(108, 170, 193, 278, 301, 386, 448, 494)$ | $\{\emptyset, 13478, 14578, 35\}$                             |
| 8531:22  | $0, 0, 0, e^{12}, e^{13}, e^{24}, e^{14}, e^{26} + e^{35}$                   | $1/29(12, 10, 15, 22, 27, 32, 34, 42)$          | $\{\emptyset, 13468, 14568, 35\}$                             |
| 8531:23  | $0, 0, 0, e^{12}, e^{13}, e^{14}, e^{35}, e^{24} + e^{16}$                   | $1/111(30, 60, 59, 90, 89, 120, 148, 150)$      | $\{\emptyset, 13478, 14578, 35\}$                             |
| 8531:24  | $0, 0, 0, e^{12}, e^{13}, e^{24}, e^{35}, e^{26} + e^{14}$                   | $1/57(30, 15, 23, 45, 53, 60, 76, 75)$          | $\{\emptyset, 23458, 248, 35\}$                               |
| 8531:27  | $0, 0, 0, e^{12}, e^{13}, e^{14} + e^{23}, e^{35}, e^{25} + e^{16}$          | $1/8(2, 5, 4, 7, 6, 9, 10, 11)$                 | $\{\emptyset, 12567, 14578, 2468\}$                           |
| 8531:28  | $0, 0, 0, e^{12}, e^{13}, e^{14}, e^{25} + e^{34}, e^{35} + e^{16}$          | $1/69(17, 40, 37, 57, 54, 74, 94, 91)$          | $\{\emptyset, 1348, 14578, 357\}$                             |
| 8531:29  | $0, 0, 0, e^{12}, e^{13}, e^{24}, e^{25} + e^{34}, e^{26} + e^{35}$          | $1/109(59, 30, 45, 89, 104, 119, 134, 149)$     | $\{\emptyset, 13468, 145678, 357\}$                           |
| 8531:31  | $0, 0, 0, e^{12}, e^{13}, e^{24}, e^{14}, e^{26} + e^{15}$                   | $1/281(100, 101, 203, 201, 303, 302, 301, 403)$ | $\{\emptyset, 12567, 13468, 234578\}$                         |
| 8531:33  | $0, 0, 0, e^{12}, e^{13}, e^{24}, e^{15}, e^{26} + e^{14}$                   | $1/21(10, 5, 11, 15, 21, 20, 31, 25)$           | $\{123478, 12458, 137, 15\}$                                  |
| 8531:34a | $0, 0, 0, e^{12}, e^{13}, e^{14}, e^{24} + e^{35}, e^{16} + e^{23}$          | $33/161(1, 3, 3, 4, 4, 5, 7, 6)$                | $\{\emptyset, 12367, 13478, 2468\}$                           |
| 8531:34b | $0, 0, 0, -e^{12}, e^{13}, e^{14}, e^{24} + e^{35}, e^{16} + e^{23}$         | $33/161(1, 3, 3, 4, 4, 5, 7, 6)$                | $\{\emptyset, 12367, 13478, 2468\}$                           |
| 8531:36  | $0, 0, 0, e^{12}, e^{13}, e^{24}, e^{14} + e^{23}, e^{26} + e^{35}$          | $5/49(3, 4, 6, 7, 9, 11, 10, 15)$               | $\{13468, 35\}$                                               |
| 8531:38  | $0, 0, 0, e^{12}, e^{13}, e^{14}, e^{24} + e^{15}, e^{35} + e^{16}$          | $61/553(3, 4, 5, 7, 8, 10, 11, 13)$             | $\{14578, 35\}$                                               |
| 8531:39  | $0, 0, 0, e^{12}, e^{13}, e^{24}, e^{35} + e^{14}, e^{26} + e^{15}$          | $67/681(5, 3, 4, 8, 9, 11, 13, 14)$             | $\{134678, 23458\}$                                           |
| 8531:40  | $0, 0, 0, e^{12}, e^{13}, e^{24}, e^{25} + e^{34}, e^{26} + e^{15}$          | $1/59(24, 19, 33, 43, 57, 62, 76, 81)$          | $\{\emptyset, 1256, 13468, 23458\}$                           |
| 8531:43  | $0, 0, 0, e^{12}, e^{13}, e^{14}, e^{35}, e^{25} + e^{34} + e^{16}$          | $1/8(2, 5, 4, 7, 6, 9, 10, 11)$                 | $\{\emptyset, 12567, 14578, 2468\}$                           |
| 8531:44a | $0, 0, 0, e^{12}, e^{13}, e^{14}, e^{24} + e^{15}, e^{16} + e^{23}$          | $9/35(1, 2, 3, 3, 4, 4, 5, 5)$                  | $\{\emptyset, 12367, 13478, 2468\}$                           |
| 8531:44b | $0, 0, 0, e^{12}, -e^{13}, e^{14}, e^{24} + e^{15}, e^{16} + e^{23}$         | $9/35(1, 2, 3, 3, 4, 4, 5, 5)$                  | $\{\emptyset, 12367, 13478, 2468\}$                           |
| 8531:45  | $0, 0, 0, e^{12}, e^{13}, e^{24}, e^{14} + e^{23}, e^{26} + e^{15}$          | $19/53(1, 1, 2, 2, 3, 3, 4)$                    | $\{\emptyset, 12567\}$                                        |
| 8531:46  | $0, 0, 0, e^{12}, a_1 e^{13}, e^{14}, e^{15} + e^{23}, e^{24} + e^{16}$      | $1/19(5, 10, 14, 15, 19, 20, 24, 25)$           | see main article                                              |
| 8531:47  | $0, 0, 0, e^{12}, e^{13}, e^{24}, e^{15} + e^{23}, e^{26} + e^{14}$          | $(0, 0, 1, 0, 1, 0, 1, 0)$                      | $\{123478, 12458\}$                                           |
| 8531:48  | $0, 0, 0, e^{12}, e^{13}, e^{14} + e^{23}, e^{24}, e^{25} + e^{16}$          | $1/12(4, 5, 8, 9, 12, 13, 14, 17)$              | $\{\emptyset, 12567, 14578, 2468\}$                           |
| 8531:51  | $0, 0, 0, e^{12}, e^{13}, e^{24}, e^{15}, e^{26} + e^{35} + e^{14}$          | $17/133(4, 2, 3, 6, 7, 8, 11, 10)$              | $\{123478, 12458\}$                                           |
| 8531:52  | $0, 0, 0, e^{12}, e^{13}, e^{14}, e^{25} + e^{34}, e^{24} + e^{16}$          | $1/179(45, 90, 119, 135, 164, 180, 254, 225)$   | $\{\emptyset, 1348, 14578, 357\}$                             |

Table A.1 – Continued to next page

Table A.1 – Continued from previous page

| Name     | $g$                                                                               | $N$                                           | Signatures $S$                                        |
|----------|-----------------------------------------------------------------------------------|-----------------------------------------------|-------------------------------------------------------|
| 8531:53  | $0, 0, 0, e^{12}, e^{13}, e^{24}, e^{25} + e^{34}, e^{26} + e^{14}$               | 1/179(90, 45, 104, 135, 194, 180, 239, 225)   | $\{0, 23458, 2478, 357\}$                             |
| 8531:54a | $0, 0, 0, e^{12}, e^{13}, e^{14} + e^{23}, e^{24} + e^{35}, e^{25} + e^{16}$      | 25/93(1, 2, 2, 3, 3, 4, 5, 5)                 | $\{0, 12567, 14578, 2468\}$                           |
| 8531:54b | $0, 0, 0, -e^{12}, e^{13}, e^{14} + e^{23}, e^{24} + e^{35}, e^{25} + e^{16}$     | 25/93(1, 2, 2, 3, 3, 4, 5, 5)                 | $\{0, 12567, 14578, 2468\}$                           |
| 8531:56a | $0, 0, 0, -e^{12}, e^{13}, e^{14} + e^{23}, e^{24} + e^{35}, e^{34} + e^{16}$     | 25/93(1, 2, 2, 3, 3, 4, 5, 5)                 | $\{0, 12567, 14578, 2468\}$                           |
| 8531:56b | $0, 0, 0, -e^{12}, -e^{13}, e^{14} + e^{23}, e^{24} + e^{35}, e^{34} + e^{16}$    | 25/93(1, 2, 2, 3, 3, 4, 5, 5)                 | $\{0, 12567, 14578, 2468\}$                           |
| 8531:57  | $0, 0, 0, e^{12}, e^{13}, e^{14}, e^{24}, e^{25} + e^{34} + e^{16}$               | 1/12(4, 5, 8, 9, 12, 13, 14, 17)              | $\{0, 12567, 14578, 2468\}$                           |
| 8531:58a | $0, 0, 0, e^{12}, a_1 e^{13}, e^{14}, e^{15} + e^{23}, e^{24} + e^{35} + e^{16}$  | 2/7(1, 2, 2, 3, 3, 4, 4, 5)                   | see main article                                      |
| 8531:58b | $0, 0, 0, -e^{12}, a_1 e^{13}, e^{14}, e^{15} + e^{23}, e^{24} + e^{35} + e^{16}$ | 2/7(1, 2, 2, 3, 3, 4, 4, 5)                   | see main article                                      |
| 8531:61  | $0, 0, 0, e^{12}, e^{13}, e^{14} + e^{23}, e^{24} + e^{15}, e^{25} + e^{16}$      | 11/71(2, 3, 4, 5, 6, 7, 8, 9)                 | $\{0, 2468\}$                                         |
| 8531:63  | $0, 0, 0, -e^{12}, e^{13}, e^{14} + e^{23}, e^{24} + e^{15}, e^{34} + e^{16}$     | 11/71(2, 3, 4, 5, 6, 7, 8, 9)                 | $\{0, 2468\}$                                         |
| 8531:64a | $0, 0, 0, e^{12}, e^{13}, e^{14}, e^{24} + e^{35}, e^{25} + e^{34} + e^{16}$      | 25/93(1, 2, 2, 3, 3, 4, 5, 5)                 | $\{0, 12567, 14578, 2468\}$                           |
| 8531:64b | $0, 0, 0, e^{12}, e^{13}, e^{14}, -e^{24} + e^{35}, e^{25} + e^{34} + e^{16}$     | 25/93(1, 2, 2, 3, 3, 4, 5, 5)                 | $\{0, 12567, 14578, 2468\}$                           |
| 8531:65a | $0, 0, 0, e^{12}, e^{13}, e^{14}, e^{25} + e^{34}, e^{24} + e^{35} + e^{16}$      | 25/93(1, 2, 2, 3, 3, 4, 5, 5)                 | $\{0, 1348, 14578, 357\}$                             |
| 8531:65b | $0, 0, 0, -e^{12}, e^{13}, e^{14}, -e^{25} + e^{34}, e^{24} + e^{35} + e^{16}$    | 25/93(1, 2, 2, 3, 3, 4, 5, 5)                 | $\{0, 1348, 14578, 357\}$                             |
| 8531:66  | $0, 0, 0, e^{12}, e^{13}, e^{24}, e^{25} + e^{34}, e^{26} + e^{35} + e^{14}$      | 49/359(4, 2, 3, 6, 7, 8, 9, 10)               | $\{13468, 145678\}$                                   |
| 8531:67  | $0, 0, 0, e^{12}, e^{13}, e^{14}, e^{24} + e^{15}, e^{25} + e^{34} + e^{16}$      | 11/71(2, 3, 4, 5, 6, 7, 8, 9)                 | $\{0, 2468\}$                                         |
| 8531:71a | $0, 0, 0, e^{12}, e^{13}, e^{14}, e^{24}, e^{27} + e^{16}$                        | 1/81(28, 28, 67, 56, 95, 84, 84, 112)         | $\{0, 12367, 12567, 13478, 14578, 234568, 2468, 35\}$ |
| 8531:71b | $0, 0, 0, e^{12}, e^{13}, -e^{14}, e^{24}, e^{27} + e^{16}$                       | 1/81(28, 28, 67, 56, 95, 84, 84, 112)         | $\{0, 12367, 12567, 13478, 14578, 234568, 2468, 35\}$ |
| 8531:72  | $0, 0, 0, e^{12}, e^{13}, e^{14}, e^{24}, e^{26} + e^{17}$                        | 1/13(4, 5, 11, 9, 15, 13, 14, 18)             | $\{0, 12367, 12567, 1347, 1457, 23456, 246, 35\}$     |
| 8531:73  | $0, 0, 0, e^{12}, e^{13}, e^{24}, e^{14} + e^{23}, e^{27} + e^{16}$               | 1/61(23, 20, 46, 43, 69, 63, 66, 86)          | $\{0, 12567, 1456, 247\}$                             |
| 8531:74a | $0, 0, 0, e^{12}, e^{13}, e^{14}, e^{24}, e^{27} + e^{35} + e^{16}$               | 18/97(2, 2, 3, 4, 5, 6, 6, 8)                 | $\{0, 13478, 14578, 35\}$                             |
| 8531:74b | $0, 0, 0, e^{12}, e^{13}, -e^{14}, e^{24}, e^{27} + e^{35} + e^{16}$              | 18/97(2, 2, 3, 4, 5, 6, 6, 8)                 | $\{0, 13478, 14578, 35\}$                             |
| 8531:75  | $0, 0, 0, e^{12}, e^{13}, e^{14}, e^{24}, e^{26} + e^{35} + e^{17}$               | 9/109(4, 5, 7, 9, 11, 13, 14, 18)             | $\{0, 23456, 246, 35\}$                               |
| 8531:76a | $0, 0, 0, -e^{12}, e^{13}, e^{24}, e^{14} + e^{23}, e^{26} + e^{34} + e^{17}$     | 19/53(1, 1, 2, 2, 3, 3, 3, 4)                 | $\{0, 12567, 14568, 2478\}$                           |
| 8531:76b | $0, 0, 0, -e^{12}, e^{13}, e^{24}, -e^{14} + e^{23}, e^{26} + e^{34} + e^{17}$    | 19/53(1, 1, 2, 2, 3, 3, 3, 4)                 | $\{0, 12567, 14568, 2478\}$                           |
| 8531:77  | $0, 0, 0, e^{12}, e^{13}, e^{24}, e^{14} + e^{23}, e^{27} + e^{35} + e^{16}$      | 15/101(2, 3, 4, 5, 6, 8, 7, 10)               | $\{23457, 35\}$                                       |
| 8531:87  | $0, 0, 0, e^{12}, e^{13}, e^{24}, e^{15}, e^{26} + e^{17}$                        | 1/123(30, 49, 87, 79, 117, 128, 147, 177)     | $\{12458, 137, 26, 345678\}$                          |
| 8531:88  | $0, 0, 0, e^{12}, e^{13}, e^{24}, e^{35}, e^{37} + e^{26}$                        | 1/15(9, 4, 4, 13, 13, 17, 17, 21)             | $\{0, 12367, 145678, 23458\}$                         |
| 8531:89  | $0, 0, 0, e^{12}, e^{13}, e^{14}, e^{24} + e^{15}, e^{26} + e^{17}$               | 1/179(37, 90, 143, 127, 180, 164, 217, 254)   | $\{0, 12367, 1347, 246\}$                             |
| 8531:91  | $0, 0, 0, e^{12}, e^{13}, e^{14}, e^{35}, e^{24} + e^{37} + e^{16}$               | 67/681(3, 6, 4, 9, 7, 12, 11, 15)             | $\{0, 14578\}$                                        |
| 8531:92  | $0, 0, 0, e^{12}, e^{13}, e^{24}, e^{35}, e^{37} + e^{26} + e^{14}$               | 23/81(2, 1, 1, 3, 3, 4, 4, 5)                 | $\{0, 23458\}$                                        |
| 8531:94  | $0, 0, 0, e^{12}, e^{13}, e^{14} + e^{23}, e^{24} + e^{15}, e^{26} + e^{17}$      | 15/101(2, 3, 4, 5, 6, 7, 8, 10)               | $\{23578, 345678\}$                                   |
| 8531:98  | $0, 0, 0, e^{12}, e^{13}, e^{14}, e^{24} + e^{15}, e^{26} + e^{35} + e^{17}$      | 15/101(2, 3, 4, 5, 6, 7, 8, 10)               | $\{0, 246\}$                                          |
| 8521:1   | $0, 0, 0, e^{12}, e^{13}, e^{23}, e^{14}, e^{17}$                                 | 1/41(10, 23, 30, 33, 40, 53, 43, 53)          | $\{12357, 1267, 134568, 148, 23478, 245678, 36, 5\}$  |
| 8521:3   | $0, 0, 0, e^{12}, e^{13}, e^{23}, e^{14}, e^{35} + e^{17}$                        | 1/81(21, 50, 46, 71, 67, 96, 92, 113)         | $\{0, 13468, 1458, 356\}$                             |
| 8521:4   | $0, 0, 0, e^{12}, e^{13}, e^{23}, e^{24}, e^{27} + e^{35}$                        | 1/29(14, 10, 15, 24, 29, 25, 34, 44)          | $\{13478, 145678, 35, 6\}$                            |
| 8521:5   | $0, 0, 0, e^{12}, e^{13}, e^{23}, e^{24}, e^{27} + e^{15}$                        | 1/293(115, 104, 197, 219, 312, 301, 323, 427) | $\{0, 12567, 134678, 23458\}$                         |
| 8521:6a  | $0, 0, 0, e^{12}, e^{13}, e^{23}, e^{14}, e^{24} + e^{35} + e^{17}$               | 2/7(1, 2, 2, 3, 3, 4, 4, 5)                   | $\{0, 13468, 1458, 356\}$                             |
| 8521:6b  | $0, 0, 0, -e^{12}, e^{13}, e^{23}, e^{14}, e^{24} + e^{35} + e^{17}$              | 2/7(1, 2, 2, 3, 3, 4, 4, 5)                   | $\{0, 13468, 1458, 356\}$                             |
| 8521:7   | $0, 0, 0, e^{12}, e^{13}, e^{23}, e^{14}, e^{25} + e^{34} + e^{17}$               | 1/16(5, 8, 10, 13, 15, 18, 18, 23)            | $\{0, 12567, 1458, 24678\}$                           |
| 8521:8   | $0, 0, 0, e^{12}, e^{13}, e^{23}, e^{24}, e^{27} + e^{35} + e^{14}$               | 15/101(4, 2, 3, 6, 7, 5, 8, 10)               | $\{13478, 145678\}$                                   |
| 8521:9   | $0, 0, 0, e^{12}, e^{13}, e^{23}, e^{14}, e^{26} + e^{35} + e^{17}$               | 59/513(3, 4, 5, 7, 8, 9, 10, 13)              | $\{0, 13468\}$                                        |
| 853:1    | $0, 0, 0, e^{12}, e^{13}, e^{14}, e^{24}, e^{15}$                                 | 1/19(5, 10, 14, 15, 19, 20, 25, 24)           | $\{0, 123678, 12567, 13478, 1457, 234568, 246, 358\}$ |
| 853:2    | $0, 0, 0, e^{12}, e^{13}, e^{14}, e^{24}, e^{35}$                                 | 1/33(12, 15, 16, 27, 28, 39, 42, 44)          | $\{0, 123678, 125678, 13478, 14578, 23456, 246, 35\}$ |
| 853:4    | $0, 0, 0, e^{12}, e^{13}, e^{24}, e^{14} + e^{23}, e^{15}$                        | 1/227(73, 110, 146, 183, 219, 293, 256, 292)  | $\{0, 12567, 1456, 247\}$                             |
| 853:5    | $0, 0, 0, e^{12}, e^{13}, e^{24}, e^{14} + e^{23}, e^{35}$                        | 1/29(8, 15, 16, 23, 24, 38, 31, 40)           | $\{123678, 13468, 23457, 35\}$                        |
| 853:6    | $0, 0, 0, e^{12}, e^{13}, e^{14}, e^{24}, e^{25} + e^{34}$                        | 1/13(5, 5, 8, 10, 13, 15, 15, 18)             | $\{0, 123678, 12567, 1347, 14578, 23456, 2468, 358\}$ |

Table A.1 – Continued to next page

Table A.1 – Continued from previous page

| Name     | $g$                                                                            | $N$                                          | Signatures $S$                                                |
|----------|--------------------------------------------------------------------------------|----------------------------------------------|---------------------------------------------------------------|
| 853:7a   | $0, 0, 0, e^{12}, e^{13}, e^{14}, e^{15}, e^{24} + e^{35}$                     | $2/7(1, 2, 2, 3, 3, 4, 4, 5)$                | $\{\emptyset, 123678, 12568, 13478, 1458, 234567, 246, 357\}$ |
| 853:7b   | $0, 0, 0, -e^{12}, e^{13}, e^{14}, e^{15}, e^{24} + e^{35}$                    | $2/7(1, 2, 2, 3, 3, 4, 4, 5)$                | $\{\emptyset, 123678, 12568, 13478, 1458, 234567, 246, 357\}$ |
| 853:8    | $0, 0, 0, e^{12}, e^{13}, e^{14}, e^{15}, e^{25} + e^{34}$                     | $2/7(1, 2, 2, 3, 3, 4, 4, 5)$                | $\{\emptyset, 123678, 1256, 1347, 1458, 234567, 2468, 3578\}$ |
| 853:9    | $0, 0, 0, e^{12}, e^{13}, e^{24}, e^{15}, e^{35} + e^{14}$                     | $1/139(53, 67, 60, 120, 113, 187, 166, 173)$ | $\{134678, 14568, 23457, 24\}$                                |
| 853:10   | $0, 0, 0, e^{12}, e^{13}, e^{24}, e^{15}, e^{25} + e^{34}$                     | $1/9(3, 4, 5, 7, 8, 11, 11, 12)$             | $\{\emptyset, 123678, 1256, 13467, 14568, 23457, 248, 3578\}$ |
| 853:11   | $0, 0, 0, e^{12}, e^{13}, e^{24}, e^{35}, e^{25} + e^{34}$                     | $1/8(4, 3, 3, 7, 7, 10, 10, 10)$             | $\{\emptyset, 123678, 12567, 13467, 145678, 2345, 248, 358\}$ |
| 853:12   | $0, 0, 0, e^{12}, e^{13}, e^{24}, e^{14} + e^{23}, e^{25} + e^{34}$            | $1/12(4, 5, 8, 9, 12, 14, 13, 17)$           | $\{123678, 1346, 23457, 358\}$                                |
| 853:15   | $0, 0, 0, e^{12}, e^{13}, e^{24}, e^{15} + e^{23}, e^{35} + e^{14}$            | $15/101(2, 4, 3, 6, 5, 10, 7, 8)$            | $\{23457, 24\}$                                               |
| 853:16   | $0, 0, 0, e^{12}, e^{13}, e^{24}, e^{15} + e^{23}, e^{25} + e^{34}$            | $1/8(2, 4, 5, 6, 7, 10, 9, 11)$              | $\{123678, 1256, 23457, 248\}$                                |
| 853:17   | $0, 0, 0, e^{12}, e^{13}, e^{14}, e^{24} + e^{15}, e^{25} + e^{34}$            | $4/61(5, 7, 9, 12, 14, 17, 19, 21)$          | $\{\emptyset, 123678, 1347, 2468\}$                           |
| 853:18a  | $0, 0, 0, e^{12}, e^{13}, e^{14}, e^{25} + e^{34}, e^{24} + e^{35}$            | $1/53(19, 25, 25, 44, 44, 63, 69, 69)$       | $\{\emptyset, 123678, 12568, 1348, 14578, 23456, 2467, 357\}$ |
| 853:18b  | $0, 0, 0, -e^{12}, e^{13}, e^{14}, -e^{25} + e^{34}, e^{24} + e^{35}$          | $1/53(19, 25, 25, 44, 44, 63, 69, 69)$       | $\{\emptyset, 123678, 12568, 1348, 14578, 23456, 2467, 357\}$ |
| 853:19   | $0, 0, 0, e^{12}, e^{13}, e^{24}, e^{35} + e^{14}, e^{25} + e^{34}$            | $1/31(14, 12, 13, 26, 27, 38, 40, 39)$       | $\{\emptyset, 123678, 12567, 358\}$                           |
| 853:20   | $0, 0, 0, e^{12}, e^{13}, e^{14} + e^{23}, e^{24} + e^{15}, e^{25} + e^{34}$   | $11/71(2, 3, 4, 5, 6, 7, 8, 9)$              | $\{123678, 1347\}$                                            |
| 853:21a  | $0, 0, 0, e^{12}, e^{13}, e^{14} + e^{23}, e^{25} + e^{34}, e^{24} + e^{35}$   | $25/93(1, 2, 2, 3, 3, 4, 5, 5)$              | $\{123678, 1348, 23456, 357\}$                                |
| 853:21b  | $0, 0, 0, -e^{12}, e^{13}, e^{14} + e^{23}, -e^{25} + e^{34}, e^{24} + e^{35}$ | $25/93(1, 2, 2, 3, 3, 4, 5, 5)$              | $\{123678, 1348, 23456, 357\}$                                |
| 853:22   | $0, 0, 0, e^{12}, e^{13}, e^{24} + e^{15}, e^{35} + e^{14}, e^{25} + e^{34}$   | $8/19(1, 1, 1, 2, 2, 3, 3)$                  | $\{\emptyset, 123678\}$                                       |
| 852:1    | $0, 0, 0, e^{12}, e^{13}, e^{23}, e^{14}, e^{24}$                              | $3/37(5, 5, 9, 10, 14, 14, 15, 15)$          | $\{\emptyset, 12378, 125678, 13468, 1458, 23457, 2467, 356\}$ |
| 852:2    | $0, 0, 0, e^{12}, e^{13}, e^{23}, e^{14}, e^{15}$                              | $1/37(11, 23, 23, 34, 34, 46, 45, 45)$       | $\{\emptyset, 12378, 12567, 13468, 145, 234578, 2467, 3568\}$ |
| 852:3    | $0, 0, 0, e^{12}, e^{13}, e^{23}, e^{24}, e^{15}$                              | $1/27(9, 13, 17, 22, 26, 30, 35, 35)$        | $\{\emptyset, 12378, 12567, 134678, 1457, 23458, 246, 3568\}$ |
| 852:4    | $0, 0, 0, e^{12}, e^{13}, e^{23}, e^{24}, e^{35}$                              | $5/11(1, 1, 1, 2, 2, 2, 3, 3)$               | $\{123678, 12578, 13478, 145678, 23456, 24, 35, 6\}$          |
| 852:5    | $0, 0, 0, e^{12}, e^{13}, e^{23}, e^{14}, e^{24} + e^{15}$                     | $1/6(2, 3, 4, 5, 6, 7, 7, 8)$                | $\{\emptyset, 12378, 13468, 2467\}$                           |
| 852:6a   | $0, 0, 0, e^{12}, e^{13}, e^{23}, e^{14}, e^{24} + e^{35}$                     | $3/17(2, 3, 3, 5, 5, 6, 7, 8)$               | $\{\emptyset, 12378, 125678, 13468, 1458, 23457, 2467, 356\}$ |
| 852:6b   | $0, 0, 0, -e^{12}, e^{13}, e^{23}, e^{14}, e^{24} + e^{35}$                    | $3/17(2, 3, 3, 5, 5, 6, 7, 8)$               | $\{\emptyset, 12378, 125678, 13468, 1458, 23457, 2467, 356\}$ |
| 852:7    | $0, 0, 0, e^{12}, e^{13}, e^{23}, e^{14}, e^{25} + e^{34}$                     | $1/19(7, 9, 11, 16, 18, 20, 23, 27)$         | $\{\emptyset, 12378, 12567, 1346, 1458, 23457, 24678, 3568\}$ |
| 852:9    | $0, 0, 0, e^{12}, e^{13}, e^{23}, e^{24}, e^{25} + e^{34}$                     | $1/19(9, 7, 11, 16, 20, 18, 23, 27)$         | $\{123678, 1257, 1347, 145678, 23456, 248, 358, 6\}$          |
| 852:12a  | $0, 0, 0, e^{12}, e^{13}, e^{23}, e^{25} + e^{34}, e^{24} + e^{35}$            | $5/11(1, 1, 1, 2, 2, 2, 3, 3)$               | $\{123678, 1258, 1348, 145678, 23456, 247, 357, 6\}$          |
| 852:12b  | $0, 0, 0, -e^{12}, e^{13}, e^{23}, -e^{25} + e^{34}, e^{24} + e^{35}$          | $5/11(1, 1, 1, 2, 2, 2, 3, 3)$               | $\{123678, 1258, 1348, 145678, 23456, 247, 357, 6\}$          |
| 852:13a  | $0, 0, 0, e^{12}, e^{13}, e^{23}, e^{14}, e^{26} + e^{15}$                     | $1/17(7, 7, 10, 14, 17, 17, 21, 24)$         | $\{\emptyset, 12378, 12567, 13468, 145, 234578, 2467, 3568\}$ |
| 852:13b  | $0, 0, 0, e^{12}, -e^{13}, e^{23}, e^{14}, e^{26} + e^{15}$                    | $1/17(7, 7, 10, 14, 17, 17, 21, 24)$         | $\{\emptyset, 12378, 12567, 13468, 145, 234578, 2467, 3568\}$ |
| 852:14   | $0, 0, 0, e^{12}, e^{13}, e^{23}, e^{14}, e^{25} + e^{16}$                     | $1/19(7, 9, 11, 16, 18, 20, 23, 27)$         | $\{\emptyset, 12378, 12567, 1346, 1458, 23457, 24678, 3568\}$ |
| 852:16   | $0, 0, 0, e^{12}, e^{13}, e^{23}, e^{14}, e^{26} + e^{35}$                     | $1/24(10, 11, 12, 21, 22, 23, 31, 34)$       | $\{\emptyset, 12378, 13468, 2467\}$                           |
| 852:20a  | $0, 0, 0, e^{12}, e^{13}, e^{23}, e^{24} + e^{15}, e^{36} + e^{14}$            | $5/11(1, 1, 1, 2, 2, 2, 3, 3)$               | $\{\emptyset, 12378, 13467, 2468\}$                           |
| 852:20b  | $0, 0, 0, -e^{12}, e^{13}, e^{23}, e^{24} + e^{15}, e^{36} + e^{14}$           | $5/11(1, 1, 1, 2, 2, 2, 3, 3)$               | $\{\emptyset, 12378, 13467, 2468\}$                           |
| 852:21   | $0, 0, 0, -e^{12}, e^{13}, e^{23}, e^{24} + e^{15}, e^{34} + e^{16}$           | $1/13(5, 6, 7, 11, 12, 13, 17, 18)$          | $\{\emptyset, 12378, 13467, 2468\}$                           |
| 852:23   | $0, 0, 0, e^{12}, a_1 e^{13}, e^{23}, e^{35} + e^{14}, e^{24} + e^{36}$        | $5/11(1, 1, 1, 2, 2, 2, 3, 3)$               | $\{\emptyset, 12378, 125678, 356\}$                           |
| 852:24a  | $0, 0, 0, e^{12}, e^{13}, e^{23}, e^{24} + e^{35}, e^{36} + e^{14}$            | $5/11(1, 1, 1, 2, 2, 2, 3, 3)$               | $\{\emptyset, 12378, 125678, 13467, 1457, 23458, 2468, 356\}$ |
| 852:24b  | $0, 0, 0, -e^{12}, e^{13}, e^{23}, e^{24} + e^{35}, e^{36} + e^{14}$           | $5/11(1, 1, 1, 2, 2, 2, 3, 3)$               | $\{\emptyset, 12378, 125678, 13467, 1457, 23458, 2468, 356\}$ |
| 852:24c  | $0, 0, 0, -e^{12}, -e^{13}, e^{23}, e^{24} + e^{35}, e^{36} + e^{14}$          | $5/11(1, 1, 1, 2, 2, 2, 3, 3)$               | $\{\emptyset, 12378, 125678, 13467, 1457, 23458, 2468, 356\}$ |
| 852:25a  | $0, 0, 0, e^{12}, e^{13}, e^{23}, e^{25} + e^{34}, e^{36} + e^{14}$            | $5/11(1, 1, 1, 2, 2, 2, 3, 3)$               | $\{\emptyset, 12378, 12568, 1346, 1457, 23458, 24678, 3567\}$ |
| 852:25b  | $0, 0, 0, -e^{12}, -e^{13}, e^{23}, e^{25} + e^{34}, e^{36} + e^{14}$          | $5/11(1, 1, 1, 2, 2, 2, 3, 3)$               | $\{\emptyset, 12378, 12568, 1346, 1457, 23458, 24678, 3567\}$ |
| 852:29   | $0, 0, 0, e^{12}, e^{13}, e^{23}, e^{25} + e^{34}, e^{24} + e^{36} + e^{15}$   | $5/11(1, 1, 1, 2, 2, 2, 3, 3)$               | $\{\emptyset, 12378\}$                                        |
| 84321:2  | $0, 0, 0, 0, e^{12}, e^{15}, e^{16}, e^{34} + e^{17}$                          | $1/47(7, 36, 32, 32, 43, 50, 57, 64)$        | $\{\emptyset, 12368, 12468, 13457, 157, 235678, 245678, 34\}$ |
| 84321:7  | $0, 0, 0, 0, e^{12}, e^{15}, e^{16}, e^{25} + e^{34} + e^{17}$                 | $11/107(2, 6, 7, 7, 8, 10, 12, 14)$          | $\{\emptyset, 12368, 12468, 34\}$                             |
| 84321:8  | $0, 0, 0, 0, -e^{12}, e^{15}, e^{16}, e^{56} + e^{34} + e^{27}$                | $1/60(10, 33, 48, 48, 43, 53, 63, 96)$       | $\{\emptyset, 12368, 12468, 13578, 14578, 234567, 2567, 34\}$ |
| 84321:11 | $0, 0, 0, 0, -e^{12}, e^{15}, e^{16} + e^{23}, e^{24} + e^{35} + e^{17}$       | $1/9(2, 5, 6, 8, 7, 9, 11, 13)$              | $\{\emptyset, 12368, 1357, 25678\}$                           |
| 84321:13 | $0, 0, 0, 0, -e^{12}, e^{15}, e^{16} + e^{23}, e^{56} + e^{34} + e^{27}$       | $1/21(5, 9, 15, 18, 14, 19, 24, 33)$         | $\{\emptyset, 12368, 13578, 2567\}$                           |

Table A.1 – Continued to next page

Table A.1 – Continued from previous page

| Name     | $g$                                                                               | $N$                                          | Signatures $S$                                                |
|----------|-----------------------------------------------------------------------------------|----------------------------------------------|---------------------------------------------------------------|
| 84321:15 | $0, 0, 0, 0, e^{12}, e^{15}, e^{25} + e^{16}, e^{26} + e^{34} + e^{17}$           | 27/109(1, 2, 3, 3, 4, 5, 6)                  | $\{\emptyset, 13457, 157, 34\}$                               |
| 84321:17 | $0, 0, 0, 0, -e^{12}, e^{15}, e^{16} + e^{23}, e^{56} + e^{27} + e^{14}$          | 1/47(13, 14, 39, 54, 27, 40, 53, 67)         | $\{123468, 134578, 24567, 4\}$                                |
| 84321:18 | $0, 0, 0, 0, -e^{12}, e^{15}, e^{25} + e^{16}, e^{34} + e^{27} + e^{56}$          | 29/257(2, 4, 7, 7, 6, 8, 10, 14)             | $\{\emptyset, 13578, 14578, 34\}$                             |
| 8431:2   | $0, 0, 0, 0, e^{12}, e^{15}, e^{25} + e^{34}, e^{16}$                             | 1/28(6, 17, 20, 20, 23, 29, 40, 35)          | $\{\emptyset, 12367, 12467, 13578, 14578, 234568, 2568, 34\}$ |
| 8431:4   | $0, 0, 0, 0, e^{12}, e^{15}, e^{25}, e^{34} + e^{16}$                             | 1/28(9, 13, 20, 20, 22, 31, 35, 40)          | $\{\emptyset, 123467, 1267, 13578, 14578, 23568, 24568, 34\}$ |
| 8431:6   | $0, 0, 0, 0, e^{12}, e^{15}, e^{13} + e^{25}, e^{34} + e^{16}$                    | 1/25(9, 10, 20, 17, 19, 28, 29, 37)          | $\{123467, 13578, 23568, 34\}$                                |
| 8431:7   | $0, 0, 0, 0, e^{12}, e^{15}, e^{25} + e^{34}, e^{16} + e^{23}$                    | 1/83(19, 49, 57, 60, 68, 87, 117, 106)       | $\{\emptyset, 12367, 13578, 2568\}$                           |
| 8431:9   | $0, 0, 0, 0, e^{12}, e^{15}, e^{13} + e^{25}, e^{24} + e^{16}$                    | 1/59(17, 28, 56, 51, 45, 62, 73, 79)         | $\{\emptyset, 12467, 14578, 2568\}$                           |
| 8431:11  | $0, 0, 0, 0, e^{12}, e^{13} + e^{25}, e^{34} + e^{15}, e^{26} + e^{35}$           | 1/36(19, 10, 20, 28, 29, 39, 48, 49)         | $\{\emptyset, 12467, 1568, 24578\}$                           |
| 8431:13  | $0, 0, 0, 0, -e^{12}, e^{15} + e^{23}, e^{25} + e^{14}, e^{35} + e^{16}$          | 1/22(7, 10, 14, 20, 17, 24, 27, 31)          | $\{\emptyset, 1267, 1578, 2568\}$                             |
| 8431:16  | $0, 0, 0, 0, -e^{12}, e^{15} + e^{23}, e^{25} + e^{14}, e^{24} + e^{35} + e^{16}$ | 11/71(2, 3, 4, 6, 5, 7, 8, 9)                | $\{1267, 1578\}$                                              |
| 8431:20a | $0, 0, 0, 0, e^{12}, e^{15}, e^{25}, e^{34} + e^{27} + e^{16}$                    | 3/8(1, 1, 2, 2, 2, 3, 3, 4)                  | $\{\emptyset, 123467, 1267, 13578, 14578, 23568, 24568, 34\}$ |
| 8431:20b | $0, 0, 0, 0, e^{12}, -e^{15}, e^{25}, e^{34} + e^{27} + e^{16}$                   | 3/8(1, 1, 2, 2, 2, 3, 3, 4)                  | $\{\emptyset, 123467, 1267, 13578, 14578, 23568, 24568, 34\}$ |
| 8431:21  | $0, 0, 0, 0, e^{12}, e^{15}, e^{25}, e^{26} + e^{34} + e^{17}$                    | 3/8(1, 1, 2, 2, 2, 3, 3, 4)                  | $\{\emptyset, 123467, 1267, 13457, 157, 23456, 256, 34\}$     |
| 8421:4   | $0, 0, 0, 0, e^{12}, e^{13}, e^{15}, e^{34} + e^{17}$                             | 1/41(10, 29, 30, 29, 39, 40, 49, 59)         | $\{123467, 127, 13568, 1458, 23578, 245678, 34, 6\}$          |
| 8421:5   | $0, 0, 0, 0, e^{12}, e^{13}, e^{25}, e^{34} + e^{27}$                             | 1/15(9, 4, 9, 12, 13, 18, 17, 21)            | $\{\emptyset, 12347, 1267, 13578, 145678, 23568, 2458, 346\}$ |
| 8421:6   | $0, 0, 0, 0, e^{12}, e^{24} + e^{13}, e^{15}, e^{17}$                             | 1/41(10, 23, 42, 29, 33, 52, 43, 53)         | $\{12367, 1247, 134568, 158, 234578, 25678, 3, 46\}$          |
| 8421:7   | $0, 0, 0, 0, e^{12}, e^{34}, e^{15}, e^{17} + e^{23}$                             | 1/39(8, 27, 24, 27, 35, 51, 43, 51)          | $\{\emptyset, 12347, 12367, 13458, 13568, 245678, 2578, 46\}$ |
| 8421:9   | $0, 0, 0, 0, e^{12}, e^{13}, e^{15}, e^{24} + e^{17}$                             | 1/31(8, 19, 27, 24, 27, 35, 35, 43)          | $\{\emptyset, 12347, 12467, 13458, 14568, 235678, 2578, 36\}$ |
| 8421:10  | $0, 0, 0, 0, e^{12}, e^{13}, e^{25}, e^{27} + e^{14}$                             | 1/24(12, 7, 18, 21, 19, 30, 26, 33)          | $\{\emptyset, 12347, 12467, 13578, 15678, 234568, 2458, 36\}$ |
| 8421:13  | $0, 0, 0, 0, e^{12}, e^{24} + e^{13}, e^{15}, e^{17} + e^{23}$                    | 1/23(7, 11, 21, 17, 18, 28, 25, 32)          | $\{12367, 134568, 25678, 46\}$                                |
| 8421:18  | $0, 0, 0, 0, e^{12}, e^{13}, e^{15}, e^{25} + e^{34} + e^{17}$                    | 1/227(67, 134, 165, 170, 201, 232, 268, 335) | $\{\emptyset, 1358, 14568, 346\}$                             |
| 8421:19  | $0, 0, 0, 0, e^{12}, e^{13}, e^{25}, e^{34} + e^{27} + e^{15}$                    | 1/81(46, 23, 50, 65, 69, 96, 92, 115)        | $\{\emptyset, 23568, 2458, 346\}$                             |
| 8421:21  | $0, 0, 0, 0, -e^{12}, e^{34}, e^{15} + e^{23}, e^{35} + e^{17}$                   | 1/8(2, 5, 4, 6, 7, 10, 9, 11)                | $\{\emptyset, 12467, 127, 14568, 158, 245678, 2578, 46\}$     |
| 8421:23  | $0, 0, 0, 0, e^{12}, e^{34}, e^{15}, e^{36} + e^{17}$                             | 1/21(5, 15, 8, 14, 20, 22, 25, 30)           | $\{\emptyset, 12367, 127, 13458, 14568, 234578, 245678, 36\}$ |
| 8421:26  | $0, 0, 0, 0, -e^{12}, e^{13}, e^{24} + e^{15}, e^{45} + e^{17}$                   | 2/7(1, 2, 3, 2, 3, 4, 4, 5)                  | $\{\emptyset, 1237, 1267, 1358, 1568, 235678, 2578, 36\}$     |
| 8421:27  | $0, 0, 0, 0, e^{12}, e^{13}, e^{25} + e^{14}, e^{27} + e^{45}$                    | 1/9(4, 3, 7, 6, 7, 11, 10, 13)               | $\{\emptyset, 1237, 1267, 13578, 15678, 23568, 258, 36\}$     |
| 8421:28  | $0, 0, 0, 0, e^{12}, e^{13}, e^{15}, e^{24} + e^{36} + e^{17}$                    | 1/297(84, 190, 179, 252, 274, 263, 358, 442) | $\{\emptyset, 13458, 14568, 36\}$                             |
| 8421:29  | $0, 0, 0, 0, e^{12}, e^{13}, e^{25}, e^{36} + e^{27} + e^{14}$                    | 1/69(36, 22, 33, 66, 58, 69, 80, 102)        | $\{\emptyset, 13578, 15678, 36\}$                             |
| 8421:30  | $0, 0, 0, 0, e^{12}, e^{13}, e^{25}, e^{34} + e^{27} + e^{16}$                    | 1/48(21, 17, 30, 42, 38, 51, 55, 72)         | $\{\emptyset, 1267, 13578, 23568\}$                           |
| 8421:32  | $0, 0, 0, 0, e^{12}, -e^{13}, e^{34} + e^{15}, e^{17} + e^{46}$                   | 1/9(2, 7, 6, 5, 9, 8, 11, 13)                | $\{\emptyset, 1237, 12467, 13458, 1568, 235678, 24578, 346\}$ |
| 8421:33  | $0, 0, 0, 0, -e^{12}, e^{24} + e^{13}, e^{15} + e^{23}, e^{35} + e^{17}$          | 3/8(1, 1, 2, 2, 2, 3, 3, 4)                  | $\{1247, 158, 25678, 46\}$                                    |
| 8421:35  | $0, 0, 0, 0, e^{12}, e^{34}, e^{15}, e^{46} + e^{17} + e^{23}$                    | 1/123(28, 90, 84, 45, 118, 129, 146, 174)    | $\{12467, 127, 234578, 235678\}$                              |
| 8421:40  | $0, 0, 0, 0, -e^{12}, e^{13}, e^{15} + e^{23}, e^{24} + e^{35} + e^{17}$          | 1/56(18, 29, 36, 54, 47, 54, 65, 83)         | $\{1247, 1458, 25678, 6\}$                                    |
| 8421:41  | $0, 0, 0, 0, e^{12}, e^{13}, e^{15} + e^{23}, e^{26} + e^{34} + e^{17}$           | 1/16(5, 9, 10, 14, 14, 15, 19, 24)           | $\{\emptyset, 1267, 14568, 24578\}$                           |
| 8421:42  | $0, 0, 0, 0, e^{12}, e^{14} + e^{23}, e^{34} + e^{15}, e^{36} + e^{17}$           | 3/109(10, 23, 15, 28, 33, 38, 43, 53)        | $\{\emptyset, 23578, 245678, 346\}$                           |
| 8421:43  | $0, 0, 0, 0, e^{12}, e^{34}, e^{15}, e^{36} + e^{25} + e^{17}$                    | 1/27(8, 16, 11, 18, 24, 29, 32, 40)          | $\{\emptyset, 13458, 14568, 36\}$                             |
| 8421:46  | $0, 0, 0, 0, -e^{12}, e^{34}, e^{15} + e^{23}, e^{35} + e^{17} + e^{46}$          | 1/39(11, 25, 22, 18, 36, 40, 47, 58)         | $\{\emptyset, 12467, 127, 46\}$                               |
| 8421:48  | $0, 0, 0, 0, e^{12}, -e^{13}, e^{34} + e^{15}, e^{25} + e^{17} + e^{46}$          | 1/69(21, 42, 44, 40, 63, 65, 84, 105)        | $\{\emptyset, 13458, 1568, 346\}$                             |
| 8421:49  | $0, 0, 0, 0, -e^{12}, e^{13}, e^{24} + e^{15}, e^{45} + e^{36} + e^{17}$          | 2/69(11, 20, 21, 22, 31, 32, 42, 53)         | $\{\emptyset, 1358, 1568, 36\}$                               |
| 8421:50  | $0, 0, 0, 0, e^{12}, e^{13}, e^{25} + e^{14}, e^{36} + e^{27} + e^{45}$           | 1/49(22, 18, 27, 36, 40, 49, 58, 76)         | $\{\emptyset, 13578, 15678, 36\}$                             |
| 8421:51  | $0, 0, 0, 0, e^{12}, e^{24} - e^{13}, e^{34} + e^{15}, e^{46} + e^{17} + e^{23}$  | 51/389(2, 5, 6, 3, 7, 8, 9, 11)              | $\{235678, 346\}$                                             |
| 8421:52  | $0, 0, 0, 0, e^{12}, e^{24} + e^{13}, e^{15}, e^{26} + e^{35} + e^{17}$           | 3/8(1, 1, 2, 2, 2, 3, 3, 4)                  | $\{\emptyset, 1267, 14568, 24578\}$                           |
| 8421:53  | $0, 0, 0, 0, e^{12}, e^{13}, e^{25} + e^{14}, e^{45} + e^{27} + e^{16}$           | 3/8(1, 1, 2, 2, 2, 3, 3, 4)                  | $\{\emptyset, 1267, 13578, 23568\}$                           |
| 8421:55  | $0, 0, 0, 0, e^{12}, e^{14} + e^{23}, e^{34} + e^{15}, e^{36} + e^{25} + e^{17}$  | 15/101(2, 4, 3, 5, 6, 7, 8, 10)              | $\{\emptyset, 346\}$                                          |
| 842:4    | $0, 0, 0, 0, e^{12}, e^{13}, e^{15}, e^{25} + e^{34}$                             | 1/19(7, 10, 13, 14, 17, 20, 24, 27)          | $\{\emptyset, 12378, 124678, 1358, 14568, 234567, 257, 346\}$ |
| 842:5    | $0, 0, 0, 0, e^{12}, e^{13}, e^{25}, e^{34} + e^{15}$                             | 1/27(13, 11, 17, 20, 24, 30, 35, 37)         | $\{\emptyset, 12378, 124678, 13457, 1567, 23568, 2458, 346\}$ |

Table A.1 – Continued to next page

Table A.1 – Continued from previous page

| Name    | $g$                                                                     | $N$                                             | Signatures $S$                                                |
|---------|-------------------------------------------------------------------------|-------------------------------------------------|---------------------------------------------------------------|
| 842:6   | $0, 0, 0, 0, e^{12}, e^{24} + e^{13}, e^{15}, e^{25}$                   | $1/37(15, 15, 32, 32, 30, 47, 45, 45)$          | $\{\emptyset, 123478, 12678, 1358, 14568, 23567, 2457, 346\}$ |
| 842:7   | $0, 0, 0, 0, e^{12}, e^{34}, e^{15}, e^{13} + e^{25}$                   | $1/11(5, 4, 8, 7, 9, 15, 14, 13)$               | $\{123478, 123678, 13458, 13568, 23457, 23567, 34, 36\}$      |
| 842:8   | $0, 0, 0, 0, e^{12}, e^{13}, e^{15}, e^{25} + e^{14}$                   | $1/23(8, 11, 19, 22, 19, 27, 27, 30)$           | $\{\emptyset, 12378, 12678, 1358, 1568, 23567, 257, 36\}$     |
| 842:9   | $0, 0, 0, 0, e^{12}, e^{13}, e^{25}, e^{24} + e^{15}$                   | $1/37(16, 15, 29, 32, 31, 45, 46, 47)$          | $\{\emptyset, 12378, 12678, 1357, 1567, 23568, 258, 36\}$     |
| 842:10  | $0, 0, 0, 0, e^{12}, e^{24} + e^{13}, e^{15}, e^{25} + e^{34}$          | $1/227(91, 110, 165, 146, 201, 256, 292, 311)$  | $\{\emptyset, 1358, 14568, 346\}$                             |
| 842:11  | $0, 0, 0, 0, e^{12}, e^{13}, e^{15} + e^{23}, e^{25} + e^{34}$          | $1/37(13, 20, 26, 27, 33, 39, 46, 53)$          | $\{12378, 1358, 234567, 346\}$                                |
| 842:12  | $0, 0, 0, 0, e^{12}, e^{13}, e^{25} + e^{14}, e^{34} + e^{15}$          | $1/26(13, 10, 16, 20, 23, 29, 33, 36)$          | $\{124678, 13457, 2458, 346\}$                                |
| 842:14  | $0, 0, 0, 0, e^{12}, e^{14} + e^{23}, e^{15}, e^{13} + e^{25}$          | $1/38(15, 16, 32, 33, 31, 48, 46, 47)$          | $\{\emptyset, 12678, 1458, 24567\}$                           |
| 842:15a | $0, 0, 0, 0, e^{12}, e^{34}, e^{15} + e^{23}, e^{13} + e^{25}$          | $1/5(2, 2, 4, 3, 4, 7, 6, 6)$                   | $\{123478, 123678, 13458, 13568, 23457, 23567, 34, 36\}$      |
| 842:15b | $0, 0, 0, 0, e^{12}, e^{34}, -e^{15} + e^{23}, e^{13} + e^{25}$         | $1/5(2, 2, 4, 3, 4, 7, 6, 6)$                   | $\{123478, 123678, 13458, 13568, 23457, 23567, 34, 36\}$      |
| 842:16  | $0, 0, 0, 0, e^{12}, e^{34}, e^{15} + e^{23}, e^{25} + e^{14}$          | $3/8(1, 1, 2, 2, 2, 4, 3, 3)$                   | $\{123478, 13458, 23457, 34\}$                                |
| 842:17  | $0, 0, 0, 0, e^{12}, e^{13}, e^{15} + e^{23}, e^{25} + e^{14}$          | $1/13(5, 6, 10, 12, 11, 15, 16, 17)$            | $\{\emptyset, 12678, 1568, 257\}$                             |
| 842:18a | $0, 0, 0, 0, e^{12}, e^{13}, e^{24} + e^{15}, e^{25} + e^{14}$          | $1/19(8, 8, 15, 16, 16, 23, 24, 24)$            | $\{\emptyset, 12378, 12678, 1358, 1568, 23567, 257, 36\}$     |
| 842:18b | $0, 0, 0, 0, e^{12}, e^{13}, e^{24} - e^{15}, e^{25} + e^{14}$          | $1/19(8, 8, 15, 16, 16, 23, 24, 24)$            | $\{\emptyset, 12378, 12678, 1358, 1568, 23567, 257, 36\}$     |
| 842:19  | $0, 0, 0, 0, e^{12}, e^{14} + e^{23}, e^{13} + e^{25}, e^{34} + e^{15}$ | $55/437(4, 3, 6, 5, 7, 9, 10, 11)$              | $\{2358, 346\}$                                               |
| 842:20  | $0, 0, 0, 0, e^{12}, e^{24} + e^{13}, e^{15} + e^{23}, e^{25} + e^{14}$ | $17/41(1, 1, 2, 2, 2, 3, 3, 3)$                 | $\{\emptyset, 12678\}$                                        |
| 842:26  | $0, 0, 0, 0, e^{12}, e^{13}, e^{15}, e^{24} + e^{16}$                   | $1/37(11, 23, 29, 28, 34, 40, 45, 51)$          | $\{\emptyset, 12378, 12467, 13458, 156, 235678, 2457, 3468\}$ |
| 842:27  | $0, 0, 0, 0, e^{12}, e^{13}, e^{25}, e^{24} + e^{16}$                   | $1/27(9, 13, 19, 24, 22, 28, 35, 37)$           | $\{\emptyset, 12378, 12467, 134578, 1567, 23568, 245, 3468\}$ |
| 842:28  | $0, 0, 0, 0, e^{12}, e^{13}, e^{15}, e^{36} + e^{14}$                   | $1/41(12, 29, 21, 42, 41, 33, 53, 54)$          | $\{123478, 124678, 13458, 14568, 234567, 2457, 346, 4\}$      |
| 842:30  | $0, 0, 0, 0, e^{12}, e^{13}, e^{15}, e^{24} + e^{36}$                   | $1/18(6, 11, 10, 15, 17, 16, 23, 26)$           | $\{\emptyset, 12378, 12678, 13458, 14568, 234567, 2457, 36\}$ |
| 842:31  | $0, 0, 0, 0, e^{12}, e^{13}, e^{25}, e^{36} + e^{14}$                   | $1/39(18, 17, 18, 36, 35, 36, 52, 54)$          | $\{\emptyset, 12378, 12678, 13578, 15678, 2356, 25, 36\}$     |
| 842:32  | $0, 0, 0, 0, e^{12}, e^{13}, e^{25}, e^{34} + e^{16}$                   | $1/15(6, 7, 9, 12, 13, 15, 20, 21)$             | $\{\emptyset, 12378, 1267, 13578, 1567, 23568, 25, 368\}$     |
| 842:33  | $0, 0, 0, 0, e^{12}, e^{13}, e^{25}, e^{24} + e^{36}$                   | $1/47(24, 19, 20, 45, 43, 44, 62, 64)$          | $\{\emptyset, 12378, 12678, 134578, 145678, 23456, 245, 36\}$ |
| 842:39  | $0, 0, 0, 0, e^{12}, e^{13}, e^{25} + e^{14}, e^{24} + e^{16}$          | $3/26(3, 4, 6, 8, 7, 9, 11, 12)$                | $\{12467, 134578, 245, 3468\}$                                |
| 842:41  | $0, 0, 0, 0, a_1 e^{12}, e^{13}, e^{24} + e^{15}, e^{34} + e^{16}$      | $1/3(1, 2, 2, 2, 3, 3, 4, 4)$                   | $\{\emptyset, 12378, 1267, 1358, 156, 235678, 257, 368\}$     |
| 842:42  | $0, 0, 0, 0, e^{12}, e^{13}, e^{25} + e^{14}, e^{24} + e^{36}$          | $3/293(46, 44, 43, 88, 90, 89, 134, 132)$       | $\{\emptyset, 12378, 12678, 36\}$                             |
| 842:43a | $0, 0, 0, 0, e^{12}, e^{13}, e^{34} + e^{15}, e^{24} + e^{16}$          | $1/3(1, 2, 2, 2, 3, 3, 4, 4)$                   | $\{\emptyset, 12378, 12467, 13458, 156, 235678, 2457, 3468\}$ |
| 842:43b | $0, 0, 0, 0, -e^{12}, e^{13}, e^{34} + e^{15}, e^{24} + e^{16}$         | $1/3(1, 2, 2, 2, 3, 3, 4, 4)$                   | $\{\emptyset, 12378, 12467, 13458, 156, 235678, 2457, 3468\}$ |
| 842:44  | $0, 0, 0, 0, e^{12}, e^{13}, e^{25} + e^{34}, e^{24} + e^{16}$          | $3/34(4, 6, 7, 9, 10, 11, 16, 15)$              | $\{\emptyset, 12378, 12467, 3468\}$                           |
| 842:45  | $0, 0, 0, 0, e^{12}, e^{13}, e^{25} + e^{34}, e^{24} + e^{36}$          | $3/29(5, 4, 4, 9, 9, 9, 13, 13)$                | $\{\emptyset, 12378, 145678, 23456\}$                         |
| 842:46  | $0, 0, 0, 0, e^{12}, e^{13}, e^{15} + e^{23}, e^{24} + e^{16}$          | $1/29(10, 17, 20, 23, 27, 30, 37, 40)$          | $\{\emptyset, 12467, 156, 2457\}$                             |
| 842:47  | $0, 0, 0, 0, e^{12}, e^{13}, e^{15} + e^{23}, e^{36} + e^{14}$          | $1/19(5, 14, 10, 20, 19, 15, 24, 25)$           | $\{123478, 13458, 234567, 346\}$                              |
| 842:49  | $0, 0, 0, 0, e^{12}, e^{13}, e^{15} + e^{23}, e^{24} + e^{36}$          | $1/17(5, 11, 10, 14, 16, 15, 21, 25)$           | $\{12378, 13458, 234567, 36\}$                                |
| 842:53a | $0, 0, 0, 0, e^{12}, e^{13}, e^{15}, e^{36} + e^{25} + e^{14}$          | $3/17(2, 3, 3, 6, 5, 5, 7, 8)$                  | $\{123478, 124678, 13458, 14568, 234567, 2457, 346, 4\}$      |
| 842:53b | $0, 0, 0, 0, -e^{12}, e^{13}, e^{15}, e^{36} + e^{25} + e^{14}$         | $3/17(2, 3, 3, 6, 5, 5, 7, 8)$                  | $\{123478, 124678, 13458, 14568, 234567, 2457, 346, 4\}$      |
| 842:54  | $0, 0, 0, 0, e^{12}, e^{13}, e^{15}, e^{26} + e^{35} + e^{14}$          | $1/19(7, 9, 11, 20, 16, 18, 23, 27)$            | $\{123478, 1267, 135, 14568, 234567, 2578, 368, 4\}$          |
| 842:56  | $0, 0, 0, 0, e^{12}, e^{13}, e^{25}, e^{24} + e^{36} + e^{15}$          | $1/29(14, 12, 13, 28, 26, 27, 38, 40)$          | $\{\emptyset, 12378, 12678, 36\}$                             |
| 842:57  | $0, 0, 0, 0, e^{12}, e^{13}, e^{25}, e^{26} + e^{35} + e^{14}$          | $1/19(9, 7, 11, 18, 16, 20, 23, 27)$            | $\{\emptyset, 12378, 12467, 13457, 15678, 2356, 2458, 3468\}$ |
| 842:59  | $0, 0, 0, 0, e^{12}, e^{13}, e^{25} + e^{14}, e^{36} + e^{15}$          | $1/293(130, 136, 133, 272, 266, 263, 402, 396)$ | $\{\emptyset, 12378, 12678, 36\}$                             |
| 842:60a | $0, 0, 0, 0, e^{12}, e^{13}, e^{24} + e^{15}, e^{36} + e^{25}$          | $1/12(5, 6, 6, 10, 11, 11, 16, 17)$             | $\{\emptyset, 12378, 12678, 1358, 1568, 23567, 257, 36\}$     |
| 842:60b | $0, 0, 0, 0, -e^{12}, e^{13}, e^{24} + e^{15}, e^{36} + e^{25}$         | $1/12(5, 6, 6, 10, 11, 11, 16, 17)$             | $\{\emptyset, 12378, 12678, 1358, 1568, 23567, 257, 36\}$     |
| 842:61  | $0, 0, 0, 0, e^{12}, e^{13}, e^{25} + e^{14}, e^{26} + e^{35}$          | $1/7(3, 3, 4, 6, 6, 7, 9, 10)$                  | $\{\emptyset, 12378, 1267, 1357, 15678, 2356, 258, 368\}$     |
| 842:62  | $0, 0, 0, 0, e^{12}, e^{13}, e^{24} + e^{15}, e^{26} + e^{35}$          | $1/7(3, 3, 4, 6, 6, 7, 9, 10)$                  | $\{\emptyset, 12378, 1267, 135, 1568, 23567, 2578, 368\}$     |
| 842:63  | $0, 0, 0, 0, e^{12}, e^{13}, e^{34} + e^{15}, e^{25} + e^{16}$          | $1/34(14, 17, 20, 25, 31, 34, 45, 48)$          | $\{\emptyset, 12378, 13458, 2457\}$                           |
| 842:64a | $0, 0, 0, 0, e^{12}, e^{13}, e^{34} + e^{15}, e^{36} + e^{25}$          | $1/12(5, 6, 6, 10, 11, 11, 16, 17)$             | $\{\emptyset, 12378, 124678, 13458, 1568, 23567, 2457, 346\}$ |
| 842:64b | $0, 0, 0, 0, -e^{12}, e^{13}, e^{34} + e^{15}, e^{36} + e^{25}$         | $1/12(5, 6, 6, 10, 11, 11, 16, 17)$             | $\{\emptyset, 12378, 124678, 13458, 1568, 23567, 2457, 346\}$ |
| 842:65  | $0, 0, 0, 0, e^{12}, e^{13}, e^{34} + e^{15}, e^{26} + e^{35}$          | $1/12(5, 6, 6, 10, 11, 11, 16, 17)$             | $\{\emptyset, 12378, 12467, 1345, 1568, 23567, 24578, 3468\}$ |

Table A.1 – Continued to next page

Table A.1 – Continued from previous page

| Name     | $g$                                                                                  | $N$                                        | Signatures $S$                                                                                                |
|----------|--------------------------------------------------------------------------------------|--------------------------------------------|---------------------------------------------------------------------------------------------------------------|
| 842:66   | $0, 0, 0, 0, e^{12}, e^{13}, e^{25} + e^{34}, e^{36} + e^{15}$                       | $5/11(1, 1, 1, 2, 2, 2, 3, 3)$             | $\{\emptyset, 12378, 124678, 346\}$                                                                           |
| 842:67   | $0, 0, 0, 0, e^{12}, e^{13}, e^{25} + e^{34}, e^{26} + e^{35}$                       | $1/13(7, 5, 6, 11, 12, 13, 17, 18)$        | $\{\emptyset, 12378, 12467, 1357, 145678, 23456, 258, 3468\}$                                                 |
| 842:71a  | $0, 0, 0, 0, e^{12}, e^{13}, e^{25} + e^{14}, e^{24} + e^{36} + e^{15}$              | $5/11(1, 1, 1, 2, 2, 2, 3, 3)$             | $\{\emptyset, 12378, 12678, 36\}$                                                                             |
| 842:71b  | $0, 0, 0, 0, e^{12}, e^{13}, e^{25} - e^{14}, e^{24} + e^{36} + e^{15}$              | $5/11(1, 1, 1, 2, 2, 2, 3, 3)$             | $\{\emptyset, 12378, 12678, 36\}$                                                                             |
| 842:73   | $0, 0, 0, 0, e^{12}, e^{13}, e^{24} + e^{15}, e^{26} + e^{35} + e^{14}$              | $1/13(6, 5, 7, 12, 11, 13, 17, 18)$        | $\{1267, 135, 2578, 368\}$                                                                                    |
| 842:74   | $0, 0, 0, 0, a_1 e^{12}, e^{13}, e^{24} + e^{15}, e^{25} + e^{34} + e^{16}$          | $1/19(7, 10, 13, 14, 17, 20, 24, 27)$      | see main article                                                                                              |
| 842:75a  | $0, 0, 0, 0, e^{12}, e^{13}, e^{34} + e^{15}, e^{36} + e^{25} + e^{14}$              | $5/11(1, 1, 1, 2, 2, 2, 3, 3)$             | $\{124678, 13458, 2457, 346\}$                                                                                |
| 842:75b  | $0, 0, 0, 0, -e^{12}, e^{13}, e^{34} + e^{15}, e^{36} + e^{25} + e^{14}$             | $5/11(1, 1, 1, 2, 2, 2, 3, 3)$             | $\{124678, 13458, 2457, 346\}$                                                                                |
| 842:79a  | $0, 0, 0, 0, e^{12}, e^{13}, e^{15} + e^{23}, e^{36} + e^{25} + e^{14}$              | $2/7(1, 2, 2, 4, 3, 3, 4, 5)$              | $\{123478, 13458, 234567, 346\}$                                                                              |
| 842:79b  | $0, 0, 0, 0, -e^{12}, e^{13}, e^{15} + e^{23}, e^{36} + e^{25} + e^{14}$             | $2/7(1, 2, 2, 4, 3, 3, 4, 5)$              | $\{123478, 13458, 234567, 346\}$                                                                              |
| 842:80   | $0, 0, 0, 0, e^{12}, e^{13}, e^{15} + e^{23}, e^{26} + e^{35} + e^{14}$              | $1/16(5, 8, 10, 18, 13, 15, 18, 23)$       | $\{123478, 135, 234567, 368\}$                                                                                |
| 842:81   | $0, 0, 0, 0, e^{12}, e^{13}, e^{15} + e^{23}, e^{25} + e^{34} + e^{16}$              | $13/73(2, 3, 4, 4, 5, 6, 7, 8)$            | $\{234567, 346\}$                                                                                             |
| 842:84a  | $0, 0, 0, 0, e^{12}, e^{13}, e^{36} + e^{25}, e^{26} + e^{35} + e^{14}$              | $5/11(1, 1, 1, 2, 2, 2, 3, 3)$             | $\{\emptyset, 12378, 12467, 13457, 15678, 2356, 2458, 3468\}$                                                 |
| 842:84b  | $0, 0, 0, 0, e^{12}, e^{13}, e^{36} - e^{25}, e^{26} + e^{35} + e^{14}$              | $5/11(1, 1, 1, 2, 2, 2, 3, 3)$             | $\{\emptyset, 12378, 12467, 13457, 15678, 2356, 2458, 3468\}$                                                 |
| 842:85a  | $0, 0, 0, 0, e^{12}, e^{13}, e^{26} + e^{35}, e^{36} + e^{25} + e^{14}$              | $5/11(1, 1, 1, 2, 2, 2, 3, 3)$             | $\{\emptyset, 12378, 1268, 1358, 15678, 2356, 257, 367\}$                                                     |
| 842:85b  | $0, 0, 0, 0, -e^{12}, e^{13}, -e^{26} + e^{35}, e^{36} + e^{25} + e^{14}$            | $5/11(1, 1, 1, 2, 2, 2, 3, 3)$             | $\{\emptyset, 12378, 1268, 1358, 15678, 2356, 257, 367\}$                                                     |
| 842:86   | $0, 0, 0, 0, e^{12}, e^{13}, e^{26} + e^{35}, e^{24} + e^{36} + e^{15}$              | $1/61(27, 29, 28, 54, 56, 55, 84, 83)$     | $\{\emptyset, 12378, 1268, 367\}$                                                                             |
| 842:87   | $0, 0, 0, 0, e^{12}, e^{13}, e^{26} + e^{35} + e^{14}, e^{24} + e^{36} + e^{15}$     | $5/11(1, 1, 1, 2, 2, 2, 3, 3)$             | $\{1268, 367\}$                                                                                               |
| 842:88   | $0, 0, 0, 0, a_1 e^{12}, e^{13}, e^{25} + e^{34} + e^{16}, e^{24} + e^{36} + e^{15}$ | $5/11(1, 1, 1, 2, 2, 2, 3, 3)$             | see main article                                                                                              |
| 842:90   | $0, 0, 0, 0, e^{12}, e^{34}, e^{13} + e^{25}, e^{36}$                                | $1/5(4, 1, 2, 3, 5, 5, 6, 7)$              | $\{123478, 12367, 134578, 13567, 23458, 2356, 348, 36\}$                                                      |
| 842:92   | $0, 0, 0, 0, e^{12}, e^{34}, e^{15}, e^{36} + e^{25}$                                | $1/21(8, 11, 8, 14, 19, 22, 27, 30)$       | $\{\emptyset, 123478, 124678, 13458, 14568, 23567, 257, 36\}$                                                 |
| 842:93   | $0, 0, 0, 0, -e^{12}, e^{14} + e^{23}, e^{15}, e^{35} + e^{16}$                      | $2/7(1, 2, 2, 3, 3, 4, 4, 5)$              | $\{\emptyset, 123478, 1267, 1356, 1458, 2357, 245678, 3468\}$                                                 |
| 842:94   | $0, 0, 0, 0, e^{12}, e^{24} + e^{13}, e^{15}, e^{26} + e^{35}$                       | $1/9(4, 3, 6, 7, 7, 10, 11, 13)$           | $\{\emptyset, 123478, 1267, 135, 14568, 23567, 24578, 3468\}$                                                 |
| 842:96   | $0, 0, 0, 0, e^{12}, e^{34}, e^{15} + e^{23}, e^{36} + e^{14}$                       | $(0, 1, 0, 1, 1, 1, 1, 1)$                 | $\{123478, 12367, 13458, 1356\}$                                                                              |
| 842:97   | $0, 0, 0, 0, e^{12}, e^{34}, e^{13} + e^{25}, e^{36} + e^{15}$                       | $1/17(11, 4, 8, 10, 15, 18, 19, 26)$       | $\{123478, 13567, 23458, 36\}$                                                                                |
| 842:98   | $0, 0, 0, 0, e^{12}, e^{34}, e^{15}, e^{13} + e^{25} + e^{46}$                       | $1/17(8, 7, 14, 4, 15, 18, 23, 22)$        | $\{123478, 123678, 13458, 13568\}$                                                                            |
| 842:99   | $0, 0, 0, 0, e^{12}, e^{34}, e^{13} + e^{25}, e^{46} + e^{15}$                       | $1/57(31, 20, 40, 21, 51, 61, 71, 82)$     | $\{123478, 123678, 23458, 23568\}$                                                                            |
| 842:100  | $0, 0, 0, 0, e^{12}, e^{34}, e^{36} + e^{15}, e^{25} + e^{46}$                       | $7/15(1, 1, 1, 1, 2, 2, 3, 3)$             | $\{\emptyset, 123478, 13568, 24567\}$                                                                         |
| 842:101  | $0, 0, 0, 0, -e^{12}, e^{14} + e^{23}, e^{13} + e^{25}, e^{35} + e^{16}$             | $3/8(1, 1, 2, 2, 2, 3, 3, 4)$              | $\{123478, 13567, 235, 3468\}$                                                                                |
| 842:102  | $0, 0, 0, 0, e^{12}, e^{24} + e^{13}, e^{15}, e^{26} + e^{35} + e^{14}$              | $1/8(4, 2, 5, 7, 6, 9, 10, 11)$            | $\{123478, 1267, 135, 14568\}$                                                                                |
| 842:104  | $0, 0, 0, 0, -e^{12}, e^{24} + e^{13}, e^{15} + e^{23}, e^{16} + e^{45}$             | $1/22(8, 11, 16, 13, 19, 24, 27, 32)$      | $\{\emptyset, 1267, 1456, 2457\}$                                                                             |
| 842:105  | $0, 0, 0, 0, -e^{12}, e^{14} + e^{23}, e^{34} + e^{15}, e^{35} + e^{16}$             | $2/61(10, 18, 15, 23, 28, 33, 38, 43)$     | $\{\emptyset, 2357, 245678, 3468\}$                                                                           |
| 842:106  | $0, 0, 0, 0, e^{12}, e^{24} + e^{13}, e^{34} + e^{15}, e^{26} + e^{35}$              | $1/106(50, 38, 63, 75, 88, 113, 138, 151)$ | $\{\emptyset, 23567, 24578, 3468\}$                                                                           |
| 842:108a | $0, 0, 0, 0, e^{12}, e^{34}, e^{13} + e^{25}, e^{46} + e^{15} + e^{23}$              | $5/23(2, 2, 4, 1, 4, 5, 6, 6)$             | $\{123478, 123678, 23458, 23568\}$                                                                            |
| 842:108b | $0, 0, 0, 0, e^{12}, e^{34}, -e^{13} + e^{25}, e^{15} + e^{23} + e^{46}$             | $5/23(2, 2, 4, 1, 4, 5, 6, 6)$             | $\{123478, 123678, 23458, 23568\}$                                                                            |
| 842:109  | $0, 0, 0, 0, e^{12}, e^{34}, e^{13} + e^{25}, e^{24} + e^{36} + e^{15}$              | $3/5(1, 0, 0, 2, 1, 2, 1, 2)$              | $\{123478, 23458\}$                                                                                           |
| 842:110  | $0, 0, 0, 0, e^{12}, e^{34}, e^{36} + e^{15}, e^{13} + e^{25} + e^{46}$              | $7/23(2, 1, 2, 1, 3, 3, 5, 4)$             | $\{123478, 13568\}$                                                                                           |
| 842:113  | $0, 0, 0, 0, -e^{12}, e^{14} + e^{23}, e^{13} + e^{25}, e^{24} + e^{35} + e^{16}$    | $1/5(1, 2, 4, 5, 3, 6, 5, 7)$              | $\{123478, 235\}$                                                                                             |
| 842:115  | $0, 0, 0, 0, -e^{12}, e^{24} + e^{13}, e^{34} + e^{15}, e^{16} + e^{23} + e^{45}$    | $11/71(2, 4, 5, 3, 6, 7, 8, 9)$            | $\{235678, 2457\}$                                                                                            |
| 841:3    | $0, 0, 0, 0, e^{12}, e^{13}, e^{34}, e^{25}$                                         | $1/21(12, 8, 12, 15, 20, 24, 27, 28)$      | $\{\emptyset, 12348, 12378, 124678, 1268, 13458, 13578, 145678, 1568, 23456, 23567, 2457, 25, 346, 367, 47\}$ |
| 841:4    | $0, 0, 0, 0, e^{12}, e^{13}, e^{14}, e^{15}$                                         | $1/8(2, 6, 7, 7, 8, 9, 9, 10)$             | $\{\emptyset, 12348, 12378, 12468, 12678, 1345, 1357, 1456, 1567, 2345678, 23568, 24578, 258, 3467, 36, 47\}$ |
| 841:5    | $0, 0, 0, 0, e^{12}, e^{13}, e^{14}, e^{25}$                                         | $1/15(6, 7, 12, 12, 13, 18, 18, 20)$       | $\{\emptyset, 12348, 12378, 12468, 12678, 13458, 13578, 14568, 15678, 234567, 2356, 2457, 25, 3467, 36, 47\}$ |
| 841:6    | $0, 0, 0, 0, e^{12}, e^{13}, e^{24}, e^{15}$                                         | $1/11(4, 6, 9, 8, 10, 13, 14, 14)$         | $\{\emptyset, 12348, 12378, 12468, 12678, 13457, 135, 14567, 156, 234568, 235678, 2458, 2578, 3467, 36, 47\}$ |

Table A.1 – Continued to next page



Table A.1 – Continued from previous page

| Name    | $g$                                                                      | $N$                                        | Signatures $S$                                                                                                |
|---------|--------------------------------------------------------------------------|--------------------------------------------|---------------------------------------------------------------------------------------------------------------|
| 841:7   | $0, 0, 0, 0, e^{12}, e^{34}, e^{24} + e^{13}, e^{15}$                    | $1/41(16, 23, 30, 23, 39, 53, 46, 55)$     | $\{123678, 12468, 13457, 15, 23458, 2578, 36, 467\}$                                                          |
| 841:8   | $0, 0, 0, 0, e^{12}, e^{13}, e^{23}, e^{34} + e^{15}$                    | $1/23(10, 13, 14, 19, 23, 24, 27, 33)$     | $\{\emptyset, 1238, 124678, 13457, 156, 23568, 24578, 3467\}$                                                 |
| 841:9   | $0, 0, 0, 0, e^{12}, e^{13}, e^{14} + e^{23}, e^{15}$                    | $1/14(5, 8, 10, 13, 13, 15, 18, 18)$       | $\{\emptyset, 12348, 12678, 1357, 1456, 23568, 24578, 3467\}$                                                 |
| 841:10  | $0, 0, 0, 0, e^{12}, e^{13}, e^{14} + e^{23}, e^{25}$                    | $1/31(13, 14, 24, 25, 27, 37, 38, 41)$     | $\{\emptyset, 12348, 12678, 13578, 14568, 2356, 2457, 3467\}$                                                 |
| 841:12  | $0, 0, 0, 0, e^{12}, e^{13}, e^{14}, e^{34} + e^{15}$                    | $5/14(1, 2, 2, 2, 3, 3, 4)$                | $\{\emptyset, 12378, 12468, 1345, 1567, 23568, 24578, 3467\}$                                                 |
| 841:13  | $0, 0, 0, 0, e^{12}, e^{13}, e^{14}, e^{25} + e^{34}$                    | $1/31(14, 15, 22, 22, 29, 36, 36, 44)$     | $\{\emptyset, 12378, 12468, 13578, 14568, 234567, 25, 3467\}$                                                 |
| 841:14  | $0, 0, 0, 0, e^{12}, e^{13}, e^{24}, e^{34} + e^{15}$                    | $3/37(5, 7, 9, 8, 12, 14, 15, 17)$         | $\{\emptyset, 12378, 12468, 13457, 156, 235678, 2458, 3467\}$                                                 |
| 841:15  | $0, 0, 0, 0, e^{12}, e^{13}, e^{34}, e^{25} + e^{14}$                    | $1/41(24, 15, 23, 30, 39, 47, 53, 54)$     | $\{12348, 124678, 13458, 145678, 23456, 2457, 346, 47\}$                                                      |
| 841:17  | $0, 0, 0, 0, e^{12}, e^{13}, e^{23}, e^{25} + e^{14}$                    | $1/16(8, 7, 11, 14, 15, 19, 18, 22)$       | $\{\emptyset, 1238, 12678, 13578, 1568, 2356, 257, 367\}$                                                     |
| 841:18  | $0, 0, 0, 0, e^{12}, e^{13}, e^{14}, e^{15} + e^{23}$                    | $1/11(4, 7, 8, 9, 11, 12, 13, 15)$         | $\{\emptyset, 12468, 12678, 1456, 1567, 24578, 258, 47\}$                                                     |
| 841:19  | $0, 0, 0, 0, e^{12}, e^{13}, e^{24}, e^{15} + e^{23}$                    | $1/23(9, 12, 18, 17, 21, 27, 29, 30)$      | $\{\emptyset, 12468, 12678, 14567, 156, 2458, 2578, 47\}$                                                     |
| 841:20  | $0, 0, 0, 0, e^{12}, e^{13}, e^{14} + e^{23}, e^{34} + e^{15}$           | $1/24(10, 14, 15, 19, 24, 25, 29, 34)$     | $\{\emptyset, 23568, 24578, 3467\}$                                                                           |
| 841:21  | $0, 0, 0, 0, e^{12}, e^{13}, e^{14} + e^{23}, e^{25} + e^{34}$           | $1/63(29, 30, 44, 45, 59, 73, 74, 89)$     | $\{\emptyset, 13578, 14568, 3467\}$                                                                           |
| 841:22a | $0, 0, 0, 0, e^{12}, e^{14} + e^{23}, e^{24} + e^{13}, e^{15}$           | $1/32(14, 14, 25, 25, 28, 39, 39, 42)$     | $\{\emptyset, 12348, 12678, 1356, 1457, 23578, 24568, 3467\}$                                                 |
| 841:22b | $0, 0, 0, 0, e^{12}, -e^{14} + e^{23}, e^{24} + e^{13}, e^{15}$          | $1/32(14, 14, 25, 25, 28, 39, 39, 42)$     | $\{\emptyset, 12348, 12678, 1356, 1457, 23578, 24568, 3467\}$                                                 |
| 841:23  | $0, 0, 0, 0, e^{12}, e^{34}, e^{14} + e^{23}, e^{13} + e^{25}$           | $1/40(23, 15, 30, 22, 38, 52, 45, 53)$     | $\{123678, 13458, 23457, 36\}$                                                                                |
| 841:24  | $0, 0, 0, 0, e^{12}, e^{13}, e^{14} + e^{23}, e^{24} + e^{15}$           | $1/17(7, 9, 12, 14, 16, 19, 21, 23)$       | $\{\emptyset, 12678, 1357, 23568\}$                                                                           |
| 841:25a | $0, 0, 0, 0, e^{12}, e^{14} + e^{23}, e^{24} + e^{13}, e^{34} + e^{15}$  | $15/64(2, 2, 3, 3, 4, 5, 5, 6)$            | $\{\emptyset, 23578, 24568, 3467\}$                                                                           |
| 841:25b | $0, 0, 0, 0, e^{12}, -e^{14} + e^{23}, e^{24} + e^{13}, e^{34} + e^{15}$ | $15/64(2, 2, 3, 3, 4, 5, 5, 6)$            | $\{\emptyset, 23578, 24568, 3467\}$                                                                           |
| 841:29  | $0, 0, 0, 0, e^{12}, e^{13}, e^{14}, e^{25} + e^{16}$                    | $1/31(10, 17, 24, 26, 27, 34, 36, 44)$     | $\{\emptyset, 12348, 12378, 13458, 13578, 2457, 25, 47\}$                                                     |
| 841:30  | $0, 0, 0, 0, e^{12}, e^{13}, e^{24}, e^{25} + e^{16}$                    | $1/19(7, 10, 13, 14, 17, 20, 24, 27)$      | $\{\emptyset, 12348, 12378, 134578, 1358, 245, 257, 47\}$                                                     |
| 841:31a | $0, 0, 0, 0, e^{12}, e^{13}, e^{14}, e^{36} + e^{25}$                    | $1/20(8, 11, 11, 16, 19, 19, 24, 30)$      | $\{\emptyset, 12348, 12378, 12468, 12678, 13458, 13578, 14568, 15678, 234567, 2356, 2457, 25, 3467, 36, 47\}$ |
| 841:31b | $0, 0, 0, 0, -e^{12}, e^{13}, e^{14}, e^{36} + e^{25}$                   | $1/20(8, 11, 11, 16, 19, 19, 24, 30)$      | $\{\emptyset, 12348, 12378, 12468, 12678, 13458, 13578, 14568, 15678, 234567, 2356, 2457, 25, 3467, 36, 47\}$ |
| 841:32  | $0, 0, 0, 0, e^{12}, e^{13}, e^{14}, e^{26} + e^{35}$                    | $1/20(8, 11, 11, 16, 19, 19, 24, 30)$      | $\{\emptyset, 12348, 12378, 1246, 1267, 1345, 1357, 14568, 15678, 234567, 2356, 24578, 258, 34678, 368, 47\}$ |
| 841:33  | $0, 0, 0, 0, e^{12}, e^{13}, e^{24}, e^{36} + e^{15}$                    | $1/18(8, 10, 9, 13, 18, 17, 23, 26)$       | $\{\emptyset, 12348, 12378, 12468, 12678, 3467, 36, 47\}$                                                     |
| 841:34a | $0, 0, 0, 0, e^{12}, e^{13}, e^{24}, e^{36} + e^{25}$                    | $1/9(5, 4, 4, 7, 9, 9, 11, 13)$            | $\{\emptyset, 12348, 12378, 12468, 12678, 134578, 1358, 145678, 1568, 23456, 23567, 245, 257, 3467, 36, 47\}$ |
| 841:34b | $0, 0, 0, 0, -e^{12}, e^{13}, e^{24}, e^{36} + e^{25}$                   | $1/9(5, 4, 4, 7, 9, 9, 11, 13)$            | $\{\emptyset, 12348, 12378, 12468, 12678, 134578, 1358, 145678, 1568, 23456, 23567, 245, 257, 3467, 36, 47\}$ |
| 841:35  | $0, 0, 0, 0, e^{12}, e^{13}, e^{24}, e^{26} + e^{35}$                    | $1/20(11, 8, 10, 16, 19, 21, 24, 29)$      | $\{\emptyset, 12348, 12378, 1246, 1267, 13457, 135, 145678, 1568, 23456, 23567, 2458, 2578, 34678, 368, 47\}$ |
| 841:36  | $0, 0, 0, 0, e^{12}, e^{13}, e^{14} + e^{23}, e^{25} + e^{16}$           | $1/112(40, 59, 78, 97, 99, 118, 137, 158)$ | $\{\emptyset, 12348, 13578, 2457\}$                                                                           |
| 841:37a | $0, 0, 0, 0, e^{12}, e^{13}, e^{14} + e^{23}, e^{36} + e^{25}$           | $1/19(7, 11, 11, 15, 18, 18, 22, 29)$      | $\{12378, 12468, 13458, 15678, 234567, 25, 36, 47\}$                                                          |
| 841:37b | $0, 0, 0, 0, -e^{12}, e^{13}, e^{14} + e^{23}, e^{36} + e^{25}$          | $1/19(7, 11, 11, 15, 18, 18, 22, 29)$      | $\{12378, 12468, 13458, 15678, 234567, 25, 36, 47\}$                                                          |
| 841:38  | $0, 0, 0, 0, e^{12}, e^{13}, e^{14} + e^{23}, e^{26} + e^{35}$           | $1/19(7, 11, 11, 15, 18, 18, 22, 29)$      | $\{12378, 1246, 1345, 15678, 234567, 258, 368, 47\}$                                                          |
| 841:39  | $0, 0, 0, 0, e^{12}, e^{13}, e^{14}, e^{24} + e^{36} + e^{15}$           | $1/79(30, 56, 43, 60, 86, 73, 90, 116)$    | $\{\emptyset, 12378, 12678, 36\}$                                                                             |
| 841:40a | $0, 0, 0, 0, e^{12}, e^{13}, e^{24}, e^{36} + e^{25} + e^{14}$           | $1/17(10, 7, 7, 14, 17, 17, 21, 24)$       | $\{12348, 12468, 134578, 145678, 23456, 245, 3467, 47\}$                                                      |
| 841:40b | $0, 0, 0, 0, -e^{12}, e^{13}, e^{24}, e^{36} + e^{25} + e^{14}$          | $1/17(10, 7, 7, 14, 17, 17, 21, 24)$       | $\{12348, 12468, 134578, 145678, 23456, 245, 3467, 47\}$                                                      |
| 841:41  | $0, 0, 0, 0, e^{12}, e^{13}, e^{24}, e^{26} + e^{35} + e^{14}$           | $1/19(11, 7, 9, 16, 18, 20, 23, 27)$       | $\{12348, 1267, 135, 145678, 23456, 2578, 368, 47\}$                                                          |
| 841:44  | $0, 0, 0, 0, e^{12}, e^{13}, e^{23}, e^{24} + e^{36} + e^{15}$           | $1/29(13, 17, 15, 26, 30, 28, 32, 43)$     | $\{\emptyset, 1238, 12678, 367\}$                                                                             |
| 841:46  | $0, 0, 0, 0, e^{12}, e^{13}, e^{14} + e^{23}, e^{24} + e^{36} + e^{15}$  | $53/401(3, 5, 4, 6, 8, 7, 9, 11)$          | $\{\emptyset, 12678\}$                                                                                        |
| 841:49  | $0, 0, 0, 0, e^{12}, e^{34}, e^{13}, e^{36} + e^{15}$                    | $1/11(5, 7, 5, 7, 12, 12, 10, 17)$         | $\{123478, 12468, 13567, 15, 23458, 245678, 36, 7\}$                                                          |
| 841:50  | $0, 0, 0, 0, e^{12}, e^{34}, e^{13}, e^{36} + e^{25}$                    | $1/47(30, 20, 19, 32, 50, 51, 49, 70)$     | $\{\emptyset, 12348, 124678, 13458, 145678, 23567, 25, 367\}$                                                 |
| 841:51  | $0, 0, 0, 0, e^{12}, e^{34}, e^{13}, e^{46} + e^{25}$                    | $1/28(16, 13, 16, 13, 29, 29, 32, 42)$     | $\{\emptyset, 12348, 12368, 13458, 13568, 2456, 25, 46\}$                                                     |

Table A.1 – Continued to next page

Table A.1 – Continued from previous page

| Name    | $\mathfrak{g}$                                                                    | $N$                                           | Signatures $\mathbf{S}$                                                                                       |
|---------|-----------------------------------------------------------------------------------|-----------------------------------------------|---------------------------------------------------------------------------------------------------------------|
| 841:52  | $0, 0, 0, 0, e^{12}, e^{34}, e^{24} + e^{13}, e^{36} + e^{15}$                    | 13/25(1, 1, 1, 1, 2, 2, 2, 3)                 | {12468, 15, 23458, 36}                                                                                        |
| 841:53  | $0, 0, 0, 0, e^{12}, e^{34}, e^{14} + e^{23}, e^{36} + e^{15}$                    | 1/29(12, 19, 12, 19, 31, 31, 31, 43)          | { $\emptyset$ , 12348, 13567, 245678}                                                                         |
| 841:54  | $0, 0, 0, 0, -e^{12}, e^{14} + e^{23}, e^{13}, e^{35} + e^{16}$                   | 1/19(7, 11, 11, 15, 18, 22, 18, 29)           | {123478, 126, 13567, 1458, 235, 245678, 3468, 7}                                                              |
| 841:55  | $0, 0, 0, 0, e^{12}, e^{14} + e^{23}, e^{13}, e^{45} + e^{26}$                    | 1/12(6, 5, 8, 7, 11, 13, 14, 18)              | { $\emptyset$ , 12348, 1267, 13568, 1457, 23578, 2456, 34678}                                                 |
| 841:56  | $0, 0, 0, 0, -e^{12}, e^{14} + e^{23}, e^{34}, e^{35} + e^{16}$                   | 1/13(5, 8, 6, 9, 13, 14, 15, 19)              | { $\emptyset$ , 12348, 126, 13567, 14578, 2357, 245678, 3468}                                                 |
| 841:57  | $0, 0, 0, 0, e^{12}, e^{34}, e^{13}, e^{46} + e^{15} + e^{23}$                    | 1/43(15, 32, 30, 16, 47, 46, 45, 62)          | {12348, 12368, 234578, 235678}                                                                                |
| 841:58  | $0, 0, 0, 0, e^{12}, e^{34}, e^{13}, e^{24} + e^{36} + e^{15}$                    | 3/8(1, 2, 1, 2, 3, 3, 2, 4)                   | {123478, 12468, 23458, 245678}                                                                                |
| 841:60a | $0, 0, 0, 0, e^{14} + e^{23}, e^{24} + e^{13}, e^{12}, e^{26} + e^{15}$           | 1/11(5, 5, 7, 7, 12, 12, 10, 17)              | {123478, 12567, 135, 1468, 236, 2458, 345678, 7}                                                              |
| 841:60b | $0, 0, 0, 0, -e^{14} + e^{23}, e^{24} + e^{13}, e^{12}, e^{26} + e^{15}$          | 1/11(5, 5, 7, 7, 12, 12, 10, 17)              | {123478, 12567, 135, 1468, 236, 2458, 345678, 7}                                                              |
| 841:61a | $0, 0, 0, 0, e^{14} + e^{23}, e^{24} + e^{13}, e^{12}, e^{46} + e^{35}$           | 1/28(16, 16, 13, 13, 29, 29, 32, 42)          | { $\emptyset$ , 12348, 12568, 1357, 1467, 23678, 24578, 3456}                                                 |
| 841:61b | $0, 0, 0, 0, e^{14} - e^{23}, e^{24} + e^{13}, e^{12}, e^{35} + e^{46}$           | 1/28(16, 16, 13, 13, 29, 29, 32, 42)          | { $\emptyset$ , 12348, 12568, 1357, 1467, 23678, 24578, 3456}                                                 |
| 841:62  | $0, 0, 0, 0, e^{12}, e^{34}, e^{24} + e^{13}, e^{46} + e^{15} + e^{23}$           | 19/53(1, 2, 2, 1, 3, 3, 3, 4)                 | {12348, 235678}                                                                                               |
| 841:63  | $0, 0, 0, 0, -e^{12}, e^{14} + e^{23}, e^{13}, e^{24} + e^{35} + e^{16}$          | 1/16(5, 10, 9, 14, 15, 19, 14, 24)            | {123478, 126, 235, 245678}                                                                                    |
| 841:64  | $0, 0, 0, 0, e^{12}, e^{24} + e^{13}, e^{34}, e^{26} + e^{35} + e^{14}$           | 1/12(8, 4, 5, 9, 12, 13, 14, 17)              | {12348, 126, 1357, 145678}                                                                                    |
| 841:66a | $0, 0, 0, 0, e^{14} + e^{23}, e^{24} + e^{13}, e^{12}, e^{26} + e^{34} + e^{15}$  | 3/8(1, 1, 2, 2, 3, 3, 2, 4)                   | {123478, 135, 236, 345678}                                                                                    |
| 841:66b | $0, 0, 0, 0, -e^{14} + e^{23}, e^{24} + e^{13}, e^{12}, e^{26} + e^{34} + e^{15}$ | 3/8(1, 1, 2, 2, 3, 3, 2, 4)                   | {123478, 135, 236, 345678}                                                                                    |
| 841:67a | $0, 0, 0, 0, e^{12}, e^{13}, e^{14}, e^{36} + e^{25} + e^{17}$                    | 1/19(7, 11, 11, 15, 18, 18, 22, 29)           | { $\emptyset$ , 12348, 12468, 13458, 14568, 2356, 25, 36}                                                     |
| 841:67b | $0, 0, 0, 0, -e^{12}, e^{13}, e^{14}, e^{36} + e^{25} + e^{17}$                   | 1/19(7, 11, 11, 15, 18, 18, 22, 29)           | { $\emptyset$ , 12348, 12468, 13458, 14568, 2356, 25, 36}                                                     |
| 841:68  | $0, 0, 0, 0, e^{12}, e^{13}, e^{14}, e^{26} + e^{35} + e^{17}$                    | 1/19(7, 11, 11, 15, 18, 18, 22, 29)           | { $\emptyset$ , 12348, 1267, 1357, 14568, 2356, 24578, 34678}                                                 |
| 841:69  | $0, 0, 0, 0, e^{12}, e^{13}, e^{24}, e^{36} + e^{27} + e^{15}$                    | 1/281(156, 118, 137, 194, 274, 293, 312, 430) | { $\emptyset$ , 12348, 12468, 36}                                                                             |
| 841:70a | $0, 0, 0, 0, e^{12}, e^{13}, e^{14}, e^{47} + e^{36} + e^{25}$                    | 1/5(2, 3, 3, 3, 5, 5, 5, 8)                   | { $\emptyset$ , 12348, 12378, 12468, 12678, 13458, 13578, 14568, 15678, 234567, 2356, 2457, 25, 3467, 36, 47} |
| 841:70b | $0, 0, 0, 0, e^{12}, -e^{13}, e^{14}, e^{36} + e^{25} + e^{47}$                   | 1/5(2, 3, 3, 3, 5, 5, 5, 8)                   | { $\emptyset$ , 12348, 12378, 12468, 12678, 13458, 13578, 14568, 15678, 234567, 2356, 2457, 25, 3467, 36, 47} |
| 841:71  | $0, 0, 0, 0, e^{12}, e^{13}, e^{14}, e^{47} + e^{26} + e^{35}$                    | 1/5(2, 3, 3, 3, 5, 5, 5, 8)                   | { $\emptyset$ , 12348, 12378, 14568, 15678, 234567, 2356, 47}                                                 |
| 841:72a | $0, 0, 0, 0, e^{12}, e^{13}, e^{24}, e^{36} + e^{15} + e^{47}$                    | 1/89(44, 50, 47, 44, 94, 91, 94, 138)         | { $\emptyset$ , 12348, 12378, 12468, 12678, 3467, 36, 47}                                                     |
| 841:72b | $0, 0, 0, 0, -e^{12}, e^{13}, e^{24}, e^{47} + e^{36} + e^{15}$                   | 1/89(44, 50, 47, 44, 94, 91, 94, 138)         | { $\emptyset$ , 12348, 12378, 12468, 12678, 3467, 36, 47}                                                     |
| 841:73  | $0, 0, 0, 0, -e^{12}, e^{13}, e^{24}, e^{36} + e^{17} + e^{45}$                   | 1/9(4, 5, 5, 5, 9, 9, 10, 14)                 | { $\emptyset$ , 12348, 12468, 1358, 1568, 23456, 245, 36}                                                     |
| 841:75a | $0, 0, 0, 0, e^{12}, e^{13}, e^{14} + e^{23}, e^{45} + e^{27} + e^{16}$           | 1/11(5, 5, 7, 7, 10, 12, 12, 17)              | { $\emptyset$ , 12348, 1267, 13578, 1456, 23568, 2457, 34678}                                                 |
| 841:75b | $0, 0, 0, 0, e^{12}, -e^{13}, e^{14} + e^{23}, e^{27} + e^{16} + e^{45}$          | 1/11(5, 5, 7, 7, 10, 12, 12, 17)              | { $\emptyset$ , 12348, 1267, 13578, 1456, 23568, 2457, 34678}                                                 |
| 841:76  | $0, 0, 0, 0, e^{12}, e^{13}, e^{14} + e^{23}, e^{46} + e^{25} + e^{37}$           | 1/100(46, 56, 51, 61, 102, 97, 107, 158)      | { $\emptyset$ , 12348, 12678, 3467}                                                                           |
| 841:77  | $0, 0, 0, 0, e^{12}, e^{34}, e^{24} + e^{13}, e^{37} + e^{26} + e^{15}$           | 1/179(97, 83, 90, 104, 180, 194, 187, 277)    | { $\emptyset$ , 12348, 1278, 347}                                                                             |
| 841:79a | $0, 0, 0, 0, e^{12}, e^{14} + e^{23}, e^{24} + e^{13}, e^{47} + e^{36} + e^{15}$  | 13/25(1, 1, 1, 1, 2, 2, 2, 3)                 | { $\emptyset$ , 12348, 12678, 1356, 1457, 23578, 24568, 3467}                                                 |
| 841:79b | $0, 0, 0, 0, e^{12}, e^{14} - e^{23}, e^{24} + e^{13}, e^{36} + e^{15} + e^{47}$  | 13/25(1, 1, 1, 1, 2, 2, 2, 3)                 | { $\emptyset$ , 12348, 12678, 1356, 1457, 23578, 24568, 3467}                                                 |
| 841:79c | $0, 0, 0, 0, -e^{12}, e^{14} + e^{23}, e^{24} + e^{13}, e^{47} + e^{36} + e^{15}$ | 13/25(1, 1, 1, 1, 2, 2, 2, 3)                 | { $\emptyset$ , 12348, 12678, 1356, 1457, 23578, 24568, 3467}                                                 |
| 841:80a | $0, 0, 0, 0, e^{12}, e^{14} + e^{23}, e^{24} + e^{13}, e^{37} + e^{15} + e^{46}$  | 13/25(1, 1, 1, 1, 2, 2, 2, 3)                 | { $\emptyset$ , 12348, 12678, 3467}                                                                           |
| 841:80b | $0, 0, 0, 0, e^{12}, -e^{14} + e^{23}, e^{24} + e^{13}, e^{46} + e^{37} + e^{15}$ | 13/25(1, 1, 1, 1, 2, 2, 2, 3)                 | { $\emptyset$ , 12348, 12678, 3467}                                                                           |
| 84:1    | $0, 0, 0, 0, e^{12}, e^{13}, e^{23}, e^{14}$                                      | 1/8(4, 5, 5, 6, 9, 9, 10, 10)                 | { $\emptyset$ , 1234, 1238, 12467, 12678, 13457, 13578, 1456, 1568, 234568, 2356, 24578, 257, 34678, 367, 48} |
| 84:2    | $0, 0, 0, 0, e^{12}, e^{13}, e^{24}, e^{34}$                                      | 3/5(1, 1, 1, 1, 2, 2, 2, 2)                   | { $\emptyset$ , 1234, 12378, 12468, 1267, 13457, 1358, 145678, 156, 23456, 235678, 2458, 257, 3467, 368, 478} |
| 84:3    | $0, 0, 0, 0, e^{12}, e^{13}, e^{24}, e^{14} + e^{23}$                             | 1/9(5, 5, 6, 6, 10, 11, 11, 11)               | { $\emptyset$ , 1234, 12678, 1358, 14567, 23567, 2458, 34678}                                                 |
| 84:4a   | $0, 0, 0, 0, e^{12}, e^{34}, e^{14} + e^{23}, e^{24} + e^{13}$                    | 3/5(1, 1, 1, 1, 2, 2, 2, 2)                   | { $\emptyset$ , 1234, 1278, 13567, 14568, 23568, 24567, 3478}                                                 |
| 84:4b   | $0, 0, 0, 0, e^{12}, e^{34}, -e^{14} + e^{23}, e^{24} + e^{13}$                   | 3/5(1, 1, 1, 1, 2, 2, 2, 2)                   | { $\emptyset$ , 1234, 1278, 13567, 14568, 23568, 24567, 3478}                                                 |
| 8321:5  | $0, 0, 0, 0, 0, e^{12}, e^{16}, e^{45} + e^{17} + e^{23}$                         | 1/24(7, 15, 21, 18, 18, 22, 29, 36)           | { $\emptyset$ , 123457, 1237, 13468, 13568, 24678, 25678, 45}                                                 |
| 8321:8  | $0, 0, 0, 0, 0, -e^{12}, e^{16} + e^{23}, e^{36} + e^{17} + e^{45}$               | 1/9(3, 5, 6, 7, 7, 8, 11, 14)                 | { $\emptyset$ , 12457, 127, 1468, 1568, 24678, 25678, 45}                                                     |
| 832:6   | $0, 0, 0, 0, 0, e^{12}, e^{34} + e^{16}, e^{26} + e^{35}$                         | 1/15(7, 7, 9, 12, 12, 14, 21, 21)             | { $\emptyset$ , 12378, 124578, 13468, 1568, 23567, 2467, 345}                                                 |

Table A.1 – Continued to next page

Table A.1 – Continued from previous page

| Name    | $g$                                                                          | $N$                                     | Signatures $S$                                                                                                |
|---------|------------------------------------------------------------------------------|-----------------------------------------|---------------------------------------------------------------------------------------------------------------|
| 832:8   | $0, 0, 0, 0, 0, e^{12}, e^{16}, e^{13} + e^{26} + e^{45}$                    | $1/41(16, 21, 42, 29, 29, 37, 53, 58)$  | $\{123478, 123578, 13468, 13568, 234567, 2367, 3, 345\}$                                                      |
| 832:9   | $0, 0, 0, 0, 0, e^{12}, e^{13} + e^{26}, e^{45} + e^{16}$                    | $1/27(13, 12, 24, 19, 19, 25, 37, 38)$  | $\{\emptyset, 12478, 12578, 14567, 167, 2468, 2568, 45\}$                                                     |
| 832:10  | $0, 0, 0, 0, 0, e^{12}, e^{34} + e^{16}, e^{13} + e^{26} + e^{45}$           | $1/14(7, 6, 12, 8, 11, 13, 20, 19)$     | $\{123578, 13468, 2367, 345\}$                                                                                |
| 832:12  | $0, 0, 0, 0, 0, e^{12}, e^{13} + e^{26}, e^{24} + e^{35} + e^{16}$           | $1/19(10, 7, 14, 20, 13, 17, 24, 27)$   | $\{123478, 134567, 23468, 345\}$                                                                              |
| 832:13  | $0, 0, 0, 0, 0, e^{12}, e^{24} + e^{35} + e^{16}, e^{13} + e^{26} + e^{45}$  | $5/11(1, 1, 2, 2, 1, 2, 3, 3)$          | $\{123478, 345\}$                                                                                             |
| 831:9   | $0, 0, 0, 0, 0, e^{12}, e^{34}, e^{35} + e^{16}$                             | $1/21(8, 14, 12, 15, 18, 22, 27, 30)$   | $\{\emptyset, 12348, 12378, 124578, 1258, 13456, 13567, 1467, 16, 23468, 23678, 245678, 2568, 345, 357, 47\}$ |
| 831:11  | $0, 0, 0, 0, 0, e^{12}, e^{45} + e^{13}, e^{26}$                             | $1/21(12, 8, 18, 15, 15, 20, 30, 28)$   | $\{\emptyset, 123458, 1238, 12478, 12578, 134568, 1368, 14678, 15678, 23467, 23567, 2456, 26, 347, 357, 45\}$ |
| 831:14  | $0, 0, 0, 0, 0, e^{12}, e^{13}, e^{16} + e^{45}$                             | $1/11(4, 8, 9, 8, 8, 12, 13, 16)$       | $\{\emptyset, 12348, 12358, 12478, 12578, 13456, 136, 14567, 167, 234678, 235678, 2468, 2568, 3457, 37, 45\}$ |
| 831:15  | $0, 0, 0, 0, 0, e^{12}, e^{13}, e^{45} + e^{26}$                             | $1/4(2, 2, 3, 3, 3, 4, 5, 6)$           | $\{\emptyset, 12348, 12358, 12478, 12578, 13468, 13568, 14678, 15678, 234567, 2367, 2456, 26, 3457, 37, 45\}$ |
| 831:18  | $0, 0, 0, 0, 0, e^{12}, e^{13} + e^{45}, e^{34} + e^{16}$                    | $1/41(16, 27, 36, 23, 29, 43, 52, 59)$  | $\{123578, 12458, 13467, 16, 2368, 24678, 345, 57\}$                                                          |
| 831:19  | $0, 0, 0, 0, 0, e^{12}, e^{45} + e^{13}, e^{26} + e^{34}$                    | $1/27(16, 11, 21, 17, 20, 27, 37, 38)$  | $\{\emptyset, 1238, 12478, 1368, 14678, 23467, 26, 347\}$                                                     |
| 831:22  | $0, 0, 0, 0, 0, e^{12}, e^{14} + e^{23}, e^{35} + e^{16}$                    | $1/37(15, 23, 24, 32, 29, 38, 47, 53)$  | $\{\emptyset, 12348, 12578, 13567, 146, 2368, 245678, 3457\}$                                                 |
| 831:23  | $0, 0, 0, 0, 0, e^{12}, e^{34}, e^{13} + e^{26} + e^{45}$                    | $1/41(28, 15, 30, 23, 35, 43, 53, 58)$  | $\{12348, 123578, 13468, 135678, 23456, 2367, 345, 37\}$                                                      |
| 831:24  | $0, 0, 0, 0, 0, e^{12}, e^{35} + e^{14}, e^{13} + e^{26}$                    | $1/41(24, 15, 30, 35, 29, 39, 59, 54)$  | $\{123458, 12378, 134568, 13678, 23467, 2356, 347, 35\}$                                                      |
| 831:25  | $0, 0, 0, 0, 0, e^{12}, e^{13} + e^{45}, e^{16} + e^{23}$                    | $1/41(18, 23, 36, 27, 27, 41, 54, 59)$  | $\{12458, 128, 1456, 16, 24678, 25678, 47, 57\}$                                                              |
| 831:27  | $0, 0, 0, 0, 0, e^{12}, e^{13}, e^{26} + e^{35} + e^{14}$                    | $1/23(12, 11, 15, 22, 19, 23, 27, 34)$  | $\{\emptyset, 1238, 12578, 1368, 15678, 23567, 26, 357\}$                                                     |
| 831:28  | $0, 0, 0, 0, 0, e^{12}, e^{13}, e^{45} + e^{16} + e^{23}$                    | $1/23(9, 16, 18, 17, 17, 25, 27, 34)$   | $\{\emptyset, 12478, 12578, 14567, 167, 2468, 2568, 45\}$                                                     |
| 831:29  | $0, 0, 0, 0, 0, e^{12}, e^{13}, e^{24} + e^{35} + e^{16}$                    | $1/16(7, 10, 11, 14, 13, 17, 18, 24)$   | $\{\emptyset, 1238, 12578, 1356, 167, 23678, 2568, 357\}$                                                     |
| 831:30  | $0, 0, 0, 0, 0, e^{12}, e^{24} + e^{13}, e^{26} + e^{15}$                    | $1/16(8, 7, 13, 14, 14, 15, 21, 22)$    | $\{\emptyset, 12348, 1278, 1368, 14678, 2367, 246, 347\}$                                                     |
| 831:32  | $0, 0, 0, 0, 0, e^{12}, e^{13} + e^{45}, e^{24} + e^{35} + e^{16}$           | $1/19(7, 13, 17, 14, 10, 20, 24, 27)$   | $\{123478, 12458, 345, 47\}$                                                                                  |
| 831:33  | $0, 0, 0, 0, 0, e^{12}, e^{24} + e^{13}, e^{26} + e^{35} + e^{14}$           | $1/38(23, 16, 25, 32, 30, 39, 48, 55)$  | $\{\emptyset, 12578, 1368, 23567\}$                                                                           |
| 831:34  | $0, 0, 0, 0, 0, e^{12}, e^{24} + e^{13}, e^{26} + e^{34} + e^{15}$           | $1/13(7, 6, 9, 10, 12, 13, 16, 19)$     | $\{\emptyset, 1368, 14678, 347\}$                                                                             |
| 831:41  | $0, 0, 0, 0, 0, e^{12}, e^{13}, e^{45} + e^{26} + e^{17}$                    | $1/68(28, 39, 50, 53, 53, 67, 78, 106)$ | $\{\emptyset, 12348, 12358, 13468, 13568, 2456, 26, 45\}$                                                     |
| 831:42a | $0, 0, 0, 0, 0, e^{12}, e^{13}, e^{37} + e^{26} + e^{45}$                    | $1/20(10, 11, 11, 16, 16, 21, 21, 32)$  | $\{\emptyset, 12348, 12358, 12478, 12578, 13468, 13568, 14678, 15678, 234567, 2367, 2456, 26, 3457, 37, 45\}$ |
| 831:42b | $0, 0, 0, 0, 0, -e^{12}, e^{13}, e^{45} + e^{37} + e^{26}$                   | $1/20(10, 11, 11, 16, 16, 21, 21, 32)$  | $\{\emptyset, 12348, 12358, 12478, 12578, 13468, 13568, 14678, 15678, 234567, 2367, 2456, 26, 3457, 37, 45\}$ |
| 831:43  | $0, 0, 0, 0, 0, e^{12}, e^{13}, e^{36} + e^{27} + e^{45}$                    | $1/20(10, 11, 11, 16, 16, 21, 21, 32)$  | $\{\emptyset, 12348, 12358, 12457, 127, 13456, 136, 14678, 15678, 234567, 2367, 2468, 2568, 3478, 3578, 45\}$ |
| 831:47  | $0, 0, 0, 0, 0, e^{12}, e^{34}, e^{37} + e^{26} + e^{15}$                    | $1/39(24, 18, 17, 26, 36, 42, 43, 60)$  | $\{\emptyset, 12348, 12478, 13468, 14678, 2367, 26, 37\}$                                                     |
| 831:50  | $0, 0, 0, 0, 0, e^{12}, e^{24} + e^{13}, e^{36} + e^{27} + e^{15}$           | $1/19(11, 7, 11, 15, 18, 18, 22, 29)$   | $\{\emptyset, 12348, 1257, 1356, 14678, 2367, 24568, 34578\}$                                                 |
| 831:51  | $0, 0, 0, 0, 0, -e^{12}, e^{24} + e^{13}, e^{46} + e^{35} + e^{17}$          | $1/7(3, 4, 5, 4, 6, 7, 8, 11)$          | $\{\emptyset, 12348, 127, 1368, 1467, 23678, 246, 3478\}$                                                     |
| 831:53a | $0, 0, 0, 0, 0, e^{13}, e^{12} + e^{34}, e^{37} + e^{26} + e^{15}$           | $1/11(7, 5, 5, 7, 10, 12, 12, 17)$      | $\{\emptyset, 12348, 1256, 1357, 14678, 2367, 24578, 34568\}$                                                 |
| 831:53b | $0, 0, 0, 0, 0, -e^{24} + e^{13}, e^{12} + e^{34}, e^{37} + e^{26} + e^{15}$ | $1/11(7, 5, 5, 7, 10, 12, 12, 17)$      | $\{\emptyset, 12348, 1256, 1357, 14678, 2367, 24578, 34568\}$                                                 |
| 831:54a | $0, 0, 0, 0, 0, e^{24} + e^{13}, e^{12} + e^{34}, e^{36} + e^{27} + e^{15}$  | $1/11(7, 5, 5, 7, 10, 12, 12, 17)$      | $\{\emptyset, 12348, 1268, 1378, 14678, 2367, 247, 346\}$                                                     |
| 831:54b | $0, 0, 0, 0, 0, e^{24} - e^{13}, e^{12} + e^{34}, e^{36} + e^{27} + e^{15}$  | $1/11(7, 5, 5, 7, 10, 12, 12, 17)$      | $\{\emptyset, 12348, 1268, 1378, 14678, 2367, 247, 346\}$                                                     |
| 831:55  | $0, 0, 0, 0, 0, e^{14} + e^{23}, e^{13} + e^{25}, e^{27} + e^{16}$           | $3/8(1, 1, 2, 2, 2, 3, 3, 4)$           | $\{\emptyset, 123458, 1267, 136, 14578, 237, 24568, 345678\}$                                                 |
| 83:9    | $0, 0, 0, 0, 0, e^{12}, e^{13}, e^{25} + e^{14}$                             | $1/8(4, 5, 6, 7, 6, 9, 10, 11)$         | $\{\emptyset, 12345, 1238, 12457, 1278, 1346, 13568, 1467, 15678, 234678, 23567, 2468, 256, 34578, 37, 458\}$ |
| 83:10   | $0, 0, 0, 0, 0, e^{12}, e^{13}, e^{23} + e^{45}$                             | $1/13(7, 9, 9, 9, 9, 16, 16, 18)$       | $\{\emptyset, 123, 12345, 12478, 12578, 13468, 13568, 14567, 167, 234567, 2367, 2468, 2568, 3478, 3578, 45\}$ |
| 83:11   | $0, 0, 0, 0, 0, e^{12}, e^{13}, e^{24} + e^{35}$                             | $1/5(3, 3, 3, 4, 4, 6, 6, 7)$           | $\{\emptyset, 12345, 1238, 1247, 12578, 13468, 1356, 145678, 167, 234567, 23678, 246, 2568, 3478, 357, 458\}$ |

Table A.1 – Continued to next page

Table A.1 – Continued from previous page

| Name   | $\mathfrak{g}$                                                         | $N$                                    | Signatures $\mathbf{S}$                                                                                       |
|--------|------------------------------------------------------------------------|----------------------------------------|---------------------------------------------------------------------------------------------------------------|
| 83:12  | $0, 0, 0, 0, 0, e^{12}, e^{34}, e^{13} + e^{25}$                       | $1/13(9, 7, 8, 9, 10, 16, 17, 17)$     | $\{\emptyset, 12345, 12357, 12478, 128, 1346, 1367, 145678, 1568, 23468, 23678, 24567, 256, 3458, 3578, 47\}$ |
| 83:13  | $0, 0, 0, 0, 0, e^{12}, e^{14} + e^{23}, e^{13} + e^{25}$              | $1/9(5, 5, 7, 7, 7, 10, 12, 12)$       | $\{\emptyset, 12345, 1278, 1367, 14568, 2368, 24567, 34578\}$                                                 |
| 83:14  | $0, 0, 0, 0, 0, e^{12}, e^{14} + e^{23}, e^{13} + e^{45}$              | $1/14(9, 8, 10, 9, 10, 17, 18, 19)$    | $\{\emptyset, 12345, 12578, 1367, 1468, 23568, 24567, 3478\}$                                                 |
| 83:15  | $0, 0, 0, 0, 0, e^{12}, e^{24} + e^{13}, e^{34} + e^{15}$              | $1/11(6, 7, 8, 7, 9, 13, 14, 15)$      | $\{\emptyset, 12345, 1257, 1368, 14678, 235678, 24568, 347\}$                                                 |
| 83:16a | $0, 0, 0, 0, 0, e^{24} + e^{13}, e^{12} + e^{34}, e^{15}$              | $1/7(4, 5, 5, 4, 5, 9, 9, 9)$          | $\{\emptyset, 12345, 12348, 1256, 1268, 1357, 1378, 14567, 14678, 235678, 2367, 24578, 247, 34568, 346, 58\}$ |
| 83:16b | $0, 0, 0, 0, 0, e^{24} - e^{13}, e^{12} + e^{34}, e^{15}$              | $1/7(4, 5, 5, 4, 5, 9, 9, 9)$          | $\{\emptyset, 12345, 12348, 1256, 1268, 1357, 1378, 14567, 14678, 235678, 2367, 24578, 247, 34568, 346, 58\}$ |
| 83:17  | $0, 0, 0, 0, 0, e^{12}, e^{35} + e^{14}, e^{23} + e^{45}$              | $1/16(10, 10, 11, 11, 10, 20, 21, 21)$ | $\{\emptyset, 12345, 1237, 1248, 12578, 3478, 358, 457\}$                                                     |
| 83:18a | $0, 0, 0, 0, 0, e^{14} + e^{23}, e^{24} + e^{13}, e^{12} + e^{35}$     | $1/15(10, 10, 9, 9, 11, 19, 19, 20)$   | $\{\emptyset, 12345, 1267, 1368, 14578, 2378, 24568, 34567\}$                                                 |
| 83:18b | $0, 0, 0, 0, 0, -e^{14} + e^{23}, e^{24} + e^{13}, e^{12} + e^{35}$    | $1/15(10, 10, 9, 9, 11, 19, 19, 20)$   | $\{\emptyset, 12345, 1267, 1368, 14578, 2378, 24568, 34567\}$                                                 |
| 83:19  | $0, 0, 0, 0, 0, e^{14} + e^{23}, e^{13} + e^{25}, e^{45} + e^{12}$     | $11/17(1, 1, 1, 1, 1, 2, 2, 2)$        | $\{\emptyset, 12345, 1267, 34567\}$                                                                           |
| 83:20  | $0, 0, 0, 0, 0, e^{24} + e^{13}, e^{15} + e^{23}, e^{25} + e^{14}$     | $1/7(4, 4, 5, 5, 5, 9, 9, 9)$          | $\{\emptyset, 12345, 12678, 345678\}$                                                                         |
| 821:5  | $0, 0, 0, 0, 0, 0, e^{12}, e^{56} + e^{34} + e^{17}$                   | $1/15(7, 10, 12, 12, 12, 12, 17, 24)$  | $\{\emptyset, 12358, 12368, 12458, 12468, 134567, 1347, 1567, 17, 23578, 23678, 24578, 24678, 34, 3456, 56\}$ |
| 82:8   | $0, 0, 0, 0, 0, 0, e^{12}, e^{24} + e^{13} + e^{56}$                   | $1/8(5, 5, 7, 7, 6, 6, 10, 12)$        | $\{\emptyset, 1234, 123456, 1258, 1268, 13567, 137, 14578, 14678, 23578, 23678, 24567, 247, 3458, 3468, 56\}$ |
| 82:9   | $0, 0, 0, 0, 0, 0, e^{24} + e^{13}, e^{56} + e^{12}$                   | $1/13(9, 9, 10, 10, 9, 9, 19, 18)$     | $\{\emptyset, 1234, 123456, 12567, 127, 1358, 1368, 14578, 14678, 23578, 23678, 2458, 2468, 34567, 347, 56\}$ |
| 82:10  | $0, 0, 0, 0, 0, 0, e^{24} + e^{13}, e^{26} + e^{15}$                   | $1/5(3, 3, 4, 4, 4, 4, 7, 7)$          | $\{\emptyset, 123456, 12348, 12567, 1278, 135, 1368, 1457, 14678, 23578, 2367, 2458, 246, 345678, 347, 568\}$ |
| 82:11a | $0, 0, 0, 0, 0, 0, e^{12} + e^{34}, e^{56} + e^{24} + e^{13}$          | $5/7(1, 1, 1, 1, 1, 1, 2, 2)$          | $\{\emptyset, 1234, 123456, 1258, 1268, 13567, 137, 14578, 14678, 23578, 23678, 24567, 247, 3458, 3468, 56\}$ |
| 82:11b | $0, 0, 0, 0, 0, 0, -e^{12} + e^{34}, e^{24} + e^{13} + e^{56}$         | $5/7(1, 1, 1, 1, 1, 1, 2, 2)$          | $\{\emptyset, 1234, 123456, 1258, 1268, 13567, 137, 14578, 14678, 23578, 23678, 24567, 247, 3458, 3468, 56\}$ |
| 82:12  | $0, 0, 0, 0, 0, 0, e^{12} + e^{34}, e^{46} + e^{13} + e^{25}$          | $1/11(8, 7, 8, 7, 9, 9, 15, 16)$       | $\{\emptyset, 123456, 1268, 137, 14578, 23678, 24567, 3458\}$                                                 |
| 82:13  | $0, 0, 0, 0, 0, 0, e^{13} + e^{25} + e^{46}, e^{12} + e^{34} + e^{56}$ | $5/7(1, 1, 1, 1, 1, 1, 2, 2)$          | $\{\emptyset, 123456, 14578, 23678\}$                                                                         |

End of Table A.1

## A.2 Nice nilpotent Lie algebras of dimension 9 with $M_\Delta$ surjective

Table A.2: Irreducible nice nilpotent Lie algebras of dimension 9 with  $M_\Delta$  surjective that admit a diagonal nilsoliton metric of type Nil4

| Name       | $\mathfrak{g}$                                                          | $N$                                                 | Signatures $\mathbf{S}$                 |
|------------|-------------------------------------------------------------------------|-----------------------------------------------------|-----------------------------------------|
| 97654321:1 | $0, 0, e^{12}, e^{13}, e^{14}, e^{15}, e^{16}, e^{17}, e^{18}$          | $1/86(2, 79, 81, 83, 85, 87, 89, 91, 93)$           | $\{\emptyset, 12468, 13579, 23456789\}$ |
| 97654321:2 | $0, 0, e^{12}, e^{13}, e^{14}, e^{15}, e^{16}, e^{17}, e^{23} + e^{18}$ | $77/765(1, 6, 7, 8, 9, 10, 11, 12, 13)$             | $\{134689, 45678\}$                     |
| 9764321:1  | $0, 0, e^{12}, e^{13}, e^{23}, e^{14}, e^{16}, e^{17}, e^{18}$          | $1/247(23, 154, 177, 200, 331, 223, 246, 269, 292)$ | $\{12568, 134579, 23, 46789\}$          |
| 9764321:2  | $0, 0, e^{12}, e^{13}, e^{23}, e^{14}, e^{16}, e^{17}, e^{25} + e^{18}$ | $91/1107(2, 5, 7, 9, 12, 11, 13, 15, 17)$           | $\{123479, 168\}$                       |
| 976421:1   | $0, 0, e^{12}, e^{13}, e^{23}, e^{14}, e^{25}, e^{16}, e^{18}$          | $1/351(61, 139, 200, 261, 339, 322, 478, 383, 444)$ | $\{123679, 148, 25, 3456789\}$          |
| 976421:4   | $0, 0, e^{12}, e^{13}, e^{23}, e^{14}, e^{25}, e^{16}, e^{27} + e^{18}$ | $49/653(3, 4, 7, 10, 11, 13, 15, 16, 19)$           | $\{148, 3456789\}$                      |
| 97642:8    | $0, 0, e^{12}, e^{13}, e^{23}, e^{14}, e^{25}, e^{16}, e^{27}$          | $14/53(1, 1, 2, 3, 3, 4, 4, 5, 5)$                  | $\{12367, 148, 259, 3456789\}$          |
| 9654321:2  | $0, 0, 0, e^{12}, e^{14}, e^{15}, e^{16}, e^{17}, e^{23} + e^{18}$      | $1/65(7, 44, 42, 51, 58, 65, 72, 79, 86)$           | $\{124689, 157, 29, 45678\}$            |

Table A.2 – Continued to next page

Table A.2 – Continued from previous page

| Name       | $g$                                                                          | $N$                                                | Signatures $S$                                                    |
|------------|------------------------------------------------------------------------------|----------------------------------------------------|-------------------------------------------------------------------|
| 965321:2   | $0, 0, 0, e^{12}, e^{14}, e^{24} + e^{13}, e^{15}, e^{17}, e^{18}$           | 1/509(68, 281, 562, 349, 417, 630, 485, 553, 621)  | {123568, 134679, 2345789, 3}                                      |
| 965321:3   | $0, 0, 0, e^{12}, e^{14}, e^{24}, e^{15}, e^{17}, e^{18} + e^{23}$           | 2/177(14, 47, 70, 61, 75, 108, 89, 103, 117)       | { $\emptyset$ , 123568, 134679, 245789}                           |
| 965321:5   | $0, 0, 0, e^{12}, e^{14}, e^{13} + e^{24}, e^{15}, e^{17}, e^{18} + e^{23}$  | 14/153(2, 5, 10, 7, 9, 12, 11, 13, 15)             | {123568, 134679}                                                  |
| 964321:1   | $0, 0, 0, e^{12}, e^{13}, e^{14}, e^{16}, e^{17}, e^{18}$                    | 1/38(2, 33, 37, 35, 39, 37, 39, 41, 43)            | { $\emptyset$ , 12368, 12568, 13479, 14579, 23456789, 246789, 35} |
| 964321:2   | $0, 0, 0, e^{12}, e^{13}, e^{24}, e^{26}, e^{27}, e^{28}$                    | 1/139(96, 14, 91, 110, 187, 124, 138, 152, 166)    | {123479, 124579, 13, 15, 23568, 268, 3456789, 46789}              |
| 964321:3   | $0, 0, 0, e^{12}, e^{13}, e^{14}, e^{16}, e^{17}, e^{35} + e^{18}$           | 7/569(8, 66, 49, 74, 57, 82, 90, 98, 106)          | {123689, 125689, 2345678, 24678}                                  |
| 964321:4   | $0, 0, 0, e^{12}, e^{13}, e^{24}, e^{26}, e^{27}, e^{35} + e^{28}$           | 1/99(64, 14, 35, 78, 99, 92, 106, 120, 134)        | { $\emptyset$ , 1346789, 1456789, 35}                             |
| 964321:5   | $0, 0, 0, e^{12}, e^{13}, e^{14}, e^{16}, e^{17}, e^{23} + e^{18}$           | 1/53(8, 33, 40, 41, 48, 49, 57, 65, 73)            | {123568, 134579, 2456789, 5}                                      |
| 964321:6   | $0, 0, 0, e^{12}, e^{13}, e^{24}, e^{26}, e^{27}, e^{28} + e^{15}$           | 1/107(45, 22, 65, 67, 110, 89, 111, 133, 155)      | {123479, 15, 268, 3456789}                                        |
| 964321:7   | $0, 0, 0, e^{12}, e^{13}, e^{14}, e^{16}, e^{17}, e^{24} + e^{18}$           | 1/109(16, 64, 101, 80, 117, 96, 112, 128, 144)     | { $\emptyset$ , 13479, 14579, 35}                                 |
| 964321:11a | $0, 0, 0, e^{12}, e^{13}, e^{14}, e^{16}, e^{17}, e^{18} + e^{35} + e^{24}$  | 49/313(1, 4, 4, 5, 5, 6, 7, 8, 9)                  | {123689, 125689, 2345678, 24678}                                  |
| 964321:11b | $0, 0, 0, -e^{12}, e^{13}, e^{14}, e^{16}, e^{17}, e^{18} + e^{35} + e^{24}$ | 49/313(1, 4, 4, 5, 5, 6, 7, 8, 9)                  | {123689, 125689, 2345678, 24678}                                  |
| 964321:13  | $0, 0, 0, e^{12}, e^{13}, e^{24}, e^{26}, e^{27}, e^{28} + e^{14} + e^{35}$  | 49/641(8, 2, 5, 10, 13, 12, 14, 16, 18)            | { $\emptyset$ , 35}                                               |
| 96531:2    | $0, 0, 0, e^{12}, e^{14}, e^{24}, e^{15}, e^{13} + e^{26}, e^{17}$           | 13/111(2, 3, 9, 5, 7, 8, 9, 11, 11)                | {12569, 134678, 245789, 3}                                        |
| 96531:3    | $0, 0, 0, e^{12}, e^{14}, e^{24}, e^{15}, e^{26}, e^{23} + e^{17}$           | 1/657(156, 235, 624, 391, 547, 626, 703, 861, 859) | { $\emptyset$ , 12569, 14678, 245789}                             |
| 96531:6    | $0, 0, 0, e^{12}, e^{14}, e^{24}, e^{15}, e^{26} + e^{13}, e^{23} + e^{17}$  | 91/1089(3, 4, 12, 7, 10, 11, 13, 15, 16)           | {12569, 245789}                                                   |
| 96421:1    | $0, 0, 0, e^{12}, e^{13}, e^{14}, e^{35}, e^{16}, e^{18}$                    | 1/69(6, 57, 43, 63, 49, 69, 92, 75, 81)            | { $\emptyset$ , 123679, 125679, 13478, 14578, 2345689, 24689, 35} |
| 96421:2    | $0, 0, 0, e^{12}, e^{13}, e^{24}, e^{35}, e^{26}, e^{28}$                    | 1/141(90, 21, 49, 111, 139, 132, 188, 153, 174)    | { $\emptyset$ , 123679, 125679, 1346789, 1456789, 23458, 248, 35} |
| 96421:3    | $0, 0, 0, e^{12}, e^{13}, e^{14}, e^{15}, e^{16}, e^{18}$                    | 1/13(1, 11, 12, 12, 13, 13, 14, 14, 15)            | { $\emptyset$ , 123679, 12569, 13478, 1458, 23456789, 24689, 357} |
| 96421:4    | $0, 0, 0, e^{12}, e^{13}, e^{24}, e^{15}, e^{26}, e^{28}$                    | 1/13(5, 3, 8, 8, 13, 11, 18, 14, 17)               | {123478, 12458, 137, 15, 235679, 269, 3456789, 4689}              |
| 96421:5    | $0, 0, 0, e^{12}, e^{13}, e^{14}, e^{24}, e^{16}, e^{18}$                    | 1/297(48, 167, 273, 215, 321, 263, 382, 311, 359)  | { $\emptyset$ , 123679, 125679, 13478, 14578, 2345689, 24689, 35} |
| 96421:6    | $0, 0, 0, e^{12}, e^{13}, e^{24}, e^{14}, e^{26}, e^{28}$                    | 1/16(8, 3, 12, 11, 20, 14, 19, 17, 20)             | { $\emptyset$ , 123679, 125679, 134689, 145689, 234578, 2478, 35} |
| 96421:7    | $0, 0, 0, e^{12}, e^{13}, e^{14}, e^{23} + e^{15}, e^{16}, e^{18}$           | 1/31(7, 14, 24, 21, 31, 28, 38, 35, 42)            | {134578, 148, 37, 5}                                              |
| 96421:8    | $0, 0, 0, e^{12}, e^{13}, e^{24}, e^{15} + e^{23}, e^{26}, e^{28}$           | 1/19(3, 6, 16, 9, 19, 15, 22, 21, 27)              | {123478, 12458, 235679, 269}                                      |
| 96421:10a  | $0, 0, 0, e^{12}, e^{13}, e^{14}, e^{24} + e^{35}, e^{16}, e^{18}$           | 1/97(13, 64, 64, 77, 77, 90, 141, 103, 116)        | { $\emptyset$ , 123679, 125679, 13478, 14578, 2345689, 24689, 35} |
| 96421:10b  | $0, 0, 0, -e^{12}, e^{13}, e^{14}, e^{35} + e^{24}, e^{16}, e^{18}$          | 1/97(13, 64, 64, 77, 77, 90, 141, 103, 116)        | { $\emptyset$ , 123679, 125679, 13478, 14578, 2345689, 24689, 35} |
| 96421:12   | $0, 0, 0, e^{12}, e^{13}, e^{24}, e^{14} + e^{35}, e^{26}, e^{28}$           | 2/63(19, 5, 12, 24, 31, 29, 43, 34, 39)            | { $\emptyset$ , 123679, 125679, 35}                               |
| 96421:14   | $0, 0, 0, e^{12}, e^{13}, e^{14}, e^{15}, e^{16}, e^{35} + e^{18}$           | 1/217(34, 164, 133, 198, 167, 232, 201, 266, 300)  | {12369, 125679, 35, 7}                                            |
| 96421:16   | $0, 0, 0, e^{12}, e^{13}, e^{24}, e^{35}, e^{26}, e^{15} + e^{28}$           | 1/59(29, 13, 23, 42, 52, 55, 75, 68, 81)           | {124578, 157, 23569, 345689}                                      |
| 96421:17   | $0, 0, 0, e^{12}, e^{13}, e^{24}, e^{23} + e^{14}, e^{26}, e^{28}$           | 3/14(2, 1, 4, 3, 6, 4, 5, 6)                       | {123679, 134689, 234578, 35}                                      |
| 96421:19   | $0, 0, 0, e^{12}, e^{13}, e^{14}, e^{15} + e^{24}, e^{16}, e^{18}$           | 11/461(7, 23, 39, 30, 46, 37, 53, 44, 51)          | {125679, 14578, 2345689, 35}                                      |
| 96421:20   | $0, 0, 0, e^{12}, e^{13}, e^{14}, e^{15} + e^{23}, e^{16}, e^{18} + e^{35}$  | 21/173(2, 4, 5, 6, 7, 8, 9, 10, 12)                | {134578, 148}                                                     |
| 96421:22   | $0, 0, 0, e^{12}, e^{13}, e^{14}, e^{24}, e^{16}, e^{35} + e^{18}$           | 8/151(4, 10, 11, 14, 15, 18, 24, 22, 26)           | { $\emptyset$ , 123679, 125679, 35}                               |
| 96421:23a  | $0, 0, 0, e^{12}, e^{13}, e^{24}, e^{14}, e^{26}, e^{35} + e^{28}$           | 4/17(2, 1, 2, 3, 4, 4, 5, 6)                       | { $\emptyset$ , 123679, 125679, 134689, 145689, 234578, 2478, 35} |
| 96421:23b  | $0, 0, 0, -e^{12}, e^{13}, e^{24}, e^{14}, e^{26}, e^{35} + e^{28}$          | 4/17(2, 1, 2, 3, 4, 4, 5, 6)                       | { $\emptyset$ , 123679, 125679, 134689, 145689, 234578, 2478, 35} |
| 96421:24   | $0, 0, 0, e^{12}, e^{13}, e^{14}, e^{35}, e^{16}, e^{18} + e^{24}$           | 4/21(1, 3, 3, 4, 4, 5, 7, 6, 7)                    | { $\emptyset$ , 123679, 125679, 35}                               |
| 96421:25   | $0, 0, 0, e^{12}, e^{13}, e^{24}, e^{35}, e^{26}, e^{28} + e^{14}$           | 4/843(117, 39, 82, 156, 199, 195, 281, 234, 273)   | { $\emptyset$ , 123679, 125679, 35}                               |
| 96421:32   | $0, 0, 0, e^{12}, e^{13}, e^{14}, e^{24}, e^{16}, e^{18} + e^{23}$           | 7/513(15, 37, 60, 52, 77, 65, 116, 78, 92, 97)     | { $\emptyset$ , 125679, 14578, 24689}                             |
| 96421:33a  | $0, 0, 0, e^{12}, e^{13}, e^{14}, e^{24} + e^{35}, e^{16}, e^{18} + e^{23}$  | 49/313(1, 4, 4, 5, 5, 6, 9, 7, 8)                  | { $\emptyset$ , 125679, 14578, 24689}                             |
| 96421:33b  | $0, 0, 0, -e^{12}, e^{13}, e^{14}, e^{24} + e^{35}, e^{16}, e^{23} + e^{18}$ | 49/313(1, 4, 4, 5, 5, 6, 9, 7, 8)                  | { $\emptyset$ , 125679, 14578, 24689}                             |
| 96421:35   | $0, 0, 0, e^{12}, e^{13}, e^{24}, e^{14}, e^{26}, e^{15} + e^{28}$           | 1/72(28, 19, 48, 47, 76, 66, 75, 85, 104)          | {12458, 157, 23569, 3456789}                                      |
| 96421:36   | $0, 0, 0, e^{12}, e^{13}, e^{14}, e^{15}, e^{16}, e^{24} + e^{18}$           | 1/69(13, 39, 56, 52, 69, 65, 82, 78, 91)           | { $\emptyset$ , 123679, 12569, 357}                               |
| 96421:37   | $0, 0, 0, e^{12}, e^{13}, e^{24}, e^{15}, e^{26}, e^{28} + e^{14}$           | 1/77(39, 13, 38, 52, 77, 65, 116, 78, 91)          | {137, 15, 235679, 269}                                            |
| 96421:38a  | $0, 0, 0, e^{12}, e^{13}, e^{24}, e^{14} + e^{23}, e^{26}, e^{28} + e^{35}$  | 4/13(1, 1, 2, 2, 3, 3, 3, 4, 5)                    | {123679, 134689, 234578, 35}                                      |
| 96421:38b  | $0, 0, 0, -e^{12}, e^{13}, e^{24}, e^{14} + e^{23}, e^{26}, e^{28} + e^{35}$ | 4/13(1, 1, 2, 2, 3, 3, 3, 4, 5)                    | {123679, 134689, 234578, 35}                                      |
| 96421:39   | $0, 0, 0, e^{12}, e^{13}, e^{14}, e^{15} + e^{24}, e^{16}, e^{18} + e^{35}$  | 44/511(3, 5, 7, 8, 10, 11, 13, 14, 17)             | {125679, 35}                                                      |
| 96421:40   | $0, 0, 0, e^{12}, e^{13}, e^{24}, e^{35} + e^{14}, e^{26}, e^{28} + e^{15}$  | 51/701(7, 3, 5, 10, 12, 13, 17, 16, 19)            | {124578, 345689}                                                  |

Table A.2 – Continued to next page

Table A.2 – Continued from previous page

| Name      | $g$                                                                          | $N$                                                  | Signatures $S$                                                    |
|-----------|------------------------------------------------------------------------------|------------------------------------------------------|-------------------------------------------------------------------|
| 96421:48  | $0, 0, 0, e^{12}, e^{13}, e^{14}, e^{24}, e^{16}, e^{27} + e^{18}$           | $1/71(18, 27, 62, 45, 80, 63, 72, 81, 99)$           | $\{\emptyset, 2345689, 24689, 35\}$                               |
| 96421:49  | $0, 0, 0, e^{12}, e^{13}, e^{24}, e^{14}, e^{26}, e^{17} + e^{28}$           | $2/143(27, 18, 58, 45, 85, 63, 72, 81, 99)$          | $\{\emptyset, 134689, 145689, 35\}$                               |
| 96421:50  | $0, 0, 0, e^{12}, e^{13}, e^{14}, e^{24} + e^{15}, e^{16}, e^{18} + e^{23}$  | $77/757(2, 5, 8, 7, 10, 9, 12, 11, 13)$              | $\{\emptyset, 24689\}$                                            |
| 96421:51  | $0, 0, 0, e^{12}, e^{13}, e^{24}, e^{23} + e^{14}, e^{26}, e^{15} + e^{28}$  | $21/232(4, 3, 8, 7, 12, 10, 11, 13, 16)$             | $\{12458, 157\}$                                                  |
| 96421:52  | $0, 0, 0, e^{12}, e^{13}, e^{14}, e^{23} + e^{15}, e^{16}, e^{18} + e^{24}$  | $(0, 0, 1, 0, 1, 0, 1, 0, 0)$                        | $\{135679, 169\}$                                                 |
| 96421:53  | $0, 0, 0, e^{12}, e^{13}, e^{24}, e^{15} + e^{23}, e^{26}, e^{28} + e^{14}$  | $(0, 0, 1, 0, 1, 0, 1, 0, 0)$                        | $\{235679, 269\}$                                                 |
| 96421:56a | $0, 0, 0, e^{12}, e^{13}, e^{14}, e^{15}, e^{16}, e^{18} + e^{35} + e^{24}$  | $19/93(1, 3, 3, 4, 4, 5, 5, 6, 7)$                   | $\{134789, 14589, 2345678, 2468\}$                                |
| 96421:56b | $0, 0, 0, -e^{12}, e^{13}, e^{14}, e^{15}, e^{16}, e^{35} + e^{18} + e^{24}$ | $19/93(1, 3, 3, 4, 4, 5, 5, 6, 7)$                   | $\{134789, 14589, 2345678, 2468\}$                                |
| 96421:88  | $0, 0, 0, e^{12}, e^{13}, e^{14}, e^{24}, e^{16}, e^{18} + e^{27} + e^{35}$  | $56/831(4, 6, 9, 10, 13, 14, 16, 18, 22)$            | $\{\emptyset, 35\}$                                               |
| 96421:89a | $0, 0, 0, e^{12}, e^{13}, e^{24}, e^{14}, e^{26}, e^{35} + e^{28} + e^{17}$  | $28/209(3, 2, 4, 5, 7, 7, 8, 9, 11)$                 | $\{\emptyset, 134689, 145689, 35\}$                               |
| 96421:89b | $0, 0, 0, -e^{12}, e^{13}, e^{24}, e^{14}, e^{26}, e^{17} + e^{35} + e^{28}$ | $28/209(3, 2, 4, 5, 7, 7, 8, 9, 11)$                 | $\{\emptyset, 134689, 145689, 35\}$                               |
| 96421:111 | $0, 0, 0, e^{12}, e^{13}, e^{14}, e^{35}, e^{16}, e^{37} + e^{18}$           | $1/129(21, 96, 53, 117, 74, 138, 127, 159, 180)$     | $\{123569, 148, 2456789, 37\}$                                    |
| 96421:112 | $0, 0, 0, e^{12}, e^{13}, e^{24}, e^{35}, e^{26}, e^{28} + e^{37}$           | $1/123(81, 21, 28, 102, 109, 123, 137, 144, 165)$    | $\{\emptyset, 125679, 1456789, 248\}$                             |
| 96421:161 | $0, 0, 0, e^{12}, e^{13}, e^{24}, e^{15}, e^{26}, e^{28} + e^{17}$           | $1/131(34, 39, 88, 73, 122, 112, 156, 151, 190)$     | $\{123478, 137, 235679, 3456789\}$                                |
| 96421:162 | $0, 0, 0, e^{12}, e^{13}, e^{24}, e^{35}, e^{26}, e^{28} + e^{37} + e^{15}$  | $21/299(8, 3, 4, 11, 12, 14, 16, 17, 20)$            | $\{\emptyset, 248\}$                                              |
| 96421:173 | $0, 0, 0, e^{12}, e^{13}, e^{14}, e^{35}, e^{16}, e^{18} + e^{24} + e^{37}$  | $6/29(1, 3, 2, 4, 3, 5, 5, 6, 7)$                    | $\{123569, 37\}$                                                  |
| 96421:174 | $0, 0, 0, e^{12}, e^{13}, e^{24}, e^{35}, e^{26}, e^{14} + e^{28} + e^{37}$  | $56/849(9, 3, 4, 12, 13, 15, 17, 18, 21)$            | $\{\emptyset, 125679\}$                                           |
| 9642:1    | $0, 0, 0, e^{12}, e^{13}, e^{14}, e^{24}, e^{16}, e^{27}$                    | $1/353(108, 117, 299, 225, 407, 333, 342, 441, 459)$ | $\{\emptyset, 12367, 12567, 134789, 145789, 2345689, 24689, 35\}$ |
| 9642:2    | $0, 0, 0, e^{12}, e^{13}, e^{24}, e^{14}, e^{26}, e^{23} + e^{17}$           | $1/593(173, 202, 519, 375, 692, 577, 548, 779, 721)$ | $\{12567, 145689, 2345789, 35\}$                                  |
| 9642:5    | $0, 0, 0, e^{12}, e^{13}, e^{14}, e^{24}, e^{16}, e^{27} + e^{35}$           | $2/71(10, 14, 21, 24, 31, 34, 38, 44, 52)$           | $\{\emptyset, 134789, 145789, 35\}$                               |
| 9642:6    | $0, 0, 0, e^{12}, e^{13}, e^{24}, e^{14}, e^{26}, e^{17} + e^{35}$           | $4/183(17, 14, 24, 31, 41, 45, 48, 59, 65)$          | $\{\emptyset, 134689, 145689, 35\}$                               |
| 9642:7    | $0, 0, 0, e^{12}, e^{13}, e^{14}, e^{24}, e^{16}, e^{15} + e^{27}$           | $1/283(80, 103, 229, 183, 309, 263, 286, 343, 389)$  | $\{\emptyset, 12567, 134789, 2345689\}$                           |
| 9642:10   | $0, 0, 0, e^{12}, e^{13}, e^{14}, e^{24}, e^{16} + e^{23}, e^{27} + e^{35}$  | $17/77(1, 2, 3, 3, 4, 4, 5, 5, 7)$                   | $\{145789, 35\}$                                                  |
| 9642:13   | $0, 0, 0, e^{12}, e^{13}, e^{24}, e^{14}, e^{15} + e^{26}, e^{17} + e^{35}$  | $10/133(5, 4, 7, 9, 12, 13, 14, 17, 19)$             | $\{145689, 35\}$                                                  |
| 9642:15   | $0, 0, 0, e^{12}, e^{13}, e^{14}, e^{24}, e^{23} + e^{16}, e^{27} + e^{15}$  | $42/457(3, 4, 9, 7, 12, 10, 11, 13, 15)$             | $\{12567, 2345689\}$                                              |
| 9642:49   | $0, 0, 0, e^{12}, e^{13}, e^{14}, e^{15}, e^{16}, e^{17}$                    | $1/22(2, 19, 19, 21, 21, 23, 23, 25, 25)$            | $\{\emptyset, 12367, 12569, 13478, 14589, 23456789, 2468, 3579\}$ |
| 9642:50   | $0, 0, 0, e^{12}, e^{13}, e^{24}, e^{15}, e^{26}, e^{17}$                    | $1/33(6, 13, 24, 19, 30, 32, 36, 45, 42)$            | $\{123478, 124589, 137, 159, 235679, 26, 3456789, 468\}$          |
| 9642:51   | $0, 0, 0, e^{12}, e^{13}, e^{24}, e^{35}, e^{26}, e^{37}$                    | $7/33(3, 1, 1, 4, 4, 5, 5, 6, 6)$                    | $\{\emptyset, 12367, 125679, 134678, 1456789, 234589, 248, 359\}$ |
| 9642:52   | $0, 0, 0, e^{12}, e^{13}, e^{14}, e^{15}, e^{16}, e^{17} + e^{23}$           | $1/184(38, 114, 127, 152, 165, 190, 203, 228, 241)$  | $\{\emptyset, 12367, 12569, 3579\}$                               |
| 9642:53   | $0, 0, 0, e^{12}, e^{13}, e^{24}, e^{15}, e^{26}, e^{17} + e^{23}$           | $1/72(10, 30, 57, 40, 67, 70, 77, 100, 87)$          | $\{137, 159, 235679, 26\}$                                        |
| 9642:54   | $0, 0, 0, e^{12}, e^{13}, e^{14}, e^{15}, e^{16}, e^{17} + e^{24}$           | $1/208(38, 121, 166, 159, 204, 197, 242, 235, 280)$  | $\{\emptyset, 12569, 14589, 2468\}$                               |
| 9642:55   | $0, 0, 0, e^{12}, e^{13}, e^{14}, e^{35}, e^{16}, e^{37} + e^{24}$           | $1/69(15, 42, 28, 57, 43, 72, 71, 87, 99)$           | $\{123569, 134589, 234678, 37\}$                                  |
| 9642:56   | $0, 0, 0, e^{12}, e^{13}, e^{24}, e^{35}, e^{26}, e^{37} + e^{14}$           | $28/1059(21, 9, 10, 30, 31, 39, 41, 48, 51)$         | $\{\emptyset, 125679, 134678, 234589\}$                           |
| 9642:58   | $0, 0, 0, e^{12}, e^{13}, e^{24}, e^{15}, e^{26} + e^{14}, e^{17}$           | $1/5(2, 1, 2, 3, 4, 4, 6, 5, 8)$                     | $\{123478, 124589, 137, 159\}$                                    |
| 9642:59   | $0, 0, 0, e^{12}, e^{13}, e^{14}, e^{35}, e^{16} + e^{24}, e^{37}$           | $1/417(114, 228, 149, 342, 263, 456, 412, 570, 561)$ | $\{134589, 148, 37, 579\}$                                        |
| 9642:60   | $0, 0, 0, e^{12}, e^{13}, e^{24}, e^{35}, e^{14} + e^{26}, e^{37}$           | $1/123(66, 33, 31, 99, 97, 132, 128, 165, 159)$      | $\{\emptyset, 234589, 248, 359\}$                                 |
| 9642:69   | $0, 0, 0, e^{12}, e^{13}, e^{14}, e^{15}, e^{16} + e^{23}, e^{17} + e^{24}$  | $35/312(2, 5, 6, 7, 8, 9, 10, 11, 12)$               | $\{\emptyset, 2468\}$                                             |
| 9642:70   | $0, 0, 0, e^{12}, e^{13}, e^{14}, e^{35}, e^{16} + e^{23}, e^{24} + e^{37}$  | $49/648(2, 9, 6, 11, 8, 13, 14, 15, 20)$             | $\{234678, 37\}$                                                  |
| 9642:71   | $0, 0, 0, e^{12}, e^{13}, e^{14}, e^{15}, e^{16} + e^{24}, e^{17} + e^{23}$  | $(0, 0, 1, 0, 1, 0, 1, 0, 1)$                        | $\{137, 159\}$                                                    |
| 9642:72   | $0, 0, 0, e^{12}, e^{13}, e^{24}, e^{15}, e^{14} + e^{26}, e^{17} + e^{23}$  | $(0, 0, 1, 0, 1, 0, 1, 0, 1)$                        | $\{137, 159\}$                                                    |
| 9642:73a  | $0, 0, 0, e^{12}, e^{13}, e^{14}, e^{15}, e^{16}, e^{35} + e^{24} + e^{17}$  | $29/109(1, 2, 2, 3, 3, 4, 4, 5, 5)$                  | $\{125679, 145789, 24678, 7\}$                                    |
| 9642:73b  | $0, 0, 0, -e^{12}, e^{13}, e^{14}, e^{15}, e^{16}, e^{35} + e^{24} + e^{17}$ | $29/109(1, 2, 2, 3, 3, 4, 4, 5, 5)$                  | $\{125679, 145789, 24678, 7\}$                                    |
| 9642:76   | $0, 0, 0, e^{12}, e^{13}, e^{14}, e^{35}, e^{16}, e^{15} + e^{24} + e^{37}$  | $11/104(4, 3, 2, 7, 6, 11, 8, 15, 10)$               | $\{123569, 134589\}$                                              |
| 9642:77   | $0, 0, 0, e^{12}, e^{13}, e^{14}, e^{15}, e^{16} + e^{24}, e^{17} + e^{35}$  | $29/109(1, 2, 2, 3, 3, 4, 4, 5, 5)$                  | $\{\emptyset, 14589\}$                                            |
| 9642:78   | $0, 0, 0, e^{12}, e^{13}, e^{24}, e^{15}, e^{26} + e^{14}, e^{17} + e^{35}$  | $43/271(2, 1, 4, 3, 6, 4, 8, 5, 10)$                 | $\{123478, 137\}$                                                 |
| 9642:79a  | $0, 0, 0, e^{12}, e^{13}, e^{24}, e^{35}, e^{14} + e^{26}, e^{15} + e^{37}$  | $14/53(2, 1, 1, 3, 3, 4, 4, 5, 5)$                   | $\{\emptyset, 234589, 248, 359\}$                                 |
| 9642:79b  | $0, 0, 0, e^{12}, e^{13}, e^{24}, e^{35}, -e^{14} + e^{26}, e^{15} + e^{37}$ | $14/53(2, 1, 1, 3, 3, 4, 4, 5, 5)$                   | $\{\emptyset, 234589, 248, 359\}$                                 |

Table A.2 – Continued to next page

Table A.2 – Continued from previous page

| Name      | $g$                                                                          | $N$                                                  | Signatures $S$                                                    |
|-----------|------------------------------------------------------------------------------|------------------------------------------------------|-------------------------------------------------------------------|
| 9642:80   | $0, 0, 0, e^{12}, e^{13}, e^{14}, e^{15}, e^{35} + e^{16}, e^{24} + e^{17}$  | $29/109(1, 2, 2, 3, 3, 4, 4, 5, 5)$                  | $\{\emptyset, 14589\}$                                            |
| 9642:81a  | $0, 0, 0, e^{12}, e^{13}, e^{24}, e^{35}, e^{26} + e^{15}, e^{37} + e^{14}$  | $14/53(2, 1, 1, 3, 3, 4, 4, 5, 5)$                   | $\{\emptyset, 125679, 134678, 234589\}$                           |
| 9642:81b  | $0, 0, 0, e^{12}, e^{13}, e^{24}, e^{35}, e^{26} - e^{15}, e^{37} + e^{14}$  | $14/53(2, 1, 1, 3, 3, 4, 4, 5, 5)$                   | $\{\emptyset, 125679, 134678, 234589\}$                           |
| 96321:1   | $0, 0, 0, e^{12}, e^{13}, e^{23}, e^{14}, e^{17}, e^{18}$                    | $1/43(7, 26, 32, 33, 39, 58, 40, 47, 54)$            | $\{123579, 12679, 134568, 148, 234789, 2456789, 36, 5\}$          |
| 96321:2   | $0, 0, 0, e^{12}, e^{13}, e^{23}, e^{14}, e^{17}, e^{35} + e^{18}$           | $3/241(14, 52, 47, 66, 61, 99, 80, 94, 108)$         | $\{134568, 148, 234789, 2456789\}$                                |
| 96321:3a  | $0, 0, 0, e^{12}, e^{13}, e^{23}, e^{24}, e^{27}, e^{35} + e^{28}$           | $1/4(2, 1, 2, 3, 4, 3, 4, 5, 6)$                     | $\{123679, 12579, 134789, 1456789, 234568, 248, 35, 6\}$          |
| 96321:3b  | $0, 0, 0, -e^{12}, e^{13}, e^{23}, e^{24}, e^{27}, e^{28} + e^{35}$          | $1/4(2, 1, 2, 3, 4, 3, 4, 5, 6)$                     | $\{123679, 12579, 134789, 1456789, 234568, 248, 35, 6\}$          |
| 96321:4   | $0, 0, 0, e^{12}, e^{13}, e^{23}, e^{24}, e^{27}, e^{15} + e^{28}$           | $1/41(16, 11, 28, 27, 44, 39, 38, 49, 60)$           | $\{12458, 156, 235679, 345789\}$                                  |
| 96321:5   | $0, 0, 0, e^{12}, e^{13}, e^{23}, e^{14}, e^{17}, e^{18} + e^{24}$           | $3/211(13, 39, 53, 52, 66, 92, 65, 78, 91)$          | $\{123579, 12679, 36, 5\}$                                        |
| 96321:7   | $0, 0, 0, e^{12}, e^{13}, e^{23}, e^{14}, e^{17}, e^{18} + e^{26} + e^{35}$  | $87/997(3, 5, 7, 8, 10, 12, 11, 14, 17)$             | $\{12468, 346789\}$                                               |
| 96321:8a  | $0, 0, 0, e^{12}, e^{13}, e^{23}, e^{14}, e^{17}, e^{18} + e^{35} + e^{24}$  | $39/197(1, 3, 3, 4, 4, 6, 5, 6, 7)$                  | $\{\emptyset, 12379, 125679, 356\}$                               |
| 96321:8b  | $0, 0, 0, -e^{12}, e^{13}, e^{23}, e^{14}, e^{17}, e^{35} + e^{18} + e^{24}$ | $39/197(1, 3, 3, 4, 4, 6, 5, 6, 7)$                  | $\{\emptyset, 12379, 125679, 356\}$                               |
| 96321:10a | $0, 0, 0, e^{12}, e^{13}, e^{23}, e^{24}, e^{27}, e^{35} + e^{28} + e^{14}$  | $6/29(3, 1, 2, 4, 5, 3, 5, 6, 7)$                    | $\{134789, 1456789, 234568, 248\}$                                |
| 96321:10b | $0, 0, 0, -e^{12}, e^{13}, e^{23}, e^{24}, e^{27}, e^{14} + e^{35} + e^{28}$ | $6/29(3, 1, 2, 4, 5, 3, 5, 6, 7)$                    | $\{134789, 1456789, 234568, 248\}$                                |
| 9641:1    | $0, 0, 0, e^{12}, e^{13}, e^{14}, e^{15}, e^{35}, e^{16}$                    | $1/59(10, 44, 35, 54, 45, 64, 55, 80, 74)$           | $\{12368, 125678, 13489, 145789, 234569, 24679, 35, 7\}$          |
| 9641:2    | $0, 0, 0, e^{12}, e^{13}, e^{24}, e^{15}, e^{35}, e^{26}$                    | $1/141(57, 43, 60, 100, 117, 143, 174, 177, 186)$    | $\{\emptyset, 123678, 12568, 1346789, 145689, 234579, 249, 357\}$ |
| 9641:3    | $0, 0, 0, e^{12}, e^{13}, e^{14}, e^{24}, e^{35}, e^{16}$                    | $1/204(48, 105, 112, 153, 160, 201, 258, 272, 249)$  | $\{\emptyset, 123678, 125678, 134789, 145789, 234569, 2469, 35\}$ |
| 9641:4    | $0, 0, 0, e^{12}, e^{13}, e^{24}, e^{14}, e^{35}, e^{26}$                    | $1/18(8, 5, 8, 13, 16, 18, 21, 24, 23)$              | $\{\emptyset, 123678, 125678, 134689, 145689, 234579, 2479, 35\}$ |
| 9641:5    | $0, 0, 0, e^{12}, e^{13}, e^{14}, e^{35}, e^{15} + e^{23}, e^{16}$           | $1/67(18, 36, 35, 54, 53, 72, 88, 71, 90)$           | $\{134589, 149, 378, 57\}$                                        |
| 9641:6    | $0, 0, 0, e^{12}, e^{13}, e^{24}, e^{35}, e^{15} + e^{23}, e^{26}$           | $1/211(43, 86, 120, 129, 163, 215, 283, 206, 301)$   | $\{123678, 12567, 234589, 249\}$                                  |
| 9641:9    | $0, 0, 0, e^{12}, e^{13}, e^{14}, e^{24}, e^{15}, e^{16}$                    | $1/20(4, 11, 16, 15, 20, 19, 26, 24, 23)$            | $\{\emptyset, 123678, 12567, 134789, 14579, 2345689, 2469, 358\}$ |
| 9641:11   | $0, 0, 0, e^{12}, e^{13}, e^{14}, e^{15}, e^{35}, e^{23} + e^{16}$           | $1/21(4, 15, 12, 19, 16, 23, 20, 28, 27)$            | $\{12368, 13489, 24679, 7\}$                                      |
| 9641:12   | $0, 0, 0, e^{12}, e^{13}, e^{24}, e^{23} + e^{14}, e^{35}, e^{26}$           | $1/14(4, 5, 8, 9, 12, 14, 13, 20, 19)$               | $\{123678, 134689, 234579, 35\}$                                  |
| 9641:13a  | $0, 0, 0, e^{12}, e^{13}, e^{14}, e^{15}, e^{24} + e^{35}, e^{16}$           | $1/55(11, 34, 34, 45, 45, 56, 56, 79, 67)$           | $\{\emptyset, 123678, 12568, 134789, 14589, 2345679, 2469, 357\}$ |
| 9641:13b  | $0, 0, 0, -e^{12}, e^{13}, e^{14}, e^{15}, e^{35} + e^{24}, e^{16}$          | $1/55(11, 34, 34, 45, 45, 56, 56, 79, 67)$           | $\{\emptyset, 123678, 12568, 134789, 14589, 2345679, 2469, 357\}$ |
| 9641:15   | $0, 0, 0, e^{12}, e^{13}, e^{24}, e^{15}, e^{14} + e^{35}, e^{26}$           | $1/351(157, 103, 130, 260, 287, 363, 444, 417, 466)$ | $\{1346789, 145689, 234579, 249\}$                                |
| 9641:17   | $0, 0, 0, e^{12}, e^{13}, e^{14}, e^{35}, e^{15} + e^{24}, e^{16}$           | $1/143(41, 60, 79, 101, 120, 142, 199, 161, 183)$    | $\{125678, 145789, 234569, 35\}$                                  |
| 9641:18   | $0, 0, 0, e^{12}, e^{13}, e^{14}, e^{24}, e^{15} + e^{23}, e^{16}$           | $1/41(10, 20, 31, 30, 41, 40, 50, 51, 50)$           | $\{\emptyset, 134789, 14579, 358\}$                               |
| 9641:19   | $0, 0, 0, e^{12}, e^{13}, e^{24}, e^{14}, e^{23} + e^{15}, e^{26}$           | $1/53(11, 22, 42, 33, 53, 55, 44, 64, 77)$           | $\{1234789, 124579, 235678, 267\}$                                |
| 9641:20   | $0, 0, 0, e^{12}, e^{13}, e^{14}, e^{24}, e^{35}, e^{23} + e^{16}$           | $1/164(32, 91, 96, 123, 128, 155, 214, 224, 187)$    | $\{125678, 145789, 234569, 35\}$                                  |
| 9641:24   | $0, 0, 0, e^{12}, e^{13}, e^{14}, e^{24}, e^{15}, e^{16} + e^{35}$           | $1/283(80, 142, 151, 222, 231, 302, 364, 311, 382)$  | $\{\emptyset, 134789, 14579, 358\}$                               |
| 9641:25   | $0, 0, 0, e^{12}, e^{13}, e^{24}, e^{14}, e^{15}, e^{26} + e^{35}$           | $1/279(97, 100, 150, 197, 247, 297, 294, 344, 397)$  | $\{\emptyset, 134689, 14569, 358\}$                               |
| 9641:26   | $0, 0, 0, e^{12}, e^{13}, e^{24}, e^{14}, e^{35}, e^{15} + e^{26}$           | $4/233(25, 17, 26, 42, 51, 59, 67, 77, 76)$          | $\{\emptyset, 125678, 134689, 234579\}$                           |
| 9641:27   | $0, 0, 0, e^{12}, e^{13}, e^{14}, e^{15}, e^{35}, e^{16} + e^{24}$           | $1/67(18, 36, 35, 54, 53, 72, 71, 88, 90)$           | $\{\emptyset, 134789, 14589, 357\}$                               |
| 9641:28   | $0, 0, 0, e^{12}, e^{13}, e^{24}, e^{15}, e^{35}, e^{26} + e^{14}$           | $1/151(74, 37, 55, 111, 129, 148, 203, 184, 185)$    | $\{1234789, 124589, 1378, 158\}$                                  |
| 9641:31   | $0, 0, 0, e^{12}, e^{13}, e^{24}, e^{15} + e^{23}, e^{14} + e^{35}, e^{26}$  | $59/499(2, 4, 3, 6, 5, 10, 7, 8, 14)$                | $\{1234789, 124589\}$                                             |
| 9641:41   | $0, 0, 0, e^{12}, e^{13}, e^{14}, e^{24}, e^{15}, e^{23} + e^{16}$           | $1/116(28, 59, 84, 87, 112, 115, 146, 140, 143)$     | $\{\emptyset, 123678, 134789, 2469\}$                             |
| 9641:42a  | $0, 0, 0, e^{12}, e^{13}, e^{14}, e^{15}, e^{35} + e^{24}, e^{16} + e^{23}$  | $19/93(1, 3, 3, 4, 4, 5, 5, 7, 6)$                   | $\{\emptyset, 123678, 134789, 2469\}$                             |
| 9641:42b  | $0, 0, 0, -e^{12}, e^{13}, e^{14}, e^{15}, e^{35} + e^{24}, e^{16} + e^{23}$ | $19/93(1, 3, 3, 4, 4, 5, 5, 7, 6)$                   | $\{\emptyset, 123678, 134789, 2469\}$                             |
| 9641:44a  | $0, 0, 0, e^{12}, e^{13}, e^{14}, e^{35}, e^{15} + e^{24}, e^{23} + e^{16}$  | $17/77(1, 2, 3, 3, 4, 4, 7, 5, 5)$                   | $\{125678, 145789, 234569, 35\}$                                  |
| 9641:44b  | $0, 0, 0, e^{12}, -e^{13}, e^{14}, e^{35}, e^{15} + e^{24}, e^{16} + e^{23}$ | $17/77(1, 2, 3, 3, 4, 4, 7, 5, 5)$                   | $\{125678, 145789, 234569, 35\}$                                  |
| 9641:48   | $0, 0, 0, e^{12}, e^{13}, e^{24}, e^{14} + e^{23}, e^{15}, e^{26} + e^{35}$  | $7/71(3, 4, 6, 7, 9, 11, 10, 12, 15)$                | $\{134689, 358\}$                                                 |
| 9641:49   | $0, 0, 0, e^{12}, e^{13}, e^{24}, e^{14} + e^{23}, e^{35}, e^{15} + e^{26}$  | $4/13(1, 1, 2, 2, 3, 3, 3, 5, 4)$                    | $\{123678, 35\}$                                                  |
| 9641:51   | $0, 0, 0, e^{12}, e^{13}, e^{24}, e^{35}, e^{15} + e^{23}, e^{14} + e^{26}$  | $1/7(0, 0, 5, 0, 5, 0, 10, 5, 0)$                    | $\{1234789, 124579\}$                                             |
| 9641:96a  | $0, 0, 0, e^{12}, e^{13}, e^{14}, e^{24}, e^{35}, e^{16} + e^{27}$           | $4/81(7, 7, 10, 14, 17, 21, 21, 27, 28)$             | $\{\emptyset, 123678, 125678, 134789, 145789, 234569, 2469, 35\}$ |
| 9641:96b  | $0, 0, 0, e^{12}, e^{13}, -e^{14}, e^{24}, e^{35}, e^{27} + e^{16}$          | $4/81(7, 7, 10, 14, 17, 21, 21, 27, 28)$             | $\{\emptyset, 123678, 125678, 134789, 145789, 234569, 2469, 35\}$ |
| 9641:101a | $0, 0, 0, e^{12}, e^{13}, e^{14}, e^{24}, e^{23} + e^{15}, e^{16} + e^{27}$  | $(0, 0, 1, 0, 1, 0, 0, 1, 0)$                        | $\{1234689, 124569, 235678, 267\}$                                |

Table A.2 – Continued to next page

Table A.2 – Continued from previous page

| Name      | $g$                                                                          | $N$                                                  | Signatures $S$                                                    |
|-----------|------------------------------------------------------------------------------|------------------------------------------------------|-------------------------------------------------------------------|
| 9641:101b | $0, 0, 0, e^{12}, e^{13}, -e^{14}, e^{24}, e^{15} + e^{23}, e^{27} + e^{16}$ | $(0, 0, 1, 0, 1, 0, 0, 1, 0)$                        | $\{1234689, 124569, 235678, 267\}$                                |
| 9641:138  | $0, 0, 0, e^{12}, e^{13}, e^{24}, e^{15}, e^{14}, e^{26} + e^{17}$           | $1/279(73, 112, 190, 185, 263, 297, 336, 258, 409)$  | $\{124589, 137, 268, 345679\}$                                    |
| 9641:139  | $0, 0, 0, e^{12}, e^{13}, e^{14}, e^{35}, e^{24}, e^{16} + e^{37}$           | $2/321(51, 75, 59, 126, 110, 177, 169, 201, 228)$    | $\{\emptyset, 123678, 145789, 234569\}$                           |
| 9641:140  | $0, 0, 0, e^{12}, e^{13}, e^{24}, e^{35}, e^{14}, e^{26} + e^{37}$           | $4/99(11, 8, 8, 19, 19, 27, 27, 30, 35)$             | $\{\emptyset, 123678, 145679, 234589\}$                           |
| 9641:141  | $0, 0, 0, e^{12}, e^{13}, e^{24}, e^{15}, e^{23} + e^{14}, e^{17} + e^{26}$  | $7/71(3, 4, 6, 7, 9, 11, 12, 10, 15)$                | $\{124589, 268\}$                                                 |
| 9641:142  | $0, 0, 0, e^{12}, e^{13}, e^{24}, e^{35}, e^{23} + e^{14}, e^{37} + e^{26}$  | $16/71(1, 2, 2, 3, 3, 5, 5, 4, 7)$                   | $\{123678, 234589\}$                                              |
| 9641:143  | $0, 0, 0, e^{12}, e^{13}, e^{24}, e^{15}, e^{14} + e^{35}, e^{17} + e^{26}$  | $10/27(1, 1, 1, 2, 2, 3, 3, 4)$                      | $\{124589, 345679\}$                                              |
| 9641:150  | $0, 0, 0, e^{12}, e^{13}, e^{24}, e^{15}, e^{14}, e^{26} + e^{35} + e^{17}$  | $7/71(3, 4, 6, 7, 9, 11, 12, 10, 15)$                | $\{145689, 8\}$                                                   |
| 9641:215a | $0, 0, 0, e^{12}, e^{13}, e^{14}, e^{24}, e^{35}, e^{27} + e^{16} + e^{38}$  | $10/27(1, 1, 1, 2, 2, 3, 3, 4)$                      | $\{\emptyset, 123678, 145789, 234569\}$                           |
| 9641:215b | $0, 0, 0, e^{12}, e^{13}, -e^{14}, e^{24}, e^{35}, e^{38} + e^{16} + e^{27}$ | $10/27(1, 1, 1, 2, 2, 3, 3, 4)$                      | $\{\emptyset, 123678, 145789, 234569\}$                           |
| 9631:1    | $0, 0, 0, e^{12}, e^{13}, e^{23}, e^{14}, e^{24}, e^{17}$                    | $1/257(70, 116, 195, 186, 265, 311, 256, 302, 326)$  | $\{\emptyset, 12378, 125678, 134689, 14589, 234579, 24679, 356\}$ |
| 9631:2    | $0, 0, 0, e^{12}, e^{13}, e^{23}, e^{14}, e^{35}, e^{17}$                    | $1/317(66, 204, 169, 270, 235, 373, 336, 404, 402)$  | $\{\emptyset, 12378, 125678, 134689, 14589, 234579, 24679, 356\}$ |
| 9631:3    | $0, 0, 0, e^{12}, e^{13}, e^{23}, e^{24}, e^{35}, e^{27}$                    | $1/17(8, 5, 8, 13, 16, 13, 18, 24, 23)$              | $\{123678, 12578, 134789, 1456789, 234569, 249, 35, 6\}$          |
| 9631:4    | $0, 0, 0, e^{12}, e^{13}, e^{23}, e^{14}, e^{15}, e^{17}$                    | $1/227(49, 137, 156, 186, 205, 293, 235, 254, 284)$  | $\{\emptyset, 12378, 12567, 134689, 1459, 2345789, 24679, 3568\}$ |
| 9631:6a   | $0, 0, 0, e^{12}, e^{13}, e^{23}, e^{14}, e^{24} + e^{35}, e^{17}$           | $1/157(36, 89, 89, 125, 125, 178, 161, 214, 197)$    | $\{\emptyset, 12378, 125678, 134689, 14589, 234579, 24679, 356\}$ |
| 9631:6b   | $0, 0, 0, -e^{12}, e^{13}, e^{23}, e^{14}, e^{35} + e^{24}, e^{17}$          | $1/157(36, 89, 89, 125, 125, 178, 161, 214, 197)$    | $\{\emptyset, 12378, 125678, 134689, 14589, 234579, 24679, 356\}$ |
| 9631:8    | $0, 0, 0, e^{12}, e^{13}, e^{23}, e^{24}, e^{14} + e^{35}, e^{27}$           | $1/71(38, 20, 29, 58, 67, 49, 78, 96, 98)$           | $\{134789, 1456789, 234569, 249\}$                                |
| 9631:10   | $0, 0, 0, e^{12}, e^{13}, e^{23}, e^{14}, e^{15}, e^{35} + e^{17}$           | $2/57(7, 18, 16, 25, 23, 34, 32, 30, 39)$            | $\{\emptyset, 134689, 1459, 3568\}$                               |
| 9631:11   | $0, 0, 0, e^{12}, e^{13}, e^{23}, e^{24}, e^{15}, e^{35} + e^{27}$           | $1/81(28, 30, 45, 58, 73, 75, 88, 101, 118)$         | $\{134789, 145679, 358, 6\}$                                      |
| 9631:12   | $0, 0, 0, e^{12}, e^{13}, e^{23}, e^{24}, e^{35}, e^{15} + e^{27}$           | $1/91(41, 28, 43, 69, 84, 71, 97, 127, 125)$         | $\{12578, 134789, 234569, 6\}$                                    |
| 9631:13   | $0, 0, 0, e^{12}, e^{13}, e^{23}, e^{14}, e^{36} + e^{15}, e^{17}$           | $1/109(43, 34, 52, 77, 95, 86, 120, 138, 163)$       | $\{123578, 149, 234789, 5\}$                                      |
| 9631:14   | $0, 0, 0, e^{12}, e^{13}, e^{23}, e^{14}, e^{26} + e^{35}, e^{17}$           | $1/657(193, 282, 371, 475, 564, 653, 668, 935, 861)$ | $\{\emptyset, 12378, 134689, 24679\}$                             |
| 9631:15   | $0, 0, 0, e^{12}, e^{13}, e^{23}, e^{14}, e^{35}, e^{17} + e^{36}$           | $1/61(18, 34, 27, 52, 45, 61, 70, 72, 88)$           | $\{234789, 2456789, 368, 58\}$                                    |
| 9631:16   | $0, 0, 0, e^{12}, e^{13}, e^{23}, e^{24}, e^{35}, e^{27} + e^{36}$           | $1/133(58, 39, 68, 97, 126, 107, 136, 194, 175)$     | $\{234569, 249, 35, 6\}$                                          |
| 9631:17   | $0, 0, 0, e^{12}, e^{13}, e^{23}, e^{14}, e^{15} + e^{24}, e^{17}$           | $1/147(37, 72, 107, 109, 144, 179, 146, 181, 183)$   | $\{\emptyset, 12378, 134689, 24679\}$                             |
| 9631:20   | $0, 0, 0, e^{12}, e^{13}, e^{23}, e^{14}, e^{24}, e^{35} + e^{17}$           | $1/231(71, 110, 126, 181, 197, 236, 252, 291, 323)$  | $\{\emptyset, 134689, 14589, 356\}$                               |
| 9631:21   | $0, 0, 0, e^{12}, e^{13}, e^{23}, e^{24}, e^{14}, e^{27} + e^{35}$           | $1/301(118, 110, 165, 228, 283, 275, 338, 346, 448)$ | $\{13479, 145679, 35, 6\}$                                        |
| 9631:22   | $0, 0, 0, e^{12}, e^{13}, e^{23}, e^{14}, e^{35}, e^{17} + e^{24}$           | $1/67(18, 36, 35, 54, 53, 71, 72, 88, 90)$           | $\{\emptyset, 134689, 14589, 356\}$                               |
| 9631:23   | $0, 0, 0, e^{12}, e^{13}, e^{23}, e^{24}, e^{35}, e^{14} + e^{27}$           | $5/133(14, 7, 12, 21, 26, 19, 28, 38, 35)$           | $\{123678, 12578, 134789, 1456789\}$                              |
| 9631:24   | $0, 0, 0, e^{12}, e^{13}, e^{23}, e^{14}, e^{15}, e^{17} + e^{36}$           | $1/107(34, 56, 51, 90, 85, 107, 124, 119, 158)$      | $\{23479, 2456789, 36, 58\}$                                      |
| 9631:25   | $0, 0, 0, e^{12}, e^{13}, e^{23}, e^{24}, e^{15}, e^{27} + e^{36}$           | $2/41(8, 7, 11, 15, 19, 18, 22, 27, 29)$             | $\{\emptyset, 234589, 2469, 3568\}$                               |
| 9631:26   | $0, 0, 0, e^{12}, e^{13}, e^{23}, e^{14}, e^{35}, e^{17} + e^{26}$           | $24/151(2, 3, 3, 5, 5, 6, 7, 8, 9)$                  | $\{\emptyset, 125678, 134689, 234579\}$                           |
| 9631:29   | $0, 0, 0, e^{12}, e^{13}, e^{23}, e^{14}, e^{36} + e^{15}, e^{35} + e^{17}$  | $7/53(3, 2, 4, 5, 7, 6, 8, 10, 11)$                  | $\{149, 5\}$                                                      |
| 9631:30   | $0, 0, 0, e^{12}, e^{13}, e^{23}, e^{24}, e^{36} + e^{15}, e^{35} + e^{27}$  | $91/1093(5, 4, 6, 9, 11, 10, 13, 16, 17)$            | $\{134789, 358\}$                                                 |
| 9631:31   | $0, 0, 0, e^{12}, e^{13}, e^{23}, e^{24}, e^{14}, e^{27} + e^{15}$           | $2/499(91, 88, 173, 179, 264, 261, 267, 270, 355)$   | $\{\emptyset, 125678, 134679, 234589\}$                           |
| 9631:32   | $0, 0, 0, e^{12}, e^{13}, e^{23}, e^{14}, e^{15}, e^{24} + e^{17}$           | $4/77(5, 10, 13, 15, 18, 23, 20, 23, 25)$            | $\{\emptyset, 134689, 1459, 3568\}$                               |
| 9631:33   | $0, 0, 0, e^{12}, e^{13}, e^{23}, e^{24}, e^{15}, e^{27} + e^{14}$           | $2/17(4, 2, 5, 6, 9, 7, 8, 13, 10)$                  | $\{1234689, 12459, 138, 156\}$                                    |
| 9631:34   | $0, 0, 0, e^{12}, e^{13}, e^{23}, e^{14}, e^{15}, e^{17} + e^{26}$           | $1/241(80, 103, 137, 183, 217, 240, 263, 297, 343)$  | $\{123489, 157, 26, 3456789\}$                                    |
| 9631:35   | $0, 0, 0, e^{12}, e^{13}, e^{23}, e^{14}, e^{15} + e^{24}, e^{17} + e^{35}$  | $35/317(3, 4, 5, 7, 8, 9, 10, 11, 13)$               | $\{145689, 35\}$                                                  |
| 9631:36   | $0, 0, 0, e^{12}, e^{13}, e^{23}, e^{24}, e^{35} + e^{14}, e^{27} + e^{15}$  | $37/365(5, 3, 4, 8, 9, 7, 11, 13, 14)$               | $\{134789, 234569\}$                                              |
| 9631:38   | $0, 0, 0, e^{12}, e^{13}, e^{23}, e^{14}, e^{24} + e^{36} + e^{15}, e^{17}$  | $19/49(1, 1, 1, 2, 2, 2, 3, 3, 4)$                   | $\{149, 234789\}$                                                 |
| 9631:44   | $0, 0, 0, e^{12}, e^{13}, e^{23}, e^{24}, e^{26} + e^{35}, e^{15} + e^{27}$  | $1/7(1, 0, -1, 1, 0, -1, 1, -1, 1)$                  | $\{123678, 249\}$                                                 |
| 9631:46   | $0, 0, 0, e^{12}, e^{13}, e^{23}, e^{24}, e^{35}, e^{15} + e^{27} + e^{36}$  | $73/709(4, 3, 5, 7, 9, 8, 10, 14, 13)$               | $\{234569, 6\}$                                                   |
| 9631:49   | $0, 0, 0, e^{12}, e^{13}, e^{23}, e^{24}, e^{14} + e^{35}, e^{36} + e^{27}$  | $17/43(2, 0, 1, 2, 3, 1, 2, 4, 2)$                   | $\{1234689, 124589\}$                                             |
| 9631:52a  | $0, 0, 0, e^{12}, e^{13}, e^{23}, e^{14}, e^{15}, e^{35} + e^{24} + e^{17}$  | $7/25(1, 2, 2, 3, 3, 4, 4, 5)$                       | $\{\emptyset, 134689, 1459, 3568\}$                               |
| 9631:52b  | $0, 0, 0, -e^{12}, e^{13}, e^{23}, e^{14}, e^{15}, e^{24} + e^{35} + e^{17}$ | $7/25(1, 2, 2, 3, 3, 4, 4, 5)$                       | $\{\emptyset, 134689, 1459, 3568\}$                               |
| 9631:54   | $0, 0, 0, e^{12}, e^{13}, e^{23}, e^{24}, e^{15}, e^{27} + e^{35} + e^{14}$  | $7/53(4, 2, 3, 6, 7, 5, 8, 11, 10)$                  | $\{1234689, 12459\}$                                              |

Table A.2 – Continued to next page



Table A.2 – Continued from previous page

| Name      | $g$                                                                          | $N$                                                | Signatures $S$                                                    |
|-----------|------------------------------------------------------------------------------|----------------------------------------------------|-------------------------------------------------------------------|
| 9631:57   | $0, 0, 0, e^{12}, e^{13}, e^{23}, e^{14}, e^{15}, e^{17} + e^{26} + e^{35}$  | $35/317(3, 4, 5, 7, 8, 9, 10, 11, 13)$             | $\{123489, 26\}$                                                  |
| 9631:58   | $0, 0, 0, e^{12}, e^{13}, e^{23}, e^{14}, e^{15} + e^{24}, e^{17} + e^{36}$  | $89/1033(4, 5, 6, 9, 10, 11, 13, 14, 17)$          | $\{23479, 36\}$                                                   |
| 9631:61   | $0, 0, 0, e^{12}, e^{13}, e^{23}, e^{14}, e^{36} + e^{15}, e^{24} + e^{17}$  | $5/16(1, 2, 0, 3, 1, 2, 4, 2, 5)$                  | $\{123578, 234789\}$                                              |
| 9631:62   | $0, 0, 0, e^{12}, e^{13}, e^{23}, e^{14}, e^{26} + e^{35}, e^{24} + e^{17}$  | $17/77(1, 2, 3, 3, 4, 5, 4, 7, 5)$                 | $\{1234589, 256\}$                                                |
| 9631:63   | $0, 0, 0, e^{12}, e^{13}, e^{23}, e^{14}, e^{35}, e^{17} + e^{36} + e^{24}$  | $53/367(2, 4, 3, 6, 5, 7, 8, 8, 10)$               | $\{234789, 2456789\}$                                             |
| 9631:70   | $0, 0, 0, e^{12}, e^{13}, e^{23}, e^{14}, e^{24} + e^{15}, e^{26} + e^{17}$  | $35/317(3, 4, 5, 7, 8, 9, 10, 11, 13)$             | $\{123489, 26\}$                                                  |
| 9631:71a  | $0, 0, 0, e^{12}, e^{13}, e^{23}, e^{14}, e^{26} + e^{15}, e^{24} + e^{17}$  | $(0, 0, 1, 0, 1, 1, 0, 1, 0)$                      | $\{1234589, 12469, 238, 256\}$                                    |
| 9631:71b  | $0, 0, 0, e^{12}, -e^{13}, e^{23}, e^{14}, e^{26} + e^{15}, e^{24} + e^{17}$ | $(0, 0, 1, 0, 1, 1, 0, 1, 0)$                      | $\{1234589, 12469, 238, 256\}$                                    |
| 9631:74   | $0, 0, 0, e^{12}, e^{13}, e^{23}, e^{14}, e^{24}, e^{26} + e^{35} + e^{17}$  | $35/317(3, 4, 5, 7, 8, 9, 10, 11, 13)$             | $\{\emptyset, 134689\}$                                           |
| 9631:75   | $0, 0, 0, e^{12}, e^{13}, e^{23}, e^{14}, e^{15}, e^{17} + e^{36} + e^{24}$  | $13/88(2, 4, 3, 6, 5, 7, 8, 7, 10)$                | $\{23479, 2456789\}$                                              |
| 9631:107a | $0, 0, 0, e^{12}, e^{13}, e^{23}, e^{14}, e^{24}, e^{28} + e^{17}$           | $1/61(21, 21, 47, 42, 68, 68, 63, 63, 84)$         | $\{\emptyset, 12378, 125678, 134689, 14589, 234579, 24679, 356\}$ |
| 9631:107b | $0, 0, 0, e^{12}, e^{13}, e^{23}, -e^{14}, e^{24}, e^{28} + e^{17}$          | $1/61(21, 21, 47, 42, 68, 68, 63, 63, 84)$         | $\{\emptyset, 12378, 125678, 134689, 14589, 234579, 24679, 356\}$ |
| 9631:109a | $0, 0, 0, e^{12}, e^{13}, e^{23}, e^{14}, e^{24}, e^{17} + e^{28} + e^{35}$  | $41/219(2, 2, 3, 4, 5, 5, 6, 6, 8)$                | $\{13489, 145689, 35, 6\}$                                        |
| 9631:109b | $0, 0, 0, e^{12}, e^{13}, e^{23}, -e^{14}, e^{24}, e^{17} + e^{28} + e^{35}$ | $41/219(2, 2, 3, 4, 5, 5, 6, 6, 8)$                | $\{13489, 145689, 35, 6\}$                                        |
| 9631:132  | $0, 0, 0, e^{12}, e^{13}, e^{23}, e^{24}, e^{15}, e^{18} + e^{27}$           | $1/211(54, 83, 141, 137, 195, 224, 220, 249, 303)$ | $\{124569, 1368, 267, 3456789\}$                                  |
| 9631:133  | $0, 0, 0, e^{12}, e^{13}, e^{23}, e^{24}, e^{35}, e^{27} + e^{38}$           | $1/23(11, 8, 8, 19, 19, 16, 27, 27, 35)$           | $\{123678, 1456789, 234569, 6\}$                                  |
| 9631:136  | $0, 0, 0, e^{12}, e^{13}, e^{23}, e^{14}, e^{35}, e^{17} + e^{24} + e^{38}$  | $7/71(3, 6, 4, 9, 7, 10, 12, 11, 15)$              | $\{145689, 6\}$                                                   |
| 9631:137  | $0, 0, 0, e^{12}, e^{13}, e^{23}, e^{24}, e^{35}, e^{14} + e^{38} + e^{27}$  | $5/17(2, 1, 1, 3, 3, 2, 4, 4, 5)$                  | $\{123678, 1456789\}$                                             |
| 9631:138  | $0, 0, 0, e^{12}, e^{13}, e^{23}, e^{24}, e^{15}, e^{27} + e^{36} + e^{18}$  | $16/203(4, 5, 7, 9, 11, 12, 14, 15, 19)$           | $\{\emptyset, 234589\}$                                           |
| 963:1     | $0, 0, 0, e^{12}, e^{13}, e^{23}, e^{14}, e^{24}, e^{15}$                    | $1/23(7, 11, 15, 18, 22, 26, 25, 29, 29)$          | $\{\emptyset, 123789, 125678, 134689, 1458, 234579, 2467, 3569\}$ |
| 963:2     | $0, 0, 0, e^{12}, e^{13}, e^{23}, e^{14}, e^{24}, e^{35}$                    | $1/139(49, 65, 69, 114, 118, 134, 163, 179, 187)$  | $\{1236789, 125789, 13489, 145689, 234567, 247, 35, 6\}$          |
| 963:4a    | $0, 0, 0, e^{12}, e^{13}, e^{23}, e^{14}, e^{15}, e^{35} + e^{24}$           | $1/13(4, 7, 7, 11, 11, 14, 15, 15, 18)$            | $\{\emptyset, 123789, 125679, 134689, 1459, 234578, 2467, 3568\}$ |
| 963:4b    | $0, 0, 0, -e^{12}, e^{13}, e^{23}, e^{14}, e^{15}, e^{35} + e^{24}$          | $1/13(4, 7, 7, 11, 11, 14, 15, 15, 18)$            | $\{\emptyset, 123789, 125679, 134689, 1459, 234578, 2467, 3568\}$ |
| 963:6     | $0, 0, 0, e^{12}, e^{13}, e^{23}, e^{24}, e^{15}, e^{14} + e^{35}$           | $1/16(6, 8, 7, 14, 13, 15, 22, 19, 20)$            | $\{134789, 145679, 234568, 24\}$                                  |
| 963:13    | $0, 0, 0, e^{12}, e^{13}, e^{23}, e^{14}, e^{15}, e^{26}$                    | $1/139(53, 57, 73, 110, 126, 130, 163, 179, 187)$  | $\{123489, 12456, 136789, 157, 23589, 26, 3456789, 47\}$          |
| 963:14    | $0, 0, 0, e^{12}, e^{13}, e^{23}, e^{24}, e^{15}, e^{36}$                    | $3/7(1, 1, 1, 2, 2, 2, 3, 3, 3)$                   | $\{\emptyset, 123789, 125679, 134678, 1457, 234589, 2469, 3568\}$ |
| 963:15a   | $0, 0, 0, e^{12}, e^{13}, e^{23}, e^{14}, e^{24}, e^{26} + e^{15}$           | $1/13(5, 5, 8, 10, 13, 13, 15, 15, 18)$            | $\{\emptyset, 123789, 125678, 134689, 1458, 234579, 2467, 3569\}$ |
| 963:15b   | $0, 0, 0, e^{12}, -e^{13}, e^{23}, e^{14}, e^{24}, e^{15} + e^{26}$          | $1/13(5, 5, 8, 10, 13, 13, 15, 15, 18)$            | $\{\emptyset, 123789, 125678, 134689, 1458, 234579, 2467, 3569\}$ |
| 963:18    | $0, 0, 0, e^{12}, e^{13}, e^{23}, e^{24}, e^{15}, e^{26} + e^{14}$           | $1/16(7, 6, 8, 13, 15, 14, 19, 22, 20)$            | $\{123489, 15, 235789, 47\}$                                      |
| 963:23    | $0, 0, 0, e^{12}, e^{13}, e^{23}, e^{24}, e^{35}, e^{14} + e^{26}$           | $1/179(77, 73, 81, 150, 158, 154, 223, 239, 227)$  | $\{125789, 13478, 249, 35\}$                                      |
| 963:25    | $0, 0, 0, e^{12}, e^{13}, e^{23}, e^{14}, e^{35}, e^{24} + e^{36}$           | $1/95(37, 45, 41, 82, 78, 86, 119, 119, 127)$      | $\{\emptyset, 123789, 1256789, 356\}$                             |
| 963:30    | $0, 0, 0, e^{12}, e^{13}, e^{23}, e^{24}, e^{15}, e^{26} + e^{35} + e^{14}$  | $3/7(1, 1, 1, 2, 2, 2, 3, 3, 3)$                   | $\{1346789, 246\}$                                                |
| 963:47    | $0, 0, 0, e^{12}, e^{13}, e^{23}, e^{24}, e^{14} + e^{35}, e^{15} + e^{36}$  | $3/7(1, 1, 1, 2, 2, 2, 3, 3, 3)$                   | $\{\emptyset, 123789\}$                                           |
| 963:50    | $0, 0, 0, e^{12}, e^{13}, e^{23}, e^{15} + e^{24}, e^{14} + e^{35}, e^{26}$  | $3/7(1, 1, 1, 2, 2, 2, 3, 3, 3)$                   | $\{\emptyset, 123789\}$                                           |
| 954321:2  | $0, 0, 0, 0, e^{12}, e^{15}, e^{16}, e^{17}, e^{34} + e^{18}$                | $7/139(2, 16, 13, 13, 18, 20, 22, 24, 26)$         | $\{123689, 124689, 13457, 157, 2345678, 25678, 39, 49\}$          |
| 954321:6  | $0, 0, 0, 0, e^{12}, e^{15}, e^{16}, e^{17}, e^{25} + e^{18} + e^{34}$       | $49/625(2, 8, 9, 9, 10, 12, 14, 16, 18)$           | $\{123689, 124689, 2345678, 25678\}$                              |
| 95421:2   | $0, 0, 0, 0, e^{12}, e^{15}, e^{34} + e^{25}, e^{16}, e^{18}$                | $1/29(4, 19, 21, 21, 23, 27, 42, 31, 35)$          | $\{\emptyset, 123679, 124679, 13578, 14578, 2345689, 25689, 34\}$ |
| 95421:4   | $0, 0, 0, 0, e^{12}, e^{15}, e^{25}, e^{16}, e^{18} + e^{34}$                | $1/23(5, 12, 16, 16, 17, 22, 29, 27, 32)$          | $\{\emptyset, 123679, 124679, 134578, 1578, 235689, 245689, 34\}$ |
| 95421:6   | $0, 0, 0, 0, e^{12}, e^{15}, e^{13} + e^{25}, e^{16}, e^{18} + e^{34}$       | $1/19(5, 8, 16, 12, 13, 18, 21, 23, 28)$           | $\{123679, 134578, 235689, 34\}$                                  |
| 95421:7   | $0, 0, 0, 0, e^{12}, e^{15}, e^{25} + e^{34}, e^{16}, e^{18} + e^{23}$       | $1/141(23, 87, 92, 105, 110, 133, 197, 156, 179)$  | $\{\emptyset, 124679, 14578, 25689\}$                             |
| 95421:15  | $0, 0, 0, 0, e^{12}, e^{15}, e^{25}, e^{16}, e^{34} + e^{27} + e^{18}$       | $56/827(4, 6, 11, 11, 10, 14, 16, 18, 22)$         | $\{\emptyset, 235689, 245689, 34\}$                               |
| 95321:4   | $0, 0, 0, 0, e^{12}, e^{34}, e^{15}, e^{17}, e^{36} + e^{18}$                | $1/141(21, 108, 49, 94, 129, 143, 150, 171, 192)$  | $\{\emptyset, 123479, 124679, 13568, 158, 2345789, 2456789, 36\}$ |
| 95321:5   | $0, 0, 0, 0, e^{12}, e^{13}, e^{15}, e^{17}, e^{18} + e^{34}$                | $1/43(7, 32, 32, 28, 39, 39, 46, 53, 60)$          | $\{123679, 12479, 134568, 158, 235789, 2456789, 34, 6\}$          |
| 95321:6   | $0, 0, 0, 0, e^{12}, e^{13}, e^{25}, e^{27}, e^{28} + e^{34}$                | $1/41(27, 7, 23, 32, 34, 50, 41, 48, 55)$          | $\{\emptyset, 12379, 124679, 135789, 1456789, 234568, 258, 346\}$ |
| 95321:7   | $0, 0, 0, 0, e^{12}, e^{24} + e^{13}, e^{15}, e^{17}, e^{18}$                | $1/43(7, 26, 47, 28, 33, 54, 40, 47, 54)$          | $\{123679, 12479, 134568, 158, 2345789, 256789, 3, 46\}$          |
| 95321:8   | $0, 0, 0, 0, e^{12}, e^{34}, e^{15}, e^{17}, e^{18} + e^{23}$                | $1/7(1, 5, 4, 5, 6, 9, 7, 8, 9)$                   | $\{\emptyset, 124679, 1279, 14568, 158, 2456789, 25789, 46\}$     |
| 95321:13  | $0, 0, 0, 0, e^{12}, e^{13}, e^{15}, e^{17}, e^{18} + e^{24}$                | $1/11(2, 7, 10, 8, 9, 12, 11, 13, 15)$             | $\{\emptyset, 12379, 12679, 1358, 1568, 2356789, 25789, 36\}$     |

Table A.2 – Continued to next page

Table A.2 – Continued from previous page

| Name      | $g$                                                                             | $N$                                                  | Signatures $S$                                                    |
|-----------|---------------------------------------------------------------------------------|------------------------------------------------------|-------------------------------------------------------------------|
| 95321:14  | $0, 0, 0, 0, e^{12}, e^{13}, e^{25}, e^{27}, e^{14} + e^{28}$                   | $1/317(170, 65, 232, 260, 235, 402, 300, 365, 430)$  | $\{\emptyset, 12379, 12679, 135789, 156789, 23568, 258, 36\}$     |
| 95321:15  | $0, 0, 0, 0, e^{12}, e^{24} + e^{13}, e^{15}, e^{17}, e^{34} + e^{18}$          | $1/71(14, 43, 64, 35, 57, 78, 71, 85, 99)$           | $\{123679, 12479, 134568, 158\}$                                  |
| 95321:18  | $0, 0, 0, 0, e^{12}, e^{34}, e^{15}, e^{17}, e^{46} + e^{23} + e^{18}$          | $1/81(13, 60, 52, 30, 73, 82, 86, 99, 112)$          | $\{\emptyset, 14568, 158, 46\}$                                   |
| 95321:22  | $0, 0, 0, 0, e^{12}, e^{13} + e^{24}, e^{15}, e^{17}, e^{23} + e^{18}$          | $1/557(130, 263, 520, 387, 393, 650, 523, 653, 783)$ | $\{12479, 158, 256789, 46\}$                                      |
| 95321:25  | $0, 0, 0, 0, e^{12}, e^{13}, e^{15}, e^{17}, e^{24} + e^{36} + e^{18}$          | $1/129(26, 84, 81, 104, 110, 107, 136, 162, 188)$    | $\{134589, 145689, 2345678, 24578\}$                              |
| 95321:26a | $0, 0, 0, 0, e^{12}, e^{13}, e^{25}, e^{27}, e^{28} + e^{36} + e^{14}$          | $1/31(17, 7, 14, 28, 24, 31, 31, 38, 45)$            | $\{\emptyset, 12379, 12679, 135789, 156789, 23568, 258, 36\}$     |
| 95321:26b | $0, 0, 0, 0, -e^{12}, e^{13}, e^{25}, e^{27}, e^{28} + e^{36} + e^{14}$         | $1/31(17, 7, 14, 28, 24, 31, 31, 38, 45)$            | $\{\emptyset, 12379, 12679, 135789, 156789, 23568, 258, 36\}$     |
| 95321:34  | $0, 0, 0, 0, e^{12}, e^{34}, e^{15}, e^{17}, e^{18} + e^{36} + e^{25}$          | $2/321(33, 99, 62, 107, 132, 169, 165, 198, 231)$    | $\{\emptyset, 123479, 124679, 36\}$                               |
| 95321:39  | $0, 0, 0, 0, e^{12}, e^{13}, e^{15}, e^{17}, e^{18} + e^{25} + e^{34}$          | $1/87(18, 54, 65, 61, 72, 83, 90, 108, 126)$         | $\{123679, 12479, 34, 6\}$                                        |
| 95321:40  | $0, 0, 0, 0, e^{12}, e^{13}, e^{25}, e^{27}, e^{15} + e^{34} + e^{28}$          | $1/283(168, 56, 169, 223, 224, 337, 280, 336, 392)$  | $\{\emptyset, 12379, 124679, 346\}$                               |
| 95321:41  | $0, 0, 0, 0, e^{12}, e^{13} + e^{24}, e^{15}, e^{17}, e^{25} + e^{18}$          | $1/211(39, 117, 224, 146, 156, 263, 195, 234, 273)$  | $\{123679, 12479, 3, 46\}$                                        |
| 95321:67  | $0, 0, 0, 0, e^{12}, e^{24} + e^{13}, e^{15}, e^{17}, e^{18} + e^{34} + e^{25}$ | $77/771(2, 6, 9, 5, 8, 11, 10, 12, 14)$              | $\{123679, 12479\}$                                               |
| 9542:2    | $0, 0, 0, 0, e^{12}, e^{15}, e^{25}, e^{16}, e^{27} + e^{34}$                   | $1/44(13, 17, 32, 32, 30, 43, 47, 56, 64)$           | $\{\emptyset, 123467, 1267, 135789, 145789, 235689, 245689, 34\}$ |
| 9542:4    | $0, 0, 0, 0, e^{12}, e^{15}, e^{25}, e^{16} + e^{23}, e^{27} + e^{34}$          | $2/151(20, 31, 60, 53, 51, 71, 82, 91, 113)$         | $\{1267, 145789, 235689, 34\}$                                    |
| 9542:7    | $0, 0, 0, 0, e^{12}, e^{15}, e^{25}, e^{16} + e^{23}, e^{27} + e^{14}$          | $12/37(1, 1, 3, 3, 2, 3, 3, 4, 4)$                   | $\{\emptyset, 123467, 135789, 245689\}$                           |
| 9531:4    | $0, 0, 0, 0, e^{12}, e^{13}, e^{15}, e^{34} + e^{25}, e^{17}$                   | $1/23(5, 14, 17, 16, 19, 22, 24, 33, 29)$            | $\{123678, 12478, 135689, 14589, 234579, 25679, 34, 6\}$          |
| 9531:5    | $0, 0, 0, 0, e^{12}, e^{13}, e^{25}, e^{15} + e^{34}, e^{27}$                   | $1/353(196, 84, 211, 265, 280, 407, 364, 476, 448)$  | $\{\emptyset, 12378, 124678, 134579, 15679, 235689, 24589, 346\}$ |
| 9531:6    | $0, 0, 0, 0, e^{12}, e^{34}, e^{15}, e^{13} + e^{25}, e^{17}$                   | $1/10(3, 4, 8, 6, 7, 14, 10, 11, 13)$                | $\{123478, 123678, 134589, 135689, 234579, 235679, 34, 36\}$      |
| 9531:10   | $0, 0, 0, 0, e^{12}, e^{13}, e^{15}, e^{25}, e^{17} + e^{34}$                   | $1/107(34, 50, 75, 77, 84, 109, 118, 134, 152)$      | $\{\emptyset, 123478, 12678, 13589, 145689, 235679, 24579, 346\}$ |
| 9531:11   | $0, 0, 0, 0, e^{12}, e^{13}, e^{25}, e^{15}, e^{34} + e^{27}$                   | $1/99(44, 32, 65, 75, 76, 109, 108, 120, 140)$       | $\{\emptyset, 123478, 12678, 13579, 145679, 235689, 24589, 346\}$ |
| 9531:12   | $0, 0, 0, 0, e^{12}, e^{24} + e^{13}, e^{15}, e^{25}, e^{17}$                   | $1/257(70, 116, 249, 203, 186, 319, 256, 302, 326)$  | $\{\emptyset, 123478, 12678, 13589, 145689, 235679, 24579, 346\}$ |
| 9531:13   | $0, 0, 0, 0, e^{12}, e^{34}, e^{15}, e^{25}, e^{17} + e^{23}$                   | $1/172(40, 89, 120, 112, 129, 232, 169, 218, 209)$   | $\{124678, 1278, 145689, 1589, 234579, 235679, 34, 36\}$          |
| 9531:14   | $0, 0, 0, 0, e^{12}, e^{13}, e^{15}, e^{25} + e^{14}, e^{17}$                   | $1/67(16, 34, 59, 68, 50, 75, 66, 84, 82)$           | $\{123478, 124678, 134589, 145689, 2345679, 24579, 346, 4\}$      |
| 9531:15   | $0, 0, 0, 0, e^{12}, e^{13}, e^{25}, e^{15} + e^{24}, e^{27}$                   | $1/34(16, 9, 26, 32, 25, 42, 34, 41, 43)$            | $\{\emptyset, 12378, 12678, 13579, 15679, 235689, 2589, 36\}$     |
| 9531:16   | $0, 0, 0, 0, e^{12}, e^{24} + e^{13}, e^{15}, e^{25} + e^{34}, e^{17}$          | $1/259(65, 142, 213, 136, 207, 278, 272, 349, 337)$  | $\{123678, 12478, 234579, 25679\}$                                |
| 9531:20   | $0, 0, 0, 0, e^{12}, e^{13}, e^{15}, e^{25}, e^{24} + e^{17}$                   | $1/28(8, 13, 24, 24, 21, 32, 29, 34, 37)$            | $\{\emptyset, 123478, 124678, 134589, 145689, 235679, 2579, 36\}$ |
| 9531:21   | $0, 0, 0, 0, e^{12}, e^{13}, e^{25}, e^{15}, e^{14} + e^{27}$                   | $1/297(124, 91, 235, 273, 215, 359, 306, 339, 397)$  | $\{\emptyset, 123478, 124678, 13579, 15679, 2345689, 24589, 36\}$ |
| 9531:24   | $0, 0, 0, 0, e^{12}, e^{13}, e^{25}, e^{23} + e^{15}, e^{27} + e^{34}$          | $1/175(65, 64, 130, 127, 129, 195, 193, 194, 257)$   | $\{123478, 13579, 235689, 346\}$                                  |
| 9531:25   | $0, 0, 0, 0, e^{12}, e^{13}, e^{15}, e^{25} + e^{34}, e^{17} + e^{23}$          | $1/131(31, 77, 93, 92, 108, 124, 139, 185, 170)$     | $\{123678, 135689, 25679, 6\}$                                    |
| 9531:26   | $0, 0, 0, 0, e^{12}, e^{13}, e^{15}, e^{14} + e^{25}, e^{17} + e^{34}$          | $1/191(68, 77, 127, 154, 145, 195, 213, 222, 281)$   | $\{123478, 145689, 24579, 346\}$                                  |
| 9531:27   | $0, 0, 0, 0, e^{12}, e^{13}, e^{25}, e^{15} + e^{24}, e^{34} + e^{27}$          | $7/139(8, 7, 13, 16, 15, 21, 22, 23, 29)$            | $\{123478, 145679, 24589, 346\}$                                  |
| 9531:28   | $0, 0, 0, 0, e^{12}, e^{13}, e^{15}, e^{25} + e^{34}, e^{24} + e^{17}$          | $1/119(27, 71, 88, 81, 98, 115, 125, 169, 152)$      | $\{12478, 14589, 25679, 6\}$                                      |
| 9531:29   | $0, 0, 0, 0, e^{12}, e^{13}, e^{25}, e^{34} + e^{15}, e^{14} + e^{27}$          | $1/53(29, 13, 32, 39, 42, 61, 55, 71, 68)$           | $\{\emptyset, 124678, 15679, 24589\}$                             |
| 9531:30   | $0, 0, 0, 0, e^{12}, e^{14} + e^{23}, e^{15}, e^{13} + e^{25}, e^{17}$          | $7/485(20, 29, 58, 67, 49, 87, 69, 78, 89)$          | $\{123478, 135689, 23579, 346\}$                                  |
| 9531:31   | $0, 0, 0, 0, e^{12}, e^{34}, e^{15}, e^{13} + e^{25}, e^{23} + e^{17}$          | $1/143(40, 60, 120, 83, 100, 203, 140, 160, 180)$    | $\{234579, 235679, 34, 36\}$                                      |
| 9531:32   | $0, 0, 0, 0, e^{12}, e^{34}, e^{15}, e^{13} + e^{25}, e^{24} + e^{17}$          | $1/29(7, 12, 24, 21, 19, 45, 26, 31, 33)$            | $\{123678, 135689, 234579, 34\}$                                  |
| 9531:33   | $0, 0, 0, 0, e^{12}, e^{13}, e^{15}, e^{36}, e^{17} + e^{34}$                   | $1/317(66, 232, 169, 261, 298, 235, 364, 404, 430)$  | $\{\emptyset, 123478, 12678, 13589, 145689, 235679, 24579, 346\}$ |
| 9531:34   | $0, 0, 0, 0, e^{12}, e^{13}, e^{25}, e^{36}, e^{34} + e^{27}$                   | $1/57(33, 14, 21, 54, 47, 54, 61, 75, 75)$           | $\{\emptyset, 123478, 12678, 135789, 1456789, 23569, 2459, 346\}$ |
| 9531:35   | $0, 0, 0, 0, e^{12}, e^{13}, e^{15}, e^{14} + e^{36}, e^{17}$                   | $1/71(12, 53, 39, 78, 65, 51, 77, 90, 89)$           | $\{123478, 124678, 134589, 145689, 2345679, 24579, 346, 4\}$      |
| 9531:36   | $0, 0, 0, 0, e^{12}, e^{13}, e^{15}, e^{16} + e^{34}, e^{17}$                   | $1/8(2, 5, 6, 4, 7, 8, 9, 10, 11)$                   | $\{123678, 127, 135689, 159, 235789, 25679, 38, 6\}$              |
| 9531:37   | $0, 0, 0, 0, e^{12}, e^{13}, e^{15}, e^{24} + e^{36}, e^{17}$                   | $1/353(70, 231, 223, 285, 301, 293, 371, 516, 441)$  | $\{\emptyset, 12378, 12678, 134589, 145689, 2345679, 24579, 36\}$ |
| 9531:38   | $0, 0, 0, 0, e^{12}, e^{13}, e^{25}, e^{36} + e^{14}, e^{27}$                   | $1/27(14, 7, 12, 24, 21, 26, 28, 38, 35)$            | $\{\emptyset, 12378, 12678, 135789, 156789, 23569, 259, 36\}$     |
| 9531:39   | $0, 0, 0, 0, e^{12}, e^{13}, e^{25}, e^{16} + e^{34}, e^{27}$                   | $1/57(24, 17, 33, 48, 41, 57, 58, 81, 75)$           | $\{\emptyset, 12378, 1267, 135789, 15679, 235689, 259, 368\}$     |
| 9531:40   | $0, 0, 0, 0, e^{12}, e^{13}, e^{25}, e^{36} + e^{24}, e^{27}$                   | $1/57(32, 14, 21, 60, 46, 53, 60, 74, 74)$           | $\{123478, 124678, 135789, 156789, 23569, 259, 346, 4\}$          |
| 9531:41   | $0, 0, 0, 0, e^{12}, e^{13} + e^{24}, e^{15}, e^{25}, e^{17} + e^{23}$          | $1/497(151, 209, 453, 395, 360, 604, 511, 569, 662)$ | $\{\emptyset, 123478, 13589, 24579\}$                             |
| 9531:45   | $0, 0, 0, 0, e^{12}, e^{13}, e^{15}, e^{16}, e^{17} + e^{34}$                   | $1/227(49, 170, 156, 161, 219, 205, 268, 254, 317)$  | $\{\emptyset, 123478, 1267, 13589, 14569, 2356789, 24579, 3468\}$ |
| 9531:46   | $0, 0, 0, 0, e^{12}, e^{13}, e^{25}, e^{16}, e^{27} + e^{34}$                   | $1/57(21, 20, 33, 48, 41, 54, 61, 75, 81)$           | $\{\emptyset, 123478, 1267, 135789, 145679, 235689, 2459, 3468\}$ |

Table A.2 – Continued to next page

Table A.2 – Continued from previous page

| Name      | $g$                                                                             | $N$                                                  | Signatures $S$                                                    |
|-----------|---------------------------------------------------------------------------------|------------------------------------------------------|-------------------------------------------------------------------|
| 9531:47   | $0, 0, 0, 0, e^{12}, e^{13}, e^{15}, e^{36}, e^{24} + e^{17}$                   | $1/93(24, 57, 50, 72, 81, 74, 105, 124, 129)$        | $\{\emptyset, 123478, 124678, 134589, 145689, 235679, 2579, 36\}$ |
| 9531:48   | $0, 0, 0, 0, e^{12}, e^{13}, e^{25}, e^{36}, e^{14} + e^{27}$                   | $1/24(12, 7, 10, 21, 19, 22, 26, 32, 33)$            | $\{\emptyset, 123478, 124678, 135789, 156789, 234569, 2459, 36\}$ |
| 9531:49   | $0, 0, 0, 0, e^{12}, e^{13}, e^{15}, e^{24} + e^{16}, e^{17}$                   | $1/227(49, 137, 200, 161, 186, 249, 235, 298, 284)$  | $\{\emptyset, 12378, 12467, 134589, 1569, 2356789, 24579, 3468\}$ |
| 9531:51   | $0, 0, 0, 0, e^{12}, e^{13}, e^{25}, e^{15} + e^{23}, e^{14} + e^{27}$          | $11/461(17, 13, 34, 39, 30, 51, 43, 47, 56)$         | $\{\emptyset, 123478, 13579, 2345689, 36\}$                       |
| 9531:52   | $0, 0, 0, 0, e^{12}, e^{13}, e^{15}, e^{25} + e^{14}, e^{17} + e^{23}$          | $1/107(29, 52, 87, 104, 81, 116, 110, 133, 139)$     | $\{\emptyset, 12378, 13589, 2579\}$                               |
| 9531:53   | $0, 0, 0, 0, e^{12}, e^{13}, e^{15}, e^{14} + e^{25}, e^{17} + e^{24}$          | $1/27(8, 12, 23, 24, 20, 31, 28, 32, 36)$            | $\{123478, 124678, 134589, 145689\}$                              |
| 9531:54   | $0, 0, 0, 0, e^{12}, e^{13}, e^{25}, e^{15} + e^{24}, e^{27} + e^{14}$          | $1/109(48, 32, 85, 96, 80, 133, 112, 128, 144)$      | $\{\emptyset, 13579, 15679, 36\}$                                 |
| 9531:56   | $0, 0, 0, 0, e^{12}, e^{24} + e^{13}, e^{15}, e^{34} + e^{25}, e^{23} + e^{17}$ | $29/109(1, 2, 3, 2, 3, 4, 4, 5, 5)$                  | $\{123678, 25679\}$                                               |
| 9531:57   | $0, 0, 0, 0, e^{12}, e^{34}, e^{15}, e^{13} + e^{46}, e^{17}$                   | $1/9(2, 6, 8, 1, 8, 9, 10, 10, 12)$                  | $\{123478, 123678, 12467, 127, 134589, 135689, 14569, 159\}$      |
| 9531:58   | $0, 0, 0, 0, e^{12}, e^{34}, e^{15}, e^{46} + e^{23}, e^{17}$                   | $1/141(25, 102, 90, 51, 127, 141, 152, 192, 177)$    | $\{\emptyset, 134589, 135689, 14569, 159, 348, 368, 46\}$         |
| 9531:66   | $0, 0, 0, 0, e^{12}, e^{13}, e^{15}, e^{36} + e^{14}, e^{17} + e^{34}$          | $3/557(44, 129, 87, 174, 173, 131, 217, 218, 261)$   | $\{123478, 145689, 24579, 346\}$                                  |
| 9531:67   | $0, 0, 0, 0, e^{12}, e^{13}, e^{15}, e^{24} + e^{36}, e^{17} + e^{34}$          | $7/597(19, 56, 50, 63, 75, 69, 94, 119, 113)$        | $\{\emptyset, 12678, 145689, 24579\}$                             |
| 9531:68   | $0, 0, 0, 0, e^{12}, e^{13}, e^{25}, e^{36} + e^{14}, e^{34} + e^{27}$          | $1/681(357, 178, 297, 594, 535, 654, 713, 951, 891)$ | $\{\emptyset, 12678, 135789, 23569\}$                             |
| 9531:69   | $0, 0, 0, 0, e^{12}, e^{13}, e^{25}, e^{24} + e^{36}, e^{34} + e^{27}$          | $1/81(46, 21, 28, 81, 67, 74, 88, 102, 109)$         | $\{123478, 135789, 23569, 346\}$                                  |
| 9531:70   | $0, 0, 0, 0, e^{12}, e^{34}, e^{15}, e^{36}, e^{46} + e^{17}$                   | $1/33(7, 24, 13, 16, 31, 29, 38, 42, 45)$            | $\{\emptyset, 124678, 127, 134589, 13569, 2345789, 235679, 468\}$ |
| 9531:71   | $0, 0, 0, 0, e^{12}, e^{13}, e^{15}, e^{34} + e^{16}, e^{36} + e^{17}$          | $1/101(29, 62, 60, 58, 91, 89, 120, 118, 149)$       | $\{123678, 127, 235789, 25679\}$                                  |
| 9531:72   | $0, 0, 0, 0, e^{12}, e^{13}, e^{25}, e^{34} + e^{16}, e^{27} + e^{36}$          | $1/69(30, 22, 33, 60, 52, 63, 74, 93, 96)$           | $\{\emptyset, 135789, 15679, 368\}$                               |
| 9531:74   | $0, 0, 0, 0, e^{12}, e^{13}, e^{15}, e^{16}, e^{24} + e^{17}$                   | $1/17(4, 11, 13, 12, 15, 17, 19, 21, 23)$            | $\{\emptyset, 123478, 12467, 134589, 14569, 2356789, 2579, 368\}$ |
| 9531:76   | $0, 0, 0, 0, e^{12}, e^{34}, e^{15}, e^{36}, e^{17} + e^{23}$                   | $1/33(4, 27, 12, 21, 31, 33, 35, 45, 39)$            | $\{124678, 127, 145689, 159, 2345789, 235679, 348, 36\}$          |
| 9531:77   | $0, 0, 0, 0, e^{12}, e^{34}, e^{15}, e^{36}, e^{17} + e^{24}$                   | $1/39(8, 27, 14, 24, 35, 38, 43, 52, 51)$            | $\{\emptyset, 123478, 124678, 134589, 145689, 235679, 2579, 36\}$ |
| 9531:78   | $0, 0, 0, 0, e^{12}, e^{14} + e^{23}, e^{15}, e^{13} + e^{25}, e^{17} + e^{24}$ | $77/753(3, 4, 8, 9, 7, 12, 10, 11, 13)$              | $\{123478, 23579\}$                                               |
| 9531:80   | $0, 0, 0, 0, e^{12}, e^{13}, e^{15}, e^{24} + e^{16}, e^{17} + e^{34}$          | $1/57(14, 36, 43, 35, 50, 57, 64, 71, 78)$           | $\{\emptyset, 2356789, 24579, 3468\}$                             |
| 9531:81   | $0, 0, 0, 0, e^{12}, e^{13}, e^{25}, e^{24} + e^{16}, e^{34} + e^{27}$          | $2/81(14, 15, 23, 36, 29, 37, 44, 51, 59)$           | $\{123478, 1267, 135789, 145679\}$                                |
| 9531:82   | $0, 0, 0, 0, e^{12}, e^{13}, e^{15}, e^{14} + e^{36}, e^{24} + e^{17}$          | $1/79(24, 43, 36, 72, 67, 60, 91, 96, 115)$          | $\{123478, 124678, 134589, 145689\}$                              |
| 9531:83   | $0, 0, 0, 0, e^{12}, e^{13}, e^{15}, e^{16} + e^{34}, e^{17} + e^{24}$          | $(0, 1, 1, 0, 1, 1, 1, 1, 1)$                        | $\{123678, 127, 135689, 159\}$                                    |
| 9531:84   | $0, 0, 0, 0, e^{12}, e^{13}, e^{25}, e^{16} + e^{34}, e^{27} + e^{14}$          | $1/111(48, 32, 63, 96, 80, 111, 112, 159, 144)$      | $\{12378, 1267, 235689, 259\}$                                    |
| 9531:85   | $0, 0, 0, 0, e^{12}, e^{13}, e^{25}, e^{24} + e^{36}, e^{14} + e^{27}$          | $1/60(28, 19, 24, 57, 47, 52, 66, 76, 85)$           | $\{123478, 124678, 135789, 156789\}$                              |
| 9531:91   | $0, 0, 0, 0, e^{12}, e^{13}, e^{25}, e^{16} + e^{23}, e^{34} + e^{27}$          | $1/46(10, 20, 33, 37, 30, 43, 50, 53, 70)$           | $\{123478, 1267, 235689, 2459\}$                                  |
| 9531:92   | $0, 0, 0, 0, e^{12}, e^{13}, e^{15}, e^{14} + e^{36}, e^{23} + e^{17}$          | $1/232(42, 169, 126, 252, 211, 168, 253, 294, 295)$  | $\{123478, 134589, 24579, 4\}$                                    |
| 9531:94   | $0, 0, 0, 0, e^{12}, e^{13}, e^{15}, e^{36} + e^{24}, e^{17} + e^{23}$          | $1/53(11, 34, 33, 43, 45, 44, 56, 77, 67)$           | $\{\emptyset, 12378, 134589, 24579\}$                             |
| 9531:95   | $0, 0, 0, 0, e^{12}, e^{34}, e^{15}, e^{36} + e^{25}, e^{17}$                   | $1/84(18, 51, 32, 56, 69, 88, 87, 120, 105)$         | $\{\emptyset, 123478, 124678, 134589, 145689, 235679, 2579, 36\}$ |
| 9531:98a  | $0, 0, 0, 0, e^{12}, e^{13}, e^{15}, e^{25} + e^{36}, e^{17} + e^{34}$          | $4/179(12, 25, 25, 36, 37, 37, 49, 62, 61)$          | $\{\emptyset, 123478, 12678, 13589, 145689, 235679, 24579, 346\}$ |
| 9531:98b  | $0, 0, 0, 0, -e^{12}, e^{13}, e^{15}, e^{36} + e^{25}, e^{17} + e^{34}$         | $4/179(12, 25, 25, 36, 37, 37, 49, 62, 61)$          | $\{\emptyset, 123478, 12678, 13589, 145689, 235679, 24579, 346\}$ |
| 9531:100  | $0, 0, 0, 0, e^{12}, e^{13}, e^{25}, e^{15} + e^{36}, e^{27} + e^{34}$          | $1/279(151, 73, 112, 258, 224, 263, 297, 375, 370)$  | $\{\emptyset, 123478, 12678, 346\}$                               |
| 9531:102a | $0, 0, 0, 0, e^{12}, e^{13}, e^{15}, e^{25} + e^{36} + e^{14}, e^{17}$          | $1/157(36, 89, 89, 178, 125, 125, 161, 214, 197)$    | $\{123478, 124678, 134589, 145689, 2345679, 24579, 346, 4\}$      |
| 9531:102b | $0, 0, 0, 0, -e^{12}, e^{13}, e^{15}, e^{14} + e^{36} + e^{25}, e^{17}$         | $1/157(36, 89, 89, 178, 125, 125, 161, 214, 197)$    | $\{123478, 124678, 134589, 145689, 2345679, 24579, 346, 4\}$      |
| 9531:104  | $0, 0, 0, 0, e^{12}, e^{13}, e^{15}, e^{34} + e^{25} + e^{16}, e^{17}$          | $1/25(7, 13, 19, 14, 20, 26, 27, 33, 34)$            | $\{123678, 135689, 25679, 6\}$                                    |
| 9531:105  | $0, 0, 0, 0, e^{12}, e^{13}, e^{25}, e^{15} + e^{24} + e^{36}, e^{27}$          | $1/211(112, 54, 83, 224, 166, 195, 220, 278, 274)$   | $\{123478, 124678, 346, 4\}$                                      |
| 9531:107  | $0, 0, 0, 0, e^{12}, e^{13}, e^{25}, e^{36}, e^{34} + e^{16} + e^{27}$          | $1/681(333, 202, 273, 666, 535, 606, 737, 879, 939)$ | $\{\emptyset, 12678, 135789, 23569\}$                             |
| 9531:108  | $0, 0, 0, 0, e^{12}, e^{13}, e^{15}, e^{16} + e^{24}, e^{17} + e^{36}$          | $2/107(17, 28, 31, 37, 45, 48, 62, 65, 79)$          | $\{1359, 145689, 36, 48\}$                                        |
| 9531:109  | $0, 0, 0, 0, e^{12}, e^{13}, e^{25}, e^{16} + e^{24}, e^{27} + e^{36}$          | $1/41(16, 14, 21, 39, 30, 37, 44, 53, 58)$           | $\{\emptyset, 1345789, 15679, 3468\}$                             |
| 9531:110  | $0, 0, 0, 0, e^{12}, e^{13}, e^{25}, e^{36} + e^{14}, e^{27} + e^{16}$          | $5/33(3, 2, 3, 6, 5, 6, 7, 9, 9)$                    | $\{\emptyset, 12678, 135789, 23569\}$                             |
| 9531:112  | $0, 0, 0, 0, e^{12}, e^{34}, e^{15}, e^{13} + e^{46}, e^{36} + e^{17}$          | $1/47(14, 29, 32, 7, 43, 39, 57, 46, 71)$            | $\{123678, 127, 134589, 14569\}$                                  |
| 9531:113  | $0, 0, 0, 0, e^{12}, e^{34}, e^{15}, e^{23} + e^{46}, e^{36} + e^{17}$          | $1/417(86, 312, 207, 156, 398, 363, 484, 519, 570)$  | $\{123678, 127, 2345789, 245679\}$                                |
| 9531:114  | $0, 0, 0, 0, e^{12}, e^{13}, e^{15}, e^{34} + e^{25}, e^{17} + e^{36}$          | $1/271(75, 148, 149, 222, 223, 224, 298, 371, 373)$  | $\{\emptyset, 13589, 145689, 346\}$                               |
| 9531:115  | $0, 0, 0, 0, e^{12}, e^{13}, e^{25}, e^{15} + e^{34}, e^{36} + e^{27}$          | $3/79(13, 8, 12, 22, 21, 25, 29, 34, 37)$            | $\{\emptyset, 134579, 15679, 346\}$                               |
| 9531:126  | $0, 0, 0, 0, e^{12}, e^{13}, e^{15}, e^{16} + e^{23}, e^{17} + e^{24}$          | $1/11(3, 6, 8, 9, 9, 11, 12, 14, 15)$                | $\{\emptyset, 134589, 14569, 368\}$                               |

Table A.2 – Continued to next page

Table A.2 – Continued from previous page

| Name      | $g$                                                                              | $N$                                                  | Signatures $S$                                                    |
|-----------|----------------------------------------------------------------------------------|------------------------------------------------------|-------------------------------------------------------------------|
| 9531:128  | $0, 0, 0, 0, e^{12}, e^{13}, e^{15}, e^{16} + e^{24}, e^{17} + e^{23}$           | $3/449(39, 82, 117, 113, 121, 156, 160, 195, 199)$   | $\{\emptyset, 12378, 134589, 24579\}$                             |
| 9531:129  | $0, 0, 0, 0, e^{12}, e^{34}, e^{15}, e^{13} + e^{46}, e^{23} + e^{17}$           | $1/29(8, 17, 24, 4, 25, 28, 33, 32, 41)$             | $\{123478, 123678, 134589, 135689\}$                              |
| 9531:130  | $0, 0, 0, 0, e^{12}, e^{34}, e^{15}, e^{36} + e^{14}, e^{23} + e^{17}$           | $(0, 1, 0, 1, 1, 1, 1, 1)$                           | $\{124678, 127, 145689, 159\}$                                    |
| 9531:131  | $0, 0, 0, 0, e^{12}, e^{34}, e^{15}, e^{24} + e^{36}, e^{23} + e^{17}$           | $1/129(17, 102, 51, 78, 119, 129, 136, 180, 153)$    | $\{145689, 159, 348, 36\}$                                        |
| 9531:132  | $0, 0, 0, 0, e^{12}, e^{34}, e^{15}, e^{25}, e^{17} + e^{36}$                    | $1/84(27, 39, 32, 56, 66, 88, 93, 105, 120)$         | $\{\emptyset, 123678, 1278, 134589, 145689, 234579, 245679, 36\}$ |
| 9531:136  | $0, 0, 0, 0, e^{12}, e^{13}, e^{15}, e^{25} + e^{16}, e^{17} + e^{34}$           | $1/557(169, 275, 381, 401, 444, 550, 613, 719, 782)$ | $\{\emptyset, 123478, 13589, 24579\}$                             |
| 9531:137a | $0, 0, 0, 0, e^{12}, e^{13}, e^{15}, e^{36} + e^{25}, e^{17} + e^{24}$           | $4/179(12, 25, 25, 36, 37, 37, 49, 62, 61)$          | $\{\emptyset, 123478, 124678, 134589, 145689, 235679, 2579, 36\}$ |
| 9531:137b | $0, 0, 0, 0, -e^{12}, e^{13}, e^{15}, e^{25} + e^{36}, e^{17} + e^{24}$          | $4/179(12, 25, 25, 36, 37, 37, 49, 62, 61)$          | $\{\emptyset, 123478, 124678, 134589, 145689, 235679, 2579, 36\}$ |
| 9531:139  | $0, 0, 0, 0, e^{12}, e^{13}, e^{25}, e^{36} + e^{15}, e^{27} + e^{14}$           | $4/249(32, 18, 25, 54, 50, 57, 68, 82, 86)$          | $\{135789, 156789, 234569, 2459\}$                                |
| 9531:141  | $0, 0, 0, 0, e^{12}, e^{13}, e^{15}, e^{16}, e^{24} + e^{36} + e^{17}$           | $1/199(53, 130, 118, 159, 183, 171, 236, 224, 289)$  | $\{\emptyset, 134589, 14569, 368\}$                               |
| 9531:142  | $0, 0, 0, 0, e^{12}, e^{13}, e^{25}, e^{16}, e^{27} + e^{36} + e^{14}$           | $1/111(42, 38, 57, 114, 80, 99, 118, 141, 156)$      | $\{1345789, 145679, 3468, 4\}$                                    |
| 9531:143  | $0, 0, 0, 0, e^{12}, e^{34}, e^{15}, e^{36}, e^{17} + e^{46} + e^{23}$           | $1/87(13, 72, 39, 36, 85, 75, 98, 114, 111)$         | $\{124678, 127, 2345789, 235679\}$                                |
| 9531:145  | $0, 0, 0, 0, e^{12}, e^{13}, e^{15}, e^{14} + e^{25}, e^{36} + e^{17}$           | $1/53(16, 26, 29, 52, 42, 45, 58, 68, 74)$           | $\{\emptyset, 13589, 15689, 36\}$                                 |
| 9531:146  | $0, 0, 0, 0, e^{12}, e^{13}, e^{25}, e^{15} + e^{24}, e^{27} + e^{36}$           | $1/141(64, 46, 69, 128, 110, 133, 156, 174, 202)$    | $\{\emptyset, 13579, 15679, 36\}$                                 |
| 9531:147  | $0, 0, 0, 0, e^{12}, e^{13}, e^{25}, e^{15} + e^{34}, e^{16} + e^{27}$           | $4/683(79, 56, 89, 125, 135, 168, 191, 214, 247)$    | $\{1267, 135789, 234569, 48\}$                                    |
| 9531:148  | $0, 0, 0, 0, e^{12}, e^{13}, e^{15}, e^{36}, e^{34} + e^{17} + e^{25}$           | $1/57(16, 32, 29, 51, 48, 45, 64, 74, 80)$           | $\{\emptyset, 13589, 145689, 346\}$                               |
| 9531:149  | $0, 0, 0, 0, e^{12}, e^{13}, e^{25}, e^{36}, e^{34} + e^{27} + e^{15}$           | $1/41(22, 11, 16, 39, 33, 38, 44, 54, 55)$           | $\{\emptyset, 23569, 2459, 346\}$                                 |
| 9531:150  | $0, 0, 0, 0, e^{12}, e^{13}, e^{15}, e^{14} + e^{36}, e^{17} + e^{25}$           | $1/561(152, 304, 291, 582, 456, 443, 608, 734, 760)$ | $\{134589, 145689, 346, 4\}$                                      |
| 9531:151  | $0, 0, 0, 0, e^{12}, e^{13}, e^{15}, e^{34} + e^{16}, e^{25} + e^{17}$           | $1/61(17, 34, 44, 34, 51, 61, 68, 78, 85)$           | $\{135689, 159, 38, 6\}$                                          |
| 9531:152  | $0, 0, 0, 0, e^{12}, e^{13}, e^{15}, e^{24} + e^{36}, e^{25} + e^{17}$           | $2/579(77, 154, 166, 255, 231, 243, 308, 409, 385)$  | $\{\emptyset, 134589, 145689, 36\}$                               |
| 9531:154  | $0, 0, 0, 0, e^{12}, e^{13}, e^{25}, e^{16} + e^{34}, e^{15} + e^{27}$           | $1/79(38, 19, 41, 76, 57, 79, 76, 117, 95)$          | $\{123589, 12569, 138, 16\}$                                      |
| 9531:155  | $0, 0, 0, 0, e^{12}, e^{13}, e^{25}, e^{24} + e^{36}, e^{15} + e^{27}$           | $1/72(38, 19, 28, 75, 57, 66, 76, 94, 95)$           | $\{23569, 259, 346, 4\}$                                          |
| 9531:156  | $0, 0, 0, 0, e^{12}, e^{34}, e^{15}, e^{46} + e^{13} + e^{25}, e^{17}$           | $1/61(18, 28, 56, 9, 46, 65, 64, 74, 82)$            | $\{123478, 123678, 134589, 135689\}$                              |
| 9531:161a | $0, 0, 0, 0, e^{12}, e^{13}, e^{15}, e^{14} + e^{25} + e^{36}, e^{17} + e^{34}$  | $24/151(2, 3, 3, 6, 5, 5, 7, 8, 9)$                  | $\{123478, 145689, 24579, 346\}$                                  |
| 9531:161b | $0, 0, 0, 0, -e^{12}, e^{13}, e^{15}, e^{14} + e^{36} + e^{25}, e^{17} + e^{34}$ | $24/151(2, 3, 3, 6, 5, 5, 7, 8, 9)$                  | $\{123478, 145689, 24579, 346\}$                                  |
| 9531:163  | $0, 0, 0, 0, e^{12}, e^{13}, e^{25}, e^{24} + e^{36} + e^{15}, e^{34} + e^{27}$  | $7/71(5, 3, 4, 10, 8, 9, 11, 13, 14)$                | $\{123478, 346\}$                                                 |
| 9531:165  | $0, 0, 0, 0, e^{12}, e^{13}, e^{15}, e^{34} + e^{16}, e^{17} + e^{36} + e^{24}$  | $1/19(0, 22, 11, 0, 22, 11, 22, 11, 22)$             | $\{123678, 127\}$                                                 |
| 9531:168  | $0, 0, 0, 0, e^{12}, e^{13}, e^{25}, e^{24} + e^{36}, e^{16} + e^{34} + e^{27}$  | $7/71(5, 3, 4, 10, 8, 9, 11, 13, 14)$                | $\{135789, 23569\}$                                               |
| 9531:169  | $0, 0, 0, 0, e^{12}, e^{34}, e^{15}, e^{36} + e^{25}, e^{46} + e^{17}$           | $8/87(3, 6, 5, 5, 9, 10, 12, 15, 15)$                | $\{\emptyset, 124678, 134589, 235679\}$                           |
| 9531:186  | $0, 0, 0, 0, e^{12}, e^{13}, e^{15}, e^{34} + e^{25} + e^{16}, e^{36} + e^{17}$  | $67/589(3, 4, 5, 6, 7, 8, 10, 11, 13)$               | $\{123678, 25679\}$                                               |
| 9531:196  | $0, 0, 0, 0, e^{12}, e^{13}, e^{15}, e^{16} + e^{25}, e^{24} + e^{17}$           | $5/19(1, 2, 3, 3, 3, 4, 4, 5, 5)$                    | $\{\emptyset, 123478, 134589, 2579\}$                             |
| 9531:200  | $0, 0, 0, 0, e^{12}, e^{13}, e^{15}, e^{25}, e^{17} + e^{36} + e^{24}$           | $14/659(15, 22, 26, 45, 37, 41, 52, 59, 67)$         | $\{\emptyset, 134589, 145689, 36\}$                               |
| 9531:201  | $0, 0, 0, 0, e^{12}, e^{13}, e^{25}, e^{15}, e^{27} + e^{36} + e^{14}$           | $7/701(42, 34, 51, 102, 76, 93, 110, 118, 144)$      | $\{134579, 145679, 346, 4\}$                                      |
| 9531:202  | $0, 0, 0, 0, e^{12}, e^{13}, e^{25}, e^{15}, e^{16} + e^{34} + e^{27}$           | $7/139(8, 7, 13, 16, 15, 21, 22, 23, 29)$            | $\{\emptyset, 12678, 13579, 235689\}$                             |
| 9531:205  | $0, 0, 0, 0, e^{12}, e^{13}, e^{25}, e^{16}, e^{34} + e^{15} + e^{27}$           | $2/133(34, 17, 29, 56, 51, 63, 68, 97, 85)$          | $\{123589, 124569, 1348, 16\}$                                    |
| 9531:206  | $0, 0, 0, 0, e^{12}, e^{13}, e^{15}, e^{24} + e^{16}, e^{25} + e^{17}$           | $2/77(10, 20, 31, 31, 30, 41, 40, 51, 50)$           | $\{\emptyset, 134589, 1569, 3468\}$                               |
| 9531:207  | $0, 0, 0, 0, e^{12}, e^{13}, e^{25}, e^{16} + e^{24}, e^{27} + e^{15}$           | $4/17(2, 1, 2, 5, 3, 4, 4, 6, 5)$                    | $\{1234589, 12569, 138, 146\}$                                    |
| 9531:208  | $0, 0, 0, 0, e^{12}, e^{34}, e^{15}, e^{36} + e^{25}, e^{17} + e^{23}$           | $1/207(31, 141, 93, 127, 172, 220, 203, 313, 234)$   | $\{124678, 145689, 235679, 36\}$                                  |
| 9531:209a | $0, 0, 0, 0, e^{12}, e^{34}, e^{15}, e^{25} + e^{36}, e^{24} + e^{17}$           | $4/73(4, 11, 7, 12, 15, 19, 19, 26, 23)$             | $\{\emptyset, 123478, 124678, 134589, 145689, 235679, 2579, 36\}$ |
| 9531:209b | $0, 0, 0, 0, e^{12}, e^{34}, -e^{15}, e^{36} + e^{25}, e^{17} + e^{24}$          | $4/73(4, 11, 7, 12, 15, 19, 19, 26, 23)$             | $\{\emptyset, 123478, 124678, 134589, 145689, 235679, 2579, 36\}$ |
| 9531:210  | $0, 0, 0, 0, e^{12}, e^{34}, e^{15}, e^{13} + e^{25}, e^{17} + e^{36}$           | $1/61(27, 16, 32, 33, 43, 65, 70, 59, 97)$           | $\{123678, 134589, 234579, 36\}$                                  |
| 9531:211  | $0, 0, 0, 0, e^{12}, e^{34}, e^{15}, e^{25} + e^{13}, e^{46} + e^{17}$           | $1/207(74, 80, 160, 71, 154, 231, 228, 234, 302)$    | $\{134589, 135689, 234579, 235679\}$                              |
| 9531:212  | $0, 0, 0, 0, e^{12}, e^{34}, e^{15}, e^{13} + e^{46}, e^{17} + e^{25}$           | $1/223(62, 124, 192, 31, 186, 223, 248, 254, 310)$   | $\{134589, 135689, 14569, 159\}$                                  |
| 9531:214a | $0, 0, 0, 0, e^{12}, e^{13}, e^{15}, e^{36} + e^{25} + e^{14}, e^{17} + e^{24}$  | $24/151(2, 3, 3, 6, 5, 5, 7, 8, 9)$                  | $\{123478, 124678, 134589, 145689\}$                              |
| 9531:214b | $0, 0, 0, 0, -e^{12}, e^{13}, e^{15}, e^{25} + e^{36} + e^{14}, e^{17} + e^{24}$ | $24/151(2, 3, 3, 6, 5, 5, 7, 8, 9)$                  | $\{123478, 124678, 134589, 145689\}$                              |
| 9531:216  | $0, 0, 0, 0, e^{12}, e^{13}, e^{15}, e^{16} + e^{34} + e^{25}, e^{17} + e^{24}$  | $1/8(0, 5, 10, 0, 5, 10, 5, 10, 5)$                  | $\{123678, 135689\}$                                              |
| 9531:217  | $0, 0, 0, 0, e^{12}, e^{13}, e^{25}, e^{36} + e^{15} + e^{24}, e^{27} + e^{14}$  | $16/203(6, 4, 5, 12, 10, 11, 14, 16, 18)$            | $\{135789, 156789\}$                                              |

Table A.2 – Continued to next page

Table A.2 – Continued from previous page

| Name      | $g$                                                                              | $N$                                         | Signatures $S$                                                    |
|-----------|----------------------------------------------------------------------------------|---------------------------------------------|-------------------------------------------------------------------|
| 9531:218  | $0, 0, 0, 0, e^{12}, e^{13}, e^{25}, e^{24} + e^{16}, e^{36} + e^{27} + e^{14}$  | $31/379(5, 4, 6, 12, 9, 11, 13, 16, 17)$    | $\{1345789, 3468\}$                                               |
| 9531:227a | $0, 0, 0, 0, e^{12}, e^{13}, e^{15}, e^{14} + e^{36} + e^{25}, e^{23} + e^{17}$  | $39/197(1, 3, 3, 6, 4, 4, 5, 7, 6)$         | $\{124678, 145689, 2345679, 346\}$                                |
| 9531:227b | $0, 0, 0, 0, -e^{12}, e^{13}, e^{15}, e^{36} + e^{25} + e^{14}, e^{23} + e^{17}$ | $39/197(1, 3, 3, 6, 4, 4, 5, 7, 6)$         | $\{124678, 145689, 2345679, 346\}$                                |
| 9531:230a | $0, 0, 0, 0, e^{12}, e^{13}, e^{15}, e^{16} + e^{23}, e^{17} + e^{36} + e^{24}$  | $9/31(1, 2, 2, 3, 3, 3, 4, 4, 5)$           | $\{\emptyset, 134589, 14569, 368\}$                               |
| 9531:230b | $0, 0, 0, 0, -e^{12}, e^{13}, e^{15}, e^{16} + e^{23}, e^{17} + e^{24} + e^{36}$ | $9/31(1, 2, 2, 3, 3, 3, 4, 4, 5)$           | $\{\emptyset, 134589, 14569, 368\}$                               |
| 9531:232  | $0, 0, 0, 0, e^{12}, e^{13}, e^{15}, e^{25} + e^{34}, e^{24} + e^{36} + e^{17}$  | $14/51(1, 2, 2, 3, 3, 3, 4, 5, 5)$          | $\{13589, 346\}$                                                  |
| 9531:233  | $0, 0, 0, 0, e^{12}, e^{13}, e^{25}, e^{34} + e^{15}, e^{27} + e^{36} + e^{14}$  | $21/289(7, 4, 6, 12, 11, 13, 15, 18, 19)$   | $\{134579, 346\}$                                                 |
| 9531:234  | $0, 0, 0, 0, e^{12}, e^{13}, e^{15}, e^{14} + e^{36}, e^{25} + e^{17} + e^{34}$  | $81/853(3, 6, 5, 10, 9, 8, 12, 13, 15)$     | $\{145689, 346\}$                                                 |
| 9531:235  | $0, 0, 0, 0, e^{12}, e^{13}, e^{15}, e^{36} + e^{24}, e^{17} + e^{25} + e^{34}$  | $14/51(1, 2, 2, 3, 3, 3, 4, 5, 5)$          | $\{\emptyset, 145689\}$                                           |
| 9531:236  | $0, 0, 0, 0, e^{12}, e^{13}, e^{25}, e^{36} + e^{14}, e^{15} + e^{27} + e^{34}$  | $87/997(6, 3, 5, 10, 9, 11, 12, 16, 15)$    | $\{\emptyset, 23569\}$                                            |
| 9531:237  | $0, 0, 0, 0, e^{12}, e^{13}, e^{25}, e^{24} + e^{36}, e^{15} + e^{34} + e^{27}$  | $21/232(6, 3, 4, 11, 9, 10, 12, 14, 15)$    | $\{23569, 346\}$                                                  |
| 9531:238  | $0, 0, 0, 0, e^{12}, e^{34}, e^{15}, e^{13} + e^{46}, e^{17} + e^{24} + e^{36}$  | $1/19(0, 22, 11, 0, 22, 11, 22, 11, 22)$    | $\{123678, 127\}$                                                 |
| 9531:239a | $0, 0, 0, 0, e^{12}, e^{34}, e^{15}, e^{46} + e^{23}, e^{24} + e^{36} + e^{17}$  | $26/183(1, 6, 3, 3, 7, 6, 8, 9, 9)$         | $\{123678, 127, 2345789, 245679\}$                                |
| 9531:239b | $0, 0, 0, 0, e^{12}, e^{34}, e^{15}, e^{46} - e^{23}, e^{24} + e^{36} + e^{17}$  | $26/183(1, 6, 3, 3, 7, 6, 8, 9, 9)$         | $\{123678, 127, 2345789, 245679\}$                                |
| 9531:240  | $0, 0, 0, 0, e^{12}, e^{34}, e^{15}, e^{36}, e^{25} + e^{17} + e^{46}$           | $1/21(6, 12, 8, 11, 18, 19, 24, 27, 30)$    | $\{\emptyset, 134589, 13569, 468\}$                               |
| 9531:250  | $0, 0, 0, 0, e^{12}, e^{13}, e^{25}, e^{36} + e^{15}, e^{27} + e^{34} + e^{16}$  | $7/71(5, 3, 4, 10, 8, 9, 11, 13, 14)$       | $\{135789, 23569\}$                                               |
| 9531:253  | $0, 0, 0, 0, e^{12}, e^{13}, e^{25}, e^{36} + e^{15} + e^{24}, e^{27} + e^{16}$  | $7/71(5, 3, 4, 10, 8, 9, 11, 13, 14)$       | $\{1345789, 234569\}$                                             |
| 9531:255  | $0, 0, 0, 0, e^{12}, e^{34}, e^{15}, e^{25} + e^{46} + e^{13}, e^{17} + e^{36}$  | $4/59(6, 5, 10, 3, 11, 13, 17, 16, 23)$     | $\{123678, 134589\}$                                              |
| 9531:266  | $0, 0, 0, 0, e^{12}, e^{13}, e^{25}, e^{34} + e^{16}, e^{36} + e^{27} + e^{15}$  | $59/463(4, 2, 3, 8, 6, 7, 8, 11, 10)$       | $\{1234589, 124569\}$                                             |
| 9531:282  | $0, 0, 0, 0, e^{12}, e^{34}, e^{15}, e^{25}, e^{46} + e^{23} + e^{17}$           | $14/53(1, 2, 3, 1, 3, 4, 4, 5, 5)$          | $\{124678, 1278, 234579, 235679\}$                                |
| 9531:283  | $0, 0, 0, 0, e^{12}, e^{13}, e^{15}, e^{25} + e^{14}, e^{24} + e^{36} + e^{17}$  | $49/621(4, 6, 7, 12, 10, 11, 14, 16, 18)$   | $\{\emptyset, 36\}$                                               |
| 9531:286  | $0, 0, 0, 0, e^{12}, e^{13}, e^{15}, e^{16} + e^{24}, e^{17} + e^{25} + e^{34}$  | $7/50(2, 4, 5, 5, 6, 7, 8, 9, 10)$          | $\{\emptyset, 3468\}$                                             |
| 9531:289  | $0, 0, 0, 0, e^{12}, e^{13}, e^{25}, e^{15} + e^{23}, e^{14} + e^{36} + e^{27}$  | $7/71(3, 4, 6, 12, 7, 9, 11, 10, 15)$       | $\{134579, 346\}$                                                 |
| 9531:290  | $0, 0, 0, 0, e^{12}, e^{13}, e^{25}, e^{23} + e^{15}, e^{34} + e^{27} + e^{16}$  | $7/19(1, 1, 2, 2, 2, 3, 3, 4)$              | $\{13579, 235689\}$                                               |
| 9531:292  | $0, 0, 0, 0, e^{12}, e^{13}, e^{25}, e^{23} + e^{16}, e^{34} + e^{27} + e^{15}$  | $1/2(0, 0, 1, -1, 0, 1, 0, 1, 0)$           | $\{123589, 124569\}$                                              |
| 9531:293a | $0, 0, 0, 0, e^{12}, e^{34}, e^{15}, e^{46} + e^{13} + e^{25}, e^{17} + e^{23}$  | $8/53(2, 3, 6, 1, 5, 7, 7, 8, 9)$           | $\{123478, 123678, 134589, 135689\}$                              |
| 9531:293b | $0, 0, 0, 0, e^{12}, e^{34}, -e^{15}, e^{13} + e^{46} + e^{25}, e^{17} + e^{23}$ | $8/53(2, 3, 6, 1, 5, 7, 7, 8, 9)$           | $\{123478, 123678, 134589, 135689\}$                              |
| 9531:294  | $0, 0, 0, 0, e^{12}, e^{34}, e^{15}, e^{25} + e^{36} + e^{14}, e^{17} + e^{23}$  | $1/8(0, 5, 0, 10, 5, 10, 5, 10, 5)$         | $\{124678, 145689\}$                                              |
| 9531:298  | $0, 0, 0, 0, e^{12}, e^{13}, e^{15}, e^{16} + e^{25}, e^{17} + e^{24} + e^{36}$  | $35/317(3, 4, 5, 9, 7, 8, 10, 11, 13)$      | $\{145689, 36\}$                                                  |
| 9531:303  | $0, 0, 0, 0, e^{12}, e^{34}, e^{15}, e^{36} + e^{25}, e^{46} + e^{17} + e^{23}$  | $56/863(3, 10, 9, 5, 13, 14, 16, 23, 19)$   | $\{124678, 235679\}$                                              |
| 9531:313  | $0, 0, 0, 0, e^{12}, e^{13}, e^{25}, e^{24} + e^{16}, e^{27} + e^{36} + e^{15}$  | $1/8(4, 2, 3, 9, 6, 7, 8, 11, 10)$          | $\{1234589, 12569\}$                                              |
| 9531:319  | $0, 0, 0, 0, e^{12}, e^{34}, e^{15}, e^{13} + e^{46}, e^{25} + e^{36} + e^{17}$  | $19/251(4, 8, 9, 2, 12, 11, 16, 13, 20)$    | $\{134589, 14569\}$                                               |
| 9531:368  | $0, 0, 0, 0, e^{12}, e^{34}, e^{15}, e^{13} + e^{25}, e^{17} + e^{23} + e^{46}$  | $49/653(4, 6, 12, 3, 10, 15, 14, 16, 18)$   | $\{234579, 235679\}$                                              |
| 9531:369  | $0, 0, 0, 0, e^{12}, e^{34}, e^{15}, e^{13} + e^{25}, e^{17} + e^{24} + e^{36}$  | $7/17(1, 0, 0, 3, 1, 3, 2, 1, 3)$           | $\{123678, 234579\}$                                              |
| 9531:520a | $0, 0, 0, 0, e^{12}, e^{13}, e^{15}, e^{25}, e^{34} + e^{17} + e^{28}$           | $1/27(10, 10, 19, 21, 20, 29, 30, 30, 40)$  | $\{\emptyset, 123478, 12678, 13589, 145689, 235679, 24579, 346\}$ |
| 9531:520b | $0, 0, 0, 0, e^{12}, e^{13}, -e^{15}, e^{25}, e^{28} + e^{17} + e^{34}$          | $1/27(10, 10, 19, 21, 20, 29, 30, 30, 40)$  | $\{\emptyset, 123478, 12678, 13589, 145689, 235679, 24579, 346\}$ |
| 9531:522a | $0, 0, 0, 0, e^{12}, e^{13} + e^{24}, e^{15}, e^{25}, e^{28} + e^{17}$           | $3/61(7, 7, 18, 18, 14, 25, 21, 21, 28)$    | $\{\emptyset, 123478, 12678, 13589, 145689, 235679, 24579, 346\}$ |
| 9531:522b | $0, 0, 0, 0, e^{12}, e^{13} + e^{24}, -e^{15}, e^{25}, e^{17} + e^{28}$          | $3/61(7, 7, 18, 18, 14, 25, 21, 21, 28)$    | $\{\emptyset, 123478, 12678, 13589, 145689, 235679, 24579, 346\}$ |
| 9531:524a | $0, 0, 0, 0, e^{12}, e^{24} + e^{13}, e^{15}, e^{25}, e^{28} + e^{17} + e^{34}$  | $7/19(1, 1, 2, 2, 2, 3, 3, 4)$              | $\{\emptyset, 123478, 12678, 13589, 145689, 235679, 24579, 346\}$ |
| 9531:524b | $0, 0, 0, 0, e^{12}, e^{24} + e^{13}, -e^{15}, e^{25}, e^{28} + e^{17} + e^{34}$ | $7/19(1, 1, 2, 2, 2, 3, 3, 4)$              | $\{\emptyset, 123478, 12678, 13589, 145689, 235679, 24579, 346\}$ |
| 9531:524c | $0, 0, 0, 0, -e^{12}, e^{24} + e^{13}, e^{15}, e^{25}, e^{34} + e^{28} + e^{17}$ | $7/19(1, 1, 2, 2, 2, 3, 3, 4)$              | $\{\emptyset, 123478, 12678, 13589, 145689, 235679, 24579, 346\}$ |
| 9531:541a | $0, 0, 0, 0, e^{12}, e^{34}, e^{15}, e^{25}, e^{36} + e^{17} + e^{28}$           | $1/24(9, 9, 10, 16, 18, 26, 27, 27, 36)$    | $\{\emptyset, 123678, 1278, 134589, 145689, 234579, 245679, 36\}$ |
| 9531:541b | $0, 0, 0, 0, e^{12}, e^{34}, -e^{15}, e^{25}, e^{28} + e^{36} + e^{17}$          | $1/24(9, 9, 10, 16, 18, 26, 27, 27, 36)$    | $\{\emptyset, 123678, 1278, 134589, 145689, 234579, 245679, 36\}$ |
| 9531:651  | $0, 0, 0, 0, e^{12}, e^{13}, e^{25}, e^{16}, e^{27} + e^{18} + e^{34}$           | $4/249(18, 25, 39, 54, 43, 57, 68, 75, 93)$ | $\{\emptyset, 123478, 145679, 235689\}$                           |
| 9531:652  | $0, 0, 0, 0, e^{12}, e^{13}, e^{25}, e^{36}, e^{14} + e^{38} + e^{27}$           | $2/33(9, 5, 5, 15, 14, 14, 19, 19, 24)$     | $\{\emptyset, 123478, 156789, 234569\}$                           |
| 9531:749  | $0, 0, 0, 0, e^{12}, e^{34}, e^{15}, e^{36}, e^{17} + e^{38}$                    | $1/33(7, 24, 7, 24, 31, 31, 38, 38, 45)$    | $\{\emptyset, 123478, 127, 13569, 145689, 235679, 2456789, 348\}$ |
| 9531:750  | $0, 0, 0, 0, e^{12}, e^{34}, e^{15}, e^{36}, e^{38} + e^{17} + e^{24}$           | $16/69(1, 3, 1, 3, 4, 4, 5, 6)$             | $\{\emptyset, 123478, 145689, 235679\}$                           |

Table A.2 – Continued to next page

Table A.2 – Continued from previous page

| Name     | $g$                                                                             | $N$                                                  | Signatures $S$                                                                                                        |
|----------|---------------------------------------------------------------------------------|------------------------------------------------------|-----------------------------------------------------------------------------------------------------------------------|
| 9531:751 | $0, 0, 0, 0, e^{12}, e^{34}, e^{15}, e^{36}, e^{38} + e^{17} + e^{25}$          | $1/21(6, 12, 5, 15, 18, 20, 24, 25, 30)$             | $\{\emptyset, 13569, 145689, 348\}$                                                                                   |
| 9531:754 | $0, 0, 0, 0, e^{12}, e^{34}, e^{15}, e^{36}, e^{17} + e^{25} + e^{46} + e^{38}$ | $5/17(1, 2, 1, 2, 3, 3, 4, 5)$                       | $\{\emptyset, 13569\}$                                                                                                |
| 9521:1   | $0, 0, 0, 0, e^{12}, e^{13}, e^{34}, e^{15}, e^{18}$                            | $1/11(2, 8, 8, 7, 10, 10, 15, 12, 14)$               | $\{123468, 123678, 12478, 128, 134569, 135679, 14579, 159, 234589, 235789, 2456789, 25689, 34, 37, 467, 6\}$          |
| 9521:2   | $0, 0, 0, 0, e^{12}, e^{13}, e^{34}, e^{25}, e^{28}$                            | $1/33(21, 7, 18, 24, 28, 39, 42, 35, 42)$            | $\{\emptyset, 12348, 12378, 124678, 1268, 134589, 135789, 1456789, 15689, 234569, 235679, 24579, 259, 346, 367, 47\}$ |
| 9521:4   | $0, 0, 0, 0, e^{12}, e^{13}, e^{14}, e^{15}, e^{18}$                            | $1/14(2, 11, 13, 13, 13, 15, 15, 15, 17)$            | $\{\emptyset, 12348, 12378, 12468, 12678, 13459, 13579, 14569, 15679, 23456789, 235689, 245789, 2589, 3467, 36, 47\}$ |
| 9521:5   | $0, 0, 0, 0, e^{12}, e^{13}, e^{14}, e^{25}, e^{28}$                            | $1/39(18, 11, 30, 30, 29, 48, 48, 40, 51)$           | $\{\emptyset, 12348, 12378, 12468, 12678, 134589, 135789, 145689, 156789, 2345679, 23569, 24579, 259, 3467, 36, 47\}$ |
| 9521:6   | $0, 0, 0, 0, e^{12}, e^{13}, e^{24}, e^{15}, e^{18}$                            | $1/27(6, 16, 24, 19, 22, 30, 35, 28, 34)$            | $\{\emptyset, 12348, 12378, 12468, 12678, 134579, 1359, 145679, 1569, 2345689, 2356789, 24589, 25789, 3467, 36, 47\}$ |
| 9521:7   | $0, 0, 0, 0, e^{12}, e^{34}, e^{24} + e^{13}, e^{15}, e^{18}$                   | $1/29(7, 17, 24, 14, 24, 38, 31, 31, 38)$            | $\{123678, 12468, 134579, 159, 234589, 25789, 36, 467\}$                                                              |
| 9521:8   | $0, 0, 0, 0, e^{12}, e^{13}, e^{23}, e^{15}, e^{34} + e^{18}$                   | $1/14(4, 8, 9, 11, 12, 13, 17, 16, 20)$              | $\{123468, 1278, 135679, 1459, 23589, 2456789, 347, 6\}$                                                              |
| 9521:9   | $0, 0, 0, 0, e^{12}, e^{13}, e^{14} + e^{23}, e^{15}, e^{18}$                   | $1/40(10, 22, 29, 41, 32, 39, 51, 42, 52)$           | $\{12368, 12478, 1345679, 159, 234589, 256789, 37, 46\}$                                                              |
| 9521:10  | $0, 0, 0, 0, e^{12}, e^{13}, e^{14} + e^{23}, e^{25}, e^{28}$                   | $1/71(29, 22, 60, 53, 51, 89, 82, 73, 95)$           | $\{12378, 12468, 134589, 156789, 2345679, 259, 36, 47\}$                                                              |
| 9521:11  | $0, 0, 0, 0, e^{12}, e^{13}, e^{34}, e^{15}, e^{23} + e^{18}$                   | $1/71(16, 47, 48, 47, 63, 64, 95, 79, 95)$           | $\{123468, 123678, 134569, 135679, 2456789, 25689, 467, 6\}$                                                          |
| 9521:12  | $0, 0, 0, 0, e^{12}, e^{13}, e^{14}, e^{15}, e^{18} + e^{34}$                   | $1/40(10, 28, 29, 29, 38, 39, 39, 48, 58)$           | $\{1234678, 128, 13569, 14579, 235789, 245689, 34, 67\}$                                                              |
| 9521:13  | $0, 0, 0, 0, e^{12}, e^{13}, e^{14}, e^{25}, e^{28} + e^{34}$                   | $1/48(24, 14, 33, 33, 38, 57, 57, 52, 66)$           | $\{\emptyset, 12348, 12678, 135789, 145689, 23569, 24579, 3467\}$                                                     |
| 9521:14  | $0, 0, 0, 0, e^{12}, e^{13}, e^{24}, e^{15}, e^{18} + e^{34}$                   | $7/81(3, 7, 9, 7, 10, 12, 14, 13, 16)$               | $\{\emptyset, 12348, 12678, 1359, 145679, 2356789, 24589, 3467\}$                                                     |
| 9521:15  | $0, 0, 0, 0, e^{12}, e^{13}, e^{34}, e^{15}, e^{18} + e^{24}$                   | $1/59(12, 41, 43, 36, 53, 55, 79, 65, 77)$           | $\{123468, 12478, 134569, 14579, 235789, 25689, 37, 6\}$                                                              |
| 9521:16  | $0, 0, 0, 0, e^{12}, e^{13}, e^{34}, e^{25}, e^{28} + e^{14}$                   | $1/69(42, 16, 39, 48, 58, 81, 87, 74, 90)$           | $\{\emptyset, 12348, 124678, 135789, 15689, 234569, 24579, 367\}$                                                     |
| 9521:17  | $0, 0, 0, 0, e^{12}, e^{13}, e^{23}, e^{15}, e^{24} + e^{18}$                   | $1/83(24, 42, 61, 72, 66, 85, 103, 90, 114)$         | $\{\emptyset, 12348, 124678, 134579, 14569, 235689, 25789, 367\}$                                                     |
| 9521:18  | $0, 0, 0, 0, e^{12}, e^{13}, e^{14}, e^{15}, e^{23} + e^{18}$                   | $1/63(16, 39, 48, 55, 55, 64, 71, 71, 87)$           | $\{\emptyset, 12348, 12378, 13459, 13579, 245789, 2589, 47\}$                                                         |
| 9521:19  | $0, 0, 0, 0, e^{12}, e^{13}, e^{24}, e^{15}, e^{23} + e^{18}$                   | $1/144(39, 76, 117, 106, 115, 156, 182, 154, 193)$   | $\{\emptyset, 12348, 12378, 134579, 1359, 24589, 25789, 47\}$                                                         |
| 9521:22a | $0, 0, 0, 0, e^{12}, e^{23} + e^{14}, e^{24} + e^{13}, e^{15}, e^{18}$          | $1/64(22, 22, 53, 53, 44, 75, 75, 66, 88)$           | $\{12378, 12468, 1345679, 159, 234589, 256789, 36, 47\}$                                                              |
| 9521:22b | $0, 0, 0, 0, e^{12}, e^{23} - e^{14}, e^{24} + e^{13}, e^{15}, e^{18}$          | $1/64(22, 22, 53, 53, 44, 75, 75, 66, 88)$           | $\{12378, 12468, 1345679, 159, 234589, 256789, 36, 47\}$                                                              |
| 9521:23  | $0, 0, 0, 0, e^{12}, e^{34}, e^{13} + e^{24}, e^{15}, e^{23} + e^{18}$          | $1/121(32, 67, 96, 61, 99, 157, 128, 131, 163)$      | $\{123678, 134579, 25789, 467\}$                                                                                      |
| 9521:24  | $0, 0, 0, 0, e^{12}, e^{13}, e^{34}, e^{15}, e^{18} + e^{25}$                   | $1/139(38, 76, 96, 91, 114, 134, 187, 152, 190)$     | $\{134569, 135679, 14579, 159, 34, 37, 467, 6\}$                                                                      |
| 9521:25  | $0, 0, 0, 0, e^{12}, e^{13}, e^{34}, e^{25}, e^{15} + e^{28}$                   | $1/41(22, 11, 24, 29, 33, 46, 53, 44, 55)$           | $\{\emptyset, 234569, 235679, 24579, 259, 346, 367, 47\}$                                                             |
| 9521:26  | $0, 0, 0, 0, e^{12}, e^{13}, e^{23} + e^{14}, e^{15}, e^{18} + e^{24}$          | $1/159(48, 77, 115, 144, 125, 163, 192, 173, 221)$   | $\{124678, 134579, 25789, 367\}$                                                                                      |
| 9521:29  | $0, 0, 0, 0, e^{12}, e^{13}, e^{14}, e^{15}, e^{25} + e^{18}$                   | $1/112(30, 60, 97, 97, 90, 127, 127, 120, 150)$      | $\{\emptyset, 13459, 13579, 14569, 15679, 3467, 36, 47\}$                                                             |
| 9521:30  | $0, 0, 0, 0, e^{12}, e^{13}, e^{14}, e^{25}, e^{15} + e^{28}$                   | $1/59(30, 15, 44, 44, 45, 74, 74, 60, 75)$           | $\{12348, 12378, 12468, 12678, 134589, 135789, 145689, 156789\}$                                                      |
| 9521:31  | $0, 0, 0, 0, e^{12}, e^{13}, e^{24}, e^{15}, e^{25} + e^{18}$                   | $1/23(6, 12, 20, 17, 18, 26, 29, 24, 30)$            | $\{\emptyset, 134579, 1359, 145679, 1569, 3467, 36, 47\}$                                                             |
| 9521:32  | $0, 0, 0, 0, e^{12}, e^{34}, e^{24} + e^{13}, e^{15}, e^{18} + e^{25}$          | $1/67(18, 36, 53, 35, 54, 88, 71, 72, 90)$           | $\{134579, 159, 36, 467\}$                                                                                            |
| 9521:33  | $0, 0, 0, 0, e^{12}, e^{13}, e^{34}, e^{15}, e^{36} + e^{18}$                   | $1/139(30, 100, 80, 99, 130, 110, 179, 160, 190)$    | $\{123468, 123678, 12478, 128, 234589, 235789, 2456789, 25689\}$                                                      |
| 9521:34  | $0, 0, 0, 0, e^{12}, e^{13}, e^{34}, e^{25}, e^{28} + e^{36}$                   | $1/15(9, 4, 6, 12, 13, 15, 18, 17, 21)$              | $\{\emptyset, 134589, 135789, 1456789, 15689, 346, 367, 47\}$                                                         |
| 9521:38  | $0, 0, 0, 0, e^{12}, e^{13}, e^{14}, e^{15}, e^{25} + e^{18} + e^{34}$          | $27/184(2, 4, 5, 5, 6, 7, 7, 8, 10)$                 | $\{\emptyset, 13579, 14569, 3467\}$                                                                                   |
| 9521:39  | $0, 0, 0, 0, e^{12}, e^{13}, e^{14}, e^{25}, e^{28} + e^{34} + e^{15}$          | $29/216(4, 2, 5, 5, 6, 9, 9, 8, 10)$                 | $\{12348, 12678, 135789, 145689\}$                                                                                    |
| 9521:40  | $0, 0, 0, 0, e^{12}, e^{13}, e^{24}, e^{15}, e^{25} + e^{18} + e^{34}$          | $4/57(4, 8, 11, 9, 12, 15, 17, 16, 20)$              | $\{\emptyset, 1359, 145679, 3467\}$                                                                                   |
| 9521:43  | $0, 0, 0, 0, e^{12}, e^{13}, e^{14}, e^{15}, e^{18} + e^{36}$                   | $1/144(30, 110, 85, 129, 140, 115, 159, 170, 200)$   | $\{\emptyset, 13459, 13579, 14569, 15679, 3467, 36, 47\}$                                                             |
| 9521:44  | $0, 0, 0, 0, e^{12}, e^{13}, e^{14}, e^{25}, e^{28} + e^{36}$                   | $1/204(90, 70, 105, 159, 160, 195, 249, 230, 300)$   | $\{\emptyset, 134589, 135789, 145689, 156789, 3467, 36, 47\}$                                                         |
| 9521:45  | $0, 0, 0, 0, e^{12}, e^{13}, e^{24}, e^{15}, e^{18} + e^{36}$                   | $1/7(2, 4, 4, 5, 6, 6, 7, 8, 10)$                    | $\{\emptyset, 134579, 1359, 145679, 1569, 3467, 36, 47\}$                                                             |
| 9521:46  | $0, 0, 0, 0, e^{12}, e^{13}, e^{24}, e^{25}, e^{28} + e^{36}$                   | $1/7(4, 2, 3, 6, 6, 7, 8, 8, 10)$                    | $\{\emptyset, 1345789, 13589, 1456789, 15689, 3467, 36, 47\}$                                                         |
| 9521:47  | $0, 0, 0, 0, e^{12}, e^{13}, e^{34}, e^{25}, e^{16} + e^{28}$                   | $1/204(93, 67, 108, 150, 160, 201, 258, 227, 294)$   | $\{\emptyset, 124678, 1268, 134589, 135789, 234569, 235679, 47\}$                                                     |
| 9521:52  | $0, 0, 0, 0, e^{12}, e^{13}, e^{14}, e^{25}, e^{16} + e^{28}$                   | $1/69(24, 25, 51, 57, 49, 75, 81, 74, 99)$           | $\{\emptyset, 12468, 12678, 134589, 135789, 2345679, 23569, 47\}$                                                     |
| 9521:53  | $0, 0, 0, 0, e^{12}, e^{13}, e^{24}, e^{25}, e^{16} + e^{28}$                   | $1/317(123, 112, 213, 261, 235, 336, 373, 347, 459)$ | $\{\emptyset, 12468, 12678, 1345789, 13589, 234569, 235679, 47\}$                                                     |

Table A.2 – Continued to next page

Table A.2 – Continued from previous page

| Name      | $g$                                                                              | $N$                                                   | Signatures $S$                                                    |
|-----------|----------------------------------------------------------------------------------|-------------------------------------------------------|-------------------------------------------------------------------|
| 9521:56a  | $0, 0, 0, 0, e^{12}, e^{23} + e^{14}, e^{24} + e^{13}, e^{15}, e^{18} + e^{25}$  | $(0, 0, 1, 1, 0, 1, 1, 0, 0)$                         | $\{123579, 124569, 234, 267\}$                                    |
| 9521:56b  | $0, 0, 0, 0, e^{12}, e^{23} - e^{14}, e^{24} + e^{13}, e^{15}, e^{25} + e^{18}$  | $(0, 0, 1, 1, 0, 1, 1, 0, 0)$                         | $\{123579, 124569, 234, 267\}$                                    |
| 9521:57   | $0, 0, 0, 0, e^{12}, e^{34}, e^{13}, e^{15}, e^{36} + e^{18}$                    | $1/17(5, 11, 8, 10, 16, 18, 13, 21, 26)$              | $\{123678, 128, 134579, 14569, 234589, 2456789, 36, 7\}$          |
| 9521:58   | $0, 0, 0, 0, e^{12}, e^{34}, e^{13}, e^{25}, e^{28} + e^{36}$                    | $1/57(39, 14, 21, 39, 53, 60, 60, 67, 81)$            | $\{\emptyset, 12368, 1278, 134589, 1456789, 234579, 24569, 367\}$ |
| 9521:59   | $0, 0, 0, 0, e^{12}, e^{34}, e^{13}, e^{15}, e^{18} + e^{46}$                    | $1/57(14, 40, 40, 21, 54, 61, 54, 68, 82)$            | $\{12468, 128, 134579, 135679, 234589, 235689, 467, 7\}$          |
| 9521:60   | $0, 0, 0, 0, e^{12}, e^{34}, e^{13}, e^{25}, e^{28} + e^{46}$                    | $1/18(11, 5, 10, 8, 16, 18, 21, 21, 26)$              | $\{\emptyset, 124678, 1278, 134589, 135689, 234579, 235679, 46\}$ |
| 9521:61   | $0, 0, 0, 0, e^{12}, e^{13}, e^{14} + e^{23}, e^{15}, e^{18} + e^{36}$           | $1/72(18, 46, 41, 69, 64, 59, 87, 82, 100)$           | $\{\emptyset, 13579, 14569, 3467\}$                               |
| 9521:62   | $0, 0, 0, 0, e^{12}, e^{13}, e^{14} + e^{23}, e^{25}, e^{28} + e^{36}$           | $1/167(53, 70, 105, 122, 123, 158, 175, 193, 263)$    | $\{134589, 156789, 36, 47\}$                                      |
| 9521:63   | $0, 0, 0, 0, e^{12}, e^{13}, e^{34}, e^{15}, e^{36} + e^{18} + e^{24}$           | $1/247(57, 172, 143, 171, 229, 200, 314, 286, 343)$   | $\{123468, 12478, 235789, 25689\}$                                |
| 9521:71   | $0, 0, 0, 0, e^{12}, e^{13}, e^{14} + e^{23}, e^{25}, e^{28} + e^{16}$           | $21/569(9, 10, 21, 22, 19, 30, 31, 29, 39)$           | $\{12468, 134589, 2345679, 47\}$                                  |
| 9521:72   | $0, 0, 0, 0, e^{12}, e^{13}, e^{14}, e^{15}, e^{18} + e^{36} + e^{24}$           | $1/15(4, 10, 9, 12, 14, 13, 16, 18, 22)$              | $\{\emptyset, 13459, 14569, 36\}$                                 |
| 9521:73   | $0, 0, 0, 0, e^{12}, e^{13}, e^{14}, e^{25}, e^{16} + e^{28} + e^{34}$           | $1/39(15, 14, 27, 30, 29, 42, 45, 43, 57)$            | $\{\emptyset, 12678, 135789, 23569\}$                             |
| 9521:75   | $0, 0, 0, 0, e^{12}, e^{13}, e^{24}, e^{25}, e^{16} + e^{34} + e^{28}$           | $7/139(8, 7, 13, 16, 15, 21, 23, 22, 29)$             | $\{\emptyset, 12678, 13589, 235679\}$                             |
| 9521:76   | $0, 0, 0, 0, e^{12}, e^{13}, e^{23}, e^{15}, e^{24} + e^{36} + e^{18}$           | $1/81(24, 46, 47, 72, 70, 71, 93, 94, 118)$           | $\{\emptyset, 134579, 14569, 367\}$                               |
| 9521:77   | $0, 0, 0, 0, e^{12}, e^{13}, e^{23}, e^{25}, e^{28} + e^{36} + e^{14}$           | $1/47(23, 16, 24, 48, 39, 47, 40, 55, 71)$            | $\{134589, 1456789, 346, 47\}$                                    |
| 9521:78   | $0, 0, 0, 0, e^{12}, e^{13}, e^{23}, e^{25}, e^{16} + e^{28} + e^{34}$           | $1/163(71, 58, 103, 142, 129, 174, 161, 187, 245)$    | $\{1268, 13589, 235679, 7\}$                                      |
| 9521:79   | $0, 0, 0, 0, e^{12}, e^{34}, e^{24} + e^{13}, e^{15}, e^{18} + e^{36}$           | $1/14(5, 7, 8, 6, 12, 14, 13, 17, 22)$                | $\{123678, 134579, 234589, 36\}$                                  |
| 9521:80   | $0, 0, 0, 0, e^{12}, e^{34}, e^{14} + e^{23}, e^{15}, e^{18} + e^{36}$           | $1/81(21, 53, 28, 60, 74, 88, 81, 95, 116)$           | $\{12368, 134579, 234589, 367\}$                                  |
| 9521:85   | $0, 0, 0, 0, e^{12}, e^{13}, e^{34}, e^{25}, e^{28} + e^{36} + e^{15}$           | $1/113(64, 32, 48, 89, 96, 112, 137, 128, 160)$       | $\{\emptyset, 346, 367, 47\}$                                     |
| 9521:92   | $0, 0, 0, 0, e^{12}, e^{34}, e^{13}, e^{15}, e^{46} + e^{23} + e^{18}$           | $1/657(156, 470, 468, 235, 626, 703, 624, 782, 938)$  | $\{12468, 128, 234589, 235689\}$                                  |
| 9521:93   | $0, 0, 0, 0, e^{12}, e^{34}, e^{13}, e^{15}, e^{24} + e^{36} + e^{18}$           | $1/13(3, 10, 5, 9, 13, 14, 8, 16, 19)$                | $\{123678, 128, 234589, 2456789\}$                                |
| 9521:94   | $0, 0, 0, 0, e^{12}, e^{34}, e^{13}, e^{25}, e^{28} + e^{36} + e^{14}$           | $13/111(6, 2, 3, 6, 8, 9, 9, 10, 12)$                 | $\{12368, 1278, 134589, 1456789\}$                                |
| 9521:95   | $0, 0, 0, 0, e^{12}, e^{13}, e^{14} + e^{23}, e^{15}, e^{36} + e^{24} + e^{18}$  | $9/31(1, 2, 2, 3, 3, 3, 4, 5)$                        | $\{\emptyset, 14569\}$                                            |
| 9521:100a | $0, 0, 0, 0, e^{12}, e^{13}, e^{14}, e^{15}, e^{36} + e^{18} + e^{25}$           | $1/137(40, 80, 80, 117, 120, 120, 157, 160, 200)$     | $\{\emptyset, 13459, 13579, 14569, 15679, 3467, 36, 47\}$         |
| 9521:100b | $0, 0, 0, 0, -e^{12}, e^{13}, e^{14}, e^{15}, e^{25} + e^{36} + e^{18}$          | $1/137(40, 80, 80, 117, 120, 120, 157, 160, 200)$     | $\{\emptyset, 13459, 13579, 14569, 15679, 3467, 36, 47\}$         |
| 9521:102  | $0, 0, 0, 0, e^{12}, e^{13}, e^{14}, e^{25}, e^{36} + e^{15} + e^{28}$           | $1/143(80, 40, 60, 103, 120, 140, 183, 160, 200)$     | $\{134589, 135789, 145689, 156789\}$                              |
| 9521:108  | $0, 0, 0, 0, e^{12}, e^{13}, e^{34}, e^{15}, e^{18} + e^{47} + e^{36}$           | $1/681(178, 476, 416, 297, 654, 594, 713, 832, 1010)$ | $\{12478, 128, 234589, 235789\}$                                  |
| 9521:109  | $0, 0, 0, 0, e^{12}, e^{13}, e^{34}, e^{25}, e^{47} + e^{28} + e^{36}$           | $4/183(27, 14, 21, 24, 41, 48, 45, 55, 69)$           | $\{\emptyset, 134589, 135789, 47\}$                               |
| 9521:116  | $0, 0, 0, 0, e^{12}, e^{34}, e^{24} + e^{13}, e^{15}, e^{46} + e^{18} + e^{23}$  | $91/1089(3, 8, 9, 4, 11, 13, 12, 14, 17)$             | $\{12468, 234589\}$                                               |
| 9521:117  | $0, 0, 0, 0, e^{12}, e^{34}, e^{13}, e^{15}, e^{25} + e^{36} + e^{18}$           | $1/91(28, 56, 43, 54, 84, 97, 71, 112, 140)$          | $\{134579, 14569, 36, 7\}$                                        |
| 9521:119  | $0, 0, 0, 0, e^{12}, e^{34}, e^{13}, e^{15}, e^{25} + e^{18} + e^{46}$           | $1/681(202, 404, 464, 273, 606, 737, 666, 808, 1010)$ | $\{134579, 135679, 467, 7\}$                                      |
| 9521:120  | $0, 0, 0, 0, e^{12}, e^{34}, e^{13}, e^{25}, e^{28} + e^{46} + e^{15}$           | $4/233(34, 17, 33, 26, 51, 59, 67, 68, 85)$           | $\{\emptyset, 234579, 235679, 46\}$                               |
| 9521:121  | $0, 0, 0, 0, e^{12}, e^{13}, e^{34}, e^{25}, e^{28} + e^{37} + e^{16}$           | $1/60(33, 19, 24, 42, 52, 57, 66, 71, 90)$            | $\{\emptyset, 1268, 134589, 234569\}$                             |
| 9521:122a | $0, 0, 0, 0, e^{12}, e^{13}, e^{34}, e^{25}, e^{16} + e^{28} + e^{47}$           | $4/81(10, 7, 11, 10, 17, 21, 21, 24, 31)$             | $\{\emptyset, 124678, 1268, 134589, 135789, 234569, 235679, 47\}$ |
| 9521:122b | $0, 0, 0, 0, e^{12}, -e^{13}, e^{34}, e^{25}, e^{47} + e^{16} + e^{28}$          | $4/81(10, 7, 11, 10, 17, 21, 21, 24, 31)$             | $\{\emptyset, 124678, 1268, 134589, 135789, 234569, 235679, 47\}$ |
| 9521:126a | $0, 0, 0, 0, e^{12}, e^{13}, e^{14}, e^{25}, e^{47} + e^{36} + e^{28}$           | $1/21(9, 8, 12, 12, 17, 21, 21, 25, 33)$              | $\{\emptyset, 134589, 135789, 145689, 156789, 3467, 36, 47\}$     |
| 9521:126b | $0, 0, 0, 0, e^{12}, -e^{13}, e^{14}, e^{25}, e^{28} + e^{47} + e^{36}$          | $1/21(9, 8, 12, 12, 17, 21, 21, 25, 33)$              | $\{\emptyset, 134589, 135789, 145689, 156789, 3467, 36, 47\}$     |
| 9521:128  | $0, 0, 0, 0, e^{12}, e^{13}, e^{24}, e^{15}, e^{47} + e^{36} + e^{18}$           | $1/43(14, 24, 26, 21, 38, 40, 45, 52, 66)$            | $\{\emptyset, 3467, 36, 47\}$                                     |
| 9521:129a | $0, 0, 0, 0, e^{12}, e^{13}, e^{23} + e^{14}, e^{15}, e^{18} + e^{36} + e^{25}$  | $9/31(1, 2, 2, 3, 3, 3, 4, 5)$                        | $\{\emptyset, 13579, 14569, 3467\}$                               |
| 9521:129b | $0, 0, 0, 0, -e^{12}, e^{13}, e^{14} + e^{23}, e^{15}, e^{25} + e^{18} + e^{36}$ | $9/31(1, 2, 2, 3, 3, 3, 4, 5)$                        | $\{\emptyset, 13579, 14569, 3467\}$                               |
| 9521:131  | $0, 0, 0, 0, e^{12}, e^{13}, e^{23} + e^{14}, e^{25}, e^{15} + e^{28} + e^{36}$  | $23/152(4, 2, 3, 1, 6, 7, 5, 8, 10)$                  | $\{123579, 124569\}$                                              |
| 9521:145  | $0, 0, 0, 0, e^{12}, e^{13}, e^{14}, e^{25}, e^{28} + e^{17} + e^{36}$           | $4/21(2, 2, 3, 4, 5, 6, 6, 8)$                        | $\{\emptyset, 134589, 145689, 36\}$                               |
| 9521:146  | $0, 0, 0, 0, e^{12}, e^{13}, e^{24}, e^{15}, e^{18} + e^{36} + e^{27}$           | $8/151(7, 8, 11, 13, 15, 18, 21, 22, 29)$             | $\{\emptyset, 134579, 145679, 36\}$                               |
| 9521:147  | $0, 0, 0, 0, e^{12}, e^{34}, e^{13} + e^{24}, e^{15}, e^{36} + e^{25} + e^{18}$  | $4/13(1, 2, 2, 1, 3, 3, 3, 4, 5)$                     | $\{123678, 234589\}$                                              |
| 9521:148  | $0, 0, 0, 0, e^{12}, e^{34}, e^{14} + e^{23}, e^{15}, e^{36} + e^{25} + e^{18}$  | $7/71(3, 6, 4, 7, 9, 11, 10, 12, 15)$                 | $\{134579, 367\}$                                                 |
| 9521:178  | $0, 0, 0, 0, e^{12}, e^{13}, e^{34}, e^{25}, e^{15} + e^{28} + e^{47} + e^{36}$  | $10/133(8, 4, 6, 7, 12, 14, 13, 16, 20)$              | $\{134589, 135789\}$                                              |
| 9521:191a | $0, 0, 0, 0, e^{12}, e^{13}, e^{14}, e^{15}, e^{18} + e^{36} + e^{25} + e^{47}$  | $25/81(1, 2, 2, 2, 3, 3, 3, 4, 5)$                    | $\{123489, 123789, 124689, 126789, 2345678, 23568, 24578, 258\}$  |

Table A.2 – Continued to next page

Table A.2 – Continued from previous page

| Name      | $g$                                                                              | $N$                                                  | Signatures $S$                                                    |
|-----------|----------------------------------------------------------------------------------|------------------------------------------------------|-------------------------------------------------------------------|
| 9521:191b | $0, 0, 0, 0, e^{12}, -e^{13}, e^{14}, e^{15}, e^{18} + e^{25} + e^{36} + e^{47}$ | $25/81(1, 2, 2, 2, 3, 3, 3, 4, 5)$                   | $\{123489, 123789, 124689, 126789, 2345678, 23568, 24578, 258\}$  |
| 9521:191c | $0, 0, 0, 0, -e^{12}, e^{13}, e^{14}, e^{15}, e^{25} + e^{47} + e^{36} + e^{18}$ | $25/81(1, 2, 2, 2, 3, 3, 3, 4, 5)$                   | $\{123489, 123789, 124689, 126789, 2345678, 23568, 24578, 258\}$  |
| 9521:194a | $0, 0, 0, 0, e^{12}, e^{13}, e^{14}, e^{25}, e^{47} + e^{36} + e^{15} + e^{28}$  | $25/168(4, 2, 3, 6, 7, 7, 8, 10)$                    | $\{134589, 135789, 145689, 156789\}$                              |
| 9521:194b | $0, 0, 0, 0, e^{12}, -e^{13}, e^{14}, e^{25}, e^{28} + e^{47} + e^{36} + e^{15}$ | $25/168(4, 2, 3, 6, 7, 7, 8, 10)$                    | $\{134589, 135789, 145689, 156789\}$                              |
| 964:1     | $0, 0, 0, e^{12}, e^{13}, e^{14}, e^{24}, e^{15}, e^{35}$                        | $1/41(13, 20, 20, 33, 33, 46, 53, 46, 53)$           | $\{\emptyset, 1236789, 125679, 134789, 14579, 234568, 246, 358\}$ |
| 964:2     | $0, 0, 0, e^{12}, e^{13}, e^{14}, e^{24}, e^{35}, e^{15} + e^{23}$               | $1/67(18, 36, 35, 54, 53, 72, 90, 88, 71)$           | $\{1236789, 125678, 234569, 246\}$                                |
| 953:6     | $0, 0, 0, 0, e^{12}, e^{13}, e^{15}, e^{25}, e^{16} + e^{24}$                    | $1/23(7, 11, 17, 20, 18, 24, 25, 29, 31)$            | $\{\emptyset, 123789, 124678, 134589, 1568, 235679, 2457, 3469\}$ |
| 953:7     | $0, 0, 0, 0, e^{12}, e^{13}, e^{15}, e^{25}, e^{14} + e^{36}$                    | $1/317(114, 145, 156, 312, 259, 270, 373, 404, 426)$ | $\{\emptyset, 123789, 126789, 13589, 15689, 23567, 257, 36\}$     |
| 953:8     | $0, 0, 0, 0, e^{12}, e^{13}, e^{15}, e^{25}, e^{34} + e^{16}$                    | $1/11(4, 5, 7, 8, 9, 11, 13, 14, 15)$                | $\{\emptyset, 123789, 12678, 13589, 1568, 235679, 257, 369\}$     |
| 953:9     | $0, 0, 0, 0, e^{12}, e^{13}, e^{15}, e^{25}, e^{24} + e^{36}$                    | $1/16(6, 7, 8, 15, 13, 14, 19, 20, 22)$              | $\{\emptyset, 123789, 126789, 134589, 145689, 234567, 2457, 36\}$ |
| 953:10    | $0, 0, 0, 0, e^{12}, e^{13}, e^{15}, e^{25} + e^{14}, e^{16}$                    | $1/37(10, 19, 27, 38, 29, 37, 39, 48, 47)$           | $\{1234789, 124678, 134589, 14568, 2345679, 2457, 3469, 4\}$      |
| 953:12    | $0, 0, 0, 0, e^{12}, e^{13}, e^{15}, e^{25} + e^{14}, e^{36}$                    | $1/69(24, 33, 34, 66, 57, 58, 81, 90, 92)$           | $\{\emptyset, 123789, 126789, 13589, 15689, 23567, 257, 36\}$     |
| 953:13    | $0, 0, 0, 0, e^{12}, e^{13}, e^{25}, e^{15} + e^{24}, e^{36}$                    | $1/111(48, 45, 50, 96, 93, 98, 138, 141, 148)$       | $\{\emptyset, 123789, 126789, 13579, 15679, 23568, 258, 36\}$     |
| 953:14    | $0, 0, 0, 0, e^{12}, e^{13}, e^{15}, e^{34} + e^{25}, e^{16}$                    | $1/14(4, 8, 9, 11, 12, 13, 16, 20, 17)$              | $\{\emptyset, 123789, 124678, 13589, 14568, 2345679, 257, 3469\}$ |
| 953:15    | $0, 0, 0, 0, e^{12}, e^{13}, e^{25}, e^{15} + e^{34}, e^{16}$                    | $1/139(53, 67, 73, 100, 120, 126, 187, 173, 179)$    | $\{123479, 1267, 135789, 145678, 234569, 25, 3689, 48\}$          |
| 953:16    | $0, 0, 0, 0, e^{12}, e^{13}, e^{15}, e^{25} + e^{34}, e^{36}$                    | $1/41(15, 20, 19, 36, 35, 34, 50, 55, 53)$           | $\{\emptyset, 123789, 1246789, 13589, 145689, 234567, 257, 346\}$ |
| 953:17    | $0, 0, 0, 0, e^{12}, e^{13}, e^{25}, e^{34} + e^{15}, e^{36}$                    | $3/7(1, 1, 2, 2, 3, 3, 3)$                           | $\{\emptyset, 123789, 1246789, 134579, 15679, 23568, 2458, 346\}$ |
| 953:24    | $0, 0, 0, 0, e^{12}, e^{13}, e^{15}, e^{25} + e^{14}, e^{16} + e^{24}$           | $1/22(7, 10, 16, 20, 17, 23, 24, 27, 30)$            | $\{124678, 134589, 2457, 3469\}$                                  |
| 953:26    | $0, 0, 0, 0, e^{12}, e^{13}, e^{15}, e^{14} + e^{25}, e^{24} + e^{36}$           | $2/127(23, 29, 32, 58, 52, 55, 75, 81, 87)$          | $\{\emptyset, 123789, 126789, 36\}$                               |
| 953:29    | $0, 0, 0, 0, e^{12}, e^{13}, e^{15}, e^{25} + e^{34}, e^{24} + e^{16}$           | $1/26(8, 14, 17, 19, 22, 25, 30, 36, 33)$            | $\{\emptyset, 123789, 124678, 3469\}$                             |
| 953:30a   | $0, 0, 0, 0, e^{12}, e^{13}, e^{25}, e^{34} + e^{15}, e^{24} + e^{16}$           | $1/8(3, 4, 4, 6, 7, 7, 11, 10, 10)$                  | $\{123479, 1267, 135789, 145678, 234569, 25, 3689, 48\}$          |
| 953:30b   | $0, 0, 0, 0, -e^{12}, e^{13}, e^{25}, e^{34} + e^{15}, e^{16} + e^{24}$          | $1/8(3, 4, 4, 6, 7, 7, 11, 10, 10)$                  | $\{123479, 1267, 135789, 145678, 234569, 25, 3689, 48\}$          |
| 953:31    | $0, 0, 0, 0, e^{12}, e^{13}, e^{15}, e^{25} + e^{34}, e^{36} + e^{14}$           | $9/241(10, 13, 12, 24, 23, 22, 33, 36, 34)$          | $\{1246789, 145689, 234567, 346\}$                                |
| 953:32    | $0, 0, 0, 0, e^{12}, e^{13}, e^{15}, e^{25} + e^{34}, e^{36} + e^{24}$           | $2/59(11, 14, 14, 25, 25, 25, 36, 39, 39)$           | $\{\emptyset, 123789, 145689, 234567\}$                           |
| 953:36a   | $0, 0, 0, 0, e^{12}, e^{13}, e^{24} + e^{15}, e^{25} + e^{14}, e^{36}$           | $2/57(12, 12, 13, 24, 24, 25, 36, 36, 38)$           | $\{\emptyset, 123789, 126789, 13589, 15689, 23567, 257, 36\}$     |
| 953:36b   | $0, 0, 0, 0, e^{12}, e^{13}, -e^{15} + e^{24}, e^{25} + e^{14}, e^{36}$          | $2/57(12, 12, 13, 24, 24, 25, 36, 36, 38)$           | $\{\emptyset, 123789, 126789, 13589, 15689, 23567, 257, 36\}$     |
| 953:37    | $0, 0, 0, 0, e^{12}, e^{13}, e^{25} + e^{14}, e^{34} + e^{15}, e^{16}$           | $1/122(53, 50, 56, 100, 103, 109, 153, 156, 162)$    | $\{123479, 145678, 234569, 48\}$                                  |
| 953:38    | $0, 0, 0, 0, e^{12}, e^{13}, e^{15} + e^{24}, e^{25} + e^{34}, e^{16}$           | $1/37(13, 18, 23, 26, 31, 36, 44, 49, 49)$           | $\{12468, 145678, 234569, 34679\}$                                |
| 953:40    | $0, 0, 0, 0, e^{12}, e^{13}, e^{15} + e^{24}, e^{34} + e^{25}, e^{36}$           | $1/67(28, 29, 30, 56, 57, 58, 85, 86, 88)$           | $\{\emptyset, 123789, 13589, 257\}$                               |
| 953:41    | $0, 0, 0, 0, e^{12}, e^{13}, e^{25}, e^{15} + e^{23}, e^{16} + e^{24}$           | $2/83(14, 19, 28, 37, 33, 42, 52, 47, 56)$           | $\{\emptyset, 124678, 1567, 2458\}$                               |
| 953:42    | $0, 0, 0, 0, e^{12}, e^{13}, e^{25}, e^{23} + e^{15}, e^{14} + e^{36}$           | $1/67(18, 35, 36, 72, 53, 54, 88, 71, 90)$           | $\{1234789, 134579, 234568, 346\}$                                |
| 953:43    | $0, 0, 0, 0, e^{12}, e^{13}, e^{25}, e^{15} + e^{23}, e^{34} + e^{16}$           | $1/85(29, 40, 58, 58, 69, 87, 109, 98, 116)$         | $\{123789, 13579, 235689, 369\}$                                  |
| 953:44    | $0, 0, 0, 0, e^{12}, e^{13}, e^{25}, e^{15} + e^{23}, e^{36} + e^{24}$           | $1/14(4, 7, 8, 13, 11, 12, 18, 15, 20)$              | $\{123789, 134579, 234568, 36\}$                                  |
| 953:45    | $0, 0, 0, 0, e^{12}, e^{13}, e^{15}, e^{14} + e^{25}, e^{16} + e^{23}$           | $1/73(19, 38, 54, 76, 57, 73, 76, 95, 92)$           | $\{1234789, 124678, 2345679, 2457\}$                              |
| 953:46    | $0, 0, 0, 0, e^{12}, e^{13}, e^{25}, e^{15} + e^{24}, e^{16} + e^{23}$           | $1/61(17, 34, 44, 34, 51, 61, 85, 68, 78)$           | $\{123589, 12568, 236789, 278\}$                                  |
| 953:48    | $0, 0, 0, 0, e^{12}, e^{13}, e^{25}, e^{15} + e^{34}, e^{23} + e^{16}$           | $2/101(15, 30, 29, 31, 45, 44, 75, 60, 59)$          | $\{123479, 1267, 234569, 25\}$                                    |
| 953:49    | $0, 0, 0, 0, e^{12}, e^{13}, e^{15} + e^{23}, e^{14} + e^{25}, e^{16}$           | $1/53(17, 26, 34, 52, 43, 51, 60, 69, 68)$           | $\{\emptyset, 12678, 1568, 257\}$                                 |
| 953:50    | $0, 0, 0, 0, e^{12}, e^{13}, e^{23} + e^{15}, e^{14} + e^{25}, e^{36}$           | $1/47(13, 24, 26, 48, 37, 39, 50, 61, 65)$           | $\{1234789, 134589, 234567, 346\}$                                |
| 953:51    | $0, 0, 0, 0, e^{12}, e^{13}, e^{15} + e^{23}, e^{34} + e^{25}, e^{16}$           | $1/199(61, 110, 122, 159, 171, 183, 232, 281, 244)$  | $\{\emptyset, 124678, 14568, 257\}$                               |
| 953:52    | $0, 0, 0, 0, e^{12}, e^{13}, e^{15} + e^{23}, e^{25} + e^{34}, e^{36}$           | $1/71(19, 40, 38, 61, 59, 57, 78, 99, 95)$           | $\{123789, 13589, 234567, 346\}$                                  |
| 953:63a   | $0, 0, 0, 0, e^{12}, e^{13}, e^{15}, e^{16}, e^{36} + e^{25} + e^{14}$           | $1/13(4, 7, 7, 14, 11, 11, 15, 15, 18)$              | $\{1234789, 124679, 134589, 14569, 2345678, 2457, 3468, 4\}$      |
| 953:63b   | $0, 0, 0, 0, -e^{12}, e^{13}, e^{15}, e^{16}, e^{25} + e^{36} + e^{14}$          | $1/13(4, 7, 7, 14, 11, 11, 15, 15, 18)$              | $\{1234789, 124679, 134589, 14569, 2345678, 2457, 3468, 4\}$      |
| 953:65    | $0, 0, 0, 0, e^{12}, e^{13}, e^{25}, e^{16}, e^{15} + e^{24} + e^{36}$           | $1/67(28, 30, 29, 56, 58, 57, 88, 85, 86)$           | $\{1345789, 145679, 234568, 245\}$                                |
| 953:72    | $0, 0, 0, 0, e^{12}, e^{13}, e^{15}, e^{36} + e^{14}, e^{25} + e^{16}$           | $1/53(20, 23, 26, 52, 43, 46, 63, 72, 66)$           | $\{126789, 15689, 23567, 36\}$                                    |
| 953:78    | $0, 0, 0, 0, e^{12}, e^{13}, e^{25}, e^{16} + e^{34}, e^{15} + e^{36}$           | $1/67(28, 30, 29, 56, 58, 57, 88, 85, 86)$           | $\{\emptyset, 123789, 12679, 368\}$                               |
| 953:86a   | $0, 0, 0, 0, e^{12}, e^{13}, e^{25} + e^{14}, e^{15} + e^{34}, e^{16} + e^{24}$  | $3/7(1, 1, 1, 2, 2, 2, 3, 3, 3)$                     | $\{123479, 145678, 234569, 48\}$                                  |
| 953:86b   | $0, 0, 0, 0, -e^{12}, e^{13}, e^{25} + e^{14}, e^{34} + e^{15}, e^{24} + e^{16}$ | $3/7(1, 1, 1, 2, 2, 2, 3, 3, 3)$                     | $\{123479, 145678, 234569, 48\}$                                  |

Table A.2 – Continued to next page



Table A.2 – Continued from previous page

| Name     | $g$                                                                              | $N$                                                 | Signatures $S$                                                                                                        |
|----------|----------------------------------------------------------------------------------|-----------------------------------------------------|-----------------------------------------------------------------------------------------------------------------------|
| 953:89   | $0, 0, 0, 0, e^{12}, e^{13}, e^{23} + e^{15}, e^{25} + e^{14}, e^{16} + e^{24}$  | $7/62(3, 4, 6, 8, 7, 9, 10, 11, 12)$                | $\{124678, 2457\}$                                                                                                    |
| 953:90a  | $0, 0, 0, 0, e^{12}, e^{13}, e^{15} + e^{23}, e^{25} + e^{14}, e^{16} + e^{34}$  | $7/19(1, 1, 2, 2, 2, 3, 3, 4)$                      | $\{123478, 13458, 234567, 346\}$                                                                                      |
| 953:90b  | $0, 0, 0, 0, -e^{12}, e^{13}, e^{15} + e^{23}, e^{14} + e^{25}, e^{16} + e^{34}$ | $7/19(1, 1, 2, 2, 2, 3, 3, 4)$                      | $\{123478, 13458, 234567, 346\}$                                                                                      |
| 953:91   | $0, 0, 0, 0, e^{12}, e^{13}, e^{15} + e^{23}, e^{25} + e^{14}, e^{36} + e^{24}$  | $8/83(3, 5, 6, 10, 8, 9, 11, 13, 15)$               | $\{134589, 234567\}$                                                                                                  |
| 953:92   | $0, 0, 0, 0, e^{12}, e^{13}, e^{23} + e^{15}, e^{25} + e^{34}, e^{24} + e^{16}$  | $37/349(3, 5, 6, 7, 8, 9, 11, 13, 12)$              | $\{\emptyset, 124678\}$                                                                                               |
| 953:93   | $0, 0, 0, 0, e^{12}, e^{13}, e^{23} + e^{15}, e^{25} + e^{34}, e^{14} + e^{36}$  | $21/173(2, 5, 4, 8, 7, 6, 9, 12, 10)$               | $\{234567, 346\}$                                                                                                     |
| 953:94   | $0, 0, 0, 0, e^{12}, e^{13}, e^{15} + e^{23}, e^{34} + e^{25}, e^{24} + e^{36}$  | $14/51(1, 2, 2, 3, 3, 4, 5, 5)$                     | $\{123789, 234567\}$                                                                                                  |
| 953:95a  | $0, 0, 0, 0, e^{12}, e^{13}, e^{15} + e^{24}, e^{25} + e^{14}, e^{23} + e^{16}$  | $(0, 0, 1, 0, 0, 1, 0, 0, 1)$                       | $\{123579, 12567, 236789, 278\}$                                                                                      |
| 953:95b  | $0, 0, 0, 0, e^{12}, e^{13}, -e^{15} + e^{24}, e^{14} + e^{25}, e^{16} + e^{23}$ | $(0, 0, 1, 0, 0, 1, 0, 0, 1)$                       | $\{123579, 12567, 236789, 278\}$                                                                                      |
| 953:96   | $0, 0, 0, 0, e^{12}, e^{13}, e^{25} + e^{14}, e^{15} + e^{34}, e^{16} + e^{23}$  | $11/38(1, 2, 0, 4, 3, 1, 5, 4, 2)$                  | $\{123479, 234569\}$                                                                                                  |
| 953:97   | $0, 0, 0, 0, e^{12}, e^{13}, e^{15} + e^{24}, e^{34} + e^{25}, e^{16} + e^{23}$  | $29/109(1, 2, 3, 2, 3, 4, 4, 5, 5)$                 | $\{123579, 278\}$                                                                                                     |
| 953:107a | $0, 0, 0, 0, e^{12}, e^{13}, e^{15}, e^{14} + e^{36}, e^{25} + e^{34} + e^{16}$  | $3/7(1, 1, 1, 2, 2, 2, 3, 3, 3)$                    | $\{1246789, 145689, 234567, 346\}$                                                                                    |
| 953:107b | $0, 0, 0, 0, e^{12}, e^{13}, e^{15}, e^{36} - e^{14}, e^{34} + e^{25} + e^{16}$  | $3/7(1, 1, 1, 2, 2, 2, 3, 3, 3)$                    | $\{1246789, 145689, 234567, 346\}$                                                                                    |
| 953:111  | $0, 0, 0, 0, e^{12}, e^{13}, e^{15}, e^{24} + e^{36}, e^{16} + e^{25} + e^{34}$  | $3/7(1, 1, 1, 2, 2, 2, 3, 3, 3)$                    | $\{1246789, 346\}$                                                                                                    |
| 953:130a | $0, 0, 0, 0, e^{12}, e^{13}, e^{15}, e^{16} + e^{23}, e^{25} + e^{36} + e^{14}$  | $7/25(1, 2, 2, 4, 3, 3, 4, 4, 5)$                   | $\{1234789, 124679, 2345678, 2457\}$                                                                                  |
| 953:130b | $0, 0, 0, 0, -e^{12}, e^{13}, e^{15}, e^{16} + e^{23}, e^{14} + e^{36} + e^{25}$ | $7/25(1, 2, 2, 4, 3, 3, 4, 4, 5)$                   | $\{1234789, 124679, 2345678, 2457\}$                                                                                  |
| 953:132  | $0, 0, 0, 0, e^{12}, e^{13}, e^{25}, e^{23} + e^{16}, e^{36} + e^{15} + e^{24}$  | $49/319(2, 4, 3, 4, 6, 5, 10, 7, 8)$                | $\{123589, 12569\}$                                                                                                   |
| 953:136  | $0, 0, 0, 0, e^{12}, e^{13}, e^{15} + e^{23}, e^{36} + e^{14}, e^{25} + e^{16}$  | $53/367(2, 3, 4, 8, 5, 6, 7, 10, 8)$                | $\{234567, 346\}$                                                                                                     |
| 953:137  | $0, 0, 0, 0, e^{12}, e^{13}, e^{15} + e^{23}, e^{24} + e^{36}, e^{16} + e^{25}$  | $13/88(2, 3, 4, 7, 5, 6, 7, 10, 8)$                 | $\{23567, 346\}$                                                                                                      |
| 953:198  | $0, 0, 0, 0, e^{12}, e^{34}, e^{15}, e^{13} + e^{25}, e^{36}$                    | $1/9(5, 2, 4, 5, 7, 9, 12, 9, 13)$                  | $\{1234789, 123678, 134589, 13568, 234579, 23567, 349, 36\}$                                                          |
| 953:199  | $0, 0, 0, 0, e^{12}, e^{34}, e^{15}, e^{25}, e^{13} + e^{46}$                    | $1/13(6, 5, 10, 3, 11, 13, 17, 16, 16)$             | $\{1234789, 1236789, 124678, 1278, 134589, 135689, 14568, 158\}$                                                      |
| 953:200  | $0, 0, 0, 0, e^{12}, e^{34}, e^{15}, e^{13} + e^{25}, e^{46}$                    | $1/33(15, 12, 24, 10, 27, 34, 42, 39, 44)$          | $\{1234789, 1236789, 134589, 135689, 234579, 235679, 349, 369\}$                                                      |
| 953:201  | $0, 0, 0, 0, e^{12}, e^{34}, e^{15}, e^{36}, e^{46} + e^{25}$                    | $1/33(13, 16, 13, 16, 29, 29, 42, 42, 45)$          | $\{\emptyset, 1234789, 123679, 134589, 13569, 245678, 257, 468\}$                                                     |
| 953:203a | $0, 0, 0, 0, e^{12}, e^{34}, e^{15} + e^{23}, e^{13} + e^{25}, e^{36}$           | $1/3(1, 1, 2, 1, 2, 3, 3, 3, 5)$                    | $\{1234789, 123678, 134589, 13568, 234579, 23567, 349, 36\}$                                                          |
| 953:203b | $0, 0, 0, 0, e^{12}, e^{34}, e^{23} - e^{15}, e^{25} + e^{13}, e^{36}$           | $1/3(1, 1, 2, 1, 2, 3, 3, 3, 5)$                    | $\{1234789, 123678, 134589, 13568, 234579, 23567, 349, 36\}$                                                          |
| 953:204  | $0, 0, 0, 0, e^{12}, e^{34}, e^{15}, e^{25} + e^{13}, e^{36} + e^{14}$           | $1/19(12, 3, 6, 13, 15, 19, 27, 18, 25)$            | $\{1234789, 123678, 134589, 13568\}$                                                                                  |
| 953:205  | $0, 0, 0, 0, e^{12}, e^{34}, e^{15}, e^{13} + e^{25}, e^{23} + e^{46}$           | $1/107(45, 44, 88, 22, 89, 110, 134, 133, 132)$     | $\{1234789, 1236789, 234579, 235679\}$                                                                                |
| 953:206  | $0, 0, 0, 0, e^{12}, e^{34}, e^{15}, e^{13} + e^{25}, e^{24} + e^{36}$           | $1/7(5, 0, 0, 7, 5, 7, 10, 5, 7)$                   | $\{1234789, 123678, 234579, 23567\}$                                                                                  |
| 953:207a | $0, 0, 0, 0, e^{12}, e^{34}, e^{15} + e^{23}, e^{13} + e^{25}, e^{46}$           | $2/15(3, 3, 6, 2, 6, 8, 9, 10)$                     | $\{1234789, 1236789, 134589, 135689, 234579, 235679, 349, 369\}$                                                      |
| 953:207b | $0, 0, 0, 0, e^{12}, e^{34}, e^{23} - e^{15}, e^{13} + e^{25}, e^{46}$           | $2/15(3, 3, 6, 2, 6, 8, 9, 10)$                     | $\{1234789, 1236789, 134589, 135689, 234579, 235679, 349, 369\}$                                                      |
| 953:208  | $0, 0, 0, 0, e^{12}, e^{34}, e^{15} + e^{23}, e^{25} + e^{14}, e^{36}$           | $1/5(1, 2, 2, 4, 3, 6, 4, 5, 8)$                    | $\{1234789, 134589, 234579, 349\}$                                                                                    |
| 953:209  | $0, 0, 0, 0, e^{12}, e^{34}, e^{15}, e^{36}, e^{46} + e^{13} + e^{25}$           | $13/47(2, 1, 2, 1, 3, 3, 5, 4)$                     | $\{1234789, 123679, 134589, 13569\}$                                                                                  |
| 953:210  | $0, 0, 0, 0, e^{12}, e^{34}, e^{13} + e^{25}, e^{36}, e^{15} + e^{46}$           | $1/223(129, 52, 104, 103, 181, 207, 233, 311, 310)$ | $\{1234789, 123679, 234589, 23569\}$                                                                                  |
| 953:211  | $0, 0, 0, 0, e^{12}, e^{34}, e^{15}, e^{46} + e^{23}, e^{25} + e^{36}$           | $1/131(46, 72, 77, 36, 118, 113, 164, 149, 190)$    | $\{1234789, 124679, 235678, 257\}$                                                                                    |
| 953:218a | $0, 0, 0, 0, e^{12}, e^{34}, e^{15} + e^{23}, e^{25} + e^{13}, e^{14} + e^{36}$  | $(0, 0, 0, 1, 0, 1, 0, 0, 1)$                       | $\{1234789, 123678, 134589, 13568\}$                                                                                  |
| 953:218b | $0, 0, 0, 0, e^{12}, e^{34}, -e^{15} + e^{23}, e^{13} + e^{25}, e^{14} + e^{36}$ | $(0, 0, 0, 1, 0, 1, 0, 0, 1)$                       | $\{1234789, 123678, 134589, 13568\}$                                                                                  |
| 953:219  | $0, 0, 0, 0, e^{12}, e^{34}, e^{23} + e^{15}, e^{25} + e^{14}, e^{46} + e^{13}$  | $19/157(4, 1, 8, 2, 5, 10, 9, 6, 12)$               | $\{1234789, 134589\}$                                                                                                 |
| 953:220a | $0, 0, 0, 0, e^{12}, e^{34}, e^{13} + e^{25}, e^{36}, e^{46} + e^{23} + e^{15}$  | $13/73(2, 2, 4, 1, 4, 5, 6, 9, 6)$                  | $\{1234789, 123679, 234589, 23569\}$                                                                                  |
| 953:220b | $0, 0, 0, 0, e^{12}, e^{34}, -e^{13} + e^{25}, e^{36}, e^{46} + e^{15} + e^{23}$ | $13/73(2, 2, 4, 1, 4, 5, 6, 9, 6)$                  | $\{1234789, 123679, 234589, 23569\}$                                                                                  |
| 953:221  | $0, 0, 0, 0, e^{12}, e^{34}, e^{15} + e^{23}, e^{13} + e^{46}, e^{25} + e^{36}$  | $29/349(4, 7, 8, 2, 11, 10, 15, 12, 18)$            | $\{1234789, 134589\}$                                                                                                 |
| 953:222  | $0, 0, 0, 0, e^{12}, e^{34}, e^{15}, e^{46} + e^{23}, e^{36} + e^{25} + e^{14}$  | $13/31(2, 0, 1, 0, 2, 1, 4, 1, 2)$                  | $\{1234789, 124679\}$                                                                                                 |
| 953:223a | $0, 0, 0, 0, e^{12}, e^{34}, e^{15} + e^{23}, e^{36} + e^{14}, e^{25} + e^{46}$  | $1/5(0, 4, 0, 4, 4, 4, 4, 8)$                       | $\{1234789, 123679, 134589, 13569\}$                                                                                  |
| 953:223b | $0, 0, 0, 0, e^{12}, e^{34}, -e^{15} + e^{23}, e^{14} + e^{36}, e^{25} + e^{46}$ | $1/5(0, 4, 0, 4, 4, 4, 4, 8)$                       | $\{1234789, 123679, 134589, 13569\}$                                                                                  |
| 952:2    | $0, 0, 0, 0, e^{12}, e^{13}, e^{34}, e^{15}, e^{25}$                             | $1/47(19, 20, 30, 32, 39, 49, 62, 58, 59)$          | $\{\emptyset, 123489, 123789, 1246789, 12689, 13459, 13579, 145679, 1569, 234568, 235678, 24578, 258, 346, 367, 47\}$ |
| 952:3    | $0, 0, 0, 0, e^{12}, e^{13}, e^{14}, e^{15}, e^{25}$                             | $1/31(10, 15, 26, 26, 25, 36, 36, 35, 40)$          | $\{\emptyset, 123489, 123789, 124689, 126789, 13459, 13579, 14569, 15679, 2345678, 23568, 24578, 258, 3467, 36, 47\}$ |

Table A.2 – Continued to next page

Table A.2 – Continued from previous page

| Name    | $g$                                                                             | $N$                                                  | Signatures $S$                                                                                                |
|---------|---------------------------------------------------------------------------------|------------------------------------------------------|---------------------------------------------------------------------------------------------------------------|
| 952:4   | $0, 0, 0, 0, e^{12}, e^{13}, e^{24}, e^{15}, e^{25}$                            | $2/5(1, 1, 2, 2, 2, 3, 3, 3)$                        | $\{0, 123489, 123789, 124689, 126789, 134579, 1359, 145679, 1569, 234568, 235678, 2458, 2578, 3467, 36, 47\}$ |
| 952:5   | $0, 0, 0, 0, e^{12}, e^{34}, e^{24} + e^{13}, e^{15}, e^{25}$                   | $1/29(12, 12, 19, 19, 24, 38, 31, 36, 36)$           | $\{0, 123489, 12789, 13569, 145679, 235678, 24568, 347\}$                                                     |
| 952:6   | $0, 0, 0, 0, e^{12}, e^{13}, e^{23}, e^{15}, e^{25} + e^{34}$                   | $1/227(91, 110, 141, 170, 201, 232, 251, 292, 311)$  | $\{0, 12389, 1246789, 13579, 14569, 234568, 2578, 3467\}$                                                     |
| 952:7   | $0, 0, 0, 0, e^{12}, e^{13}, e^{14} + e^{23}, e^{15}, e^{25}$                   | $1/112(40, 50, 87, 97, 90, 127, 137, 130, 140)$      | $\{0, 123489, 126789, 13579, 14569, 23568, 24578, 3467\}$                                                     |
| 952:8   | $0, 0, 0, 0, e^{12}, e^{13}, e^{34}, e^{25}, e^{15} + e^{23}$                   | $1/43(15, 20, 30, 28, 35, 45, 58, 55, 50)$           | $\{123489, 123789, 13458, 13578, 234569, 235679, 346, 367\}$                                                  |
| 952:9   | $0, 0, 0, 0, e^{12}, e^{13}, e^{14}, e^{15}, e^{25} + e^{34}$                   | $3/17(2, 3, 4, 4, 5, 6, 6, 7, 8)$                    | $\{0, 123789, 124689, 13579, 14569, 2345678, 258, 3467\}$                                                     |
| 952:10  | $0, 0, 0, 0, e^{12}, e^{13}, e^{14}, e^{25}, e^{34} + e^{15}$                   | $1/144(64, 62, 95, 95, 126, 159, 159, 188, 190)$     | $\{0, 123789, 124689, 13458, 15678, 23569, 24579, 3467\}$                                                     |
| 952:11  | $0, 0, 0, 0, e^{12}, e^{13}, e^{24}, e^{15}, e^{25} + e^{34}$                   | $1/23(9, 11, 16, 15, 20, 25, 26, 29, 31)$            | $\{0, 123789, 124689, 1359, 145679, 234568, 2578, 3467\}$                                                     |
| 952:12  | $0, 0, 0, 0, e^{12}, e^{13}, e^{34}, e^{15}, e^{14} + e^{25}$                   | $1/43(19, 16, 26, 32, 35, 45, 58, 54, 51)$           | $\{123489, 1246789, 13459, 145679, 234568, 24578, 346, 47\}$                                                  |
| 952:14  | $0, 0, 0, 0, e^{12}, e^{13}, e^{23}, e^{15}, e^{25} + e^{14}$                   | $1/29(11, 13, 21, 26, 24, 32, 34, 35, 37)$           | $\{0, 12389, 126789, 13579, 1569, 23568, 2578, 367\}$                                                         |
| 952:15  | $0, 0, 0, 0, e^{12}, e^{13}, e^{14}, e^{25}, e^{23} + e^{15}$                   | $1/79(30, 35, 60, 64, 65, 90, 94, 100, 95)$          | $\{0, 124689, 126789, 14568, 15678, 24579, 259, 47\}$                                                         |
| 952:17  | $0, 0, 0, 0, e^{12}, e^{13}, e^{23} + e^{14}, e^{15}, e^{34} + e^{25}$          | $9/184(8, 10, 13, 15, 18, 21, 23, 26, 28)$           | $\{0, 13579, 14569, 3467\}$                                                                                   |
| 952:18  | $0, 0, 0, 0, e^{12}, e^{13}, e^{14} + e^{23}, e^{25}, e^{15} + e^{34}$          | $1/113(50, 49, 75, 74, 99, 125, 124, 148, 149)$      | $\{123789, 124689, 13458, 15678\}$                                                                            |
| 952:19a | $0, 0, 0, 0, e^{12}, e^{14} + e^{23}, e^{13} + e^{24}, e^{15}, e^{25}$          | $2/5(1, 1, 2, 2, 2, 3, 3, 3)$                        | $\{0, 123489, 126789, 13569, 14579, 23578, 24568, 3467\}$                                                     |
| 952:19b | $0, 0, 0, 0, e^{12}, -e^{14} + e^{23}, e^{24} + e^{13}, e^{15}, e^{25}$         | $2/5(1, 1, 2, 2, 2, 3, 3, 3)$                        | $\{0, 123489, 126789, 13569, 14579, 23578, 24568, 3467\}$                                                     |
| 952:20  | $0, 0, 0, 0, e^{12}, e^{34}, e^{23} + e^{14}, e^{15}, e^{13} + e^{25}$          | $1/53(24, 19, 38, 33, 43, 71, 57, 67, 62)$           | $\{123489, 135679, 23568, 347\}$                                                                              |
| 952:23  | $0, 0, 0, 0, e^{12}, e^{13}, e^{24}, e^{15} + e^{23}, e^{34} + e^{25}$          | $1/22(8, 11, 16, 14, 19, 24, 25, 27, 30)$            | $\{123789, 1359, 234568, 3467\}$                                                                              |
| 952:24  | $0, 0, 0, 0, e^{12}, e^{13}, e^{23} + e^{14}, e^{25}, e^{15} + e^{24}$          | $1/401(159, 169, 308, 318, 328, 467, 477, 497, 487)$ | $\{0, 126789, 13578, 23569\}$                                                                                 |
| 952:25  | $0, 0, 0, 0, e^{12}, e^{13}, e^{34}, e^{23} + e^{15}, e^{25} + e^{14}$          | $1/31(11, 12, 22, 24, 23, 33, 46, 34, 35)$           | $\{123489, 13459, 234568, 346\}$                                                                              |
| 952:27a | $0, 0, 0, 0, e^{12}, e^{23} + e^{14}, e^{24} + e^{13}, e^{15}, e^{34} + e^{25}$ | $9/41(2, 2, 3, 3, 4, 5, 5, 6, 6)$                    | $\{123789, 124689, 23458, 25678\}$                                                                            |
| 952:27b | $0, 0, 0, 0, e^{12}, e^{23} - e^{14}, e^{24} + e^{13}, e^{15}, e^{25} + e^{34}$ | $9/41(2, 2, 3, 3, 4, 5, 5, 6, 6)$                    | $\{123789, 124689, 23458, 25678\}$                                                                            |
| 952:28a | $0, 0, 0, 0, e^{12}, e^{13}, e^{23}, e^{24} + e^{15}, e^{14} + e^{25}$          | $1/43(18, 18, 31, 36, 36, 49, 49, 54, 54)$           | $\{0, 12389, 126789, 13579, 1569, 23568, 2578, 367\}$                                                         |
| 952:28b | $0, 0, 0, 0, e^{12}, e^{13}, e^{23}, e^{24} - e^{15}, e^{25} + e^{14}$          | $1/43(18, 18, 31, 36, 36, 49, 49, 54, 54)$           | $\{0, 12389, 126789, 13579, 1569, 23568, 2578, 367\}$                                                         |
| 952:30  | $0, 0, 0, 0, e^{12}, e^{13}, e^{14} + e^{23}, e^{15} + e^{24}, e^{25} + e^{34}$ | $21/167(3, 4, 5, 6, 7, 8, 9, 10, 11)$                | $\{14569, 3467\}$                                                                                             |
| 952:31  | $0, 0, 0, 0, e^{12}, e^{34}, e^{13} + e^{24}, e^{15} + e^{23}, e^{25} + e^{14}$ | $7/19(1, 1, 2, 2, 2, 4, 3, 3)$                       | $\{123489, 347\}$                                                                                             |
| 952:35  | $0, 0, 0, 0, e^{12}, e^{13}, e^{14}, e^{15}, e^{16}$                            | $1/11(2, 9, 9, 10, 11, 11, 12, 13, 13)$              | $\{0, 123489, 123789, 12468, 12678, 13459, 13579, 1456, 1567, 23456789, 235689, 24578, 258, 34679, 369, 47\}$ |
| 952:36  | $0, 0, 0, 0, e^{12}, e^{13}, e^{14}, e^{25}, e^{16}$                            | $1/24(6, 13, 18, 21, 19, 24, 27, 32, 30)$            | $\{0, 123489, 123789, 12468, 12678, 134589, 135789, 14568, 15678, 2345679, 23569, 2457, 25, 34679, 369, 47\}$ |
| 952:37  | $0, 0, 0, 0, e^{12}, e^{13}, e^{24}, e^{15}, e^{16}$                            | $1/19(5, 12, 14, 13, 17, 19, 25, 22, 24)$            | $\{0, 123489, 123789, 12468, 12678, 134579, 1359, 14567, 156, 2345689, 2356789, 2458, 2578, 34679, 369, 47\}$ |
| 952:38  | $0, 0, 0, 0, e^{12}, e^{13}, e^{24}, e^{25}, e^{16}$                            | $1/47(15, 22, 32, 36, 37, 47, 58, 59, 62)$           | $\{0, 123489, 123789, 12468, 12678, 1345789, 13589, 145678, 1568, 234569, 235679, 245, 257, 34679, 369, 47\}$ |
| 952:39  | $0, 0, 0, 0, e^{12}, e^{13}, e^{14}, e^{25}, e^{36}$                            | $1/15(6, 7, 7, 12, 13, 13, 18, 20, 20)$              | $\{0, 123489, 123789, 124689, 126789, 134589, 135789, 145689, 156789, 234567, 2356, 2457, 25, 3467, 36, 47\}$ |
| 952:40  | $0, 0, 0, 0, e^{12}, e^{13}, e^{24}, e^{15}, e^{36}$                            | $2/33(6, 9, 8, 12, 15, 14, 21, 21, 22)$              | $\{0, 123489, 123789, 124689, 126789, 134579, 1359, 145679, 1569, 234568, 235678, 2458, 2578, 3467, 36, 47\}$ |
| 952:41  | $0, 0, 0, 0, e^{12}, e^{13}, e^{24}, e^{25}, e^{36}$                            | $1/33(18, 12, 13, 27, 30, 31, 39, 42, 44)$           | $\{0, 123489, 123789, 124689, 126789, 1345789, 13589, 1456789, 15689, 23456, 23567, 245, 257, 3467, 36, 47\}$ |
| 952:42  | $0, 0, 0, 0, e^{12}, e^{13}, e^{14} + e^{23}, e^{15}, e^{16}$                   | $1/38(11, 24, 24, 37, 35, 35, 48, 46, 46)$           | $\{0, 123489, 12678, 13579, 1456, 235689, 24578, 34679\}$                                                     |
| 952:43  | $0, 0, 0, 0, e^{12}, e^{13}, e^{14} + e^{23}, e^{25}, e^{16}$                   | $1/144(42, 73, 98, 129, 115, 140, 171, 188, 182)$    | $\{0, 123489, 12678, 135789, 14568, 23569, 2457, 34679\}$                                                     |
| 952:44  | $0, 0, 0, 0, e^{12}, e^{13}, e^{23} + e^{14}, e^{25}, e^{36}$                   | $1/13(4, 7, 7, 10, 11, 11, 14, 18, 18)$              | $\{123789, 124689, 134589, 156789, 234567, 25, 36, 47\}$                                                      |
| 952:45  | $0, 0, 0, 0, e^{12}, e^{13}, e^{14}, e^{15}, e^{16} + e^{24}$                   | $1/38(11, 24, 30, 28, 35, 41, 39, 46, 52)$           | $\{0, 123789, 12468, 13459, 1567, 235689, 24578, 34679\}$                                                     |
| 952:46  | $0, 0, 0, 0, e^{12}, e^{13}, e^{14}, e^{25}, e^{24} + e^{16}$                   | $1/144(42, 73, 106, 117, 115, 148, 159, 188, 190)$   | $\{0, 123789, 12468, 134589, 15678, 23569, 2457, 34679\}$                                                     |
| 952:48  | $0, 0, 0, 0, e^{12}, e^{13}, e^{14}, e^{15}, e^{36} + e^{24}$                   | $1/297(90, 193, 167, 231, 283, 257, 321, 373, 424)$  | $\{0, 123789, 126789, 13459, 14569, 2345678, 24578, 36\}$                                                     |
| 952:49  | $0, 0, 0, 0, e^{12}, e^{13}, e^{14}, e^{25}, e^{16} + e^{34}$                   | $1/33(12, 16, 21, 24, 28, 33, 36, 44, 45)$           | $\{0, 123789, 12678, 135789, 15678, 23569, 25, 369\}$                                                         |

Table A.2 – Continued to next page

Table A.2 – Continued from previous page

| Name    | $g$                                                                    | $N$                                                  | Signatures $S$                                                                                                        |
|---------|------------------------------------------------------------------------|------------------------------------------------------|-----------------------------------------------------------------------------------------------------------------------|
| 952:50  | $0, 0, 0, 0, e^{12}, e^{13}, e^{14}, e^{25}, e^{36} + e^{24}$          | $1/52(20, 25, 24, 43, 45, 44, 63, 70, 68)$           | $\{123489, 124689, 135789, 156789, 2356, 25, 3467, 47\}$                                                              |
| 952:51  | $0, 0, 0, 0, e^{12}, e^{13}, e^{24}, e^{15}, e^{14} + e^{36}$          | $2/29(6, 7, 6, 12, 13, 12, 19, 19, 18)$              | $\{123489, 124689, 134579, 145679, 234568, 2458, 3467, 47\}$                                                          |
| 952:52  | $0, 0, 0, 0, e^{12}, e^{13}, e^{24}, e^{15}, e^{16} + e^{34}$          | $1/13(4, 8, 9, 8, 12, 13, 16, 16, 17)$               | $\{\emptyset, 123789, 12678, 1359, 156, 2356789, 2578, 369\}$                                                         |
| 952:53  | $0, 0, 0, 0, e^{12}, e^{13}, e^{24}, e^{25}, e^{36} + e^{14}$          | $1/317(170, 117, 128, 256, 287, 298, 373, 404, 426)$ | $\{\emptyset, 123789, 126789, 13589, 15689, 23567, 257, 36\}$                                                         |
| 952:54  | $0, 0, 0, 0, e^{12}, e^{13}, e^{24}, e^{25}, e^{34} + e^{16}$          | $1/11(4, 5, 7, 8, 9, 11, 13, 14, 15)$                | $\{\emptyset, 123789, 12678, 13589, 1568, 235679, 257, 369\}$                                                         |
| 952:55  | $0, 0, 0, 0, e^{12}, e^{13}, e^{34}, e^{15}, e^{24} + e^{16}$          | $1/23(7, 15, 15, 14, 22, 22, 29, 29, 29)$            | $\{\emptyset, 123789, 124678, 13459, 156, 2356789, 24578, 3469\}$                                                     |
| 952:56  | $0, 0, 0, 0, e^{12}, e^{13}, e^{34}, e^{25}, e^{16} + e^{24}$          | $1/139(49, 69, 75, 104, 118, 124, 179, 187, 173)$    | $\{123489, 1268, 135789, 145678, 234569, 25, 3679, 47\}$                                                              |
| 952:57  | $0, 0, 0, 0, e^{12}, e^{13}, e^{34}, e^{15}, e^{36} + e^{14}$          | $1/43(15, 28, 18, 36, 43, 33, 54, 58, 51)$           | $\{123489, 1246789, 13459, 145679, 234568, 24578, 346, 47\}$                                                          |
| 952:58  | $0, 0, 0, 0, e^{12}, e^{13}, e^{34}, e^{15}, e^{36} + e^{24}$          | $1/281(96, 176, 139, 198, 272, 235, 337, 368, 374)$  | $\{\emptyset, 123789, 12689, 13459, 145679, 234568, 24578, 367\}$                                                     |
| 952:59  | $0, 0, 0, 0, e^{12}, e^{13}, e^{34}, e^{25}, e^{14} + e^{36}$          | $1/69(36, 28, 27, 54, 64, 63, 81, 92, 90)$           | $\{\emptyset, 123789, 12689, 135789, 15689, 23567, 25, 367\}$                                                         |
| 952:60  | $0, 0, 0, 0, e^{12}, e^{13}, e^{34}, e^{25}, e^{36} + e^{24}$          | $1/139(75, 56, 49, 117, 131, 124, 166, 187, 173)$    | $\{123489, 1246789, 135789, 15689, 23567, 25, 346, 47\}$                                                              |
| 952:61  | $0, 0, 0, 0, e^{12}, e^{13}, e^{23}, e^{15}, e^{24} + e^{16}$          | $1/49(17, 26, 32, 40, 43, 49, 58, 60, 66)$           | $\{\emptyset, 12389, 124678, 134579, 156, 235689, 24578, 34679\}$                                                     |
| 952:62  | $0, 0, 0, 0, e^{12}, e^{13}, e^{23}, e^{25}, e^{24} + e^{16}$          | $1/11(4, 5, 7, 10, 9, 11, 12, 14, 15)$               | $\{\emptyset, 12389, 124678, 1345789, 1568, 23569, 2457, 34679\}$                                                     |
| 952:63  | $0, 0, 0, 0, e^{12}, e^{13}, e^{23}, e^{15}, e^{36} + e^{14}$          | $1/227(75, 143, 111, 222, 218, 186, 254, 293, 297)$  | $\{\emptyset, 12389, 126789, 13579, 1569, 23568, 2578, 367\}$                                                         |
| 952:65  | $0, 0, 0, 0, e^{12}, e^{13}, e^{23}, e^{15}, e^{36} + e^{24}$          | $1/297(108, 166, 155, 252, 274, 263, 321, 382, 418)$ | $\{\emptyset, 12389, 126789, 134579, 14569, 234568, 24578, 367\}$                                                     |
| 952:66  | $0, 0, 0, 0, e^{12}, e^{13}, e^{23}, e^{25}, e^{36} + e^{14}$          | $1/59(26, 27, 28, 56, 53, 54, 55, 80, 82)$           | $\{123789, 12689, 13589, 156789, 23567, 25, 36, 7\}$                                                                  |
| 952:67  | $0, 0, 0, 0, e^{12}, e^{13}, e^{23}, e^{25}, e^{16} + e^{34}$          | $1/81(33, 37, 47, 66, 70, 80, 84, 107, 113)$         | $\{\emptyset, 12389, 12678, 135789, 1568, 23569, 257, 3679\}$                                                         |
| 952:68  | $0, 0, 0, 0, e^{12}, e^{13}, e^{23}, e^{25}, e^{24} + e^{36}$          | $1/43(20, 19, 20, 41, 39, 40, 39, 58, 60)$           | $\{123789, 12689, 134589, 1456789, 234567, 245, 36, 7\}$                                                              |
| 952:69  | $0, 0, 0, 0, e^{12}, e^{13}, e^{14}, e^{15}, e^{16} + e^{23}$          | $1/13(4, 8, 9, 11, 12, 13, 15, 16, 17)$              | $\{\emptyset, 13459, 13579, 1456, 1567, 34679, 369, 47\}$                                                             |
| 952:70  | $0, 0, 0, 0, e^{12}, e^{13}, e^{14}, e^{25}, e^{23} + e^{16}$          | $1/83(22, 44, 61, 72, 66, 83, 94, 110, 105)$         | $\{\emptyset, 134589, 135789, 14568, 15678, 34679, 369, 47\}$                                                         |
| 952:71  | $0, 0, 0, 0, e^{12}, e^{13}, e^{24}, e^{15}, e^{23} + e^{16}$          | $1/17(5, 10, 12, 12, 15, 17, 22, 20, 22)$            | $\{\emptyset, 134579, 1359, 14567, 156, 34679, 369, 47\}$                                                             |
| 952:72  | $0, 0, 0, 0, e^{12}, e^{13}, e^{24}, e^{25}, e^{23} + e^{16}$          | $1/43(11, 22, 32, 32, 33, 43, 54, 55, 54)$           | $\{123489, 123789, 12468, 12678, 234569, 235679, 245, 257\}$                                                          |
| 952:73  | $0, 0, 0, 0, e^{12}, e^{13}, e^{24}, e^{23} + e^{15}, e^{16}$          | $1/227(73, 132, 146, 161, 205, 219, 293, 278, 292)$  | $\{\emptyset, 12468, 12678, 14567, 156, 2458, 2578, 47\}$                                                             |
| 952:74  | $0, 0, 0, 0, e^{12}, e^{13}, e^{24}, e^{15} + e^{23}, e^{36}$          | $2/29(4, 9, 8, 10, 13, 12, 19, 17, 20)$              | $\{123489, 123789, 134579, 1359, 234568, 235678, 3467, 36\}$                                                          |
| 952:80  | $0, 0, 0, 0, e^{12}, e^{13}, e^{14}, e^{15}, e^{16} + e^{25}$          | $1/79(22, 43, 64, 68, 65, 86, 90, 87, 108)$          | $\{\emptyset, 123489, 123789, 13459, 13579, 24578, 258, 47\}$                                                         |
| 952:81  | $0, 0, 0, 0, e^{12}, e^{13}, e^{24}, e^{15}, e^{16} + e^{25}$          | $1/23(7, 12, 17, 17, 19, 24, 29, 26, 31)$            | $\{\emptyset, 123489, 123789, 134579, 1359, 2458, 2578, 47\}$                                                         |
| 952:82a | $0, 0, 0, 0, e^{12}, e^{13}, e^{14}, e^{15}, e^{25} + e^{36}$          | $1/81(24, 47, 47, 69, 71, 71, 93, 95, 118)$          | $\{\emptyset, 123489, 123789, 124689, 126789, 13459, 13579, 14569, 15679, 2345678, 23568, 24578, 258, 3467, 36, 47\}$ |
| 952:82b | $0, 0, 0, 0, -e^{12}, e^{13}, e^{14}, e^{15}, e^{36} + e^{25}$         | $1/81(24, 47, 47, 69, 71, 71, 93, 95, 118)$          | $\{\emptyset, 123489, 123789, 124689, 126789, 13459, 13579, 14569, 15679, 2345678, 23568, 24578, 258, 3467, 36, 47\}$ |
| 952:84  | $0, 0, 0, 0, e^{12}, e^{13}, e^{14}, e^{25}, e^{36} + e^{15}$          | $1/52(22, 24, 23, 41, 46, 45, 63, 70, 68)$           | $\{134589, 135789, 145689, 156789, 234567, 2356, 2457, 25\}$                                                          |
| 952:86a | $0, 0, 0, 0, e^{12}, e^{13}, e^{24}, e^{15}, e^{36} + e^{25}$          | $1/8(3, 4, 4, 6, 7, 7, 10, 10, 11)$                  | $\{\emptyset, 123489, 123789, 124689, 126789, 134579, 1359, 145679, 1569, 234568, 235678, 2458, 2578, 3467, 36, 47\}$ |
| 952:86b | $0, 0, 0, 0, -e^{12}, e^{13}, e^{24}, e^{15}, e^{36} + e^{25}$         | $1/8(3, 4, 4, 6, 7, 7, 10, 10, 11)$                  | $\{\emptyset, 123489, 123789, 124689, 126789, 134579, 1359, 145679, 1569, 234568, 235678, 2458, 2578, 3467, 36, 47\}$ |
| 952:88  | $0, 0, 0, 0, e^{12}, e^{13}, e^{24}, e^{25}, e^{15} + e^{36}$          | $1/16(8, 6, 7, 13, 14, 15, 19, 20, 22)$              | $\{\emptyset, 123489, 123789, 124689, 126789, 3467, 36, 47\}$                                                         |
| 952:90  | $0, 0, 0, 0, e^{12}, e^{13}, e^{34}, e^{15}, e^{16} + e^{25}$          | $1/281(100, 137, 174, 194, 237, 274, 368, 337, 374)$ | $\{\emptyset, 123489, 123789, 13459, 13579, 24578, 258, 47\}$                                                         |
| 952:91a | $0, 0, 0, 0, e^{12}, e^{13}, e^{34}, e^{15}, e^{36} + e^{25}$          | $1/8(3, 4, 4, 6, 7, 7, 10, 10, 11)$                  | $\{\emptyset, 123489, 123789, 1246789, 12689, 13459, 13579, 145679, 1569, 234568, 235678, 24578, 258, 346, 367, 47\}$ |
| 952:91b | $0, 0, 0, 0, -e^{12}, e^{13}, e^{34}, e^{15}, e^{25} + e^{36}$         | $1/8(3, 4, 4, 6, 7, 7, 10, 10, 11)$                  | $\{\emptyset, 123489, 123789, 1246789, 12689, 13459, 13579, 145679, 1569, 234568, 235678, 24578, 258, 346, 367, 47\}$ |
| 952:93  | $0, 0, 0, 0, e^{12}, e^{13}, e^{34}, e^{25}, e^{36} + e^{15}$          | $1/41(19, 17, 18, 32, 36, 37, 50, 53, 55)$           | $\{\emptyset, 123489, 123789, 1246789, 12689, 346, 367, 47\}$                                                         |
| 952:95  | $0, 0, 0, 0, e^{12}, e^{13}, e^{14} + e^{23}, e^{15}, e^{24} + e^{16}$ | $1/97(34, 51, 63, 80, 85, 97, 114, 119, 131)$        | $\{12389, 124678, 134579, 156\}$                                                                                      |
| 952:96  | $0, 0, 0, 0, e^{12}, e^{13}, e^{23} + e^{14}, e^{25}, e^{16} + e^{24}$ | $1/56(18, 27, 38, 47, 45, 56, 65, 72, 74)$           | $\{\emptyset, 23569, 2457, 34679\}$                                                                                   |
| 952:98  | $0, 0, 0, 0, e^{12}, e^{13}, e^{14} + e^{23}, e^{15}, e^{36} + e^{24}$ | $1/15(5, 9, 8, 12, 14, 13, 17, 19, 21)$              | $\{\emptyset, 126789, 14569, 24578\}$                                                                                 |
| 952:99  | $0, 0, 0, 0, e^{12}, e^{13}, e^{14} + e^{23}, e^{25}, e^{16} + e^{34}$ | $1/171(63, 82, 107, 126, 145, 170, 189, 227, 233)$   | $\{\emptyset, 12678, 135789, 23569\}$                                                                                 |
| 952:100 | $0, 0, 0, 0, e^{12}, e^{13}, e^{23} + e^{14}, e^{25}, e^{36} + e^{24}$ | $1/45(13, 25, 24, 36, 38, 37, 49, 63, 61)$           | $\{124689, 156789, 25, 47\}$                                                                                          |

Table A.2 – Continued to next page

Table A.2 – Continued from previous page

| Name     | $g$                                                                              | $N$                                                  | Signatures $S$                                                    |
|----------|----------------------------------------------------------------------------------|------------------------------------------------------|-------------------------------------------------------------------|
| 952:104  | $0, 0, 0, 0, e^{12}, e^{13}, e^{14}, e^{25} + e^{34}, e^{16} + e^{24}$           | $1/109(35, 59, 71, 82, 94, 106, 117, 153, 141)$      | $\{\emptyset, 123789, 12468, 34679\}$                             |
| 952:105  | $0, 0, 0, 0, e^{12}, e^{13}, e^{14}, e^{25} + e^{34}, e^{36} + e^{24}$           | $2/59(11, 14, 14, 25, 25, 25, 36, 39, 39)$           | $\{123489, 156789, 2356, 47\}$                                    |
| 952:106  | $0, 0, 0, 0, e^{12}, e^{13}, e^{24}, e^{15} + e^{34}, e^{14} + e^{36}$           | $1/122(49, 58, 52, 104, 107, 101, 162, 156, 153)$    | $\{123489, 145679, 234568, 47\}$                                  |
| 952:107  | $0, 0, 0, 0, e^{12}, e^{13}, e^{24}, e^{25} + e^{34}, e^{14} + e^{36}$           | $1/53(28, 19, 22, 44, 47, 50, 63, 66, 72)$           | $\{126789, 15689, 23567, 36\}$                                    |
| 952:111  | $0, 0, 0, 0, e^{12}, e^{13}, e^{23}, e^{25} + e^{14}, e^{24} + e^{36}$           | $1/217(98, 100, 101, 200, 198, 199, 201, 298, 300)$  | $\{123789, 12689, 36, 7\}$                                        |
| 952:112a | $0, 0, 0, 0, e^{12}, e^{13}, e^{23}, e^{34} + e^{15}, e^{16} + e^{24}$           | $1/19(7, 11, 11, 14, 18, 18, 22, 25, 25)$            | $\{\emptyset, 12389, 124678, 134579, 156, 235689, 24578, 34679\}$ |
| 952:112b | $0, 0, 0, 0, -e^{12}, e^{13}, e^{23}, e^{15} + e^{34}, e^{16} + e^{24}$          | $1/19(7, 11, 11, 14, 18, 18, 22, 25, 25)$            | $\{\emptyset, 12389, 124678, 134579, 156, 235689, 24578, 34679\}$ |
| 952:113  | $0, 0, 0, 0, e^{12}, e^{13}, e^{23}, e^{34} + e^{25}, e^{16} + e^{24}$           | $1/109(41, 55, 62, 89, 96, 103, 117, 151, 144)$      | $\{\emptyset, 12389, 124678, 34679\}$                             |
| 952:114  | $0, 0, 0, 0, e^{12}, e^{13}, e^{23}, e^{25} + e^{34}, e^{24} + e^{36}$           | $1/53(25, 24, 24, 49, 49, 49, 48, 73, 73)$           | $\{123789, 1456789, 234567, 7\}$                                  |
| 952:115  | $0, 0, 0, 0, e^{12}, e^{13}, e^{14}, e^{15} + e^{23}, e^{16} + e^{24}$           | $1/86(29, 52, 58, 64, 81, 87, 93, 110, 116)$         | $\{\emptyset, 12468, 1567, 24578\}$                               |
| 952:117  | $0, 0, 0, 0, e^{12}, e^{13}, e^{14}, e^{15} + e^{23}, e^{24} + e^{36}$           | $1/461(133, 305, 266, 360, 438, 399, 493, 571, 665)$ | $\{123789, 13459, 2345678, 36\}$                                  |
| 952:118  | $0, 0, 0, 0, e^{12}, e^{13}, e^{24}, e^{15} + e^{23}, e^{36} + e^{14}$           | $2/17(2, 5, 4, 8, 7, 6, 13, 9, 10)$                  | $\{123489, 134579, 234568, 3467\}$                                |
| 952:119  | $0, 0, 0, 0, e^{12}, e^{13}, e^{24}, e^{15} + e^{23}, e^{16} + e^{34}$           | $1/49(16, 29, 32, 32, 45, 48, 61, 61, 64)$           | $\{\emptyset, 12678, 156, 2578\}$                                 |
| 952:120  | $0, 0, 0, 0, e^{12}, e^{13}, e^{34}, e^{15} + e^{23}, e^{16} + e^{24}$           | $1/193(61, 124, 122, 120, 185, 183, 242, 246, 244)$  | $\{\emptyset, 124678, 156, 24578\}$                               |
| 952:121  | $0, 0, 0, 0, e^{12}, e^{13}, e^{34}, e^{15} + e^{23}, e^{14} + e^{36}$           | $1/31(7, 24, 14, 28, 31, 21, 42, 38, 35)$            | $\{123489, 13459, 234568, 346\}$                                  |
| 952:122  | $0, 0, 0, 0, e^{12}, e^{13}, e^{34}, e^{15} + e^{23}, e^{24} + e^{36}$           | $1/509(139, 352, 278, 343, 491, 417, 621, 630, 695)$ | $\{123789, 13459, 234568, 367\}$                                  |
| 952:123  | $0, 0, 0, 0, e^{12}, e^{13}, e^{23} + e^{14}, e^{15}, e^{25} + e^{16}$           | $1/131(41, 67, 93, 119, 108, 134, 160, 149, 175)$    | $\{\emptyset, 123489, 13579, 24578\}$                             |
| 952:124a | $0, 0, 0, 0, e^{12}, e^{13}, e^{14} + e^{23}, e^{15}, e^{36} + e^{25}$           | $1/137(41, 79, 79, 117, 120, 120, 158, 161, 199)$    | $\{\emptyset, 123489, 126789, 13579, 14569, 23568, 24578, 3467\}$ |
| 952:124b | $0, 0, 0, 0, -e^{12}, e^{13}, e^{14} + e^{23}, e^{15}, e^{36} + e^{25}$          | $1/137(41, 79, 79, 117, 120, 120, 158, 161, 199)$    | $\{\emptyset, 123489, 126789, 13579, 14569, 23568, 24578, 3467\}$ |
| 952:126  | $0, 0, 0, 0, e^{12}, e^{13}, e^{23} + e^{14}, e^{25}, e^{15} + e^{36}$           | $1/28(10, 16, 13, 19, 26, 23, 29, 42, 36)$           | $\{134589, 156789, 234567, 25\}$                                  |
| 952:129  | $0, 0, 0, 0, e^{12}, e^{13}, e^{14}, e^{25}, e^{15} + e^{36} + e^{24}$           | $2/59(12, 14, 13, 24, 26, 25, 36, 40, 38)$           | $\{135789, 156789, 2356, 25\}$                                    |
| 952:130a | $0, 0, 0, 0, e^{12}, e^{13}, e^{24}, e^{15}, e^{14} + e^{36} + e^{25}$           | $3/7(1, 1, 1, 2, 2, 2, 3, 3, 3)$                     | $\{123489, 124689, 134579, 145679, 234568, 2458, 3467, 47\}$      |
| 952:130b | $0, 0, 0, 0, -e^{12}, e^{13}, e^{24}, e^{15}, e^{36} + e^{25} + e^{14}$          | $3/7(1, 1, 1, 2, 2, 2, 3, 3, 3)$                     | $\{123489, 124689, 134579, 145679, 234568, 2458, 3467, 47\}$      |
| 952:132  | $0, 0, 0, 0, e^{12}, e^{13}, e^{24}, e^{15}, e^{16} + e^{25} + e^{34}$           | $2/77(13, 20, 27, 26, 33, 40, 46, 46, 53)$           | $\{\emptyset, 123789, 1359, 2578\}$                               |
| 952:134a | $0, 0, 0, 0, e^{12}, e^{13}, e^{34}, e^{15}, e^{14} + e^{36} + e^{25}$           | $3/7(1, 1, 1, 2, 2, 2, 3, 3, 3)$                     | $\{123489, 1246789, 13459, 145679, 234568, 24578, 346, 47\}$      |
| 952:134b | $0, 0, 0, 0, -e^{12}, e^{13}, e^{34}, e^{15}, e^{36} + e^{25} + e^{14}$          | $3/7(1, 1, 1, 2, 2, 2, 3, 3, 3)$                     | $\{123489, 1246789, 13459, 145679, 234568, 24578, 346, 47\}$      |
| 952:136  | $0, 0, 0, 0, e^{12}, e^{13}, e^{34}, e^{25}, e^{36} + e^{15} + e^{24}$           | $1/67(28, 30, 29, 56, 58, 57, 85, 88, 86)$           | $\{123489, 1246789, 346, 47\}$                                    |
| 952:139a | $0, 0, 0, 0, e^{12}, e^{13}, e^{14}, e^{15} + e^{24}, e^{25} + e^{36}$           | $1/51(19, 27, 27, 38, 46, 46, 57, 65, 73)$           | $\{\emptyset, 123789, 126789, 13579, 15679, 23568, 258, 36\}$     |
| 952:139b | $0, 0, 0, 0, -e^{12}, e^{13}, e^{14}, e^{15} + e^{24}, e^{36} + e^{25}$          | $1/51(19, 27, 27, 38, 46, 46, 57, 65, 73)$           | $\{\emptyset, 123789, 126789, 13579, 15679, 23568, 258, 36\}$     |
| 952:141  | $0, 0, 0, 0, e^{12}, e^{13}, e^{24}, e^{25} + e^{14}, e^{36} + e^{15}$           | $2/127(31, 25, 28, 50, 56, 59, 75, 81, 87)$          | $\{\emptyset, 123789, 126789, 36\}$                               |
| 952:143  | $0, 0, 0, 0, e^{12}, e^{13}, e^{14}, e^{15} + e^{34}, e^{16} + e^{25}$           | $1/109(43, 55, 67, 74, 98, 110, 117, 141, 153)$      | $\{\emptyset, 123789, 13459, 24578\}$                             |
| 952:144  | $0, 0, 0, 0, e^{12}, e^{13}, e^{24}, e^{34} + e^{15}, e^{25} + e^{16}$           | $1/26(10, 13, 16, 17, 23, 26, 30, 33, 36)$           | $\{\emptyset, 123789, 134579, 2458\}$                             |
| 952:145a | $0, 0, 0, 0, e^{12}, e^{13}, e^{14}, e^{34} + e^{15}, e^{36} + e^{25}$           | $1/51(19, 27, 27, 38, 46, 46, 57, 65, 73)$           | $\{\emptyset, 123789, 124689, 13459, 15679, 23568, 24578, 3467\}$ |
| 952:145b | $0, 0, 0, 0, -e^{12}, e^{13}, e^{14}, e^{15} + e^{34}, e^{25} + e^{36}$          | $1/51(19, 27, 27, 38, 46, 46, 57, 65, 73)$           | $\{\emptyset, 123789, 124689, 13459, 15679, 23568, 24578, 3467\}$ |
| 952:147  | $0, 0, 0, 0, e^{12}, e^{13}, e^{14}, e^{25} + e^{34}, e^{36} + e^{15}$           | $3/7(1, 1, 1, 2, 2, 2, 3, 3, 3)$                     | $\{134589, 156789, 2356, 2457\}$                                  |
| 952:153  | $0, 0, 0, 0, e^{12}, e^{13}, e^{34}, e^{24} + e^{15}, e^{25} + e^{16}$           | $1/37(13, 18, 23, 26, 31, 36, 49, 44, 49)$           | $\{123489, 13459, 24578, 47\}$                                    |
| 952:154  | $0, 0, 0, 0, e^{12}, e^{13}, e^{34}, e^{14} + e^{25}, e^{36} + e^{15}$           | $3/241(38, 32, 35, 64, 70, 73, 99, 102, 108)$        | $\{123489, 1246789, 346, 47\}$                                    |
| 952:159a | $0, 0, 0, 0, e^{12}, e^{13}, e^{14} + e^{23}, e^{15} + e^{34}, e^{16} + e^{24}$  | $7/37(2, 3, 3, 4, 5, 5, 6, 7, 7)$                    | $\{12389, 124678, 134579, 156\}$                                  |
| 952:159b | $0, 0, 0, 0, -e^{12}, e^{13}, e^{14} + e^{23}, e^{15} + e^{34}, e^{16} + e^{24}$ | $7/37(2, 3, 3, 4, 5, 5, 6, 7, 7)$                    | $\{12389, 124678, 134579, 156\}$                                  |
| 952:160  | $0, 0, 0, 0, e^{12}, e^{13}, e^{14} + e^{23}, e^{34} + e^{25}, e^{16} + e^{24}$  | $7/81(4, 6, 7, 9, 10, 11, 13, 16, 15)$               | $\{\emptyset, 34679\}$                                            |
| 952:161  | $0, 0, 0, 0, e^{12}, e^{13}, e^{23} + e^{14}, e^{34} + e^{25}, e^{36} + e^{24}$  | $14/51(1, 2, 2, 3, 3, 3, 4, 5, 5)$                   | $\{156789, 47\}$                                                  |
| 952:162a | $0, 0, 0, 0, e^{12}, e^{13}, e^{23}, e^{15}, e^{25} + e^{36} + e^{14}$           | $1/25(9, 13, 13, 26, 22, 22, 26, 31, 35)$            | $\{123489, 1246789, 134579, 14569, 234568, 24578, 3467, 4\}$      |
| 952:162b | $0, 0, 0, 0, -e^{12}, e^{13}, e^{23}, e^{15}, e^{14} + e^{36} + e^{25}$          | $1/25(9, 13, 13, 26, 22, 22, 26, 31, 35)$            | $\{123489, 1246789, 134579, 14569, 234568, 24578, 3467, 4\}$      |
| 952:164  | $0, 0, 0, 0, e^{12}, e^{13}, e^{23}, e^{15}, e^{34} + e^{25} + e^{16}$           | $1/26(10, 13, 16, 20, 23, 26, 29, 33, 36)$           | $\{\emptyset, 12389, 13579, 2578\}$                               |
| 952:165  | $0, 0, 0, 0, e^{12}, e^{13}, e^{23}, e^{25}, e^{15} + e^{24} + e^{36}$           | $1/59(28, 26, 27, 56, 54, 55, 53, 80, 82)$           | $\{134589, 1456789, 234567, 245\}$                                |
| 952:167  | $0, 0, 0, 0, e^{12}, e^{13}, e^{23}, e^{24} + e^{15}, e^{16} + e^{25}$           | $1/26(10, 13, 16, 20, 23, 26, 29, 33, 36)$           | $\{\emptyset, 12389, 13579, 2578\}$                               |
| 952:172  | $0, 0, 0, 0, e^{12}, e^{13}, e^{23}, e^{15} + e^{34}, e^{16} + e^{25}$           | $1/147(61, 72, 83, 111, 133, 144, 155, 194, 205)$    | $\{\emptyset, 12389, 134579, 24578\}$                             |

Table A.2 – Continued to next page

Table A.2 – Continued from previous page

| Name     | $g$                                                                              | $N$                                                 | Signatures $S$                                                    |
|----------|----------------------------------------------------------------------------------|-----------------------------------------------------|-------------------------------------------------------------------|
| 952:175  | $0, 0, 0, 0, e^{12}, e^{13}, e^{23}, e^{34} + e^{25}, e^{36} + e^{15}$           | $1/85(38, 40, 39, 79, 78, 77, 79, 118, 116)$        | $\{123789, 124689, 346, 7\}$                                      |
| 952:177  | $0, 0, 0, 0, e^{12}, e^{13}, e^{14}, e^{15} + e^{23}, e^{16} + e^{25}$           | $1/41(14, 21, 28, 34, 35, 42, 48, 49, 56)$          | $\{\emptyset, 24578, 258, 47\}$                                   |
| 952:178  | $0, 0, 0, 0, e^{12}, e^{13}, e^{24}, e^{15} + e^{23}, e^{25} + e^{16}$           | $2/83(14, 21, 28, 31, 35, 42, 52, 49, 56)$          | $\{\emptyset, 2458, 2578, 47\}$                                   |
| 952:179a | $0, 0, 0, 0, e^{12}, e^{13}, e^{14}, e^{15} + e^{23}, e^{36} + e^{25}$           | $1/137(40, 80, 80, 117, 120, 120, 157, 160, 200)$   | $\{123489, 123789, 13459, 13579, 2345678, 23568, 3467, 36\}$      |
| 952:179b | $0, 0, 0, 0, -e^{12}, e^{13}, e^{14}, e^{15} + e^{23}, e^{25} + e^{36}$          | $1/137(40, 80, 80, 117, 120, 120, 157, 160, 200)$   | $\{123489, 123789, 13459, 13579, 2345678, 23568, 3467, 36\}$      |
| 952:181a | $0, 0, 0, 0, e^{12}, e^{13}, e^{24}, e^{15} + e^{23}, e^{25} + e^{36}$           | $1/7(2, 4, 4, 5, 6, 6, 9, 8, 10)$                   | $\{123489, 123789, 134579, 1359, 234568, 235678, 3467, 36\}$      |
| 952:181b | $0, 0, 0, 0, -e^{12}, e^{13}, e^{24}, e^{23} + e^{15}, e^{36} + e^{25}$          | $1/7(2, 4, 4, 5, 6, 6, 9, 8, 10)$                   | $\{123489, 123789, 134579, 1359, 234568, 235678, 3467, 36\}$      |
| 952:183  | $0, 0, 0, 0, e^{12}, e^{13}, e^{34}, e^{15} + e^{23}, e^{25} + e^{16}$           | $1/211(70, 105, 140, 141, 175, 210, 281, 245, 280)$ | $\{123489, 123789, 13459, 13579\}$                                |
| 952:184a | $0, 0, 0, 0, e^{12}, e^{13}, e^{34}, e^{15} + e^{23}, e^{25} + e^{36}$           | $1/7(2, 4, 4, 5, 6, 6, 9, 8, 10)$                   | $\{123489, 123789, 13459, 13579, 234568, 235678, 346, 367\}$      |
| 952:184b | $0, 0, 0, 0, -e^{12}, e^{13}, e^{34}, e^{23} + e^{15}, e^{36} + e^{25}$          | $1/7(2, 4, 4, 5, 6, 6, 9, 8, 10)$                   | $\{123489, 123789, 13459, 13579, 234568, 235678, 346, 367\}$      |
| 952:189  | $0, 0, 0, 0, e^{12}, e^{13}, e^{14}, e^{25} + e^{16}, e^{15} + e^{36}$           | $2/59(13, 13, 13, 23, 26, 26, 36, 39, 39)$          | $\{145689, 156789, 234567, 2356\}$                                |
| 952:191  | $0, 0, 0, 0, e^{12}, e^{13}, e^{24}, e^{16} + e^{25}, e^{15} + e^{36}$           | $2/59(13, 13, 13, 23, 26, 26, 36, 39, 39)$          | $\{\emptyset, 123489, 123789, 47\}$                               |
| 952:196  | $0, 0, 0, 0, e^{12}, e^{13}, e^{23} + e^{14}, e^{15}, e^{16} + e^{25} + e^{34}$  | $21/167(3, 4, 5, 6, 7, 8, 9, 10, 11)$               | $\{\emptyset, 13579\}$                                            |
| 952:197  | $0, 0, 0, 0, e^{12}, e^{13}, e^{14} + e^{23}, e^{25}, e^{15} + e^{24} + e^{36}$  | $11/95(3, 5, 4, 6, 8, 7, 9, 13, 11)$                | $\{156789, 25\}$                                                  |
| 952:198  | $0, 0, 0, 0, e^{12}, e^{13}, e^{14} + e^{23}, e^{24} + e^{15}, e^{25} + e^{16}$  | $21/167(3, 4, 5, 6, 7, 8, 9, 10, 11)$               | $\{\emptyset, 13579\}$                                            |
| 952:199a | $0, 0, 0, 0, e^{12}, e^{13}, e^{14} + e^{23}, e^{24} + e^{15}, e^{36} + e^{25}$  | $43/237(2, 3, 3, 4, 5, 5, 6, 7, 8)$                 | $\{123789, 15679, 258, 36\}$                                      |
| 952:199b | $0, 0, 0, 0, -e^{12}, e^{13}, e^{23} + e^{14}, e^{15} + e^{24}, e^{36} + e^{25}$ | $43/237(2, 3, 3, 4, 5, 5, 6, 7, 8)$                 | $\{123789, 15679, 258, 36\}$                                      |
| 952:201  | $0, 0, 0, 0, e^{12}, e^{13}, e^{14} + e^{23}, e^{15} + e^{34}, e^{16} + e^{25}$  | $79/793(4, 5, 6, 7, 9, 10, 11, 13, 14)$             | $\{\emptyset, 24578\}$                                            |
| 952:202a | $0, 0, 0, 0, e^{12}, e^{13}, e^{14} + e^{23}, e^{34} + e^{15}, e^{25} + e^{36}$  | $43/237(2, 3, 3, 4, 5, 5, 6, 7, 8)$                 | $\{123789, 124689, 13459, 15679\}$                                |
| 952:202b | $0, 0, 0, 0, -e^{12}, e^{13}, e^{14} + e^{23}, e^{15} + e^{34}, e^{36} + e^{25}$ | $43/237(2, 3, 3, 4, 5, 5, 6, 7, 8)$                 | $\{123789, 124689, 13459, 15679\}$                                |
| 952:204  | $0, 0, 0, 0, e^{12}, e^{13}, e^{23} + e^{14}, e^{25} + e^{34}, e^{15} + e^{36}$  | $1/8(0, 6, 3, 9, 6, 3, 9, 12, 6)$                   | $\{123579, 124569\}$                                              |
| 952:211a | $0, 0, 0, 0, e^{12}, e^{13}, e^{34}, e^{25} + e^{14}, e^{15} + e^{24} + e^{36}$  | $3/7(1, 1, 1, 2, 2, 2, 3, 3, 3)$                    | $\{123489, 1246789, 346, 47\}$                                    |
| 952:211b | $0, 0, 0, 0, e^{12}, e^{13}, e^{34}, e^{25} - e^{14}, e^{36} + e^{24} + e^{15}$  | $3/7(1, 1, 1, 2, 2, 2, 3, 3, 3)$                    | $\{123489, 1246789, 346, 47\}$                                    |
| 952:218a | $0, 0, 0, 0, e^{12}, e^{13}, e^{23}, e^{15} + e^{34}, e^{25} + e^{14} + e^{36}$  | $17/37(1, 1, 1, 2, 2, 2, 2, 3, 3)$                  | $\{124689, 13459, 2458, 346\}$                                    |
| 952:218b | $0, 0, 0, 0, -e^{12}, e^{13}, e^{23}, e^{15} + e^{34}, e^{14} + e^{25} + e^{36}$ | $17/37(1, 1, 1, 2, 2, 2, 2, 3, 3)$                  | $\{124689, 13459, 2458, 346\}$                                    |
| 952:220  | $0, 0, 0, 0, e^{12}, e^{13}, e^{23}, e^{25} + e^{34}, e^{24} + e^{36} + e^{15}$  | $17/37(1, 1, 1, 2, 2, 2, 2, 3, 3)$                  | $\{123789, 7\}$                                                   |
| 952:223a | $0, 0, 0, 0, e^{12}, e^{13}, e^{24}, e^{15} + e^{23}, e^{25} + e^{14} + e^{36}$  | $1/4(1, 2, 2, 4, 3, 3, 6, 4, 5)$                    | $\{123489, 134579, 234568, 3467\}$                                |
| 952:223b | $0, 0, 0, 0, -e^{12}, e^{13}, e^{24}, e^{23} + e^{15}, e^{36} + e^{25} + e^{14}$ | $1/4(1, 2, 2, 4, 3, 3, 6, 4, 5)$                    | $\{123489, 134579, 234568, 3467\}$                                |
| 952:225  | $0, 0, 0, 0, e^{12}, e^{13}, e^{24}, e^{15} + e^{23}, e^{25} + e^{16} + e^{34}$  | $23/134(2, 3, 4, 4, 5, 6, 7, 7, 8)$                 | $\{\emptyset, 2578\}$                                             |
| 952:226a | $0, 0, 0, 0, e^{12}, e^{13}, e^{34}, e^{15} + e^{23}, e^{14} + e^{36} + e^{25}$  | $1/4(1, 2, 2, 4, 3, 3, 6, 4, 5)$                    | $\{123489, 13459, 234568, 346\}$                                  |
| 952:226b | $0, 0, 0, 0, -e^{12}, e^{13}, e^{34}, e^{15} + e^{23}, e^{25} + e^{14} + e^{36}$ | $1/4(1, 2, 2, 4, 3, 3, 6, 4, 5)$                    | $\{123489, 13459, 234568, 346\}$                                  |
| 952:228  | $0, 0, 0, 0, e^{12}, e^{13}, e^{23} + e^{14}, e^{25} + e^{16}, e^{36} + e^{15}$  | $8/17(1, 1, 1, 1, 2, 2, 2, 3, 3)$                   | $\{156789, 234567\}$                                              |
| 952:235  | $0, 0, 0, 0, e^{12}, e^{13}, e^{24}, e^{36} + e^{15}, e^{34} + e^{25} + e^{16}$  | $3/7(1, 1, 1, 2, 2, 2, 3, 3, 3)$                    | $\{1345789, 245\}$                                                |
| 952:241  | $0, 0, 0, 0, e^{12}, e^{13}, e^{23}, e^{16} + e^{25}, e^{36} + e^{15} + e^{24}$  | $17/37(1, 1, 1, 2, 2, 2, 2, 3, 3)$                  | $\{134589, 245\}$                                                 |
| 952:259a | $0, 0, 0, 0, e^{12}, e^{13}, e^{23}, e^{15}, e^{34} + e^{27} + e^{16}$           | $1/7(3, 3, 4, 6, 6, 7, 7, 9, 10)$                   | $\{\emptyset, 12389, 12678, 13579, 156, 235689, 2578, 3679\}$     |
| 952:259b | $0, 0, 0, 0, e^{12}, -e^{13}, e^{23}, e^{15}, e^{34} + e^{27} + e^{16}$          | $1/7(3, 3, 4, 6, 6, 7, 7, 9, 10)$                   | $\{\emptyset, 12389, 12678, 13579, 156, 235689, 2578, 3679\}$     |
| 952:263  | $0, 0, 0, 0, e^{12}, e^{13}, e^{23}, e^{25} + e^{14}, e^{16} + e^{37}$           | $1/54(25, 24, 26, 48, 49, 51, 50, 73, 76)$          | $\{\emptyset, 12389, 1568, 23569\}$                               |
| 952:264  | $0, 0, 0, 0, e^{12}, e^{13}, e^{23}, e^{15} + e^{24}, e^{16} + e^{37}$           | $17/37(1, 1, 1, 2, 2, 2, 2, 3, 3)$                  | $\{12789, 13567, 256789, 37\}$                                    |
| 952:265a | $0, 0, 0, 0, e^{12}, e^{13}, e^{23}, e^{15} + e^{34}, e^{16} + e^{27}$           | $1/149(67, 67, 76, 125, 134, 143, 143, 201, 210)$   | $\{\emptyset, 12389, 124678, 134579, 156, 235689, 24578, 34679\}$ |
| 952:265b | $0, 0, 0, 0, e^{12}, -e^{13}, e^{23}, e^{34} + e^{15}, e^{27} + e^{16}$          | $1/149(67, 67, 76, 125, 134, 143, 143, 201, 210)$   | $\{\emptyset, 12389, 124678, 134579, 156, 235689, 24578, 34679\}$ |
| 952:267  | $0, 0, 0, 0, e^{12}, e^{13}, e^{23}, e^{15} + e^{34}, e^{16} + e^{37}$           | $1/59(27, 28, 26, 56, 55, 53, 54, 82, 80)$          | $\{124789, 134567, 2456789, 347\}$                                |
| 952:268  | $0, 0, 0, 0, e^{12}, e^{13}, e^{23}, e^{34} + e^{15}, e^{36} + e^{27}$           | $1/117(53, 54, 55, 105, 107, 108, 109, 160, 163)$   | $\{\emptyset, 12389, 134579, 24578\}$                             |
| 952:282  | $0, 0, 0, 0, e^{12}, e^{13}, e^{23}, e^{15} + e^{34}, e^{14} + e^{27} + e^{36}$  | $17/37(1, 1, 1, 2, 2, 2, 2, 3, 3)$                  | $\{134579, 24578\}$                                               |
| 952:285  | $0, 0, 0, 0, e^{12}, e^{13}, e^{23}, e^{15} + e^{34}, e^{16} + e^{25} + e^{37}$  | $17/37(1, 1, 1, 2, 2, 2, 2, 3, 3)$                  | $\{124789, 347\}$                                                 |
| 952:287a | $0, 0, 0, 0, e^{12}, e^{13}, e^{23}, e^{25} + e^{16}, e^{37} + e^{24} + e^{15}$  | $17/37(1, 1, 1, 2, 2, 2, 2, 3, 3)$                  | $\{\emptyset, 12389, 13578, 2579\}$                               |
| 952:287b | $0, 0, 0, 0, -e^{12}, e^{13}, e^{23}, e^{25} + e^{16}, e^{24} + e^{37} + e^{15}$ | $17/37(1, 1, 1, 2, 2, 2, 2, 3, 3)$                  | $\{\emptyset, 12389, 13578, 2579\}$                               |
| 952:292a | $0, 0, 0, 0, e^{12}, e^{13}, e^{23}, e^{36} + e^{25}, e^{37} + e^{24} + e^{15}$  | $17/37(1, 1, 1, 2, 2, 2, 2, 3, 3)$                  | $\{\emptyset, 12389, 126789, 13578, 1568, 23569, 2579, 367\}$     |

Table A.2 – Continued to next page

Table A.2 – Continued from previous page

| Name     | $g$                                                                               | $N$                                                | Signatures $S$                                                                                                        |
|----------|-----------------------------------------------------------------------------------|----------------------------------------------------|-----------------------------------------------------------------------------------------------------------------------|
| 952:292b | $0, 0, 0, 0, e^{12}, -e^{13}, e^{23}, e^{25} + e^{36}, e^{15} + e^{37} + e^{24}$  | $17/37(1, 1, 1, 2, 2, 2, 2, 3, 3)$                 | $\{\emptyset, 12389, 126789, 13578, 1568, 23569, 2579, 367\}$                                                         |
| 952:292c | $0, 0, 0, 0, -e^{12}, e^{13}, e^{23}, e^{36} + e^{25}, e^{15} + e^{24} + e^{37}$  | $17/37(1, 1, 1, 2, 2, 2, 2, 3, 3)$                 | $\{\emptyset, 12389, 126789, 13578, 1568, 23569, 2579, 367\}$                                                         |
| 952:292d | $0, 0, 0, 0, -e^{12}, -e^{13}, e^{23}, e^{25} + e^{36}, e^{15} + e^{24} + e^{37}$ | $17/37(1, 1, 1, 2, 2, 2, 2, 3, 3)$                 | $\{\emptyset, 12389, 126789, 13578, 1568, 23569, 2579, 367\}$                                                         |
| 952:293a | $0, 0, 0, 0, e^{12}, e^{13}, e^{23}, e^{25} + e^{36}, e^{15} + e^{34} + e^{27}$   | $17/37(1, 1, 1, 2, 2, 2, 2, 3, 3)$                 | $\{\emptyset, 12389, 1568, 23569\}$                                                                                   |
| 952:293b | $0, 0, 0, 0, -e^{12}, e^{13}, e^{23}, e^{36} + e^{25}, e^{34} + e^{15} + e^{27}$  | $17/37(1, 1, 1, 2, 2, 2, 2, 3, 3)$                 | $\{\emptyset, 12389, 1568, 23569\}$                                                                                   |
| 952:313  | $0, 0, 0, 0, e^{12}, e^{34}, e^{13}, e^{15}, e^{36}$                              | $1/5(2, 3, 2, 3, 5, 5, 4, 7, 7)$                   | $\{1234789, 123678, 124689, 128, 134579, 13567, 14569, 15, 234589, 23568, 2456789, 2578, 349, 36, 4679, 7\}$          |
| 952:315  | $0, 0, 0, 0, e^{12}, e^{34}, e^{13}, e^{25}, e^{46}$                              | $4/21(3, 2, 3, 2, 5, 5, 6, 7, 7)$                  | $\{\emptyset, 123489, 123689, 124678, 1278, 134589, 135689, 145678, 1578, 234579, 235679, 2456, 25, 3479, 3679, 46\}$ |
| 952:316  | $0, 0, 0, 0, e^{12}, e^{34}, e^{13} + e^{24}, e^{15}, e^{36}$                     | $8/17(1, 1, 1, 1, 2, 2, 2, 3, 3)$                  | $\{123678, 124689, 134579, 15, 234589, 2578, 36, 4679\}$                                                              |
| 952:318  | $0, 0, 0, 0, e^{12}, e^{34}, e^{13}, e^{15} + e^{23}, e^{36}$                     | $1/4(1, 3, 2, 2, 4, 4, 3, 5, 6)$                   | $\{1234789, 123678, 134579, 13567, 234589, 23568, 349, 36\}$                                                          |
| 952:320  | $0, 0, 0, 0, e^{12}, e^{34}, e^{13}, e^{15}, e^{24} + e^{36}$                     | $1/21(8, 14, 7, 14, 22, 21, 15, 30, 28)$           | $\{1234789, 123678, 124689, 128, 234589, 23568, 2456789, 2578\}$                                                      |
| 952:322  | $0, 0, 0, 0, e^{12}, e^{34}, e^{13}, e^{25}, e^{23} + e^{46}$                     | $4/17(2, 2, 3, 1, 4, 4, 5, 6, 5)$                  | $\{123489, 123689, 124678, 1278, 234579, 235679, 2456, 25\}$                                                          |
| 952:323  | $0, 0, 0, 0, e^{12}, e^{34}, e^{13}, e^{25}, e^{24} + e^{36}$                     | $1/21(14, 8, 4, 17, 22, 21, 18, 30, 25)$           | $\{1234789, 123678, 124689, 128, 23459, 2356, 245679, 257\}$                                                          |
| 952:324  | $0, 0, 0, 0, e^{12}, e^{34}, e^{13}, e^{15}, e^{25} + e^{36}$                     | $1/31(13, 16, 13, 19, 29, 32, 26, 42, 45)$         | $\{1234789, 124689, 134579, 14569, 23568, 2578, 36, 7\}$                                                              |
| 952:325  | $0, 0, 0, 0, e^{12}, e^{34}, e^{13}, e^{25}, e^{15} + e^{36}$                     | $1/57(31, 21, 23, 37, 52, 60, 54, 73, 83)$         | $\{1234789, 124689, 135678, 158, 23459, 245679, 36, 7\}$                                                              |
| 952:326  | $0, 0, 0, 0, e^{12}, e^{34}, e^{13}, e^{15}, e^{46} + e^{25}$                     | $1/123(46, 65, 80, 48, 111, 128, 126, 157, 176)$   | $\{\emptyset, 123489, 123689, 13459, 13569, 24568, 258, 46\}$                                                         |
| 952:327  | $0, 0, 0, 0, e^{12}, e^{34}, e^{13}, e^{25}, e^{15} + e^{46}$                     | $1/10(5, 4, 6, 4, 9, 10, 11, 13, 14)$              | $\{\emptyset, 123489, 123689, 145678, 1578, 234579, 235679, 46\}$                                                     |
| 952:328  | $0, 0, 0, 0, e^{12}, e^{34}, e^{14} + e^{23}, e^{13} + e^{25}, e^{36}$            | $4/13(2, 1, 2, 1, 3, 3, 3, 4, 5)$                  | $\{123678, 134589, 234579, 36\}$                                                                                      |
| 952:331  | $0, 0, 0, 0, e^{12}, e^{34}, e^{14} + e^{23}, e^{15}, e^{36} + e^{25}$            | $1/211(75, 117, 89, 131, 192, 220, 206, 267, 309)$ | $\{124689, 13459, 258, 36\}$                                                                                          |
| 952:338  | $0, 0, 0, 0, e^{12}, e^{34}, e^{13}, e^{15} + e^{23}, e^{36} + e^{14}$            | $(0, 1, 0, 1, 1, 1, 0, 1, 1)$                      | $\{1234789, 123678, 134579, 13567\}$                                                                                  |
| 952:339  | $0, 0, 0, 0, e^{12}, e^{34}, e^{13}, e^{15} + e^{23}, e^{24} + e^{36}$            | $1/33(7, 28, 14, 19, 35, 33, 21, 42, 47)$          | $\{1234789, 123678, 234589, 23568\}$                                                                                  |
| 952:340  | $0, 0, 0, 0, e^{12}, e^{34}, e^{13}, e^{25} + e^{14}, e^{46} + e^{23}$            | $4/5(1, 0, 1, 0, 1, 1, 2, 1, 1)$                   | $\{123489, 124678, 234579, 2456\}$                                                                                    |
| 952:341  | $0, 0, 0, 0, e^{12}, e^{34}, e^{13}, e^{15} + e^{24}, e^{46} + e^{23}$            | $1/121(24, 96, 79, 48, 120, 127, 103, 144, 175)$   | $\{134579, 1456, 349, 467\}$                                                                                          |
| 952:342  | $0, 0, 0, 0, e^{12}, e^{34}, e^{13}, e^{23} + e^{15}, e^{36} + e^{25}$            | $1/49(13, 32, 26, 25, 45, 51, 39, 58, 77)$         | $\{1234789, 134579, 23568, 36\}$                                                                                      |
| 952:343  | $0, 0, 0, 0, e^{12}, e^{34}, e^{13}, e^{15}, e^{36} + e^{25} + e^{14}$            | $1/49(26, 19, 13, 38, 45, 51, 39, 71, 64)$         | $\{1234789, 124689, 134579, 14569\}$                                                                                  |
| 952:344  | $0, 0, 0, 0, e^{12}, e^{34}, e^{13}, e^{25}, e^{15} + e^{23} + e^{46}$            | $1/8(3, 4, 6, 2, 7, 8, 9, 11, 10)$                 | $\{123489, 123689, 234579, 235679\}$                                                                                  |
| 952:345  | $0, 0, 0, 0, e^{12}, e^{34}, e^{13}, e^{25}, e^{36} + e^{24} + e^{15}$            | $1/109(47, 52, 26, 94, 99, 120, 73, 151, 146)$     | $\{1234789, 124689, 23459, 245679\}$                                                                                  |
| 952:346  | $0, 0, 0, 0, e^{12}, e^{34}, e^{13}, e^{15} + e^{23}, e^{25} + e^{46}$            | $1/111(38, 61, 76, 42, 99, 118, 114, 137, 160)$    | $\{123489, 123689, 13459, 13569\}$                                                                                    |
| 952:347  | $0, 0, 0, 0, e^{12}, e^{34}, e^{13}, e^{14} + e^{25}, e^{15} + e^{36}$            | $1/41(23, 14, 16, 28, 37, 44, 39, 51, 60)$         | $\{1234789, 124689, 23459, 245679\}$                                                                                  |
| 952:348  | $0, 0, 0, 0, e^{12}, e^{34}, e^{13}, e^{15} + e^{24}, e^{25} + e^{36}$            | $1/127(44, 73, 51, 88, 117, 139, 95, 161, 190)$    | $\{1234789, 124689, 134579, 14569\}$                                                                                  |
| 952:349  | $0, 0, 0, 0, e^{12}, e^{34}, e^{13}, e^{25} + e^{14}, e^{46} + e^{15}$            | $1/8(5, 2, 4, 4, 7, 8, 9, 9, 12)$                  | $\{123489, 145678, 234579, 46\}$                                                                                      |
| 952:350  | $0, 0, 0, 0, e^{12}, e^{34}, e^{13}, e^{24} + e^{15}, e^{46} + e^{25}$            | $1/71(16, 47, 46, 32, 63, 78, 62, 79, 110)$        | $\{1234789, 134579, 245678, 467\}$                                                                                    |
| 952:351  | $0, 0, 0, 0, e^{12}, e^{34}, e^{13}, e^{36} + e^{15}, e^{25} + e^{46}$            | $1/81(39, 37, 39, 37, 76, 76, 78, 115, 113)$       | $\{1234789, 135679, 245678, 7\}$                                                                                      |
| 952:352  | $0, 0, 0, 0, e^{12}, e^{34}, e^{13}, e^{36} + e^{25}, e^{46} + e^{15}$            | $8/17(1, 1, 1, 1, 2, 2, 2, 3, 3)$                  | $\{1234789, 14568, 23569, 7\}$                                                                                        |
| 952:358  | $0, 0, 0, 0, e^{12}, e^{34}, e^{23} + e^{14}, e^{13} + e^{25}, e^{46} + e^{15}$   | $31/379(7, 4, 8, 5, 11, 13, 12, 15, 18)$           | $\{123689, 23459\}$                                                                                                   |
| 952:371a | $0, 0, 0, 0, e^{12}, e^{34}, e^{24} + e^{13}, e^{36} + e^{15}, e^{25} + e^{46}$   | $8/17(1, 1, 1, 1, 2, 2, 2, 3, 3)$                  | $\{1234789, 135679, 245678, 7\}$                                                                                      |
| 952:371b | $0, 0, 0, 0, e^{12}, e^{34}, -e^{13} + e^{24}, e^{36} + e^{15}, e^{46} + e^{25}$  | $8/17(1, 1, 1, 1, 2, 2, 2, 3, 3)$                  | $\{1234789, 135679, 245678, 7\}$                                                                                      |
| 952:375  | $0, 0, 0, 0, e^{12}, e^{34}, e^{13}, e^{15} + e^{23}, e^{36} + e^{25} + e^{14}$   | $1/5(0, 3, 0, 6, 3, 6, 0, 3, 6)$                   | $\{1234789, 134579\}$                                                                                                 |
| 952:376  | $0, 0, 0, 0, e^{12}, e^{34}, e^{13}, e^{25} + e^{14}, e^{15} + e^{23} + e^{46}$   | $1/2(1, 0, 2, 0, 1, 2, 3, 1, 2)$                   | $\{123489, 234579\}$                                                                                                  |
| 952:377a | $0, 0, 0, 0, e^{12}, e^{34}, e^{13}, e^{25} + e^{14}, e^{36} + e^{24} + e^{15}$   | $11/49(2, 2, 1, 4, 4, 5, 3, 6, 6)$                 | $\{1234789, 124689, 23459, 245679\}$                                                                                  |
| 952:377b | $0, 0, 0, 0, e^{12}, e^{34}, e^{13}, e^{25} - e^{14}, e^{15} + e^{36} + e^{24}$   | $11/49(2, 2, 1, 4, 4, 5, 3, 6, 6)$                 | $\{1234789, 124689, 23459, 245679\}$                                                                                  |
| 952:378a | $0, 0, 0, 0, e^{12}, e^{34}, e^{13}, e^{15} + e^{24}, e^{14} + e^{36} + e^{25}$   | $11/49(2, 2, 1, 4, 4, 5, 3, 6, 6)$                 | $\{1234789, 124689, 134579, 14569\}$                                                                                  |
| 952:378b | $0, 0, 0, 0, e^{12}, e^{34}, e^{13}, -e^{15} + e^{24}, e^{36} + e^{25} + e^{14}$  | $11/49(2, 2, 1, 4, 4, 5, 3, 6, 6)$                 | $\{1234789, 124689, 134579, 14569\}$                                                                                  |
| 952:379  | $0, 0, 0, 0, e^{12}, e^{34}, e^{13}, e^{25} + e^{36}, e^{46} + e^{23} + e^{15}$   | $4/13(1, 2, 2, 1, 3, 3, 3, 5, 4)$                  | $\{1234789, 23569\}$                                                                                                  |
| 952:380  | $0, 0, 0, 0, e^{12}, e^{34}, e^{13}, e^{46} + e^{25}, e^{24} + e^{36} + e^{15}$   | $23/73(1, 2, 1, 2, 3, 3, 2, 5, 4)$                 | $\{1234789, 245679\}$                                                                                                 |
| 952:401  | $0, 0, 0, 0, e^{12}, e^{13}, e^{24}, e^{15}, e^{27} + e^{16}$                     | $1/139(53, 57, 99, 91, 110, 152, 148, 163, 205)$   | $\{123459, 12567, 134789, 168, 23469, 27, 3456789, 58\}$                                                              |

Table A.2 – Continued to next page

Table A.2 – Continued from previous page

| Name     | $g$                                                                     | $N$                                                  | Signatures $S$                                                                                                        |
|----------|-------------------------------------------------------------------------|------------------------------------------------------|-----------------------------------------------------------------------------------------------------------------------|
| 952:402  | $0, 0, 0, 0, e^{12}, e^{13}, e^{14}, e^{15}, e^{17} + e^{36}$           | $1/83(20, 63, 46, 72, 83, 66, 92, 103, 112)$         | $\{\emptyset, 123489, 124689, 13459, 14569, 23568, 258, 36\}$                                                         |
| 952:403  | $0, 0, 0, 0, e^{12}, e^{13}, e^{14}, e^{25}, e^{17} + e^{36}$           | $1/93(30, 47, 51, 72, 77, 81, 102, 124, 132)$        | $\{\emptyset, 123489, 124689, 134589, 145689, 2356, 25, 36\}$                                                         |
| 952:404  | $0, 0, 0, 0, e^{12}, e^{13}, e^{24}, e^{15}, e^{36} + e^{27}$           | $1/23(10, 9, 12, 16, 19, 22, 25, 29, 34)$            | $\{\emptyset, 123489, 124689, 134579, 145679, 235678, 2578, 36\}$                                                     |
| 952:405  | $0, 0, 0, 0, e^{12}, e^{13}, e^{24}, e^{25}, e^{36} + e^{27}$           | $1/41(24, 13, 17, 32, 37, 41, 45, 50, 58)$           | $\{\emptyset, 123489, 124689, 1345789, 1456789, 23567, 257, 36\}$                                                     |
| 952:406  | $0, 0, 0, 0, e^{12}, e^{13}, e^{34}, e^{15}, e^{37} + e^{16}$           | $1/21(10, 11, 8, 12, 21, 18, 20, 31, 28)$            | $\{1234689, 128, 134569, 15, 234589, 2568, 349, 6\}$                                                                  |
| 952:407  | $0, 0, 0, 0, e^{12}, e^{13}, e^{34}, e^{25}, e^{37} + e^{16}$           | $1/57(30, 23, 21, 39, 53, 51, 60, 76, 81)$           | $\{\emptyset, 123489, 1268, 134589, 1568, 234569, 25, 3469\}$                                                         |
| 952:408a | $0, 0, 0, 0, e^{12}, e^{13}, e^{14}, e^{15}, e^{47} + e^{36}$           | $1/8(2, 6, 5, 5, 8, 7, 7, 10, 12)$                   | $\{\emptyset, 123489, 123789, 124689, 126789, 13459, 13579, 14569, 15679, 2345678, 23568, 24578, 258, 3467, 36, 47\}$ |
| 952:408b | $0, 0, 0, 0, e^{12}, -e^{13}, e^{14}, e^{15}, e^{36} + e^{47}$          | $1/8(2, 6, 5, 5, 8, 7, 7, 10, 12)$                   | $\{\emptyset, 123489, 123789, 124689, 126789, 13459, 13579, 14569, 15679, 2345678, 23568, 24578, 258, 3467, 36, 47\}$ |
| 952:410a | $0, 0, 0, 0, e^{12}, e^{13}, e^{14}, e^{25}, e^{47} + e^{36}$           | $1/60(24, 28, 33, 33, 52, 57, 57, 80, 90)$           | $\{\emptyset, 123489, 123789, 124689, 126789, 134589, 135789, 145689, 156789, 234567, 2356, 2457, 25, 3467, 36, 47\}$ |
| 952:410b | $0, 0, 0, 0, e^{12}, -e^{13}, e^{14}, e^{25}, e^{36} + e^{47}$          | $1/60(24, 28, 33, 33, 52, 57, 57, 80, 90)$           | $\{\emptyset, 123489, 123789, 124689, 126789, 134589, 135789, 145689, 156789, 234567, 2356, 2457, 25, 3467, 36, 47\}$ |
| 952:412  | $0, 0, 0, 0, e^{12}, e^{13}, e^{24}, e^{15}, e^{36} + e^{47}$           | $1/44(16, 24, 25, 21, 40, 41, 45, 56, 66)$           | $\{\emptyset, 123489, 123789, 124689, 126789, 3467, 36, 47\}$                                                         |
| 952:415a | $0, 0, 0, 0, e^{12}, e^{13}, e^{34}, e^{25}, e^{16} + e^{47}$           | $1/9(4, 4, 5, 4, 8, 9, 9, 12, 13)$                   | $\{\emptyset, 123489, 123789, 124678, 1268, 134589, 135789, 145678, 1568, 234569, 235679, 2457, 25, 3469, 3679, 47\}$ |
| 952:415b | $0, 0, 0, 0, e^{12}, -e^{13}, e^{34}, e^{25}, e^{47} + e^{16}$          | $1/9(4, 4, 5, 4, 8, 9, 9, 12, 13)$                   | $\{\emptyset, 123489, 123789, 124678, 1268, 134589, 135789, 145678, 1568, 234569, 235679, 2457, 25, 3469, 3679, 47\}$ |
| 952:417  | $0, 0, 0, 0, e^{12}, e^{13}, e^{34}, e^{15}, e^{36} + e^{47}$           | $1/123(40, 83, 68, 54, 123, 108, 122, 163, 176)$     | $\{\emptyset, 123489, 123789, 13459, 13579, 24578, 258, 47\}$                                                         |
| 952:418  | $0, 0, 0, 0, e^{12}, e^{13}, e^{34}, e^{25}, e^{47} + e^{36}$           | $1/18(10, 7, 8, 9, 17, 18, 17, 24, 26)$              | $\{\emptyset, 123489, 123789, 134589, 135789, 2457, 25, 47\}$                                                         |
| 952:425  | $0, 0, 0, 0, e^{12}, e^{13}, e^{24}, e^{15} + e^{23}, e^{16} + e^{27}$  | $3/65(8, 9, 16, 14, 17, 24, 23, 25, 32)$             | $\{12567, 168, 27, 58\}$                                                                                              |
| 952:426  | $0, 0, 0, 0, e^{12}, e^{13}, e^{14}, e^{15} + e^{23}, e^{17} + e^{36}$  | $1/11(3, 8, 6, 9, 11, 9, 12, 14, 15)$                | $\{\emptyset, 124689, 14569, 258\}$                                                                                   |
| 952:427  | $0, 0, 0, 0, e^{12}, e^{13}, e^{24}, e^{23} + e^{15}, e^{36} + e^{27}$  | $3/19(2, 3, 4, 5, 6, 7, 7, 10)$                      | $\{123489, 134579, 235678, 36\}$                                                                                      |
| 952:428  | $0, 0, 0, 0, e^{12}, e^{13}, e^{34}, e^{23} + e^{15}, e^{37} + e^{16}$  | $1/3(1, 2, 2, 0, 3, 3, 2, 4, 4)$                     | $\{1234689, 134569, 234589, 349\}$                                                                                    |
| 952:429  | $0, 0, 0, 0, e^{12}, e^{13}, e^{14}, e^{15}, e^{47} + e^{23} + e^{16}$  | $1/461(146, 292, 360, 253, 438, 506, 399, 584, 652)$ | $\{124689, 126789, 2345678, 23568\}$                                                                                  |
| 952:430  | $0, 0, 0, 0, e^{12}, e^{13}, e^{14}, e^{25}, e^{23} + e^{47} + e^{16}$  | $4/587(40, 80, 122, 81, 120, 162, 121, 200, 202)$    | $\{123489, 123789, 2457, 25\}$                                                                                        |
| 952:431  | $0, 0, 0, 0, e^{12}, e^{13}, e^{24}, e^{15}, e^{16} + e^{47} + e^{23}$  | $1/241(73, 146, 192, 96, 219, 265, 242, 292, 338)$   | $\{123489, 123789, 2345689, 2356789\}$                                                                                |
| 952:432  | $0, 0, 0, 0, e^{12}, e^{13}, e^{24}, e^{15}, e^{27} + e^{36} + e^{14}$  | $1/19(10, 5, 8, 16, 15, 18, 21, 25, 26)$             | $\{123489, 124689, 134579, 145679\}$                                                                                  |
| 952:433  | $0, 0, 0, 0, e^{12}, e^{13}, e^{24}, e^{15}, e^{16} + e^{34} + e^{27}$  | $1/61(22, 23, 46, 44, 45, 68, 67, 67, 90)$           | $\{123459, 134789, 23469, 3456789\}$                                                                                  |
| 952:434  | $0, 0, 0, 0, e^{12}, e^{13}, e^{14}, e^{15} + e^{23}, e^{47} + e^{16}$  | $1/81(28, 53, 56, 42, 81, 84, 70, 109, 112)$         | $\{\emptyset, 24578, 258, 47\}$                                                                                       |
| 952:435  | $0, 0, 0, 0, e^{12}, e^{13}, e^{24}, e^{23} + e^{15}, e^{47} + e^{16}$  | $1/283(101, 156, 202, 124, 257, 303, 280, 358, 404)$ | $\{\emptyset, 14567, 156, 47\}$                                                                                       |
| 952:436a | $0, 0, 0, 0, e^{12}, e^{13}, e^{14}, e^{23} + e^{15}, e^{47} + e^{36}$  | $1/27(8, 19, 16, 16, 27, 24, 24, 35, 40)$            | $\{\emptyset, 124689, 126789, 14569, 15679, 24578, 258, 47\}$                                                         |
| 952:436b | $0, 0, 0, 0, e^{12}, -e^{13}, e^{14}, e^{15} + e^{23}, e^{36} + e^{47}$ | $1/27(8, 19, 16, 16, 27, 24, 24, 35, 40)$            | $\{\emptyset, 124689, 126789, 14569, 15679, 24578, 258, 47\}$                                                         |
| 952:438  | $0, 0, 0, 0, e^{12}, e^{13}, e^{24}, e^{15} + e^{23}, e^{36} + e^{47}$  | $2/151(23, 45, 46, 35, 68, 69, 80, 91, 115)$         | $\{123489, 123789, 3467, 36\}$                                                                                        |
| 952:440  | $0, 0, 0, 0, e^{12}, e^{13}, e^{34}, e^{15}, e^{16} + e^{24} + e^{37}$  | $1/17(8, 10, 5, 11, 18, 13, 16, 26, 21)$             | $\{1234689, 128, 234589, 2568\}$                                                                                      |
| 952:442a | $0, 0, 0, 0, e^{12}, e^{13}, e^{34}, e^{25}, e^{23} + e^{16} + e^{47}$  | $1/7(2, 4, 5, 2, 6, 7, 7, 10, 9)$                    | $\{123489, 123789, 124678, 1268, 234569, 235679, 2457, 25\}$                                                          |
| 952:442b | $0, 0, 0, 0, e^{12}, -e^{13}, e^{34}, e^{25}, e^{16} + e^{23} + e^{47}$ | $1/7(2, 4, 5, 2, 6, 7, 7, 10, 9)$                    | $\{123489, 123789, 124678, 1268, 234569, 235679, 2457, 25\}$                                                          |
| 952:443  | $0, 0, 0, 0, e^{12}, e^{13}, e^{34}, e^{25}, e^{37} + e^{24} + e^{16}$  | $10/133(7, 6, 3, 11, 13, 10, 14, 19, 17)$            | $\{123678, 124789, 2357, 245679\}$                                                                                    |
| 952:447  | $0, 0, 0, 0, e^{12}, e^{13}, e^{34}, e^{23} + e^{15}, e^{36} + e^{47}$  | $1/111(32, 79, 64, 48, 111, 96, 112, 143, 160)$      | $\{123489, 123789, 13459, 13579\}$                                                                                    |
| 952:448  | $0, 0, 0, 0, e^{12}, e^{13}, e^{24}, e^{15} + e^{34}, e^{27} + e^{16}$  | $1/277(113, 120, 180, 166, 233, 293, 286, 346, 406)$ | $\{123459, 12567, 23469, 27\}$                                                                                        |
| 952:449  | $0, 0, 0, 0, e^{12}, e^{13}, e^{14}, e^{15} + e^{34}, e^{17} + e^{36}$  | $1/449(125, 339, 238, 351, 464, 363, 476, 589, 601)$ | $\{\emptyset, 124689, 13459, 23568\}$                                                                                 |
| 952:450  | $0, 0, 0, 0, e^{12}, e^{13}, e^{14}, e^{25} + e^{34}, e^{17} + e^{36}$  | $28/611(7, 11, 12, 17, 18, 19, 24, 29, 31)$          | $\{123489, 134589, 2356, 36\}$                                                                                        |
| 952:451  | $0, 0, 0, 0, e^{12}, e^{13}, e^{24}, e^{34} + e^{15}, e^{36} + e^{27}$  | $8/619(33, 30, 41, 55, 63, 74, 85, 96, 115)$         | $\{123489, 145679, 2578, 36\}$                                                                                        |
| 952:452  | $0, 0, 0, 0, e^{12}, e^{13}, e^{24}, e^{25} + e^{34}, e^{36} + e^{27}$  | $1/67(39, 21, 28, 53, 60, 67, 74, 81, 95)$           | $\{123489, 1345789, 23567, 36\}$                                                                                      |
| 952:453  | $0, 0, 0, 0, e^{12}, e^{13}, e^{34}, e^{25} + e^{14}, e^{37} + e^{16}$  | $2/81(22, 15, 14, 30, 37, 36, 44, 52, 58)$           | $\{123489, 134589, 234569, 3469\}$                                                                                    |
| 952:454  | $0, 0, 0, 0, e^{12}, e^{13}, e^{34}, e^{15} + e^{24}, e^{37} + e^{16}$  | $1/2(1, 1, 0, 2, 2, 1, 2, 3, 2)$                     | $\{1234689, 134569, 234589, 349\}$                                                                                    |

Table A.2 – Continued to next page

Table A.2 – Continued from previous page

| Name     | $g$                                                                              | $N$                                                  | Signatures $S$                                                                                                        |
|----------|----------------------------------------------------------------------------------|------------------------------------------------------|-----------------------------------------------------------------------------------------------------------------------|
| 952:457a | $0, 0, 0, 0, e^{12}, e^{13}, e^{14}, e^{34} + e^{25}, e^{36} + e^{47}$           | $1/47(16, 21, 29, 29, 37, 45, 45, 58, 74)$           | $\{123489, 126789, 134589, 156789, 2356, 2457, 36, 47\}$                                                              |
| 952:457b | $0, 0, 0, 0, e^{12}, -e^{13}, e^{14}, e^{34} + e^{25}, e^{36} + e^{47}$          | $1/47(16, 21, 29, 29, 37, 45, 45, 58, 74)$           | $\{123489, 126789, 134589, 156789, 2356, 2457, 36, 47\}$                                                              |
| 952:459  | $0, 0, 0, 0, e^{12}, e^{13}, e^{24}, e^{34} + e^{15}, e^{47} + e^{36}$           | $1/167(53, 87, 105, 88, 140, 158, 175, 193, 263)$    | $\{123489, 126789, 36, 47\}$                                                                                          |
| 952:460a | $0, 0, 0, 0, e^{12}, e^{13}, e^{34}, e^{14} + e^{25}, e^{47} + e^{16}$           | $1/7(4, 2, 3, 4, 6, 7, 7, 8, 11)$                    | $\{123489, 124678, 134589, 145678, 234569, 2457, 3469, 47\}$                                                          |
| 952:460b | $0, 0, 0, 0, e^{12}, -e^{13}, e^{34}, e^{25} + e^{14}, e^{47} + e^{16}$          | $1/7(4, 2, 3, 4, 6, 7, 7, 8, 11)$                    | $\{123489, 124678, 134589, 145678, 234569, 2457, 3469, 47\}$                                                          |
| 952:461a | $0, 0, 0, 0, e^{12}, e^{13}, e^{34}, e^{15} + e^{24}, e^{47} + e^{16}$           | $(0, 1, 1, 0, 1, 1, 1, 1, 1)$                        | $\{1234689, 12478, 134569, 1457, 234589, 245678, 349, 467\}$                                                          |
| 952:461b | $0, 0, 0, 0, e^{12}, -e^{13}, e^{34}, e^{24} + e^{15}, e^{16} + e^{47}$          | $(0, 1, 1, 0, 1, 1, 1, 1, 1)$                        | $\{1234689, 12478, 134569, 1457, 234589, 245678, 349, 467\}$                                                          |
| 952:464  | $0, 0, 0, 0, e^{12}, e^{13}, e^{34}, e^{25} + e^{14}, e^{47} + e^{36}$           | $28/209(5, 2, 3, 4, 7, 8, 7, 9, 11)$                 | $\{123489, 134589, 2457, 47\}$                                                                                        |
| 952:465  | $0, 0, 0, 0, e^{12}, e^{13}, e^{34}, e^{15} + e^{24}, e^{47} + e^{36}$           | $1/53(11, 42, 33, 22, 53, 44, 55, 64, 77)$           | $\{12478, 1457, 234589, 349\}$                                                                                        |
| 952:466a | $0, 0, 0, 0, e^{12}, e^{13}, e^{14}, e^{15}, e^{36} + e^{17} + e^{25}$           | $1/137(41, 79, 79, 117, 120, 120, 158, 161, 199)$    | $\{123789, 126789, 13579, 15679, 2345678, 24578, 3467, 47\}$                                                          |
| 952:466b | $0, 0, 0, 0, -e^{12}, e^{13}, e^{14}, e^{15}, e^{25} + e^{36} + e^{17}$          | $1/137(41, 79, 79, 117, 120, 120, 158, 161, 199)$    | $\{123789, 126789, 13579, 15679, 2345678, 24578, 3467, 47\}$                                                          |
| 952:469  | $0, 0, 0, 0, e^{12}, e^{13}, e^{24}, e^{25}, e^{36} + e^{15} + e^{27}$           | $2/177(49, 29, 39, 69, 78, 88, 98, 107, 127)$        | $\{\emptyset, 123489, 124689, 36\}$                                                                                   |
| 952:470  | $0, 0, 0, 0, e^{12}, e^{13}, e^{34}, e^{15}, e^{25} + e^{37} + e^{16}$           | $1/65(32, 29, 26, 38, 61, 58, 64, 93, 90)$           | $\{1234689, 134569, 2568, 6\}$                                                                                        |
| 952:471a | $0, 0, 0, 0, e^{12}, e^{13}, e^{14}, e^{15}, e^{47} + e^{36} + e^{25}$           | $1/25(7, 16, 16, 16, 23, 23, 23, 30, 39)$            | $\{\emptyset, 123489, 123789, 124689, 126789, 13459, 13579, 14569, 15679, 2345678, 23568, 24578, 258, 3467, 36, 47\}$ |
| 952:471b | $0, 0, 0, 0, e^{12}, -e^{13}, e^{14}, e^{15}, e^{36} + e^{47} + e^{25}$          | $1/25(7, 16, 16, 16, 23, 23, 23, 30, 39)$            | $\{\emptyset, 123489, 123789, 124689, 126789, 13459, 13579, 14569, 15679, 2345678, 23568, 24578, 258, 3467, 36, 47\}$ |
| 952:471c | $0, 0, 0, 0, -e^{12}, e^{13}, e^{14}, e^{15}, e^{25} + e^{47} + e^{36}$          | $1/25(7, 16, 16, 16, 23, 23, 23, 30, 39)$            | $\{\emptyset, 123489, 123789, 124689, 126789, 13459, 13579, 14569, 15679, 2345678, 23568, 24578, 258, 3467, 36, 47\}$ |
| 952:474a | $0, 0, 0, 0, e^{12}, e^{13}, e^{14}, e^{25}, e^{47} + e^{15} + e^{36}$           | $1/47(23, 21, 22, 22, 44, 45, 45, 65, 67)$           | $\{134589, 135789, 145689, 156789, 234567, 2356, 2457, 25\}$                                                          |
| 952:474b | $0, 0, 0, 0, e^{12}, -e^{13}, e^{14}, e^{25}, e^{15} + e^{36} + e^{47}$          | $1/47(23, 21, 22, 22, 44, 45, 45, 65, 67)$           | $\{134589, 135789, 145689, 156789, 234567, 2356, 2457, 25\}$                                                          |
| 952:482a | $0, 0, 0, 0, e^{12}, e^{13}, e^{34}, e^{15}, e^{36} + e^{47} + e^{25}$           | $2/39(7, 11, 11, 9, 18, 18, 20, 25, 29)$             | $\{\emptyset, 123489, 123789, 13459, 13579, 24578, 258, 47\}$                                                         |
| 952:482b | $0, 0, 0, 0, -e^{12}, e^{13}, e^{34}, e^{15}, e^{25} + e^{47} + e^{36}$          | $2/39(7, 11, 11, 9, 18, 18, 20, 25, 29)$             | $\{\emptyset, 123489, 123789, 13459, 13579, 24578, 258, 47\}$                                                         |
| 952:484  | $0, 0, 0, 0, e^{12}, e^{13}, e^{34}, e^{25}, e^{15} + e^{36} + e^{47}$           | $4/233(31, 23, 27, 29, 54, 58, 56, 77, 85)$          | $\{\emptyset, 123489, 123789, 47\}$                                                                                   |
| 952:486  | $0, 0, 0, 0, e^{12}, e^{13}, e^{24}, e^{16} + e^{25}, e^{27} + e^{15}$           | $8/17(1, 1, 1, 1, 2, 2, 2, 3, 3)$                    | $\{1234589, 138, 249, 5\}$                                                                                            |
| 952:487  | $0, 0, 0, 0, e^{12}, e^{13}, e^{14}, e^{15} + e^{36}, e^{17} + e^{25}$           | $4/587(53, 81, 67, 109, 134, 120, 162, 187, 215)$    | $\{134589, 145689, 2356, 25\}$                                                                                        |
| 952:491  | $0, 0, 0, 0, e^{12}, e^{13}, e^{34}, e^{16} + e^{25}, e^{37} + e^{15}$           | $1/681(335, 297, 259, 449, 632, 594, 708, 929, 967)$ | $\{124789, 158, 23459, 37\}$                                                                                          |
| 952:492  | $0, 0, 0, 0, e^{12}, e^{13}, e^{34}, e^{36} + e^{15}, e^{37} + e^{25}$           | $1/79(31, 43, 37, 43, 74, 68, 80, 105, 117)$         | $\{1234689, 124789, 37, 6\}$                                                                                          |
| 952:496a | $0, 0, 0, 0, e^{12}, e^{13}, e^{14}, e^{15} + e^{36}, e^{25} + e^{47}$           | $16/203(5, 7, 6, 7, 12, 11, 12, 17, 19)$             | $\{\emptyset, 123489, 123789, 124689, 126789, 3467, 36, 47\}$                                                         |
| 952:496b | $0, 0, 0, 0, -e^{12}, e^{13}, e^{14}, e^{36} + e^{15}, e^{25} + e^{47}$          | $16/203(5, 7, 6, 7, 12, 11, 12, 17, 19)$             | $\{\emptyset, 123489, 123789, 124689, 126789, 3467, 36, 47\}$                                                         |
| 952:501a | $0, 0, 0, 0, e^{12}, e^{13}, e^{24}, e^{36} + e^{15}, e^{47} + e^{25}$           | $8/17(1, 1, 1, 1, 2, 2, 2, 3, 3)$                    | $\{\emptyset, 123489, 123789, 124689, 126789, 3467, 36, 47\}$                                                         |
| 952:501b | $0, 0, 0, 0, e^{12}, -e^{13}, e^{24}, e^{36} + e^{15}, e^{47} + e^{25}$          | $8/17(1, 1, 1, 1, 2, 2, 2, 3, 3)$                    | $\{\emptyset, 123489, 123789, 124689, 126789, 3467, 36, 47\}$                                                         |
| 952:502a | $0, 0, 0, 0, e^{12}, e^{13}, e^{24}, e^{25} + e^{36}, e^{15} + e^{47}$           | $8/17(1, 1, 1, 1, 2, 2, 2, 3, 3)$                    | $\{\emptyset, 123489, 123789, 124689, 126789, 134578, 1358, 145678, 1568, 234569, 235679, 2459, 2579, 3467, 36, 47\}$ |
| 952:502b | $0, 0, 0, 0, e^{12}, -e^{13}, e^{24}, e^{25} + e^{36}, e^{15} + e^{47}$          | $8/17(1, 1, 1, 1, 2, 2, 2, 3, 3)$                    | $\{\emptyset, 123489, 123789, 124689, 126789, 134578, 1358, 145678, 1568, 234569, 235679, 2459, 2579, 3467, 36, 47\}$ |
| 952:502c | $0, 0, 0, 0, -e^{12}, -e^{13}, e^{24}, e^{25} + e^{36}, e^{15} + e^{47}$         | $8/17(1, 1, 1, 1, 2, 2, 2, 3, 3)$                    | $\{\emptyset, 123489, 123789, 124689, 126789, 134578, 1358, 145678, 1568, 234569, 235679, 2459, 2579, 3467, 36, 47\}$ |
| 952:505  | $0, 0, 0, 0, e^{12}, e^{13}, e^{34}, e^{16} + e^{25}, e^{15} + e^{47}$           | $4/233(25, 29, 33, 23, 54, 58, 56, 83, 79)$          | $\{\emptyset, 123489, 123789, 47\}$                                                                                   |
| 952:506  | $0, 0, 0, 0, e^{12}, e^{13}, e^{34}, e^{36} + e^{15}, e^{47} + e^{25}$           | $16/747(20, 24, 22, 23, 44, 42, 45, 64, 68)$         | $\{\emptyset, 123489, 123789, 47\}$                                                                                   |
| 952:507a | $0, 0, 0, 0, e^{12}, e^{13}, e^{34}, e^{25} + e^{36}, e^{15} + e^{47}$           | $8/17(1, 1, 1, 1, 2, 2, 2, 3, 3)$                    | $\{\emptyset, 123489, 123789, 145678, 1568, 234569, 235679, 47\}$                                                     |
| 952:507b | $0, 0, 0, 0, -e^{12}, e^{13}, e^{34}, e^{36} + e^{25}, e^{47} + e^{15}$          | $8/17(1, 1, 1, 1, 2, 2, 2, 3, 3)$                    | $\{\emptyset, 123489, 123789, 145678, 1568, 234569, 235679, 47\}$                                                     |
| 952:551  | $0, 0, 0, 0, e^{12}, e^{13}, e^{14}, e^{15} + e^{23}, e^{24} + e^{36} + e^{17}$  | $9/31(1, 2, 2, 3, 3, 3, 4, 5)$                       | $\{134579, 367\}$                                                                                                     |
| 952:552  | $0, 0, 0, 0, e^{12}, e^{13}, e^{24}, e^{15} + e^{23}, e^{27} + e^{36} + e^{14}$  | $1/7(2, 1, 4, 8, 3, 6, 9, 5, 10)$                    | $\{123489, 134579\}$                                                                                                  |
| 952:553a | $0, 0, 0, 0, e^{12}, e^{13}, e^{24}, e^{15} + e^{23}, e^{27} + e^{16} + e^{34}$  | $7/19(1, 1, 2, 2, 2, 3, 3, 4)$                       | $\{123459, 134789, 23469, 3456789\}$                                                                                  |
| 952:553b | $0, 0, 0, 0, -e^{12}, e^{13}, e^{24}, e^{15} + e^{23}, e^{27} + e^{16} + e^{34}$ | $7/19(1, 1, 2, 2, 2, 3, 3, 4)$                       | $\{123459, 134789, 23469, 3456789\}$                                                                                  |
| 952:554  | $0, 0, 0, 0, e^{12}, e^{13}, e^{34}, e^{15} + e^{23}, e^{16} + e^{24} + e^{37}$  | $9/37(1, 4, 2, 0, 5, 3, 2, 6, 4)$                    | $\{1234689, 234589\}$                                                                                                 |

Table A.2 – Continued to next page



Table A.2 – Continued from previous page

| Name     | $g$                                                                               | $N$                                      | Signatures $S$                                                    |
|----------|-----------------------------------------------------------------------------------|------------------------------------------|-------------------------------------------------------------------|
| 952:555  | $0, 0, 0, 0, e^{12}, e^{13}, e^{14}, e^{34} + e^{15}, e^{47} + e^{23} + e^{16}$   | $73/677(3, 6, 7, 5, 9, 10, 8, 12, 13)$   | $\{124689, 23568\}$                                               |
| 952:556  | $0, 0, 0, 0, e^{12}, e^{13}, e^{14}, e^{25} + e^{34}, e^{16} + e^{23} + e^{47}$   | $14/51(1, 2, 3, 2, 3, 4, 3, 5, 5)$       | $\{123789, 25\}$                                                  |
| 952:557  | $0, 0, 0, 0, e^{12}, e^{13}, e^{24}, e^{34} + e^{15}, e^{23} + e^{47} + e^{16}$   | $77/767(3, 6, 8, 4, 9, 11, 10, 12, 14)$  | $\{123489, 2345689\}$                                             |
| 952:558  | $0, 0, 0, 0, e^{12}, e^{13}, e^{24}, e^{34} + e^{15}, e^{27} + e^{36} + e^{14}$   | $44/511(6, 3, 5, 10, 9, 11, 13, 15, 16)$ | $\{123489, 145679\}$                                              |
| 952:559a | $0, 0, 0, 0, e^{12}, e^{13}, e^{34}, e^{25} + e^{14}, e^{23} + e^{47} + e^{16}$   | $(0, 0, 1, 0, 0, 1, 1, 0, 1)$            | $\{123489, 124678, 234569, 2457\}$                                |
| 952:559b | $0, 0, 0, 0, e^{12}, -e^{13}, e^{34}, e^{25} + e^{14}, e^{16} + e^{47} + e^{23}$  | $(0, 0, 1, 0, 0, 1, 1, 0, 1)$            | $\{123489, 124678, 234569, 2457\}$                                |
| 952:560  | $0, 0, 0, 0, e^{12}, e^{13}, e^{34}, e^{25} + e^{14}, e^{16} + e^{37} + e^{24}$   | $35/326(5, 4, 2, 8, 9, 7, 10, 13, 12)$   | $\{124789, 245679\}$                                              |
| 952:562a | $0, 0, 0, 0, e^{12}, e^{13}, e^{34}, e^{15} + e^{24}, e^{16} + e^{23} + e^{47}$   | $(0, 0, 1, 0, 0, 1, 1, 0, 1)$            | $\{134569, 1457, 349, 467\}$                                      |
| 952:562b | $0, 0, 0, 0, e^{12}, -e^{13}, e^{34}, e^{15} + e^{24}, e^{23} + e^{16} + e^{47}$  | $(0, 0, 1, 0, 0, 1, 1, 0, 1)$            | $\{134569, 1457, 349, 467\}$                                      |
| 952:564a | $0, 0, 0, 0, e^{12}, e^{13}, e^{14}, e^{23} + e^{15}, e^{25} + e^{36} + e^{17}$   | $9/31(1, 2, 2, 3, 3, 3, 4, 4, 5)$        | $\{123789, 13579, 2345678, 3467\}$                                |
| 952:564b | $0, 0, 0, 0, -e^{12}, e^{13}, e^{14}, e^{23} + e^{15}, e^{36} + e^{17} + e^{25}$  | $9/31(1, 2, 2, 3, 3, 3, 4, 4, 5)$        | $\{123789, 13579, 2345678, 3467\}$                                |
| 952:566  | $0, 0, 0, 0, e^{12}, e^{13}, e^{34}, e^{15} + e^{23}, e^{25} + e^{37} + e^{16}$   | $13/73(2, 3, 4, 0, 5, 6, 4, 7, 8)$       | $\{1234689, 134569\}$                                             |
| 952:567a | $0, 0, 0, 0, e^{12}, e^{13}, e^{14}, e^{15} + e^{23}, e^{47} + e^{16} + e^{25}$   | $43/237(2, 3, 4, 3, 5, 6, 5, 7, 8)$      | $\{\emptyset, 24578, 258, 47\}$                                   |
| 952:567b | $0, 0, 0, 0, -e^{12}, e^{13}, e^{14}, e^{15} + e^{23}, e^{47} + e^{16} + e^{25}$  | $43/237(2, 3, 4, 3, 5, 6, 5, 7, 8)$      | $\{\emptyset, 24578, 258, 47\}$                                   |
| 952:569  | $0, 0, 0, 0, e^{12}, e^{13}, e^{24}, e^{15} + e^{23}, e^{25} + e^{16} + e^{47}$   | $43/479(4, 6, 8, 5, 10, 12, 11, 14, 16)$ | $\{\emptyset, 47\}$                                               |
| 952:570a | $0, 0, 0, 0, e^{12}, e^{13}, e^{14}, e^{15} + e^{23}, e^{36} + e^{25} + e^{47}$   | $25/81(1, 2, 2, 2, 3, 3, 3, 4, 5)$       | $\{\emptyset, 124689, 126789, 14569, 15679, 24578, 258, 47\}$     |
| 952:570b | $0, 0, 0, 0, e^{12}, -e^{13}, e^{14}, e^{15} + e^{23}, e^{36} + e^{47} + e^{25}$  | $25/81(1, 2, 2, 2, 3, 3, 3, 4, 5)$       | $\{\emptyset, 124689, 126789, 14569, 15679, 24578, 258, 47\}$     |
| 952:570c | $0, 0, 0, 0, -e^{12}, e^{13}, e^{14}, e^{23} + e^{15}, e^{25} + e^{47} + e^{36}$  | $25/81(1, 2, 2, 2, 3, 3, 3, 4, 5)$       | $\{\emptyset, 124689, 126789, 14569, 15679, 24578, 258, 47\}$     |
| 952:570d | $0, 0, 0, 0, -e^{12}, -e^{13}, e^{14}, e^{23} + e^{15}, e^{47} + e^{36} + e^{25}$ | $25/81(1, 2, 2, 2, 3, 3, 3, 4, 5)$       | $\{\emptyset, 124689, 126789, 14569, 15679, 24578, 258, 47\}$     |
| 952:579a | $0, 0, 0, 0, e^{12}, e^{13}, e^{34}, e^{15} + e^{23}, e^{47} + e^{36} + e^{25}$   | $5/33(2, 4, 4, 3, 6, 6, 7, 8, 10)$       | $\{123489, 123789, 13459, 13579\}$                                |
| 952:579b | $0, 0, 0, 0, -e^{12}, e^{13}, e^{34}, e^{15} + e^{23}, e^{36} + e^{47} + e^{25}$  | $5/33(2, 4, 4, 3, 6, 6, 7, 8, 10)$       | $\{123489, 123789, 13459, 13579\}$                                |
| 952:581a | $0, 0, 0, 0, e^{12}, e^{13}, e^{14}, e^{15} + e^{34}, e^{17} + e^{25} + e^{36}$   | $43/237(2, 3, 3, 4, 5, 5, 6, 7, 8)$      | $\{\emptyset, 124689, 13459, 23568\}$                             |
| 952:581b | $0, 0, 0, 0, -e^{12}, e^{13}, e^{14}, e^{34} + e^{15}, e^{36} + e^{17} + e^{25}$  | $43/237(2, 3, 3, 4, 5, 5, 6, 7, 8)$      | $\{\emptyset, 124689, 13459, 23568\}$                             |
| 952:584  | $0, 0, 0, 0, e^{12}, e^{13}, e^{24}, e^{34} + e^{25}, e^{27} + e^{36} + e^{15}$   | $35/317(5, 3, 4, 7, 8, 9, 10, 11, 13)$   | $\{\emptyset, 124689\}$                                           |
| 952:585  | $0, 0, 0, 0, e^{12}, e^{13}, e^{34}, e^{15} + e^{24}, e^{37} + e^{16} + e^{25}$   | $25/91(2, 1, 0, 4, 3, 2, 4, 5, 4)$       | $\{1234689, 134569\}$                                             |
| 952:586a | $0, 0, 0, 0, e^{12}, e^{13}, e^{14}, e^{15} + e^{34}, e^{36} + e^{47} + e^{25}$   | $25/81(1, 2, 2, 2, 3, 3, 3, 4, 5)$       | $\{\emptyset, 123789, 124689, 13459, 15679, 23568, 24578, 3467\}$ |
| 952:586b | $0, 0, 0, 0, e^{12}, -e^{13}, e^{14}, e^{15} + e^{34}, e^{25} + e^{47} + e^{36}$  | $25/81(1, 2, 2, 2, 3, 3, 3, 4, 5)$       | $\{\emptyset, 123789, 124689, 13459, 15679, 23568, 24578, 3467\}$ |
| 952:586c | $0, 0, 0, 0, -e^{12}, e^{13}, e^{14}, e^{15} + e^{34}, e^{47} + e^{36} + e^{25}$  | $25/81(1, 2, 2, 2, 3, 3, 3, 4, 5)$       | $\{\emptyset, 123789, 124689, 13459, 15679, 23568, 24578, 3467\}$ |
| 952:589a | $0, 0, 0, 0, e^{12}, e^{13}, e^{14}, e^{34} + e^{25}, e^{36} + e^{47} + e^{15}$   | $3/8(2, 0, 1, 1, 2, 3, 3, 2, 4)$         | $\{123579, 124569, 345678, 58\}$                                  |
| 952:589b | $0, 0, 0, 0, e^{12}, -e^{13}, e^{14}, e^{25} + e^{34}, e^{15} + e^{47} + e^{36}$  | $3/8(2, 0, 1, 1, 2, 3, 3, 2, 4)$         | $\{123579, 124569, 345678, 58\}$                                  |
| 952:595a | $0, 0, 0, 0, e^{12}, e^{13}, e^{34}, e^{15} + e^{24}, e^{47} + e^{16} + e^{25}$   | $1/19(0, 11, 22, 0, 11, 22, 22, 11, 22)$ | $\{1234689, 134569, 245678, 467\}$                                |
| 952:595b | $0, 0, 0, 0, e^{12}, -e^{13}, e^{34}, e^{24} + e^{15}, e^{16} + e^{47} + e^{25}$  | $1/19(0, 11, 22, 0, 11, 22, 22, 11, 22)$ | $\{1234689, 134569, 245678, 467\}$                                |
| 952:597  | $0, 0, 0, 0, e^{12}, e^{13}, e^{34}, e^{25} + e^{14}, e^{15} + e^{47} + e^{36}$   | $14/157(7, 3, 5, 6, 10, 12, 11, 13, 17)$ | $\{123489, 47\}$                                                  |
| 952:599a | $0, 0, 0, 0, e^{12}, e^{13}, e^{34}, e^{15} + e^{24}, e^{47} + e^{36} + e^{25}$   | $17/77(1, 3, 3, 2, 4, 4, 5, 5, 7)$       | $\{1234689, 134569, 245678, 467\}$                                |
| 952:599b | $0, 0, 0, 0, -e^{12}, e^{13}, e^{34}, e^{15} + e^{24}, e^{25} + e^{36} + e^{47}$  | $17/77(1, 3, 3, 2, 4, 4, 5, 5, 7)$       | $\{1234689, 134569, 245678, 467\}$                                |
| 952:601  | $0, 0, 0, 0, e^{12}, e^{13}, e^{14}, e^{16} + e^{25}, e^{15} + e^{23} + e^{47}$   | $14/153(4, 6, 8, 5, 10, 12, 9, 16, 14)$  | $\{134589, 135789\}$                                              |
| 952:603  | $0, 0, 0, 0, e^{12}, e^{13}, e^{24}, e^{16} + e^{25}, e^{27} + e^{34} + e^{15}$   | $1/2(0, 1, 2, -1, 1, 2, 0, 2, 1)$        | $\{1234589, 138\}$                                                |
| 952:605  | $0, 0, 0, 0, e^{12}, e^{13}, e^{14}, e^{36} + e^{15}, e^{17} + e^{25} + e^{34}$   | $6/29(1, 3, 2, 5, 4, 3, 6, 5, 7)$        | $\{123578, 345679\}$                                              |
| 952:606a | $0, 0, 0, 0, e^{12}, e^{13}, e^{14}, e^{25} + e^{36}, e^{23} + e^{15} + e^{47}$   | $8/51(2, 4, 4, 3, 6, 6, 5, 10, 8)$       | $\{123489, 123789, 3467, 36\}$                                    |
| 952:606b | $0, 0, 0, 0, -e^{12}, e^{13}, e^{14}, e^{36} + e^{25}, e^{15} + e^{23} + e^{47}$  | $8/51(2, 4, 4, 3, 6, 6, 5, 10, 8)$       | $\{123489, 123789, 3467, 36\}$                                    |
| 952:610a | $0, 0, 0, 0, e^{12}, e^{13}, e^{24}, e^{25} + e^{36}, e^{15} + e^{23} + e^{47}$   | $4/13(1, 2, 2, 1, 3, 3, 3, 5, 4)$        | $\{123489, 123789, 134578, 1358, 234569, 235679, 3467, 36\}$      |
| 952:610b | $0, 0, 0, 0, e^{12}, -e^{13}, e^{24}, e^{25} + e^{36}, e^{23} + e^{47} + e^{15}$  | $4/13(1, 2, 2, 1, 3, 3, 3, 5, 4)$        | $\{123489, 123789, 134578, 1358, 234569, 235679, 3467, 36\}$      |
| 952:610c | $0, 0, 0, 0, -e^{12}, e^{13}, e^{24}, e^{36} + e^{25}, e^{23} + e^{47} + e^{15}$  | $4/13(1, 2, 2, 1, 3, 3, 3, 5, 4)$        | $\{123489, 123789, 134578, 1358, 234569, 235679, 3467, 36\}$      |
| 952:610d | $0, 0, 0, 0, -e^{12}, -e^{13}, e^{24}, e^{36} + e^{25}, e^{47} + e^{15} + e^{23}$ | $4/13(1, 2, 2, 1, 3, 3, 3, 5, 4)$        | $\{123489, 123789, 134578, 1358, 234569, 235679, 3467, 36\}$      |
| 952:611a | $0, 0, 0, 0, e^{12}, e^{13}, e^{24}, e^{25} + e^{36}, e^{15} + e^{27} + e^{34}$   | $5/8(1, 0, 0, 2, 1, 1, 2, 1, 2)$         | $\{123578, 134789, 2367, 345679\}$                                |
| 952:611b | $0, 0, 0, 0, -e^{12}, e^{13}, e^{24}, e^{36} + e^{25}, e^{27} + e^{34} + e^{15}$  | $5/8(1, 0, 0, 2, 1, 1, 2, 1, 2)$         | $\{123578, 134789, 2367, 345679\}$                                |
| 952:616  | $0, 0, 0, 0, e^{12}, e^{13}, e^{34}, e^{25} + e^{16}, e^{15} + e^{47} + e^{23}$   | $14/157(4, 6, 8, 3, 10, 12, 11, 16, 14)$ | $\{123489, 123789\}$                                              |

Table A.2 – Continued to next page

Table A.2 – Continued from previous page

| Name     | $g$                                                                              | $N$                                                  | Signatures $S$                                                                                                        |
|----------|----------------------------------------------------------------------------------|------------------------------------------------------|-----------------------------------------------------------------------------------------------------------------------|
| 952:617  | $0, 0, 0, 0, e^{12}, e^{13}, e^{34}, e^{16} + e^{25}, e^{15} + e^{24} + e^{37}$  | $43/253(3, 2, 1, 6, 5, 4, 7, 7, 8)$                  | $\{1234689, 245679\}$                                                                                                 |
| 952:618  | $0, 0, 0, 0, e^{12}, e^{13}, e^{34}, e^{36} + e^{15}, e^{37} + e^{25} + e^{14}$  | $5/13(2, 0, 1, 0, 2, 3, 1, 4, 2)$                    | $\{123678, 128\}$                                                                                                     |
| 952:619a | $0, 0, 0, 0, e^{12}, e^{13}, e^{34}, e^{25} + e^{36}, e^{23} + e^{47} + e^{15}$  | $4/13(1, 2, 2, 1, 3, 3, 3, 5, 4)$                    | $\{123489, 123789, 234569, 235679\}$                                                                                  |
| 952:619b | $0, 0, 0, 0, -e^{12}, e^{13}, e^{34}, e^{36} + e^{25}, e^{23} + e^{47} + e^{15}$ | $4/13(1, 2, 2, 1, 3, 3, 3, 5, 4)$                    | $\{123489, 123789, 234569, 235679\}$                                                                                  |
| 952:620a | $0, 0, 0, 0, e^{12}, e^{13}, e^{34}, e^{36} + e^{25}, e^{24} + e^{37} + e^{15}$  | $5/8(1, 0, 0, 2, 1, 1, 2, 1, 2)$                     | $\{1234689, 124789, 23459, 245679\}$                                                                                  |
| 952:620b | $0, 0, 0, 0, -e^{12}, e^{13}, e^{34}, e^{36} + e^{25}, e^{37} + e^{15} + e^{24}$ | $5/8(1, 0, 0, 2, 1, 1, 2, 1, 2)$                     | $\{1234689, 124789, 23459, 245679\}$                                                                                  |
| 952:626  | $0, 0, 0, 0, e^{12}, e^{13}, e^{34}, e^{15} + e^{24} + e^{36}, e^{25} + e^{37}$  | $49/319(2, 4, 3, 4, 6, 5, 7, 8, 10)$                 | $\{1234689, 124789\}$                                                                                                 |
| 952:628a | $0, 0, 0, 0, e^{12}, e^{13}, e^{34}, e^{25} + e^{14} + e^{36}, e^{15} + e^{47}$  | $4/13(2, 1, 1, 2, 3, 3, 3, 4, 5)$                    | $\{123489, 145678, 234569, 47\}$                                                                                      |
| 952:628b | $0, 0, 0, 0, -e^{12}, e^{13}, e^{34}, e^{14} + e^{25} + e^{36}, e^{15} + e^{47}$ | $4/13(2, 1, 1, 2, 3, 3, 3, 4, 5)$                    | $\{123489, 145678, 234569, 47\}$                                                                                      |
| 952:630  | $0, 0, 0, 0, e^{12}, e^{13}, e^{34}, e^{24} + e^{36} + e^{15}, e^{47} + e^{25}$  | $40/431(3, 7, 5, 6, 10, 8, 11, 13, 17)$              | $\{134569, 245678\}$                                                                                                  |
| 952:637a | $0, 0, 0, 0, e^{12}, e^{13}, e^{14}, e^{16} + e^{25}, e^{15} + e^{47} + e^{36}$  | $8/17(1, 1, 1, 1, 2, 2, 2, 3, 3)$                    | $\{134589, 135789, 2457, 25\}$                                                                                        |
| 952:637b | $0, 0, 0, 0, e^{12}, -e^{13}, e^{14}, e^{16} + e^{25}, e^{36} + e^{47} + e^{15}$ | $8/17(1, 1, 1, 1, 2, 2, 2, 3, 3)$                    | $\{134589, 135789, 2457, 25\}$                                                                                        |
| 951:1    | $0, 0, 0, 0, e^{12}, e^{13}, e^{23}, e^{34}, e^{15}$                             | $1/41(16, 23, 24, 29, 39, 40, 47, 53, 55)$           | $\{123469, 123689, 124789, 1279, 134567, 135678, 1458, 15, 23459, 23589, 2456789, 25679, 347, 378, 468, 6\}$          |
| 951:3    | $0, 0, 0, 0, e^{12}, e^{13}, e^{14}, e^{34}, e^{25}$                             | $1/24(12, 10, 15, 15, 22, 27, 27, 30, 32)$           | $\{\emptyset, 12349, 123789, 124689, 12679, 13459, 135789, 145689, 15679, 234567, 23568, 24578, 25, 3467, 368, 478\}$ |
| 951:4    | $0, 0, 0, 0, e^{12}, e^{13}, e^{24}, e^{34}, e^{15}$                             | $1/19(7, 11, 13, 11, 18, 20, 22, 24, 25)$            | $\{\emptyset, 12349, 123789, 124689, 12679, 13457, 1358, 145678, 156, 234569, 2356789, 24589, 2579, 3467, 368, 478\}$ |
| 951:5    | $0, 0, 0, 0, e^{12}, e^{13}, e^{23}, e^{14}, e^{15}$                             | $1/23(8, 13, 16, 19, 21, 24, 29, 27, 29)$            | $\{\emptyset, 12349, 12389, 124679, 126789, 13457, 13578, 1456, 1568, 2345689, 23569, 245789, 2579, 34678, 367, 48\}$ |
| 951:6    | $0, 0, 0, 0, e^{12}, e^{13}, e^{23}, e^{14}, e^{25}$                             | $1/31(14, 13, 22, 24, 27, 36, 35, 38, 40)$           | $\{\emptyset, 12349, 12389, 124679, 126789, 134579, 135789, 14569, 15689, 234568, 2356, 24578, 257, 34678, 367, 48\}$ |
| 951:7    | $0, 0, 0, 0, e^{12}, e^{13}, e^{34}, e^{14} + e^{23}, e^{15}$                    | $1/40(16, 22, 23, 29, 38, 39, 52, 45, 54)$           | $\{123679, 124789, 134568, 15, 23459, 25689, 378, 467\}$                                                              |
| 951:8    | $0, 0, 0, 0, e^{12}, e^{13}, e^{34}, e^{14} + e^{23}, e^{25}$                    | $1/23(11, 10, 15, 14, 21, 26, 29, 25, 31)$           | $\{123789, 124679, 13459, 15689, 234568, 25, 367, 478\}$                                                              |
| 951:9    | $0, 0, 0, 0, e^{12}, e^{13}, e^{23}, e^{14}, e^{34} + e^{15}$                    | $1/38(15, 22, 24, 28, 37, 39, 46, 43, 52)$           | $\{\emptyset, 12389, 124679, 13457, 1568, 23569, 245789, 34678\}$                                                     |
| 951:10   | $0, 0, 0, 0, e^{12}, e^{13}, e^{23}, e^{14}, e^{34} + e^{25}$                    | $1/79(38, 35, 52, 56, 73, 90, 87, 94, 108)$          | $\{\emptyset, 12389, 124679, 135789, 14569, 234568, 257, 34678\}$                                                     |
| 951:11   | $0, 0, 0, 0, e^{12}, e^{13}, e^{23}, e^{34}, e^{14} + e^{25}$                    | $1/19(11, 7, 11, 14, 18, 22, 18, 25, 25)$            | $\{123479, 124689, 13459, 1456789, 234567, 2458, 346, 478\}$                                                          |
| 951:12   | $0, 0, 0, 0, e^{12}, e^{13}, e^{24}, e^{14} + e^{23}, e^{15}$                    | $1/63(26, 29, 45, 48, 55, 71, 77, 74, 81)$           | $\{\emptyset, 12349, 126789, 1358, 14567, 235679, 24589, 34678\}$                                                     |
| 951:14   | $0, 0, 0, 0, e^{12}, e^{13}, e^{24}, e^{34}, e^{15} + e^{23}$                    | $1/37(13, 22, 26, 21, 35, 39, 43, 47, 48)$           | $\{12349, 123789, 13457, 1358, 234569, 2356789, 3467, 368\}$                                                          |
| 951:15a  | $0, 0, 0, 0, e^{12}, e^{34}, e^{23} + e^{14}, e^{24} + e^{13}, e^{15}$           | $1/11(5, 5, 7, 7, 10, 14, 12, 12, 15)$               | $\{123689, 124679, 134578, 15, 23459, 25789, 367, 468\}$                                                              |
| 951:15b  | $0, 0, 0, 0, e^{12}, e^{34}, -e^{14} + e^{23}, e^{13} + e^{24}, e^{15}$          | $1/11(5, 5, 7, 7, 10, 14, 12, 12, 15)$               | $\{123689, 124679, 134578, 15, 23459, 25789, 367, 468\}$                                                              |
| 951:16   | $0, 0, 0, 0, e^{12}, e^{13}, e^{23}, e^{14}, e^{24} + e^{15}$                    | $1/13(5, 7, 9, 10, 12, 14, 16, 15, 17)$              | $\{\emptyset, 12389, 126789, 13578, 1568, 23569, 2579, 367\}$                                                         |
| 951:17   | $0, 0, 0, 0, e^{12}, e^{13}, e^{24}, e^{23} + e^{14}, e^{15} + e^{34}$           | $7/159(10, 11, 15, 16, 21, 25, 27, 26, 31)$          | $\{\emptyset, 235679, 24589, 34678\}$                                                                                 |
| 951:18   | $0, 0, 0, 0, e^{12}, e^{13}, e^{34}, e^{23} + e^{14}, e^{24} + e^{15}$           | $7/37(2, 3, 3, 4, 5, 5, 7, 6, 7)$                    | $\{124789, 134568, 23459, 467\}$                                                                                      |
| 951:19   | $0, 0, 0, 0, e^{12}, e^{13}, e^{14}, e^{24}, e^{25} + e^{16}$                    | $3/17(2, 3, 4, 4, 5, 6, 6, 7, 8)$                    | $\{\emptyset, 12349, 123789, 134589, 13579, 2457, 258, 478\}$                                                         |
| 951:20   | $0, 0, 0, 0, e^{12}, e^{13}, e^{14}, e^{24}, e^{15} + e^{36}$                    | $1/297(124, 176, 150, 197, 300, 274, 321, 373, 424)$ | $\{\emptyset, 12349, 123789, 12469, 126789, 34678, 36, 478\}$                                                         |
| 951:21a  | $0, 0, 0, 0, e^{12}, e^{13}, e^{14}, e^{24}, e^{36} + e^{25}$                    | $1/81(38, 40, 40, 55, 78, 78, 93, 95, 118)$          | $\{\emptyset, 12349, 123789, 12469, 126789, 134589, 13579, 145689, 15679, 234567, 23568, 2457, 258, 34678, 36, 478\}$ |
| 951:21b  | $0, 0, 0, 0, -e^{12}, e^{13}, e^{14}, e^{24}, e^{25} + e^{36}$                   | $1/81(38, 40, 40, 55, 78, 78, 93, 95, 118)$          | $\{\emptyset, 12349, 123789, 12469, 126789, 134589, 13579, 145689, 15679, 234567, 23568, 2457, 258, 34678, 36, 478\}$ |
| 951:23   | $0, 0, 0, 0, e^{12}, e^{13}, e^{24}, e^{34}, e^{25} + e^{16}$                    | $1/14(6, 7, 8, 9, 13, 14, 16, 17, 20)$               | $\{\emptyset, 12349, 123789, 134579, 13589, 2458, 257, 478\}$                                                         |
| 951:24a  | $0, 0, 0, 0, e^{12}, e^{13}, e^{24}, e^{34}, e^{36} + e^{25}$                    | $1/7(4, 3, 3, 5, 7, 7, 8, 8, 10)$                    | $\{\emptyset, 12349, 123789, 124689, 12679, 134579, 13589, 1456789, 1569, 23456, 235678, 2458, 257, 3467, 368, 478\}$ |
| 951:24b  | $0, 0, 0, 0, -e^{12}, e^{13}, e^{24}, e^{34}, e^{36} + e^{25}$                   | $1/7(4, 3, 3, 5, 7, 7, 8, 8, 10)$                    | $\{\emptyset, 12349, 123789, 124689, 12679, 134579, 13589, 1456789, 1569, 23456, 235678, 2458, 257, 3467, 368, 478\}$ |
| 951:26   | $0, 0, 0, 0, e^{12}, e^{13}, e^{23}, e^{14}, e^{16} + e^{25}$                    | $1/49(18, 25, 32, 40, 43, 50, 57, 58, 68)$           | $\{\emptyset, 12349, 12389, 134579, 135789, 24578, 257, 48\}$                                                         |
| 951:27   | $0, 0, 0, 0, e^{12}, e^{13}, e^{23}, e^{24}, e^{25} + e^{16}$                    | $1/227(91, 114, 137, 170, 205, 228, 251, 284, 319)$  | $\{\emptyset, 12349, 12389, 1345789, 13579, 2457, 2578, 48\}$                                                         |

Table A.2 – Continued to next page

Table A.2 – Continued from previous page

| Name    | $g$                                                                             | $N$                                                  | Signatures $S$                                                                                                        |
|---------|---------------------------------------------------------------------------------|------------------------------------------------------|-----------------------------------------------------------------------------------------------------------------------|
| 951:28a | $0, 0, 0, 0, e^{12}, e^{13}, e^{23}, e^{14}, e^{36} + e^{25}$                   | $1/19(8, 10, 10, 15, 18, 18, 20, 23, 28)$            | $\{\emptyset, 12349, 12389, 124679, 126789, 134579, 135789, 14569, 15689, 234568, 2356, 24578, 257, 34678, 367, 48\}$ |
| 951:28b | $0, 0, 0, 0, -e^{12}, e^{13}, e^{23}, e^{14}, e^{36} + e^{25}$                  | $1/19(8, 10, 10, 15, 18, 18, 20, 23, 28)$            | $\{\emptyset, 12349, 12389, 124679, 126789, 134579, 135789, 14569, 15689, 234568, 2356, 24578, 257, 34678, 367, 48\}$ |
| 951:30  | $0, 0, 0, 0, e^{12}, e^{13}, e^{23}, e^{24}, e^{15} + e^{36}$                   | $1/257(116, 138, 127, 188, 254, 243, 265, 326, 370)$ | $\{\emptyset, 12349, 12389, 124679, 126789, 34678, 367, 48\}$                                                         |
| 951:31a | $0, 0, 0, 0, e^{12}, e^{13}, e^{23}, e^{24}, e^{36} + e^{25}$                   | $1/17(9, 8, 8, 13, 17, 17, 16, 21, 25)$              | $\{123479, 123789, 12469, 12689, 134589, 1359, 1456789, 15679, 234567, 235678, 245, 258, 3468, 36, 478, 7\}$          |
| 951:31b | $0, 0, 0, 0, -e^{12}, e^{13}, e^{23}, e^{24}, e^{36} + e^{25}$                  | $1/17(9, 8, 8, 13, 17, 17, 16, 21, 25)$              | $\{123479, 123789, 12469, 12689, 134589, 1359, 1456789, 15679, 234567, 235678, 245, 258, 3468, 36, 478, 7\}$          |
| 951:33  | $0, 0, 0, 0, e^{12}, e^{13}, e^{24}, e^{23} + e^{14}, e^{16} + e^{25}$          | $3/184(24, 31, 38, 45, 55, 62, 76, 69, 86)$          | $\{\emptyset, 12349, 13589, 2458\}$                                                                                   |
| 951:34  | $0, 0, 0, 0, e^{12}, e^{13}, e^{24}, e^{23} + e^{14}, e^{36} + e^{15}$          | $1/497(209, 291, 250, 332, 500, 459, 623, 541, 709)$ | $\{\emptyset, 12349, 126789, 34678\}$                                                                                 |
| 951:35a | $0, 0, 0, 0, e^{12}, e^{13}, e^{24}, e^{14} + e^{23}, e^{25} + e^{36}$          | $1/149(63, 80, 80, 97, 143, 143, 177, 160, 223)$     | $\{123789, 12469, 134579, 15689, 234568, 257, 36, 478\}$                                                              |
| 951:35b | $0, 0, 0, 0, -e^{12}, e^{13}, e^{24}, e^{14} + e^{23}, e^{36} + e^{25}$         | $1/149(63, 80, 80, 97, 143, 143, 177, 160, 223)$     | $\{123789, 12469, 134579, 15689, 234568, 257, 36, 478\}$                                                              |
| 951:38a | $0, 0, 0, 0, e^{12}, e^{13}, e^{24}, e^{34}, e^{25} + e^{36} + e^{14}$          | $1/13(8, 5, 5, 10, 13, 13, 15, 15, 18)$              | $\{12349, 124689, 134579, 1456789, 23456, 2458, 3467, 478\}$                                                          |
| 951:38b | $0, 0, 0, 0, -e^{12}, e^{13}, e^{24}, e^{34}, e^{14} + e^{36} + e^{25}$         | $1/13(8, 5, 5, 10, 13, 13, 15, 15, 18)$              | $\{12349, 124689, 134579, 1456789, 23456, 2458, 3467, 478\}$                                                          |
| 951:40  | $0, 0, 0, 0, e^{12}, e^{13}, e^{23}, e^{14}, e^{24} + e^{36} + e^{15}$          | $1/41(16, 26, 21, 32, 42, 37, 47, 48, 58)$           | $\{\emptyset, 12389, 126789, 367\}$                                                                                   |
| 951:41a | $0, 0, 0, 0, e^{12}, e^{13}, e^{23}, e^{24}, e^{36} + e^{25} + e^{14}$          | $1/7(4, 3, 3, 6, 7, 7, 6, 9, 10)$                    | $\{123479, 12469, 134589, 1456789, 234567, 245, 3468, 478\}$                                                          |
| 951:41b | $0, 0, 0, 0, -e^{12}, e^{13}, e^{23}, e^{24}, e^{36} + e^{14} + e^{25}$         | $1/7(4, 3, 3, 6, 7, 7, 6, 9, 10)$                    | $\{123479, 12469, 134589, 1456789, 234567, 245, 3468, 478\}$                                                          |
| 951:44  | $0, 0, 0, 0, e^{12}, e^{13}, e^{24}, e^{14} + e^{23}, e^{16} + e^{34} + e^{25}$ | $21/167(3, 4, 5, 6, 7, 8, 10, 9, 11)$                | $\{12349, 2458\}$                                                                                                     |
| 951:45  | $0, 0, 0, 0, e^{12}, e^{13}, e^{23}, e^{14}, e^{37} + e^{16} + e^{25}$          | $1/49(24, 24, 24, 37, 48, 48, 48, 61, 72)$           | $\{\emptyset, 12349, 12389, 48\}$                                                                                     |
| 951:47  | $0, 0, 0, 0, e^{12}, e^{34}, e^{13}, e^{23}, e^{36} + e^{15}$                   | $1/43(20, 26, 19, 28, 46, 47, 39, 45, 66)$           | $\{123479, 124689, 135678, 15, 23459, 2456789, 368, 7\}$                                                              |
| 951:48  | $0, 0, 0, 0, e^{12}, e^{34}, e^{13}, e^{23}, e^{46} + e^{15}$                   | $1/107(49, 62, 60, 50, 111, 110, 109, 122, 160)$     | $\{\emptyset, 12349, 12369, 14567, 157, 234579, 235679, 46\}$                                                         |
| 951:49  | $0, 0, 0, 0, e^{12}, e^{34}, e^{13}, e^{24}, e^{36} + e^{15}$                   | $1/23(11, 13, 11, 13, 24, 24, 22, 26, 35)$           | $\{123479, 12469, 13567, 15, 23459, 245679, 36, 7\}$                                                                  |
| 951:50  | $0, 0, 0, 0, e^{12}, e^{34}, e^{13}, e^{24}, e^{25} + e^{36}$                   | $1/17(11, 7, 7, 11, 18, 18, 18, 18, 25)$             | $\{\emptyset, 12349, 124679, 134589, 1456789, 235678, 258, 367\}$                                                     |
| 951:51  | $0, 0, 0, 0, e^{12}, e^{34}, e^{13}, e^{23} + e^{14}, e^{36} + e^{15}$          | $3/53(8, 11, 8, 11, 19, 19, 16, 19, 27)$             | $\{123479, 135678, 2456789, 7\}$                                                                                      |
| 951:52  | $0, 0, 0, 0, e^{12}, e^{34}, e^{13}, e^{14} + e^{23}, e^{25} + e^{36}$          | $1/191(97, 100, 98, 101, 197, 199, 195, 198, 297)$   | $\{124679, 13459, 25, 367\}$                                                                                          |
| 951:53  | $0, 0, 0, 0, e^{12}, e^{34}, e^{13}, e^{14} + e^{23}, e^{46} + e^{25}$          | $1/65(37, 30, 37, 30, 67, 67, 74, 67, 97)$           | $\{\emptyset, 12349, 135689, 24568\}$                                                                                 |
| 951:57  | $0, 0, 0, 0, e^{12}, e^{34}, e^{13}, e^{23}, e^{36} + e^{25} + e^{14}$          | $1/31(22, 12, 11, 24, 34, 35, 33, 23, 46)$           | $\{123489, 124679, 13459, 1456789\}$                                                                                  |
| 951:58  | $0, 0, 0, 0, e^{12}, e^{34}, e^{13}, e^{24}, e^{46} + e^{23} + e^{15}$          | $11/31(1, 2, 2, 1, 3, 3, 3, 3, 4)$                   | $\{12349, 123689, 234579, 2356789\}$                                                                                  |
| 951:62  | $0, 0, 0, 0, e^{12}, e^{34}, e^{13}, e^{23} + e^{14}, e^{36} + e^{15} + e^{24}$ | $7/19(1, 2, 1, 2, 3, 3, 2, 3, 4)$                    | $\{123479, 2456789\}$                                                                                                 |
| 951:64a | $0, 0, 0, 0, e^{12}, e^{13}, e^{14}, e^{23}, e^{36} + e^{17} + e^{25}$          | $3/16(2, 3, 3, 4, 5, 5, 6, 6, 8)$                    | $\{\emptyset, 12349, 124689, 134589, 14569, 2356, 258, 368\}$                                                         |
| 951:64b | $0, 0, 0, 0, -e^{12}, e^{13}, e^{14}, e^{23}, e^{17} + e^{25} + e^{36}$         | $3/16(2, 3, 3, 4, 5, 5, 6, 6, 8)$                    | $\{\emptyset, 12349, 124689, 134589, 14569, 2356, 258, 368\}$                                                         |
| 951:66  | $0, 0, 0, 0, e^{12}, e^{13}, e^{24}, e^{23}, e^{15} + e^{27} + e^{36}$          | $3/211(39, 31, 35, 47, 70, 74, 78, 66, 109)$         | $\{123489, 12469, 36, 8\}$                                                                                            |
| 951:67a | $0, 0, 0, 0, e^{12}, e^{13}, e^{14}, e^{23}, e^{16} + e^{25} + e^{47}$          | $1/149(63, 80, 97, 80, 143, 160, 143, 177, 223)$     | $\{\emptyset, 12349, 12379, 134589, 135789, 24578, 258, 47\}$                                                         |
| 951:67b | $0, 0, 0, 0, -e^{12}, e^{13}, e^{14}, e^{23}, e^{16} + e^{25} + e^{47}$         | $1/149(63, 80, 97, 80, 143, 160, 143, 177, 223)$     | $\{\emptyset, 12349, 12379, 134589, 135789, 24578, 258, 47\}$                                                         |
| 951:69  | $0, 0, 0, 0, e^{12}, e^{13}, e^{24}, e^{23}, e^{47} + e^{25} + e^{16}$          | $1/557(256, 294, 332, 275, 550, 588, 569, 626, 844)$ | $\{\emptyset, 12349, 12379, 47\}$                                                                                     |
| 951:70a | $0, 0, 0, 0, e^{12}, e^{13}, e^{14}, e^{23}, e^{47} + e^{36} + e^{25}$          | $1/9(4, 5, 5, 5, 9, 9, 9, 10, 14)$                   | $\{\emptyset, 12349, 12379, 124689, 126789, 134589, 135789, 14569, 15679, 234567, 2356, 24578, 258, 34678, 368, 47\}$ |
| 951:70b | $0, 0, 0, 0, e^{12}, -e^{13}, e^{14}, e^{23}, e^{47} + e^{25} + e^{36}$         | $1/9(4, 5, 5, 5, 9, 9, 9, 10, 14)$                   | $\{\emptyset, 12349, 12379, 124689, 126789, 134589, 135789, 14569, 15679, 234567, 2356, 24578, 258, 34678, 368, 47\}$ |
| 951:70c | $0, 0, 0, 0, -e^{12}, -e^{13}, e^{14}, e^{23}, e^{36} + e^{47} + e^{25}$        | $1/9(4, 5, 5, 5, 9, 9, 9, 10, 14)$                   | $\{\emptyset, 12349, 12379, 124689, 126789, 134589, 135789, 14569, 15679, 234567, 2356, 24578, 258, 34678, 368, 47\}$ |
| 951:73a | $0, 0, 0, 0, e^{12}, e^{13}, e^{24}, e^{23}, e^{15} + e^{47} + e^{36}$          | $1/79(40, 42, 41, 40, 82, 81, 82, 83, 122)$          | $\{\emptyset, 12349, 12379, 124689, 126789, 34678, 368, 47\}$                                                         |
| 951:73b | $0, 0, 0, 0, -e^{12}, e^{13}, e^{24}, e^{23}, e^{15} + e^{36} + e^{47}$         | $1/79(40, 42, 41, 40, 82, 81, 82, 83, 122)$          | $\{\emptyset, 12349, 12379, 124689, 126789, 34678, 368, 47\}$                                                         |
| 951:75a | $0, 0, 0, 0, e^{12}, e^{13}, e^{24}, e^{23}, e^{25} + e^{36} + e^{47}$          | $5/161(18, 16, 16, 17, 34, 34, 33, 32, 50)$          | $\{123489, 123789, 12469, 12679, 3467, 36, 478, 8\}$                                                                  |
| 951:75b | $0, 0, 0, 0, -e^{12}, e^{13}, e^{24}, e^{23}, e^{25} + e^{47} + e^{36}$         | $5/161(18, 16, 16, 17, 34, 34, 33, 32, 50)$          | $\{123489, 123789, 12469, 12679, 3467, 36, 478, 8\}$                                                                  |
| 951:77  | $0, 0, 0, 0, e^{12}, e^{13}, e^{24}, e^{34}, e^{36} + e^{15} + e^{27}$          | $1/43(23, 19, 21, 27, 42, 44, 46, 48, 65)$           | $\{\emptyset, 12349, 124689, 368\}$                                                                                   |

Table A.2 – Continued to next page

Table A.2 – Continued from previous page

| Name     | $g$                                                                                 | $N$                                                 | Signatures $S$                                                                                                        |
|----------|-------------------------------------------------------------------------------------|-----------------------------------------------------|-----------------------------------------------------------------------------------------------------------------------|
| 951:78a  | $0, 0, 0, 0, e^{12}, e^{13}, e^{24}, e^{34}, e^{36} + e^{15} + e^{47}$              | $1/55(27, 31, 29, 27, 58, 56, 58, 56, 85)$          | $\{\emptyset, 12349, 123789, 124689, 12679, 3467, 368, 478\}$                                                         |
| 951:78b  | $0, 0, 0, 0, -e^{12}, e^{13}, e^{24}, e^{34}, e^{47} + e^{36} + e^{15}$             | $1/55(27, 31, 29, 27, 58, 56, 58, 56, 85)$          | $\{\emptyset, 12349, 123789, 124689, 12679, 3467, 368, 478\}$                                                         |
| 951:80   | $0, 0, 0, 0, e^{12}, e^{13}, e^{24}, e^{14} + e^{23}, e^{36} + e^{15} + e^{27}$     | $15/29(1, 1, 1, 1, 2, 2, 2, 2, 3)$                  | $\{134579, 257\}$                                                                                                     |
| 951:81a  | $0, 0, 0, 0, e^{12}, e^{13}, e^{24}, e^{14} + e^{23}, e^{15} + e^{47} + e^{36}$     | $15/29(1, 1, 1, 1, 2, 2, 2, 2, 3)$                  | $\{12379, 124689, 368, 47\}$                                                                                          |
| 951:81b  | $0, 0, 0, 0, -e^{12}, e^{13}, e^{24}, e^{14} + e^{23}, e^{15} + e^{36} + e^{47}$    | $15/29(1, 1, 1, 1, 2, 2, 2, 2, 3)$                  | $\{12379, 124689, 368, 47\}$                                                                                          |
| 951:94a  | $0, 0, 0, 0, e^{12}, e^{13}, e^{23}, e^{14}, e^{16} + e^{25} + e^{48} + e^{37}$     | $15/29(1, 1, 1, 1, 2, 2, 2, 2, 3)$                  | $\{\emptyset, 12349, 12389, 48\}$                                                                                     |
| 951:94b  | $0, 0, 0, 0, -e^{12}, e^{13}, e^{23}, e^{14}, e^{48} + e^{25} + e^{37} + e^{16}$    | $15/29(1, 1, 1, 1, 2, 2, 2, 2, 3)$                  | $\{\emptyset, 12349, 12389, 48\}$                                                                                     |
| 951:97   | $0, 0, 0, 0, e^{12}, e^{13}, e^{24}, e^{34}, e^{36} + e^{48} + e^{15} + e^{27}$     | $15/29(1, 1, 1, 1, 2, 2, 2, 2, 3)$                  | $\{\emptyset, 12349\}$                                                                                                |
| 94321:4  | $0, 0, 0, 0, 0, e^{12}, e^{16}, e^{17}, e^{18} + e^{45} + e^{23}$                   | $1/317(65, 204, 260, 232, 232, 269, 334, 399, 464)$ | $\{\emptyset, 12479, 12579, 14568, 168, 246789, 256789, 45\}$                                                         |
| 9431:5   | $0, 0, 0, 0, 0, e^{12}, e^{16}, e^{26} + e^{34}, e^{35} + e^{17}$                   | $1/29(8, 16, 17, 23, 23, 24, 32, 40, 40)$           | $\{\emptyset, 123578, 12478, 13689, 145689, 234679, 25679, 345\}$                                                     |
| 9431:6   | $0, 0, 0, 0, 0, e^{12}, e^{16}, e^{26} + e^{45} + e^{13}, e^{17}$                   | $1/25(6, 14, 28, 17, 17, 20, 26, 34, 32)$           | $\{123478, 123578, 134689, 135689, 2345679, 23679, 3, 345\}$                                                          |
| 9431:10  | $0, 0, 0, 0, 0, e^{12}, e^{16}, e^{26} + e^{13}, e^{17} + e^{45}$                   | $1/83(26, 40, 80, 59, 59, 66, 92, 106, 118)$        | $\{\emptyset, 124578, 1278, 14689, 15689, 24679, 25679, 45\}$                                                         |
| 9431:11  | $0, 0, 0, 0, 0, e^{12}, e^{16}, e^{26} + e^{34}, e^{17} + e^{25}$                   | $4/29(2, 4, 5, 5, 6, 6, 8, 10, 10)$                 | $\{\emptyset, 123578, 124578, 135689, 145689, 234679, 2679, 34\}$                                                     |
| 9431:12  | $0, 0, 0, 0, 0, e^{12}, e^{16}, e^{45} + e^{13} + e^{26}, e^{34} + e^{17}$          | $1/49(16, 23, 46, 25, 37, 39, 55, 62, 71)$          | $\{123478, 135689, 23679, 345\}$                                                                                      |
| 9431:15  | $0, 0, 0, 0, 0, e^{12}, e^{16}, e^{26}, e^{23} + e^{45} + e^{17}$                   | $7/107(5, 7, 15, 11, 11, 12, 17, 19, 22)$           | $\{\emptyset, 1234578, 12378, 134689, 135689, 24679, 25679, 45\}$                                                     |
| 9431:16  | $0, 0, 0, 0, 0, e^{12}, e^{16}, e^{26} + e^{34}, e^{45} + e^{23} + e^{17}$          | $7/701(27, 56, 81, 58, 79, 83, 110, 139, 137)$      | $\{124578, 14689, 234679, 345\}$                                                                                      |
| 9431:17  | $0, 0, 0, 0, 0, e^{12}, e^{16}, e^{26} + e^{13} + e^{45}, e^{23} + e^{17}$          | $4/25(2, 3, 6, 4, 4, 5, 7, 8, 9)$                   | $\{123478, 123578, 134689, 135689\}$                                                                                  |
| 9431:18  | $0, 0, 0, 0, 0, e^{12}, e^{16}, e^{35} + e^{14} + e^{26}, e^{23} + e^{17}$          | $1/224(52, 127, 156, 254, 150, 179, 231, 306, 283)$ | $\{124578, 145689, 2345679, 345\}$                                                                                    |
| 9431:19  | $0, 0, 0, 0, 0, e^{12}, e^{16}, e^{13} + e^{26}, e^{45} + e^{17} + e^{23}$          | $49/617(4, 6, 12, 9, 9, 10, 14, 16, 18)$            | $\{\emptyset, 24679, 25679, 45\}$                                                                                     |
| 9431:20  | $0, 0, 0, 0, 0, e^{12}, e^{16}, e^{26} + e^{13}, e^{17} + e^{35} + e^{24}$          | $7/139(7, 8, 16, 21, 13, 15, 22, 23, 29)$           | $\{123578, 13689, 234679, 345\}$                                                                                      |
| 9431:21  | $0, 0, 0, 0, 0, e^{12}, e^{16}, e^{14} + e^{26} + e^{35}, e^{45} + e^{17} + e^{23}$ | $7/71(3, 5, 9, 10, 4, 8, 11, 13, 14)$               | $\{124578, 345\}$                                                                                                     |
| 9421:4   | $0, 0, 0, 0, 0, e^{12}, e^{34}, e^{16}, e^{18} + e^{35}$                            | $1/33(7, 24, 18, 24, 27, 31, 42, 38, 45)$           | $\{\emptyset, 123458, 123578, 12478, 128, 13469, 13679, 145679, 1569, 234689, 236789, 2456789, 25689, 345, 357, 47\}$ |
| 9421:5   | $0, 0, 0, 0, 0, e^{12}, e^{13} + e^{45}, e^{16}, e^{18}$                            | $1/11(2, 8, 12, 7, 7, 10, 14, 12, 14)$              | $\{123478, 123578, 12458, 128, 134679, 135679, 14569, 169, 2345689, 23689, 246789, 256789, 3, 345, 47, 57\}$          |
| 9421:6   | $0, 0, 0, 0, 0, e^{12}, e^{13} + e^{45}, e^{26}, e^{28}$                            | $1/33(21, 7, 27, 24, 24, 28, 48, 35, 42)$           | $\{\emptyset, 123458, 1238, 12478, 12578, 1345689, 13689, 146789, 156789, 234679, 235679, 24569, 269, 347, 357, 45\}$ |
| 9421:11  | $0, 0, 0, 0, 0, e^{12}, e^{13}, e^{16}, e^{18} + e^{45}$                            | $1/27(6, 20, 24, 19, 19, 26, 30, 32, 38)$           | $\{\emptyset, 123458, 1238, 124578, 1278, 13469, 13569, 14679, 15679, 2346789, 2356789, 24689, 25689, 3457, 37, 45\}$ |
| 9421:12  | $0, 0, 0, 0, 0, e^{12}, e^{13}, e^{26}, e^{28} + e^{45}$                            | $2/33(9, 5, 12, 12, 12, 14, 21, 19, 24)$            | $\{\emptyset, 123458, 1238, 124578, 1278, 134689, 135689, 146789, 156789, 234679, 235679, 2469, 2569, 3457, 37, 45\}$ |
| 9421:14  | $0, 0, 0, 0, 0, e^{12}, e^{45} + e^{13}, e^{16}, e^{18} + e^{34}$                   | $1/29(7, 20, 27, 14, 20, 27, 34, 34, 41)$           | $\{123478, 128, 135679, 14569, 23689, 246789, 345, 57\}$                                                              |
| 9421:15  | $0, 0, 0, 0, 0, e^{12}, e^{45} + e^{13}, e^{26}, e^{28} + e^{34}$                   | $1/111(72, 26, 81, 69, 84, 98, 153, 124, 150)$      | $\{\emptyset, 123458, 12578, 13689, 146789, 235679, 24569, 347\}$                                                     |
| 9421:20  | $0, 0, 0, 0, 0, e^{12}, e^{24} + e^{13}, e^{16}, e^{18} + e^{35}$                   | $2/29(5, 7, 12, 10, 10, 12, 17, 17, 22)$            | $\{123578, 1248, 134679, 1569, 234689, 256789, 35, 47\}$                                                              |
| 9421:21  | $0, 0, 0, 0, 0, e^{12}, e^{23} + e^{14}, e^{16}, e^{18} + e^{35}$                   | $1/81(21, 50, 49, 78, 64, 71, 99, 92, 113)$         | $\{\emptyset, 123458, 1278, 13679, 14569, 23689, 2456789, 3457\}$                                                     |
| 9421:22  | $0, 0, 0, 0, 0, e^{12}, e^{34}, e^{16}, e^{23} + e^{45} + e^{18}$                   | $1/69(16, 48, 48, 39, 57, 64, 87, 80, 96)$          | $\{\emptyset, 123458, 12378, 13469, 135679, 246789, 25689, 457\}$                                                     |
| 9421:23  | $0, 0, 0, 0, 0, e^{12}, e^{13} + e^{45}, e^{16}, e^{23} + e^{18}$                   | $1/13(4, 7, 12, 8, 8, 11, 16, 15, 19)$              | $\{123478, 123578, 134679, 135679, 246789, 256789, 47, 57\}$                                                          |
| 9421:24  | $0, 0, 0, 0, 0, e^{12}, e^{35} + e^{14}, e^{16}, e^{23} + e^{18}$                   | $1/59(12, 41, 36, 63, 39, 53, 75, 65, 77)$          | $\{123478, 12358, 134679, 13569, 24689, 256789, 4, 57\}$                                                              |
| 9421:25  | $0, 0, 0, 0, 0, e^{12}, e^{35} + e^{14}, e^{26}, e^{28} + e^{13}$                   | $1/69(42, 16, 48, 57, 51, 58, 99, 74, 90)$          | $\{\emptyset, 123458, 12378, 14689, 156789, 234679, 23569, 457\}$                                                     |
| 9421:28  | $0, 0, 0, 0, 0, e^{12}, e^{13}, e^{16}, e^{45} + e^{18} + e^{23}$                   | $1/144(39, 95, 117, 106, 106, 134, 156, 173, 212)$  | $\{\emptyset, 123458, 1238, 13469, 13569, 24689, 25689, 45\}$                                                         |
| 9421:29  | $0, 0, 0, 0, 0, e^{12}, e^{13}, e^{16}, e^{18} + e^{35} + e^{24}$                   | $1/83(24, 52, 61, 72, 63, 76, 85, 100, 124)$        | $\{\emptyset, 123458, 12478, 13469, 145679, 236789, 25689, 357\}$                                                     |
| 9421:30  | $0, 0, 0, 0, 0, e^{12}, e^{13}, e^{26}, e^{14} + e^{28} + e^{35}$                   | $1/33(18, 10, 21, 30, 27, 28, 39, 38, 48)$          | $\{\emptyset, 123458, 12478, 13689, 156789, 234679, 24569, 357\}$                                                     |
| 9421:31  | $0, 0, 0, 0, 0, e^{12}, e^{24} + e^{13}, e^{16}, e^{18} + e^{25}$                   | $3/83(8, 14, 27, 21, 24, 22, 35, 30, 38)$           | $\{\emptyset, 123458, 12578, 13569, 145679, 236789, 24689, 347\}$                                                     |
| 9421:32  | $0, 0, 0, 0, 0, e^{12}, e^{45} + e^{13}, e^{16}, e^{24} + e^{35} + e^{18}$          | $11/47(1, 3, 4, 3, 2, 4, 5, 5, 6)$                  | $\{123578, 128, 345, 47\}$                                                                                            |
| 9421:33a | $0, 0, 0, 0, 0, e^{12}, e^{13} + e^{45}, e^{26}, e^{14} + e^{35} + e^{28}$          | $2/57(18, 7, 21, 21, 18, 25, 39, 32, 39)$           | $\{\emptyset, 123458, 12478, 13689, 156789, 234679, 24569, 357\}$                                                     |
| 9421:33b | $0, 0, 0, 0, 0, e^{12}, e^{45} - e^{13}, e^{26}, e^{28} + e^{35} + e^{14}$          | $2/57(18, 7, 21, 21, 18, 25, 39, 32, 39)$           | $\{\emptyset, 123458, 12478, 13689, 156789, 234679, 24569, 357\}$                                                     |
| 9421:36  | $0, 0, 0, 0, 0, e^{12}, e^{34}, e^{16}, e^{26} + e^{35} + e^{18}$                   | $1/7(2, 4, 4, 5, 6, 6, 9, 8, 10)$                   | $\{\emptyset, 13469, 13679, 145679, 1569, 345, 357, 47\}$                                                             |

Table A.2 – Continued to next page

Table A.2 – Continued from previous page

| Name      | $g$                                                                         | $N$                                                  | Signatures $S$                                                                                                        |
|-----------|-----------------------------------------------------------------------------|------------------------------------------------------|-----------------------------------------------------------------------------------------------------------------------|
| 9421:37   | $0, 0, 0, 0, 0, e^{12}, e^{45} + e^{13}, e^{16}, e^{18} + e^{26}$           | $1/139(38, 76, 144, 91, 91, 114, 182, 152, 190)$     | $\{134679, 135679, 14569, 169, 3, 345, 47, 57\}$                                                                      |
| 9421:38   | $0, 0, 0, 0, 0, e^{12}, e^{45} + e^{13}, e^{26}, e^{16} + e^{28}$           | $1/41(22, 11, 36, 29, 29, 33, 58, 44, 55)$           | $\{\emptyset, 234679, 235679, 24569, 269, 347, 357, 45\}$                                                             |
| 9421:39   | $0, 0, 0, 0, 0, e^{12}, e^{24} + e^{13}, e^{16}, e^{45} + e^{18} + e^{23}$  | $1/171(51, 95, 153, 109, 139, 146, 204, 197, 248)$   | $\{\emptyset, 123458, 13569, 24689\}$                                                                                 |
| 9421:46   | $0, 0, 0, 0, 0, e^{12}, e^{13}, e^{16}, e^{45} + e^{18} + e^{26}$           | $1/34(10, 20, 29, 25, 25, 30, 39, 40, 50)$           | $\{\emptyset, 13469, 13569, 14679, 15679, 3457, 37, 45\}$                                                             |
| 9421:47   | $0, 0, 0, 0, 0, e^{12}, e^{13}, e^{26}, e^{16} + e^{28} + e^{45}$           | $1/139(80, 40, 99, 100, 100, 120, 179, 160, 200)$    | $\{123458, 1238, 124578, 1278, 134689, 135689, 146789, 156789\}$                                                      |
| 9421:48   | $0, 0, 0, 0, 0, e^{12}, e^{45} + e^{13}, e^{16}, e^{18} + e^{34} + e^{26}$  | $1/107(31, 62, 99, 56, 74, 93, 130, 124, 155)$       | $\{135679, 14569, 345, 57\}$                                                                                          |
| 9421:49   | $0, 0, 0, 0, 0, e^{12}, e^{13} + e^{45}, e^{26}, e^{28} + e^{16} + e^{34}$  | $1/57(32, 16, 45, 35, 42, 48, 77, 64, 80)$           | $\{\emptyset, 235679, 24569, 347\}$                                                                                   |
| 9421:55   | $0, 0, 0, 0, 0, e^{12}, e^{13} + e^{24}, e^{16}, e^{18} + e^{26} + e^{35}$  | $2/101(15, 30, 44, 29, 31, 45, 59, 60, 75)$          | $\{123578, 1248, 234689, 256789\}$                                                                                    |
| 9421:56   | $0, 0, 0, 0, 0, e^{12}, e^{14} + e^{23}, e^{16}, e^{18} + e^{26} + e^{35}$  | $1/14(4, 8, 9, 13, 11, 12, 17, 16, 20)$              | $\{\emptyset, 13679, 14569, 3457\}$                                                                                   |
| 9421:57   | $0, 0, 0, 0, 0, e^{12}, e^{13}, e^{16}, e^{18} + e^{45} + e^{37}$           | $1/83(22, 60, 52, 63, 63, 82, 74, 104, 126)$         | $\{\emptyset, 13469, 13569, 14679, 15679, 3457, 37, 45\}$                                                             |
| 9421:58   | $0, 0, 0, 0, 0, e^{12}, e^{13}, e^{26}, e^{28} + e^{37} + e^{45}$           | $1/204(108, 70, 105, 159, 159, 178, 213, 248, 318)$  | $\{\emptyset, 134689, 135689, 146789, 156789, 3457, 37, 45\}$                                                         |
| 9421:69   | $0, 0, 0, 0, 0, e^{12}, e^{13}, e^{26}, e^{45} + e^{17} + e^{28}$           | $1/93(39, 35, 66, 72, 72, 74, 105, 109, 144)$        | $\{\emptyset, 124578, 1278, 134689, 135689, 234679, 235679, 45\}$                                                     |
| 9421:70   | $0, 0, 0, 0, 0, e^{12}, e^{34}, e^{16}, e^{18} + e^{47} + e^{35}$           | $1/27(7, 19, 16, 12, 24, 26, 28, 33, 40)$            | $\{\emptyset, 12478, 128, 13469, 13679, 234689, 236789, 47\}$                                                         |
| 9421:84   | $0, 0, 0, 0, 0, e^{12}, e^{34}, e^{16}, e^{25} + e^{37} + e^{18}$           | $1/24(7, 15, 10, 16, 21, 22, 26, 29, 36)$            | $\{\emptyset, 123578, 1258, 134569, 145679, 234689, 246789, 37\}$                                                     |
| 9421:104a | $0, 0, 0, 0, 0, e^{12}, e^{13}, e^{16}, e^{18} + e^{37} + e^{26} + e^{45}$  | $25/161(2, 4, 4, 5, 5, 6, 6, 8, 10)$                 | $\{\emptyset, 13469, 13569, 14679, 15679, 3457, 37, 45\}$                                                             |
| 9421:104b | $0, 0, 0, 0, 0, -e^{12}, e^{13}, e^{16}, e^{18} + e^{26} + e^{37} + e^{45}$ | $25/161(2, 4, 4, 5, 5, 6, 6, 8, 10)$                 | $\{\emptyset, 13469, 13569, 14679, 15679, 3457, 37, 45\}$                                                             |
| 9421:106  | $0, 0, 0, 0, 0, e^{12}, e^{13}, e^{26}, e^{16} + e^{28} + e^{37} + e^{45}$  | $25/164(4, 2, 3, 5, 5, 6, 7, 8, 10)$                 | $\{134689, 135689, 146789, 156789\}$                                                                                  |
| 9421:114  | $0, 0, 0, 0, 0, e^{12}, e^{34}, e^{16}, e^{18} + e^{26} + e^{35} + e^{47}$  | $5/33(2, 4, 4, 3, 6, 6, 7, 8, 10)$                   | $\{\emptyset, 13469, 13679, 47\}$                                                                                     |
| 942:8     | $0, 0, 0, 0, 0, e^{12}, e^{34}, e^{16}, e^{35} + e^{26}$                    | $1/33(13, 16, 18, 24, 27, 29, 42, 42, 45)$           | $\{\emptyset, 123489, 123789, 1245789, 12589, 13469, 13679, 145679, 1569, 234568, 235678, 24678, 268, 345, 357, 47\}$ |
| 942:9     | $0, 0, 0, 0, 0, e^{12}, e^{13} + e^{45}, e^{16}, e^{26}$                    | $1/47(19, 20, 45, 32, 32, 39, 64, 58, 59)$           | $\{\emptyset, 1234589, 12389, 124789, 125789, 134569, 1369, 14679, 15679, 234678, 235678, 24568, 268, 347, 357, 45\}$ |
| 942:12    | $0, 0, 0, 0, 0, e^{12}, e^{13}, e^{16}, e^{26} + e^{45}$                    | $1/18(6, 10, 15, 13, 13, 16, 21, 22, 26)$            | $\{\emptyset, 123489, 123589, 124789, 125789, 13469, 13569, 14679, 15679, 2345678, 23678, 24568, 268, 3457, 37, 45\}$ |
| 942:13    | $0, 0, 0, 0, 0, e^{12}, e^{13}, e^{26}, e^{45} + e^{16}$                    | $2/47(11, 10, 18, 16, 16, 21, 29, 31, 32)$           | $\{\emptyset, 123489, 123589, 124789, 125789, 134568, 1368, 145678, 1678, 234679, 235679, 2469, 2569, 3457, 37, 45\}$ |
| 942:16    | $0, 0, 0, 0, 0, e^{12}, e^{34}, e^{16} + e^{35}, e^{26} + e^{45}$           | $1/111(50, 50, 69, 69, 81, 100, 138, 150, 150)$      | $\{\emptyset, 123489, 12589, 135679, 14679, 23678, 245678, 345\}$                                                     |
| 942:17    | $0, 0, 0, 0, 0, e^{12}, e^{45} + e^{13}, e^{16}, e^{26} + e^{34}$           | $1/139(56, 67, 117, 73, 100, 123, 173, 179, 190)$    | $\{1235789, 124589, 135679, 14569, 234568, 25678, 345, 57\}$                                                          |
| 942:18    | $0, 0, 0, 0, 0, e^{12}, e^{13} + e^{45}, e^{26}, e^{16} + e^{34}$           | $1/317(152, 126, 255, 175, 232, 278, 407, 404, 430)$ | $\{\emptyset, 12389, 124789, 134568, 15678, 235679, 24569, 347\}$                                                     |
| 942:25    | $0, 0, 0, 0, 0, e^{12}, e^{13}, e^{16} + e^{34}, e^{26} + e^{35}$           | $1/81(37, 38, 47, 65, 66, 75, 84, 112, 113)$         | $\{\emptyset, 12389, 1245789, 13469, 15679, 235678, 2468, 3457\}$                                                     |
| 942:26    | $0, 0, 0, 0, 0, e^{12}, e^{13}, e^{34} + e^{16}, e^{45} + e^{26}$           | $1/24(10, 12, 17, 15, 19, 22, 27, 32, 34)$           | $\{\emptyset, 123589, 124789, 13469, 15679, 23678, 24568, 3457\}$                                                     |
| 942:27    | $0, 0, 0, 0, 0, e^{12}, e^{13}, e^{26} + e^{34}, e^{45} + e^{16}$           | $1/11(5, 5, 8, 7, 8, 10, 13, 15, 15)$                | $\{\emptyset, 123589, 124789, 1368, 145678, 234679, 2569, 3457\}$                                                     |
| 942:29    | $0, 0, 0, 0, 0, e^{12}, e^{23} + e^{14}, e^{16}, e^{26} + e^{35}$           | $1/34(12, 18, 23, 29, 25, 30, 41, 42, 48)$           | $\{\emptyset, 123489, 125789, 13679, 14569, 23568, 24678, 3457\}$                                                     |
| 942:30    | $0, 0, 0, 0, 0, e^{12}, e^{34}, e^{13} + e^{26}, e^{35} + e^{16}$           | $1/29(16, 9, 18, 20, 23, 25, 38, 34, 41)$            | $\{123489, 123789, 134568, 135678, 23469, 23679, 345, 357\}$                                                          |
| 942:31    | $0, 0, 0, 0, 0, e^{12}, e^{34}, e^{16}, e^{26} + e^{45} + e^{13}$           | $1/29(13, 12, 24, 14, 23, 25, 38, 38, 37)$           | $\{123489, 1235789, 13469, 135679, 234568, 23678, 345, 37\}$                                                          |
| 942:32    | $0, 0, 0, 0, 0, e^{12}, e^{34}, e^{26} + e^{13}, e^{16} + e^{45}$           | $1/139(69, 52, 104, 75, 115, 121, 179, 173, 190)$    | $\{123489, 1235789, 134568, 13678, 23469, 235679, 345, 37\}$                                                          |
| 942:33    | $0, 0, 0, 0, 0, e^{12}, e^{34}, e^{15} + e^{26}, e^{35} + e^{16}$           | $1/317(151, 128, 174, 230, 256, 279, 404, 407, 430)$ | $\{\emptyset, 123489, 123789, 14678, 168, 23469, 23679, 47\}$                                                         |
| 942:34    | $0, 0, 0, 0, 0, e^{12}, e^{14} + e^{35}, e^{16}, e^{13} + e^{26}$           | $1/43(19, 16, 32, 41, 28, 35, 60, 54, 51)$           | $\{1234589, 123789, 134569, 13679, 234678, 23568, 347, 35\}$                                                          |
| 942:35    | $0, 0, 0, 0, 0, e^{12}, e^{13} + e^{45}, e^{26}, e^{23} + e^{16}$           | $1/293(132, 115, 264, 198, 198, 247, 396, 362, 379)$ | $\{\emptyset, 124789, 125789, 14678, 15678, 24569, 269, 45\}$                                                         |
| 942:37    | $0, 0, 0, 0, 0, e^{12}, e^{45} + e^{13}, e^{34} + e^{16}, e^{35} + e^{26}$  | $1/561(258, 251, 423, 344, 337, 509, 681, 767, 760)$ | $\{124589, 134679, 24678, 345\}$                                                                                      |
| 942:40    | $0, 0, 0, 0, 0, e^{12}, e^{13}, e^{16}, e^{14} + e^{26} + e^{35}$           | $1/37(14, 19, 25, 38, 27, 33, 39, 47, 52)$           | $\{123489, 1245789, 13469, 145679, 2345678, 2468, 3457, 4\}$                                                          |
| 942:41    | $0, 0, 0, 0, 0, e^{12}, e^{13}, e^{26}, e^{16} + e^{45} + e^{23}$           | $2/43(9, 10, 18, 14, 14, 19, 27, 29, 28)$            | $\{123489, 123589, 134568, 1368, 234679, 235679, 3457, 37\}$                                                          |
| 942:42    | $0, 0, 0, 0, 0, e^{12}, e^{13}, e^{26}, e^{16} + e^{35} + e^{24}$           | $1/227(111, 91, 143, 222, 170, 202, 254, 293, 313)$  | $\{\emptyset, 12389, 125789, 13568, 1678, 23679, 2569, 357\}$                                                         |
| 942:43    | $0, 0, 0, 0, 0, e^{12}, e^{13}, e^{23} + e^{16}, e^{45} + e^{26}$           | $1/297(114, 155, 228, 212, 212, 269, 342, 383, 424)$ | $\{\emptyset, 124789, 125789, 14679, 15679, 24568, 268, 45\}$                                                         |
| 942:44    | $0, 0, 0, 0, 0, e^{12}, e^{13}, e^{14} + e^{26}, e^{16} + e^{35}$           | $1/11(5, 5, 7, 10, 8, 10, 12, 15, 15)$               | $\{\emptyset, 12389, 125789, 13568, 1678, 23679, 2569, 357\}$                                                         |
| 942:45    | $0, 0, 0, 0, 0, e^{12}, e^{13}, e^{24} + e^{16}, e^{35} + e^{26}$           | $1/23(10, 11, 15, 20, 17, 21, 25, 31, 32)$           | $\{\emptyset, 12389, 125789, 1369, 15679, 235678, 268, 357\}$                                                         |
| 942:46    | $0, 0, 0, 0, 0, e^{12}, e^{13}, e^{26} + e^{14}, e^{45} + e^{16}$           | $2/43(11, 8, 16, 16, 14, 19, 27, 27, 30)$            | $\{123489, 124789, 134568, 145678, 234679, 2469, 3457, 45\}$                                                          |

Table A.2 – Continued to next page

Table A.2 – Continued from previous page

| Name    | $g$                                                                                  | $N$                                                | Signatures $S$                                                    |
|---------|--------------------------------------------------------------------------------------|----------------------------------------------------|-------------------------------------------------------------------|
| 942:47  | $0, 0, 0, 0, 0, e^{12}, e^{13}, e^{16} + e^{24}, e^{26} + e^{45}$                    | 1/257(90, 139, 212, 180, 188, 229, 302, 319, 368)  | $\{\emptyset, 123589, 125789, 13569, 15679, 23678, 268, 37\}$     |
| 942:48  | $0, 0, 0, 0, 0, e^{12}, e^{24} + e^{13}, e^{16}, e^{26} + e^{15}$                    | 1/29(11, 13, 26, 24, 26, 24, 37, 35, 37)           | $\{\emptyset, 123489, 12789, 1369, 14679, 23678, 2468, 347\}$     |
| 942:49  | $0, 0, 0, 0, 0, e^{12}, e^{34}, e^{16} + e^{23}, e^{26} + e^{15}$                    | 1/59(21, 28, 42, 38, 56, 49, 80, 70, 77)           | $\{123489, 123789, 13469, 13679, 23468, 23678, 34, 37\}$          |
| 942:52  | $0, 0, 0, 0, 0, e^{12}, e^{24} + e^{13}, e^{16} + e^{34}, e^{26} + e^{35}$           | 2/85(20, 19, 29, 30, 29, 39, 49, 59, 58)           | $\{123789, 124589, 134679, 1569\}$                                |
| 942:54a | $0, 0, 0, 0, 0, e^{12}, e^{24} + e^{13}, e^{35} + e^{16}, e^{45} + e^{26}$           | 1/11(5, 5, 8, 8, 7, 10, 13, 15, 15)                | $\{\emptyset, 123489, 125789, 13569, 14679, 23678, 24568, 3457\}$ |
| 942:54b | $0, 0, 0, 0, 0, e^{12}, -e^{13} + e^{24}, e^{35} + e^{16}, e^{45} + e^{26}$          | 1/11(5, 5, 8, 8, 7, 10, 13, 15, 15)                | $\{\emptyset, 123489, 125789, 13569, 14679, 23678, 24568, 3457\}$ |
| 942:56  | $0, 0, 0, 0, 0, e^{12}, e^{34}, e^{35} + e^{16}, e^{26} + e^{13} + e^{45}$           | 1/191(100, 69, 138, 107, 131, 169, 245, 269, 238)  | $\{123489, 135679, 23678, 345\}$                                  |
| 942:57  | $0, 0, 0, 0, 0, e^{12}, e^{35} + e^{14}, e^{13} + e^{26}, e^{34} + e^{16}$           | 1/557(304, 175, 350, 433, 387, 479, 737, 654, 783) | $\{123789, 134568, 23569, 347\}$                                  |
| 942:58  | $0, 0, 0, 0, 0, e^{12}, e^{13} + e^{45}, e^{16} + e^{23}, e^{26} + e^{34}$           | 1/53(22, 25, 44, 28, 38, 47, 66, 69, 72)           | $\{124589, 14569, 25678, 57\}$                                    |
| 942:59  | $0, 0, 0, 0, 0, e^{12}, e^{35} + e^{14}, e^{16} + e^{23}, e^{26} + e^{34}$           | 1/101(29, 60, 58, 91, 62, 89, 120, 118, 149)       | $\{123589, 13569, 234568, 345\}$                                  |
| 942:60a | $0, 0, 0, 0, 0, e^{12}, e^{13} + e^{45}, e^{16}, e^{14} + e^{26} + e^{35}$           | 1/61(28, 25, 50, 50, 28, 53, 78, 81, 78)           | $\{1234789, 124589, 134679, 14569, 234568, 24678, 345, 47\}$      |
| 942:60b | $0, 0, 0, 0, 0, e^{12}, e^{45} - e^{13}, e^{16}, e^{35} + e^{14} + e^{26}$           | 1/61(28, 25, 50, 50, 28, 53, 78, 81, 78)           | $\{1234789, 124589, 134679, 14569, 234568, 24678, 345, 47\}$      |
| 942:61  | $0, 0, 0, 0, 0, e^{12}, e^{45} + e^{13}, e^{26}, e^{24} + e^{35} + e^{16}$           | 1/67(28, 30, 57, 56, 29, 58, 85, 88, 86)           | $\{1234789, 124589, 345, 47\}$                                    |
| 942:62  | $0, 0, 0, 0, 0, e^{12}, e^{14} + e^{35}, e^{13} + e^{26}, e^{45} + e^{16}$           | 1/53(26, 20, 40, 43, 29, 46, 69, 66, 72)           | $\{134568, 13678, 234679, 23569\}$                                |
| 942:63a | $0, 0, 0, 0, 0, e^{12}, e^{35} + e^{14}, e^{23} + e^{16}, e^{45} + e^{26}$           | 1/8(3, 4, 6, 7, 4, 7, 10, 10, 11)                  | $\{1234789, 123589, 134679, 13569, 234568, 23678, 345, 37\}$      |
| 942:63b | $0, 0, 0, 0, 0, e^{12}, -e^{14} + e^{35}, e^{23} + e^{16}, e^{26} + e^{45}$          | 1/8(3, 4, 6, 7, 4, 7, 10, 10, 11)                  | $\{1234789, 123589, 134679, 13569, 234568, 23678, 345, 37\}$      |
| 942:64  | $0, 0, 0, 0, 0, e^{12}, e^{13}, e^{16} + e^{24}, e^{26} + e^{15}$                    | 1/29(12, 13, 23, 24, 26, 25, 35, 37, 38)           | $\{\emptyset, 12389, 12789, 1369, 1679, 23678, 268, 37\}$         |
| 942:66  | $0, 0, 0, 0, 0, e^{12}, e^{13}, e^{16} + e^{34}, e^{26} + e^{35} + e^{14}$           | 1/151(74, 65, 83, 130, 121, 139, 157, 213, 204)    | $\{1245789, 13469, 2468, 3457\}$                                  |
| 942:67  | $0, 0, 0, 0, 0, e^{12}, e^{13}, e^{26} + e^{34}, e^{45} + e^{16} + e^{23}$           | 1/10(4, 5, 8, 6, 7, 9, 12, 14, 13)                 | $\{123589, 1368, 234679, 3457\}$                                  |
| 942:71  | $0, 0, 0, 0, 0, e^{12}, e^{24} + e^{13}, e^{16}, e^{26} + e^{34} + e^{15}$           | 1/53(21, 26, 39, 34, 52, 47, 60, 68, 73)           | $\{\emptyset, 1369, 14679, 347\}$                                 |
| 942:72  | $0, 0, 0, 0, 0, e^{12}, e^{23} + e^{14}, e^{13} + e^{26}, e^{45} + e^{16}$           | 1/109(55, 43, 86, 74, 79, 98, 129, 141, 153)       | $\{\emptyset, 125789, 14568, 24679\}$                             |
| 942:73a | $0, 0, 0, 0, 0, e^{12}, e^{34}, e^{13} + e^{26}, e^{45} + e^{16} + e^{23}$           | 1/61(26, 26, 52, 29, 49, 52, 81, 78, 78)           | $\{123489, 1235789, 134568, 13678, 23469, 235679, 345, 37\}$      |
| 942:73b | $0, 0, 0, 0, 0, e^{12}, e^{34}, e^{26} - e^{13}, e^{16} + e^{45} + e^{23}$           | 1/61(26, 26, 52, 29, 49, 52, 81, 78, 78)           | $\{123489, 1235789, 134568, 13678, 23469, 235679, 345, 37\}$      |
| 942:74  | $0, 0, 0, 0, 0, e^{12}, e^{34}, e^{26} + e^{13}, e^{16} + e^{35} + e^{24}$           | 1/17(8, 5, 10, 16, 11, 13, 26, 18, 21)             | $\{123489, 134568, 23469, 345\}$                                  |
| 942:75  | $0, 0, 0, 0, 0, e^{12}, e^{24} + e^{13}, e^{16} + e^{34}, e^{15} + e^{26}$           | 1/83(38, 37, 56, 57, 74, 75, 94, 113, 112)         | $\{\emptyset, 23678, 2468, 347\}$                                 |
| 942:76  | $0, 0, 0, 0, 0, e^{12}, e^{13}, e^{16} + e^{45}, e^{14} + e^{35} + e^{26}$           | 1/10(5, 4, 7, 8, 6, 9, 12, 14, 13)                 | $\{123489, 145679, 2468, 3457\}$                                  |
| 942:77  | $0, 0, 0, 0, 0, e^{12}, e^{13}, e^{45} + e^{26}, e^{35} + e^{24} + e^{16}$           | 1/155(63, 79, 110, 126, 95, 142, 173, 221, 205)    | $\{123489, 14678, 24569, 3457\}$                                  |
| 942:78  | $0, 0, 0, 0, 0, e^{12}, e^{24} + e^{13}, e^{26} + e^{15}, e^{35} + e^{16}$           | 1/457(239, 165, 313, 387, 330, 404, 552, 569, 643) | $\{\emptyset, 123489, 14678, 23679\}$                             |
| 942:79  | $0, 0, 0, 0, 0, e^{12}, e^{23} + e^{14}, e^{15} + e^{26}, e^{16} + e^{35}$           | 2/61(17, 11, 23, 17, 22, 28, 34, 39, 45)           | $\{123578, 156789, 234567, 4579\}$                                |
| 942:80  | $0, 0, 0, 0, 0, e^{12}, e^{34}, e^{26} + e^{15}, e^{16} + e^{45} + e^{23}$           | 1/67(29, 28, 58, 30, 56, 57, 88, 85, 86)           | $\{1235789, 134568, 235679, 345\}$                                |
| 942:82  | $0, 0, 0, 0, 0, e^{12}, e^{13} + e^{45}, e^{23} + e^{16}, e^{14} + e^{26}$           | 1/217(100, 79, 200, 158, 142, 179, 300, 279, 258)  | $\{124789, 14679, 24568, 45\}$                                    |
| 942:83  | $0, 0, 0, 0, 0, e^{12}, e^{15} + e^{34}, e^{16} + e^{23}, e^{14} + e^{26}$           | 1/61(23, 22, 46, 44, 67, 45, 90, 68, 67)           | $\{123489, 13469, 234568, 345\}$                                  |
| 942:84a | $0, 0, 0, 0, 0, e^{12}, e^{13} + e^{45}, e^{34} + e^{16}, e^{14} + e^{35} + e^{26}$  | 43/241(3, 2, 4, 4, 3, 5, 7, 8, 7)                  | $\{124589, 134679, 24678, 345\}$                                  |
| 942:84b | $0, 0, 0, 0, 0, e^{12}, -e^{13} + e^{45}, e^{34} + e^{16}, e^{26} + e^{35} + e^{14}$ | 43/241(3, 2, 4, 4, 3, 5, 7, 8, 7)                  | $\{124589, 134679, 24678, 345\}$                                  |
| 942:85  | $0, 0, 0, 0, 0, e^{12}, e^{45} + e^{13}, e^{34} + e^{26}, e^{35} + e^{16} + e^{24}$  | 67/589(3, 5, 7, 6, 4, 8, 10, 13, 11)               | $\{124589, 345\}$                                                 |
| 942:86  | $0, 0, 0, 0, 0, e^{12}, e^{13}, e^{16} + e^{23}, e^{14} + e^{26} + e^{35}$           | 3/17(2, 3, 4, 6, 4, 5, 6, 7, 8)                    | $\{123489, 13469, 2345678, 3457\}$                                |
| 942:87  | $0, 0, 0, 0, 0, e^{12}, e^{13}, e^{14} + e^{26}, e^{23} + e^{16} + e^{45}$           | 2/31(7, 6, 14, 12, 8, 13, 21, 19, 20)              | $\{123489, 134568, 234679, 3457\}$                                |
| 942:91  | $0, 0, 0, 0, 0, e^{12}, e^{13}, e^{16} + e^{24}, e^{15} + e^{26} + e^{34}$           | 1/73(27, 38, 49, 54, 76, 65, 76, 92, 103)          | $\{1245789, 145679, 2345678, 3457\}$                              |
| 942:92  | $0, 0, 0, 0, 0, e^{12}, e^{24} + e^{13}, e^{16} + e^{23}, e^{26} + e^{15}$           | 1/86(36, 37, 72, 71, 74, 73, 108, 109, 110)        | $\{\emptyset, 12789, 14679, 2468\}$                               |
| 942:93a | $0, 0, 0, 0, 0, e^{12}, e^{13} + e^{24}, e^{25} + e^{16}, e^{26} + e^{15}$           | 1/43(18, 18, 37, 37, 36, 36, 55, 54, 54)           | $\{\emptyset, 123489, 12789, 1369, 14679, 23678, 2468, 347\}$     |
| 942:93b | $0, 0, 0, 0, 0, e^{12}, e^{24} + e^{13}, -e^{16} + e^{25}, e^{15} + e^{26}$          | 1/43(18, 18, 37, 37, 36, 36, 55, 54, 54)           | $\{\emptyset, 123489, 12789, 1369, 14679, 23678, 2468, 347\}$     |
| 942:94  | $0, 0, 0, 0, 0, e^{12}, e^{24} + e^{13}, e^{34} + e^{16}, e^{35} + e^{14} + e^{26}$  | 10/77(4, 3, 5, 6, 5, 7, 9, 11, 10)                 | $\{124589, 134679\}$                                              |
| 942:95  | $0, 0, 0, 0, 0, e^{12}, e^{24} + e^{13}, e^{35} + e^{16}, e^{34} + e^{26} + e^{15}$  | 77/757(5, 4, 6, 7, 8, 9, 11, 14, 13)               | $\{13569, 3457\}$                                                 |
| 942:97  | $0, 0, 0, 0, 0, e^{12}, e^{14} + e^{23}, e^{35} + e^{16}, e^{26} + e^{34} + e^{15}$  | 7/38(3, 2, 4, 3, 4, 5, 6, 8, 7)                    | $\{123579, 234567\}$                                              |
| 942:98  | $0, 0, 0, 0, 0, e^{12}, e^{34}, e^{35} + e^{24} + e^{16}, e^{26} + e^{13} + e^{45}$  | 19/49(1, 1, 2, 2, 1, 2, 4, 3, 3)                   | $\{123489, 345\}$                                                 |
| 942:99a | $0, 0, 0, 0, 0, e^{12}, e^{35} + e^{14}, e^{13} + e^{26}, e^{45} + e^{23} + e^{16}$  | 3/7(1, 1, 2, 2, 1, 2, 3, 3, 3)                     | $\{1234789, 123589, 345, 37\}$                                    |

Table A.2 – Continued to next page

Table A.2 – Continued from previous page

| Name     | $g$                                                                                       | $N$                                                  | Signatures $S$                                                                                                        |
|----------|-------------------------------------------------------------------------------------------|------------------------------------------------------|-----------------------------------------------------------------------------------------------------------------------|
| 942:99b  | $0, 0, 0, 0, 0, e^{12},$<br>$e^{14} + e^{35}, -e^{13} + e^{26}, e^{45} + e^{16} + e^{23}$ | $3/7(1, 1, 2, 2, 1, 2, 3, 3, 3)$                     | $\{1234789, 123589, 345, 37\}$                                                                                        |
| 942:100  | $0, 0, 0, 0, 0, e^{12}, e^{35} + e^{14}, e^{26} + e^{13}, e^{25} + e^{16} + e^{34}$       | $41/229(3, 1, 2, 5, 6, 4, 8, 5, 7)$                  | $\{123589, 345\}$                                                                                                     |
| 942:101a | $0, 0, 0, 0, 0, e^{12}, e^{45} + e^{13}, e^{16} + e^{23}, e^{14} + e^{26} + e^{35}$       | $3/7(1, 1, 2, 2, 1, 2, 3, 3, 3)$                     | $\{1234789, 134679, 234568, 345\}$                                                                                    |
| 942:101b | $0, 0, 0, 0, 0, e^{12},$<br>$-e^{13} + e^{45}, e^{23} + e^{16}, e^{14} + e^{26} + e^{35}$ | $3/7(1, 1, 2, 2, 1, 2, 3, 3, 3)$                     | $\{1234789, 134679, 234568, 345\}$                                                                                    |
| 942:102a | $0, 0, 0, 0, 0, e^{12}, e^{14} + e^{35}, e^{16} + e^{23}, e^{13} + e^{45} + e^{26}$       | $3/7(1, 1, 2, 2, 1, 2, 3, 3, 3)$                     | $\{1234789, 123589, 134679, 13569, 234568, 23678, 345, 37\}$                                                          |
| 942:102b | $0, 0, 0, 0, 0, e^{12}, e^{14} + e^{35}, e^{23} - e^{16}, e^{13} + e^{45} + e^{26}$       | $3/7(1, 1, 2, 2, 1, 2, 3, 3, 3)$                     | $\{1234789, 123589, 134679, 13569, 234568, 23678, 345, 37\}$                                                          |
| 942:102c | $0, 0, 0, 0, 0, e^{12}, e^{35} - e^{14}, e^{23} + e^{16}, e^{45} + e^{26} + e^{13}$       | $3/7(1, 1, 2, 2, 1, 2, 3, 3, 3)$                     | $\{1234789, 123589, 134679, 13569, 234568, 23678, 345, 37\}$                                                          |
| 942:102d | $0, 0, 0, 0, 0, e^{12},$<br>$-e^{14} + e^{35}, e^{23} - e^{16}, e^{13} + e^{26} + e^{45}$ | $3/7(1, 1, 2, 2, 1, 2, 3, 3, 3)$                     | $\{1234789, 123589, 134679, 13569, 234568, 23678, 345, 37\}$                                                          |
| 942:103a | $0, 0, 0, 0, 0, e^{12}, e^{35} + e^{14}, e^{16} + e^{23}, e^{26} + e^{34} + e^{15}$       | $1/19(0, 11, 0, 22, 22, 11, 22, 11, 22)$             | $\{123589, 13569, 234568, 345\}$                                                                                      |
| 942:103b | $0, 0, 0, 0, 0, e^{12}, e^{35} - e^{14}, e^{16} + e^{23}, e^{26} + e^{15} + e^{34}$       | $1/19(0, 11, 0, 22, 22, 11, 22, 11, 22)$             | $\{123589, 13569, 234568, 345\}$                                                                                      |
| 942:105  | $0, 0, 0, 0, 0, e^{12}, e^{23} + e^{14}, e^{13} + e^{26}, e^{16} + e^{25} + e^{34}$       | $21/167(4, 3, 6, 5, 8, 7, 9, 10, 11)$                | $\{23569, 3457\}$                                                                                                     |
| 942:106  | $0, 0, 0, 0, 0, e^{12}, e^{13}, e^{23} + e^{45} + e^{16}, e^{35} + e^{26} + e^{14}$       | $3/7(1, 1, 2, 2, 1, 2, 3, 3, 3)$                     | $\{123489, 3457\}$                                                                                                    |
| 942:107  | $0, 0, 0, 0, 0, e^{12}, e^{13}, e^{25} + e^{34} + e^{16}, e^{14} + e^{35} + e^{26}$       | $17/37(1, 1, 1, 2, 2, 2, 2, 3, 3)$                   | $\{124589, 345\}$                                                                                                     |
| 942:108  | $0, 0, 0, 0, 0, e^{12}, e^{24} + e^{13}, e^{26} + e^{15}, e^{23} + e^{16} + e^{45}$       | $1/2(0, 1, 0, -1, 2, 1, 0, 2, 1)$                    | $\{124578, 156789\}$                                                                                                  |
| 942:126  | $0, 0, 0, 0, 0, e^{12}, e^{13}, e^{16}, e^{45} + e^{17}$                                  | $1/19(5, 14, 16, 13, 13, 19, 21, 24, 26)$            | $\{\emptyset, 123489, 123589, 124578, 1278, 13469, 13569, 14567, 167, 2346789, 2356789, 24568, 268, 3479, 3579, 45\}$ |
| 942:127  | $0, 0, 0, 0, 0, e^{12}, e^{13}, e^{26}, e^{45} + e^{17}$                                  | $4/33(3, 4, 6, 6, 6, 7, 9, 11, 12)$                  | $\{\emptyset, 123489, 123589, 124578, 1278, 134689, 135689, 145678, 1678, 234679, 235679, 2456, 26, 3479, 3579, 45\}$ |
| 942:128  | $0, 0, 0, 0, 0, e^{12}, e^{13}, e^{16}, e^{45} + e^{37}$                                  | $1/28(8, 20, 17, 21, 21, 28, 25, 36, 42)$            | $\{\emptyset, 123489, 123589, 124789, 125789, 13469, 13569, 14679, 15679, 2345678, 23678, 24568, 268, 3457, 37, 45\}$ |
| 942:129  | $0, 0, 0, 0, 0, e^{12}, e^{13}, e^{26}, e^{37} + e^{45}$                                  | $1/12(6, 5, 6, 9, 9, 11, 12, 16, 18)$                | $\{\emptyset, 123489, 123589, 124789, 125789, 134689, 135689, 146789, 156789, 234567, 2367, 2456, 26, 3457, 37, 45\}$ |
| 942:142  | $0, 0, 0, 0, 0, e^{12}, e^{13}, e^{26} + e^{14}, e^{17} + e^{45}$                         | $4/29(3, 3, 5, 6, 5, 6, 8, 9, 11)$                   | $\{123489, 124578, 134689, 145678, 234679, 2456, 3479, 45\}$                                                          |
| 942:143  | $0, 0, 0, 0, 0, e^{12}, e^{13}, e^{16} + e^{24}, e^{17} + e^{45}$                         | $1/13(4, 9, 10, 8, 10, 13, 14, 17, 18)$              | $\{\emptyset, 123589, 1278, 13569, 167, 2356789, 268, 3579\}$                                                         |
| 942:144  | $0, 0, 0, 0, 0, e^{12}, e^{13}, e^{14} + e^{26}, e^{45} + e^{37}$                         | $1/172(90, 67, 85, 134, 126, 157, 175, 224, 260)$    | $\{123489, 124789, 134689, 146789, 234567, 2456, 3457, 45\}$                                                          |
| 942:145  | $0, 0, 0, 0, 0, e^{12}, e^{13}, e^{16} + e^{24}, e^{45} + e^{37}$                         | $1/99(34, 65, 56, 68, 78, 99, 90, 133, 146)$         | $\{\emptyset, 123589, 125789, 13569, 15679, 23678, 268, 37\}$                                                         |
| 942:146  | $0, 0, 0, 0, 0, e^{12}, e^{13}, e^{34} + e^{16}, e^{45} + e^{17}$                         | $1/23(7, 17, 17, 14, 17, 24, 24, 31, 31)$            | $\{\emptyset, 123589, 124578, 13469, 167, 2356789, 24568, 3479\}$                                                     |
| 942:147  | $0, 0, 0, 0, 0, e^{12}, e^{13}, e^{26} + e^{34}, e^{45} + e^{17}$                         | $1/16(6, 8, 11, 11, 12, 14, 17, 22, 23)$             | $\{\emptyset, 123589, 124578, 135689, 145678, 234679, 26, 3479\}$                                                     |
| 942:148  | $0, 0, 0, 0, 0, e^{12}, e^{13}, e^{34} + e^{16}, e^{37} + e^{45}$                         | $1/83(25, 59, 49, 60, 63, 84, 74, 109, 123)$         | $\{\emptyset, 123589, 124789, 13469, 15679, 23678, 24568, 3457\}$                                                     |
| 942:149  | $0, 0, 0, 0, 0, e^{12}, e^{13}, e^{34} + e^{26}, e^{37} + e^{45}$                         | $1/172(84, 70, 89, 135, 127, 154, 173, 224, 262)$    | $\{123489, 125789, 134689, 156789, 2367, 2456, 37, 45\}$                                                              |
| 942:154  | $0, 0, 0, 0, 0, e^{12}, e^{13}, e^{16}, e^{37} + e^{14} + e^{25}$                         | $1/17(6, 10, 9, 18, 14, 16, 15, 22, 24)$             | $\{123489, 124789, 134569, 145679, 2345678, 24568, 347, 4\}$                                                          |
| 942:155  | $0, 0, 0, 0, 0, e^{12}, e^{13}, e^{16}, e^{17} + e^{45} + e^{23}$                         | $1/227(73, 146, 176, 161, 161, 219, 249, 292, 322)$  | $\{\emptyset, 13469, 13569, 14567, 167, 3479, 3579, 45\}$                                                             |
| 942:157  | $0, 0, 0, 0, 0, e^{12}, e^{13}, e^{26}, e^{37} + e^{25} + e^{14}$                         | $1/293(138, 125, 136, 272, 285, 263, 274, 388, 410)$ | $\{\emptyset, 12389, 12789, 135689, 156789, 23567, 256, 37\}$                                                         |
| 942:158  | $0, 0, 0, 0, 0, e^{12}, e^{13}, e^{26}, e^{17} + e^{23} + e^{45}$                         | $4/29(2, 4, 6, 5, 5, 6, 8, 10, 10)$                  | $\{123489, 123589, 124578, 1278, 234679, 235679, 2456, 26\}$                                                          |
| 942:159  | $0, 0, 0, 0, 0, e^{12}, e^{13}, e^{26}, e^{35} + e^{24} + e^{17}$                         | $1/81(33, 37, 49, 78, 66, 70, 82, 107, 115)$         | $\{\emptyset, 12389, 12478, 134689, 1678, 23679, 246, 3479\}$                                                         |
| 942:160  | $0, 0, 0, 0, 0, e^{12}, e^{13}, e^{23} + e^{16}, e^{45} + e^{17}$                         | $1/20(7, 13, 14, 14, 14, 20, 21, 27, 28)$            | $\{\emptyset, 124578, 1278, 14567, 167, 24568, 268, 45\}$                                                             |
| 942:161  | $0, 0, 0, 0, 0, e^{12}, e^{13}, e^{23} + e^{16}, e^{37} + e^{45}$                         | $1/107(32, 75, 64, 80, 80, 107, 96, 139, 160)$       | $\{\emptyset, 124789, 125789, 14679, 15679, 24568, 268, 45\}$                                                         |
| 942:162  | $0, 0, 0, 0, 0, e^{12}, e^{13}, e^{26} + e^{14}, e^{17} + e^{25}$                         | $1/227(75, 111, 161, 222, 200, 186, 236, 297, 311)$  | $\{\emptyset, 12389, 12578, 135689, 1678, 23679, 256, 3579\}$                                                         |
| 942:164  | $0, 0, 0, 0, 0, e^{12}, e^{13}, e^{14} + e^{26}, e^{15} + e^{37}$                         | $1/32(14, 15, 15, 30, 30, 29, 29, 44, 44)$           | $\{\emptyset, 12389, 12789, 13689, 16789, 2367, 26, 37\}$                                                             |
| 942:165  | $0, 0, 0, 0, 0, e^{12}, e^{13}, e^{16} + e^{24}, e^{15} + e^{37}$                         | $1/81(32, 49, 39, 64, 78, 81, 71, 113, 110)$         | $\{\emptyset, 12389, 12789, 1369, 1679, 23678, 268, 37\}$                                                             |
| 942:166  | $0, 0, 0, 0, 0, e^{12}, e^{13}, e^{16} + e^{24}, e^{17} + e^{35}$                         | $1/13(5, 8, 8, 10, 10, 13, 13, 18, 18)$              | $\{\emptyset, 12389, 1278, 1369, 167, 236789, 268, 379\}$                                                             |
| 942:167  | $0, 0, 0, 0, 0, e^{12}, e^{13}, e^{14} + e^{26}, e^{37} + e^{25}$                         | $1/281(132, 127, 128, 254, 261, 259, 260, 386, 388)$ | $\{\emptyset, 12389, 12789, 135689, 156789, 23567, 256, 37\}$                                                         |
| 942:168  | $0, 0, 0, 0, 0, e^{12}, e^{13}, e^{24} + e^{16}, e^{25} + e^{37}$                         | $1/24(10, 13, 12, 20, 21, 23, 22, 33, 34)$           | $\{\emptyset, 12389, 12789, 13569, 15679, 235678, 2568, 37\}$                                                         |
| 942:169  | $0, 0, 0, 0, 0, e^{12}, e^{13}, e^{34} + e^{16}, e^{17} + e^{25}$                         | $1/13(5, 8, 8, 10, 10, 13, 13, 18, 18)$              | $\{\emptyset, 12389, 124578, 134569, 167, 236789, 24568, 34579\}$                                                     |

Table A.2 – Continued to next page

Table A.2 – Continued from previous page

| Name     | $g$                                                                         | $N$                                                  | Signatures $S$                                                                                                        |
|----------|-----------------------------------------------------------------------------|------------------------------------------------------|-----------------------------------------------------------------------------------------------------------------------|
| 942:170  | $0, 0, 0, 0, 0, e^{12}, e^{13}, e^{26} + e^{34}, e^{17} + e^{25}$           | $1/61(24, 31, 36, 50, 53, 55, 60, 86, 84)$           | $\{\emptyset, 12389, 124578, 135689, 14678, 234679, 256, 34579\}$                                                     |
| 942:171  | $0, 0, 0, 0, 0, e^{12}, e^{13}, e^{26} + e^{34}, e^{25} + e^{37}$           | $1/17(9, 7, 7, 16, 16, 16, 16, 23, 23)$              | $\{\emptyset, 12389, 124789, 135689, 1456789, 234567, 256, 347\}$                                                     |
| 942:190  | $0, 0, 0, 0, 0, e^{12}, e^{13}, e^{16}, e^{17} + e^{26} + e^{45}$           | $1/257(82, 147, 212, 188, 188, 229, 294, 311, 376)$  | $\{\emptyset, 123489, 123589, 13469, 13569, 24568, 268, 45\}$                                                         |
| 942:191a | $0, 0, 0, 0, 0, e^{12}, e^{13}, e^{16}, e^{26} + e^{45} + e^{37}$           | $1/89(28, 55, 55, 69, 69, 83, 83, 111, 138)$         | $\{\emptyset, 123489, 123589, 124789, 125789, 13469, 13569, 14679, 15679, 2345678, 23678, 24568, 268, 3457, 37, 45\}$ |
| 942:191b | $0, 0, 0, 0, 0, -e^{12}, e^{13}, e^{16}, e^{37} + e^{45} + e^{26}$          | $1/89(28, 55, 55, 69, 69, 83, 83, 111, 138)$         | $\{\emptyset, 123489, 123589, 124789, 125789, 13469, 13569, 14679, 15679, 2345678, 23678, 24568, 268, 3457, 37, 45\}$ |
| 942:193  | $0, 0, 0, 0, 0, e^{12}, e^{13}, e^{26}, e^{37} + e^{45} + e^{16}$           | $1/172(92, 70, 81, 127, 127, 162, 173, 232, 254)$    | $\{134689, 135689, 146789, 156789, 234567, 2367, 2456, 26\}$                                                          |
| 942:195  | $0, 0, 0, 0, 0, e^{12}, e^{13}, e^{45} + e^{16}, e^{26} + e^{17}$           | $1/139(53, 76, 99, 91, 91, 129, 152, 182, 205)$      | $\{123459, 1239, 134689, 135689, 2456, 26, 48, 58\}$                                                                  |
| 942:196a | $0, 0, 0, 0, 0, e^{12}, e^{13}, e^{16} + e^{45}, e^{37} + e^{26}$           | $2/23(5, 6, 6, 8, 8, 11, 11, 16, 17)$                | $\{\emptyset, 123489, 123589, 124789, 125789, 134569, 1369, 145679, 1679, 234678, 235678, 2468, 2568, 3457, 37, 45\}$ |
| 942:196b | $0, 0, 0, 0, 0, -e^{12}, e^{13}, e^{45} + e^{16}, e^{37} + e^{26}$          | $2/23(5, 6, 6, 8, 8, 11, 11, 16, 17)$                | $\{\emptyset, 123489, 123589, 124789, 125789, 134569, 1369, 145679, 1679, 234678, 235678, 2468, 2568, 3457, 37, 45\}$ |
| 942:198  | $0, 0, 0, 0, 0, e^{12}, e^{13}, e^{26} + e^{45}, e^{16} + e^{37}$           | $1/23(10, 12, 11, 17, 17, 22, 21, 34, 32)$           | $\{\emptyset, 123489, 123589, 124789, 125789, 3457, 37, 45\}$                                                         |
| 942:203  | $0, 0, 0, 0, 0, e^{12}, e^{13}, e^{16} + e^{45}, e^{14} + e^{25} + e^{37}$  | $3/14(2, 3, 2, 4, 3, 5, 4, 7, 6)$                    | $\{123489, 124789, 134569, 145679\}$                                                                                  |
| 942:204  | $0, 0, 0, 0, 0, e^{12}, e^{13}, e^{45} + e^{16}, e^{35} + e^{17} + e^{24}$  | $1/77(26, 53, 54, 53, 52, 79, 80, 105, 106)$         | $\{\emptyset, 12478, 167, 2468\}$                                                                                     |
| 942:205  | $0, 0, 0, 0, 0, e^{12}, e^{13}, e^{45} + e^{26}, e^{14} + e^{25} + e^{37}$  | $6/47(4, 4, 3, 6, 6, 8, 7, 12, 10)$                  | $\{134689, 146789, 3457, 45\}$                                                                                        |
| 942:206  | $0, 0, 0, 0, 0, e^{12}, e^{13}, e^{45} + e^{26}, e^{35} + e^{24} + e^{17}$  | $1/525(181, 296, 345, 411, 362, 477, 526, 773, 707)$ | $\{\emptyset, 12478, 134689, 23679\}$                                                                                 |
| 942:207  | $0, 0, 0, 0, 0, e^{12}, e^{13}, e^{26} + e^{14}, e^{24} + e^{37} + e^{15}$  | $1/117(52, 54, 55, 108, 110, 106, 107, 160, 162)$    | $\{\emptyset, 12389, 12789, 37\}$                                                                                     |
| 942:208  | $0, 0, 0, 0, 0, e^{12}, e^{13}, e^{14} + e^{26}, e^{17} + e^{45} + e^{23}$  | $4/17(1, 2, 4, 4, 2, 3, 5, 5, 6)$                    | $\{123489, 124578, 234679, 2456\}$                                                                                    |
| 942:209  | $0, 0, 0, 0, 0, e^{12}, e^{13}, e^{14} + e^{26}, e^{24} + e^{17} + e^{35}$  | $1/102(41, 48, 62, 96, 82, 89, 103, 137, 144)$       | $\{\emptyset, 12389, 1678, 23679\}$                                                                                   |
| 942:212  | $0, 0, 0, 0, 0, e^{12}, e^{13}, e^{24} + e^{16}, e^{45} + e^{23} + e^{17}$  | $1/49(16, 32, 37, 32, 37, 48, 53, 64, 69)$           | $\{\emptyset, 13569, 167, 3579\}$                                                                                     |
| 942:214  | $0, 0, 0, 0, 0, e^{12}, e^{13}, e^{34} + e^{16}, e^{25} + e^{37} + e^{14}$  | $1/113(48, 63, 53, 106, 91, 111, 101, 159, 154)$     | $\{124789, 134569, 24568, 347\}$                                                                                      |
| 942:215  | $0, 0, 0, 0, 0, e^{12}, e^{13}, e^{16} + e^{34}, e^{15} + e^{24} + e^{37}$  | $1/25(9, 15, 13, 20, 26, 24, 22, 33, 35)$            | $\{123589, 134569, 24568, 5\}$                                                                                        |
| 942:216  | $0, 0, 0, 0, 0, e^{12}, e^{13}, e^{16} + e^{34}, e^{17} + e^{45} + e^{23}$  | $1/83(28, 56, 59, 53, 62, 84, 87, 112, 115)$         | $\{\emptyset, 13469, 167, 3479\}$                                                                                     |
| 942:217a | $0, 0, 0, 0, 0, e^{12}, e^{13}, e^{16} + e^{34}, e^{17} + e^{35} + e^{24}$  | $1/13(5, 8, 8, 10, 10, 13, 13, 18, 18)$              | $\{\emptyset, 12389, 12478, 13469, 167, 236789, 2468, 3479\}$                                                         |
| 942:217b | $0, 0, 0, 0, 0, -e^{12}, e^{13}, e^{16} + e^{34}, e^{17} + e^{35} + e^{24}$ | $1/13(5, 8, 8, 10, 10, 13, 13, 18, 18)$              | $\{\emptyset, 12389, 12478, 13469, 167, 236789, 2468, 3479\}$                                                         |
| 942:218  | $0, 0, 0, 0, 0, e^{12}, e^{13}, e^{26} + e^{34}, e^{25} + e^{14} + e^{37}$  | $1/49(24, 21, 22, 44, 47, 45, 46, 66, 68)$           | $\{\emptyset, 12389, 135689, 256\}$                                                                                   |
| 942:219  | $0, 0, 0, 0, 0, e^{12}, e^{13}, e^{34} + e^{26}, e^{24} + e^{37} + e^{15}$  | $1/53(25, 24, 24, 49, 48, 49, 49, 73, 73)$           | $\{\emptyset, 12389, 146789, 23467\}$                                                                                 |
| 942:220  | $0, 0, 0, 0, 0, e^{12}, e^{13}, e^{26} + e^{34}, e^{45} + e^{23} + e^{17}$  | $1/14(4, 8, 11, 9, 10, 12, 15, 20, 19)$              | $\{123589, 124578, 234679, 26\}$                                                                                      |
| 942:230  | $0, 0, 0, 0, 0, e^{12}, e^{13}, e^{16} + e^{24}, e^{17} + e^{45} + e^{26}$  | $1/41(14, 23, 32, 28, 32, 37, 46, 51, 60)$           | $\{\emptyset, 123589, 13569, 268\}$                                                                                   |
| 942:231  | $0, 0, 0, 0, 0, e^{12}, e^{13}, e^{14} + e^{26}, e^{37} + e^{45} + e^{16}$  | $2/47(13, 9, 11, 18, 17, 22, 24, 31, 35)$            | $\{134689, 146789, 234567, 2456\}$                                                                                    |
| 942:233a | $0, 0, 0, 0, 0, e^{12}, e^{13}, e^{16} + e^{24}, e^{26} + e^{37} + e^{45}$  | $1/153(55, 89, 89, 110, 123, 144, 144, 199, 233)$    | $\{\emptyset, 123589, 125789, 13569, 15679, 23678, 268, 37\}$                                                         |
| 942:233b | $0, 0, 0, 0, 0, -e^{12}, e^{13}, e^{16} + e^{24}, e^{26} + e^{37} + e^{45}$ | $1/153(55, 89, 89, 110, 123, 144, 144, 199, 233)$    | $\{\emptyset, 123589, 125789, 13569, 15679, 23678, 268, 37\}$                                                         |
| 942:235  | $0, 0, 0, 0, 0, e^{12}, e^{13}, e^{34} + e^{16}, e^{45} + e^{17} + e^{26}$  | $1/489(191, 261, 331, 312, 401, 452, 522, 643, 713)$ | $\{\emptyset, 123589, 13469, 24568\}$                                                                                 |
| 942:236a | $0, 0, 0, 0, 0, e^{12}, e^{13}, e^{34} + e^{16}, e^{37} + e^{45} + e^{26}$  | $1/153(55, 89, 89, 110, 123, 144, 144, 199, 233)$    | $\{\emptyset, 123589, 124789, 13469, 15679, 23678, 24568, 3457\}$                                                     |
| 942:236b | $0, 0, 0, 0, 0, -e^{12}, e^{13}, e^{34} + e^{16}, e^{37} + e^{45} + e^{26}$ | $1/153(55, 89, 89, 110, 123, 144, 144, 199, 233)$    | $\{\emptyset, 123589, 124789, 13469, 15679, 23678, 24568, 3457\}$                                                     |
| 942:238  | $0, 0, 0, 0, 0, e^{12}, e^{13}, e^{26} + e^{34}, e^{45} + e^{37} + e^{16}$  | $1/28(16, 10, 13, 23, 19, 26, 29, 36, 42)$           | $\{134689, 156789, 2367, 2456\}$                                                                                      |
| 942:240a | $0, 0, 0, 0, 0, e^{12}, e^{13}, e^{16} + e^{45}, e^{37} + e^{14} + e^{26}$  | $2/19(5, 4, 4, 8, 6, 9, 9, 14, 13)$                  | $\{123489, 124789, 134569, 145679, 234678, 2468, 3457, 45\}$                                                          |
| 942:240b | $0, 0, 0, 0, 0, -e^{12}, e^{13}, e^{16} + e^{45}, e^{37} + e^{26} + e^{14}$ | $2/19(5, 4, 4, 8, 6, 9, 9, 14, 13)$                  | $\{123489, 124789, 134569, 145679, 234678, 2468, 3457, 45\}$                                                          |
| 942:242  | $0, 0, 0, 0, 0, e^{12}, e^{13}, e^{16} + e^{45}, e^{17} + e^{26} + e^{34}$  | $2/61(11, 17, 23, 22, 17, 28, 34, 39, 45)$           | $\{123459, 134689, 2456, 48\}$                                                                                        |
| 942:243  | $0, 0, 0, 0, 0, e^{12}, e^{13}, e^{45} + e^{26}, e^{16} + e^{24} + e^{37}$  | $16/201(5, 7, 6, 10, 9, 12, 11, 19, 17)$             | $\{123489, 124789, 3457, 45\}$                                                                                        |
| 942:245  | $0, 0, 0, 0, 0, e^{12}, e^{13}, e^{23} + e^{16}, e^{37} + e^{25} + e^{14}$  | $1/14(4, 9, 8, 16, 11, 13, 12, 17, 20)$              | $\{123489, 134569, 2345678, 347\}$                                                                                    |
| 942:246  | $0, 0, 0, 0, 0, e^{12}, e^{13}, e^{23} + e^{16}, e^{24} + e^{35} + e^{17}$  | $1/73(26, 43, 52, 61, 52, 69, 78, 95, 104)$          | $\{123458, 1356, 2345678, 357\}$                                                                                      |
| 942:250  | $0, 0, 0, 0, 0, e^{12}, e^{13}, e^{23} + e^{16}, e^{45} + e^{17} + e^{26}$  | $43/235(2, 3, 4, 4, 4, 5, 6, 7, 8)$                  | $\{\emptyset, 24568, 268, 45\}$                                                                                       |
| 942:251a | $0, 0, 0, 0, 0, e^{12}, e^{13}, e^{23} + e^{16}, e^{26} + e^{37} + e^{45}$  | $25/161(2, 4, 4, 5, 5, 6, 6, 8, 10)$                 | $\{123489, 123589, 13469, 13569, 2345678, 23678, 3457, 37\}$                                                          |
| 942:251b | $0, 0, 0, 0, 0, -e^{12}, e^{13}, e^{23} + e^{16}, e^{37} + e^{45} + e^{26}$ | $25/161(2, 4, 4, 5, 5, 6, 6, 8, 10)$                 | $\{123489, 123589, 13469, 13569, 2345678, 23678, 3457, 37\}$                                                          |

Table A.2 – Continued to next page



Table A.2 – Continued from previous page

| Name     | $g$                                                                                  | $N$                                             | Signatures $S$                                                                                                        |
|----------|--------------------------------------------------------------------------------------|-------------------------------------------------|-----------------------------------------------------------------------------------------------------------------------|
| 942:253  | $0, 0, 0, 0, 0, e^{12}, e^{13}, e^{14} + e^{26}, e^{37} + e^{16} + e^{25}$           | 1/159(74, 72, 73, 144, 148, 146, 147, 218, 220) | $\{\emptyset, 12389, 12789, 37\}$                                                                                     |
| 942:257  | $0, 0, 0, 0, 0, e^{12}, e^{13}, e^{16} + e^{24}, e^{35} + e^{17} + e^{26}$           | 1/77(31, 40, 49, 62, 62, 71, 80, 102, 111)      | $\{\emptyset, 12389, 1369, 268\}$                                                                                     |
| 942:260  | $0, 0, 0, 0, 0, e^{12}, e^{13}, e^{34} + e^{16}, e^{26} + e^{35} + e^{17}$           | 1/14(6, 7, 8, 11, 12, 13, 14, 19, 20)           | $\{\emptyset, 12389, 13469, 2468\}$                                                                                   |
| 942:261  | $0, 0, 0, 0, 0, e^{12}, e^{13}, e^{26} + e^{34}, e^{16} + e^{25} + e^{37}$           | 1/59(28, 26, 27, 53, 56, 54, 55, 80, 82)        | $\{\emptyset, 12389, 124789, 347\}$                                                                                   |
| 942:263  | $0, 0, 0, 0, 0, e^{12}, e^{13}, e^{16} + e^{45} + e^{23}, e^{17} + e^{26}$           | 6/65(4, 6, 8, 7, 7, 10, 12, 14, 16)             | $\{2456, 26, 48, 58\}$                                                                                                |
| 942:265  | $0, 0, 0, 0, 0, e^{12}, e^{13}, e^{14} + e^{26} + e^{35}, e^{16} + e^{37}$           | 1/59(26, 28, 27, 56, 55, 54, 53, 82, 80)        | $\{\emptyset, 12389, 125789, 357\}$                                                                                   |
| 942:266a | $0, 0, 0, 0, 0, e^{12}, e^{13}, e^{23} + e^{16} + e^{45}, e^{26} + e^{37}$           | 6/19(1, 2, 2, 2, 2, 3, 3, 4, 5)                 | $\{123489, 123589, 134569, 1369, 234678, 235678, 3457, 37\}$                                                          |
| 942:266b | $0, 0, 0, 0, 0, -e^{12}, e^{13}, e^{16} + e^{23} + e^{45}, e^{37} + e^{26}$          | 6/19(1, 2, 2, 2, 2, 3, 3, 4, 5)                 | $\{123489, 123589, 134569, 1369, 234678, 235678, 3457, 37\}$                                                          |
| 942:267a | $0, 0, 0, 0, 0, e^{12}, e^{13}, e^{35} + e^{24} + e^{16}, e^{37} + e^{26}$           | 1/27(12, 13, 13, 24, 24, 25, 25, 37, 38)        | $\{\emptyset, 12389, 125789, 13569, 1679, 23678, 2568, 357\}$                                                         |
| 942:267b | $0, 0, 0, 0, 0, -e^{12}, e^{13}, e^{35} + e^{24} + e^{16}, e^{26} + e^{37}$          | 1/27(12, 13, 13, 24, 24, 25, 25, 37, 38)        | $\{\emptyset, 12389, 125789, 13569, 1679, 23678, 2568, 357\}$                                                         |
| 942:276  | $0, 0, 0, 0, 0, e^{12}, e^{13}, e^{17} + e^{26}, e^{37} + e^{45} + e^{16}$           | 16/67(2, 2, 2, 3, 3, 4, 4, 6, 6)                | $\{134689, 135689, 2456, 26\}$                                                                                        |
| 942:281  | $0, 0, 0, 0, 0, e^{12}, e^{13}, e^{26} + e^{15} + e^{34}, e^{37} + e^{14} + e^{25}$  | 17/37(1, 1, 1, 2, 2, 2, 2, 3, 3)                | $\{\emptyset, 12389\}$                                                                                                |
| 942:282  | $0, 0, 0, 0, 0, e^{12}, e^{13}, e^{23} + e^{16} + e^{45}, e^{14} + e^{25} + e^{37}$  | 1/8(2, 7, 4, 8, 3, 9, 6, 11, 10)                | $\{123489, 134569\}$                                                                                                  |
| 942:284a | $0, 0, 0, 0, 0, e^{12}, e^{13}, e^{24} + e^{35} + e^{16}, e^{23} + e^{45} + e^{17}$  | 23/67(1, 2, 2, 2, 2, 3, 3, 4, 4)                | $\{\emptyset, 13569, 167, 3579\}$                                                                                     |
| 942:284b | $0, 0, 0, 0, 0, e^{12}, e^{13}, e^{35} - e^{24} + e^{16}, e^{45} + e^{23} + e^{17}$  | 23/67(1, 2, 2, 2, 2, 3, 3, 4, 4)                | $\{\emptyset, 13569, 167, 3579\}$                                                                                     |
| 942:286  | $0, 0, 0, 0, 0, e^{12}, e^{13}, e^{35} + e^{24} + e^{16}, e^{45} + e^{26} + e^{17}$  | 59/445(3, 4, 5, 6, 5, 7, 8, 10, 11)             | $\{\emptyset, 13569\}$                                                                                                |
| 942:287  | $0, 0, 0, 0, 0, e^{12}, e^{13}, e^{14} + e^{26} + e^{35}, e^{16} + e^{37} + e^{45}$  | 11/95(5, 3, 4, 6, 7, 8, 9, 11, 13)              | $\{146789, 2456\}$                                                                                                    |
| 942:288a | $0, 0, 0, 0, 0, e^{12}, e^{13}, e^{16} + e^{24} + e^{35}, e^{37} + e^{26} + e^{45}$  | 41/217(2, 3, 3, 4, 4, 5, 5, 7, 8)               | $\{\emptyset, 125789, 13569, 23678\}$                                                                                 |
| 942:288b | $0, 0, 0, 0, 0, -e^{12}, e^{13}, e^{16} + e^{35} + e^{24}, e^{26} + e^{37} + e^{45}$ | 41/217(2, 3, 3, 4, 4, 5, 5, 7, 8)               | $\{\emptyset, 125789, 13569, 23678\}$                                                                                 |
| 942:291a | $0, 0, 0, 0, 0, e^{12}, e^{13}, e^{16} + e^{23} + e^{45}, e^{14} + e^{26} + e^{37}$  | 2/7(1, 2, 2, 4, 0, 3, 3, 4, 5)                  | $\{123489, 134569, 234678, 3457\}$                                                                                    |
| 942:291b | $0, 0, 0, 0, 0, -e^{12}, e^{13}, e^{45} + e^{23} + e^{16}, e^{37} + e^{14} + e^{26}$ | 2/7(1, 2, 2, 4, 0, 3, 3, 4, 5)                  | $\{123489, 134569, 234678, 3457\}$                                                                                    |
| 942:293a | $0, 0, 0, 0, 0, e^{12}, e^{13}, e^{16} + e^{25} + e^{34}, e^{37} + e^{14} + e^{26}$  | 17/37(1, 1, 1, 2, 2, 2, 2, 3, 3)                | $\{124789, 13469, 2468, 347\}$                                                                                        |
| 942:293b | $0, 0, 0, 0, 0, -e^{12}, e^{13}, e^{25} + e^{16} + e^{34}, e^{26} + e^{37} + e^{14}$ | 17/37(1, 1, 1, 2, 2, 2, 2, 3, 3)                | $\{124789, 13469, 2468, 347\}$                                                                                        |
| 942:294a | $0, 0, 0, 0, 0, e^{12}, e^{13}, e^{14} + e^{26} + e^{35}, e^{16} + e^{24} + e^{37}$  | 17/37(1, 1, 1, 2, 2, 2, 2, 3, 3)                | $\{\emptyset, 12389, 125789, 357\}$                                                                                   |
| 942:294b | $0, 0, 0, 0, 0, e^{12}, e^{13}, -e^{14} + e^{26} + e^{35}, e^{16} + e^{24} + e^{37}$ | 17/37(1, 1, 1, 2, 2, 2, 2, 3, 3)                | $\{\emptyset, 12389, 125789, 357\}$                                                                                   |
| 942:295  | $0, 0, 0, 0, 0, e^{12}, e^{13}, e^{15} + e^{34} + e^{26}, e^{16} + e^{24} + e^{37}$  | 17/37(1, 1, 1, 2, 2, 2, 2, 3, 3)                | $\{\emptyset, 12389\}$                                                                                                |
| 942:300  | $0, 0, 0, 0, 0, e^{12}, e^{13}, e^{45} + e^{23} + e^{16}, e^{17} + e^{26} + e^{34}$  | 7/38(2, 3, 4, 4, 3, 5, 6, 7, 8)                 | $\{123459, 134689\}$                                                                                                  |
| 942:311  | $0, 0, 0, 0, 0, e^{12}, e^{13}, e^{26} + e^{17} + e^{34}, e^{16} + e^{25} + e^{37}$  | 17/37(1, 1, 1, 2, 2, 2, 2, 3, 3)                | $\{\emptyset, 12389\}$                                                                                                |
| 942:316  | $0, 0, 0, 0, 0, e^{12}, e^{34}, e^{16}, e^{25} + e^{37}$                             | 2/21(4, 6, 4, 7, 9, 10, 11, 14, 15)             | $\{\emptyset, 123489, 123578, 124789, 1258, 134569, 1367, 145679, 16, 234689, 235678, 246789, 2568, 3459, 37, 4579\}$ |
| 942:319  | $0, 0, 0, 0, 0, e^{12}, e^{34}, e^{16} + e^{25}, e^{15} + e^{37}$                    | 1/123(54, 69, 40, 82, 108, 123, 122, 177, 162)  | $\{12378, 128, 1367, 16, 234689, 246789, 349, 479\}$                                                                  |
| 942:321  | $0, 0, 0, 0, 0, e^{12}, e^{34}, e^{35} + e^{16}, e^{25} + e^{37}$                    | 1/57(21, 32, 23, 37, 51, 53, 60, 74, 83)        | $\{123578, 124789, 1367, 145679, 235678, 246789, 37, 4579\}$                                                          |
| 942:322a | $0, 0, 0, 0, 0, e^{12}, e^{34}, e^{26} + e^{15}, e^{35} + e^{47}$                    | 1/5(3, 2, 3, 2, 4, 5, 5, 7, 7)                  | $\{\emptyset, 123489, 123789, 12478, 128, 134689, 136789, 14678, 168, 23469, 23679, 2467, 26, 349, 379, 47\}$         |
| 942:322b | $0, 0, 0, 0, 0, -e^{12}, e^{34}, e^{26} + e^{15}, e^{35} + e^{47}$                   | 1/5(3, 2, 3, 2, 4, 5, 5, 7, 7)                  | $\{\emptyset, 123489, 123789, 12478, 128, 134689, 136789, 14678, 168, 23469, 23679, 2467, 26, 349, 379, 47\}$         |
| 942:323a | $0, 0, 0, 0, 0, e^{12}, e^{34}, e^{35} + e^{16}, e^{47} + e^{25}$                    | 1/5(2, 3, 3, 2, 4, 5, 5, 7, 7)                  | $\{\emptyset, 123489, 123789, 124578, 1258, 134569, 135679, 1467, 16, 234689, 236789, 245678, 2568, 3459, 3579, 47\}$ |
| 942:323b | $0, 0, 0, 0, 0, -e^{12}, e^{34}, e^{16} + e^{35}, e^{47} + e^{25}$                   | 1/5(2, 3, 3, 2, 4, 5, 5, 7, 7)                  | $\{\emptyset, 123489, 123789, 124578, 1258, 134569, 135679, 1467, 16, 234689, 236789, 245678, 2568, 3459, 3579, 47\}$ |
| 942:328  | $0, 0, 0, 0, 0, e^{12}, e^{34}, e^{26} + e^{13}, e^{15} + e^{37}$                    | 2/17(6, 2, 4, 5, 7, 8, 9, 10, 13)               | $\{123489, 123578, 134689, 135678, 234569, 2367, 3459, 37\}$                                                          |
| 942:329  | $0, 0, 0, 0, 0, e^{12}, e^{34}, e^{16} + e^{23}, e^{15} + e^{37}$                    | 1/21(4, 17, 8, 12, 24, 21, 20, 25, 28)          | $\{1234589, 12378, 134569, 1367, 234689, 235678, 349, 357\}$                                                          |
| 942:330  | $0, 0, 0, 0, 0, e^{12}, e^{34}, e^{16}, e^{47} + e^{13} + e^{25}$                    | 2/17(4, 4, 7, 2, 7, 8, 9, 12, 11)               | $\{123489, 123789, 124578, 1258, 134569, 135679, 1467, 16\}$                                                          |

Table A.2 – Continued to next page

Table A.2 – Continued from previous page

| Name     | $g$                                                                                  | $N$                                                   | Signatures $S$                                                    |
|----------|--------------------------------------------------------------------------------------|-------------------------------------------------------|-------------------------------------------------------------------|
| 942:332  | $0, 0, 0, 0, 0, e^{12}, e^{34}, e^{13} + e^{26}, e^{47} + e^{15}$                    | $1/57(34, 20, 40, 21, 48, 54, 61, 74, 82)$            | $\{123489, 123789, 134689, 136789, 234569, 235679, 3459, 3579\}$  |
| 942:334  | $0, 0, 0, 0, 0, e^{12}, e^{34}, e^{13} + e^{26}, e^{47} + e^{35}$                    | $1/57(40, 17, 34, 24, 48, 57, 58, 74, 82)$            | $\{123489, 123789, 134689, 136789, 23469, 23679, 349, 379\}$      |
| 942:335  | $0, 0, 0, 0, 0, e^{12}, e^{34}, e^{26} + e^{13}, e^{37} + e^{45}$                    | $1/31(24, 7, 14, 17, 28, 31, 31, 38, 45)$             | $\{123489, 12378, 134689, 13678, 23469, 2367, 349, 37\}$          |
| 942:339  | $0, 0, 0, 0, 0, e^{12}, e^{34}, e^{16}, e^{26} + e^{15} + e^{37}$                    | $1/123(48, 63, 46, 82, 126, 111, 128, 159, 174)$      | $\{1234589, 1245789, 134569, 145679, 235678, 2568, 357, 5\}$      |
| 942:340  | $0, 0, 0, 0, 0, e^{12}, e^{34}, e^{16}, e^{47} + e^{26} + e^{35}$                    | $1/27(10, 15, 16, 12, 24, 25, 28, 35, 40)$            | $\{\emptyset, 123489, 123789, 13469, 13679, 24678, 268, 47\}$     |
| 942:341  | $0, 0, 0, 0, 0, e^{12}, e^{34}, e^{15} + e^{26}, e^{37} + e^{16}$                    | $1/27(13, 12, 10, 18, 24, 25, 28, 37, 38)$            | $\{\emptyset, 123489, 124789, 13678, 168, 23469, 24679, 37\}$     |
| 942:342  | $0, 0, 0, 0, 0, e^{12}, e^{34}, e^{35} + e^{16}, e^{37} + e^{26}$                    | $1/57(23, 29, 21, 39, 54, 52, 60, 75, 81)$            | $\{\emptyset, 123489, 1245789, 134569, 14679, 23678, 2568, 357\}$ |
| 942:343  | $0, 0, 0, 0, 0, e^{12}, e^{34}, e^{35} + e^{16}, e^{47} + e^{26}$                    | $1/18(8, 9, 10, 8, 15, 17, 18, 25, 26)$               | $\{\emptyset, 123489, 123789, 134569, 135679, 245678, 2568, 47\}$ |
| 942:345  | $0, 0, 0, 0, 0, e^{12}, e^{34}, e^{26} + e^{15}, e^{13} + e^{25} + e^{47}$           | $1/657(386, 282, 460, 193, 564, 668, 653, 950, 846)$  | $\{12478, 128, 134689, 136789\}$                                  |
| 942:346a | $0, 0, 0, 0, 0, e^{12}, e^{34}, e^{35} + e^{16}, e^{47} + e^{13} + e^{25}$           | $1/4(2, 2, 3, 1, 3, 4, 4, 6, 5)$                      | $\{123489, 123789, 124578, 1258, 134569, 135679, 1467, 16\}$      |
| 942:346b | $0, 0, 0, 0, 0, -e^{12}, e^{34}, e^{16} + e^{35}, e^{13} + e^{47} + e^{25}$          | $1/4(2, 2, 3, 1, 3, 4, 4, 6, 5)$                      | $\{123489, 123789, 124578, 1258, 134569, 135679, 1467, 16\}$      |
| 942:347  | $0, 0, 0, 0, 0, e^{12}, e^{34}, e^{16} + e^{35}, e^{15} + e^{47} + e^{23}$           | $2/41(8, 14, 12, 7, 18, 22, 19, 30, 26)$              | $\{234689, 236789, 245678, 2568\}$                                |
| 942:348  | $0, 0, 0, 0, 0, e^{12}, e^{34}, e^{16} + e^{35}, e^{14} + e^{25} + e^{37}$           | $2/109(26, 17, 13, 47, 56, 43, 60, 69, 73)$           | $\{123578, 124789, 1367, 145679\}$                                |
| 942:351  | $0, 0, 0, 0, 0, e^{12}, e^{34}, e^{35} + e^{16}, e^{26} + e^{37} + e^{15}$           | $1/211(89, 103, 75, 145, 206, 192, 220, 281, 295)$    | $\{1245789, 134569, 2568, 357\}$                                  |
| 942:352a | $0, 0, 0, 0, 0, e^{12}, e^{34}, e^{15} + e^{26}, e^{47} + e^{16} + e^{35}$           | $1/31(16, 13, 19, 13, 26, 29, 32, 42, 45)$            | $\{\emptyset, 123489, 123789, 14678, 168, 23469, 23679, 47\}$     |
| 942:352b | $0, 0, 0, 0, 0, -e^{12}, e^{34}, e^{26} + e^{15}, e^{16} + e^{47} + e^{35}$          | $1/31(16, 13, 19, 13, 26, 29, 32, 42, 45)$            | $\{\emptyset, 123489, 123789, 14678, 168, 23469, 23679, 47\}$     |
| 942:353  | $0, 0, 0, 0, 0, e^{12}, e^{34}, e^{16} + e^{35}, e^{26} + e^{15} + e^{47}$           | $16/747(23, 21, 25, 20, 42, 44, 45, 67, 65)$          | $\{134569, 135679, 245678, 2568\}$                                |
| 942:354  | $0, 0, 0, 0, 0, e^{12}, e^{34}, e^{16} + e^{35}, e^{45} + e^{26} + e^{37}$           | $1/681(259, 373, 297, 411, 594, 632, 708, 891, 1005)$ | $\{\emptyset, 123489, 14679, 23678\}$                             |
| 942:372  | $0, 0, 0, 0, 0, e^{12}, e^{34}, e^{13} + e^{26}, e^{15} + e^{23} + e^{47}$           | $1/46(23, 20, 40, 10, 37, 43, 50, 63, 60)$            | $\{123489, 123789, 234569, 235679\}$                              |
| 942:373  | $0, 0, 0, 0, 0, e^{12}, e^{34}, e^{13} + e^{26}, e^{14} + e^{25} + e^{37}$           | $1/121(96, 24, 48, 67, 139, 120, 115, 144, 163)$      | $\{234569, 2367, 349, 357\}$                                      |
| 942:374  | $0, 0, 0, 0, 0, e^{12}, e^{34}, e^{13} + e^{26}, e^{37} + e^{24} + e^{15}$           | $2/5(2, 0, 0, 3, 1, 2, 3, 2, 3)$                      | $\{123489, 123578, 234569, 2367\}$                                |
| 942:377  | $0, 0, 0, 0, 0, e^{12}, e^{34}, e^{26} + e^{13}, e^{25} + e^{37} + e^{16}$           | $1/13(8, 3, 6, 7, 16, 11, 13, 14, 19)$                | $\{1234589, 135678, 234569, 357\}$                                |
| 942:378  | $0, 0, 0, 0, 0, e^{12}, e^{34}, e^{13} + e^{26}, e^{47} + e^{16} + e^{25}$           | $1/279(147, 100, 200, 97, 294, 247, 297, 347, 394)$   | $\{1234589, 1235789, 234569, 235679\}$                            |
| 942:379  | $0, 0, 0, 0, 0, e^{12}, e^{34}, e^{13} + e^{26}, e^{47} + e^{16} + e^{35}$           | $1/69(41, 22, 44, 30, 60, 63, 74, 85, 104)$           | $\{123489, 123789, 23469, 23679\}$                                |
| 942:380  | $0, 0, 0, 0, 0, e^{12}, e^{34}, e^{26} + e^{13}, e^{16} + e^{37} + e^{45}$           | $1/91(59, 22, 44, 52, 88, 81, 96, 103, 140)$          | $\{123489, 13678, 23469, 37\}$                                    |
| 942:381  | $0, 0, 0, 0, 0, e^{12}, e^{34}, e^{15} + e^{26}, e^{16} + e^{23} + e^{47}$           | $1/91(37, 44, 74, 22, 88, 81, 96, 125, 118)$          | $\{123489, 123789, 23469, 23679\}$                                |
| 942:382  | $0, 0, 0, 0, 0, e^{12}, e^{34}, e^{16} + e^{35}, e^{13} + e^{26} + e^{47}$           | $1/14(8, 5, 10, 4, 11, 13, 14, 21, 18)$               | $\{123489, 123789, 134569, 135679\}$                              |
| 942:383  | $0, 0, 0, 0, 0, e^{12}, e^{34}, e^{35} + e^{16}, e^{37} + e^{26} + e^{14}$           | $5/133(12, 11, 6, 22, 29, 23, 28, 35, 34)$            | $\{1234589, 124789, 13469, 145679\}$                              |
| 942:384  | $0, 0, 0, 0, 0, e^{12}, e^{34}, e^{13} + e^{45} + e^{26}, e^{37} + e^{16}$           | $1/14(9, 4, 8, 6, 11, 13, 14, 17, 22)$                | $\{123489, 135678, 234569, 37\}$                                  |
| 942:385  | $0, 0, 0, 0, 0, e^{12}, e^{34}, e^{26} + e^{35} + e^{14}, e^{37} + e^{16}$           | $1/81(43, 30, 28, 60, 75, 73, 88, 103, 116)$          | $\{123489, 1245789, 234569, 24679\}$                              |
| 942:387  | $0, 0, 0, 0, 0, e^{12}, e^{34}, e^{16} + e^{37}, e^{15} + e^{47} + e^{26}$           | $1/81(37, 39, 37, 39, 78, 76, 76, 113, 115)$          | $\{\emptyset, 123489, 13679, 24678\}$                             |
| 942:397  | $0, 0, 0, 0, 0, e^{12}, e^{34}, e^{35} + e^{14} + e^{26}, e^{25} + e^{13} + e^{47}$  | $11/98(8, 2, 3, 4, 9, 10, 7, 12, 11)$                 | $\{134689, 145678\}$                                              |
| 942:398a | $0, 0, 0, 0, 0, e^{12}, e^{34}, e^{16} + e^{35} + e^{24}, e^{25} + e^{47} + e^{13}$  | $(0, 1, 1, 0, 0, 1, 1, 1, 1)$                         | $\{123489, 124578, 134569, 1467\}$                                |
| 942:398b | $0, 0, 0, 0, 0, -e^{12}, e^{34}, e^{16} + e^{35} + e^{24}, e^{25} + e^{13} + e^{47}$ | $(0, 1, 1, 0, 0, 1, 1, 1, 1)$                         | $\{123489, 124578, 134569, 1467\}$                                |
| 942:401  | $0, 0, 0, 0, 0, e^{12}, e^{34}, e^{45} + e^{23} + e^{16}, e^{37} + e^{15} + e^{26}$  | $32/287(3, 5, 6, 1, 10, 8, 7, 11, 13)$                | $\{134569, 235678\}$                                              |
| 942:402  | $0, 0, 0, 0, 0, e^{12}, e^{34}, e^{16} + e^{24} + e^{35}, e^{15} + e^{37} + e^{26}$  | $7/71(4, 5, 3, 8, 10, 9, 11, 13, 14)$                 | $\{1245789, 134569\}$                                             |
| 942:403  | $0, 0, 0, 0, 0, e^{12}, e^{34}, e^{13} + e^{45} + e^{26}, e^{35} + e^{47} + e^{16}$  | $91/1093(7, 4, 8, 5, 10, 11, 13, 15, 18)$             | $\{123489, 23679\}$                                               |
| 942:425a | $0, 0, 0, 0, 0, e^{12}, e^{34}, e^{25} + e^{37} + e^{16}, e^{26} + e^{15} + e^{47}$  | $8/17(1, 1, 1, 1, 2, 2, 2, 3, 3)$                     | $\{\emptyset, 123489, 13679, 24678\}$                             |
| 942:425b | $0, 0, 0, 0, 0, e^{12}, e^{34}, e^{37} - e^{16} + e^{25}, e^{47} + e^{15} + e^{26}$  | $8/17(1, 1, 1, 1, 2, 2, 2, 3, 3)$                     | $\{\emptyset, 123489, 13679, 24678\}$                             |
| 942:426a | $0, 0, 0, 0, 0, e^{12}, e^{34}, e^{37} + e^{26} + e^{15}, e^{47} + e^{16} + e^{35}$  | $8/17(1, 1, 1, 1, 2, 2, 2, 3, 3)$                     | $\{\emptyset, 123489, 14678, 23679\}$                             |
| 942:426b | $0, 0, 0, 0, 0, -e^{12}, e^{34}, e^{26} + e^{15} + e^{37}, e^{16} + e^{35} + e^{47}$ | $8/17(1, 1, 1, 1, 2, 2, 2, 3, 3)$                     | $\{\emptyset, 123489, 14678, 23679\}$                             |
| 942:430a | $0, 0, 0, 0, 0, e^{12}, e^{34}, e^{45} + e^{16} + e^{23}, e^{47} + e^{26} + e^{13}$  | $35/163(2, 2, 4, 1, 5, 4, 5, 6, 6)$                   | $\{1234589, 123789, 13469, 135679\}$                              |
| 942:430b | $0, 0, 0, 0, 0, e^{12}, e^{34}, e^{45} + e^{23} - e^{16}, e^{47} + e^{13} + e^{26}$  | $35/163(2, 2, 4, 1, 5, 4, 5, 6, 6)$                   | $\{1234589, 123789, 13469, 135679\}$                              |
| 942:431  | $0, 0, 0, 0, 0, e^{12}, e^{34}, e^{16} + e^{24} + e^{35}, e^{13} + e^{47} + e^{26}$  | $1/2(0, 1, 2, 0, -1, 1, 2, 1, 2)$                     | $\{123489, 134569\}$                                              |
| 942:433  | $0, 0, 0, 0, 0, e^{12}, e^{34}, e^{23} + e^{47} + e^{16}, e^{37} + e^{26} + e^{15}$  | $5/17(1, 2, 2, 1, 4, 3, 3, 4, 5)$                     | $\{1234589, 235678\}$                                             |

Table A.2 – Continued to next page

Table A.2 – Continued from previous page

| Name    | $g$                                                                | $N$                                       | Signatures $S$                                                                                                   |
|---------|--------------------------------------------------------------------|-------------------------------------------|------------------------------------------------------------------------------------------------------------------|
| 941:11  | $0, 0, 0, 0, 0, e^{12}, e^{34}, e^{45} + e^{13}, e^{16}$           | 1/11(4, 7, 9, 5, 8, 11, 14, 13, 15)       | {123489, 1235789, 124579, 129, 13468, 135678, 14567, 16, 234569, 23679, 246789, 25689, 345, 37, 478, 58}         |
| 941:12  | $0, 0, 0, 0, 0, e^{12}, e^{34}, e^{13} + e^{45}, e^{26}$           | 1/39(24, 14, 27, 21, 30, 38, 48, 51, 52)  | {0, 123459, 12379, 124789, 12589, 134569, 13679, 146789, 15689, 23468, 235678, 24567, 26, 348, 3578, 457}        |
| 941:13  | $0, 0, 0, 0, 0, e^{12}, e^{34}, e^{35}, e^{16} + e^{45}$           | 1/39(14, 26, 21, 27, 27, 40, 48, 48, 54)  | {0, 123489, 123579, 12479, 12589, 13456, 13678, 145678, 16, 234689, 235679, 24679, 25689, 345, 378, 4578}        |
| 941:23  | $0, 0, 0, 0, 0, e^{12}, e^{13}, e^{34}, e^{16} + e^{35}$           | 1/41(16, 27, 24, 29, 35, 43, 40, 53, 59)  | {123479, 123789, 124589, 1259, 134567, 135678, 1468, 16, 23469, 23689, 2456789, 25679, 345, 358, 478, 7}         |
| 941:24  | $0, 0, 0, 0, 0, e^{12}, e^{13}, e^{34}, e^{26} + e^{35}$           | 1/27(16, 11, 14, 20, 24, 27, 30, 34, 38)  | {0, 12349, 12389, 1245789, 12579, 13469, 13689, 1456789, 15679, 234567, 235678, 2468, 26, 3457, 3578, 48}        |
| 941:25  | $0, 0, 0, 0, 0, e^{12}, e^{13}, e^{34}, e^{16} + e^{45}$           | 1/19(7, 13, 13, 11, 16, 20, 20, 24, 27)   | {0, 12349, 123589, 124789, 12579, 13456, 1368, 145678, 167, 234679, 2356789, 24689, 2569, 3457, 378, 458}        |
| 941:26  | $0, 0, 0, 0, 0, e^{12}, e^{13}, e^{34}, e^{45} + e^{26}$           | 1/18(10, 8, 11, 11, 15, 18, 21, 22, 26)   | {0, 12349, 123589, 124789, 12579, 13469, 135689, 146789, 15679, 234567, 23678, 24568, 26, 3457, 378, 458}        |
| 941:28  | $0, 0, 0, 0, 0, e^{12}, e^{13}, e^{35} + e^{14}, e^{26}$           | 1/24(12, 10, 15, 21, 18, 22, 27, 33, 32)  | {0, 123459, 12389, 12479, 125789, 134569, 13689, 14679, 156789, 234678, 23567, 24568, 26, 3478, 357, 458}        |
| 941:29  | $0, 0, 0, 0, 0, e^{12}, e^{13}, e^{45} + e^{23}, e^{16}$           | 1/27(9, 17, 21, 19, 19, 26, 30, 38, 35)   | {0, 123459, 1239, 124789, 125789, 13468, 13568, 14567, 167, 2345679, 23679, 24689, 25689, 3478, 3578, 45}        |
| 941:30  | $0, 0, 0, 0, 0, e^{12}, e^{13}, e^{24} + e^{35}, e^{16}$           | 1/19(7, 11, 13, 16, 14, 18, 20, 27, 25)   | {0, 123459, 12389, 12479, 125789, 13468, 1356, 145678, 167, 2345679, 236789, 2469, 25689, 3478, 357, 458}        |
| 941:31  | $0, 0, 0, 0, 0, e^{12}, e^{13}, e^{45} + e^{23}, e^{26}$           | 1/11(5, 5, 9, 7, 7, 10, 14, 14, 15)       | {123489, 123589, 124579, 1279, 134569, 1369, 146789, 156789, 234678, 235678, 2456, 26, 3457, 37, 48, 58}         |
| 941:32  | $0, 0, 0, 0, 0, e^{12}, e^{13}, e^{35} + e^{24}, e^{26}$           | 1/19(11, 7, 11, 18, 14, 18, 22, 25, 25)   | {0, 123459, 12389, 12479, 125789, 134689, 13569, 1456789, 1679, 234567, 23678, 246, 2568, 3478, 357, 458}        |
| 941:33  | $0, 0, 0, 0, 0, e^{12}, e^{13}, e^{45}, e^{34} + e^{16}$           | 1/27(9, 19, 21, 16, 19, 28, 30, 35, 37)   | {0, 123589, 1239, 124579, 124789, 13456, 13468, 15678, 167, 2356789, 23679, 24569, 24689, 3457, 3478, 58}        |
| 941:34  | $0, 0, 0, 0, 0, e^{12}, e^{13}, e^{45}, e^{34} + e^{26}$           | 2/47(12, 10, 17, 15, 16, 22, 29, 31, 32)  | {0, 123589, 1239, 124579, 124789, 135689, 1369, 145679, 146789, 234567, 234678, 2568, 26, 3457, 3478, 58}        |
| 941:35  | $0, 0, 0, 0, 0, e^{12}, e^{34}, e^{13} + e^{25}, e^{16}$           | 1/11(5, 5, 8, 7, 8, 10, 15, 13, 15)       | {123489, 123789, 124579, 1259, 134568, 135678, 1467, 16, 234569, 235679, 246789, 2689, 34, 37, 4578, 58}         |
| 941:36  | $0, 0, 0, 0, 0, e^{12}, e^{34}, e^{15} + e^{23}, e^{16}$           | 1/27(9, 17, 16, 19, 24, 26, 35, 33, 35)   | {0, 123459, 123579, 124789, 1289, 13468, 13678, 14567, 156, 23469, 23679, 2456789, 25689, 3458, 3578, 47}        |
| 941:37  | $0, 0, 0, 0, 0, e^{12}, e^{34}, e^{35}, e^{13} + e^{26}$           | 1/11(8, 3, 6, 8, 8, 11, 14, 14, 14)       | {123459, 123489, 123579, 123789, 134569, 134689, 135679, 136789, 23456, 23468, 23567, 23678, 345, 348, 357, 378} |
| 941:38  | $0, 0, 0, 0, 0, e^{12}, e^{34}, e^{35}, e^{26} + e^{14}$           | 1/47(30, 17, 24, 34, 35, 47, 58, 59, 64)  | {0, 123579, 123789, 12589, 129, 135679, 136789, 15689, 169, 23567, 23678, 2568, 26, 357, 378, 58}                |
| 941:39  | $0, 0, 0, 0, 0, e^{12}, e^{34}, e^{45} + e^{13}, e^{16} + e^{35}$  | 1/71(28, 45, 54, 35, 47, 73, 89, 82, 101) | {123489, 124579, 135678, 16, 23679, 25689, 345, 478}                                                             |
| 941:40  | $0, 0, 0, 0, 0, e^{12}, e^{34}, e^{45} + e^{13}, e^{26} + e^{35}$  | 1/32(20, 12, 21, 18, 23, 32, 39, 41, 44)  | {0, 12379, 12589, 13679, 15689, 235678, 26, 3578}                                                                |
| 941:41a | $0, 0, 0, 0, 0, e^{12}, e^{35} + e^{14}, e^{45} + e^{13}, e^{16}$  | 1/5(2, 3, 4, 4, 2, 5, 6, 6, 7)            | {1234789, 123589, 124579, 129, 134678, 13568, 14567, 16, 234569, 23679, 24689, 256789, 345, 37, 48, 578}         |
| 941:41b | $0, 0, 0, 0, 0, e^{12}, -e^{14} + e^{35}, e^{13} + e^{45}, e^{16}$ | 1/5(2, 3, 4, 4, 2, 5, 6, 6, 7)            | {1234789, 123589, 124579, 129, 134678, 13568, 14567, 16, 234569, 23679, 24689, 256789, 345, 37, 48, 578}         |
| 941:42a | $0, 0, 0, 0, 0, e^{12}, e^{14} + e^{35}, e^{13} + e^{45}, e^{26}$  | 1/21(12, 8, 15, 15, 12, 20, 27, 27, 28)   | {0, 123459, 12379, 12489, 125789, 134569, 13679, 14689, 156789, 234678, 23568, 24567, 26, 3478, 358, 457}        |
| 941:42b | $0, 0, 0, 0, 0, e^{12}, e^{35} - e^{14}, e^{13} + e^{45}, e^{26}$  | 1/21(12, 8, 15, 15, 12, 20, 27, 27, 28)   | {0, 123459, 12379, 12489, 125789, 134569, 13679, 14689, 156789, 234678, 23568, 24567, 26, 3478, 358, 457}        |
| 941:43  | $0, 0, 0, 0, 0, e^{12}, e^{35} + e^{14}, e^{45} + e^{23}, e^{16}$  | 1/59(22, 36, 41, 48, 29, 58, 70, 77, 80)  | {134678, 13568, 14567, 16, 234569, 23679, 24689, 256789}                                                         |

Table A.2 – Continued to next page

Table A.2 – Continued from previous page

| Name    | $g$                                                                        | $N$                                                  | Signatures $S$                                                                                                        |
|---------|----------------------------------------------------------------------------|------------------------------------------------------|-----------------------------------------------------------------------------------------------------------------------|
| 941:47  | $0, 0, 0, 0, 0, e^{12}, e^{13}, e^{23}, e^{45} + e^{16}$                   | $1/68(31, 38, 45, 50, 50, 69, 76, 83, 100)$          | $\{\emptyset, 12349, 12359, 124789, 125789, 134568, 1368, 14567, 167, 234679, 235679, 24689, 25689, 34578, 378, 45\}$ |
| 941:48  | $0, 0, 0, 0, 0, e^{12}, e^{13}, e^{14}, e^{16} + e^{35}$                   | $1/23(8, 17, 16, 19, 17, 25, 24, 27, 33)$            | $\{\emptyset, 12349, 12389, 124579, 125789, 13456, 13568, 1467, 1678, 2346789, 23679, 245689, 2569, 34578, 357, 48\}$ |
| 941:49  | $0, 0, 0, 0, 0, e^{12}, e^{13}, e^{14}, e^{26} + e^{35}$                   | $1/68(30, 35, 46, 53, 54, 65, 76, 83, 100)$          | $\{\emptyset, 12349, 12389, 124579, 125789, 13469, 13689, 145679, 156789, 2345678, 23567, 2468, 26, 34578, 357, 48\}$ |
| 941:50  | $0, 0, 0, 0, 0, e^{12}, e^{13}, e^{24}, e^{16} + e^{35}$                   | $1/68(31, 36, 45, 50, 53, 67, 76, 86, 98)$           | $\{\emptyset, 12349, 12389, 124579, 125789, 134568, 1356, 14678, 167, 234679, 236789, 24569, 25689, 34578, 357, 48\}$ |
| 941:51  | $0, 0, 0, 0, 0, e^{12}, e^{13}, e^{24}, e^{35} + e^{26}$                   | $1/5(3, 2, 3, 4, 4, 5, 6, 6, 7)$                     | $\{\emptyset, 12349, 12389, 124579, 125789, 134689, 1369, 1456789, 15679, 234567, 235678, 246, 268, 34578, 357, 48\}$ |
| 941:52  | $0, 0, 0, 0, 0, e^{12}, e^{13}, e^{34}, e^{26} + e^{15}$                   | $1/27(14, 12, 16, 19, 24, 26, 30, 35, 38)$           | $\{\emptyset, 12349, 12389, 124789, 1279, 13469, 13689, 146789, 1679, 23467, 23678, 2468, 26, 347, 378, 48\}$         |
| 941:53  | $0, 0, 0, 0, 0, e^{12}, e^{13}, e^{34}, e^{25} + e^{16}$                   | $1/19(8, 11, 12, 13, 16, 19, 20, 25, 27)$            | $\{\emptyset, 12349, 12389, 124789, 1279, 1346, 1368, 14678, 167, 234679, 236789, 24689, 269, 347, 378, 48\}$         |
| 941:54  | $0, 0, 0, 0, 0, e^{12}, e^{13}, e^{25} + e^{14}, e^{16}$                   | $1/23(8, 13, 19, 22, 17, 21, 27, 30, 29)$            | $\{\emptyset, 123459, 12389, 124579, 12789, 1346, 13568, 1467, 15678, 2346789, 235679, 24689, 2569, 34578, 37, 458\}$ |
| 941:55  | $0, 0, 0, 0, 0, e^{12}, e^{13}, e^{25} + e^{14}, e^{26}$                   | $1/31(14, 13, 24, 26, 27, 27, 38, 40, 40)$           | $\{\emptyset, 123459, 12389, 124579, 12789, 13469, 135689, 14679, 156789, 234678, 23567, 2468, 256, 34578, 37, 458\}$ |
| 941:57  | $0, 0, 0, 0, 0, e^{12}, e^{13}, e^{45}, e^{26} + e^{14}$                   | $1/11(6, 4, 8, 8, 7, 10, 14, 15, 14)$                | $\{123459, 123489, 124579, 124789, 134569, 134689, 145679, 146789, 234567, 234678, 2456, 2468, 3457, 3478, 45, 48\}$  |
| 941:58  | $0, 0, 0, 0, 0, e^{12}, e^{13}, e^{45}, e^{16} + e^{24}$                   | $1/19(6, 13, 16, 12, 13, 19, 22, 25, 25)$            | $\{\emptyset, 123589, 1239, 125789, 1279, 13568, 136, 15678, 167, 2356789, 23679, 25689, 269, 3578, 37, 58\}$         |
| 941:63  | $0, 0, 0, 0, 0, e^{12}, e^{34}, e^{24} + e^{13}, e^{16} + e^{35}$          | $1/17(8, 9, 11, 10, 14, 17, 21, 19, 25)$             | $\{123789, 124579, 134568, 16, 23469, 25689, 357, 478\}$                                                              |
| 941:64  | $0, 0, 0, 0, 0, e^{12}, e^{34}, e^{14} + e^{23}, e^{16} + e^{35}$          | $1/227(91, 137, 119, 165, 200, 228, 284, 256, 319)$  | $\{\emptyset, 12349, 12589, 135678, 1467, 23679, 2456789, 3458\}$                                                     |
| 941:65  | $0, 0, 0, 0, 0, e^{12}, e^{13}, e^{14} + e^{35}, e^{34} + e^{16}$          | $1/40(16, 26, 23, 35, 28, 42, 39, 51, 58)$           | $\{123579, 124589, 134678, 16, 23689, 24679, 345, 578\}$                                                              |
| 941:66  | $0, 0, 0, 0, 0, e^{12}, e^{13}, e^{35} + e^{14}, e^{26} + e^{34}$          | $1/144(76, 62, 83, 117, 110, 138, 159, 193, 200)$    | $\{\emptyset, 12389, 12479, 13689, 14679, 234678, 26, 3478\}$                                                         |
| 941:67  | $0, 0, 0, 0, 0, e^{12}, e^{13}, e^{45} + e^{23}, e^{34} + e^{16}$          | $1/11(4, 7, 8, 7, 8, 11, 12, 15, 15)$                | $\{\emptyset, 1239, 124789, 13468, 167, 23679, 24689, 3478\}$                                                         |
| 941:68  | $0, 0, 0, 0, 0, e^{12}, e^{13}, e^{24} + e^{35}, e^{16} + e^{34}$          | $1/227(91, 135, 141, 176, 170, 226, 232, 311, 317)$  | $\{\emptyset, 12389, 12479, 13468, 167, 236789, 2469, 3478\}$                                                         |
| 941:69  | $0, 0, 0, 0, 0, e^{12}, e^{13}, e^{23} + e^{45}, e^{34} + e^{26}$          | $2/43(10, 10, 17, 13, 14, 20, 27, 27, 30)$           | $\{123589, 124579, 1369, 146789, 234678, 26, 3457, 58\}$                                                              |
| 941:70  | $0, 0, 0, 0, 0, e^{12}, e^{13}, e^{35} + e^{24}, e^{26} + e^{34}$          | $1/227(135, 91, 119, 198, 170, 226, 254, 289, 317)$  | $\{\emptyset, 12389, 12479, 13569, 1456789, 234567, 2568, 3478\}$                                                     |
| 941:71  | $0, 0, 0, 0, 0, e^{12}, e^{24} + e^{13}, e^{35}, e^{16} + e^{34}$          | $2/43(10, 10, 15, 15, 14, 20, 25, 29, 30)$           | $\{123579, 123789, 124589, 1249, 134567, 134678, 1568, 16\}$                                                          |
| 941:72  | $0, 0, 0, 0, 0, e^{12}, e^{23} + e^{14}, e^{35}, e^{34} + e^{16}$          | $1/11(4, 7, 6, 9, 8, 11, 13, 14, 15)$                | $\{\emptyset, 23569, 23689, 2456789, 24679, 3457, 3478, 58\}$                                                         |
| 941:73  | $0, 0, 0, 0, 0, e^{12}, e^{14} + e^{23}, e^{13} + e^{45}, e^{16}$          | $1/10(5, 4, 8, 7, 6, 9, 12, 13, 14)$                 | $\{123589, 124579, 134678, 16, 234569, 256789, 37, 48\}$                                                              |
| 941:74  | $0, 0, 0, 0, 0, e^{12}, e^{24} + e^{13}, e^{34} + e^{15}, e^{16}$          | $7/37(2, 3, 4, 3, 5, 5, 6, 7, 7)$                    | $\{123789, 12489, 134567, 156, 23469, 2679, 358, 4578\}$                                                              |
| 941:75  | $0, 0, 0, 0, 0, e^{12}, e^{23} + e^{14}, e^{13} + e^{45}, e^{26}$          | $1/144(80, 54, 117, 91, 106, 134, 171, 197, 188)$    | $\{\emptyset, 123459, 125789, 13679, 14689, 23568, 24567, 3478\}$                                                     |
| 941:76  | $0, 0, 0, 0, 0, e^{12}, e^{24} + e^{13}, e^{34} + e^{15}, e^{26}$          | $1/83(42, 34, 53, 61, 72, 76, 95, 114, 110)$         | $\{\emptyset, 123459, 12579, 13689, 146789, 235678, 24568, 347\}$                                                     |
| 941:77  | $0, 0, 0, 0, 0, e^{12}, e^{34}, e^{35} + e^{14}, e^{26} + e^{13}$          | $1/71(48, 21, 42, 47, 53, 69, 89, 95, 90)$           | $\{123459, 123789, 134569, 136789, 23468, 23567, 348, 357\}$                                                          |
| 941:78  | $0, 0, 0, 0, 0, e^{12}, e^{34}, e^{13} + e^{45}, e^{16} + e^{23}$          | $1/43(17, 26, 34, 20, 31, 43, 54, 51, 60)$           | $\{124579, 129, 14567, 16, 246789, 25689, 478, 58\}$                                                                  |
| 941:79  | $0, 0, 0, 0, 0, e^{12}, e^{34}, e^{35} + e^{14}, e^{23} + e^{16}$          | $1/8(2, 6, 4, 7, 5, 8, 11, 9, 10)$                   | $\{123489, 123579, 13468, 13567, 234569, 236789, 345, 378\}$                                                          |
| 941:80  | $0, 0, 0, 0, 0, e^{12}, e^{13}, e^{35} + e^{14}, e^{45} + e^{16}$          | $1/37(14, 25, 25, 32, 21, 39, 39, 46, 53)$           | $\{123489, 12359, 145678, 167, 2469, 25689, 3457, 378\}$                                                              |
| 941:81  | $0, 0, 0, 0, 0, e^{12}, e^{13}, e^{14} + e^{35}, e^{45} + e^{26}$          | $1/297(152, 136, 190, 231, 193, 288, 342, 383, 424)$ | $\{\emptyset, 12479, 125789, 14679, 156789, 24568, 26, 458\}$                                                         |
| 941:82  | $0, 0, 0, 0, 0, e^{12}, e^{13}, e^{35} + e^{24}, e^{16} + e^{45}$          | $1/23(9, 14, 16, 17, 15, 23, 25, 31, 32)$            | $\{\emptyset, 12479, 125789, 145678, 167, 2469, 25689, 458\}$                                                         |
| 941:83  | $0, 0, 0, 0, 0, e^{12}, e^{13}, e^{35} + e^{24}, e^{45} + e^{26}$          | $1/257(144, 112, 158, 207, 161, 256, 302, 319, 368)$ | $\{\emptyset, 12479, 125789, 134689, 13569, 234567, 23678, 458\}$                                                     |
| 941:85  | $0, 0, 0, 0, 0, e^{12}, e^{34}, e^{15} + e^{23}, e^{16} + e^{45}$          | $1/34(14, 20, 21, 21, 27, 34, 42, 41, 48)$           | $\{\emptyset, 123579, 124789, 13678, 14567, 23469, 25689, 3458\}$                                                     |
| 941:86  | $0, 0, 0, 0, 0, e^{12}, e^{34}, e^{35}, e^{45} + e^{26} + e^{13}$          | $1/71(52, 21, 42, 47, 47, 73, 89, 89, 94)$           | $\{123489, 123579, 134689, 135679, 23456, 23678, 345, 378\}$                                                          |
| 941:87  | $0, 0, 0, 0, 0, e^{12}, e^{34}, e^{13} + e^{45}, e^{15} + e^{26}$          | $1/293(176, 110, 203, 159, 220, 286, 362, 379, 396)$ | $\{\emptyset, 12379, 124789, 13679, 146789, 23468, 26, 348\}$                                                         |
| 941:89a | $0, 0, 0, 0, 0, e^{12}, e^{14} + e^{35}, e^{13} + e^{45}, e^{34} + e^{16}$ | $1/64(28, 38, 47, 47, 28, 66, 75, 75, 94)$           | $\{123589, 124579, 134678, 16, 23679, 24689, 345, 578\}$                                                              |

Table A.2 – Continued to next page

Table A.2 – Continued from previous page

| Name     | $g$                                                                        | $N$                                                  | Signatures $S$                                                                                                |
|----------|----------------------------------------------------------------------------|------------------------------------------------------|---------------------------------------------------------------------------------------------------------------|
| 941:89b  | $0, 0, 0, 0, 0, e^{12}, e^{35} - e^{14}, e^{45} + e^{13}, e^{34} + e^{16}$ | $1/64(28, 38, 47, 47, 28, 66, 75, 75, 94)$           | $\{123589, 124579, 134678, 16, 23679, 24689, 345, 578\}$                                                      |
| 941:90a  | $0, 0, 0, 0, 0, e^{12}, e^{14} + e^{35}, e^{13} + e^{45}, e^{26} + e^{34}$ | $4/41(6, 4, 7, 7, 6, 10, 13, 13, 14)$                | $\{\emptyset, 12379, 12489, 13679, 14689, 234678, 26, 3478\}$                                                 |
| 941:90b  | $0, 0, 0, 0, 0, e^{12}, e^{35} - e^{14}, e^{45} + e^{13}, e^{26} + e^{34}$ | $4/41(6, 4, 7, 7, 6, 10, 13, 13, 14)$                | $\{\emptyset, 12379, 12489, 13679, 14689, 234678, 26, 3478\}$                                                 |
| 941:91   | $0, 0, 0, 0, 0, e^{12}, e^{35} + e^{14}, e^{45} + e^{23}, e^{16} + e^{34}$ | $1/232(92, 144, 151, 177, 118, 236, 269, 295, 328)$  | $\{134678, 16, 23679, 24689\}$                                                                                |
| 941:92   | $0, 0, 0, 0, 0, e^{12}, e^{13}, e^{14}, e^{15} + e^{26}$                   | $1/31(12, 15, 25, 25, 30, 27, 37, 37, 42)$           | $\{\emptyset, 12349, 12389, 12479, 12789, 13469, 13689, 14679, 16789, 234678, 2367, 2468, 26, 3478, 37, 48\}$ |
| 941:93   | $0, 0, 0, 0, 0, e^{12}, e^{13}, e^{14}, e^{16} + e^{25}$                   | $1/16(6, 10, 13, 13, 12, 16, 19, 19, 22)$            | $\{\emptyset, 12349, 12389, 12479, 12789, 1346, 1368, 1467, 1678, 2346789, 23679, 24689, 269, 3478, 37, 48\}$ |
| 941:94   | $0, 0, 0, 0, 0, e^{12}, e^{13}, e^{24}, e^{26} + e^{15}$                   | $1/37(18, 16, 28, 29, 32, 34, 46, 45, 50)$           | $\{\emptyset, 12349, 12389, 12479, 12789, 134689, 1369, 146789, 1679, 23467, 23678, 246, 268, 3478, 37, 48\}$ |
| 941:96   | $0, 0, 0, 0, 0, e^{12}, e^{13}, e^{14} + e^{23}, e^{35} + e^{16}$          | $3/38(5, 8, 8, 11, 10, 13, 13, 16, 18)$              | $\{\emptyset, 12349, 125789, 13568, 1467, 23679, 245689, 34578\}$                                             |
| 941:97   | $0, 0, 0, 0, 0, e^{12}, e^{13}, e^{14} + e^{23}, e^{26} + e^{35}$          | $1/67(29, 35, 46, 52, 53, 64, 75, 81, 99)$           | $\{12389, 124579, 13469, 156789, 2345678, 26, 357, 48\}$                                                      |
| 941:98   | $0, 0, 0, 0, 0, e^{12}, e^{13}, e^{23} + e^{14}, e^{45} + e^{16}$          | $1/67(31, 37, 44, 50, 49, 68, 75, 81, 99)$           | $\{12359, 124789, 134568, 167, 234679, 25689, 378, 45\}$                                                      |
| 941:99   | $0, 0, 0, 0, 0, e^{12}, e^{13}, e^{14} + e^{23}, e^{26} + e^{45}$          | $1/44(22, 21, 31, 30, 34, 43, 53, 52, 64)$           | $\{\emptyset, 12349, 125789, 135689, 14679, 2367, 24568, 34578\}$                                             |
| 941:100  | $0, 0, 0, 0, 0, e^{12}, e^{13}, e^{34}, e^{26} + e^{35} + e^{14}$          | $1/26(16, 10, 13, 20, 23, 26, 29, 33, 36)$           | $\{12349, 1245789, 13469, 1456789, 234567, 2468, 3457, 48\}$                                                  |
| 941:101  | $0, 0, 0, 0, 0, e^{12}, e^{13}, e^{34}, e^{16} + e^{23} + e^{45}$          | $1/37(13, 26, 26, 21, 31, 39, 39, 47, 52)$           | $\{12349, 123589, 13456, 1368, 234679, 2356789, 3457, 378\}$                                                  |
| 941:102  | $0, 0, 0, 0, 0, e^{12}, e^{13}, e^{34}, e^{35} + e^{16} + e^{24}$          | $1/19(7, 13, 11, 14, 16, 20, 18, 25, 27)$            | $\{123479, 124589, 134567, 1468, 23469, 2456789, 345, 478\}$                                                  |
| 941:103  | $0, 0, 0, 0, 0, e^{12}, e^{34}, e^{24} + e^{13}, e^{26} + e^{15}$          | $1/227(119, 100, 137, 156, 200, 219, 293, 256, 319)$ | $\{\emptyset, 12349, 1289, 13679, 146789, 23678, 2467, 348\}$                                                 |
| 941:105  | $0, 0, 0, 0, 0, e^{12}, e^{13}, e^{35} + e^{24}, e^{23} + e^{16}$          | $1/37(13, 22, 26, 31, 27, 35, 39, 53, 48)$           | $\{123459, 12389, 13468, 1356, 2345679, 236789, 3478, 357\}$                                                  |
| 941:106  | $0, 0, 0, 0, 0, e^{12}, e^{13}, e^{25} + e^{14}, e^{16} + e^{34}$          | $1/67(31, 35, 44, 53, 49, 66, 75, 84, 97)$           | $\{12359, 124789, 134568, 167, 236789, 24569, 347, 58\}$                                                      |
| 941:107  | $0, 0, 0, 0, 0, e^{12}, e^{13}, e^{24} + e^{15}, e^{16} + e^{34}$          | $1/29(11, 18, 21, 19, 26, 29, 32, 37, 40)$           | $\{\emptyset, 12389, 124579, 13468, 1567, 2356789, 2469, 34578\}$                                             |
| 941:108  | $0, 0, 0, 0, 0, e^{12}, e^{13}, e^{25} + e^{14}, e^{26} + e^{34}$          | $1/49(26, 21, 32, 36, 41, 47, 58, 62, 68)$           | $\{\emptyset, 12389, 124579, 135689, 14679, 234678, 256, 34578\}$                                             |
| 941:109  | $0, 0, 0, 0, 0, e^{12}, e^{13}, e^{15} + e^{24}, e^{26} + e^{34}$          | $1/59(27, 29, 40, 45, 47, 56, 67, 74, 85)$           | $\{\emptyset, 12389, 124579, 13569, 146789, 23467, 2568, 34578\}$                                             |
| 941:110  | $0, 0, 0, 0, 0, e^{12}, e^{13}, e^{34} + e^{15}, e^{14} + e^{26}$          | $1/23(12, 9, 14, 18, 20, 21, 26, 32, 30)$            | $\{123459, 124789, 134569, 146789, 23467, 24568, 347, 458\}$                                                  |
| 941:111  | $0, 0, 0, 0, 0, e^{12}, e^{13}, e^{35} + e^{14}, e^{24} + e^{16}$          | $1/37(16, 21, 23, 32, 25, 37, 39, 48, 53)$           | $\{12359, 1279, 1356, 167, 236789, 25689, 378, 58\}$                                                          |
| 941:113  | $0, 0, 0, 0, 0, e^{12}, e^{13}, e^{23} + e^{45}, e^{26} + e^{14}$          | $1/8(4, 3, 7, 6, 4, 7, 11, 10, 10)$                  | $\{123489, 124579, 134569, 146789, 234678, 2456, 3457, 48\}$                                                  |
| 941:114  | $0, 0, 0, 0, 0, e^{12}, e^{13}, e^{35} + e^{24}, e^{14} + e^{26}$          | $1/227(119, 99, 135, 198, 162, 218, 254, 297, 317)$  | $\{\emptyset, 12389, 125789, 13569, 1679, 23678, 2568, 357\}$                                                 |
| 941:116  | $0, 0, 0, 0, 0, e^{12}, e^{13}, e^{45} + e^{23}, e^{16} + e^{24}$          | $1/227(78, 141, 176, 156, 161, 219, 254, 317, 297)$  | $\{\emptyset, 1239, 125789, 13568, 167, 23679, 25689, 3578\}$                                                 |
| 941:118  | $0, 0, 0, 0, 0, e^{12}, e^{23} + e^{14}, e^{13} + e^{25}, e^{16}$          | $1/63(26, 29, 52, 55, 49, 55, 81, 78, 81)$           | $\{\emptyset, 123459, 12789, 1367, 14568, 23689, 245679, 34578\}$                                             |
| 941:119  | $0, 0, 0, 0, 0, e^{12}, e^{34}, e^{15} + e^{23}, e^{13} + e^{26}$          | $1/10(5, 4, 8, 6, 7, 9, 14, 12, 13)$                 | $\{123489, 123789, 134569, 135679, 234568, 235678, 34, 37\}$                                                  |
| 941:121  | $0, 0, 0, 0, 0, e^{12}, e^{24} + e^{13}, e^{15}, e^{26} + e^{34}$          | $1/21(10, 10, 15, 15, 16, 20, 25, 26, 30)$           | $\{\emptyset, 13569, 13689, 145679, 146789, 34578, 347, 58\}$                                                 |
| 941:122  | $0, 0, 0, 0, 0, e^{12}, e^{34}, e^{13} + e^{25}, e^{14} + e^{26}$          | $1/227(141, 78, 137, 156, 200, 219, 293, 278, 297)$  | $\{\emptyset, 123579, 1289, 13679, 15689, 23678, 256, 3578\}$                                                 |
| 941:123  | $0, 0, 0, 0, 0, e^{12}, e^{34}, e^{23} + e^{15}, e^{26} + e^{14}$          | $1/8(4, 3, 6, 6, 5, 7, 12, 9, 10)$                   | $\{123489, 124579, 134569, 146789, 234568, 2467, 34, 4578\}$                                                  |
| 941:124  | $0, 0, 0, 0, 0, e^{12}, e^{13} + e^{24}, e^{35}, e^{26} + e^{14}$          | $1/144(83, 57, 88, 114, 100, 140, 171, 188, 197)$    | $\{\emptyset, 125789, 1279, 13569, 13689, 23567, 23678, 58\}$                                                 |
| 941:125  | $0, 0, 0, 0, 0, e^{12}, e^{13}, e^{45}, e^{14} + e^{26} + e^{35}$          | $2/43(12, 8, 15, 16, 13, 20, 27, 29, 28)$            | $\{123489, 124579, 134689, 145679, 234567, 2468, 3457, 48\}$                                                  |
| 941:126  | $0, 0, 0, 0, 0, e^{12}, e^{13}, e^{45}, e^{16} + e^{24} + e^{35}$          | $1/227(78, 157, 176, 156, 137, 235, 254, 293, 313)$  | $\{\emptyset, 1239, 125789, 13568, 167, 23679, 25689, 3578\}$                                                 |
| 941:128  | $0, 0, 0, 0, 0, e^{12}, e^{14} + e^{23}, e^{13} + e^{45}, e^{16} + e^{34}$ | $2/39(10, 8, 15, 13, 12, 18, 23, 25, 28)$            | $\{123589, 124579, 134678, 16\}$                                                                              |
| 941:129  | $0, 0, 0, 0, 0, e^{12}, e^{14} + e^{23}, e^{13} + e^{45}, e^{26} + e^{34}$ | $1/56(32, 22, 43, 33, 42, 54, 65, 75, 76)$           | $\{\emptyset, 13679, 14689, 3478\}$                                                                           |
| 941:131  | $0, 0, 0, 0, 0, e^{12}, e^{24} + e^{13}, e^{34} + e^{15}, e^{35} + e^{16}$ | $7/485(32, 37, 46, 41, 55, 69, 78, 87, 101)$         | $\{123789, 134567, 23469, 358\}$                                                                              |
| 941:132  | $0, 0, 0, 0, 0, e^{12}, e^{14} + e^{23}, e^{15} + e^{34}, e^{16} + e^{35}$ | $1/53(21, 32, 28, 39, 46, 53, 60, 67, 74)$           | $\{\emptyset, 12579, 1468, 2456789\}$                                                                         |
| 941:133  | $0, 0, 0, 0, 0, e^{12}, e^{14} + e^{23}, e^{45} + e^{13}, e^{26} + e^{35}$ | $1/109(59, 47, 82, 70, 71, 106, 129, 141, 153)$      | $\{\emptyset, 125789, 13679, 23568\}$                                                                         |
| 941:134  | $0, 0, 0, 0, 0, e^{12}, e^{24} + e^{13}, e^{15} + e^{34}, e^{26} + e^{35}$ | $1/449(246, 187, 269, 328, 351, 433, 515, 597, 620)$ | $\{\emptyset, 12579, 13689, 235678\}$                                                                         |
| 941:135  | $0, 0, 0, 0, 0, e^{12}, e^{23} + e^{14}, e^{15} + e^{34}, e^{26} + e^{35}$ | $1/461(233, 216, 305, 288, 360, 449, 521, 593, 665)$ | $\{123789, 15679, 26, 358\}$                                                                                  |
| 941:137  | $0, 0, 0, 0, 0, e^{12}, e^{34}, e^{45} + e^{13}, e^{35} + e^{24} + e^{16}$ | $1/25(7, 19, 20, 14, 13, 26, 34, 27, 33)$            | $\{123489, 124579, 345, 478\}$                                                                                |
| 941:138a | $0, 0, 0, 0, 0, e^{12}, e^{15} + e^{34}, e^{14} + e^{35}, e^{13} + e^{26}$ | $1/19(12, 6, 12, 13, 13, 18, 25, 25, 24)$            | $\{123459, 123789, 134569, 136789, 23468, 23567, 348, 357\}$                                                  |
| 941:138b | $0, 0, 0, 0, 0, e^{12}, e^{34} - e^{15}, e^{35} + e^{14}, e^{13} + e^{26}$ | $1/19(12, 6, 12, 13, 13, 18, 25, 25, 24)$            | $\{123459, 123789, 134569, 136789, 23468, 23567, 348, 357\}$                                                  |
| 941:140a | $0, 0, 0, 0, 0, e^{12}, e^{34} + e^{15}, e^{35} + e^{14}, e^{23} + e^{16}$ | $(0, 1, 0, 1, 1, 1, 1, 1)$                           | $\{123489, 123579, 13468, 13567, 234569, 236789, 345, 378\}$                                                  |

Table A.2 – Continued to next page

Table A.2 – Continued from previous page

| Name     | g                                                                                    | N                                                  | Signatures S                                             |
|----------|--------------------------------------------------------------------------------------|----------------------------------------------------|----------------------------------------------------------|
| 941:140b | $0, 0, 0, 0, 0, e^{12}, -e^{15} + e^{34}, e^{14} + e^{35}, e^{16} + e^{23}$          | $(0, 1, 0, 1, 1, 1, 1, 1)$                         | {123489, 123579, 13468, 13567, 234569, 236789, 345, 378} |
| 941:141  | $0, 0, 0, 0, 0, e^{12}, e^{14} + e^{35}, e^{45} + e^{23}, e^{13} + e^{26}$           | 1/217(128, 86, 172, 151, 107, 214, 279, 258, 300)  | {14689, 156789, 24567, 26}                               |
| 941:143  | $0, 0, 0, 0, 0, e^{12}, e^{13}, e^{23}, e^{35} + e^{14} + e^{26}$                    | 1/13(7, 6, 8, 12, 11, 13, 15, 14, 19)              | {0, 1239, 125789, 13689, 15679, 23567, 268, 3578}        |
| 941:144  | $0, 0, 0, 0, 0, e^{12}, e^{13}, e^{14} + e^{23}, e^{26} + e^{15}$                    | 1/17(7, 8, 13, 14, 16, 15, 20, 21, 23)             | {0, 12349, 12789, 13689, 14679, 2367, 2468, 3478}        |
| 941:145  | $0, 0, 0, 0, 0, e^{12}, e^{13}, e^{14} + e^{23}, e^{25} + e^{16}$                    | 1/22(9, 12, 16, 19, 18, 21, 25, 28, 30)            | {0, 12349, 12789, 1368, 1467, 23679, 24689, 3478}        |
| 941:146  | $0, 0, 0, 0, 0, e^{12}, e^{13}, e^{14}, e^{15} + e^{26} + e^{34}$                    | 1/63(28, 31, 45, 45, 62, 59, 73, 73, 90)           | {0, 12389, 12479, 13689, 14679, 234678, 26, 3478}        |
| 941:147  | $0, 0, 0, 0, 0, e^{12}, e^{13}, e^{14}, e^{45} + e^{23} + e^{16}$                    | 1/13(5, 9, 10, 9, 10, 14, 15, 14, 19)              | {0, 12479, 125789, 14567, 1678, 24689, 2569, 458}        |
| 941:148  | $0, 0, 0, 0, 0, e^{12}, e^{13}, e^{14}, e^{16} + e^{25} + e^{34}$                    | 1/22(9, 14, 16, 16, 18, 23, 25, 25, 32)            | {0, 12389, 12479, 1346, 1678, 23679, 24689, 3478}        |
| 941:150  | $0, 0, 0, 0, 0, e^{12}, e^{13}, e^{24}, e^{26} + e^{34} + e^{15}$                    | 1/29(15, 13, 20, 21, 26, 28, 35, 34, 41)           | {0, 12389, 12479, 1369, 146789, 23467, 268, 3478}        |
| 941:151  | $0, 0, 0, 0, 0, e^{12}, e^{13}, e^{25} + e^{14}, e^{23} + e^{16}$                    | 1/13(5, 7, 10, 12, 10, 12, 15, 17, 17)             | {0, 124579, 12789, 1467, 15678, 24689, 2569, 458}        |
| 941:152  | $0, 0, 0, 0, 0, e^{12}, e^{13}, e^{24} + e^{15}, e^{26} + e^{14}$                    | 1/63(28, 27, 49, 54, 53, 55, 77, 81, 82)           | {0, 12389, 12789, 13569, 15679, 235678, 2568, 37}        |
| 941:153  | $0, 0, 0, 0, 0, e^{12}, e^{13}, e^{25} + e^{14}, e^{16} + e^{24}$                    | 1/38(16, 19, 30, 32, 29, 35, 46, 48, 51)           | {0, 12389, 12789, 13568, 15678, 235679, 2569, 37}        |
| 941:155  | $0, 0, 0, 0, 0, e^{12}, e^{34}, e^{24} + e^{13}, e^{35} + e^{26} + e^{14}$           | 1/437(274, 165, 221, 330, 383, 439, 551, 495, 604) | {12349, 1456789, 2467, 3458}                             |
| 941:156  | $0, 0, 0, 0, 0, e^{12}, e^{14} + e^{23}, e^{13} + e^{25}, e^{34} + e^{16}$           | 1/41(20, 19, 30, 29, 31, 39, 49, 50, 59)           | {23569, 246789, 347, 58}                                 |
| 941:157  | $0, 0, 0, 0, 0, e^{12}, e^{24} + e^{13}, e^{15} + e^{23}, e^{34} + e^{16}$           | 3/97(14, 17, 24, 21, 27, 31, 38, 41, 45)           | {123579, 12489, 134678, 156}                             |
| 941:158  | $0, 0, 0, 0, 0, e^{12}, e^{23} + e^{14}, e^{34} + e^{15}, e^{13} + e^{26}$           | 1/159(84, 61, 122, 99, 137, 145, 183, 221, 206)    | {123459, 136789, 23568, 347}                             |
| 941:159  | $0, 0, 0, 0, 0, e^{12}, e^{13} + e^{24}, e^{14} + e^{35}, e^{16} + e^{23}$           | 3/7(1, 1, 2, 2, 1, 2, 3, 3, 3)                     | {123579, 134678, 234569, 38}                             |
| 941:162  | $0, 0, 0, 0, 0, e^{12}, e^{13}, e^{35} + e^{14}, e^{23} + e^{45} + e^{16}$           | 3/17(2, 4, 4, 5, 3, 6, 6, 7, 8)                    | {123489, 12359, 3457, 378}                               |
| 941:163  | $0, 0, 0, 0, 0, e^{12}, e^{13}, e^{14} + e^{35}, e^{25} + e^{34} + e^{16}$           | 1/32(12, 22, 17, 29, 24, 34, 29, 41, 46)           | {123579, 124589, 345, 578}                               |
| 941:164  | $0, 0, 0, 0, 0, e^{12}, e^{13}, e^{45} + e^{23}, e^{26} + e^{35} + e^{14}$           | 2/31(8, 6, 13, 12, 7, 14, 21, 19, 20)              | {123489, 124579, 3457, 48}                               |
| 941:169  | $0, 0, 0, 0, 0, e^{12}, e^{14} + e^{23}, e^{13} + e^{25}, e^{16} + e^{45}$           | 1/107(50, 54, 77, 81, 73, 104, 131, 127, 154)      | {0, 1367, 14568, 34578}                                  |
| 941:172  | $0, 0, 0, 0, 0, e^{12}, e^{34}, e^{25} + e^{13}, e^{16} + e^{35} + e^{24}$           | 2/31(6, 8, 11, 12, 9, 14, 23, 17, 20)              | {123489, 124579, 134568, 1467}                           |
| 941:173  | $0, 0, 0, 0, 0, e^{12}, e^{14} + e^{23}, e^{45} + e^{13}, e^{15} + e^{26}$           | 1/113(63, 42, 92, 71, 84, 105, 134, 155, 147)      | {123459, 125789, 23568, 24567}                           |
| 941:174  | $0, 0, 0, 0, 0, e^{12}, e^{23} + e^{14}, e^{13} + e^{45}, e^{16} + e^{25}$           | 1/2(1, 0, 2, 1, 2, 1, 2, 3, 2)                     | {123589, 124579, 234569, 256789}                         |
| 941:175  | $0, 0, 0, 0, 0, e^{12}, e^{13} + e^{24}, e^{15} + e^{34}, e^{16} + e^{25}$           | 1/53(23, 28, 37, 32, 46, 51, 60, 69, 74)           | {0, 1368, 14678, 347}                                    |
| 941:177a | $0, 0, 0, 0, 0, e^{12}, e^{35} + e^{14}, e^{45} + e^{13}, e^{16} + e^{25} + e^{34}$  | 1/8(0, 10, 5, 5, 0, 10, 5, 5, 10)                  | {123589, 124579, 345, 578}                               |
| 941:177b | $0, 0, 0, 0, 0, e^{12}, e^{35} - e^{14}, e^{45} + e^{13}, e^{25} + e^{16} + e^{34}$  | 1/8(0, 10, 5, 5, 0, 10, 5, 5, 10)                  | {123589, 124579, 345, 578}                               |
| 941:178a | $0, 0, 0, 0, 0, e^{12}, e^{14} + e^{35}, e^{23} + e^{45}, e^{15} + e^{26} + e^{34}$  | 29/109(3, 1, 3, 2, 2, 4, 5, 4, 5)                  | {123589, 124579, 345, 578}                               |
| 941:178b | $0, 0, 0, 0, 0, e^{12}, -e^{14} + e^{35}, e^{23} + e^{45}, e^{15} + e^{26} + e^{34}$ | 29/109(3, 1, 3, 2, 2, 4, 5, 4, 5)                  | {123589, 124579, 345, 578}                               |
| 941:179  | $0, 0, 0, 0, 0, e^{12}, e^{13}, e^{14} + e^{23}, e^{15} + e^{34} + e^{26}$           | 1/33(15, 16, 23, 24, 32, 31, 38, 39, 47)           | {0, 13689, 14679, 3478}                                  |
| 941:180  | $0, 0, 0, 0, 0, e^{12}, e^{13}, e^{14} + e^{23}, e^{35} + e^{24} + e^{16}$           | 1/41(17, 25, 26, 34, 33, 42, 43, 51, 59)           | {0, 125789, 13568, 23679}                                |
| 941:181  | $0, 0, 0, 0, 0, e^{12}, e^{13}, e^{14} + e^{23}, e^{34} + e^{25} + e^{16}$           | 1/32(14, 18, 21, 25, 28, 32, 35, 39, 46)           | {0, 23679, 24689, 3478}                                  |
| 941:182a | $0, 0, 0, 0, 0, e^{12}, e^{23} + e^{14}, e^{24} + e^{13}, e^{15} + e^{26}$           | 1/40(18, 18, 31, 31, 36, 36, 49, 49, 54)           | {0, 12349, 12789, 13679, 14689, 2368, 2467, 3478}        |
| 941:182b | $0, 0, 0, 0, 0, e^{12}, -e^{14} + e^{23}, e^{13} + e^{24}, e^{26} + e^{15}$          | 1/40(18, 18, 31, 31, 36, 36, 49, 49, 54)           | {0, 12349, 12789, 13679, 14689, 2368, 2467, 3478}        |
| 941:183  | $0, 0, 0, 0, 0, e^{12}, e^{13} + e^{24}, e^{15} + e^{23}, e^{26} + e^{14}$           | 1/33(15, 14, 27, 28, 26, 29, 42, 41, 43)           | {0, 12789, 13689, 2367}                                  |
| 941:184  | $0, 0, 0, 0, 0, e^{12}, e^{13}, e^{14} + e^{25}, e^{15} + e^{26} + e^{34}$           | 1/97(52, 41, 63, 71, 82, 93, 115, 123, 134)        | {124579, 135689, 256, 34578}                             |
| 941:186  | $0, 0, 0, 0, 0, e^{12}, e^{13}, e^{25} + e^{14}, e^{24} + e^{35} + e^{16}$           | 1/86(36, 49, 62, 72, 59, 85, 98, 108, 121)         | {0, 12389, 13568, 2569}                                  |
| 941:189  | $0, 0, 0, 0, 0, e^{12}, e^{23} + e^{14}, e^{45} + e^{13}, e^{16} + e^{25} + e^{34}$  | 2/7(2, 0, 3, 1, 4, 2, 3, 5, 4)                     | {123589, 124579}                                         |
| 941:191  | $0, 0, 0, 0, 0, e^{12}, e^{24} + e^{13}, e^{34} + e^{15}, e^{45} + e^{23} + e^{16}$  | 21/167(3, 5, 6, 4, 7, 8, 9, 10, 11)                | {12349, 3457}                                            |
| 941:192a | $0, 0, 0, 0, 0, e^{12}, e^{23} + e^{14}, e^{24} + e^{13}, e^{34} + e^{26} + e^{15}$  | 17/72(2, 2, 3, 3, 4, 4, 5, 5, 6)                   | {0, 13679, 14689, 3478}                                  |
| 941:192b | $0, 0, 0, 0, 0, e^{12}, -e^{14} + e^{23}, e^{13} + e^{24}, e^{26} + e^{34} + e^{15}$ | 17/72(2, 2, 3, 3, 4, 4, 5, 5, 6)                   | {0, 13679, 14689, 3478}                                  |
| 941:193  | $0, 0, 0, 0, 0, e^{12}, e^{14} + e^{23}, e^{13} + e^{25}, e^{26} + e^{34} + e^{15}$  | 5/47(5, 4, 7, 6, 8, 9, 11, 12, 13)                 | {123579, 256}                                            |
| 941:214  | $0, 0, 0, 0, 0, e^{12}, e^{13}, e^{14}, e^{45} + e^{26} + e^{17}$                    | 1/21(8, 12, 16, 15, 17, 20, 24, 23, 32)            | {0, 12349, 123589, 13469, 135689, 24568, 26, 458}        |
| 941:215  | $0, 0, 0, 0, 0, e^{12}, e^{13}, e^{24}, e^{26} + e^{45} + e^{17}$                    | 1/20(8, 11, 14, 13, 17, 19, 22, 24, 30)            | {0, 12349, 123589, 134689, 13569, 2456, 268, 458}        |

Table A.2 – Continued to next page

Table A.2 – Continued from previous page

| Name     | $g$                                                                        | $N$                                                  | Signatures $S$                                                                                                        |
|----------|----------------------------------------------------------------------------|------------------------------------------------------|-----------------------------------------------------------------------------------------------------------------------|
| 941:216a | $0, 0, 0, 0, 0, e^{12}, e^{13}, e^{14}, e^{26} + e^{37} + e^{45}$          | $1/7(3, 4, 4, 5, 6, 7, 7, 8, 11)$                    | $\{\emptyset, 12349, 123589, 12479, 125789, 13469, 135689, 14679, 156789, 2345678, 2367, 24568, 26, 34578, 37, 458\}$ |
| 941:216b | $0, 0, 0, 0, 0, -e^{12}, e^{13}, e^{14}, e^{45} + e^{26} + e^{37}$         | $1/7(3, 4, 4, 5, 6, 7, 7, 8, 11)$                    | $\{\emptyset, 12349, 123589, 12479, 125789, 13469, 135689, 14679, 156789, 2345678, 2367, 24568, 26, 34578, 37, 458\}$ |
| 941:218  | $0, 0, 0, 0, 0, e^{12}, e^{13}, e^{24}, e^{16} + e^{45} + e^{37}$          | $1/61(28, 36, 32, 39, 53, 64, 60, 75, 92)$           | $\{\emptyset, 12349, 123589, 12479, 125789, 34578, 37, 458\}$                                                         |
| 941:219a | $0, 0, 0, 0, 0, e^{12}, e^{13}, e^{24}, e^{37} + e^{45} + e^{26}$          | $1/81(44, 40, 40, 55, 69, 84, 84, 95, 124)$          | $\{\emptyset, 12349, 123589, 12479, 125789, 134689, 13569, 146789, 15679, 234567, 23678, 2456, 268, 34578, 37, 458\}$ |
| 941:219b | $0, 0, 0, 0, 0, -e^{12}, e^{13}, e^{24}, e^{37} + e^{45} + e^{26}$         | $1/81(44, 40, 40, 55, 69, 84, 84, 95, 124)$          | $\{\emptyset, 12349, 123589, 12479, 125789, 134689, 13569, 146789, 15679, 234567, 23678, 2456, 268, 34578, 37, 458\}$ |
| 941:221  | $0, 0, 0, 0, 0, e^{12}, e^{13}, e^{25} + e^{14}, e^{26} + e^{17}$          | $1/17(6, 9, 12, 16, 13, 15, 18, 22, 24)$             | $\{\emptyset, 123459, 12389, 13469, 135689, 2468, 256, 458\}$                                                         |
| 941:222  | $0, 0, 0, 0, 0, e^{12}, e^{13}, e^{25} + e^{14}, e^{16} + e^{37}$          | $1/297(124, 176, 150, 273, 221, 300, 274, 397, 424)$ | $\{\emptyset, 123459, 12389, 124579, 12789, 34578, 37, 458\}$                                                         |
| 941:223a | $0, 0, 0, 0, 0, e^{12}, e^{13}, e^{25} + e^{14}, e^{37} + e^{26}$          | $1/81(38, 40, 40, 69, 67, 78, 78, 107, 118)$         | $\{\emptyset, 123459, 12389, 124579, 12789, 13469, 135689, 14679, 156789, 234678, 23567, 2468, 256, 34578, 37, 458\}$ |
| 941:223b | $0, 0, 0, 0, 0, -e^{12}, e^{13}, e^{25} + e^{14}, e^{26} + e^{37}$         | $1/81(38, 40, 40, 69, 67, 78, 78, 107, 118)$         | $\{\emptyset, 123459, 12389, 124579, 12789, 13469, 135689, 14679, 156789, 234678, 23567, 2468, 256, 34578, 37, 458\}$ |
| 941:225  | $0, 0, 0, 0, 0, e^{12}, e^{13}, e^{45} + e^{23}, e^{17} + e^{26}$          | $7/139(7, 11, 15, 13, 13, 18, 22, 26, 29)$           | $\{123489, 123589, 134569, 1369, 2456, 26, 48, 58\}$                                                                  |
| 941:226  | $0, 0, 0, 0, 0, e^{12}, e^{13}, e^{24} + e^{35}, e^{17} + e^{26}$          | $1/14(6, 7, 8, 12, 11, 13, 14, 19, 20)$              | $\{\emptyset, 123459, 12389, 134689, 13569, 246, 2568, 458\}$                                                         |
| 941:227a | $0, 0, 0, 0, 0, e^{12}, e^{13}, e^{23} + e^{45}, e^{37} + e^{26}$          | $1/5(2, 3, 3, 3, 3, 5, 5, 6, 8)$                     | $\{123489, 123589, 124579, 1279, 134569, 1369, 146789, 156789, 234678, 235678, 2456, 26, 3457, 37, 48, 58\}$          |
| 941:227b | $0, 0, 0, 0, 0, -e^{12}, e^{13}, e^{45} + e^{23}, e^{37} + e^{26}$         | $1/5(2, 3, 3, 3, 3, 5, 5, 6, 8)$                     | $\{123489, 123589, 124579, 1279, 134569, 1369, 146789, 156789, 234678, 235678, 2456, 26, 3457, 37, 48, 58\}$          |
| 941:228a | $0, 0, 0, 0, 0, e^{12}, e^{13}, e^{35} + e^{24}, e^{26} + e^{37}$          | $1/7(4, 3, 3, 6, 6, 7, 7, 9, 10)$                    | $\{\emptyset, 123459, 12389, 12479, 125789, 134689, 13569, 1456789, 1679, 234567, 23678, 246, 2568, 3478, 357, 458\}$ |
| 941:228b | $0, 0, 0, 0, 0, -e^{12}, e^{13}, e^{35} + e^{24}, e^{37} + e^{26}$         | $1/7(4, 3, 3, 6, 6, 7, 7, 9, 10)$                    | $\{\emptyset, 123459, 12389, 12479, 125789, 134689, 13569, 1456789, 1679, 234567, 23678, 246, 2568, 3478, 357, 458\}$ |
| 941:231a | $0, 0, 0, 0, 0, e^{12}, e^{13}, e^{45}, e^{37} + e^{14} + e^{26}$          | $1/5(3, 2, 2, 4, 3, 5, 5, 7, 7)$                     | $\{123459, 123489, 124579, 124789, 134569, 134689, 145679, 146789, 234567, 234678, 2456, 2468, 3457, 3478, 45, 48\}$  |
| 941:231b | $0, 0, 0, 0, 0, -e^{12}, e^{13}, e^{45}, e^{26} + e^{37} + e^{14}$         | $1/5(3, 2, 2, 4, 3, 5, 5, 7, 7)$                     | $\{123459, 123489, 124579, 124789, 134569, 134689, 145679, 146789, 234567, 234678, 2456, 2468, 3457, 3478, 45, 48\}$  |
| 941:232  | $0, 0, 0, 0, 0, e^{12}, e^{13}, e^{45}, e^{16} + e^{24} + e^{37}$          | $1/139(48, 104, 76, 96, 91, 152, 124, 187, 200)$     | $\{123459, 123489, 124579, 124789, 3457, 3478, 45, 48\}$                                                              |
| 941:237  | $0, 0, 0, 0, 0, e^{12}, e^{13}, e^{23}, e^{45} + e^{17} + e^{26}$          | $1/13(6, 7, 8, 10, 10, 13, 14, 15, 20)$              | $\{\emptyset, 12349, 12359, 134689, 135689, 24568, 268, 45\}$                                                         |
| 941:238a | $0, 0, 0, 0, 0, e^{12}, e^{13}, e^{23}, e^{37} + e^{45} + e^{26}$          | $5/19(2, 2, 2, 3, 3, 4, 4, 4, 6)$                    | $\{\emptyset, 12349, 12359, 124789, 125789, 134689, 135689, 14679, 15679, 234567, 2367, 24568, 268, 34578, 378, 45\}$ |
| 941:238b | $0, 0, 0, 0, 0, -e^{12}, e^{13}, e^{23}, e^{37} + e^{45} + e^{26}$         | $5/19(2, 2, 2, 3, 3, 4, 4, 4, 6)$                    | $\{\emptyset, 12349, 12359, 124789, 125789, 134689, 135689, 14679, 15679, 234567, 2367, 24568, 268, 34578, 378, 45\}$ |
| 941:240a | $0, 0, 0, 0, 0, e^{12}, e^{13}, e^{14}, e^{26} + e^{37} + e^{15}$          | $1/19(8, 10, 10, 15, 20, 18, 18, 23, 28)$            | $\{123459, 123589, 124579, 125789, 134569, 135689, 145679, 156789, 2345678, 23567, 24568, 256, 34578, 357, 458, 5\}$  |
| 941:240b | $0, 0, 0, 0, 0, -e^{12}, e^{13}, e^{14}, e^{15} + e^{37} + e^{26}$         | $1/19(8, 10, 10, 15, 20, 18, 18, 23, 28)$            | $\{123459, 123589, 124579, 125789, 134569, 135689, 145679, 156789, 2345678, 23567, 24568, 256, 34578, 357, 458, 5\}$  |
| 941:241  | $0, 0, 0, 0, 0, e^{12}, e^{13}, e^{14}, e^{16} + e^{37} + e^{25}$          | $1/59(24, 40, 32, 47, 48, 64, 56, 71, 88)$           | $\{\emptyset, 12349, 12389, 12479, 12789, 3478, 37, 48\}$                                                             |
| 941:243a | $0, 0, 0, 0, 0, e^{12}, e^{13}, e^{24}, e^{26} + e^{15} + e^{37}$          | $1/17(9, 8, 8, 13, 16, 17, 17, 21, 25)$              | $\{\emptyset, 12349, 12389, 12479, 12789, 134689, 1369, 146789, 1679, 23467, 23678, 246, 268, 3478, 37, 48\}$         |
| 941:243b | $0, 0, 0, 0, 0, -e^{12}, e^{13}, e^{24}, e^{15} + e^{26} + e^{37}$         | $1/17(9, 8, 8, 13, 16, 17, 17, 21, 25)$              | $\{\emptyset, 12349, 12389, 12479, 12789, 134689, 1369, 146789, 1679, 23467, 23678, 246, 268, 3478, 37, 48\}$         |
| 941:244  | $0, 0, 0, 0, 0, e^{12}, e^{13}, e^{24}, e^{37} + e^{16} + e^{25}$          | $1/34(16, 18, 17, 25, 32, 34, 33, 43, 50)$           | $\{\emptyset, 12349, 12389, 12479, 12789, 3478, 37, 48\}$                                                             |
| 941:246  | $0, 0, 0, 0, 0, e^{12}, e^{13}, e^{24}, e^{17} + e^{35} + e^{26}$          | $1/23(10, 12, 14, 17, 20, 22, 24, 29, 34)$           | $\{\emptyset, 12349, 12389, 134689, 1369, 246, 268, 48\}$                                                             |
| 941:247  | $0, 0, 0, 0, 0, e^{12}, e^{13}, e^{14} + e^{25}, e^{45} + e^{17} + e^{26}$ | $1/69(27, 38, 49, 57, 46, 65, 76, 84, 103)$          | $\{\emptyset, 13469, 135689, 458\}$                                                                                   |

Table A.2 – Continued to next page

Table A.2 – Continued from previous page

| Name     | $g$                                                                         | $N$                                                  | Signatures $S$                                                                                                        |
|----------|-----------------------------------------------------------------------------|------------------------------------------------------|-----------------------------------------------------------------------------------------------------------------------|
| 941:248  | $0, 0, 0, 0, 0, e^{12}, e^{13}, e^{25} + e^{14}, e^{37} + e^{16} + e^{45}$  | $1/59(26, 36, 31, 49, 39, 62, 57, 75, 88)$           | $\{\emptyset, 34578, 37, 458\}$                                                                                       |
| 941:249a | $0, 0, 0, 0, 0, e^{12}, e^{13}, e^{25} + e^{14}, e^{37} + e^{45} + e^{26}$  | $1/27(13, 14, 14, 21, 20, 27, 27, 34, 41)$           | $\{\emptyset, 13469, 135689, 14679, 156789, 34578, 37, 458\}$                                                         |
| 941:249b | $0, 0, 0, 0, 0, -e^{12}, e^{13}, e^{14} + e^{25}, e^{37} + e^{26} + e^{45}$ | $1/27(13, 14, 14, 21, 20, 27, 27, 34, 41)$           | $\{\emptyset, 13469, 135689, 14679, 156789, 34578, 37, 458\}$                                                         |
| 941:251  | $0, 0, 0, 0, 0, e^{12}, e^{13}, e^{35} + e^{24}, e^{17} + e^{26} + e^{45}$  | $1/223(99, 116, 133, 174, 157, 215, 232, 290, 331)$  | $\{\emptyset, 134689, 13569, 458\}$                                                                                   |
| 941:252a | $0, 0, 0, 0, 0, e^{12}, e^{13}, e^{35} + e^{24}, e^{45} + e^{26} + e^{37}$  | $1/61(34, 29, 29, 46, 46, 63, 63, 75, 92)$           | $\{\emptyset, 12479, 125789, 134689, 13569, 234567, 23678, 458\}$                                                     |
| 941:252b | $0, 0, 0, 0, 0, -e^{12}, e^{13}, e^{24} + e^{35}, e^{26} + e^{45} + e^{37}$ | $1/61(34, 29, 29, 46, 46, 63, 63, 75, 92)$           | $\{\emptyset, 12479, 125789, 134689, 13569, 234567, 23678, 458\}$                                                     |
| 941:255  | $0, 0, 0, 0, 0, e^{12}, e^{13}, e^{14} + e^{23}, e^{17} + e^{45} + e^{26}$  | $1/473(209, 256, 303, 350, 371, 465, 512, 559, 721)$ | $\{\emptyset, 12349, 135689, 24568\}$                                                                                 |
| 941:258  | $0, 0, 0, 0, 0, e^{12}, e^{13}, e^{25} + e^{14}, e^{16} + e^{24} + e^{37}$  | $1/109(48, 62, 55, 96, 82, 110, 103, 144, 158)$      | $\{\emptyset, 12389, 12789, 37\}$                                                                                     |
| 941:259  | $0, 0, 0, 0, 0, e^{12}, e^{13}, e^{25} + e^{14}, e^{17} + e^{26} + e^{34}$  | $1/193(82, 101, 120, 164, 145, 183, 202, 246, 284)$  | $\{\emptyset, 12389, 135689, 256\}$                                                                                   |
| 941:260a | $0, 0, 0, 0, 0, e^{12}, e^{13}, e^{15} + e^{24}, e^{26} + e^{37} + e^{14}$  | $1/149(76, 67, 67, 134, 125, 143, 143, 201, 210)$    | $\{123459, 124579, 134689, 146789, 23467, 246, 34578, 458\}$                                                          |
| 941:260b | $0, 0, 0, 0, 0, -e^{12}, e^{13}, e^{15} + e^{24}, e^{14} + e^{26} + e^{37}$ | $1/149(76, 67, 67, 134, 125, 143, 143, 201, 210)$    | $\{123459, 124579, 134689, 146789, 23467, 246, 34578, 458\}$                                                          |
| 941:262  | $0, 0, 0, 0, 0, e^{12}, e^{13}, e^{15} + e^{24}, e^{17} + e^{26} + e^{34}$  | $1/32(12, 17, 22, 24, 29, 29, 34, 41, 46)$           | $\{\emptyset, 12389, 13569, 2568\}$                                                                                   |
| 941:263a | $0, 0, 0, 0, 0, e^{12}, e^{13}, e^{23} + e^{45}, e^{14} + e^{37} + e^{26}$  | $1/2(1, 1, 1, 2, 0, 2, 2, 2, 3)$                     | $\{123489, 124579, 134569, 146789, 234678, 2456, 3457, 48\}$                                                          |
| 941:263b | $0, 0, 0, 0, 0, -e^{12}, e^{13}, e^{45} + e^{23}, e^{37} + e^{14} + e^{26}$ | $1/2(1, 1, 1, 2, 0, 2, 2, 2, 3)$                     | $\{123489, 124579, 134569, 146789, 234678, 2456, 3457, 48\}$                                                          |
| 941:264  | $0, 0, 0, 0, 0, e^{12}, e^{13}, e^{23} + e^{45}, e^{24} + e^{37} + e^{16}$  | $2/65(11, 25, 18, 22, 21, 36, 29, 43, 47)$           | $\{123489, 124579, 3457, 48\}$                                                                                        |
| 941:269a | $0, 0, 0, 0, 0, e^{12}, e^{13}, e^{14} + e^{23}, e^{15} + e^{26} + e^{37}$  | $3/16(2, 3, 3, 4, 6, 5, 5, 6, 8)$                    | $\{123589, 124579, 134569, 156789, 2345678, 256, 357, 458\}$                                                          |
| 941:269b | $0, 0, 0, 0, 0, -e^{12}, e^{13}, e^{23} + e^{14}, e^{15} + e^{26} + e^{37}$ | $3/16(2, 3, 3, 4, 6, 5, 5, 6, 8)$                    | $\{123589, 124579, 134569, 156789, 2345678, 256, 357, 458\}$                                                          |
| 941:270  | $0, 0, 0, 0, 0, e^{12}, e^{13}, e^{23} + e^{14}, e^{25} + e^{37} + e^{16}$  | $1/176(72, 118, 95, 141, 144, 190, 167, 213, 262)$   | $\{\emptyset, 12349, 12789, 3478\}$                                                                                   |
| 941:274  | $0, 0, 0, 0, 0, e^{12}, e^{13}, e^{23}, e^{45} + e^{38} + e^{17} + e^{26}$  | $5/19(2, 2, 2, 3, 3, 4, 4, 6)$                       | $\{\emptyset, 12349, 12359, 45\}$                                                                                     |
| 941:279  | $0, 0, 0, 0, 0, e^{12}, e^{34}, e^{15}, e^{37} + e^{16}$                    | $1/33(12, 24, 13, 22, 27, 36, 35, 39, 48)$           | $\{\emptyset, 123459, 123489, 124579, 124789, 13567, 13678, 156, 168, 2345689, 23469, 2456789, 24679, 3578, 37, 58\}$ |
| 941:280  | $0, 0, 0, 0, 0, e^{12}, e^{34}, e^{15}, e^{37} + e^{26}$                    | $1/12(6, 6, 5, 8, 9, 12, 13, 15, 18)$                | $\{\emptyset, 123459, 123489, 124579, 124789, 134569, 134689, 145679, 146789, 235678, 2367, 2568, 26, 3578, 37, 58\}$ |
| 941:283  | $0, 0, 0, 0, 0, e^{12}, e^{34}, e^{25} + e^{13}, e^{16} + e^{37}$           | $1/10(6, 4, 5, 6, 7, 10, 11, 11, 16)$                | $\{123489, 124579, 135678, 16, 234569, 246789, 37, 58\}$                                                              |
| 941:284  | $0, 0, 0, 0, 0, e^{12}, e^{34}, e^{15} + e^{23}, e^{16} + e^{37}$           | $7/139(7, 15, 8, 13, 16, 22, 21, 23, 29)$            | $\{123489, 124579, 13567, 168, 2345689, 24679, 37, 58\}$                                                              |
| 941:285  | $0, 0, 0, 0, 0, e^{12}, e^{34}, e^{25} + e^{13}, e^{16} + e^{47}$           | $1/172(89, 82, 120, 70, 127, 171, 190, 209, 260)$    | $\{123489, 123789, 1467, 16, 234569, 235679, 4578, 58\}$                                                              |
| 941:286  | $0, 0, 0, 0, 0, e^{12}, e^{34}, e^{15} + e^{23}, e^{47} + e^{16}$           | $1/353(143, 230, 212, 152, 299, 373, 364, 442, 516)$ | $\{\emptyset, 123459, 123579, 14567, 156, 23469, 23679, 47\}$                                                         |
| 941:287  | $0, 0, 0, 0, 0, e^{12}, e^{34}, e^{15}, e^{16} + e^{25} + e^{37}$           | $1/69(27, 48, 28, 46, 54, 75, 74, 81, 102)$          | $\{\emptyset, 123489, 124789, 13678, 168, 23469, 24679, 37\}$                                                         |
| 941:288  | $0, 0, 0, 0, 0, e^{12}, e^{34}, e^{35}, e^{37} + e^{26} + e^{15}$           | $1/317(208, 128, 117, 230, 256, 336, 347, 373, 464)$ | $\{\emptyset, 123489, 12479, 134689, 14679, 23678, 26, 378\}$                                                         |
| 941:289  | $0, 0, 0, 0, 0, e^{12}, e^{34}, e^{15}, e^{26} + e^{35} + e^{47}$           | $1/172(84, 85, 120, 67, 134, 169, 187, 218, 254)$    | $\{123459, 123579, 134569, 135679, 245678, 2568, 4578, 58\}$                                                          |
| 941:299  | $0, 0, 0, 0, 0, e^{12}, e^{34}, e^{13}, e^{37} + e^{15} + e^{26}$           | $1/293(176, 136, 125, 198, 272, 312, 323, 301, 448)$ | $\{\emptyset, 12349, 124789, 13469, 146789, 23678, 26, 378\}$                                                         |
| 941:300  | $0, 0, 0, 0, 0, e^{12}, e^{34}, e^{13}, e^{37} + e^{16} + e^{25}$           | $1/59(28, 36, 27, 38, 56, 64, 65, 55, 92)$           | $\{123489, 12479, 13678, 16, 23469, 246789, 37, 8\}$                                                                  |
| 941:301  | $0, 0, 0, 0, 0, e^{12}, e^{34}, e^{13}, e^{26} + e^{15} + e^{47}$           | $1/83(46, 40, 48, 39, 80, 86, 87, 94, 126)$          | $\{\emptyset, 12349, 12379, 13469, 13679, 2467, 26, 47\}$                                                             |
| 941:302  | $0, 0, 0, 0, 0, e^{12}, e^{34}, e^{13}, e^{47} + e^{16} + e^{25}$           | $1/281(127, 176, 174, 128, 254, 303, 302, 301, 430)$ | $\{\emptyset, 12349, 12379, 14678, 168, 234689, 236789, 47\}$                                                         |
| 941:303  | $0, 0, 0, 0, 0, e^{12}, e^{34}, e^{15}, e^{47} + e^{13} + e^{26}$           | $1/10(6, 4, 8, 3, 7, 10, 11, 13, 14)$                | $\{123459, 123489, 123579, 123789, 134569, 134689, 135679, 136789\}$                                                  |
| 941:304  | $0, 0, 0, 0, 0, e^{12}, e^{34}, e^{15}, e^{16} + e^{23} + e^{47}$           | $1/139(48, 104, 96, 52, 115, 152, 148, 163, 200)$    | $\{123459, 123489, 123579, 123789, 2345689, 23469, 2356789, 23679\}$                                                  |
| 941:305  | $0, 0, 0, 0, 0, e^{12}, e^{34}, e^{13} + e^{25}, e^{37} + e^{26} + e^{15}$  | $7/569(59, 31, 34, 53, 62, 90, 87, 93, 121)$         | $\{123489, 14679, 268, 37\}$                                                                                          |
| 941:306  | $0, 0, 0, 0, 0, e^{12}, e^{34}, e^{13} + e^{25}, e^{47} + e^{26} + e^{15}$  | $1/53(34, 22, 32, 23, 44, 56, 55, 66, 78)$           | $\{\emptyset, 13469, 13679, 47\}$                                                                                     |
| 941:307  | $0, 0, 0, 0, 0, e^{12}, e^{34}, e^{13} + e^{25}, e^{47} + e^{16} + e^{35}$  | $2/47(12, 11, 17, 9, 18, 23, 26, 29, 35)$            | $\{234569, 235679, 4578, 58\}$                                                                                        |
| 941:308  | $0, 0, 0, 0, 0, e^{12}, e^{34}, e^{25} + e^{13}, e^{16} + e^{37} + e^{45}$  | $1/29(19, 7, 12, 21, 24, 26, 33, 31, 45)$            | $\{124579, 135678, 234569, 58\}$                                                                                      |
| 941:309  | $0, 0, 0, 0, 0, e^{12}, e^{34}, e^{15} + e^{23}, e^{16} + e^{35} + e^{47}$  | $1/129(52, 84, 78, 55, 110, 136, 133, 162, 188)$     | $\{123459, 123579, 14567, 156\}$                                                                                      |
| 941:330  | $0, 0, 0, 0, 0, e^{12}, e^{34}, e^{24} + e^{13}, e^{15} + e^{26} + e^{37}$  | $3/53(11, 8, 8, 11, 16, 19, 19, 19, 27)$             | $\{\emptyset, 12349, 146789, 23678\}$                                                                                 |
| 941:331  | $0, 0, 0, 0, 0, e^{12}, e^{34}, e^{24} + e^{13}, e^{25} + e^{37} + e^{16}$  | $1/224(115, 118, 117, 114, 230, 233, 231, 232, 348)$ | $\{124579, 156, 234569, 357\}$                                                                                        |
| 941:332  | $0, 0, 0, 0, 0, e^{12}, e^{34}, e^{13} + e^{25}, e^{23} + e^{47} + e^{16}$  | $1/143(60, 82, 120, 41, 98, 142, 161, 180, 202)$     | $\{123489, 123789, 234569, 235679\}$                                                                                  |
| 941:333  | $0, 0, 0, 0, 0, e^{12}, e^{34}, e^{13} + e^{25}, e^{26} + e^{37} + e^{14}$  | $1/65(50, 22, 25, 44, 53, 72, 69, 75, 94)$           | $\{123489, 124579, 1345689, 14679\}$                                                                                  |
| 941:334  | $0, 0, 0, 0, 0, e^{12}, e^{34}, e^{13} + e^{25}, e^{37} + e^{16} + e^{24}$  | $1/4(2, 2, 1, 4, 1, 4, 5, 3, 6)$                     | $\{123489, 124579, 234569, 246789\}$                                                                                  |

Table A.2 – Continued to next page



Table A.2 – Continued from previous page

| Name     | $g$                                                                         | $N$                                                | Signatures $S$                                                                                                                                                                                                                |
|----------|-----------------------------------------------------------------------------|----------------------------------------------------|-------------------------------------------------------------------------------------------------------------------------------------------------------------------------------------------------------------------------------|
| 941:397a | $0, 0, 0, 0, 0, e^{12}, e^{13}, e^{14}, e^{37} + e^{26} + e^{15} + e^{48}$  | $1/9(4, 5, 5, 5, 10, 9, 9, 9, 14)$                 | {123459, 123589, 124579, 125789, 134569, 135689, 145679, 156789, 2345678, 23567, 24568, 256, 34578, 357, 458, 5}                                                                                                              |
| 941:397b | $0, 0, 0, 0, 0, e^{12}, -e^{13}, e^{14}, e^{26} + e^{15} + e^{37} + e^{48}$ | $1/9(4, 5, 5, 5, 10, 9, 9, 9, 14)$                 | {123459, 123589, 124579, 125789, 134569, 135689, 145679, 156789, 2345678, 23567, 24568, 256, 34578, 357, 458, 5}                                                                                                              |
| 941:401a | $0, 0, 0, 0, 0, e^{12}, e^{13}, e^{24}, e^{48} + e^{37} + e^{26} + e^{15}$  | $5/161(18, 16, 16, 17, 32, 34, 34, 33, 50)$        | { $\emptyset$ , 12349, 12389, 12479, 12789, 3478, 37, 48}                                                                                                                                                                     |
| 941:401b | $0, 0, 0, 0, 0, -e^{12}, e^{13}, e^{24}, e^{37} + e^{48} + e^{26} + e^{15}$ | $5/161(18, 16, 16, 17, 32, 34, 34, 33, 50)$        | { $\emptyset$ , 12349, 12389, 12479, 12789, 3478, 37, 48}                                                                                                                                                                     |
| 941:403  | $0, 0, 0, 0, 0, e^{12}, e^{13}, e^{24}, e^{48} + e^{26} + e^{35} + e^{17}$  | $5/109(10, 12, 14, 11, 20, 22, 24, 23, 34)$        | { $\emptyset$ , 12349, 12389, 48}                                                                                                                                                                                             |
| 941:439  | $0, 0, 0, 0, 0, e^{12}, e^{13}, e^{45}, e^{48} + e^{26} + e^{17}$           | $1/204(84, 117, 150, 91, 136, 201, 234, 227, 318)$ | { $\emptyset$ , 123459, 123589, 134569, 135689, 2468, 26, 48}                                                                                                                                                                 |
| 941:440a | $0, 0, 0, 0, 0, e^{12}, e^{13}, e^{45}, e^{37} + e^{26} + e^{48}$           | $1/60(30, 33, 33, 28, 40, 63, 63, 68, 96)$         | { $\emptyset$ , 123459, 123589, 124579, 125789, 134569, 135689, 145679, 156789, 234678, 2367, 2468, 26, 3478, 37, 48}                                                                                                         |
| 941:440b | $0, 0, 0, 0, 0, -e^{12}, e^{13}, e^{45}, e^{26} + e^{37} + e^{48}$          | $1/60(30, 33, 33, 28, 40, 63, 63, 68, 96)$         | { $\emptyset$ , 123459, 123589, 124579, 125789, 134569, 135689, 145679, 156789, 234678, 2367, 2468, 26, 3478, 37, 48}                                                                                                         |
| 941:449a | $0, 0, 0, 0, 0, e^{12}, e^{13}, e^{45}, e^{58} + e^{14} + e^{26} + e^{37}$  | $5/47(6, 4, 4, 8, 3, 10, 10, 11, 14)$              | {123459, 123489, 124579, 124789, 134569, 134689, 145679, 146789}                                                                                                                                                              |
| 941:449b | $0, 0, 0, 0, 0, -e^{12}, e^{13}, e^{45}, e^{58} + e^{37} + e^{14} + e^{26}$ | $5/47(6, 4, 4, 8, 3, 10, 10, 11, 14)$              | {123459, 123489, 124579, 124789, 134569, 134689, 145679, 146789}                                                                                                                                                              |
| 941:450  | $0, 0, 0, 0, 0, e^{12}, e^{13}, e^{45}, e^{16} + e^{24} + e^{58} + e^{37}$  | $5/164(12, 26, 19, 24, 13, 38, 31, 37, 50)$        | {123459, 123489, 124579, 124789}                                                                                                                                                                                              |
| 95:1     | $0, 0, 0, 0, 0, e^{12}, e^{13}, e^{23}, e^{14}, e^{24}$                     | $1/11(6, 6, 7, 7, 12, 13, 13, 13, 13)$             | { $\emptyset$ , 1234, 12389, 12467, 126789, 134579, 13578, 14569, 1568, 234568, 23569, 24578, 2579, 346789, 367, 489}                                                                                                         |
| 95:2     | $0, 0, 0, 0, 0, e^{12}, e^{13}, e^{24}, e^{34}, e^{14} + e^{23}$            | $7/12(1, 1, 1, 1, 2, 2, 2, 2, 2)$                  | { $\emptyset$ , 1234, 12679, 13589, 145678, 235678, 24589, 34679}                                                                                                                                                             |
| 94:6     | $0, 0, 0, 0, 0, e^{12}, e^{13}, e^{14}, e^{15}$                             | $1/6(2, 5, 5, 5, 5, 7, 7, 7, 7)$                   | { $\emptyset$ , 12345, 12349, 12358, 12389, 12457, 12479, 12578, 12789, 13456, 13469, 13568, 13689, 14567, 14679, 15678, 16789, 23456789, 234678, 235679, 2367, 245689, 2468, 2569, 26, 345789, 3478, 3579, 37, 4589, 48, 59} |
| 94:7     | $0, 0, 0, 0, 0, e^{12}, e^{13}, e^{14}, e^{25}$                             | $1/13(6, 8, 10, 10, 9, 14, 16, 16, 17)$            | { $\emptyset$ , 12345, 12349, 12358, 12389, 12457, 12479, 12578, 12789, 134569, 1346, 135689, 1368, 145679, 1467, 156789, 1678, 2345678, 2346789, 23567, 23679, 24568, 24689, 256, 269, 345789, 3478, 3579, 37, 4589, 48, 59} |
| 94:8     | $0, 0, 0, 0, 0, e^{12}, e^{13}, e^{24}, e^{35}$                             | $1/11(7, 6, 6, 8, 8, 13, 13, 14, 14)$              | { $\emptyset$ , 12345, 12349, 12358, 12389, 124579, 1247, 125789, 1278, 134568, 134689, 1356, 1369, 1456789, 14678, 15679, 167, 234567, 234679, 235678, 236789, 24569, 246, 25689, 268, 34578, 34789, 357, 379, 4589, 48, 59} |
| 94:9     | $0, 0, 0, 0, 0, e^{12}, e^{13}, e^{23}, e^{14} + e^{25}$                    | $1/11(6, 6, 7, 9, 9, 12, 13, 13, 15)$              | { $\emptyset$ , 12345, 1239, 124578, 12789, 13468, 135689, 1467, 15679, 234679, 23567, 24689, 2568, 345789, 378, 459}                                                                                                         |
| 94:10    | $0, 0, 0, 0, 0, e^{12}, e^{13}, e^{14}, e^{15} + e^{23}$                    | $1/9(4, 6, 6, 7, 8, 10, 10, 11, 12)$               | { $\emptyset$ , 12345, 12358, 12479, 12789, 13469, 13689, 14567, 15678, 234678, 2367, 245689, 2569, 345789, 3579, 48}                                                                                                         |
| 94:11    | $0, 0, 0, 0, 0, e^{12}, e^{13}, e^{24}, e^{15} + e^{23}$                    | $1/14(7, 8, 10, 10, 11, 15, 17, 18, 18)$           | { $\emptyset$ , 12345, 12358, 12479, 12789, 134689, 1369, 145678, 1567, 23467, 23678, 24569, 25689, 345789, 3579, 48}                                                                                                         |
| 94:12    | $0, 0, 0, 0, 0, e^{12}, e^{13}, e^{14}, e^{45} + e^{23}$                    | $1/16(8, 11, 11, 10, 12, 19, 19, 18, 22)$          | { $\emptyset$ , 12345, 1238, 12479, 125789, 13469, 135689, 14567, 1678, 2345678, 2367, 24689, 2569, 34789, 3579, 458}                                                                                                         |
| 94:13    | $0, 0, 0, 0, 0, e^{12}, e^{13}, e^{24}, e^{35} + e^{14}$                    | $1/23(14, 13, 13, 16, 17, 27, 27, 29, 30)$         | { $\emptyset$ , 12345, 12389, 1247, 125789, 134568, 1369, 14678, 15679, 234679, 235678, 24569, 268, 34789, 357, 4589}                                                                                                         |
| 94:14    | $0, 0, 0, 0, 0, e^{12}, e^{13}, e^{24}, e^{15} + e^{34}$                    | $1/16(8, 10, 11, 10, 13, 18, 19, 20, 21)$          | { $\emptyset$ , 12345, 12389, 12479, 12578, 134568, 1369, 146789, 1567, 23467, 2356789, 24569, 268, 3478, 3579, 4589}                                                                                                         |
| 94:15    | $0, 0, 0, 0, 0, e^{12}, e^{13}, e^{23} + e^{14}, e^{45}$                    | $1/31(18, 19, 19, 20, 21, 37, 37, 38, 41)$         | { $\emptyset$ , 12345, 12349, 125789, 1278, 135689, 1368, 14567, 14679, 235679, 2367, 24568, 24689, 34578, 34789, 59}                                                                                                         |
| 94:16    | $0, 0, 0, 0, 0, e^{12}, e^{34}, e^{13} + e^{24}, e^{15}$                    | $1/23(12, 15, 16, 13, 17, 27, 29, 28, 29)$         | { $\emptyset$ , 12345, 12349, 1258, 1289, 13567, 13679, 145678, 146789, 2356789, 23678, 245679, 2467, 34589, 348, 59}                                                                                                         |

Table A.2 – Continued to next page

Table A.2 – Continued from previous page

| Name   | $g$                                                                                  | $N$                                        | Signatures $S$                                                                                                        |
|--------|--------------------------------------------------------------------------------------|--------------------------------------------|-----------------------------------------------------------------------------------------------------------------------|
| 94:17  | $0, 0, 0, 0, 0, e^{12}, e^{13}, e^{45}, e^{35} + e^{24}$                             | $1/37(21, 24, 24, 23, 23, 45, 45, 46, 47)$ | $\{\emptyset, 12345, 1239, 12478, 125789, 134689, 13568, 145679, 167, 234567, 23679, 2468, 25689, 34789, 3578, 459\}$ |
| 94:18  | $0, 0, 0, 0, 0, e^{12}, e^{13}, e^{23} + e^{14}, e^{15} + e^{24}$                    | $1/12(6, 7, 8, 9, 10, 13, 14, 15, 16)$     | $\{\emptyset, 12345, 12789, 13568, 14679, 235679, 2468, 345789\}$                                                     |
| 94:19  | $0, 0, 0, 0, 0, e^{12}, e^{13}, e^{14} + e^{23}, e^{24} + e^{35}$                    | $1/17(9, 11, 10, 12, 13, 20, 19, 21, 23)$  | $\{\emptyset, 12345, 125789, 13568, 145679, 23679, 2468, 34789\}$                                                     |
| 94:20a | $0, 0, 0, 0, 0, e^{12}, e^{14} + e^{23}, e^{13} + e^{24}, e^{15}$                    | $1/15(8, 8, 11, 11, 11, 16, 19, 19, 19)$   | $\{\emptyset, 12345, 12349, 12578, 12789, 13567, 13679, 14568, 14689, 235689, 2368, 245679, 2467, 345789, 3478, 59\}$ |
| 94:20b | $0, 0, 0, 0, 0, e^{12}, -e^{14} + e^{23}, e^{24} + e^{13}, e^{15}$                   | $1/15(8, 8, 11, 11, 11, 16, 19, 19, 19)$   | $\{\emptyset, 12345, 12349, 12578, 12789, 13567, 13679, 14568, 14689, 235689, 2368, 245679, 2467, 345789, 3478, 59\}$ |
| 94:21  | $0, 0, 0, 0, 0, e^{12}, e^{34}, e^{23} + e^{14}, e^{13} + e^{25}$                    | $1/24(15, 13, 16, 14, 18, 28, 30, 29, 31)$ | $\{\emptyset, 12345, 1289, 13678, 145679, 23679, 245678, 34589\}$                                                     |
| 94:22a | $0, 0, 0, 0, 0, e^{12}, e^{14} + e^{23}, e^{13} + e^{24}, e^{35}$                    | $1/32(19, 19, 20, 20, 22, 38, 39, 39, 42)$ | $\{\emptyset, 12345, 12349, 125789, 1278, 13567, 13679, 145689, 1468, 23568, 23689, 245679, 2467, 34578, 34789, 59\}$ |
| 94:22b | $0, 0, 0, 0, 0, e^{12}, -e^{14} + e^{23}, e^{13} + e^{24}, e^{35}$                   | $1/32(19, 19, 20, 20, 22, 38, 39, 39, 42)$ | $\{\emptyset, 12345, 12349, 125789, 1278, 13567, 13679, 145689, 1468, 23568, 23689, 245679, 2467, 34578, 34789, 59\}$ |
| 94:23  | $0, 0, 0, 0, 0, e^{12}, e^{13}, e^{15} + e^{24}, e^{14} + e^{35}$                    | $1/24(14, 14, 14, 17, 17, 28, 28, 31, 31)$ | $\{\emptyset, 12345, 12389, 14678, 15679, 234679, 235678, 4589\}$                                                     |
| 94:24  | $0, 0, 0, 0, 0, e^{12}, e^{13}, e^{25} + e^{14}, e^{23} + e^{45}$                    | $1/13(7, 8, 9, 9, 8, 15, 16, 16, 17)$      | $\{\emptyset, 12345, 1238, 13469, 135689, 24689, 2569, 458\}$                                                         |
| 94:25  | $0, 0, 0, 0, 0, e^{12}, e^{13}, e^{25} + e^{14}, e^{24} + e^{35}$                    | $1/22(12, 13, 14, 16, 15, 25, 26, 28, 29)$ | $\{\emptyset, 12345, 12389, 13469, 13568, 2468, 2569, 4589\}$                                                         |
| 94:26a | $0, 0, 0, 0, 0, e^{12}, e^{13}, e^{35} + e^{24}, e^{45} + e^{23}$                    | $1/19(11, 12, 12, 12, 12, 23, 23, 24, 24)$ | $\{\emptyset, 12345, 1238, 12479, 125789, 134689, 13569, 145678, 167, 234567, 23678, 2469, 25689, 34789, 3579, 458\}$ |
| 94:26b | $0, 0, 0, 0, 0, e^{12}, e^{13}, e^{35} - e^{24}, e^{45} + e^{23}$                    | $1/19(11, 12, 12, 12, 12, 23, 23, 24, 24)$ | $\{\emptyset, 12345, 1238, 12479, 125789, 134689, 13569, 145678, 167, 234567, 23678, 2469, 25689, 34789, 3579, 458\}$ |
| 94:27a | $0, 0, 0, 0, 0, e^{12}, e^{13}, e^{25} + e^{34}, e^{24} + e^{35}$                    | $1/11(7, 6, 6, 8, 8, 13, 13, 14, 14)$      | $\{\emptyset, 12345, 12389, 12478, 12579, 13469, 13568, 1456789, 167, 234567, 236789, 2468, 2569, 3479, 3578, 4589\}$ |
| 94:27b | $0, 0, 0, 0, 0, e^{12}, e^{13}, -e^{25} + e^{34}, e^{24} + e^{35}$                   | $1/11(7, 6, 6, 8, 8, 13, 13, 14, 14)$      | $\{\emptyset, 12345, 12389, 12478, 12579, 13469, 13568, 1456789, 167, 234567, 236789, 2468, 2569, 3479, 3578, 4589\}$ |
| 94:28  | $0, 0, 0, 0, 0, e^{12}, e^{34}, e^{15} + e^{23}, e^{25} + e^{14}$                    | $1/17(10, 10, 11, 11, 11, 20, 22, 21, 21)$ | $\{\emptyset, 12345, 1289, 13468, 1569, 23469, 2568, 34589\}$                                                         |
| 94:29  | $0, 0, 0, 0, 0, e^{12}, e^{34}, e^{15} + e^{23}, e^{13} + e^{45}$                    | $1/38(23, 24, 24, 22, 25, 47, 46, 48, 47)$ | $\{\emptyset, 12345, 124789, 13678, 1569, 23469, 245678, 35789\}$                                                     |
| 94:30  | $0, 0, 0, 0, 0, e^{12}, e^{34}, e^{15} + e^{23}, e^{35} + e^{14}$                    | $1/13(7, 9, 7, 9, 9, 16, 16, 16, 16)$      | $\{\emptyset, 12345, 12478, 136789, 1569, 23469, 2456789, 3578\}$                                                     |
| 94:31a | $0, 0, 0, 0, 0, e^{12}, e^{23} + e^{14}, e^{24} + e^{13}, e^{34} + e^{15}$           | $1/9(5, 5, 6, 6, 7, 10, 11, 11, 12)$       | $\{\emptyset, 12345, 12578, 13679, 14689, 235689, 245679, 3478\}$                                                     |
| 94:31b | $0, 0, 0, 0, 0, e^{12}, -e^{14} + e^{23}, e^{13} + e^{24}, e^{34} + e^{15}$          | $1/9(5, 5, 6, 6, 7, 10, 11, 11, 12)$       | $\{\emptyset, 12345, 12578, 13679, 14689, 235689, 245679, 3478\}$                                                     |
| 94:32a | $0, 0, 0, 0, 0, e^{14} + e^{23}, e^{24} + e^{13}, e^{34} + e^{12}, e^{15}$           | $1/33(20, 20, 20, 20, 23, 40, 40, 40, 43)$ | $\{\emptyset, 12345, 12349, 12567, 12679, 13568, 13689, 14578, 14789, 235789, 2378, 245689, 2468, 345679, 3467, 59\}$ |
| 94:32b | $0, 0, 0, 0, 0, e^{23} + e^{14}, e^{24} - e^{13}, e^{34} + e^{12}, e^{15}$           | $1/33(20, 20, 20, 20, 23, 40, 40, 40, 43)$ | $\{\emptyset, 12345, 12349, 12567, 12679, 13568, 13689, 14578, 14789, 235789, 2378, 245689, 2468, 345679, 3467, 59\}$ |
| 94:33  | $0, 0, 0, 0, 0, e^{12}, e^{13} + e^{24}, e^{15} + e^{23}, e^{14} + e^{25}$           | $1/15(8, 8, 11, 11, 11, 16, 19, 19, 19)$   | $\{\emptyset, 12345, 12789, 345789\}$                                                                                 |
| 94:34  | $0, 0, 0, 0, 0, e^{12}, e^{13} + e^{24}, e^{15} + e^{23}, e^{35} + e^{14}$           | $1/27(16, 15, 18, 19, 17, 31, 34, 33, 35)$ | $\{\emptyset, 12345, 13689, 245689\}$                                                                                 |
| 94:35a | $0, 0, 0, 0, 0, e^{12}, e^{14} + e^{23}, e^{15} + e^{34}, e^{45} + e^{13}$           | $1/39(24, 23, 25, 24, 25, 47, 48, 49, 49)$ | $\{\emptyset, 12345, 12579, 13678, 14689, 235689, 245678, 3479\}$                                                     |
| 94:35b | $0, 0, 0, 0, 0, e^{12}, e^{23} + e^{14}, -e^{15} + e^{34}, e^{13} + e^{45}$          | $1/39(24, 23, 25, 24, 25, 47, 48, 49, 49)$ | $\{\emptyset, 12345, 12579, 13678, 14689, 235689, 245678, 3479\}$                                                     |
| 94:36  | $0, 0, 0, 0, 0, e^{12}, e^{13} + e^{24}, e^{14} + e^{35}, e^{23} + e^{45}$           | $1/41(25, 25, 26, 26, 25, 50, 51, 51, 51)$ | $\{\emptyset, 12345, 125789, 34789\}$                                                                                 |
| 94:37  | $0, 0, 0, 0, 0, e^{12}, e^{13} + e^{24}, e^{34} + e^{15}, e^{45} + e^{23}$           | $1/32(18, 20, 21, 19, 22, 38, 39, 40, 41)$ | $\{\emptyset, 12345, 12579, 3479\}$                                                                                   |
| 94:38a | $0, 0, 0, 0, 0, e^{24} + e^{13}, e^{34} + e^{12}, e^{15}, e^{45} + e^{23}$           | $1/40(24, 25, 25, 24, 26, 49, 49, 50, 50)$ | $\{\emptyset, 12345, 12569, 13579, 14567, 2367, 2479, 3469\}$                                                         |
| 94:38b | $0, 0, 0, 0, 0, e^{24} - e^{13}, e^{12} + e^{34}, e^{15}, e^{23} + e^{45}$           | $1/40(24, 25, 25, 24, 26, 49, 49, 50, 50)$ | $\{\emptyset, 12345, 12569, 13579, 14567, 2367, 2479, 3469\}$                                                         |
| 94:39a | $0, 0, 0, 0, 0, e^{24} + e^{13}, e^{34} + e^{12}, e^{23} + e^{15}, e^{25} + e^{14}$  | $13/21(1, 1, 1, 1, 1, 2, 2, 2, 2)$         | $\{\emptyset, 12345, 12689, 345689\}$                                                                                 |
| 94:39b | $0, 0, 0, 0, 0, -e^{13} + e^{24}, e^{34} + e^{12}, e^{15} + e^{23}, e^{25} + e^{14}$ | $13/21(1, 1, 1, 1, 1, 2, 2, 2, 2)$         | $\{\emptyset, 12345, 12689, 345689\}$                                                                                 |
| 94:40  | $0, 0, 0, 0, 0, e^{34} + e^{12}, e^{15} + e^{23}, e^{14} + e^{25}, e^{45} + e^{13}$  | $13/21(1, 1, 1, 1, 1, 2, 2, 2, 2)$         | $\{\emptyset, 12345\}$                                                                                                |
| 9321:4 | $0, 0, 0, 0, 0, 0, e^{12}, e^{17}, e^{18} + e^{34} + e^{56}$                         | $1/39(11, 27, 30, 30, 30, 30, 38, 49, 60)$ | $\{\emptyset, 1234568, 12348, 12568, 128, 13579, 13679, 14579, 14679, 235789, 236789, 245789, 246789, 34, 3456, 56\}$ |

Table A.2 – Continued to next page

Table A.2 – Continued from previous page

| Name    | $g$                                                                             | $N$                                                  | Signatures $S$                                                                                                        |
|---------|---------------------------------------------------------------------------------|------------------------------------------------------|-----------------------------------------------------------------------------------------------------------------------|
| 9321:8  | $0, 0, 0, 0, 0, 0, e^{12}, e^{17}, e^{56} + e^{34} + e^{27} + e^{18}$           | $5/32(2, 4, 5, 5, 5, 5, 6, 8, 10)$                   | $\{\emptyset, 13579, 13679, 14579, 14679, 34, 3456, 56\}$                                                             |
| 932:10  | $0, 0, 0, 0, 0, 0, e^{12}, e^{17}, e^{56} + e^{34} + e^{27}$                    | $1/39(14, 23, 30, 30, 30, 30, 37, 51, 60)$           | $\{\emptyset, 123589, 123689, 124589, 124689, 13579, 13679, 14579, 14679, 2345678, 23478, 25678, 278, 34, 3456, 56\}$ |
| 932:11  | $0, 0, 0, 0, 0, 0, e^{12}, e^{34} + e^{17}, e^{27} + e^{56}$                    | $8/33(2, 2, 3, 3, 3, 3, 4, 6, 6)$                    | $\{\emptyset, 123589, 123689, 124589, 124689, 134579, 134679, 1579, 1679, 235678, 2378, 245678, 2478, 34, 3456, 56\}$ |
| 932:13  | $0, 0, 0, 0, 0, 0, e^{12}, e^{17} + e^{34}, e^{27} + e^{35} + e^{46}$           | $1/48(20, 26, 33, 33, 39, 39, 46, 66, 72)$           | $\{\emptyset, 123689, 124589, 13479, 15679, 23578, 24678, 3456\}$                                                     |
| 932:16  | $0, 0, 0, 0, 0, 0, e^{12}, e^{13} + e^{27}, e^{56} + e^{17} + e^{34}$           | $1/293(169, 110, 220, 228, 224, 224, 279, 389, 448)$ | $\{\emptyset, 124589, 124689, 15678, 178, 24579, 24679, 56\}$                                                         |
| 932:17  | $0, 0, 0, 0, 0, 0, e^{12}, e^{17} + e^{34}, e^{27} + e^{13} + e^{56}$           | $4/29(4, 3, 6, 5, 5, 5, 7, 11, 10)$                  | $\{123589, 123689, 134579, 134679, 235678, 2378, 34, 3456\}$                                                          |
| 932:18  | $0, 0, 0, 0, 0, 0, e^{12}, e^{17} + e^{34}, e^{15} + e^{27} + e^{36}$           | $1/81(37, 39, 49, 64, 78, 66, 76, 113, 115)$         | $\{\emptyset, 12389, 124689, 13479, 1679, 23678, 2478, 346\}$                                                         |
| 932:19a | $0, 0, 0, 0, 0, 0, e^{12}, e^{35} + e^{46} + e^{17}, e^{34} + e^{56} + e^{27}$  | $8/33(2, 2, 3, 3, 3, 3, 4, 6, 6)$                    | $\{\emptyset, 123689, 124589, 13579, 14679, 23478, 25678, 3456\}$                                                     |
| 932:19b | $0, 0, 0, 0, 0, 0, e^{12}, e^{46} - e^{35} + e^{17}, e^{56} + e^{34} + e^{27}$  | $8/33(2, 2, 3, 3, 3, 3, 4, 6, 6)$                    | $\{\emptyset, 123689, 124589, 13579, 14679, 23478, 25678, 3456\}$                                                     |
| 932:20  | $0, 0, 0, 0, 0, 0, e^{12}, e^{13} + e^{27}, e^{24} + e^{17} + e^{56}$           | $1/227(111, 100, 200, 222, 161, 161, 211, 311, 322)$ | $\{\emptyset, 12589, 12689, 15678, 178, 2579, 2679, 56\}$                                                             |
| 932:22  | $0, 0, 0, 0, 0, 0, e^{12}, e^{45} + e^{27} + e^{13}, e^{56} + e^{34} + e^{17}$  | $1/163(89, 67, 134, 111, 112, 133, 156, 223, 245)$   | $\{123589, 13478, 23679, 3456\}$                                                                                      |
| 932:23a | $0, 0, 0, 0, 0, 0, e^{12}, e^{23} + e^{17} + e^{45}, e^{13} + e^{27} + e^{46}$  | $1/51(24, 24, 48, 31, 41, 41, 48, 72, 72)$           | $\{\emptyset, 12489, 125689, 14579, 1679, 24678, 2578, 456\}$                                                         |
| 932:23b | $0, 0, 0, 0, 0, 0, e^{12}, -e^{17} + e^{45} + e^{23}, e^{27} + e^{46} + e^{13}$ | $1/51(24, 24, 48, 31, 41, 41, 48, 72, 72)$           | $\{\emptyset, 12489, 125689, 14579, 1679, 24678, 2578, 456\}$                                                         |
| 932:24  | $0, 0, 0, 0, 0, 0, e^{12}, e^{17} + e^{35} + e^{24}, e^{27} + e^{46} + e^{13}$  | $8/17(1, 1, 2, 2, 1, 1, 2, 3, 3)$                    | $\{123489, 134579, 234678, 3456\}$                                                                                    |
| 931:22  | $0, 0, 0, 0, 0, 0, e^{12}, e^{35} + e^{46}, e^{34} + e^{17}$                    | $1/39(14, 26, 27, 27, 30, 30, 40, 57, 54)$           | $\{\emptyset, 12359, 123689, 124589, 12469, 134567, 13478, 15678, 17, 23579, 236789, 245789, 24679, 3456, 348, 568\}$ |
| 931:30  | $0, 0, 0, 0, 0, 0, e^{12}, e^{34}, e^{46} + e^{35} + e^{17}$                    | $1/24(10, 16, 15, 15, 21, 21, 26, 30, 36)$           | $\{\emptyset, 12349, 123689, 124589, 12569, 134567, 13578, 14678, 17, 23479, 236789, 245789, 25679, 3456, 358, 468\}$ |
| 931:31  | $0, 0, 0, 0, 0, 0, e^{12}, e^{13} + e^{45}, e^{36} + e^{17}$                    | $1/11(5, 7, 9, 7, 7, 8, 12, 14, 17)$                 | $\{123489, 123589, 124569, 1269, 134678, 135678, 1457, 17, 234579, 2379, 246789, 256789, 3456, 36, 48, 58\}$          |
| 931:32  | $0, 0, 0, 0, 0, 0, e^{12}, e^{35} + e^{14}, e^{36} + e^{17}$                    | $1/19(7, 13, 11, 18, 14, 16, 20, 25, 27)$            | $\{\emptyset, 123459, 12389, 12469, 125689, 134567, 13678, 147, 1578, 234789, 23579, 2456789, 2679, 3468, 356, 458\}$ |
| 931:33  | $0, 0, 0, 0, 0, 0, e^{12}, e^{45} + e^{13}, e^{27} + e^{36}$                    | $2/47(15, 10, 17, 16, 16, 18, 25, 32, 35)$           | $\{\emptyset, 123459, 1239, 124689, 125689, 134579, 1379, 146789, 156789, 234678, 235678, 2457, 27, 3468, 3568, 45\}$ |
| 931:34  | $0, 0, 0, 0, 0, 0, e^{12}, e^{14} + e^{35}, e^{36} + e^{27}$                    | $1/18(10, 8, 11, 15, 14, 15, 18, 25, 26)$            | $\{\emptyset, 123459, 12389, 12469, 125689, 134579, 13789, 14679, 156789, 234678, 23567, 24578, 27, 3468, 356, 458\}$ |
| 931:35  | $0, 0, 0, 0, 0, 0, e^{12}, e^{56} + e^{13} + e^{24}, e^{17}$                    | $1/41(16, 23, 42, 35, 29, 29, 39, 58, 55)$           | $\{123589, 123689, 124569, 1249, 134578, 134678, 1567, 17, 2345679, 23479, 25789, 26789, 3, 356, 458, 468\}$          |
| 931:36  | $0, 0, 0, 0, 0, 0, e^{12}, e^{56} + e^{34}, e^{27} + e^{13}$                    | $1/47(30, 17, 34, 36, 35, 35, 47, 70, 64)$           | $\{\emptyset, 124589, 124689, 12569, 129, 145789, 146789, 15679, 179, 24578, 24678, 2567, 27, 458, 468, 56\}$         |
| 931:37a | $0, 0, 0, 0, 0, 0, e^{12}, e^{34} + e^{56}, e^{35} + e^{46} + e^{17}$           | $1/21(8, 14, 15, 15, 15, 15, 22, 30, 30)$            | $\{\emptyset, 12349, 123689, 124589, 12569, 134567, 13578, 14678, 17, 23479, 236789, 245789, 25679, 3456, 358, 468\}$ |
| 931:37b | $0, 0, 0, 0, 0, 0, e^{12}, e^{56} - e^{34}, e^{17} + e^{46} + e^{35}$           | $1/21(8, 14, 15, 15, 15, 15, 22, 30, 30)$            | $\{\emptyset, 12349, 123689, 124589, 12569, 134567, 13578, 14678, 17, 23479, 236789, 245789, 25679, 3456, 358, 468\}$ |
| 931:42  | $0, 0, 0, 0, 0, 0, e^{12}, e^{13}, e^{17} + e^{34} + e^{56}$                    | $1/31(13, 22, 22, 26, 24, 24, 35, 35, 48)$           | $\{\emptyset, 12359, 12369, 124589, 124689, 134567, 1347, 15678, 178, 235789, 236789, 24579, 24679, 34568, 348, 56\}$ |
| 931:43  | $0, 0, 0, 0, 0, 0, e^{12}, e^{13}, e^{56} + e^{34} + e^{27}$                    | $1/68(36, 35, 46, 60, 53, 53, 71, 82, 106)$          | $\{\emptyset, 12359, 12369, 124589, 124689, 13579, 13679, 145789, 146789, 2345678, 23478, 2567, 27, 34568, 348, 56\}$ |
| 931:44  | $0, 0, 0, 0, 0, 0, e^{12}, e^{24} + e^{13}, e^{56} + e^{17}$                    | $1/68(31, 38, 60, 53, 50, 50, 69, 91, 100)$          | $\{\emptyset, 123459, 123469, 12589, 12689, 13567, 137, 145678, 1478, 235789, 236789, 24579, 24679, 34568, 348, 56\}$ |
| 931:45  | $0, 0, 0, 0, 0, 0, e^{12}, e^{34}, e^{27} + e^{56} + e^{13}$                    | $1/11(8, 4, 8, 7, 8, 8, 12, 15, 16)$                 | $\{123459, 123469, 123589, 123689, 134579, 134679, 135789, 136789, 234567, 2347, 235678, 2378, 34, 3456, 3568, 38\}$  |
| 931:46  | $0, 0, 0, 0, 0, 0, e^{12}, e^{34}, e^{15} + e^{27} + e^{36}$                    | $1/27(16, 12, 16, 19, 24, 24, 28, 35, 40)$           | $\{\emptyset, 12349, 12389, 124689, 1269, 13479, 13789, 146789, 1679, 23467, 23678, 2478, 27, 346, 368, 48\}$         |

Table A.2 – Continued to next page

Table A.2 – Continued from previous page

| Name    | $g$                                                                            | $N$                                                  | Signatures $S$                                                                                                                                                                                                        |
|---------|--------------------------------------------------------------------------------|------------------------------------------------------|-----------------------------------------------------------------------------------------------------------------------------------------------------------------------------------------------------------------------|
| 931:47  | $0, 0, 0, 0, 0, 0, e^{12}, e^{45} + e^{13}, e^{16} + e^{27}$                   | $1/27(14, 12, 24, 19, 19, 24, 26, 38, 38)$           | $\{0, 123459, 1239, 12489, 12589, 134579, 1379, 14789, 15789, 23478, 23578, 2457, 27, 348, 358, 45\}$                                                                                                                 |
| 931:48  | $0, 0, 0, 0, 0, 0, e^{12}, e^{13} + e^{45}, e^{17} + e^{26}$                   | $1/19(8, 11, 18, 13, 13, 16, 19, 26, 27)$            | $\{0, 123459, 1239, 12489, 12589, 13457, 137, 1478, 1578, 234789, 235789, 24579, 279, 348, 358, 45\}$                                                                                                                 |
| 931:51  | $0, 0, 0, 0, 0, 0, e^{12}, e^{13} + e^{45}, e^{17} + e^{56} + e^{34}$          | $1/83(34, 56, 71, 53, 52, 72, 90, 105, 124)$         | $\{0, 12369, 124689, 134567, 15678, 235789, 24579, 348\}$                                                                                                                                                             |
| 931:52  | $0, 0, 0, 0, 0, 0, e^{12}, e^{13} + e^{45}, e^{56} + e^{34} + e^{27}$          | $1/297(170, 136, 231, 211, 190, 252, 306, 401, 442)$ | $\{0, 12369, 124689, 13679, 146789, 23478, 27, 348\}$                                                                                                                                                                 |
| 931:53  | $0, 0, 0, 0, 0, 0, e^{12}, e^{24} + e^{13} + e^{56}, e^{34} + e^{17}$          | $2/43(10, 13, 18, 15, 14, 14, 23, 28, 33)$           | $\{123589, 123689, 124569, 1249, 134578, 134678, 1567, 17\}$                                                                                                                                                          |
| 931:54  | $0, 0, 0, 0, 0, 0, e^{12}, e^{46} + e^{13} + e^{25}, e^{17} + e^{34}$          | $1/17(8, 9, 15, 10, 14, 13, 17, 23, 25)$             | $\{123689, 124569, 134578, 17, 23579, 24789, 346, 568\}$                                                                                                                                                              |
| 931:55  | $0, 0, 0, 0, 0, 0, e^{12}, e^{15} + e^{46} + e^{23}, e^{17} + e^{34}$          | $1/227(91, 137, 176, 143, 222, 170, 228, 313, 319)$  | $\{0, 12359, 12489, 13478, 157, 2379, 245789, 3458\}$                                                                                                                                                                 |
| 931:56  | $0, 0, 0, 0, 0, 0, e^{12}, e^{34} + e^{56}, e^{27} + e^{45} + e^{13}$          | $1/293(190, 110, 220, 207, 203, 224, 300, 427, 410)$ | $\{0, 124689, 12569, 146789, 15679, 24578, 27, 458\}$                                                                                                                                                                 |
| 931:58  | $0, 0, 0, 0, 0, 0, e^{12}, e^{13}, e^{17} + e^{24} + e^{56}$                   | $1/37(16, 24, 29, 32, 28, 28, 40, 45, 56)$           | $\{0, 12359, 12369, 12589, 12689, 13567, 137, 15678, 178, 235789, 236789, 2579, 2679, 3568, 38, 56\}$                                                                                                                 |
| 931:61  | $0, 0, 0, 0, 0, 0, e^{12}, e^{24} + e^{13}, e^{56} + e^{34} + e^{17}$          | $1/21(10, 12, 17, 15, 16, 16, 22, 27, 32)$           | $\{0, 235789, 236789, 24579, 24679, 34568, 348, 56\}$                                                                                                                                                                 |
| 931:62  | $0, 0, 0, 0, 0, 0, e^{12}, e^{13} + e^{24}, e^{46} + e^{35} + e^{17}$          | $1/59(29, 33, 44, 40, 47, 51, 62, 73, 91)$           | $\{0, 12349, 125689, 1357, 14678, 236789, 24579, 34568\}$                                                                                                                                                             |
| 931:63  | $0, 0, 0, 0, 0, 0, e^{12}, e^{45} + e^{13}, e^{27} + e^{36} + e^{14}$          | $2/43(15, 8, 15, 16, 14, 16, 23, 30, 31)$            | $\{123459, 124689, 134579, 146789, 234678, 2457, 3468, 45\}$                                                                                                                                                          |
| 931:64  | $0, 0, 0, 0, 0, 0, e^{12}, e^{13} + e^{45}, e^{16} + e^{27} + e^{34}$          | $1/11(6, 5, 9, 7, 8, 10, 11, 15, 16)$                | $\{0, 1239, 12489, 1379, 14789, 23478, 27, 348\}$                                                                                                                                                                     |
| 931:65  | $0, 0, 0, 0, 0, 0, e^{12}, e^{45} + e^{13}, e^{23} + e^{17} + e^{46}$          | $1/227(99, 137, 198, 135, 162, 200, 236, 297, 335)$  | $\{0, 12489, 125689, 14678, 1578, 24579, 2679, 456\}$                                                                                                                                                                 |
| 931:66  | $0, 0, 0, 0, 0, 0, e^{12}, e^{45} + e^{13}, e^{17} + e^{36} + e^{24}$          | $1/8(3, 6, 7, 6, 4, 5, 9, 10, 12)$                   | $\{123489, 124569, 134678, 1457, 234579, 246789, 3456, 48\}$                                                                                                                                                          |
| 931:67  | $0, 0, 0, 0, 0, 0, e^{12}, e^{13} + e^{45}, e^{17} + e^{26} + e^{34}$          | $1/227(100, 135, 198, 137, 161, 200, 235, 298, 335)$ | $\{0, 1239, 12489, 13457, 1578, 235789, 24579, 348\}$                                                                                                                                                                 |
| 931:68  | $0, 0, 0, 0, 0, 0, e^{12}, e^{34} + e^{15}, e^{46} + e^{27} + e^{13}$          | $1/17(10, 7, 14, 10, 14, 14, 17, 24, 24)$            | $\{123459, 123689, 134579, 136789, 23467, 23578, 346, 358\}$                                                                                                                                                          |
| 931:70  | $0, 0, 0, 0, 0, 0, e^{12}, e^{56} + e^{14} + e^{23}, e^{13} + e^{27}$          | $1/26(13, 12, 24, 23, 18, 18, 25, 36, 37)$           | $\{124569, 1249, 15789, 16789, 2567, 27, 458, 468\}$                                                                                                                                                                  |
| 931:71  | $0, 0, 0, 0, 0, 0, e^{12}, e^{36} + e^{25} + e^{14}, e^{27} + e^{13}$          | $1/19(11, 7, 14, 16, 20, 13, 18, 27, 25)$            | $\{123469, 123589, 1345679, 13789, 234578, 2367, 348, 356\}$                                                                                                                                                          |
| 931:72  | $0, 0, 0, 0, 0, 0, e^{12}, e^{46} + e^{13} + e^{25}, e^{17} + e^{56} + e^{34}$ | $1/461(216, 257, 401, 288, 360, 329, 473, 617, 689)$ | $\{123689, 17, 23579, 568\}$                                                                                                                                                                                          |
| 931:73  | $0, 0, 0, 0, 0, 0, e^{12}, e^{13} + e^{24}, e^{36} + e^{15} + e^{27}$          | $1/29(17, 13, 20, 24, 26, 23, 30, 37, 43)$           | $\{0, 12349, 12689, 1379, 146789, 23678, 247, 3468\}$                                                                                                                                                                 |
| 931:74  | $0, 0, 0, 0, 0, 0, e^{12}, e^{13} + e^{24}, e^{17} + e^{23} + e^{56}$          | $1/67(30, 38, 60, 52, 49, 49, 68, 90, 98)$           | $\{123459, 123469, 13567, 137, 235789, 236789, 34568, 348\}$                                                                                                                                                          |
| 931:77  | $0, 0, 0, 0, 0, 0, e^{12}, e^{14} + e^{25} + e^{36}, e^{13} + e^{45} + e^{27}$ | $2/31(11, 6, 12, 9, 14, 8, 17, 20, 23)$              | $\{123469, 123589, 234578, 2367\}$                                                                                                                                                                                    |
| 931:79  | $0, 0, 0, 0, 0, 0, e^{12}, e^{16} + e^{24} + e^{35}, e^{13} + e^{27} + e^{45}$ | $1/14(8, 6, 12, 13, 7, 11, 14, 19, 20)$              | $\{123489, 123569, 345, 368\}$                                                                                                                                                                                        |
| 931:89a | $0, 0, 0, 0, 0, 0, e^{12}, e^{13}, e^{38} + e^{27} + e^{56} + e^{14}$          | $5/19(2, 2, 2, 4, 3, 3, 4, 4, 6)$                    | $\{123459, 123469, 124589, 124689, 134579, 134679, 145789, 146789, 2345678, 23478, 24567, 247, 34568, 348, 4, 456\}$                                                                                                  |
| 931:89b | $0, 0, 0, 0, 0, 0, -e^{12}, e^{13}, e^{56} + e^{27} + e^{38} + e^{14}$         | $5/19(2, 2, 2, 4, 3, 3, 4, 4, 6)$                    | $\{123459, 123469, 124589, 124689, 134579, 134679, 145789, 146789, 2345678, 23478, 24567, 247, 34568, 348, 4, 456\}$                                                                                                  |
| 931:90  | $0, 0, 0, 0, 0, 0, e^{12}, e^{13}, e^{38} + e^{17} + e^{24} + e^{56}$          | $5/44(4, 6, 5, 8, 7, 7, 10, 9, 14)$                  | $\{0, 12359, 12369, 12589, 12689, 3568, 38, 56\}$                                                                                                                                                                     |
| 931:96  | $0, 0, 0, 0, 0, 0, e^{12}, e^{34}, e^{17} + e^{56} + e^{38}$                   | $1/15(7, 10, 7, 10, 12, 12, 17, 17, 24)$             | $\{0, 123459, 123469, 124589, 124689, 135678, 1378, 1567, 17, 234579, 234679, 245789, 246789, 3568, 38, 56\}$                                                                                                         |
| 931:102 | $0, 0, 0, 0, 0, 0, e^{12}, e^{34}, e^{48} + e^{56} + e^{27} + e^{13}$          | $5/13(2, 1, 2, 1, 2, 2, 3, 3, 4)$                    | $\{123459, 123469, 123589, 123689, 134579, 134679, 135789, 136789\}$                                                                                                                                                  |
| 931:103 | $0, 0, 0, 0, 0, 0, e^{12}, e^{34}, e^{36} + e^{48} + e^{15} + e^{27}$          | $5/32(4, 3, 4, 3, 6, 6, 7, 7, 10)$                   | $\{0, 12349, 12389, 13479, 13789, 2478, 27, 48\}$                                                                                                                                                                     |
| 93:22   | $0, 0, 0, 0, 0, 0, e^{12}, e^{13}, e^{14} + e^{56}$                            | $1/13(6, 10, 10, 12, 9, 9, 16, 16, 18)$              | $\{0, 1234, 123456, 12359, 12369, 124568, 1248, 12589, 12689, 134567, 1347, 13579, 13679, 145678, 1478, 15789, 16789, 2345789, 2346789, 235678, 2378, 24579, 24679, 2567, 27, 34589, 34689, 3568, 38, 459, 469, 56\}$ |
| 93:23   | $0, 0, 0, 0, 0, 0, e^{12}, e^{13}, e^{56} + e^{24}$                            | $1/11(6, 7, 8, 9, 8, 8, 13, 14, 16)$                 | $\{0, 1234, 123456, 12359, 12369, 124568, 1248, 12589, 12689, 134579, 134679, 13567, 137, 145789, 146789, 15678, 178, 2345678, 23478, 235789, 236789, 24567, 247, 2579, 2679, 34589, 34689, 3568, 38, 459, 469, 56\}$ |

Table A.2 – Continued to next page

Table A.2 – Continued from previous page

| Name   | $g$                                                                    | $N$                                        | Signatures $S$                                                                                                                                                                                                                |
|--------|------------------------------------------------------------------------|--------------------------------------------|-------------------------------------------------------------------------------------------------------------------------------------------------------------------------------------------------------------------------------|
| 93:26  | $0, 0, 0, 0, 0, 0, e^{12}, e^{34}, e^{15} + e^{36}$                    | $1/11(6, 8, 6, 8, 9, 9, 14, 14, 15)$       | $\{\emptyset, 123456, 12349, 123568, 12389, 12458, 124689, 125, 1269, 134567, 13479, 135678, 13789, 14578, 146789, 157, 1679, 234579, 23467, 235789, 23678, 2456789, 2478, 25679, 27, 3459, 346, 3589, 368, 45689, 48, 569\}$ |
| 93:27  | $0, 0, 0, 0, 0, 0, e^{12}, e^{13}, e^{14} + e^{23} + e^{56}$           | $1/14(7, 10, 10, 13, 10, 10, 17, 17, 20)$  | $\{\emptyset, 1234, 123456, 12589, 12689, 13579, 13679, 145678, 1478, 235678, 2378, 24579, 24679, 34589, 34689, 56\}$                                                                                                         |
| 93:28  | $0, 0, 0, 0, 0, 0, e^{12}, e^{13}, e^{36} + e^{25} + e^{14}$           | $1/11(6, 7, 7, 10, 9, 9, 13, 13, 16)$      | $\{\emptyset, 123456, 1239, 12458, 12689, 13467, 13579, 1478, 156789, 234789, 235678, 24679, 257, 34589, 368, 4569\}$                                                                                                         |
| 93:29  | $0, 0, 0, 0, 0, 0, e^{12}, e^{24} + e^{13}, e^{26} + e^{15}$           | $3/11(2, 2, 3, 3, 3, 3, 4, 5, 5)$          | $\{\emptyset, 123456, 12349, 12568, 1289, 1357, 13679, 14578, 146789, 235789, 23678, 24579, 2467, 345689, 348, 569\}$                                                                                                         |
| 93:30  | $0, 0, 0, 0, 0, 0, e^{12}, e^{14} + e^{23}, e^{13} + e^{56}$           | $1/31(18, 19, 24, 25, 21, 21, 37, 43, 42)$ | $\{\emptyset, 1234, 123456, 12589, 12689, 135678, 1378, 14579, 14679, 23579, 23679, 245678, 2478, 34589, 34689, 56\}$                                                                                                         |
| 93:31  | $0, 0, 0, 0, 0, 0, e^{12}, e^{24} + e^{13}, e^{36} + e^{15}$           | $1/23(14, 13, 16, 17, 19, 17, 27, 30, 33)$ | $\{\emptyset, 123456, 12349, 1258, 12689, 13567, 1379, 14578, 146789, 235789, 23678, 245679, 247, 34589, 3468, 569\}$                                                                                                         |
| 93:32  | $0, 0, 0, 0, 0, 0, e^{12}, e^{23} + e^{14}, e^{15} + e^{36}$           | $1/16(8, 11, 10, 13, 14, 12, 19, 21, 22)$  | $\{\emptyset, 123456, 12349, 1258, 12689, 135678, 13789, 1457, 14679, 23579, 2367, 2456789, 2478, 34589, 3468, 569\}$                                                                                                         |
| 93:34  | $0, 0, 0, 0, 0, 0, e^{12}, e^{34}, e^{25} + e^{46} + e^{13}$           | $1/23(16, 13, 16, 13, 19, 19, 29, 29, 32)$ | $\{\emptyset, 123456, 12358, 12489, 1269, 13467, 1378, 145789, 15679, 23479, 236789, 245678, 257, 3459, 35689, 468\}$                                                                                                         |
| 93:35  | $0, 0, 0, 0, 0, 0, e^{12}, e^{24} + e^{13}, e^{56} + e^{34}$           | $1/31(19, 19, 22, 22, 22, 22, 38, 41, 44)$ | $\{\emptyset, 1234, 123456, 12568, 128, 13579, 13679, 145789, 146789, 235789, 236789, 24579, 24679, 34568, 348, 56\}$                                                                                                         |
| 93:36  | $0, 0, 0, 0, 0, 0, e^{12}, e^{24} + e^{13}, e^{35} + e^{46}$           | $1/37(23, 23, 24, 24, 29, 29, 46, 47, 53)$ | $\{\emptyset, 123456, 12349, 125689, 128, 1357, 13679, 145789, 14678, 23578, 236789, 24579, 2467, 34568, 3489, 569\}$                                                                                                         |
| 93:39  | $0, 0, 0, 0, 0, 0, e^{12}, e^{34} + e^{15}, e^{13} + e^{46}$           | $1/23(12, 17, 18, 13, 19, 17, 29, 31, 30)$ | $\{\emptyset, 123456, 1238, 12489, 12569, 134567, 1378, 14789, 15679, 23479, 2356789, 245678, 27, 349, 35689, 4568\}$                                                                                                         |
| 93:40  | $0, 0, 0, 0, 0, 0, e^{12}, e^{13} + e^{45}, e^{23} + e^{46}$           | $1/37(23, 23, 27, 21, 29, 29, 46, 50, 50)$ | $\{\emptyset, 123, 123456, 12489, 125689, 134579, 13679, 14678, 1578, 234678, 23578, 24579, 2679, 3489, 35689, 456\}$                                                                                                         |
| 93:42  | $0, 0, 0, 0, 0, 0, e^{12}, e^{15} + e^{34}, e^{46} + e^{23}$           | $1/37(21, 24, 27, 23, 29, 28, 45, 50, 51)$ | $\{\emptyset, 123456, 1238, 12489, 12569, 134579, 136789, 14678, 157, 23467, 23578, 245789, 2679, 349, 35689, 4568\}$                                                                                                         |
| 93:43  | $0, 0, 0, 0, 0, 0, e^{34} + e^{12}, e^{15}, e^{46} + e^{23}$           | $1/31(18, 22, 21, 19, 22, 24, 40, 40, 43)$ | $\{\emptyset, 123456, 123468, 12569, 12689, 135679, 136789, 14567, 14678, 23578, 237, 245789, 2479, 34589, 349, 58\}$                                                                                                         |
| 93:44a | $0, 0, 0, 0, 0, 0, e^{12}, e^{24} + e^{13}, e^{56} + e^{14} + e^{23}$  | $1/32(19, 19, 25, 25, 22, 22, 38, 44, 44)$ | $\{\emptyset, 1234, 123456, 12589, 12689, 13579, 13679, 145678, 1478, 235678, 2378, 24579, 24679, 34589, 34689, 56\}$                                                                                                         |
| 93:44b | $0, 0, 0, 0, 0, 0, e^{12}, e^{24} - e^{13}, e^{56} + e^{23} + e^{14}$  | $1/32(19, 19, 25, 25, 22, 22, 38, 44, 44)$ | $\{\emptyset, 1234, 123456, 12589, 12689, 13579, 13679, 145678, 1478, 235678, 2378, 24579, 24679, 34589, 34689, 56\}$                                                                                                         |
| 93:45  | $0, 0, 0, 0, 0, 0, e^{12}, e^{13} + e^{24}, e^{15} + e^{46} + e^{23}$  | $1/17(9, 11, 13, 11, 15, 13, 20, 22, 24)$  | $\{\emptyset, 123456, 12689, 13679, 145678, 2378, 24579, 34589\}$                                                                                                                                                             |
| 93:46  | $0, 0, 0, 0, 0, 0, e^{12}, e^{13} + e^{24}, e^{26} + e^{34} + e^{15}$  | $1/7(4, 4, 5, 5, 6, 6, 8, 9, 10)$          | $\{\emptyset, 123456, 12568, 13679, 146789, 235789, 24579, 348\}$                                                                                                                                                             |
| 93:48a | $0, 0, 0, 0, 0, 0, e^{24} + e^{13}, e^{34} + e^{12}, e^{26} + e^{15}$  | $3/19(4, 4, 4, 4, 5, 5, 8, 8, 9)$          | $\{\emptyset, 123456, 12349, 12567, 1279, 1358, 13689, 14578, 146789, 235789, 23678, 24589, 2468, 345679, 347, 569\}$                                                                                                         |
| 93:48b | $0, 0, 0, 0, 0, 0, -e^{13} + e^{24}, e^{34} + e^{12}, e^{26} + e^{15}$ | $3/19(4, 4, 4, 4, 5, 5, 8, 8, 9)$          | $\{\emptyset, 123456, 12349, 12567, 1279, 1358, 13689, 14578, 146789, 235789, 23678, 24589, 2468, 345679, 347, 569\}$                                                                                                         |
| 93:49a | $0, 0, 0, 0, 0, 0, e^{14} + e^{23}, e^{24} + e^{13}, e^{15} + e^{26}$  | $1/11(6, 6, 8, 8, 9, 9, 14, 14, 15)$       | $\{\emptyset, 123456, 12349, 125678, 12789, 1357, 13679, 1458, 14689, 23589, 2368, 24579, 2467, 3456789, 3478, 569\}$                                                                                                         |
| 93:49b | $0, 0, 0, 0, 0, 0, e^{23} - e^{14}, e^{24} + e^{13}, e^{15} + e^{26}$  | $1/11(6, 6, 8, 8, 9, 9, 14, 14, 15)$       | $\{\emptyset, 123456, 12349, 125678, 12789, 1357, 13679, 1458, 14689, 23589, 2368, 24579, 2467, 3456789, 3478, 569\}$                                                                                                         |
| 93:51  | $0, 0, 0, 0, 0, 0, e^{14} + e^{23}, e^{13} + e^{25}, e^{46} + e^{12}$  | $1/63(44, 38, 43, 37, 49, 45, 81, 87, 82)$ | $\{\emptyset, 123456, 1278, 13679, 14589, 23689, 24579, 345678\}$                                                                                                                                                             |
| 93:52  | $0, 0, 0, 0, 0, 0, e^{34} + e^{12}, e^{13} + e^{25}, e^{26} + e^{14}$  | $3/38(9, 7, 8, 8, 10, 10, 16, 17, 17)$     | $\{\emptyset, 123456, 1289, 13679, 14578, 23678, 24579, 345689\}$                                                                                                                                                             |
| 93:54  | $0, 0, 0, 0, 0, 0, e^{13} + e^{24}, e^{15} + e^{23}, e^{14} + e^{26}$  | $1/13(7, 7, 10, 10, 10, 10, 17, 17, 17)$   | $\{\emptyset, 123456, 12789, 13689, 1457, 2367, 24589, 3456789\}$                                                                                                                                                             |

Table A.2 – Continued to next page

Table A.2 – Continued from previous page

| Name   | $g$                                                                                      | $N$                                                  | Signatures $S$                                                                                                                                                                                                                |
|--------|------------------------------------------------------------------------------------------|------------------------------------------------------|-------------------------------------------------------------------------------------------------------------------------------------------------------------------------------------------------------------------------------|
| 93:55  | $0, 0, 0, 0, 0, 0, e^{12}, e^{13} + e^{45}, e^{56} + e^{14} + e^{23}$                    | $1/38(23, 24, 28, 29, 22, 30, 47, 51, 52)$           | $\{\emptyset, 123456, 12589, 13679, 1478, 235678, 24579, 34689\}$                                                                                                                                                             |
| 93:57a | $0, 0, 0, 0, 0, 0, e^{12}, e^{13} + e^{45}, e^{14} + e^{26} + e^{35}$                    | $1/19(12, 11, 14, 14, 12, 15, 23, 26, 26)$           | $\{\emptyset, 123456, 1239, 12468, 12589, 13457, 13679, 1478, 156789, 234789, 235678, 24579, 267, 34689, 358, 4569\}$                                                                                                         |
| 93:57b | $0, 0, 0, 0, 0, 0, e^{12}, e^{45} - e^{13}, e^{35} + e^{26} + e^{14}$                    | $1/19(12, 11, 14, 14, 12, 15, 23, 26, 26)$           | $\{\emptyset, 123456, 1239, 12468, 12589, 13457, 13679, 1478, 156789, 234789, 235678, 24579, 267, 34689, 358, 4569\}$                                                                                                         |
| 93:58  | $0, 0, 0, 0, 0, 0, e^{12}, e^{13} + e^{45}, e^{35} + e^{24} + e^{16}$                    | $1/13(7, 9, 10, 9, 8, 11, 16, 17, 18)$               | $\{\emptyset, 123456, 1239, 12468, 12589, 34689, 358, 4569\}$                                                                                                                                                                 |
| 93:59  | $0, 0, 0, 0, 0, 0, e^{24} + e^{13}, e^{35} + e^{12}, e^{56} + e^{14}$                    | $1/112(72, 73, 79, 78, 66, 84, 151, 145, 150)$       | $\{\emptyset, 123456, 12679, 13689, 145678, 2378, 24589, 34579\}$                                                                                                                                                             |
| 93:60  | $0, 0, 0, 0, 0, 0, e^{12} + e^{34}, e^{15} + e^{23}, e^{14} + e^{56}$                    | $1/79(52, 53, 49, 56, 50, 58, 105, 102, 108)$        | $\{\emptyset, 123456, 12689, 136789, 14567, 237, 245789, 34589\}$                                                                                                                                                             |
| 93:62  | $0, 0, 0, 0, 0, 0, e^{14} + e^{23}, e^{35} + e^{12}, e^{16} + e^{45}$                    | $1/29(17, 20, 18, 21, 19, 23, 38, 37, 40)$           | $\{\emptyset, 123456, 1267, 13678, 14568, 238, 24578, 3457\}$                                                                                                                                                                 |
| 93:63  | $0, 0, 0, 0, 0, 0, e^{12}, e^{34} + e^{56}, e^{25} + e^{13} + e^{46}$                    | $1/79(50, 50, 56, 53, 56, 53, 100, 109, 106)$        | $\{\emptyset, 123456, 12358, 145789, 15679, 23479, 236789, 468\}$                                                                                                                                                             |
| 93:64a | $0, 0, 0, 0, 0, 0, e^{24} + e^{13}, e^{15} + e^{26}, e^{34} + e^{56}$                    | $2/3(1, 1, 1, 1, 1, 2, 2, 2)$                        | $\{\emptyset, 123456, 12348, 12567, 1278, 1359, 13689, 14579, 146789, 235789, 23679, 24589, 2469, 345678, 347, 568\}$                                                                                                         |
| 93:64b | $0, 0, 0, 0, 0, 0, e^{24} - e^{13}, e^{26} + e^{15}, e^{56} + e^{34}$                    | $2/3(1, 1, 1, 1, 1, 2, 2, 2)$                        | $\{\emptyset, 123456, 12348, 12567, 1278, 1359, 13689, 14579, 146789, 235789, 23679, 24589, 2469, 345678, 347, 568\}$                                                                                                         |
| 93:65a | $0, 0, 0, 0, 0, 0, e^{13} + e^{24}, e^{26} + e^{15}, e^{46} + e^{35}$                    | $2/3(1, 1, 1, 1, 1, 2, 2, 2)$                        | $\{\emptyset, 123456, 123489, 125679, 1278, 135, 13689, 14579, 14678, 23578, 23679, 24589, 246, 345678, 3479, 5689\}$                                                                                                         |
| 93:65b | $0, 0, 0, 0, 0, 0, e^{24} - e^{13}, e^{26} + e^{15}, e^{35} + e^{46}$                    | $2/3(1, 1, 1, 1, 1, 2, 2, 2)$                        | $\{\emptyset, 123456, 123489, 125679, 1278, 135, 13689, 14579, 14678, 23578, 23679, 24589, 246, 345678, 3479, 5689\}$                                                                                                         |
| 93:68a | $0, 0, 0, 0, 0, 0, e^{24} + e^{13}, e^{34} + e^{12}, e^{46} + e^{15} + e^{23}$           | $1/23(13, 16, 16, 13, 19, 19, 29, 29, 32)$           | $\{\emptyset, 123456, 12679, 13689, 145678, 2378, 24589, 34579\}$                                                                                                                                                             |
| 93:68b | $0, 0, 0, 0, 0, 0, e^{24} - e^{13}, e^{12} + e^{34}, e^{15} + e^{23} + e^{46}$           | $1/23(13, 16, 16, 13, 19, 19, 29, 29, 32)$           | $\{\emptyset, 123456, 12679, 13689, 145678, 2378, 24589, 34579\}$                                                                                                                                                             |
| 93:69a | $0, 0, 0, 0, 0, 0, e^{13} + e^{24}, e^{12} + e^{35}, e^{14} + e^{56} + e^{23}$           | $1/113(73, 73, 79, 79, 67, 85, 152, 146, 152)$       | $\{\emptyset, 123456, 12679, 13689, 145678, 2378, 24589, 34579\}$                                                                                                                                                             |
| 93:69b | $0, 0, 0, 0, 0, 0, -e^{13} + e^{24}, e^{35} + e^{12}, e^{14} + e^{23} + e^{56}$          | $1/113(73, 73, 79, 79, 67, 85, 152, 146, 152)$       | $\{\emptyset, 123456, 12679, 13689, 145678, 2378, 24589, 34579\}$                                                                                                                                                             |
| 93:70  | $0, 0, 0, 0, 0, 0, e^{24} + e^{13}, e^{35} + e^{12}, e^{36} + e^{25} + e^{14}$           | $1/41(29, 25, 23, 27, 31, 33, 52, 54, 56)$           | $\{\emptyset, 123456, 12679, 34579\}$                                                                                                                                                                                         |
| 93:73  | $0, 0, 0, 0, 0, 0, e^{12}, e^{15} + e^{46} + e^{23}, e^{56} + e^{13} + e^{24}$           | $1/41(25, 25, 31, 31, 31, 25, 50, 56, 56)$           | $\{\emptyset, 123456, 12689, 34589\}$                                                                                                                                                                                         |
| 93:75  | $0, 0, 0, 0, 0, 0, e^{24} + e^{13}, e^{12} + e^{56}, e^{15} + e^{23} + e^{46}$           | $1/401(265, 259, 277, 283, 271, 253, 542, 524, 536)$ | $\{\emptyset, 123456, 13689, 24589\}$                                                                                                                                                                                         |
| 93:76a | $0, 0, 0, 0, 0, 0, e^{24} + e^{13}, e^{56} + e^{12}, e^{34} + e^{26} + e^{15}$           | $2/3(1, 1, 1, 1, 1, 2, 2, 2)$                        | $\{\emptyset, 123456, 12567, 13689, 146789, 235789, 24589, 347\}$                                                                                                                                                             |
| 93:76b | $0, 0, 0, 0, 0, 0, e^{13} + e^{24}, e^{56} - e^{12}, e^{26} + e^{34} + e^{15}$           | $2/3(1, 1, 1, 1, 1, 2, 2, 2)$                        | $\{\emptyset, 123456, 12567, 13689, 146789, 235789, 24589, 347\}$                                                                                                                                                             |
| 93:78a | $0, 0, 0, 0, 0, 0, e^{13} + e^{24}, e^{26} + e^{15}, e^{14} + e^{23} + e^{56}$           | $1/43(26, 26, 32, 32, 29, 29, 58, 55, 58)$           | $\{\emptyset, 123456, 12348, 1359, 13689, 24589, 2469, 568\}$                                                                                                                                                                 |
| 93:78b | $0, 0, 0, 0, 0, 0, e^{24} - e^{13}, e^{15} + e^{26}, e^{14} + e^{23} + e^{56}$           | $1/43(26, 26, 32, 32, 29, 29, 58, 55, 58)$           | $\{\emptyset, 123456, 12348, 1359, 13689, 24589, 2469, 568\}$                                                                                                                                                                 |
| 93:82a | $0, 0, 0, 0, 0, 0, e^{34} + e^{12}, e^{46} + e^{15} + e^{23}, e^{56} + e^{24} + e^{13}$  | $2/3(1, 1, 1, 1, 1, 2, 2, 2)$                        | $\{\emptyset, 123456, 12689, 34589\}$                                                                                                                                                                                         |
| 93:82b | $0, 0, 0, 0, 0, 0, -e^{12} + e^{34}, e^{15} + e^{23} + e^{46}, e^{24} + e^{13} + e^{56}$ | $2/3(1, 1, 1, 1, 1, 2, 2, 2)$                        | $\{\emptyset, 123456, 12689, 34589\}$                                                                                                                                                                                         |
| 921:6  | $0, 0, 0, 0, 0, 0, e^{12}, e^{67} + e^{45} + e^{28} + e^{13}$                            | $5/31(4, 3, 6, 5, 5, 5, 5, 7, 10)$                   | $\{\emptyset, 12469, 12479, 12569, 12579, 14689, 14789, 15689, 15789, 245678, 2458, 2678, 28, 45, 4567, 67\}$                                                                                                                 |
| 92:14  | $0, 0, 0, 0, 0, 0, 0, e^{12}, e^{45} + e^{67} + e^{13}$                                  | $1/13(8, 9, 12, 10, 10, 10, 10, 17, 20)$             | $\{\emptyset, 123, 12345, 1234567, 12367, 12469, 12479, 12569, 12579, 1345678, 13458, 13678, 138, 14689, 14789, 15689, 15789, 234689, 234789, 235689, 235789, 245678, 2458, 2678, 28, 3469, 3479, 3569, 3579, 45, 4567, 67\}$ |
| 92:15  | $0, 0, 0, 0, 0, 0, 0, e^{12} + e^{34}, e^{67} + e^{15}$                                  | $1/11(7, 9, 8, 8, 9, 8, 8, 16, 16)$                  | $\{\emptyset, 12345, 1234567, 123469, 123479, 125, 12567, 1269, 1279, 135678, 1358, 13689, 13789, 145678, 1458, 14689, 14789, 235689, 235789, 23678, 238, 245689, 245789, 24678, 248, 34, 34569, 34579, 3467, 569, 579, 67\}$ |
| 92:16  | $0, 0, 0, 0, 0, 0, 0, e^{34} + e^{12}, e^{13} + e^{25} + e^{67}$                         | $1/23(18, 15, 16, 17, 19, 17, 17, 33, 34)$           | $\{\emptyset, 12345, 1234567, 1269, 1279, 13678, 138, 145689, 145789, 23689, 23789, 245678, 2458, 34569, 34579, 67\}$                                                                                                         |
| 92:17  | $0, 0, 0, 0, 0, 0, 0, e^{34} + e^{12}, e^{37} + e^{15} + e^{26}$                         | $1/16(11, 11, 10, 12, 13, 13, 14, 22, 24)$           | $\{\emptyset, 1234567, 12349, 1256, 1279, 13578, 13689, 1458, 146789, 23589, 23678, 245789, 2468, 34569, 347, 5679\}$                                                                                                         |

Table A.2 – Continued to next page

Table A.2 – Continued from previous page

| Name   | $\mathfrak{g}$                                                         | $N$                                     | Signatures $\mathbf{S}$                                                                                                                                                                                                       |
|--------|------------------------------------------------------------------------|-----------------------------------------|-------------------------------------------------------------------------------------------------------------------------------------------------------------------------------------------------------------------------------|
| 92:18a | $0, 0, 0, 0, 0, 0, e^{13} + e^{56} + e^{24}, e^{12} + e^{57} + e^{34}$ | $1/11(8, 8, 8, 8, 7, 9, 9, 16, 16)$     | $\{\emptyset, 1234, 1234567, 12578, 1268, 13569, 1379, 14589, 146789, 23589, 236789, 24569, 2479, 34578, 3468, 567\}$                                                                                                         |
| 92:18b | $0, 0, 0, 0, 0, 0, e^{56} - e^{13} + e^{24}, e^{57} + e^{34} + e^{12}$ | $1/11(8, 8, 8, 8, 7, 9, 9, 16, 16)$     | $\{\emptyset, 1234, 1234567, 12578, 1268, 13569, 1379, 14589, 146789, 23589, 236789, 24569, 2479, 34578, 3468, 567\}$                                                                                                         |
| 92:19  | $0, 0, 0, 0, 0, 0, e^{46} + e^{25} + e^{13}, e^{57} + e^{34} + e^{12}$ | $1/13(9, 10, 10, 9, 9, 10, 10, 19, 19)$ | $\{\emptyset, 1234567, 1268, 1379, 14589, 236789, 24569, 34578\}$                                                                                                                                                             |
| 91:4   | $0, 0, 0, 0, 0, 0, 0, e^{12} + e^{34} + e^{56} + e^{78}$               | $5/6(1, 1, 1, 1, 1, 1, 1, 2)$           | $\{\emptyset, 12, 1234, 123456, 12345678, 123478, 1256, 125678, 1278, 13579, 13589, 13679, 13689, 14579, 14589, 14679, 14689, 23579, 23589, 23679, 23689, 24579, 24589, 24679, 24689, 34, 3456, 345678, 3478, 56, 5678, 78\}$ |

End of Table A.2

### A.3 Nice nilpotent Lie algebras of dimension 8 with $\dim \text{coker } M_\Delta > 1$

Table A.3: Irreducible nice nilpotent Lie algebras of dimension 8 with  $\dim \text{coker } M_\Delta > 1$  that admit a Riemannian nilsoliton metric

| Name       | $\mathfrak{g}$                                                                                                                                   | $N$                                            | $\mathbf{S}_0$                        | $\mathbf{S} = \mathbf{S}_0$ |
|------------|--------------------------------------------------------------------------------------------------------------------------------------------------|------------------------------------------------|---------------------------------------|-----------------------------|
| 8654321:5  | $0, 0, -e^{12}, -e^{13}, e^{14}, e^{15}, e^{16}, e^{45} + e^{36} + e^{27}$                                                                       | $1/185(10, 123, 133, 143, 153, 163, 173, 296)$ | $\{\emptyset, 12468, 13578, 234567\}$ |                             |
| 8654321:7  | $0, 0, e^{12}, e^{13}, e^{14}, e^{15} + e^{23}, e^{24} + e^{16}, e^{34} + e^{17}$                                                                | $43/281(1, 3, 4, 5, 6, 7, 8, 9)$               | $\{\emptyset, 12468\}$                |                             |
| 8654321:11 | $0, 0, -e^{12}, -e^{13}, e^{14}, e^{15}, e^{16} + e^{23}, e^{36} + e^{27} + e^{45}$                                                              | $53/441(1, 4, 5, 6, 7, 8, 9, 13)$              | $\{\emptyset, 13578\}$                |                             |
| 8654321:14 | $0, 0, -e^{12}(-1 + a_3), e^{13}, e^{14}a_3, e^{15} + e^{23}, e^{24} + e^{16}, e^{25} + e^{34} + e^{17}$                                         | $43/281(1, 3, 4, 5, 6, 7, 8, 9)$               | $\{\emptyset, 12468\}$                |                             |
| 8654321:17 | $0, 0, -e^{12}, e^{13}, e^{14}, -e^{15} + e^{23}, e^{24} + e^{16}, e^{36} + e^{27} + e^{45}$                                                     | $15/107(1, 3, 4, 5, 6, 7, 8, 11)$              | $\{\emptyset, 12468\}$                |                             |
| 8654321:19 | $0, 0, e^{12}, e^{13}, e^{23} + e^{14}, e^{24} + e^{15}, e^{25} + e^{34} + 2e^{16}, e^{35} + e^{17}$                                             | $3/17(1, 2, 3, 4, 5, 6, 7, 8)$                 | $\{\emptyset, 1357\}$                 |                             |
| 8654321:20 | $0, 0, e^{12}, -e^{13}, e^{23} + e^{14}, e^{24} - e^{15}, e^{34} + e^{16}, e^{35} + e^{26} + e^{17}$                                             | $3/17(1, 2, 3, 4, 5, 6, 7, 8)$                 | $\{\emptyset, 1357\}$                 |                             |
| 8654321:24 | $0, 0, -e^{12}(-1 + a_4), e^{13}a_4, e^{23} + e^{14}, e^{24} + e^{15}a_4, -e^{16}(-2 + a_4) + e^{25} + e^{34}, e^{35} + e^{26} + e^{17}$         | $3/17(1, 2, 3, 4, 5, 6, 7, 8)$                 | $\{\emptyset, 1357\}$                 |                             |
| 8654321:25 | $0, 0, -e^{12}, -e^{13}, -\frac{1}{2}e^{23} + \frac{3}{2}e^{14}, \frac{1}{2}e^{24} + e^{15}, e^{25} + e^{34} + e^{16}, e^{36} + e^{27} + e^{45}$ | $37/221(1, 2, 3, 4, 5, 6, 7, 9)$               | $\{\emptyset, 13578\}$                |                             |
| 865431:4   | $0, 0, -e^{12}, e^{13}, e^{14}, e^{15} + e^{23}, e^{25} + e^{34}, e^{24} + e^{16}$                                                               | $43/281(1, 3, 4, 5, 6, 7, 9, 8)$               | $\{\emptyset, 12467\}$                |                             |
| 865431:7   | $0, 0, -e^{12}, e^{13}, e^{14}, 2e^{15}, e^{25} + e^{34}, e^{35} + e^{26} + e^{17}$                                                              | $9/76(1, 4, 5, 6, 7, 8, 11, 12)$               | $\{\emptyset, 12467, 1357, 23456\}$   |                             |
| 865431:8   | $0, 0, -e^{12}, e^{13}, e^{14}, 2e^{15} + e^{23}, e^{25} + e^{34}, e^{35} + e^{26} + e^{17}$                                                     | $45/317(1, 3, 4, 5, 6, 7, 9, 10)$              | $\{\emptyset, 12467\}$                |                             |
| 865431:9   | $0, 0, -e^{12}, 2e^{13}, e^{23} + e^{14}, e^{24} + 2e^{15}, e^{25} + e^{34}, e^{35} + e^{26} + e^{17}$                                           | $3/17(1, 2, 3, 4, 5, 6, 7, 8)$                 | $\{\emptyset, 1357\}$                 |                             |
| 86532:3    | $0, 0, e^{12}, -e^{13}, e^{23}, e^{24} - e^{15}, e^{34} + e^{16}, e^{35} + e^{26}$                                                               | $4/15(1, 1, 2, 3, 3, 4, 5, 5)$                 | $\{\emptyset, 124578, 1357, 2348\}$   |                             |
| 86532:4a   | $0, 0, e^{12}, e^{13}, e^{23}, e^{25} - e^{14}, e^{26} + e^{34}, e^{35} + e^{16}$                                                                | $4/15(1, 1, 2, 3, 3, 4, 5, 5)$                 | $\{\emptyset, 124578, 13567, 23468\}$ |                             |
| 86532:4b   | $0, 0, e^{12}, -e^{13}, e^{23}, e^{25} - e^{14}, e^{26} + e^{34}, e^{35} + e^{16}$                                                               | $4/15(1, 1, 2, 3, 3, 4, 5, 5)$                 | $\{\emptyset, 124578, 13567, 23468\}$ |                             |
| 86531:5    | $0, 0, -e^{12}, e^{13}, e^{23}, e^{14}, e^{24} + e^{15}, e^{26} + e^{34}$                                                                        | $1/5(1, 2, 3, 4, 5, 5, 6, 7)$                  | $\{\emptyset, 12458, 13568, 2346\}$   |                             |
| 86531:7    | $0, 0, -e^{12}, e^{13}, e^{23}, e^{24} + e^{15}, e^{14}, e^{35} + e^{26}$                                                                        | $1/30(9, 8, 17, 26, 25, 34, 35, 42)$           | $\{\emptyset, 12458, 1357, 23478\}$   |                             |
| 86531:9a   | $0, 0, e^{12}, e^{13}, e^{23}, e^{25} - e^{14}, e^{24} + e^{15}, e^{26} + e^{34}$                                                                | $23/81(1, 1, 2, 3, 3, 4, 4, 5)$                | $\{\emptyset, 12458, 13568, 2346\}$   |                             |
| 86531:9b   | $0, 0, -e^{12}, e^{13}, e^{23}, e^{25} + e^{14}, e^{24} + e^{15}, e^{26} + e^{34}$                                                               | $23/81(1, 1, 2, 3, 3, 4, 4, 5)$                | $\{\emptyset, 12458, 13568, 2346\}$   |                             |
| 86531:14   | $0, 0, e^{12}a_1, e^{13}, e^{23}, -e^{14}(-1 + a_1), e^{24} + e^{15}, e^{26} + e^{34} + e^{17}$                                                  | $1/5(1, 2, 3, 4, 5, 5, 6, 7)$                  | $\{\emptyset, 12458, 13568, 2346\}$   |                             |
| 86531:15a  | $0, 0, -e^{12}, e^{13}, e^{23}, e^{14}, e^{24} + e^{15}, e^{27} + e^{35} + e^{16}$                                                               | $23/81(1, 1, 2, 3, 3, 4, 4, 5)$                | $\{\emptyset, 12458, 1356, 23468\}$   |                             |
| 86531:15b  | $0, 0, -e^{12}, e^{13}, e^{23}, -e^{14}, e^{24} + e^{15}, e^{27} + e^{35} + e^{16}$                                                              | $23/81(1, 1, 2, 3, 3, 4, 4, 5)$                | $\{\emptyset, 12458, 1356, 23468\}$   |                             |
| 86531:16a  | $0, 0, e^{12}a_1, e^{13}, e^{23}, e^{24} + e^{15}, e^{25} - e^{14}(-1 + a_1), e^{27} + e^{34} + e^{16}$                                          | $23/81(1, 1, 2, 3, 3, 4, 4, 5)$                | $\{\emptyset, 12458, 13578, 2347\}$   |                             |
| 86531:16b  | $0, 0, e^{12}a_1, -e^{13}, e^{23}, e^{24} - e^{15}, e^{25} - e^{14}(-1 + a_1), e^{27} + e^{34} + e^{16}$                                         | $23/81(1, 1, 2, 3, 3, 4, 4, 5)$                | $\{\emptyset, 12458, 13578, 2347\}$   |                             |

Table A.3 – Continued to next page

Table A.3 – Continued from previous page

| Name      | $g$                                                                                                                           | $N$                                           | $S_0$                                                         | $S = S_0$ |
|-----------|-------------------------------------------------------------------------------------------------------------------------------|-----------------------------------------------|---------------------------------------------------------------|-----------|
| 854321:5  | $0, 0, 0, -e^{12}, e^{14}, e^{15} + e^{23}, e^{34} + e^{16}, e^{35} + e^{17}$                                                 | $1/55(8, 35, 24, 43, 51, 59, 67, 75)$         | $\{\emptyset, 12357, 13468, 245678\}$                         |           |
| 854321:11 | $0, 0, 0, -e^{12}, e^{14}, e^{15} + e^{23}, e^{34} + e^{16}, e^{24} + e^{35} + e^{17}$                                        | $43/281(1, 4, 3, 5, 6, 7, 8, 9)$              | $\{\emptyset, 13468\}$                                        |           |
| 854321:18 | $0, 0, 0, -e^{12}, e^{23} + e^{14}, e^{34} + e^{15}, e^{35} + e^{16}, e^{36} + e^{17}$                                        | $2/15(1, 5, 2, 6, 7, 8, 9, 10)$               | $\{\emptyset, 1257, 1468, 245678\}$                           |           |
| 854321:23 | $0, 0, 0, -e^{12}, e^{23} + e^{14}, e^{34} + e^{15}, e^{35} + e^{16}, e^{24} + e^{36} + e^{17}$                               | $7/46(1, 4, 2, 5, 6, 7, 8, 9)$                | $\{\emptyset, 1468\}$                                         |           |
| 854321:25 | $0, 0, 0, -e^{12}, e^{23} + e^{14}, e^{34} + e^{15}, e^{24} + e^{35} + e^{16}, e^{25} + e^{36} + e^{17}$                      | $3/17(1, 3, 2, 4, 5, 6, 7, 8)$                | $\{\emptyset, 1257\}$                                         |           |
| 85432:5   | $0, 0, 0, -e^{12}, e^{14}, e^{15} + e^{23}, e^{34} + e^{16}, e^{26} + e^{45}$                                                 | $1/185(41, 71, 123, 112, 153, 194, 235, 265)$ | $\{\emptyset, 123578, 13468, 24567\}$                         |           |
| 85421:17  | $0, 0, 0, e^{12}(-1 + a_2), e^{14}, e^{24} + a_2 e^{13}, e^{15} + e^{23}, e^{26} + e^{34} + e^{17}$                           | $51/389(2, 3, 6, 5, 7, 8, 9, 11)$             | $\{\emptyset, 24578\}$                                        |           |
| 85421:18  | $0, 0, 0, e^{12}, e^{13} + e^{24}, e^{14}, e^{25} + e^{34}, e^{27} + e^{35}$                                                  | $7/30(2, 1, 2, 3, 4, 5, 5, 6)$                | $\{\emptyset, 12568, 14578, 2467\}$                           |           |
| 85421:23  | $0, 0, 0, e^{12}, e^{13} + e^{24}, e^{14}, e^{25} + e^{34}, e^{27} + e^{35} + e^{16}$                                         | $49/369(3, 2, 4, 5, 7, 8, 9, 11)$             | $\{\emptyset, 14578\}$                                        |           |
| 85421:24  | $0, 0, 0, e^{12}, e^{13} + e^{24}, 2e^{14}, e^{25} + e^{34}, e^{36} + e^{17} + e^{45}$                                        | $1/76(25, 22, 44, 47, 69, 72, 91, 116)$       | $\{\emptyset, 12568, 1457, 24678\}$                           |           |
| 85421:31  | $0, 0, 0, e^{12}, e^{14}, e^{13} + e^{24}, e^{25} + e^{16}, e^{17} + e^{45}$                                                  | $1/31(5, 14, 28, 19, 24, 33, 38, 43)$         | $\{\emptyset, 12568, 1468, 245\}$                             |           |
| 85421:34  | $0, 0, 0, -e^{12}, e^{14}, e^{13} + e^{24}, e^{25} + e^{16}, e^{27} + e^{35} + e^{46}$                                        | $1/15(4, 5, 10, 9, 13, 14, 18, 23)$           | $\{\emptyset, 12568, 146, 2458\}$                             |           |
| 85421:37a | $0, 0, 0, e^{12}, e^{23} + e^{14}, e^{13} + e^{24}, e^{26} + e^{15}, e^{46} + e^{35} + e^{17}$                                | $7/23(1, 1, 2, 2, 3, 3, 4, 5)$                | $\{\emptyset, 12568, 1467, 24578\}$                           |           |
| 85421:37b | $0, 0, 0, e^{12}, -e^{23} - e^{14}, -e^{13} + e^{24}, e^{26} + e^{15}, e^{35} + e^{17} + e^{46}$                              | $7/23(1, 1, 2, 2, 3, 3, 4, 5)$                | $\{\emptyset, 12568, 1467, 24578\}$                           |           |
| 85421:38a | $0, 0, 0, e^{12}, e^{13} + e^{24}, e^{23} + e^{14}, e^{26} + e^{15}, e^{46} + e^{35} + e^{17}$                                | $7/23(1, 1, 2, 2, 3, 3, 4, 5)$                | $\{\emptyset, 12568, 1458, 246\}$                             |           |
| 85421:38b | $0, 0, 0, e^{12}, -e^{13} + e^{24}, e^{23} + e^{14}, e^{26} + e^{15}, e^{35} + e^{17} + e^{46}$                               | $7/23(1, 1, 2, 2, 3, 3, 4, 5)$                | $\{\emptyset, 12568, 1458, 246\}$                             |           |
| 85421:39a | $0, 0, 0, e^{12}, 2e^{14}, e^{13} + e^{24}, e^{26} + e^{34} + e^{15}, e^{46} + e^{35} + e^{17}$                               | $7/23(1, 1, 2, 2, 3, 3, 4, 5)$                | $\{\emptyset, 12568, 1467, 24578\}$                           |           |
| 85421:39b | $0, 0, 0, e^{12}, 2e^{14}, e^{13} + e^{24}, e^{26} + e^{34} - e^{15}, e^{35} + e^{17} + e^{46}$                               | $7/23(1, 1, 2, 2, 3, 3, 4, 5)$                | $\{\emptyset, 12568, 1467, 24578\}$                           |           |
| 85421:40a | $0, 0, 0, -e^{12}, e^{14}, -e^{13} + e^{24}, e^{26} + e^{34} + e^{15}, e^{45} + e^{36} + e^{27}$                              | $7/23(1, 1, 2, 2, 3, 3, 4, 5)$                | $\{\emptyset, 12568, 14678, 2457\}$                           |           |
| 85421:40b | $0, 0, 0, -e^{12}, -e^{14}, -e^{13} + e^{24}, e^{26} + e^{34} + e^{15}, e^{36} + e^{27} + e^{45}$                             | $7/23(1, 1, 2, 2, 3, 3, 4, 5)$                | $\{\emptyset, 12568, 14678, 2457\}$                           |           |
| 85421:41a | $0, 0, 0, e^{12}, e^{14}(1 + a_3) + e^{23}(-1 + a_3), e^{24} + e^{13}a_3, e^{26} + e^{34} + e^{15}, e^{46} + e^{35} + e^{17}$ | $7/23(1, 1, 2, 2, 3, 3, 4, 5)$                | $\{\emptyset, 12568, 1467, 24578\}$                           |           |
| 85421:41b | $0, 0, 0, e^{12}, e^{14}(1 + a_3) - e^{23}(-1 + a_3), e^{24} + e^{13}a_3, e^{26} + e^{34} - e^{15}, e^{35} + e^{17} + e^{46}$ | $7/23(1, 1, 2, 2, 3, 3, 4, 5)$                | $\{\emptyset, 12568, 1467, 24578\}$                           |           |
| 85321:22  | $0, 0, 0, (-1 + a_2)e^{12}, e^{13}a_2, e^{14}, e^{16} + e^{23}, e^{25} + e^{34} + e^{17}$                                     | $1/9(2, 5, 6, 7, 8, 9, 11, 13)$               | $\{\emptyset, 12368, 1347, 24678\}$                           |           |
| 85321:45  | $0, 0, 0, e^{12}, e^{13}, e^{23} + e^{14}, e^{25} + e^{16}, e^{45} + e^{36} + e^{17}$                                         | $1/4(1, 2, 2, 3, 3, 4, 5, 6)$                 | $\{\emptyset, 12568, 1457, 24678\}$                           |           |
| 85321:47  | $0, 0, 0, -e^{12}, -2e^{13}, -e^{23} + e^{14}, e^{25} + e^{34} + e^{16}, e^{46} + e^{27}$                                     | $3/76(8, 7, 16, 15, 24, 23, 31, 38)$          | $\{\emptyset, 12568, 14578, 2467\}$                           |           |
| 85321:48  | $0, 0, 0, e^{12}, e^{13}(-1 + a_3), e^{23} + e^{14}a_3, (-2 + a_3)e^{16} + e^{25} + e^{34}, e^{36} + e^{17} + e^{45}$         | $1/4(1, 2, 2, 3, 3, 4, 5, 6)$                 | $\{\emptyset, 12568, 1457, 24678\}$                           |           |
| 85321:49a | $0, 0, 0, -e^{12}, -2e^{13}, -e^{23} + e^{14}, e^{25} + e^{34} + e^{16}, e^{46} + e^{27} + e^{35}$                            | $7/23(1, 1, 2, 2, 3, 3, 4, 5)$                | $\{\emptyset, 12568, 14578, 2467\}$                           |           |
| 85321:49b | $0, 0, 0, -e^{12}, -2e^{13}, -e^{23} - e^{14}, e^{25} + e^{34} + e^{16}, e^{27} + e^{35} + e^{46}$                            | $7/23(1, 1, 2, 2, 3, 3, 4, 5)$                | $\{\emptyset, 12568, 14578, 2467\}$                           |           |
| 8542:11   | $0, 0, 0, e^{12}, e^{13} + e^{24}, e^{14}, e^{25} + e^{34}, e^{26} + e^{15}$                                                  | $1/3(1, 1, 2, 2, 3, 3, 4, 4)$                 | $\{\emptyset, 1256, 1457, 2467\}$                             |           |
| 8542:15a  | $0, 0, 0, e^{12}a_1, e^{24} + e^{13}(1 + a_1), e^{23} + e^{14}, e^{26} + e^{15}, e^{25} + e^{34} + e^{16}$                    | $1/3(1, 1, 2, 2, 3, 3, 4, 4)$                 | $\{\emptyset, 1256, 1458, 2468\}$                             |           |
| 8542:15b  | $0, 0, 0, e^{12}a_1, e^{24} + e^{13}(1 + a_1), e^{23} - e^{14}, e^{26} - e^{15}, e^{25} + e^{34} + e^{16}$                    | $1/3(1, 1, 2, 2, 3, 3, 4, 4)$                 | $\{\emptyset, 1256, 1458, 2468\}$                             |           |
| 8531:55   | $0, 0, 0, e^{12}(-1 + a_2), e^{13}a_2, e^{23} + e^{14}, e^{35}, e^{25} + e^{34} + e^{16}$                                     | $1/8(2, 5, 4, 7, 6, 9, 10, 11)$               | $\{\emptyset, 12567, 14578, 2468\}$                           |           |
| 8531:62   | $0, 0, 0, e^{12}a_1, e^{13}(1 + a_1), e^{23} + e^{14}, e^{15}, e^{25} + e^{34} + e^{16}$                                      | $2/7(1, 2, 2, 3, 3, 4, 4, 5)$                 | $\{\emptyset, 1256, 1458, 2468\}$                             |           |
| 8531:68   | $0, 0, 0, e^{12}(-1 + a_2), e^{13}a_2, e^{23} + e^{14}, e^{24}, e^{25} + e^{34} + e^{16}$                                     | $1/12(4, 5, 8, 9, 12, 13, 14, 17)$            | $\{\emptyset, 12567, 14578, 2468\}$                           |           |
| 8531:69a  | $0, 0, 0, e^{12}a_1, e^{13}(1 + a_1), e^{23} + e^{14}, e^{24} + e^{35}, e^{25} + e^{34} + e^{16}$                             | $25/93(1, 2, 2, 3, 3, 4, 5, 5)$               | $\{\emptyset, 12567, 14578, 2468\}$                           |           |
| 8531:69b  | $0, 0, 0, e^{12}a_1, e^{13}(1 + a_1), e^{23} + e^{14}, -e^{24} + e^{35}, e^{25} + e^{34} + e^{16}$                            | $25/93(1, 2, 2, 3, 3, 4, 5, 5)$               | $\{\emptyset, 12567, 14578, 2468\}$                           |           |
| 8531:70   | $0, 0, 0, e^{12}a_1, e^{13}(1 + a_1), e^{23} + e^{14}, e^{24} + e^{15}, e^{25} + e^{34} + e^{16}$                             | $11/71(2, 3, 4, 5, 6, 7, 8, 9)$               | $\{\emptyset, 2468\}$                                         |           |
| 8531:90   | $0, 0, 0, e^{12}, e^{13}, e^{14}, e^{15}, e^{25} + e^{34}, e^{36} + e^{27}$                                                   | $1/5(3, 1, 2, 4, 5, 5, 6, 7)$                 | $\{\emptyset, 12367, 12568, 1346, 145678, 23458, 247, 3578\}$ |           |
| 8531:93   | $0, 0, 0, -e^{12}, e^{13}, e^{14}, e^{15}, e^{36} + e^{27} + e^{45}$                                                          | $1/5(1, 3, 3, 4, 4, 5, 5, 8)$                 | $\{\emptyset, 12367, 12568, 13478, 145, 234567, 2468, 3578\}$ |           |
| 8531:95a  | $0, 0, 0, e^{12}, e^{13}, e^{25} + e^{34}, e^{24} + e^{35}, e^{37} + e^{26}$                                                  | $1/15(9, 4, 4, 13, 13, 17, 17, 21)$           | $\{\emptyset, 12367, 12578, 1347, 145678, 23458, 246, 3568\}$ |           |
| 8531:95b  | $0, 0, 0, -e^{12}, e^{13}, -e^{25} + e^{34}, e^{24} + e^{35}, e^{37} + e^{26}$                                                | $1/15(9, 4, 4, 13, 13, 17, 17, 21)$           | $\{\emptyset, 12367, 12578, 1347, 145678, 23458, 246, 3568\}$ |           |
| 8531:99   | $0, 0, 0, e^{12}, e^{13}, e^{24}, e^{25} + e^{34}, e^{36} + e^{27} + e^{15}$                                                  | $1/31(16, 8, 13, 24, 29, 32, 37, 45)$         | $\{\emptyset, 23458, 247, 3578\}$                             |           |
| 8531:100  | $0, 0, 0, -e^{12}, e^{13}, e^{14}, e^{15} + e^{23}, e^{45} + e^{36} + e^{27}$                                                 | $1/31(8, 16, 17, 24, 25, 32, 33, 49)$         | $\{\emptyset, 13478, 145, 3578\}$                             |           |
| 8531:101  | $0, 0, 0, -e^{12}, e^{13}, e^{14}, e^{24} + e^{15}, e^{36} + e^{27} + e^{45}$                                                 | $1/30(8, 13, 18, 21, 26, 29, 34, 47)$         | $\{\emptyset, 12367, 13478, 2468\}$                           |           |

Table A.3 – Continued to next page



Table A.3 – Continued from previous page

| Name      | $\mathfrak{g}$                                                                                          | $N$                                     | $S_0$                                                         | $S = S_0$ |
|-----------|---------------------------------------------------------------------------------------------------------|-----------------------------------------|---------------------------------------------------------------|-----------|
| 8531:103  | $0, 0, 0, e^{12}, e^{13}, 2e^{14}, e^{25} + e^{34}, e^{45} + e^{36} + e^{17}$                           | $1/4(1, 2, 2, 3, 3, 4, 5, 6)$           | $\{\emptyset, 12367, 12568, 1348, 1457, 23456, 24678, 3578\}$ |           |
| 8531:104  | $0, 0, 0, e^{12}a_1, e^{13}, e^{23} + e^{14}, e^{24} + e^{15}, e^{35} + e^{26} + e^{17}$                | $15/101(2, 3, 4, 5, 6, 7, 8, 10)$       | $\{\emptyset, 246\}$                                          |           |
| 8531:105a | $0, 0, 0, e^{12}, e^{13}, e^{25} + e^{34}, e^{24} + e^{35}, e^{37} + e^{26} + e^{14}$                   | $23/81(2, 1, 1, 3, 3, 4, 4, 5)$         | $\{\emptyset, 12578, 1347, 23458\}$                           |           |
| 8531:105b | $0, 0, 0, -e^{12}, e^{13}, -e^{25} + e^{34}, e^{24} + e^{35}, e^{37} + e^{26} + e^{14}$                 | $23/81(2, 1, 1, 3, 3, 4, 4, 5)$         | $\{\emptyset, 12578, 1347, 23458\}$                           |           |
| 8531:106a | $0, 0, 0, e^{12}, e^{13}, e^{25} + e^{34}, e^{24} + e^{35}, e^{36} + e^{27} + e^{14}$                   | $23/81(2, 1, 1, 3, 3, 4, 4, 5)$         | $\{\emptyset, 23458, 2468, 356\}$                             |           |
| 8531:106b | $0, 0, 0, e^{12}, e^{13}, e^{25} + e^{34}, -e^{24} + e^{35}, e^{36} + e^{27} + e^{14}$                  | $23/81(2, 1, 1, 3, 3, 4, 4, 5)$         | $\{\emptyset, 23458, 2468, 356\}$                             |           |
| 8531:107  | $0, 0, 0, -e^{12}, e^{13}, e^{23} + e^{14}, e^{24} + e^{15}, e^{45} + e^{36} + e^{27}$                  | $23/162(2, 3, 4, 5, 6, 7, 8, 11)$       | $\{\emptyset, 2468\}$                                         |           |
| 8531:109  | $0, 0, 0, -e^{12}, -e^{13}, e^{24} + 2e^{15}, e^{25} + e^{34}, e^{45} + e^{26} + e^{17}$                | $1/72(20, 29, 38, 49, 58, 78, 87, 107)$ | $\{\emptyset, 12367, 13468, 2478\}$                           |           |
| 8531:110  | $0, 0, 0, -e^{12}, e^{13}, e^{24} + e^{15}, e^{35} + e^{14}, e^{37} + e^{26} + e^{45}$                  | $17/45(1, 1, 1, 2, 2, 3, 3, 4)$         | $\{\emptyset, 12367\}$                                        |           |
| 8521:12   | $0, 0, 0, e^{12}, -e^{13}, e^{23}, e^{25} + e^{34} - 2e^{16}, e^{45} + e^{17}$                          | $1/4(1, 2, 2, 3, 3, 4, 5, 6)$           | $\{\emptyset, 1237, 12568, 13468, 1457, 2345, 24678, 35678\}$ |           |
| 852:18    | $0, 0, 0, e^{12}(-1 + a_2), e^{13}a_2, e^{23}, e^{14}, e^{25} + e^{34} + e^{16}$                        | $1/19(7, 9, 11, 16, 18, 20, 23, 27)$    | $\{\emptyset, 12378, 12567, 1346, 1458, 23457, 24678, 3568\}$ |           |
| 852:27    | $0, 0, 0, e^{12}(-1 + a_2), e^{13}a_2, e^{23}, e^{24} + e^{15}, e^{25} + e^{34} + e^{16}$               | $1/13(5, 6, 7, 11, 12, 13, 17, 18)$     | $\{\emptyset, 12378, 13467, 2468\}$                           |           |
| 852:28a   | $0, 0, 0, e^{12}(-1 + a_2), e^{13}a_2, e^{23}, e^{24} + e^{35}, e^{25} + e^{34} + e^{16}$               | $5/11(1, 1, 1, 2, 2, 2, 3, 3)$          | $\{\emptyset, 12378, 12567, 13467, 14578, 2345, 2468, 3568\}$ |           |
| 852:28b   | $0, 0, 0, e^{12}(-1 + a_2), e^{13}a_2, e^{23}, -e^{24} + e^{35}, e^{25} + e^{34} + e^{16}$              | $5/11(1, 1, 1, 2, 2, 2, 3, 3)$          | $\{\emptyset, 12378, 12567, 13467, 14578, 2345, 2468, 3568\}$ |           |
| 852:30    | $0, 0, 0, e^{12}a_1, e^{13}a_2, e^{23}, e^{35} + e^{26} + e^{14}, e^{24} + e^{36} + e^{15}$             | $5/11(1, 1, 1, 2, 2, 2, 3, 3)$          | $\{\emptyset, 12378\}$                                        |           |
| 852:31    | $0, 0, 0, e^{12}a_1, (1 + a_1)e^{13}, e^{23}, e^{25} + e^{34} + e^{16}, e^{24} + e^{36} + e^{15}$       | $5/11(1, 1, 1, 2, 2, 2, 3, 3)$          | $\{\emptyset, 12378\}$                                        |           |
| 84321:22  | $0, 0, 0, 0, -e^{12}, e^{15} + e^{23}, e^{35} + e^{16}, e^{24} + e^{36} + e^{17}$                       | $1/31(7, 17, 14, 28, 24, 31, 38, 45)$   | $\{\emptyset, 1268, 157, 25678\}$                             |           |
| 84321:29  | $0, 0, 0, 0, -e^{12}, e^{15} + e^{23}, e^{24} + e^{35} + e^{16}, e^{36} + e^{17} + e^{45}$              | $1/4(1, 2, 2, 3, 3, 4, 5, 6)$           | $\{\emptyset, 12468, 1457, 25678\}$                           |           |
| 8431:31   | $0, 0, 0, 0, e^{12}a_1, e^{15} + e^{23}, e^{25} + e^{14}, e^{26} + e^{34} + e^{17}$                     | $3/8(1, 1, 2, 2, 2, 3, 3, 4)$           | $\{\emptyset, 1267, 157, 256\}$                               |           |
| 8421:56   | $0, 0, 0, 0, e^{12}(-1 + a_2), e^{23} + e^{14}, e^{25} + e^{13}a_2, e^{27} + e^{35} + e^{16}$           | $3/8(1, 1, 2, 2, 2, 3, 3, 4)$           | $\{\emptyset, 1267, 14578, 24568\}$                           |           |
| 842:107   | $0, 0, 0, 0, -e^{12}, e^{23} - e^{14}, e^{35} + e^{16}, e^{45} + e^{26}$                                | $1/5(2, 2, 3, 3, 4, 5, 7, 7)$           | $\{\emptyset, 123478, 126, 13568, 1457, 2358, 24567, 34678\}$ |           |
| 842:111a  | $0, 0, 0, 0, e^{23} + e^{14}, e^{13} + e^{24}, e^{25} + e^{16}, e^{26} + e^{15}$                        | $1/3(1, 1, 2, 2, 3, 3, 4, 4)$           | $\{\emptyset, 123478, 1256, 1357, 1468, 2367, 2458, 345678\}$ |           |
| 842:111b  | $0, 0, 0, 0, e^{23} - e^{14}, e^{13} + e^{24}, e^{25} - e^{16}, e^{26} + e^{15}$                        | $1/3(1, 1, 2, 2, 3, 3, 4, 4)$           | $\{\emptyset, 123478, 1256, 1357, 1468, 2367, 2458, 345678\}$ |           |
| 842:112a  | $0, 0, 0, 0, e^{23} + e^{14}, e^{13} + e^{24}, e^{26} + e^{15}, e^{35} + e^{46}$                        | $7/15(1, 1, 1, 1, 2, 2, 3, 3)$          | $\{\emptyset, 123478, 12568, 135, 1467, 2368, 24578, 34567\}$ |           |
| 842:112b  | $0, 0, 0, 0, -e^{23} - e^{14}, -e^{13} + e^{24}, e^{26} + e^{15}, e^{46} + e^{35}$                      | $7/15(1, 1, 1, 1, 2, 2, 3, 3)$          | $\{\emptyset, 123478, 12568, 135, 1467, 2368, 24578, 34567\}$ |           |
| 841:74    | $0, 0, 0, 0, e^{12}(-1 + a_2), e^{13}a_2, e^{23} + e^{14}, e^{35} + e^{26} + e^{17}$                    | $1/19(7, 11, 11, 15, 18, 18, 22, 29)$   | $\{\emptyset, 12348, 1267, 1357, 14568, 2356, 24578, 34678\}$ |           |
| 841:78a   | $0, 0, 0, 0, e^{12}a_1, e^{23} + e^{14}, e^{13}(1 + a_1) + e^{24}, e^{27} + e^{35} + e^{16}$            | $1/11(5, 5, 7, 7, 10, 12, 12, 17)$      | $\{\emptyset, 12348, 1267, 1356, 14578, 2357, 24568, 34678\}$ |           |
| 841:78b   | $0, 0, 0, 0, e^{12}a_1, e^{23} - e^{14}, e^{13}(1 + a_1) + e^{24}, e^{27} + e^{35} + e^{16}$            | $1/11(5, 5, 7, 7, 10, 12, 12, 17)$      | $\{\emptyset, 12348, 1267, 1356, 14578, 2357, 24568, 34678\}$ |           |
| 841:81a   | $0, 0, 0, 0, e^{23} + e^{14}, e^{24} + e^{13}a_1, e^{34} + e^{12}(-1 + a_1), e^{37} + e^{26} + e^{15}$  | $13/25(1, 1, 1, 1, 2, 2, 2, 3)$         | $\{\emptyset, 12348, 1256, 1357, 14678, 2367, 24578, 34568\}$ | ✓         |
| 841:81b   | $0, 0, 0, 0, e^{23} + e^{14}, -e^{24} + e^{13}a_1, e^{34} + e^{12}(-1 + a_1), e^{37} + e^{26} + e^{15}$ | $13/25(1, 1, 1, 1, 2, 2, 2, 3)$         | $\{\emptyset, 12348, 1256, 1357, 14678, 2367, 24578, 34568\}$ | ✓         |

End of Table A.3

## A.4 Nice nilpotent Lie algebras of dimension 9 with $\dim \text{coker } M_\Delta > 0$

Table A.4: Irreducible nice nilpotent Lie algebras of dimension 9 with  $\dim \text{coker } M_\Delta > 0$  that admit a Riemannian nilsoliton metric

| Name        | $\mathfrak{g}$                                                                                                                               | $N$                                   | $S_0$                  | $S = S_0$ |
|-------------|----------------------------------------------------------------------------------------------------------------------------------------------|---------------------------------------|------------------------|-----------|
| 97654321:12 | $0, 0, a_1e^{12}, e^{13}, -e^{14}(-1 + a_1), e^{15}, e^{16} + e^{23}, e^{17} + e^{24}, e^{18} + e^{34} + e^{25}$                             | $61/493(1, 4, 5, 6, 7, 8, 9, 10, 11)$ | $\{\emptyset, 13579\}$ |           |
| 97654321:21 | $0, 0, e^{12}, e^{13}, e^{14}, -e^{15} + e^{23}, e^{16} + e^{24}, e^{34} + e^{17}, e^{26} + e^{18} + e^{35}$                                 | $53/381(1, 3, 4, 5, 6, 7, 8, 9, 10)$  | $\{\emptyset, 12468\}$ |           |
| 97654321:25 | $0, 0, (-1 + a_5)e^{12}, e^{13}, e^{14}, -(-2 + a_5)e^{15} + e^{23}, e^{16} + e^{24}, e^{25} + e^{34} + e^{17}a_5, e^{18} + e^{26} + e^{35}$ | $53/381(1, 3, 4, 5, 6, 7, 8, 9, 10)$  | $\{\emptyset, 12468\}$ |           |
| 97654321:31 | $0, 0, e^{12}, e^{13}, e^{14} - e^{23}, -e^{15} + e^{24}, e^{34} + e^{16}, e^{35} + e^{17} + e^{26}, e^{45} + e^{18} + e^{27}$               | $3/19(1, 2, 3, 4, 5, 6, 7, 8, 9)$     | $\{\emptyset, 13579\}$ |           |

Table A.4 – Continued to next page

Table A.4 – Continued from previous page

| Name        | g                                                                                                                                                                                                                                                                                                                                                     | N                                                 | S <sub>0</sub>              | S = S <sub>0</sub> |
|-------------|-------------------------------------------------------------------------------------------------------------------------------------------------------------------------------------------------------------------------------------------------------------------------------------------------------------------------------------------------------|---------------------------------------------------|-----------------------------|--------------------|
| 97654321:40 | $0, 0, e^{12}, \frac{1}{2}e^{13}, \frac{3}{2}e^{14} + e^{23},$<br>$\frac{1}{2}e^{15} + e^{24}, \frac{5}{2}e^{16} + e^{34} + e^{25}, \frac{3}{2}e^{17} + e^{35} + e^{26}, e^{18} + e^{36} + e^{45}$                                                                                                                                                    | 3/19(1, 2, 3, 4, 5, 6, 7, 8, 9)                   | {0, 13579}                  |                    |
| 97654321:42 | $0, 0, e^{12}, \frac{3}{5}e^{13}, -3e^{23} + e^{14},$<br>$-2e^{24} + \frac{2}{5}e^{15}, -e^{16} + e^{25} + e^{34}, e^{35} + e^{17}, e^{36} + e^{45} + e^{27} + e^{18}$                                                                                                                                                                                | 3/19(1, 2, 3, 4, 5, 6, 7, 8, 9)                   | {0, 13579}                  |                    |
| 97654321:43 | $0, 0, -2\frac{(a_8 - a_8^2)e^{12}}{(2+a_8)(-1+2a_8)},$<br>$\frac{(-1+a_8)e^{13}}{-1+2a_8}, (-1+a_8)e^{23} + 3\frac{a_8^2e^{14}}{(2+a_8)(-1+2a_8)}, \frac{a_8e^{15}}{-1+2a_8} + a_8e^{24},$<br>$\frac{e^{16}(-2+5a_8)}{-2+3a_8+2a_8^2} + e^{25} + e^{34}, e^{26} + e^{35} + 3\frac{a_8^2e^{17}}{(2+a_8)(-1+2a_8)}, e^{18} + e^{45} + e^{36} + e^{27}$ | 3/19(1, 2, 3, 4, 5, 6, 7, 8, 9)                   | {0, 13579}                  |                    |
| 9765432:4   | $0, 0, -e^{12}, e^{13}, e^{14}, -e^{15}, e^{16} + e^{23}, e^{17} + e^{24}, e^{27} + e^{36} + e^{45}$                                                                                                                                                                                                                                                  | 63/541(1, 4, 5, 6, 7, 8, 9, 10, 13)               | {0, 13579}                  |                    |
| 9765432:6   | $0, 0, -e^{12}, e^{13}, e^{14}, -e^{15} + e^{23}, e^{16} + e^{24}, e^{17} + e^{25}, e^{27} + e^{45} + e^{36}$                                                                                                                                                                                                                                         | 9/67(1, 3, 4, 5, 6, 7, 8, 9, 11)                  | {0, 124689}                 |                    |
| 9765432:7   | $0, 0, e^{12}, -e^{13}, e^{14}, e^{15} + e^{23}, -e^{16} + e^{24}, e^{17} + e^{34}, e^{27} + e^{36} + e^{45}$                                                                                                                                                                                                                                         | 9/67(1, 3, 4, 5, 6, 7, 8, 9, 11)                  | {0, 124689}                 |                    |
| 9765432:12  | $0, 0, -e^{12}a_1, e^{13}a_1, e^{14}(1+a_1),$<br>$-e^{15}a_1 + e^{23}, e^{16}a_1 + e^{24}, e^{17} + e^{25} + e^{34}, e^{36} + e^{45} + e^{27}$                                                                                                                                                                                                        | 9/67(1, 3, 4, 5, 6, 7, 8, 9, 11)                  | {0, 124689}                 |                    |
| 9765432:16  | $0, 0, -\frac{2}{3}e^{12}, -\frac{5}{3}e^{13}, e^{14} - \frac{1}{2}e^{23},$<br>$\frac{1}{2}e^{24} + \frac{5}{3}e^{15}, e^{25} + e^{34} + \frac{2}{3}e^{16}, e^{26} + e^{35} + e^{17}, e^{36} + e^{27} + e^{45}$                                                                                                                                       | 3/19(1, 2, 3, 4, 5, 6, 7, 8, 9)                   | {0, 13579}                  |                    |
| 9765421:1   | $0, 0, -e^{12}, e^{13}, e^{14}, e^{15}, e^{34} + e^{25}, e^{16}, e^{18}$                                                                                                                                                                                                                                                                              | 1/191(16, 117, 133, 149, 165, 181, 282, 197, 213) | {0, 124679, 13578, 2345689} |                    |
| 9765421:2   | $0, 0, -e^{12}, e^{13}, e^{14}, e^{15}, e^{34} + e^{25}, e^{16}, e^{18} + e^{23}$                                                                                                                                                                                                                                                                     | 35/323(1, 5, 6, 7, 8, 9, 13, 10, 11)              | {0, 124679}                 |                    |
| 9765421:3   | $0, 0, -e^{12}, e^{13}, e^{14}, e^{15}, e^{25} + e^{34}, e^{16} + e^{23}, e^{18} + e^{24}$                                                                                                                                                                                                                                                            | 61/493(1, 4, 5, 6, 7, 8, 11, 9, 10)               | {0, 13578}                  |                    |
| 9765421:6   | $0, 0, -e^{12}, -e^{13}, e^{14}, e^{15}, e^{25} + e^{34}, e^{16}, e^{28} + e^{36} + e^{45}$                                                                                                                                                                                                                                                           | 2/23(1, 6, 7, 8, 9, 10, 15, 11, 17)               | {0, 124679, 135789, 234568} |                    |
| 9765421:9   | $0, 0, -e^{12}, -e^{13}, e^{14}, e^{15}, e^{25} + e^{34}, e^{23} + e^{16}, e^{28} + e^{45} + e^{36}$                                                                                                                                                                                                                                                  | 32/281(1, 4, 5, 6, 7, 8, 11, 9, 13)               | {0, 135789}                 |                    |
| 9765421:13  | $0, 0, -e^{12}, e^{13}, e^{14}, e^{23} - e^{15}, e^{34} + e^{25}, e^{24} + e^{16}, e^{28} + e^{36} + e^{45}$                                                                                                                                                                                                                                          | 9/67(1, 3, 4, 5, 6, 7, 9, 8, 11)                  | {0, 124679}                 |                    |
| 9765421:16  | $0, 0, -e^{12}, e^{13}, e^{14}, e^{25} + e^{34}, 2e^{15}, e^{25} + e^{27} + e^{16}, e^{36} + e^{28}$                                                                                                                                                                                                                                                  | 1/72(13, 18, 31, 44, 57, 75, 70, 88, 106)         | {0, 124679, 1356, 234579}   |                    |
| 9765421:19  | $0, 0, e^{12}, 3e^{13}, -e^{14}, -2e^{15}, e^{25} + e^{34}, e^{26} - e^{17} + e^{35}, e^{45} + e^{18} + e^{36}$                                                                                                                                                                                                                                       | 1/221(17, 109, 126, 143, 160, 177, 269, 286, 303) | {0, 124679, 13579, 23456}   |                    |
| 9765421:22  | $0, 0, e^{12}, 3e^{13}, -e^{14}, -2e^{15} + e^{23}, e^{25} + e^{34}, -e^{17} + e^{26} + e^{35}, e^{36} + e^{18} + e^{45}$                                                                                                                                                                                                                             | 28/219(1, 3, 4, 5, 6, 7, 9, 10, 11)               | {0, 124679}                 |                    |
| 9765421:25  | $0, 0, e^{12}, 3e^{13}, -e^{14} - \frac{3}{5}e^{23},$<br>$-2e^{15} + \frac{2}{5}e^{24}, e^{34} + e^{25}, e^{35} - e^{17} + e^{26}, e^{45} + e^{36} + e^{18} + e^{27}$                                                                                                                                                                                 | 3/19(1, 2, 3, 4, 5, 6, 7, 8, 9)                   | {0, 13579}                  |                    |
| 9764321:5   | $0, 0, -e^{12}, -e^{13}, e^{23}, e^{14}, e^{16}, e^{17}, e^{28} + e^{37} + e^{46}$                                                                                                                                                                                                                                                                    | 2/419(19, 113, 132, 151, 245, 170, 189, 208, 321) | {0, 124579, 135689, 234678} |                    |
| 9764321:6a  | $0, 0, -e^{12}, -e^{13}, e^{23}, e^{14}, e^{16}, e^{17} + e^{25}, e^{28} + e^{37} + e^{46}$                                                                                                                                                                                                                                                           | 7/41(1, 2, 3, 4, 5, 5, 6, 7, 9)                   | {0, 124579, 135689, 234678} |                    |
| 9764321:6b  | $0, 0, -e^{12}, -e^{13}, e^{23}, -e^{14}, e^{16}, e^{17} + e^{25}, e^{28} + e^{37} + e^{46}$                                                                                                                                                                                                                                                          | 7/41(1, 2, 3, 4, 5, 5, 6, 7, 9)                   | {0, 124579, 135689, 234678} |                    |
| 976542:3    | $0, 0, -e^{12}, e^{13}, e^{14}, 2e^{15}, e^{34} + e^{25}, e^{16}, e^{35} + e^{17} + e^{26}$                                                                                                                                                                                                                                                           | 1/293(32, 143, 175, 207, 239, 271, 382, 303, 414) | {0, 12467, 13578, 234568}   |                    |
| 976542:5    | $0, 0, -e^{12}, e^{13}, e^{14}, 2e^{15}, e^{34} + e^{25}, e^{16} + e^{23}, e^{17} + e^{35} + e^{26}$                                                                                                                                                                                                                                                  | 21/179(1, 4, 5, 6, 7, 8, 11, 9, 12)               | {0, 13578}                  |                    |
| 976542:6    | $0, 0, -e^{12}, e^{13}, e^{14}, e^{23} + 2e^{15}, e^{25} + e^{34}, e^{24} + e^{16}, e^{35} + e^{17} + e^{26}$                                                                                                                                                                                                                                         | 53/381(1, 3, 4, 5, 6, 7, 9, 8, 10)                | {0, 12467}                  |                    |
| 976431:1    | $0, 0, -e^{12}, e^{13}, e^{23}, e^{14}, e^{16}, e^{26} + e^{34}, e^{17}$                                                                                                                                                                                                                                                                              | 10/79(1, 4, 5, 6, 9, 7, 8, 11, 9)                 | {0, 124578, 135689, 234679} |                    |
| 976431:2a   | $0, 0, -e^{12}, e^{13}, e^{23}, e^{14}, e^{16}, e^{26} + e^{34}, e^{25} + e^{17}$                                                                                                                                                                                                                                                                     | 20/107(1, 2, 3, 4, 5, 5, 6, 7, 7)                 | {0, 124578, 135689, 234679} |                    |
| 976431:2b   | $0, 0, -e^{12}, -e^{13}, e^{23}, e^{14}, e^{16}, e^{26} + e^{34}, e^{17} + e^{25}$                                                                                                                                                                                                                                                                    | 20/107(1, 2, 3, 4, 5, 5, 6, 7, 7)                 | {0, 124578, 135689, 234679} |                    |
| 976431:5    | $0, 0, e^{12}, e^{13}, e^{23}, -e^{14}, e^{16} + e^{25}, e^{26} + e^{34}, e^{17} + e^{35}$                                                                                                                                                                                                                                                            | 35/333(2, 3, 5, 7, 8, 9, 11, 12, 13)              | {0, 234679}                 |                    |
| 976431:7    | $0, 0, -e^{12}, e^{13}, e^{23}, e^{14}, 2e^{16}, e^{26} + e^{34}, e^{36} + e^{18} + e^{27}$                                                                                                                                                                                                                                                           | 1/293(37, 133, 170, 207, 303, 244, 281, 377, 414) | {0, 124578, 13568, 23467}   |                    |
| 976431:8    | $0, 0, -e^{12}, e^{13}, e^{23}, e^{14}, e^{26} + e^{34}, e^{25} + 2e^{16}, e^{17} + e^{28} + e^{36}$                                                                                                                                                                                                                                                  | 71/693(2, 3, 5, 7, 8, 9, 12, 11, 14)              | {0, 23468}                  |                    |
| 976431:13   | $0, 0, e^{12}, e^{13}, -e^{23}, e^{24} - e^{15}, e^{34} + e^{16}, e^{35} + e^{26}, e^{27} + e^{45} + e^{18}$                                                                                                                                                                                                                                          | 5/21(1, 1, 2, 3, 3, 4, 5, 5, 6)                   | {0, 124578, 13579, 23489}   |                    |
| 976431:14a  | $0, 0, e^{12}, e^{13}, -e^{23}, -e^{14} + e^{25}, e^{26} + e^{34}, e^{35} + e^{16}, e^{45} + e^{27} + e^{18}$                                                                                                                                                                                                                                         | 5/21(1, 1, 2, 3, 3, 4, 5, 5, 6)                   | {0, 124578, 135679, 234689} |                    |
| 976431:14b  | $0, 0, -e^{12}, e^{13}, -e^{23}, e^{25} + e^{14}, e^{26} + e^{34}, e^{35} - e^{16}, e^{27} + e^{18} + e^{45}$                                                                                                                                                                                                                                         | 5/21(1, 1, 2, 3, 3, 4, 5, 5, 6)                   | {0, 124578, 135679, 234689} |                    |
| 976421:2    | $0, 0, e^{12}, e^{13}, e^{23}, e^{14}, e^{15} + e^{24}, e^{16}, e^{18}$                                                                                                                                                                                                                                                                               | 1/413(56, 211, 267, 323, 478, 379, 534, 435, 491) | {0, 12458, 13569, 234689}   |                    |
| 976421:6    | $0, 0, -e^{12}, e^{13}, e^{23}, e^{14}, e^{25}, e^{16}, e^{34} + e^{26} + e^{18}$                                                                                                                                                                                                                                                                     | 20/107(1, 2, 3, 4, 5, 5, 7, 6, 7)                 | {0, 135679}                 |                    |
| 976421:7    | $0, 0, e^{12}, e^{13}, e^{23}, e^{14}, e^{24} + e^{15}, e^{16} + e^{25}, e^{35} + e^{18}$                                                                                                                                                                                                                                                             | 34/311(2, 3, 5, 7, 8, 9, 10, 11, 13)              | {0, 234689}                 |                    |
| 976421:11   | $0, 0, -e^{12}, e^{13}, e^{23}, e^{14}, e^{24} + e^{15}, e^{16}, e^{18} + e^{27} + e^{35}$                                                                                                                                                                                                                                                            | 34/311(2, 3, 5, 7, 8, 9, 10, 11, 13)              | {0, 234689}                 |                    |

Table A.4 – Continued to next page

Table A.4 – Continued from previous page

| Name       | g                                                                                                                                                            | N                                                 | S <sub>0</sub>              | S = S <sub>0</sub> |
|------------|--------------------------------------------------------------------------------------------------------------------------------------------------------------|---------------------------------------------------|-----------------------------|--------------------|
| 976421:14  | $0, 0, -(-1 + a_3)e^{12}, a_3e^{13}, e^{23}, e^{14}, a_3e^{15} + e^{24}, e^{16} + e^{25}, e^{27} + e^{18} + e^{35}$                                          | 34/311(2, 3, 5, 7, 8, 9, 10, 11, 13)              | {0, 234689}                 |                    |
| 976421:21  | $0, 0, e^{12}, e^{13}, e^{23}, e^{14}, e^{15} + e^{24}, 2e^{17} + e^{26} + e^{34}, e^{36} + e^{18}$                                                          | 1/16(2, 7, 9, 11, 16, 13, 18, 20, 22)             | {0, 12458, 13568, 2346}     |                    |
| 976421:23  | $0, 0, e^{12}, e^{13}, e^{23}, e^{14}, e^{15} + e^{24}, e^{34} + 2e^{17} + e^{26}, e^{36} + e^{18} + e^{25}$                                                 | 53/381(1, 3, 4, 5, 7, 6, 8, 9, 10)                | {0, 12458}                  |                    |
| 976421:25  | $0, 0, -e^{12}, -e^{13}, -\frac{1}{2}e^{23}, \frac{1}{2}e^{24} + e^{15}, \frac{3}{2}e^{14}, e^{34} + e^{27} + e^{16}, e^{28} + e^{36} + e^{45}$              | 1/221(49, 62, 111, 160, 173, 222, 209, 271, 333)  | {0, 12458, 135789, 23479}   |                    |
| 976421:28a | $0, 0, -e^{12}, e^{13}, -\frac{1}{2}e^{23}, \frac{1}{2}e^{24} - e^{15}, \frac{3}{2}e^{14} + e^{25}, e^{27} + e^{16} + e^{34}, e^{36} + e^{45} + e^{28}$      | 29/117(1, 1, 2, 3, 3, 4, 4, 5, 6)                 | {0, 12458, 135789, 23479}   |                    |
| 976421:28b | $0, 0, -e^{12}, -e^{13}, -\frac{1}{2}e^{23}, \frac{1}{2}e^{24} + e^{15}, e^{25} + \frac{3}{2}e^{14}, e^{34} + e^{27} + e^{16}, e^{36} + e^{28} + e^{45}$     | 29/117(1, 1, 2, 3, 3, 4, 4, 5, 6)                 | {0, 12458, 135789, 23479}   |                    |
| 97642:1    | $0, 0, -e^{12}, e^{13}, e^{23}, e^{14}, e^{25}, e^{16}, e^{26} + e^{34}$                                                                                     | 4/483(25, 42, 67, 92, 109, 117, 151, 142, 159)    | {0, 124589, 135679, 234678} |                    |
| 97642:2    | $0, 0, -e^{12}, e^{13}, e^{23}, e^{14}, e^{15} + e^{24}, e^{16}, e^{26} + e^{34}$                                                                            | 1/281(47, 121, 168, 215, 289, 262, 336, 309, 383) | {0, 124589, 13569, 23468}   |                    |
| 97642:3    | $0, 0, -e^{12}, e^{13}, e^{23}, e^{14}, e^{15} + e^{24}, e^{26} + e^{34}, e^{16} + e^{25}$                                                                   | 67/597(2, 3, 5, 7, 8, 9, 10, 12, 11)              | {0, 23469}                  |                    |
| 97642:4    | $0, 0, e^{12}, -e^{13}, e^{23}, -e^{15} + e^{24}, e^{14}, e^{34} + e^{16}, e^{35} + e^{26}$                                                                  | 1/83(21, 23, 44, 65, 67, 88, 86, 109, 111)        | {0, 124589, 13578, 23479}   |                    |
| 97642:5a   | $0, 0, e^{12}, -e^{13}, e^{23}, -e^{15} + e^{24}, e^{14} + e^{25}, e^{16} + e^{34}, e^{35} + e^{26}$                                                         | 14/53(1, 1, 2, 3, 3, 4, 4, 5, 5)                  | {0, 124589, 13578, 23479}   |                    |
| 97642:5b   | $0, 0, e^{12}, -e^{13}, e^{23}, e^{24} - e^{15}, -e^{14} + e^{25}, e^{16} + e^{34}, e^{35} + e^{26}$                                                         | 14/53(1, 1, 2, 3, 3, 4, 4, 5, 5)                  | {0, 124589, 13578, 23479}   |                    |
| 97642:6a   | $0, 0, e^{12}, e^{13}, e^{23}, e^{25} - e^{14}, e^{24} + e^{15}, e^{26} + e^{34}, e^{35} + e^{16}$                                                           | 14/53(1, 1, 2, 3, 3, 4, 4, 5, 5)                  | {0, 124589, 13568, 23469}   |                    |
| 97642:6b   | $0, 0, e^{12}, -e^{13}, e^{23}, e^{25} - e^{14}, -e^{15} + e^{24}, e^{26} + e^{34}, e^{16} + e^{35}$                                                         | 14/53(1, 1, 2, 3, 3, 4, 4, 5, 5)                  | {0, 124589, 13568, 23469}   |                    |
| 97642:9    | $0, 0, -e^{12}, e^{13}, e^{23}, e^{14}, e^{25}, e^{26} + e^{34}, e^{27}$                                                                                     | 1/279(83, 66, 149, 232, 215, 315, 281, 381, 347)  | {0, 124589, 1356789, 23467} |                    |
| 97642:11   | $0, 0, e^{12}, e^{13}, e^{23}, e^{14}, e^{15} + e^{24}, e^{16}, e^{17} + e^{34}$                                                                             | 1/281(47, 121, 168, 215, 289, 262, 336, 309, 383) | {0, 124589, 13569, 23468}   |                    |
| 97642:12   | $0, 0, -e^{12}, e^{13}, e^{23}, e^{14}, e^{15} + e^{24}, e^{16}, e^{35} + e^{27}$                                                                            | 2/99(11, 16, 27, 38, 43, 49, 54, 60, 70)          | {0, 124589, 1356, 234689}   |                    |
| 97642:13   | $0, 0, -e^{12}, e^{13}, e^{23}, e^{14}, e^{25}, e^{26} + e^{34}, e^{27} + e^{16}$                                                                            | 14/53(1, 1, 2, 3, 3, 4, 4, 5, 5)                  | {0, 124589}                 |                    |
| 97642:14   | $0, 0, e^{12}, e^{13}, e^{23}, -e^{14}, e^{25}, e^{26} + e^{34}, e^{35} + e^{17}$                                                                            | 14/53(1, 1, 2, 3, 3, 4, 4, 5, 5)                  | {0, 124589, 135678, 234679} |                    |
| 97642:16   | $0, 0, e^{12}, e^{13}, e^{23}, e^{14}, e^{15} + e^{24}, e^{16}, e^{34} + e^{17} + e^{25}$                                                                    | 13/67(1, 2, 3, 4, 5, 5, 6, 6, 7)                  | {0, 13569}                  |                    |
| 97642:17   | $0, 0, e^{12}, e^{13}, e^{23}, e^{14}, e^{24} + e^{15}, e^{16} + e^{25}, e^{34} + e^{17}$                                                                    | 67/597(2, 3, 5, 7, 8, 9, 10, 11, 12)              | {0, 23468}                  |                    |
| 97642:19   | $0, 0, e^{12}a_1, e^{13}, e^{23}, -(-1 + a_1)e^{14}, e^{15} + e^{24}, e^{16}, e^{17} + e^{26} + e^{34}$                                                      | 1/281(47, 121, 168, 215, 289, 262, 336, 309, 383) | {0, 124589, 13569, 23468}   |                    |
| 97642:20   | $0, 0, -e^{12}, e^{13}, e^{23}, e^{14}, e^{24} + e^{15}, e^{34} + e^{26}, e^{35} + e^{27}$                                                                   | 1/83(21, 23, 44, 65, 67, 86, 88, 109, 111)        | {0, 124589, 13568, 23469}   |                    |
| 97642:21   | $0, 0, -e^{12}, e^{13}, e^{23}, e^{24} + e^{15}, e^{14}, e^{35} + e^{26}, e^{27} + e^{16}$                                                                   | 1/83(21, 23, 44, 65, 67, 88, 86, 111, 109)        | {0, 124589, 13579, 23478}   |                    |
| 97642:22a  | $0, 0, e^{12}, e^{13}, e^{23}, e^{24} + e^{15}, e^{25} + e^{14}, e^{34} + e^{16}, e^{35} + e^{17}$                                                           | 14/53(1, 1, 2, 3, 3, 4, 4, 5, 5)                  | {0, 124589, 13578, 23479}   |                    |
| 97642:22b  | $0, 0, e^{12}, -e^{13}, e^{23}, -e^{15} + e^{24}, e^{25} + e^{14}, e^{16} + e^{34}, e^{17} + e^{35}$                                                         | 14/53(1, 1, 2, 3, 3, 4, 4, 5, 5)                  | {0, 124589, 13578, 23479}   |                    |
| 97642:23a  | $0, 0, e^{12}, e^{13}, e^{23}, e^{24} + e^{15}, e^{25} + e^{14}, e^{16} + e^{34}, e^{17} + e^{26}$                                                           | 14/53(1, 1, 2, 3, 3, 4, 4, 5, 5)                  | {0, 124589, 13578, 23479}   |                    |
| 97642:23b  | $0, 0, e^{12}, e^{13}, e^{23}, e^{15} + e^{24}, e^{25} - e^{14}, e^{16} + e^{34}, e^{17} + e^{26}$                                                           | 14/53(1, 1, 2, 3, 3, 4, 4, 5, 5)                  | {0, 124589, 13578, 23479}   |                    |
| 97642:24a  | $0, 0, e^{12}, e^{13}, e^{23}, -e^{14} + e^{25}, e^{15} + e^{24}, e^{26} + e^{34}, e^{16} + e^{27}$                                                          | 14/53(1, 1, 2, 3, 3, 4, 4, 5, 5)                  | {0, 124589, 13568, 23469}   |                    |
| 97642:24b  | $0, 0, -e^{12}, e^{13}, e^{23}, e^{25} + e^{14}, e^{15} + e^{24}, e^{34} + e^{26}, e^{27} + e^{16}$                                                          | 14/53(1, 1, 2, 3, 3, 4, 4, 5, 5)                  | {0, 124589, 13568, 23469}   |                    |
| 97642:26   | $0, 0, e^{12}a_1, e^{13}, e^{23}, -(-1 + a_1)e^{14}, e^{24} + e^{15}, e^{25} + e^{16}, e^{26} + e^{34} + e^{17}$                                             | 67/597(2, 3, 5, 7, 8, 9, 10, 11, 12)              | {0, 23468}                  |                    |
| 97642:30   | $0, 0, -a_3e^{12}, a_3e^{13}, e^{23}, a_3e^{15} + e^{24}, (1 + a_3)e^{14}, e^{35} + e^{26}, e^{27} + e^{16} + e^{34}$                                        | 1/83(21, 23, 44, 65, 67, 88, 86, 111, 109)        | {0, 124589, 13579, 23478}   |                    |
| 97642:31a  | $0, 0, e^{12}a_1, -(-1 + a_1)e^{13}, e^{23}, e^{24} - (-1 + a_1)e^{15}, e^{25} + e^{14}, e^{16}a_1 + e^{34}, e^{26} + e^{35} + e^{17}$                       | 14/53(1, 1, 2, 3, 3, 4, 4, 5, 5)                  | {0, 124589, 13578, 23479}   |                    |
| 97642:31b  | $0, 0, e^{12}a_1, -(-1 + a_1)e^{13}, e^{23}, e^{24} - (-1 + a_1)e^{15}, e^{25} - e^{14}, e^{16}a_1 + e^{34}, e^{26} + e^{17} + e^{35}$                       | 14/53(1, 1, 2, 3, 3, 4, 4, 5, 5)                  | {0, 124589, 13578, 23479}   |                    |
| 97642:32a  | $0, 0, e^{12}, (-1 + a_4)e^{13}, e^{23}, e^{25}a_4 - e^{14}, (-1 + a_4)e^{15} + e^{24}, e^{26} + e^{34}, e^{16} + e^{27} + e^{35}$                           | 14/53(1, 1, 2, 3, 3, 4, 4, 5, 5)                  | {0, 124589, 13568, 23469}   |                    |
| 97642:32b  | $0, 0, -e^{12}, (1 + a_4)e^{13}, e^{23}, e^{25}a_4 + e^{14}, (1 + a_4)e^{15} + e^{24}, e^{26} + e^{34}, e^{27} + e^{16} + e^{35}$                            | 14/53(1, 1, 2, 3, 3, 4, 4, 5, 5)                  | {0, 124589, 13568, 23469}   |                    |
| 97642:33a  | $0, 0, -(-1 + a_2)e^{12}, e^{13}, e^{23}, a_2e^{14} + e^{25}, e^{15} + e^{24}, e^{16} + e^{27}, e^{17} + e^{26} + e^{34}$                                    | 14/53(1, 1, 2, 3, 3, 4, 4, 5, 5)                  | {0, 124589, 13569, 23468}   |                    |
| 97642:33b  | $0, 0, -(-1 + a_2)e^{12}, -e^{13}, e^{23}, a_2e^{14} + e^{25}, -e^{15} + e^{24}, e^{27} - e^{16}, e^{17} + e^{26} + e^{34}$                                  | 14/53(1, 1, 2, 3, 3, 4, 4, 5, 5)                  | {0, 124589, 13569, 23468}   |                    |
| 97642:36a  | $0, 0, e^{12}a_1, e^{13}, e^{23}, -(-1 + a_1)(e^{15} + e^{24}), -(a_4a_1 - a_4 + a_1)e^{14} + e^{25}, e^{16}a_4 + e^{27} + e^{34}, e^{26} + e^{35} + e^{17}$ | 14/53(1, 1, 2, 3, 3, 4, 4, 5, 5)                  | {0, 124589, 13578, 23479}   |                    |

Table A.4 – Continued to next page

Table A.4 – Continued from previous page

| Name       | $g$                                                                                                                                                              | $N$                                               | $S_0$                       | $S = S_0$ |
|------------|------------------------------------------------------------------------------------------------------------------------------------------------------------------|---------------------------------------------------|-----------------------------|-----------|
| 97642:36b  | $0, 0, e^{12}a_1, -e^{13}, e^{23}, -(1 + a_1)(e^{15} - e^{24}),$<br>$e^{14}(a_4a_1 - a_4 - a_1) + e^{25}, e^{16}a_4 + e^{27} + e^{34}, e^{17} + e^{26} + e^{35}$ | 14/53(1, 1, 2, 3, 3, 4, 4, 5, 5)                  | {0, 124589, 13578, 23479}   |           |
| 9654321:4  | $0, 0, 0, -e^{12}, e^{14}, e^{15}, e^{16}, e^{17} + e^{23}, e^{18} + e^{34}$                                                                                     | 1/9(1, 6, 5, 7, 8, 9, 10, 11, 12)                 | {0, 123579, 13468, 2456789} |           |
| 9654321:5  | $0, 0, 0, -e^{12}, e^{14}, e^{15}, e^{23} + e^{16}, e^{34} + e^{17}, e^{35} + e^{18}$                                                                            | 1/9(1, 6, 4, 7, 8, 9, 10, 11, 12)                 | {0, 12579, 1468, 2456789}   |           |
| 9654321:7  | $0, 0, 0, -e^{12}, e^{14}, e^{23} + e^{15}, e^{34} + e^{16}, e^{35} + e^{17}, e^{36} + e^{18}$                                                                   | 1/19(2, 13, 6, 15, 17, 19, 21, 23, 25)            | {0, 123579, 13468, 2456789} |           |
| 9654321:10 | $0, 0, 0, -e^{12}, e^{14}, e^{15}, e^{23} + e^{16}, e^{17} + e^{34}, e^{35} + e^{24} + e^{18}$                                                                   | 61/493(1, 5, 4, 6, 7, 8, 9, 10, 11)               | {0, 12579}                  |           |
| 9654321:12 | $0, 0, 0, -e^{12}, -e^{14}, e^{15}, e^{16}, e^{17} + e^{23}, e^{28} + e^{56} + e^{47}$                                                                           | 2/145(10, 33, 50, 43, 53, 63, 73, 83, 116)        | {0, 123579, 134689, 245678} |           |
| 9654321:20 | $0, 0, 0, -e^{12}, e^{14}, e^{23} + e^{15}, e^{16} + e^{34}, e^{17} + e^{35}, e^{18} + e^{36} + e^{24}$                                                          | 10/81(1, 5, 3, 6, 7, 8, 9, 10, 11)                | {0, 123579}                 |           |
| 9654321:24 | $0, 0, 0, e^{12}, e^{14}, e^{15}, e^{16} + e^{24}, e^{17} + e^{25}, e^{45} + e^{18} + e^{23}$                                                                    | 49/317(1, 3, 6, 4, 5, 6, 7, 8, 9)                 | {0, 12579}                  |           |
| 9654321:29 | $0, 0, 0, -e^{12}, e^{14}, e^{15} - e^{23}, e^{34} - e^{16}, e^{35} + e^{17}, e^{47} + e^{56} + e^{28}$                                                          | 8/55(1, 3, 3, 4, 5, 6, 7, 8, 11)                  | {0, 123579, 134689, 245678} |           |
| 9654321:41 | $0, 0, 0, -e^{12}, e^{14}, e^{23} + e^{15}, e^{16} + e^{34}, e^{35} + e^{24} + e^{17}, e^{36} + e^{25} + e^{18}$                                                 | 53/381(1, 4, 3, 5, 6, 7, 8, 9, 10)                | {0, 13468}                  |           |
| 9654321:45 | $0, 0, 0, -e^{12}, e^{14} + e^{23}, e^{34} + e^{15}, e^{35} + e^{16}, e^{36} + e^{17}, e^{37} + e^{18}$                                                          | 1/11(1, 8, 2, 9, 10, 11, 12, 13, 14)              | {0, 12579, 1468, 2456789}   |           |
| 9654321:65 | $0, 0, 0, -e^{12}, e^{14} + e^{23}, e^{15} + e^{34}, e^{16} + e^{35}, e^{17} + e^{36}, e^{18} + e^{24} + e^{37}$                                                 | 59/481(1, 5, 2, 6, 7, 8, 9, 10, 11)               | {0, 12579}                  |           |
| 9654321:78 | $0, 0, 0, -e^{12}, e^{23} + e^{14}, e^{15} + e^{34}, e^{35} + e^{16}, e^{24} + e^{36} + e^{17}, e^{37} + e^{25} + e^{18}$                                        | 13/94(1, 4, 2, 5, 6, 7, 8, 9, 10)                 | {0, 1468}                   |           |
| 9654321:88 | $0, 0, 0, -e^{12}, e^{14} + e^{23},$<br>$e^{15} + e^{34}, e^{16} + e^{24} + e^{35}, e^{25} + e^{17} + e^{36}, e^{37} + e^{26} + e^{18}$                          | 3/19(1, 3, 2, 4, 5, 6, 7, 8, 9)                   | {0, 12579}                  |           |
| 965431:3   | $0, 0, 0, -e^{12}, e^{14}, e^{15}, e^{16}, e^{26} + e^{45}, e^{17} + e^{23}$                                                                                     | 8/51(1, 3, 5, 4, 5, 6, 7, 9, 8)                   | {0, 123578, 134689, 245679} |           |
| 965431:6   | $0, 0, 0, -e^{12}, e^{14}, e^{15}, e^{23} + e^{16}, e^{26} + e^{45}, e^{17} + e^{34}$                                                                            | 1/369(62, 165, 248, 227, 289, 351, 413, 516, 475) | {0, 12578, 14689, 245679}   |           |
| 965431:12  | $0, 0, 0, -e^{12}, e^{14}, e^{15} + e^{23}, e^{34} + e^{16}, e^{45} + e^{26}, e^{17} + e^{35}$                                                                   | 2/23(2, 5, 6, 7, 9, 11, 13, 16, 15)               | {0, 123578, 134689, 245679} |           |
| 965431:41  | $0, 0, 0, -e^{12}, e^{14}, e^{15}, e^{23} + 2e^{16}, e^{45} + e^{26}, e^{46} + e^{27} + e^{18}$                                                                  | 1/36(7, 12, 28, 19, 26, 33, 40, 45, 52)           | {0, 12578, 1468, 24567}     |           |
| 965321:6   | $0, 0, 0, -e^{12}, e^{14}, e^{24}, e^{15}, e^{17} + e^{23}, e^{18} + e^{34}$                                                                                     | 1/441(74, 227, 296, 301, 375, 528, 449, 523, 597) | {0, 12568, 14679, 245789}   |           |
| 965321:9   | $0, 0, 0, -e^{12}, e^{14}, e^{24}, e^{15} + e^{23}, e^{17} + e^{34}, e^{18} + e^{35}$                                                                            | 4/371(16, 47, 48, 63, 79, 110, 95, 111, 127)      | {0, 123568, 134679, 245789} |           |
| 965321:10a | $0, 0, 0, e^{12}, e^{14}, e^{13} + e^{24}, e^{15}, e^{17}, e^{26} + e^{18} + e^{34}$                                                                             | 37/181(1, 2, 4, 3, 4, 5, 5, 6, 7)                 | {0, 12568, 14679, 245789}   |           |
| 965321:10b | $0, 0, 0, e^{12}, -e^{14}, e^{24} + e^{13}, e^{15}, e^{17}, e^{18} + e^{26} + e^{34}$                                                                            | 37/181(1, 2, 4, 3, 4, 5, 5, 6, 7)                 | {0, 12568, 14679, 245789}   |           |
| 965321:11a | $0, 0, 0, -e^{12}, e^{14}, e^{24}, e^{15}, e^{17} + e^{23}, e^{18} + e^{26} + e^{34}$                                                                            | 37/181(1, 2, 4, 3, 4, 5, 5, 6, 7)                 | {0, 12568, 14679, 245789}   |           |
| 965321:11b | $0, 0, 0, -e^{12}, -e^{14}, e^{24}, e^{15}, e^{17} + e^{23}, e^{34} + e^{18} + e^{26}$                                                                           | 37/181(1, 2, 4, 3, 4, 5, 5, 6, 7)                 | {0, 12568, 14679, 245789}   |           |
| 965321:16a | $0, 0, 0, (-1 + a_2)e^{12}, e^{14}, e^{13}a_2 + e^{24}, e^{15}, e^{23} + e^{17}, e^{18} + e^{26} + e^{34}$                                                       | 37/181(1, 2, 4, 3, 4, 5, 5, 6, 7)                 | {0, 12568, 14679, 245789}   |           |
| 965321:16b | $0, 0, 0, (-1 + a_2)e^{12}, -e^{14}, e^{13}a_2 + e^{24}, e^{15}, e^{17} + e^{23}, e^{18} + e^{26} + e^{34}$                                                      | 37/181(1, 2, 4, 3, 4, 5, 5, 6, 7)                 | {0, 12568, 14679, 245789}   |           |
| 965321:18a | $0, 0, 0, -e^{12}, e^{14}, e^{24}, e^{15} + e^{23}, e^{17} + e^{34}, e^{26} + e^{18} + e^{35}$                                                                   | 6/29(1, 2, 3, 3, 4, 5, 5, 6, 7)                   | {0, 123568, 134679, 245789} |           |
| 965321:18b | $0, 0, 0, -e^{12}, e^{14}, e^{24}, e^{23} - e^{15}, e^{17} + e^{34}, e^{18} + e^{26} + e^{35}$                                                                   | 6/29(1, 2, 3, 3, 4, 5, 5, 6, 7)                   | {0, 123568, 134679, 245789} |           |
| 965321:32  | $0, 0, 0, e^{12}, e^{24} + e^{13}, e^{14}, e^{34} + e^{25}, e^{35} + e^{27}, e^{28} + e^{37}$                                                                    | 1/107(55, 18, 36, 73, 91, 128, 109, 127, 145)     | {0, 12568, 145789, 24679}   |           |
| 965321:33  | $0, 0, 0, e^{12}, e^{14}, e^{24} + e^{13}, e^{23} + e^{15}, e^{17} + e^{26}, e^{35} + e^{46} + e^{18}$                                                           | 32/279(2, 3, 6, 5, 7, 8, 9, 11, 13)               | {0, 245789}                 |           |
| 965321:35  | $0, 0, 0, e^{12}, e^{14}, e^{24}, e^{15} + e^{23}, e^{26} + e^{34} - e^{17}, e^{35} + e^{18} + e^{46}$                                                           | 32/279(2, 3, 6, 5, 7, 8, 9, 11, 13)               | {0, 245789}                 |           |
| 965321:36  | $0, 0, 0, e^{12}, 2e^{14}, e^{13} + e^{24}, e^{15}, e^{17} + e^{34} + e^{26}, e^{18} + e^{46} + e^{35}$                                                          | 32/279(2, 3, 6, 5, 7, 8, 9, 11, 13)               | {0, 245789}                 |           |
| 965321:38  | $0, 0, 0, e^{12}, (2 + a_4)e^{14},$<br>$e^{24} + (1 + a_4)e^{13}, e^{15} + e^{23}, a_4e^{17} + e^{26} + e^{34}, e^{18} + e^{35} + e^{46}$                        | 32/279(2, 3, 6, 5, 7, 8, 9, 11, 13)               | {0, 245789}                 |           |
| 965321:40a | $0, 0, 0, e^{12}, e^{13} + e^{24}, e^{14}, e^{34} + e^{25}, e^{35} + e^{27}, e^{37} + e^{28} + e^{16}$                                                           | 35/169(2, 1, 2, 3, 4, 5, 5, 6, 7)                 | {0, 12568, 145789, 24679}   |           |
| 965321:40b | $0, 0, 0, e^{12}, e^{24} + e^{13}, -e^{14}, e^{34} + e^{25}, e^{35} + e^{27}, e^{28} + e^{37} + e^{16}$                                                          | 35/169(2, 1, 2, 3, 4, 5, 5, 6, 7)                 | {0, 12568, 145789, 24679}   |           |
| 965321:45  | $0, 0, 0, -e^{12}, e^{24} - e^{13}, e^{14}, e^{25} + e^{34}, e^{35} + e^{27} + e^{16}, e^{37} + e^{46} + e^{28}$                                                 | 31/269(3, 2, 4, 5, 7, 8, 9, 11, 13)               | {0, 145789}                 |           |
| 964321:16  | $0, 0, 0, a_1e^{12}, (1 + a_1)e^{13}, e^{14}, e^{16}, e^{17} + e^{23}, e^{25} + e^{18} + e^{34}$                                                                 | 1/119(20, 69, 80, 89, 100, 109, 129, 149, 169)    | {0, 12568, 14579, 246789}   |           |
| 964321:17  | $0, 0, 0, e^{12}, e^{13}, e^{14}, e^{16}, e^{17} + e^{24}, e^{18} + e^{26}$                                                                                      | 1/401(68, 204, 367, 272, 435, 340, 408, 476, 544) | {0, 12368, 12568, 35}       |           |
| 964321:21  | $0, 0, 0, e^{12}, -e^{13}, e^{14}, e^{23} + e^{16}, -2e^{17} + e^{25} + e^{34}, e^{45} + e^{18}$                                                                 | 1/87(16, 47, 48, 63, 64, 79, 95, 111, 127)        | {0, 12368, 13479, 246789}   |           |
| 964321:24  | $0, 0, 0, e^{12}, e^{13}, e^{14}, e^{16}, e^{24} + e^{17}, e^{26} + e^{18} + e^{35}$                                                                             | 14/155(2, 6, 7, 8, 9, 10, 12, 14, 16)             | {0, 35}                     |           |
| 964321:25  | $0, 0, 0, e^{12}, e^{13}, e^{24}, e^{26}, e^{27} + e^{14}, e^{16} + e^{28} + e^{35}$                                                                             | 42/473(6, 2, 5, 8, 11, 10, 12, 14, 16)            | {0, 35}                     |           |
| 964321:29  | $0, 0, 0, e^{12}, e^{13}, e^{14}, e^{16} + e^{23}, e^{17} + e^{25}, e^{45} + e^{36} + e^{18}$                                                                    | 1/87(16, 47, 48, 63, 64, 79, 95, 111, 127)        | {0, 12368, 13479, 246789}   |           |
| 964321:31  | $0, 0, 0, e^{12}, e^{13}, 2e^{14}, e^{16}, e^{34} + e^{17} + e^{25}, e^{45} + e^{36} + e^{18}$                                                                   | 1/87(16, 47, 48, 63, 64, 79, 95, 111, 127)        | {0, 12368, 13479, 246789}   |           |
| 964321:39  | $0, 0, 0, -e^{12}, e^{13}, e^{24}, e^{26} + e^{14}, e^{27} + e^{16}, e^{28} + e^{46}$                                                                            | 1/71(28, 14, 57, 42, 85, 56, 70, 84, 98)          | {0, 234579, 2479, 35}       |           |

Table A.4 – Continued to next page

Table A.4 – Continued from previous page

| Name       | g                                                                                                                                                                             | N                                                 | S <sub>0</sub>            | S = S <sub>0</sub> |
|------------|-------------------------------------------------------------------------------------------------------------------------------------------------------------------------------|---------------------------------------------------|---------------------------|--------------------|
| 964321:45  | $0, 0, 0, e^{12}, (1 + a_4)e^{13},$<br>$(2 + a_4)e^{14}, e^{16} + e^{23}, e^{34} + e^{25} + a_4e^{17}, e^{18} + e^{36} + e^{45}$                                              | 1/87(16, 47, 48, 63, 64, 79, 95, 111, 127)        | {0, 12368, 13479, 246789} |                    |
| 964321:47a | $0, 0, 0, e^{12}, e^{13}, e^{14}, e^{24} + e^{16}, e^{17} + e^{26}, e^{35} + e^{46} + e^{18}$                                                                                 | 7/33(1, 2, 3, 3, 4, 4, 5, 6, 7)                   | {0, 13479, 14579, 35}     |                    |
| 964321:47b | $0, 0, 0, e^{12}, -e^{13}, e^{14}, e^{24} + e^{16}, e^{26} + e^{17}, e^{35} + e^{18} + e^{46}$                                                                                | 7/33(1, 2, 3, 3, 4, 4, 5, 6, 7)                   | {0, 13479, 14579, 35}     |                    |
| 964321:48  | $0, 0, 0, -e^{12}, e^{13}, e^{24}, e^{14} + e^{26}, e^{27} + e^{16}, e^{28} + e^{46} + e^{35}$                                                                                | 35/333(4, 2, 5, 6, 9, 8, 10, 12, 14)              | {0, 35}                   |                    |
| 964321:49a | $0, 0, 0, e^{12}, e^{13}, e^{14}, e^{16} + e^{24}, e^{26} + e^{17}, e^{27} + e^{18} + e^{35}$                                                                                 | 7/33(1, 2, 3, 3, 4, 4, 5, 6, 7)                   | {0, 13479, 14579, 35}     |                    |
| 964321:49b | $0, 0, 0, -e^{12}, e^{13}, e^{14}, e^{24} + e^{16}, e^{17} + e^{26}, e^{27} + e^{18} + e^{35}$                                                                                | 7/33(1, 2, 3, 3, 4, 4, 5, 6, 7)                   | {0, 13479, 14579, 35}     |                    |
| 964321:64  | $0, 0, 0, a_1e^{12}, e^{13},$<br>$e^{14}, -(-1 + a_1)e^{16} + e^{24}, e^{26} + e^{17}, e^{18} + e^{46} + e^{27}$                                                              | 1/281(56, 112, 253, 168, 309, 224, 280, 336, 392) | {0, 13479, 14579, 35}     |                    |
| 964321:65  | $0, 0, 0, a_1e^{12}, e^{13},$<br>$e^{24}, -(-1 + a_1)e^{14} + e^{26}, -(-1 + a_1)e^{16} + e^{27}, e^{17} + e^{46} + e^{28}$                                                   | 1/71(28, 14, 57, 42, 85, 56, 70, 84, 98)          | {0, 234579, 2479, 35}     |                    |
| 964321:68a | $0, 0, 0, -(-1 + a_3)e^{12}, e^{13}, e^{14}, e^{16}a_3 + e^{24}, e^{17} + e^{26}, e^{18} + e^{27} + e^{46} + e^{35}$                                                          | 7/33(1, 2, 3, 3, 4, 4, 5, 6, 7)                   | {0, 13479, 14579, 35}     |                    |
| 964321:68b | $0, 0, 0, -(-1 + a_3)e^{12}, -e^{13}, e^{14}, e^{16}a_3 + e^{24}, e^{17} + e^{26}, e^{27} + e^{18} + e^{35} + e^{46}$                                                         | 7/33(1, 2, 3, 3, 4, 4, 5, 6, 7)                   | {0, 13479, 14579, 35}     |                    |
| 964321:69  | $0, 0, 0, a_1e^{12}, e^{13},$<br>$e^{24}, -(-1 + a_1)e^{14} + e^{26}, -(-1 + a_1)e^{16} + e^{27}, e^{28} + e^{17} + e^{35} + e^{46}$                                          | 35/333(4, 2, 5, 6, 9, 8, 10, 12, 14)              | {0, 35}                   |                    |
| 97641:1    | $0, 0, e^{12}, e^{13}, e^{23}, e^{14}, e^{25}, e^{24} + e^{15}, e^{16}$                                                                                                       | 1/151(34, 53, 87, 121, 140, 155, 193, 174, 189)   | {0, 12459, 13567, 234679} |                    |
| 97641:2    | $0, 0, -e^{12}, e^{13}, e^{23}, e^{14}, e^{25}, e^{24} + e^{15}, e^{26} + e^{34}$                                                                                             | 1/309(77, 96, 173, 250, 269, 327, 365, 346, 423)  | {0, 12459, 135679, 23467} |                    |
| 97641:3    | $0, 0, e^{12}, e^{13}, e^{23}, e^{15} + e^{24}, e^{14}, e^{25}, e^{34} + e^{16}$                                                                                              | 1/309(77, 96, 173, 250, 269, 346, 327, 365, 423)  | {0, 12459, 135789, 23478} |                    |
| 97641:6    | $0, 0, a_1e^{12}, e^{13}, e^{23}, -e^{14}(-1 + a_1), e^{15} + e^{24}, e^{25}, e^{17} + e^{26} + e^{34}$                                                                       | 1/309(77, 96, 173, 250, 269, 327, 346, 365, 423)  | {0, 12459, 135689, 23468} |                    |
| 97641:7a   | $0, 0, -e^{12}, e^{13}, e^{23}, e^{14}, e^{15} + e^{24}, e^{25}, e^{27} + e^{16} + e^{35}$                                                                                    | 27/97(1, 1, 2, 3, 3, 4, 4, 4, 5)                  | {0, 12459, 13568, 234689} |                    |
| 97641:7b   | $0, 0, -e^{12}, e^{13}, e^{23}, -e^{14}, e^{15} + e^{24}, e^{25}, e^{16} + e^{35} + e^{27}$                                                                                   | 27/97(1, 1, 2, 3, 3, 4, 4, 4, 5)                  | {0, 12459, 13568, 234689} |                    |
| 96532:2    | $0, 0, 0, -e^{12}, e^{14}, e^{24} + e^{13}, e^{15}, e^{17}, e^{45} + e^{27}$                                                                                                  | 1/373(57, 181, 362, 238, 295, 419, 352, 409, 533) | {0, 125689, 14679, 24578} |                    |
| 96532:4    | $0, 0, 0, -e^{12}, e^{14}, e^{24}, e^{15}, e^{23} + e^{17}, e^{45} + e^{27}$                                                                                                  | 1/417(85, 171, 340, 256, 341, 427, 426, 511, 597) | {0, 125689, 14679, 24578} |                    |
| 96532:12   | $0, 0, 0, -e^{12}, e^{14}, e^{13} + e^{24}, e^{15} + e^{23}, e^{27} + e^{45}, e^{26} + e^{17}$                                                                                | 63/533(2, 3, 6, 5, 7, 8, 9, 12, 11)               | {0, 24579}                |                    |
| 96532:14   | $0, 0, 0, -e^{12}, e^{14}, e^{24}, e^{15} + e^{23}, e^{27} + e^{45}, e^{17} + e^{26} + e^{34}$                                                                                | 63/533(2, 3, 6, 5, 7, 8, 9, 12, 11)               | {0, 24579}                |                    |
| 96532:15   | $0, 0, 0, -e^{12}a_3, e^{14},$<br>$-(-1 + a_3)e^{13} + e^{24}, e^{23} + e^{15}a_3, e^{45} + e^{27}, e^{34} + e^{17} + e^{26}$                                                 | 63/533(2, 3, 6, 5, 7, 8, 9, 12, 11)               | {0, 24579}                |                    |
| 96532:20   | $0, 0, 0, e^{12}, e^{24} + e^{13}, 2e^{14}, e^{25} + e^{34}, e^{27} + e^{35}, e^{45} + e^{36} + e^{17}$                                                                       | 1/261(99, 59, 118, 158, 217, 257, 276, 335, 375)  | {0, 125689, 14578, 24679} |                    |
| 96532:23   | $0, 0, 0, e^{12}, e^{24} + e^{13}, 2e^{14}, e^{25} + e^{34}, e^{27} + e^{16} + e^{35}, e^{17} + e^{36} + e^{45}$                                                              | 61/513(3, 2, 4, 5, 7, 8, 9, 11, 12)               | {0, 14578}                |                    |
| 96532:34   | $0, 0, 0, e^{12}, -e^{14}, e^{24} - e^{13}, -e^{16} + e^{25}, e^{45} + e^{17}, e^{46} + e^{27} + e^{35}$                                                                      | 2/11(1, 2, 4, 3, 4, 5, 6, 7, 8)                   | {0, 125689, 1468, 2459}   |                    |
| 96532:38a  | $0, 0, 0, e^{12}, -e^{13} + 3e^{24},$<br>$e^{14} + 2e^{23}, -e^{16} + e^{34} + e^{25}, e^{17} + e^{45}, e^{46} + e^{35} + e^{27}$                                             | 13/47(1, 1, 2, 2, 3, 3, 4, 5, 5)                  | {0, 125689, 14579, 24678} |                    |
| 96532:38b  | $0, 0, 0, e^{12}, 3e^{24} - e^{13}, 2e^{23} - e^{14}, -e^{16} + e^{25} + e^{34}, e^{45} + e^{17}, e^{35} + e^{46} + e^{27}$                                                   | 13/47(1, 1, 2, 2, 3, 3, 4, 5, 5)                  | {0, 125689, 14579, 24678} |                    |
| 96532:40a  | $0, 0, 0, e^{12}, e^{14} + e^{23}, e^{24} - e^{13}, e^{26} - e^{15}, e^{46} - e^{35} + e^{17}, e^{45} + e^{36} + e^{27}$                                                      | 13/47(1, 1, 2, 2, 3, 3, 4, 5, 5)                  | {0, 125689, 14679, 24578} |                    |
| 96532:40b  | $0, 0, 0, e^{12}, -e^{14} + e^{23}, -e^{13} + e^{24}, e^{26} - e^{15}, e^{17} + e^{46} + e^{35}, e^{45} + e^{27} + e^{36}$                                                    | 13/47(1, 1, 2, 2, 3, 3, 4, 5, 5)                  | {0, 125689, 14679, 24578} |                    |
| 96532:41a  | $0, 0, 0, e^{12}, -e^{24} + e^{13}, e^{23} + e^{14}, e^{26} - e^{15}, e^{17} + e^{46} - e^{35}, e^{27} + e^{36} + e^{45}$                                                     | 13/47(1, 1, 2, 2, 3, 3, 4, 5, 5)                  | {0, 125689, 1458, 2469}   |                    |
| 96532:41b  | $0, 0, 0, e^{12}, e^{24} - e^{13}, e^{23} - e^{14}, -e^{15} + e^{26}, e^{17} + e^{35} + e^{46}, e^{27} + e^{36} + e^{45}$                                                     | 13/47(1, 1, 2, 2, 3, 3, 4, 5, 5)                  | {0, 125689, 1458, 2469}   |                    |
| 96532:42a  | $0, 0, 0, e^{12}, e^{14}, e^{13} + e^{24}, -e^{15} + e^{26} + e^{34}, e^{17} + 2e^{35} + e^{46}, e^{36} + e^{27} + e^{45}$                                                    | 13/47(1, 1, 2, 2, 3, 3, 4, 5, 5)                  | {0, 125689, 14679, 24578} |                    |
| 96532:42b  | $0, 0, 0, e^{12}, -e^{14}, e^{13} + e^{24}, e^{26} - e^{15} + e^{34}, e^{17} + e^{46} - 2e^{35}, e^{27} + e^{45} + e^{36}$                                                    | 13/47(1, 1, 2, 2, 3, 3, 4, 5, 5)                  | {0, 125689, 14679, 24578} |                    |
| 96532:43a  | $0, 0, 0,$<br>$e^{12}, a_4e^{23} + e^{14}, -e^{13}(-1 + a_4) + (1 + a_4)e^{24},$<br>$-e^{15} + e^{34} + e^{26}, e^{17} + e^{46} - (-2 + a_4)e^{35}, e^{27} + e^{36} + e^{45}$ | 13/47(1, 1, 2, 2, 3, 3, 4, 5, 5)                  | {0, 125689, 14679, 24578} |                    |
| 96532:43b  | $0, 0, 0,$<br>$e^{12}, a_4e^{23} - e^{14}, -e^{13}(-1 + a_4) + (1 + a_4)e^{24},$<br>$-e^{15} + e^{26} + e^{34}, e^{46} + e^{17} + (-2 + a_4)e^{35}, e^{36} + e^{45} + e^{27}$ | 13/47(1, 1, 2, 2, 3, 3, 4, 5, 5)                  | {0, 125689, 14679, 24578} |                    |

Table A.4 – Continued to next page

Table A.4 – Continued from previous page

| Name      | g                                                                                                                                                                | N                                                  | S <sub>0</sub>              | S = S <sub>0</sub> |
|-----------|------------------------------------------------------------------------------------------------------------------------------------------------------------------|----------------------------------------------------|-----------------------------|--------------------|
| 96531:5   | $0, 0, 0, e^{12}, e^{14}, e^{24} + e^{13}, e^{15}, e^{26} + e^{34}, e^{17}$                                                                                      | 1/501(106, 201, 402, 307, 413, 508, 519, 709, 625) | {0, 12569, 14678, 245789}   |                    |
| 96531:8   | $0, 0, 0, e^{12}, e^{14}, e^{13} + e^{24}, e^{15}, e^{25} + e^{16}, e^{17}$                                                                                      | 1/178(31, 86, 172, 117, 148, 203, 179, 234, 210)   | {0, 12569, 1467, 24579}     |                    |
| 96531:9   | $0, 0, 0, -e^{12}, e^{14}, e^{24}, e^{15} + e^{23}, e^{26}, e^{34} + e^{17}$                                                                                     | 2/177(23, 30, 69, 53, 76, 83, 99, 113, 122)        | {0, 123569, 134678, 245789} |                    |
| 96531:10  | $0, 0, 0, e^{12}, e^{14}, e^{24}, e^{15}, e^{16} + e^{25}, e^{17} + e^{23}$                                                                                      | 3/14(1, 2, 4, 3, 4, 5, 5, 6, 6)                    | {0, 12569, 1467, 24579}     |                    |
| 96531:12  | $0, 0, 0, -e^{12}, e^{14}, e^{24}, e^{15}, e^{26} + e^{13}, e^{27} + e^{45}$                                                                                     | 2/491(61, 80, 240, 141, 202, 221, 263, 301, 343)   | {0, 123569, 146789, 234578} |                    |
| 96531:15  | $0, 0, 0, -e^{12}, e^{14}, e^{24}, e^{15} + e^{23}, e^{26}, e^{45} + e^{27}$                                                                                     | 1/223(64, 65, 192, 129, 193, 194, 257, 259, 322)   | {0, 123569, 1346789, 24578} |                    |
| 96531:19  | $0, 0, 0, -e^{12}, e^{14}, e^{24}, e^{15} + e^{23}, e^{16} + e^{25}, e^{17} + e^{34}$                                                                            | 1/47(11, 19, 33, 30, 41, 49, 52, 60, 63)           | {0, 123569, 13467, 24579}   |                    |
| 96531:21  | $0, 0, 0, -e^{12}, e^{14}, -e^{13} + e^{24}, e^{15}, e^{34} + e^{26}, e^{27} + e^{45}$                                                                           | 1/361(79, 134, 268, 213, 292, 347, 371, 481, 505)  | {0, 12569, 146789, 24578}   |                    |
| 96531:24  | $0, 0, 0, -e^{12}, e^{14}, e^{13} + e^{24}, e^{15}, e^{25} + e^{16}, e^{27} + e^{45}$                                                                            | 1/128(22, 57, 114, 79, 101, 136, 123, 158, 180)    | {0, 12569, 14679, 2457}     |                    |
| 96531:25  | $0, 0, 0, -e^{12}, e^{14}, e^{24}, e^{15} + e^{23}, e^{16} + e^{25}, e^{27} + e^{45}$                                                                            | 1/71(19, 23, 57, 42, 61, 65, 80, 84, 103)          | {0, 123569, 134679, 2457}   |                    |
| 96531:26  | $0, 0, 0, -e^{12}, e^{14}, e^{24} - e^{13}, e^{15} + e^{23}, e^{26} + e^{34}, e^{27} + e^{45}$                                                                   | 63/533(2, 3, 6, 5, 7, 8, 9, 11, 12)                | {0, 24578}                  |                    |
| 96531:29  | $0, 0, 0, e^{12}, e^{13} + e^{24}, e^{14}, e^{34} + e^{25}, e^{16}, e^{35} + e^{27}$                                                                             | 5/441(29, 24, 48, 53, 77, 82, 101, 111, 125)       | {0, 12569, 145789, 24678}   |                    |
| 96531:30  | $0, 0, 0, -e^{12}, e^{14}, e^{24}, e^{23} + e^{15}, e^{16} + e^{25}, e^{17} + e^{26} + e^{34}$                                                                   | 61/489(2, 3, 6, 5, 7, 8, 9, 10, 11)                | {0, 24579}                  |                    |
| 96531:31  | $0, 0, 0, e^{12}, e^{14}, e^{24} + e^{13}, e^{15}, e^{25} + e^{16}, e^{26} + e^{34} + e^{17}$                                                                    | 61/489(2, 3, 6, 5, 7, 8, 9, 10, 11)                | {0, 24579}                  |                    |
| 96531:32  | $0, 0, 0, -e^{12}, e^{14}, e^{13} + e^{24}, e^{15} + e^{23}, e^{25} + e^{16}, e^{45} + e^{27}$                                                                   | 31/256(2, 3, 6, 5, 7, 8, 9, 10, 12)                | {0, 2457}                   |                    |
| 96531:36  | $0, 0, 0, a_1 e^{12}, e^{14}, e^{24} + (1 + a_1) e^{13}, e^{15} + e^{23}, e^{16} + e^{25}, e^{17} + e^{26} + e^{34}$                                             | 61/489(2, 3, 6, 5, 7, 8, 9, 10, 11)                | {0, 24579}                  |                    |
| 96531:38  | $0, 0, 0, e^{12}, e^{13} + e^{24}, e^{14}, e^{25} + e^{34}, e^{26} + e^{15}, e^{27} + e^{35}$                                                                    | 1/33(13, 8, 16, 21, 29, 34, 37, 42, 45)            | {0, 12569, 14579, 2467}     |                    |
| 96531:39  | $0, 0, 0, e^{12}, e^{24} + e^{13}, e^{14}, e^{34} + e^{25}, e^{16}, e^{36} + e^{45} + e^{17}$                                                                    | 1/341(92, 107, 214, 199, 306, 291, 413, 383, 505)  | {0, 12569, 14578, 246789}   |                    |
| 96531:44  | $0, 0, 0, e^{12}, e^{13} + e^{24}, e^{14}, e^{34} + e^{25}, e^{26} + e^{15}, e^{27} + e^{35} + e^{16}$                                                           | 59/469(3, 2, 4, 5, 7, 8, 9, 10, 11)                | {0, 14579}                  |                    |
| 96531:46  | $0, 0, 0, e^{12}, e^{24} + e^{13}, 2e^{14}, e^{25} + e^{34}, 2e^{15} + e^{26}, e^{17} + e^{36} + e^{45}$                                                         | 5/17(1, 1, 2, 2, 3, 3, 4, 4, 5)                    | {0, 12569, 1457, 24679}     |                    |
| 96531:52  | $0, 0, 0, -e^{12}, e^{14}, e^{24}, e^{16} + e^{25}, e^{23} + e^{15}, e^{46} + e^{27}$                                                                            | 1/123(39, 31, 117, 70, 109, 101, 140, 148, 171)    | {0, 123569, 13468, 24589}   |                    |
| 96531:64  | $0, 0, 0, e^{12}, e^{13} + e^{24}, e^{14}, e^{26} + e^{15}, e^{34} + e^{25}, e^{46} + e^{17}$                                                                    | 1/33(7, 12, 24, 19, 31, 26, 38, 43, 45)            | {0, 12569, 14589, 2468}     |                    |
| 96531:66  | $0, 0, 0, -e^{12}, e^{14}, e^{24} + e^{13}, e^{16} + e^{25}, e^{15}, e^{46} + e^{27} + e^{35}$                                                                   | 1/46(11, 16, 32, 27, 38, 43, 54, 49, 70)           | {0, 12569, 1468, 24589}     |                    |
| 96531:70  | $0, 0, 0, -e^{12}, e^{13} - e^{24}, -e^{14}, e^{26} + e^{15}, e^{25} + e^{34}, e^{45} + e^{27} + e^{36}$                                                         | 5/17(1, 1, 2, 2, 3, 3, 4, 4, 5)                    | {0, 12569, 1458, 24689}     |                    |
| 96531:73a | $0, 0, 0, e^{12}, -e^{14} - e^{23}, e^{24} - e^{13}, -e^{16} + e^{25}, e^{15} + e^{34}, e^{27} + e^{35} + e^{46}$                                                | 5/17(1, 1, 2, 2, 3, 3, 4, 4, 5)                    | {0, 12569, 1468, 24589}     |                    |
| 96531:73b | $0, 0, 0, -e^{12}, e^{14} + e^{23}, e^{13} + e^{24}, e^{25} + e^{16}, e^{15} + e^{34}, e^{27} + e^{46} + e^{35}$                                                 | 5/17(1, 1, 2, 2, 3, 3, 4, 4, 5)                    | {0, 12569, 1468, 24589}     |                    |
| 96531:74a | $0, 0, 0, e^{12}, -e^{13} + e^{24}, e^{14} + e^{23}, -2e^{16} + e^{34} + e^{25}, e^{15} + e^{26}, e^{17} + e^{45}$                                               | 5/17(1, 1, 2, 2, 3, 3, 4, 4, 5)                    | {0, 12569, 1457, 24679}     |                    |
| 96531:74b | $0, 0, 0, e^{12}, e^{24} - e^{13}, e^{23} - e^{14}, -2e^{16} + e^{25} + e^{34}, -e^{15} + e^{26}, e^{45} + e^{17}$                                               | 5/17(1, 1, 2, 2, 3, 3, 4, 4, 5)                    | {0, 12569, 1457, 24679}     |                    |
| 96531:78a | $0, 0, 0, e^{12}, e^{14} + e^{23}, e^{24} + e^{13}, e^{16} + e^{25}, e^{15} + e^{26}, e^{17} + e^{36} + e^{45}$                                                  | 5/17(1, 1, 2, 2, 3, 3, 4, 4, 5)                    | {0, 12569, 14689, 2458}     |                    |
| 96531:78b | $0, 0, 0, -e^{12}, -e^{14} + e^{23}, e^{13} + e^{24}, e^{25} - e^{16}, e^{26} + e^{15}, e^{17} + e^{45} + e^{36}$                                                | 5/17(1, 1, 2, 2, 3, 3, 4, 4, 5)                    | {0, 12569, 14689, 2458}     |                    |
| 96531:79a | $0, 0, 0, e^{12}, e^{24} + e^{13}, e^{23} + e^{14}, e^{25} + e^{16}, e^{26} + e^{15}, e^{36} + e^{45} + e^{17}$                                                  | 5/17(1, 1, 2, 2, 3, 3, 4, 4, 5)                    | {0, 12569, 1457, 24679}     |                    |
| 96531:79b | $0, 0, 0, e^{12}, -e^{24} - e^{13}, e^{23} - e^{14}, -e^{16} + e^{25}, e^{15} + e^{26}, e^{36} + e^{45} + e^{17}$                                                | 5/17(1, 1, 2, 2, 3, 3, 4, 4, 5)                    | {0, 12569, 1457, 24679}     |                    |
| 96531:81a | $0, 0, 0, e^{12}, e^{14}, e^{24} + e^{13}, e^{26} + e^{34} - e^{15}, e^{16} + e^{25}, e^{27} + e^{36} + e^{45}$                                                  | 5/17(1, 1, 2, 2, 3, 3, 4, 4, 5)                    | {0, 12569, 14679, 2457}     |                    |
| 96531:81b | $0, 0, 0, -e^{12}, e^{14}, e^{24} - e^{13}, e^{15} + e^{26} + e^{34}, e^{16} + e^{25}, e^{27} + e^{36} + e^{45}$                                                 | 5/17(1, 1, 2, 2, 3, 3, 4, 4, 5)                    | {0, 12569, 14679, 2457}     |                    |
| 96531:82a | $0, 0, 0, e^{12}, (1 + a_4) e^{13} + e^{24}, e^{14} + e^{23}, e^{15} + e^{26}, a_4 e^{16} + e^{25} + e^{34}, e^{17} + e^{35} + e^{46}$                           | 5/17(1, 1, 2, 2, 3, 3, 4, 4, 5)                    | {0, 12569, 14589, 2468}     |                    |
| 96531:82b | $0, 0, 0, e^{12}, (1 + a_4) e^{13} + e^{24}, -e^{14} + e^{23}, e^{26} - e^{15}, a_4 e^{16} + e^{34} + e^{25}, e^{46} + e^{35} + e^{17}$                          | 5/17(1, 1, 2, 2, 3, 3, 4, 4, 5)                    | {0, 12569, 14589, 2468}     |                    |
| 96531:83a | $0, 0, 0, e^{12}, (1 + a_4) e^{13} + (2 + a_4) e^{24}, (2 + a_4) e^{14} + e^{23}, a_4 e^{16} + e^{34} + e^{25}, e^{26} + e^{15}, e^{36} + e^{45} + e^{17}$       | 5/17(1, 1, 2, 2, 3, 3, 4, 4, 5)                    | {0, 12569, 1457, 24679}     |                    |
| 96531:83b | $0, 0, 0, e^{12}, -e^{13}(-1 + a_4) + (-2 + a_4) e^{24}, -(-2 + a_4) e^{14} + e^{23}, -a_4 e^{16} + e^{25} + e^{34}, -e^{15} + e^{26}, e^{36} + e^{45} + e^{17}$ | 5/17(1, 1, 2, 2, 3, 3, 4, 4, 5)                    | {0, 12569, 1457, 24679}     |                    |
| 96531:87  | $0, 0, 0, e^{12}, e^{14}, e^{24}, e^{15}, e^{13} + e^{26}, e^{34} + e^{17} + e^{28}$                                                                             | 13/45(1, 1, 3, 2, 3, 3, 4, 4, 5)                   | {0, 123569}                 |                    |
| 96531:89  | $0, 0, 0, (-1 + a_2) e^{12}, e^{14}, e^{24}, e^{15} + e^{23}, e^{13} a_2 + e^{26}, e^{28} + e^{17} + e^{34}$                                                     | 13/45(1, 1, 3, 2, 3, 3, 4, 4, 5)                   | {0, 123569}                 |                    |

Table A.4 – Continued to next page

Table A.4 – Continued from previous page

| Name       | g                                                                                                                                                                                                               | N                                                   | S <sub>0</sub>                                                    | S = S <sub>0</sub> |
|------------|-----------------------------------------------------------------------------------------------------------------------------------------------------------------------------------------------------------------|-----------------------------------------------------|-------------------------------------------------------------------|--------------------|
| 96531:94   | $0, 0, 0, a_1 e^{12}, e^{14}, e^{24}, -e^{15}(-1 + a_1) + e^{23}, e^{25} + e^{16}, e^{18} + e^{27} + e^{45}$                                                                                                    | $1/71(19, 23, 57, 42, 61, 65, 80, 84, 103)$         | $\{\emptyset, 123569, 134679, 2457\}$                             |                    |
| 96531:96   | $0, 0, 0, e^{12}, e^{24} + e^{13}, e^{14}, e^{25} + e^{34}, e^{16}, e^{35} + e^{27} + e^{18}$                                                                                                                   | $5/17(1, 1, 2, 2, 3, 3, 4, 4, 5)$                   | $\{\emptyset, 12569\}$                                            |                    |
| 96531:98   | $0, 0, 0, a_1 e^{12}, e^{14}, e^{24} + e^{13}, -e^{15}(-1 + a_1), e^{25} + e^{16}, e^{18} + e^{45} + e^{27}$                                                                                                    | $1/128(22, 57, 114, 79, 101, 136, 123, 158, 180)$   | $\{\emptyset, 12569, 14679, 2457\}$                               |                    |
| 96531:100  | $0, 0, 0, e^{12}, e^{24} + e^{13}, e^{14}, e^{25} + e^{34}, e^{15} + e^{26}, e^{28} + e^{17} + e^{36}$                                                                                                          | $5/17(1, 1, 2, 2, 3, 3, 4, 4, 5)$                   | $\{\emptyset, 12569, 1457, 24679\}$                               |                    |
| 96531:101  | $0, 0, 0, -e^{12}(-1 + a_3), e^{14}, e^{24} + e^{13}, e^{23} + a_3 e^{15}, e^{16} + e^{25}, e^{45} + e^{18} + e^{27}$                                                                                           | $31/256(2, 3, 6, 5, 7, 8, 9, 10, 12)$               | $\{\emptyset, 2457\}$                                             |                    |
| 96531:102  | $0, 0, 0, -e^{12}, -e^{13} + e^{24}, 2e^{14}, e^{25} + e^{34}, e^{26} + 2e^{15}, e^{17} + e^{28} + e^{45}$                                                                                                      | $5/17(1, 1, 2, 2, 3, 3, 4, 4, 5)$                   | $\{\emptyset, 12569, 1457, 24679\}$                               |                    |
| 96531:106a | $0, 0, 0, e^{12}, -e^{14} + e^{23}, e^{24} - e^{13}, -e^{15} + e^{34}, -e^{16} + e^{25}, e^{28} + e^{17} + e^{46}$                                                                                              | $5/17(1, 1, 2, 2, 3, 3, 4, 4, 5)$                   | $\{\emptyset, 12569, 1467, 24579\}$                               |                    |
| 96531:106b | $0, 0, 0, -e^{12}, e^{14} + e^{23}, -e^{13} + e^{24}, e^{34} + e^{15}, e^{25} + e^{16}, e^{46} + e^{17} + e^{28}$                                                                                               | $5/17(1, 1, 2, 2, 3, 3, 4, 4, 5)$                   | $\{\emptyset, 12569, 1467, 24579\}$                               |                    |
| 96531:108a | $0, 0, 0, e^{12}, e^{24} + e^{13}, e^{14}, e^{26} + e^{15}, e^{25} + e^{34} + e^{16}, e^{28} + e^{35} + e^{17}$                                                                                                 | $5/17(1, 1, 2, 2, 3, 3, 4, 4, 5)$                   | $\{\emptyset, 12569, 14589, 2468\}$                               |                    |
| 96531:108b | $0, 0, 0, e^{12}, e^{13} + e^{24}, -e^{14}, e^{26} - e^{15}, e^{25} + e^{16} + e^{34}, e^{17} + e^{35} + e^{28}$                                                                                                | $5/17(1, 1, 2, 2, 3, 3, 4, 4, 5)$                   | $\{\emptyset, 12569, 14589, 2468\}$                               |                    |
| 96531:109  | $0, 0, 0, e^{12}(-1 + a_3), e^{13}(-1 + a_3) - \frac{a_3 e^{24}}{-2 + a_3},$<br>$a_3 e^{14}, e^{34} + e^{25}, -(-2 + a_3) e^{15} + e^{26}, e^{17} + e^{28} + e^{36} + e^{45}$                                   | $5/17(1, 1, 2, 2, 3, 3, 4, 4, 5)$                   | $\{\emptyset, 12569, 1457, 24679\}$                               |                    |
| 96531:110a | $0, 0, 0, e^{12}, e^{24} + e^{13}, e^{14}, e^{25} + e^{34}, e^{15} + e^{26}, e^{27} + e^{18} + e^{35} + e^{46}$                                                                                                 | $5/17(1, 1, 2, 2, 3, 3, 4, 4, 5)$                   | $\{\emptyset, 12569, 14579, 2467\}$                               |                    |
| 96531:110b | $0, 0, 0, e^{12}, e^{24} + e^{13},$<br>$-e^{14}, e^{25} + e^{34}, -e^{15} + e^{26}, e^{46} + e^{18} + e^{27} + e^{35}$                                                                                          | $5/17(1, 1, 2, 2, 3, 3, 4, 4, 5)$                   | $\{\emptyset, 12569, 14579, 2467\}$                               |                    |
| 96531:112a | $0, 0, 0, a_1 e^{12}, e^{24} + (1 + a_1) e^{13},$<br>$e^{23} + e^{14}, e^{15} + e^{26}, e^{16} + e^{25} + e^{34}, e^{35} + e^{28} + e^{17}$                                                                     | $5/17(1, 1, 2, 2, 3, 3, 4, 4, 5)$                   | $\{\emptyset, 12569, 14589, 2468\}$                               |                    |
| 96531:112b | $0, 0, 0, a_1 e^{12}, e^{24} + (1 + a_1) e^{13},$<br>$-e^{14} + e^{23}, e^{26} - e^{15}, e^{25} + e^{34} + e^{16}, e^{35} + e^{17} + e^{28}$                                                                    | $5/17(1, 1, 2, 2, 3, 3, 4, 4, 5)$                   | $\{\emptyset, 12569, 14589, 2468\}$                               |                    |
| 96531:113a | $0, 0, 0, -e^{12} a_5, (e^{14} + e^{23}) a_5,$<br>$e^{24} + (-1 + a_5) e^{13}, e^{34} + e^{15}, e^{16} a_5 + e^{25}, e^{17} + e^{28} + e^{46} + e^{35}$                                                         | $5/17(1, 1, 2, 2, 3, 3, 4, 4, 5)$                   | $\{\emptyset, 12569, 1467, 24579\}$                               |                    |
| 96531:113b | $0, 0, 0, e^{12} a_5, -(e^{14} - e^{23}) a_5,$<br>$e^{24} - e^{13}(1 + a_5), -e^{15} + e^{34}, -e^{16} a_5 + e^{25}, e^{28} + e^{46} + e^{35} + e^{17}$                                                         | $5/17(1, 1, 2, 2, 3, 3, 4, 4, 5)$                   | $\{\emptyset, 12569, 1467, 24579\}$                               |                    |
| 96531:115a | $0, 0, 0, -e^{12}(-1 + a_3), -e^{13} + e^{24},$<br>$(-2 + a_3) e^{23} + a_3 e^{14}, e^{26} + a_3 e^{15}, e^{25} + e^{16} + e^{34}, e^{18} + e^{27} + e^{45}$                                                    | $5/17(1, 1, 2, 2, 3, 3, 4, 4, 5)$                   | $\{\emptyset, 12569, 1458, 24689\}$                               |                    |
| 96531:115b | $0, 0, 0, -e^{12}(-1 + a_3), -e^{13} + e^{24},$<br>$-(-2 + a_3) e^{23} + a_3 e^{14}, e^{26} + a_3 e^{15}, -e^{16} + e^{34} + e^{25}, e^{18} + e^{27} + e^{45}$                                                  | $5/17(1, 1, 2, 2, 3, 3, 4, 4, 5)$                   | $\{\emptyset, 12569, 1458, 24689\}$                               |                    |
| 96531:116a | $0, 0, 0, -(-1 + a_2) e^{12}, e^{23} + e^{14},$<br>$e^{13} a_2 + e^{24}, e^{16} + e^{25}, e^{15} a_2 + e^{26}, e^{36} + e^{45} + e^{28} + e^{17}$                                                               | $5/17(1, 1, 2, 2, 3, 3, 4, 4, 5)$                   | $\{\emptyset, 12569, 14689, 2458\}$                               |                    |
| 96531:116b | $0, 0, 0, -(-1 + a_2) e^{12}, -e^{14} + e^{23},$<br>$e^{13} a_2 + e^{24}, e^{25} - e^{16}, e^{15} a_2 + e^{26}, e^{28} + e^{45} + e^{36} + e^{17}$                                                              | $5/17(1, 1, 2, 2, 3, 3, 4, 4, 5)$                   | $\{\emptyset, 12569, 14689, 2458\}$                               |                    |
| 96531:117a | $0, 0, 0, e^{12} a_2, e^{14},$<br>$e^{13} a_2 + e^{24}, e^{25} + e^{16}, -(-1 + a_2) e^{15} + e^{26} + e^{34}, e^{17} + e^{45} + e^{28} + e^{36}$                                                               | $5/17(1, 1, 2, 2, 3, 3, 4, 4, 5)$                   | $\{\emptyset, 12569, 14689, 2458\}$                               |                    |
| 96531:117b | $0, 0, 0, e^{12} a_2, -e^{14},$<br>$e^{13} a_2 + e^{24}, -e^{16} + e^{25}, -(-1 + a_2) e^{15} + e^{26} + e^{34}, e^{17} + e^{28} + e^{36} + e^{45}$                                                             | $5/17(1, 1, 2, 2, 3, 3, 4, 4, 5)$                   | $\{\emptyset, 12569, 14689, 2458\}$                               |                    |
| 96531:119a | $0, 0, 0,$<br>$a_1 e^{12}, (a_6 + a_1 - a_6 a_1) e^{13} + (1 + a_6) e^{24}, e^{14} + a_6 e^{23},$<br>$e^{26} + \frac{e^{15}}{1 + a_6}, -e^{16}(-1 + a_1) + e^{25} + e^{34}, e^{17} + e^{28} + e^{46} + e^{35}$  | $5/17(1, 1, 2, 2, 3, 3, 4, 4, 5)$                   | $\{\emptyset, 12569, 14589, 2468\}$                               |                    |
| 96531:119b | $0, 0, 0,$<br>$a_1 e^{12}, (a_6 + a_1 - a_6 a_1) e^{13} + (1 + a_6) e^{24}, -e^{14} + a_6 e^{23},$<br>$e^{26} - \frac{e^{15}}{1 + a_6}, -e^{16}(-1 + a_1) + e^{34} + e^{25}, e^{17} + e^{46} + e^{35} + e^{28}$ | $5/17(1, 1, 2, 2, 3, 3, 4, 4, 5)$                   | $\{\emptyset, 12569, 14589, 2468\}$                               |                    |
| 96432:1    | $0, 0, 0, -e^{12}, e^{13}, e^{14}, e^{16}, e^{17}, e^{46} + e^{27}$                                                                                                                                             | $1/31(4, 17, 29, 21, 33, 25, 29, 33, 46)$           | $\{\emptyset, 123689, 125689, 13479, 14579, 2345678, 24678, 35\}$ |                    |
| 96432:2    | $0, 0, 0, e^{12}, e^{13}, e^{24}, e^{26}, e^{27}, e^{17} + e^{46}$                                                                                                                                              | $1/124(56, 21, 96, 77, 152, 98, 119, 140, 175)$     | $\{\emptyset, 123689, 125689, 134678, 145678, 234579, 2479, 35\}$ |                    |
| 96432:3a   | $0, 0, 0, -e^{12}, e^{13}, e^{14}, e^{16}, e^{17}, e^{27} + e^{46} + e^{35}$                                                                                                                                    | $1/67(8, 41, 49, 49, 57, 57, 65, 73, 106)$          | $\{\emptyset, 123689, 125689, 13479, 14579, 2345678, 24678, 35\}$ |                    |
| 96432:3b   | $0, 0, 0, -e^{12}, -e^{13}, e^{14}, e^{16}, e^{17}, e^{27} + e^{46} + e^{35}$                                                                                                                                   | $1/67(8, 41, 49, 49, 57, 57, 65, 73, 106)$          | $\{\emptyset, 123689, 125689, 13479, 14579, 2345678, 24678, 35\}$ |                    |
| 96432:4    | $0, 0, 0, e^{12}, e^{13}, e^{24}, e^{26}, e^{27}, e^{17} + e^{35} + e^{46}$                                                                                                                                     | $2/603(155, 49, 151, 204, 306, 253, 302, 351, 457)$ | $\{\emptyset, 123689, 125689, 35\}$                               |                    |

Table A.4 – Continued to next page

Table A.4 – Continued from previous page

| Name      | $g$                                                                                                                       | $N$                                               | $S_0$                                                             | $S = S_0$ |
|-----------|---------------------------------------------------------------------------------------------------------------------------|---------------------------------------------------|-------------------------------------------------------------------|-----------|
| 96432:8   | $0, 0, 0, -e^{12}, e^{13}, e^{14}, e^{16}, e^{17} + e^{23}, e^{46} + e^{27}$                                              | 1/473(95, 199, 380, 294, 475, 389, 484, 579, 683) | $\{\emptyset, 125689, 14579, 24678\}$                             |           |
| 96432:10  | $0, 0, 0, e^{12}, e^{13}, e^{24}, e^{26}, e^{15} + e^{27}, e^{17} + e^{46}$                                               | 1/144(42, 37, 106, 79, 148, 116, 153, 190, 195)   | $\{\emptyset, 123689, 134678, 2479\}$                             |           |
| 96432:11  | $0, 0, 0, -e^{12}, e^{13}, e^{14}, e^{16}, e^{17} + e^{24}, e^{27} + e^{46}$                                              | 2/87(7, 21, 40, 28, 47, 35, 42, 49, 63)           | $\{\emptyset, 123689, 125689, 35\}$                               |           |
| 96432:13a | $0, 0, 0, -e^{12}, e^{13}, e^{14}, e^{16}, e^{17} + e^{23}, e^{46} + e^{35} + e^{27}$                                     | 22/129(1, 3, 4, 4, 5, 5, 6, 7, 9)                 | $\{\emptyset, 125689, 14579, 24678\}$                             |           |
| 96432:13b | $0, 0, 0, -e^{12}, -e^{13}, e^{14}, e^{16}, e^{17} + e^{23}, e^{46} + e^{35} + e^{27}$                                    | 22/129(1, 3, 4, 4, 5, 5, 6, 7, 9)                 | $\{\emptyset, 125689, 14579, 24678\}$                             |           |
| 96432:15  | $0, 0, 0, e^{12}, e^{13}, e^{24}, e^{26}, e^{27} + e^{15}, e^{17} + e^{46} + e^{35}$                                      | 48/629(5, 3, 7, 8, 12, 11, 14, 17, 19)            | $\{\emptyset, 123689\}$                                           |           |
| 96432:18  | $0, 0, 0, -e^{12}, e^{13}, e^{14}, e^{16} + e^{23}, e^{17} + e^{25}, e^{46} + e^{27}$                                     | 1/47(11, 17, 33, 28, 44, 39, 50, 61, 67)          | $\{\emptyset, 123689, 13479, 24678\}$                             |           |
| 96432:24a | $0, 0, 0, -e^{12}, e^{13}, e^{14}, e^{16}, e^{17} + e^{24}, e^{27} + e^{35} + e^{46}$                                     | 22/129(1, 3, 4, 4, 5, 5, 6, 7, 9)                 | $\{\emptyset, 123689, 125689, 35\}$                               |           |
| 96432:24b | $0, 0, 0, -e^{12}, -e^{13}, e^{14}, e^{16}, e^{17} + e^{24}, e^{27} + e^{46} + e^{35}$                                    | 22/129(1, 3, 4, 4, 5, 5, 6, 7, 9)                 | $\{\emptyset, 123689, 125689, 35\}$                               |           |
| 96432:25a | $0, 0, 0, e^{12}, e^{13}, e^{24}, e^{26}, e^{27} + e^{14}, e^{46} + e^{35} + e^{17}$                                      | 22/131(3, 1, 3, 4, 6, 5, 6, 7, 9)                 | $\{\emptyset, 123689, 125689, 35\}$                               | ✓         |
| 96432:25b | $0, 0, 0, e^{12}, -e^{13}, e^{24}, e^{26}, e^{14} + e^{27}, e^{35} + e^{46} + e^{17}$                                     | 22/131(3, 1, 3, 4, 6, 5, 6, 7, 9)                 | $\{\emptyset, 123689, 125689, 35\}$                               | ✓         |
| 96432:26a | $0, 0, 0, -e^{12}, e^{13}, e^{14}, e^{16} + e^{23}, e^{25} + e^{17}, e^{27} + e^{35} + e^{46}$                            | 7/33(1, 2, 3, 3, 4, 4, 5, 6, 7)                   | $\{\emptyset, 123689, 13479, 24678\}$                             |           |
| 96432:26b | $0, 0, 0, -e^{12}, e^{13}, -e^{14}, e^{23} + e^{16}, e^{17} + e^{25}, e^{27} + e^{46} + e^{35}$                           | 7/33(1, 2, 3, 3, 4, 4, 5, 6, 7)                   | $\{\emptyset, 123689, 13479, 24678\}$                             |           |
| 96432:32  | $0, 0, 0, -e^{12}, e^{13}, e^{14}, e^{16} + e^{24}, e^{17} + e^{26}, e^{27} + e^{46}$                                     | 1/281(56, 112, 253, 168, 309, 224, 280, 336, 392) | $\{\emptyset, 13479, 14579, 35\}$                                 |           |
| 96432:33  | $0, 0, 0, e^{12}, e^{13}, e^{24}, e^{26} + e^{14}, e^{27} + e^{16}, e^{17} + e^{46}$                                      | 1/71(28, 14, 57, 42, 85, 56, 70, 84, 98)          | $\{\emptyset, 234579, 2479, 35\}$                                 |           |
| 96432:34  | $0, 0, 0, (-1 + a_2)e^{12}, a_2e^{13}, e^{14}, -(-1 + a_2)e^{16} + e^{23}, e^{17} + e^{25} + e^{34}, e^{46} + e^{27}$     | 1/47(11, 17, 33, 28, 44, 39, 50, 61, 67)          | $\{\emptyset, 123689, 13479, 24678\}$                             |           |
| 96432:39a | $0, 0, 0, -e^{12}a_1, -(-1 + a_1)e^{13}, e^{14}, e^{16}a_1 + e^{23}, e^{34} + e^{17} + e^{25}, e^{46} + e^{35} + e^{27}$  | 7/33(1, 2, 3, 3, 4, 4, 5, 6, 7)                   | $\{\emptyset, 123689, 13479, 24678\}$                             |           |
| 96432:39b | $0, 0, 0, -e^{12}a_1, -(-1 + a_1)e^{13}, -e^{14}, e^{16}a_1 + e^{23}, e^{17} + e^{34} + e^{25}, e^{46} + e^{35} + e^{27}$ | 7/33(1, 2, 3, 3, 4, 4, 5, 6, 7)                   | $\{\emptyset, 123689, 13479, 24678\}$                             |           |
| 96432:42a | $0, 0, 0, -e^{12}, e^{13}, e^{14}, e^{16} + e^{24}, e^{17} + e^{26}, e^{27} + e^{46} + e^{35}$                            | 7/33(1, 2, 3, 3, 4, 4, 5, 6, 7)                   | $\{\emptyset, 13479, 14579, 35\}$                                 |           |
| 96432:42b | $0, 0, 0, -e^{12}, -e^{13}, e^{14}, e^{16} + e^{24}, e^{17} + e^{26}, e^{27} + e^{35} + e^{46}$                           | 7/33(1, 2, 3, 3, 4, 4, 5, 6, 7)                   | $\{\emptyset, 13479, 14579, 35\}$                                 |           |
| 96432:43  | $0, 0, 0, e^{12}, e^{13}, e^{24}, e^{14} + e^{26}, e^{16} + e^{27}, e^{46} + e^{17} + e^{35}$                             | 35/333(4, 2, 5, 6, 9, 8, 10, 12, 14)              | $\{\emptyset, 35\}$                                               |           |
| 96432:58  | $0, 0, 0, e^{12}, 2e^{13}, 3e^{14} - e^{23}, -e^{16} + e^{25} + e^{34}, e^{27} + e^{46}, e^{17} + e^{36} + e^{45}$        | 1/221(59, 67, 118, 126, 177, 185, 244, 311, 303)  | $\{\emptyset, 125689, 14578, 24679\}$                             |           |
| 96421:11  | $0, 0, 0, e^{12}, e^{13}, e^{14}, e^{25} + e^{34}, e^{16}, e^{18}$                                                        | 1/109(16, 67, 76, 83, 92, 99, 159, 115, 131)      | $\{\emptyset, 123679, 12569, 1348, 14578, 2345689, 246789, 357\}$ |           |
| 96421:13  | $0, 0, 0, e^{12}, e^{13}, e^{24}, e^{25} + e^{34}, e^{26}, e^{28}$                                                        | 1/109(67, 16, 59, 83, 126, 99, 142, 115, 131)     | $\{\emptyset, 123679, 12569, 134689, 1456789, 23458, 2478, 357\}$ |           |
| 96421:26  | $0, 0, 0, e^{12}, e^{13}, e^{14}, e^{34} + e^{25}, e^{16}, e^{18} + e^{35}$                                               | 5/213(7, 27, 24, 34, 31, 41, 58, 48, 55)          | $\{\emptyset, 123679, 12569, 357\}$                               |           |
| 96421:27a | $0, 0, 0, e^{12}, e^{13}, e^{24}, e^{25} + e^{34}, e^{26}, e^{28} + e^{35}$                                               | 1/37(22, 7, 14, 29, 36, 36, 43, 43, 50)           | $\{\emptyset, 123679, 12569, 134689, 1456789, 23458, 2478, 357\}$ | ✓         |
| 96421:27b | $0, 0, 0, e^{12}, e^{13}, -e^{24}, e^{25} + e^{34}, e^{26}, e^{28} + e^{35}$                                              | 1/37(22, 7, 14, 29, 36, 36, 43, 43, 50)           | $\{\emptyset, 123679, 12569, 134689, 1456789, 23458, 2478, 357\}$ | ✓         |
| 96421:28  | $0, 0, 0, e^{12}, e^{13}, e^{14}, e^{35}, e^{23} + e^{16}, e^{18} + e^{25}$                                               | 1/17(3, 11, 9, 14, 12, 17, 21, 20, 23)            | $\{\emptyset, 123679, 13478, 24689\}$                             |           |
| 96421:30  | $0, 0, 0, -e^{12}, e^{13}, e^{14}, e^{35}, e^{16}, e^{46} + e^{28}$                                                       | 1/156(24, 81, 92, 105, 116, 129, 208, 153, 234)   | $\{\emptyset, 123679, 125679, 134789, 145789, 234568, 2468, 35\}$ |           |
| 96421:31  | $0, 0, 0, e^{12}, e^{13}, e^{24}, e^{35}, e^{26}, e^{18} + e^{46}$                                                        | 1/60(24, 13, 28, 37, 52, 50, 80, 63, 87)          | $\{\emptyset, 123679, 125679, 134678, 145678, 234589, 2489, 35\}$ |           |
| 96421:34  | $0, 0, 0, e^{12}, e^{13}, e^{14}, e^{34} + e^{25}, e^{16}, e^{23} + e^{18}$                                               | 1/119(20, 69, 80, 89, 100, 109, 169, 129, 149)    | $\{\emptyset, 12569, 14578, 246789\}$                             |           |
| 96421:41  | $0, 0, 0, e^{12}, e^{13}, e^{24}, e^{34} + e^{25}, e^{26}, e^{15} + e^{28}$                                               | 2/123(26, 15, 34, 41, 60, 56, 75, 71, 86)         | $\{\emptyset, 123679, 134689, 2478\}$                             |           |
| 96421:43  | $0, 0, 0, e^{12}, e^{13}, e^{14}, e^{35}, e^{16}, e^{25} + e^{18} + e^{34}$                                               | 1/17(3, 11, 9, 14, 12, 17, 21, 20, 23)            | $\{\emptyset, 123679, 13478, 24689\}$                             |           |
| 96421:45  | $0, 0, 0, -e^{12}, e^{13}, e^{14}, e^{15}, e^{16}, e^{46} + e^{28}$                                                       | 1/16(2, 9, 14, 11, 16, 13, 18, 15, 24)            | $\{\emptyset, 123679, 12569, 134789, 14589, 2345678, 2468, 357\}$ |           |
| 96421:46  | $0, 0, 0, e^{12}, e^{13}, e^{24}, e^{15}, e^{26}, e^{46} + e^{18}$                                                        | 1/24(6, 7, 18, 13, 24, 20, 30, 27, 33)            | $\{\emptyset, 123679, 12569, 134678, 14568, 2345789, 2489, 357\}$ |           |
| 96421:47  | $0, 0, 0, -e^{12}, e^{13}, e^{14}, e^{35}, e^{16} + e^{23}, e^{28} + e^{46}$                                              | 3/32(2, 5, 6, 7, 8, 9, 14, 11, 16)                | $\{\emptyset, 123679, 134789, 2468\}$                             |           |
| 96421:54  | $0, 0, 0, -e^{12}, e^{13}, e^{14}, e^{24}, e^{16}, e^{46} + e^{28}$                                                       | 1/11(2, 5, 10, 7, 12, 9, 12, 11, 16)              | $\{\emptyset, 123679, 125679, 134789, 145789, 234568, 2468, 35\}$ |           |
| 96421:55  | $0, 0, 0, e^{12}, e^{13}, e^{24}, e^{14}, e^{26}, e^{18} + e^{46}$                                                        | 1/233(92, 51, 187, 143, 279, 194, 235, 245, 337)  | $\{\emptyset, 123679, 125679, 13468, 14568, 2345789, 24789, 35\}$ |           |
| 96421:59  | $0, 0, 0, e^{12}, e^{13}, e^{14}, e^{25} + e^{34}, e^{16}, e^{24} + e^{18}$                                               | 1/217(39, 117, 152, 156, 191, 195, 308, 234, 273) | $\{\emptyset, 123679, 12569, 357\}$                               |           |
| 96421:60  | $0, 0, 0, e^{12}, e^{13}, e^{24}, e^{25} + e^{34}, e^{26}, e^{28} + e^{14}$                                               | 3/217(39, 13, 42, 52, 81, 65, 94, 78, 91)         | $\{\emptyset, 123679, 12569, 357\}$                               |           |
| 96421:62  | $0, 0, 0, e^{12}, e^{13}, e^{14}, e^{24}, e^{23} + e^{16}, e^{25} + e^{18}$                                               | 1/123(29, 57, 87, 86, 116, 115, 143, 144, 173)    | $\{\emptyset, 123679, 13478, 24689\}$                             |           |
| 96421:63  | $0, 0, 0, -e^{12}, e^{13}, e^{14}, e^{15} + e^{23}, e^{16}, e^{28} + e^{46}$                                              | 1/53(11, 22, 42, 33, 53, 44, 64, 55, 77)          | $\{\emptyset, 134789, 14589, 357\}$                               |           |
| 96421:66a | $0, 0, 0, e^{12}, e^{13}, e^{14}, e^{35} + e^{24}, e^{16} + e^{23}, e^{25} + e^{18}$                                      | 4/21(1, 3, 3, 4, 4, 5, 7, 6, 7)                   | $\{\emptyset, 123679, 13478, 24689\}$                             |           |
| 96421:66b | $0, 0, 0, -e^{12}, e^{13}, e^{14}, e^{24} + e^{35}, e^{16} + e^{23}, e^{25} + e^{18}$                                     | 4/21(1, 3, 3, 4, 4, 5, 7, 6, 7)                   | $\{\emptyset, 123679, 13478, 24689\}$                             |           |

Table A.4 – Continued to next page



Table A.4 – Continued from previous page

| Name       | g                                                                                                          | N                                                   | S <sub>0</sub>                                                    | S = S <sub>0</sub> |
|------------|------------------------------------------------------------------------------------------------------------|-----------------------------------------------------|-------------------------------------------------------------------|--------------------|
| 96421:67   | $0, 0, 0, a_1 e^{12}, e^{13}(1 + a_1), e^{14}, e^{35}, e^{23} + e^{16}, e^{34} + e^{18} + e^{25}$          | $1/17(3, 11, 9, 14, 12, 17, 21, 20, 23)$            | $\{\emptyset, 123679, 13478, 24689\}$                             |                    |
| 96421:70   | $0, 0, 0, -e^{12}, -e^{13}, e^{14}, e^{34} + e^{25}, e^{16}, e^{28} + e^{46}$                              | $1/185(38, 74, 135, 112, 173, 150, 247, 188, 262)$  | $\{\emptyset, 123679, 12569, 13489, 145789, 234568, 24678, 357\}$ |                    |
| 96421:72   | $0, 0, 0, e^{12}, e^{13}, e^{24}, e^{25} + e^{34}, e^{26}, e^{46} + e^{18}$                                | $1/185(74, 38, 123, 112, 197, 150, 235, 188, 262)$  | $\{\emptyset, 123679, 12569, 13468, 145678, 234589, 24789, 357\}$ |                    |
| 96421:73a  | $0, 0, 0, -e^{12}, e^{13}, e^{14}, e^{15}, e^{16}, e^{46} + e^{35} + e^{28}$                               | $1/47(7, 27, 34, 34, 41, 41, 48, 48, 75)$           | $\{\emptyset, 123679, 12569, 134789, 14589, 2345678, 2468, 357\}$ |                    |
| 96421:73b  | $0, 0, 0, -e^{12}, -e^{13}, e^{14}, e^{15}, e^{16}, e^{46} + e^{35} + e^{28}$                              | $1/47(7, 27, 34, 34, 41, 41, 48, 48, 75)$           | $\{\emptyset, 123679, 12569, 134789, 14589, 2345678, 2468, 357\}$ |                    |
| 96421:74   | $0, 0, 0, e^{12}, e^{13}, e^{24}, e^{15}, e^{26}, e^{35} + e^{46} + e^{18}$                                | $1/327(102, 92, 189, 194, 291, 286, 393, 378, 480)$ | $\{\emptyset, 123679, 12569, 357\}$                               |                    |
| 96421:76   | $0, 0, 0, -e^{12}, e^{13}, e^{14}, e^{15}, e^{23} + e^{16}, e^{28} + e^{46}$                               | $1/112(26, 45, 78, 71, 104, 97, 130, 123, 168)$     | $\{\emptyset, 123679, 134789, 2468\}$                             |                    |
| 96421:77   | $0, 0, 0, e^{12}, e^{13}, e^{14}, e^{35}, e^{16} + e^{24}, e^{26} + e^{18}$                                | $1/183(42, 84, 101, 126, 143, 168, 244, 210, 252)$  | $\{\emptyset, 13478, 14578, 35\}$                                 |                    |
| 96421:78   | $0, 0, 0, e^{12}, e^{13}, e^{24}, e^{35}, e^{26} + e^{14}, e^{16} + e^{28}$                                | $1/93(42, 21, 41, 63, 83, 84, 124, 105, 126)$       | $\{\emptyset, 23458, 248, 35\}$                                   |                    |
| 96421:79   | $0, 0, 0, -e^{12}, e^{13}, e^{14}, e^{35}, e^{16} + e^{24}, e^{46} + e^{28}$                               | $4/57(3, 6, 8, 9, 11, 12, 19, 15, 21)$              | $\{\emptyset, 134789, 145789, 35\}$                               |                    |
| 96421:81   | $0, 0, 0, e^{12}, e^{13}, e^{24}, e^{14} + e^{23}, e^{26}, e^{18} + e^{46}$                                | $1/143(57, 31, 114, 88, 171, 119, 145, 150, 207)$   | $\{\emptyset, 125679, 14568, 24789\}$                             |                    |
| 96421:85   | $0, 0, 0, e^{12}, e^{13}, e^{14}, e^{24}, e^{16}, e^{18} + e^{25} + e^{34}$                                | $1/123(29, 57, 87, 86, 116, 115, 143, 144, 173)$    | $\{\emptyset, 123679, 13478, 24689\}$                             |                    |
| 96421:87a  | $0, 0, 0, e^{12}, e^{13}, e^{14}, e^{24} + e^{15}, e^{16} + e^{23}, e^{18} + e^{25}$                       | $11/47(1, 2, 3, 3, 4, 4, 5, 5, 6)$                  | $\{\emptyset, 123679, 13478, 24689\}$                             | ✓                  |
| 96421:87b  | $0, 0, 0, e^{12}, e^{13}, -e^{14}, e^{15} + e^{24}, e^{16} + e^{23}, e^{25} + e^{18}$                      | $11/47(1, 2, 3, 3, 4, 4, 5, 5, 6)$                  | $\{\emptyset, 123679, 13478, 24689\}$                             | ✓                  |
| 96421:90a  | $0, 0, 0, e^{12}, e^{13}, e^{14}, e^{24} + e^{35}, e^{16}, e^{25} + e^{18} + e^{34}$                       | $4/21(1, 3, 3, 4, 4, 5, 7, 6, 7)$                   | $\{\emptyset, 123679, 13478, 24689\}$                             | ✓                  |
| 96421:90b  | $0, 0, 0, e^{12}, e^{13}, e^{14}, -e^{24} + e^{35}, e^{16}, e^{18} + e^{25} + e^{34}$                      | $4/21(1, 3, 3, 4, 4, 5, 7, 6, 7)$                   | $\{\emptyset, 123679, 13478, 24689\}$                             | ✓                  |
| 96421:91a  | $0, 0, 0, e^{12}, e^{13}, e^{14}, e^{34} + e^{25}, e^{16}, e^{18} + e^{35} + e^{24}$                       | $4/21(1, 3, 3, 4, 4, 5, 7, 6, 7)$                   | $\{\emptyset, 123679, 12569, 357\}$                               | ✓                  |
| 96421:91b  | $0, 0, 0, -e^{12}, e^{13}, e^{14}, -e^{25} + e^{34}, e^{16}, e^{35} + e^{24} + e^{18}$                     | $4/21(1, 3, 3, 4, 4, 5, 7, 6, 7)$                   | $\{\emptyset, 123679, 12569, 357\}$                               | ✓                  |
| 96421:92a  | $0, 0, 0, e^{12}, e^{13}, e^{24}, e^{25} + e^{34}, e^{26}, e^{35} + e^{14} + e^{28}$                       | $13/67(3, 1, 2, 4, 5, 5, 6, 6, 7)$                  | $\{\emptyset, 123679, 12569, 357\}$                               | ✓                  |
| 96421:92b  | $0, 0, 0, e^{12}, e^{13}, -e^{24}, e^{34} + e^{25}, e^{26}, e^{28} + e^{35} + e^{14}$                      | $13/67(3, 1, 2, 4, 5, 5, 6, 6, 7)$                  | $\{\emptyset, 123679, 12569, 357\}$                               | ✓                  |
| 96421:93   | $0, 0, 0, (-1 + a_2)e^{12}, e^{13}a_2, e^{14}, e^{15}, e^{23} + e^{16}, e^{18} + e^{34} + e^{25}$          | $1/61(13, 35, 39, 48, 52, 61, 65, 74, 87)$          | $\{\emptyset, 123679, 13478, 24689\}$                             |                    |
| 96421:95   | $0, 0, 0, -e^{12}, e^{13}, e^{14}, e^{15} + e^{24}, e^{16}, e^{28} + e^{46}$                               | $1/47(7, 24, 41, 31, 48, 38, 55, 45, 69)$           | $\{\emptyset, 123679, 134789, 2468\}$                             |                    |
| 96421:99a  | $0, 0, 0, -e^{12}, e^{13}, e^{14}, e^{24}, e^{16}, e^{35} + e^{28} + e^{46}$                               | $2/131(13, 31, 44, 44, 57, 57, 75, 70, 101)$        | $\{\emptyset, 123679, 125679, 134789, 145789, 234568, 2468, 35\}$ |                    |
| 96421:99b  | $0, 0, 0, -e^{12}, -e^{13}, e^{14}, e^{24}, e^{16}, e^{28} + e^{35} + e^{46}$                              | $2/131(13, 31, 44, 44, 57, 57, 75, 70, 101)$        | $\{\emptyset, 123679, 125679, 134789, 145789, 234568, 2468, 35\}$ |                    |
| 96421:100  | $0, 0, 0, e^{12}, e^{13}, e^{24}, e^{14}, e^{26}, e^{18} + e^{35} + e^{46}$                                | $4/185(19, 11, 26, 30, 45, 41, 49, 52, 71)$         | $\{\emptyset, 123679, 125679, 35\}$                               |                    |
| 96421:103a | $0, 0, 0, -e^{12}, -e^{13}, e^{14}, e^{25} + e^{34}, e^{16}, e^{35} + e^{46} + e^{28}$                     | $5/101(4, 9, 13, 13, 17, 17, 26, 21, 30)$           | $\{\emptyset, 123679, 12569, 13489, 145789, 234568, 24678, 357\}$ |                    |
| 96421:103b | $0, 0, 0, -e^{12}, -e^{13}, -e^{14}, e^{25} + e^{34}, e^{16}, e^{35} + e^{28} + e^{46}$                    | $5/101(4, 9, 13, 13, 17, 17, 26, 21, 30)$           | $\{\emptyset, 123679, 12569, 13489, 145789, 234568, 24678, 357\}$ |                    |
| 96421:104  | $0, 0, 0, e^{12}, e^{13}, e^{24}, e^{34} + e^{25}, e^{26}, e^{18} + e^{46} + e^{35}$                       | $1/183(79, 39, 98, 118, 177, 157, 216, 196, 275)$   | $\{\emptyset, 123679, 12569, 357\}$                               |                    |
| 96421:106  | $0, 0, 0, -e^{12}, -e^{13}, e^{14}, e^{25} + e^{34}, e^{16} + e^{23}, e^{46} + e^{28}$                     | $1/47(11, 17, 33, 28, 44, 39, 61, 50, 67)$          | $\{\emptyset, 123679, 13489, 24678\}$                             |                    |
| 96421:107a | $0, 0, 0, -e^{12}, e^{13}, e^{14}, e^{15}, e^{23} + e^{16}, e^{46} + e^{35} + e^{28}$                      | $17/77(1, 2, 3, 3, 4, 4, 5, 5, 7)$                  | $\{\emptyset, 123679, 134789, 2468\}$                             |                    |
| 96421:107b | $0, 0, 0, -e^{12}, -e^{13}, e^{14}, e^{15}, e^{16} + e^{23}, e^{46} + e^{35} + e^{28}$                     | $17/77(1, 2, 3, 3, 4, 4, 5, 5, 7)$                  | $\{\emptyset, 123679, 134789, 2468\}$                             |                    |
| 96421:109  | $0, 0, 0, -e^{12}, e^{13}, e^{14}, e^{15}, e^{16} + e^{24}, e^{46} + e^{28}$                               | $1/53(11, 22, 42, 33, 53, 44, 64, 55, 77)$          | $\{\emptyset, 134789, 14589, 357\}$                               |                    |
| 96421:114a | $0, 0, 0, e^{12}, e^{13}, e^{14}, e^{15} + e^{24}, e^{16}, e^{25} + e^{18} + e^{34}$                       | $11/47(1, 2, 3, 3, 4, 4, 5, 5, 6)$                  | $\{\emptyset, 123679, 13478, 24689\}$                             |                    |
| 96421:114b | $0, 0, 0, e^{12}, e^{13}, -e^{14}, e^{15} + e^{24}, e^{16}, e^{18} + e^{25} + e^{34}$                      | $11/47(1, 2, 3, 3, 4, 4, 5, 5, 6)$                  | $\{\emptyset, 123679, 13478, 24689\}$                             |                    |
| 96421:117  | $0, 0, 0, a_1 e^{12}, e^{13}(1 + a_1), e^{14}, e^{24}, e^{16} + e^{23}, e^{25} + e^{34} + e^{18}$          | $1/123(29, 57, 87, 86, 116, 115, 143, 144, 173)$    | $\{\emptyset, 123679, 13478, 24689\}$                             |                    |
| 96421:120  | $0, 0, 0, e^{12}, a_1 e^{13}, e^{14}, e^{15} + e^{23}, e^{16} + e^{24}, e^{18} + e^{26}$                   | $1/31(7, 14, 24, 21, 31, 28, 38, 35, 42)$           | $\{\emptyset, 13478, 1458, 357\}$                                 |                    |
| 96421:122a | $0, 0, 0, a_1 e^{12}, e^{13}(1 + a_1), e^{14}, e^{35} + e^{24}, e^{23} + e^{16}, e^{34} + e^{18} + e^{25}$ | $4/21(1, 3, 3, 4, 4, 5, 7, 6, 7)$                   | $\{\emptyset, 123679, 13478, 24689\}$                             |                    |
| 96421:122b | $0, 0, 0, a_1 e^{12}, e^{13}(1 + a_1), e^{14}, e^{35} - e^{24}, e^{23} + e^{16}, e^{34} + e^{25} + e^{18}$ | $4/21(1, 3, 3, 4, 4, 5, 7, 6, 7)$                   | $\{\emptyset, 123679, 13478, 24689\}$                             |                    |
| 96421:127  | $0, 0, 0, e^{12}, e^{13}, e^{14}, e^{15}, e^{24} + e^{16}, e^{35} + e^{26} + e^{18}$                       | $21/173(2, 4, 5, 6, 7, 8, 9, 10, 12)$               | $\{\emptyset, 357\}$                                              |                    |
| 96421:129  | $0, 0, 0, e^{12}, e^{13}, e^{14}, e^{34} + e^{25}, e^{16} + e^{24}, e^{18} + e^{26}$                       | $1/41(9, 18, 29, 27, 38, 36, 56, 45, 54)$           | $\{\emptyset, 1348, 14578, 357\}$                                 |                    |
| 96421:130  | $0, 0, 0, e^{12}, e^{13}, e^{24}, e^{34} + e^{25}, e^{14} + e^{26}, e^{28} + e^{16}$                       | $1/41(18, 9, 26, 27, 44, 36, 53, 45, 54)$           | $\{\emptyset, 23458, 2478, 357\}$                                 |                    |
| 96421:131a | $0, 0, 0, -e^{12}, e^{13}, e^{14}, e^{24}, e^{16} + e^{23}, e^{28} + e^{35} + e^{46}$                      | $17/77(1, 2, 3, 3, 4, 4, 5, 5, 7)$                  | $\{\emptyset, 123679, 134789, 2468\}$                             |                    |
| 96421:131b | $0, 0, 0, -e^{12}, -e^{13}, e^{14}, e^{24}, e^{16} + e^{23}, e^{46} + e^{28} + e^{35}$                     | $17/77(1, 2, 3, 3, 4, 4, 5, 5, 7)$                  | $\{\emptyset, 123679, 134789, 2468\}$                             |                    |
| 96421:132  | $0, 0, 0, -e^{12}, e^{13}a_2, e^{14}, e^{15} + e^{23}, e^{16} + e^{24}, e^{46} + e^{28}$                   | $1/53(11, 22, 42, 33, 53, 44, 64, 55, 77)$          | $\{\emptyset, 134789, 14589, 357\}$                               |                    |
| 96421:135a | $0, 0, 0, -e^{12}, -e^{13}, e^{14}, e^{25} + e^{34}, e^{16} + e^{23}, e^{28} + e^{46} + e^{35}$            | $7/33(1, 2, 3, 3, 4, 4, 6, 5, 7)$                   | $\{\emptyset, 123679, 13489, 24678\}$                             |                    |
| 96421:135b | $0, 0, 0, -e^{12}, -e^{13}, -e^{14}, e^{25} + e^{34}, e^{23} + e^{16}, e^{46} + e^{35} + e^{28}$           | $7/33(1, 2, 3, 3, 4, 4, 6, 5, 7)$                   | $\{\emptyset, 123679, 13489, 24678\}$                             |                    |
| 96421:138a | $0, 0, 0, -e^{12}, e^{13}, e^{14}, e^{15}, e^{16} + e^{24}, e^{28} + e^{35} + e^{46}$                      | $17/77(1, 2, 3, 3, 4, 4, 5, 5, 7)$                  | $\{\emptyset, 134789, 14589, 357\}$                               |                    |

Table A.4 – Continued to next page

Table A.4 – Continued from previous page

| Name       | $g$                                                                                                                         | $N$                                                  | $S_0$                                   | $S = S_0$ |
|------------|-----------------------------------------------------------------------------------------------------------------------------|------------------------------------------------------|-----------------------------------------|-----------|
| 96421:138b | $0, 0, 0, -e^{12}, -e^{13}, e^{14}, e^{15}, e^{16} + e^{24}, e^{28} + e^{46} + e^{35}$                                      | $17/77(1, 2, 3, 3, 4, 4, 5, 5, 7)$                   | $\{\emptyset, 134789, 14589, 357\}$     |           |
| 96421:143  | $0, 0, 0, -e^{12}, e^{13}, e^{24}, e^{14} + e^{23}, e^{26}, e^{28} + e^{34} + e^{17}$                                       | $6/47(3, 2, 6, 5, 9, 7, 8, 9, 11)$                   | $\{\emptyset, 145689\}$                 |           |
| 96421:144  | $0, 0, 0, -e^{12}, e^{13}, e^{14}, e^{24}, e^{23} + e^{16}, e^{34} + e^{27} + e^{18}$                                       | $59/453(2, 3, 6, 5, 8, 7, 8, 9, 11)$                 | $\{\emptyset, 24689\}$                  |           |
| 96421:145a | $0, 0, 0, (-1 + a_2)e^{12}, e^{13}a_2, e^{14}, e^{15} + e^{24}, e^{16} + e^{23}, e^{25} + e^{18} + e^{34}$                  | $11/47(1, 2, 3, 3, 4, 4, 5, 5, 6)$                   | $\{\emptyset, 123679, 13478, 24689\}$   |           |
| 96421:145b | $0, 0, 0, (-1 + a_2)e^{12}, e^{13}a_2, -e^{14}, e^{15} + e^{24}, e^{23} + e^{16}, e^{18} + e^{25} + e^{34}$                 | $11/47(1, 2, 3, 3, 4, 4, 5, 5, 6)$                   | $\{\emptyset, 123679, 13478, 24689\}$   |           |
| 96421:146  | $0, 0, 0, e^{12}, a_1e^{13}, e^{14}, e^{23} + e^{15}, e^{24} + e^{16}, e^{35} + e^{26} + e^{18}$                            | $21/173(2, 4, 5, 6, 7, 8, 9, 10, 12)$                | $\{\emptyset, 357\}$                    |           |
| 96421:150a | $0, 0, 0, -e^{12}, e^{13}, e^{14}, e^{15}a_2 + e^{24}, e^{16} + e^{23}, e^{28} + e^{35} + e^{46}$                           | $17/77(1, 2, 3, 3, 4, 4, 5, 5, 7)$                   | $\{\emptyset, 123679, 134789, 2468\}$   |           |
| 96421:150b | $0, 0, 0, -e^{12}, -e^{13}, e^{14}, e^{15}a_2 + e^{24}, e^{23} + e^{16}, e^{46} + e^{35} + e^{28}$                          | $17/77(1, 2, 3, 3, 4, 4, 5, 5, 7)$                   | $\{\emptyset, 123679, 134789, 2468\}$   |           |
| 96421:153  | $0, 0, 0, e^{12}, e^{13}, e^{14}, e^{25} + e^{34}, e^{16} + e^{24}, e^{18} + e^{26} + e^{35}$                               | $5/43(2, 4, 5, 6, 7, 8, 11, 10, 12)$                 | $\{\emptyset, 357\}$                    |           |
| 96421:154a | $0, 0, 0, e^{12}, e^{13}, e^{24}, e^{25} + e^{34}, e^{14} + e^{26}, e^{28} + e^{16} + e^{35}$                               | $4/17(2, 1, 2, 3, 4, 4, 5, 5, 6)$                    | $\{\emptyset, 23458, 2478, 357\}$       |           |
| 96421:154b | $0, 0, 0, e^{12}, e^{13}, -e^{24}, e^{34} + e^{25}, -e^{14} + e^{26}, e^{16} + e^{35} + e^{28}$                             | $4/17(2, 1, 2, 3, 4, 4, 5, 5, 6)$                    | $\{\emptyset, 23458, 2478, 357\}$       |           |
| 96421:156a | $0, 0, 0, -e^{12}, e^{13}, e^{14}, e^{15}a_2 + e^{23}, e^{24} + e^{16}, e^{28} + e^{46} + e^{35}$                           | $17/77(1, 2, 3, 3, 4, 4, 5, 5, 7)$                   | $\{\emptyset, 134789, 14589, 357\}$     |           |
| 96421:156b | $0, 0, 0, -e^{12}, -e^{13}, e^{14}, e^{15}a_2 + e^{23}, e^{16} + e^{24}, e^{46} + e^{35} + e^{28}$                          | $17/77(1, 2, 3, 3, 4, 4, 5, 5, 7)$                   | $\{\emptyset, 134789, 14589, 357\}$     |           |
| 96421:158a | $0, 0, 0, -e^{12}, -e^{13}, e^{14}, e^{25} + e^{34}, e^{16} + e^{24}, e^{46} + e^{28} + e^{35}$                             | $7/33(1, 2, 3, 3, 4, 4, 6, 5, 7)$                    | $\{\emptyset, 13489, 145789, 357\}$     |           |
| 96421:158b | $0, 0, 0, -e^{12}, -e^{13}, -e^{14}, e^{25} + e^{34}, e^{16} + e^{24}, e^{28} + e^{46} + e^{35}$                            | $7/33(1, 2, 3, 3, 4, 4, 6, 5, 7)$                    | $\{\emptyset, 13489, 145789, 357\}$     |           |
| 96421:159  | $0, 0, 0, e^{12}, e^{13}, e^{24}, e^{34} + e^{25}, e^{26} + e^{14}, e^{46} + e^{35} + e^{18}$                               | $69/643(4, 2, 5, 6, 9, 8, 11, 10, 14)$               | $\{\emptyset, 357\}$                    |           |
| 96421:163  | $0, 0, 0, e^{12}, e^{13}, e^{24}, e^{35}, e^{15} + e^{26}, e^{46} + e^{18}$                                                 | $2/771(123, 104, 189, 227, 312, 331, 501, 435, 558)$ | $\{\emptyset, 125679, 134678, 234589\}$ |           |
| 96421:166  | $0, 0, 0, e^{12}, e^{13}, e^{24}, e^{25} + e^{34}, e^{26} + e^{35}, e^{28} + e^{37}$                                        | $1/11(7, 2, 3, 9, 10, 11, 12, 13, 15)$               | $\{\emptyset, 134689, 1456789, 357\}$   |           |
| 96421:176  | $0, 0, 0, e^{12}, e^{13}, e^{24}, e^{35}, e^{26}, e^{37} + e^{18} + e^{46}$                                                 | $2/39(9, 4, 7, 13, 16, 17, 23, 21, 30)$              | $\{\emptyset, 125679, 134678, 234589\}$ |           |
| 96421:185  | $0, 0, 0, e^{12}, -e^{13}, e^{14} + e^{23}, e^{35}, e^{34} + e^{25} - 2e^{16}, e^{45} + e^{18}$                             | $1/49(11, 27, 22, 38, 33, 49, 55, 60, 71)$           | $\{\emptyset, 125679, 14578, 24689\}$   |           |
| 96421:188  | $0, 0, 0, e^{12}, e^{13}, e^{14}, e^{15}, e^{35} + e^{16}, e^{24} + e^{37} + e^{18}$                                        | $73/699(2, 6, 5, 8, 7, 10, 9, 12, 14)$               | $\{\emptyset, 357\}$                    |           |
| 96421:192  | $0, 0, 0, e^{12}, e^{13}, e^{24}, e^{25} + e^{34}, e^{15} + e^{26}, e^{46} + e^{18}$                                        | $5/441(22, 27, 59, 49, 81, 76, 108, 103, 125)$       | $\{\emptyset, 12569, 13468, 234589\}$   |           |
| 96421:193  | $0, 0, 0, e^{12}, e^{13}, e^{24}, e^{15}, e^{26} + e^{35}, e^{18} + e^{46} + e^{37}$                                        | $1/51(15, 16, 24, 31, 39, 47, 54, 63, 78)$           | $\{\emptyset, 134678, 14568, 357\}$     |           |
| 96421:194a | $0, 0, 0, e^{12}, e^{13}, e^{24}, e^{35}, e^{15} + e^{26}, e^{18} + e^{46} + e^{37}$                                        | $28/219(3, 2, 3, 5, 6, 7, 9, 9, 12)$                 | $\{\emptyset, 125679, 134678, 234589\}$ |           |
| 96421:194b | $0, 0, 0, e^{12}, e^{13}, e^{24}, e^{35}, -e^{15} + e^{26}, e^{37} + e^{46} + e^{18}$                                       | $28/219(3, 2, 3, 5, 6, 7, 9, 9, 12)$                 | $\{\emptyset, 125679, 134678, 234589\}$ |           |
| 96421:197  | $0, 0, 0, e^{12}, e^{13}, e^{24}, e^{25} + e^{34}, e^{26} + e^{35}, e^{37} + e^{15} + e^{28}$                               | $34/311(5, 2, 3, 7, 8, 9, 10, 11, 13)$               | $\{\emptyset, 134689\}$                 |           |
| 96421:204  | $0, 0, 0, e^{12}, e^{13}, e^{23} + e^{14}, e^{35}, e^{16} + e^{25}, e^{18} + e^{36} + e^{45}$                               | $1/49(11, 27, 22, 38, 33, 49, 55, 60, 71)$           | $\{\emptyset, 125679, 14578, 24689\}$   |           |
| 96421:206  | $0, 0, 0, e^{12}, e^{13}, 2e^{14}, e^{35}, e^{16} + e^{25} + e^{34}, e^{45} + e^{36} + e^{18}$                              | $1/49(11, 27, 22, 38, 33, 49, 55, 60, 71)$           | $\{\emptyset, 125679, 14578, 24689\}$   |           |
| 96421:207  | $0, 0, 0, -e^{12}, -2e^{13}, e^{14} - e^{23}, e^{35}, e^{25} + e^{16} + e^{34}, e^{28} + e^{46}$                            | $1/8(2, 3, 4, 5, 6, 7, 10, 9, 12)$                   | $\{\emptyset, 125679, 145789, 2468\}$   |           |
| 96421:213  | $0, 0, 0, e^{12}, e^{13}, e^{24}, e^{35}, e^{26} + e^{14}, e^{16} + e^{28} + e^{37}$                                        | $7/87(6, 3, 4, 9, 10, 12, 14, 15, 18)$               | $\{\emptyset, 248\}$                    |           |
| 96421:218  | $0, 0, 0, -e^{12}, e^{13}, e^{24}, e^{14}, e^{26} + e^{15}, e^{28} + e^{45} + e^{37}$                                       | $6/419(23, 21, 40, 44, 63, 65, 67, 86, 107)$         | $\{\emptyset, 125679, 134689, 234578\}$ |           |
| 96421:219  | $0, 0, 0, -e^{12}, e^{13}, e^{14}, e^{35}, e^{16} + e^{24}, e^{37} + e^{46} + e^{28}$                                       | $16/71(1, 2, 2, 3, 3, 4, 5, 5, 7)$                   | $\{\emptyset, 145789\}$                 |           |
| 96421:220  | $0, 0, 0, e^{12}, e^{13}, e^{24}, e^{35}, e^{14} + e^{26}, e^{18} + e^{37} + e^{46}$                                        | $49/669(6, 3, 5, 9, 11, 12, 16, 15, 21)$             | $\{\emptyset, 234589\}$                 |           |
| 96421:221  | $0, 0, 0, e^{12}, e^{13}, e^{24}, e^{25} + e^{34}, e^{26} + e^{35}, e^{28} + e^{37} + e^{14}$                               | $15/151(6, 2, 3, 8, 9, 10, 11, 12, 14)$              | $\{\emptyset, 357\}$                    |           |
| 96421:222  | $0, 0, 0, e^{12}, e^{13}, e^{24}, e^{25} + e^{34}, e^{15} + e^{26}, e^{18} + e^{35} + e^{46}$                               | $5/17(1, 1, 2, 2, 3, 3, 4, 4, 5)$                    | $\{\emptyset, 12569\}$                  |           |
| 96421:230  | $0, 0, 0, -e^{12}, e^{13}, e^{24}, e^{14} + e^{35}, e^{26} + e^{15}, e^{28} + e^{37} + e^{45}$                              | $42/485(5, 3, 4, 8, 9, 11, 13, 14, 17)$              | $\{\emptyset, 125679\}$                 |           |
| 96421:231  | $0, 0, 0, -e^{12}, -e^{13}, e^{14}, e^{25} + e^{34}, e^{16} + e^{35}, e^{28} + e^{37} + e^{46}$                             | $1/55(14, 22, 25, 36, 39, 50, 61, 64, 86)$           | $\{\emptyset, 13489, 145789, 357\}$     |           |
| 96421:237  | $0, 0, 0, -e^{12}, -2e^{13}, e^{14} - e^{23}, e^{15}, e^{16} + e^{34} + e^{25}, e^{46} + e^{28}$                            | $1/28(8, 9, 16, 17, 24, 25, 32, 33, 42)$             | $\{\emptyset, 12569, 14589, 2468\}$     |           |
| 96421:238a | $0, 0, 0, e^{12}, -e^{13}, e^{23} + e^{14}, e^{35} + e^{24}, -2e^{16} + e^{25} + e^{34}, e^{45} + e^{18}$                   | $31/129(1, 2, 2, 3, 3, 4, 5, 5, 6)$                  | $\{\emptyset, 125679, 14578, 24689\}$   |           |
| 96421:238b | $0, 0, 0, e^{12}, -e^{13}, e^{14} + e^{23}, -e^{24} + e^{35}, e^{25} + e^{34} - 2e^{16}, e^{45} + e^{18}$                   | $31/129(1, 2, 2, 3, 3, 4, 5, 5, 6)$                  | $\{\emptyset, 125679, 14578, 24689\}$   |           |
| 96421:239  | $0, 0, 0, e^{12}, -e^{13}, e^{14} + e^{23}, e^{35}, e^{25} - 2e^{16} + e^{34}, e^{37} + e^{45} + e^{18}$                    | $6/29(1, 3, 2, 4, 3, 5, 5, 6, 7)$                    | $\{\emptyset, 125679\}$                 |           |
| 96421:240  | $0, 0, 0, e^{12}, e^{13}(1 + a_4), e^{23} + (2 + a_4)e^{14}, e^{35}, a_4e^{16} + e^{34} + e^{25}, e^{18} + e^{36} + e^{45}$ | $1/49(11, 27, 22, 38, 33, 49, 55, 60, 71)$           | $\{\emptyset, 125679, 14578, 24689\}$   |           |
| 96421:255  | $0, 0, 0, e^{12}, e^{13}, e^{14} + e^{23}, e^{24}, e^{16} + e^{25}, e^{45} + e^{36} + e^{18}$                               | $1/87(23, 37, 46, 60, 69, 83, 97, 106, 129)$         | $\{\emptyset, 125679, 14578, 24689\}$   |           |
| 96421:256  | $0, 0, 0, -e^{12}, -e^{13}, e^{24}, e^{34} + e^{25}, e^{26} + 2e^{15}, e^{45} + e^{17} + e^{28}$                            | $1/341(113, 98, 181, 211, 294, 309, 392, 407, 505)$  | $\{\emptyset, 12569, 134689, 23458\}$   |           |
| 96421:259  | $0, 0, 0, e^{12}, e^{13}, 2e^{14}, e^{24}, e^{16} + e^{25} + e^{34}, e^{36} + e^{45} + e^{18}$                              | $1/87(23, 37, 46, 60, 69, 83, 97, 106, 129)$         | $\{\emptyset, 125679, 14578, 24689\}$   |           |
| 96421:264a | $0, 0, 0, e^{12}, e^{13}, e^{14} + e^{23}, e^{24} + e^{35}, e^{16} + e^{25}, e^{45} + e^{36} + e^{18}$                      | $31/129(1, 2, 2, 3, 3, 4, 5, 5, 6)$                  | $\{\emptyset, 125679, 14578, 24689\}$   |           |

Table A.4 – Continued to next page

Table A.4 – Continued from previous page

| Name       | g                                                                                                                                                                           | N                                            | S <sub>0</sub>                        | S = S <sub>0</sub> |
|------------|-----------------------------------------------------------------------------------------------------------------------------------------------------------------------------|----------------------------------------------|---------------------------------------|--------------------|
| 96421:264b | $0, 0, 0, e^{12}, -e^{13}, -e^{14} + e^{23}, e^{24} + e^{35}, e^{25} - e^{16}, e^{18} + e^{45} + e^{36}$                                                                    | $31/129(1, 2, 2, 3, 3, 4, 5, 5, 6)$          | $\{\emptyset, 125679, 14578, 24689\}$ |                    |
| 96421:265a | $0, 0, 0, e^{12}, e^{13}, 2e^{14}, e^{35} + e^{24}, e^{16} + e^{34} + e^{25}, e^{18} + e^{36} + e^{45}$                                                                     | $31/129(1, 2, 2, 3, 3, 4, 5, 5, 6)$          | $\{\emptyset, 125679, 14578, 24689\}$ |                    |
| 96421:265b | $0, 0, 0, e^{12}, e^{13}, 2e^{14}, e^{35} - e^{24}, e^{16} + e^{25} + e^{34}, e^{36} + e^{45} + e^{18}$                                                                     | $31/129(1, 2, 2, 3, 3, 4, 5, 5, 6)$          | $\{\emptyset, 125679, 14578, 24689\}$ |                    |
| 96421:270a | $0, 0, 0, -e^{12}, e^{13}, e^{14} - e^{23}, e^{35}, e^{16} + e^{34} - 2e^{25}, e^{46} + e^{28} + e^{37}$                                                                    | $16/71(1, 2, 2, 3, 3, 4, 5, 5, 7)$           | $\{\emptyset, 125679, 145789, 2468\}$ |                    |
| 96421:270b | $0, 0, 0, -e^{12}, -e^{13}, -e^{23} + e^{14}, e^{35}, e^{16} + 2e^{25} + e^{34}, e^{37} + e^{46} + e^{28}$                                                                  | $16/71(1, 2, 2, 3, 3, 4, 5, 5, 7)$           | $\{\emptyset, 125679, 145789, 2468\}$ |                    |
| 96421:278  | $0, 0, 0, -e^{12}, e^{13}, e^{23} + e^{14}, e^{24}, e^{25} + e^{16}, e^{46} + e^{28} + e^{37}$                                                                              | $4/13(1, 1, 2, 2, 3, 3, 3, 4, 5)$            | $\{\emptyset, 125679, 145789, 2468\}$ |                    |
| 96421:281a | $0, 0, 0, e^{12}, a_1 e^{13}, e^{14}, e^{15} + e^{23}, e^{24} + e^{35} + e^{16}, e^{18} + e^{37} + e^{26}$                                                                  | $1/4(1, 2, 2, 3, 3, 4, 4, 5, 6)$             | $\{\emptyset, 13478, 1458, 357\}$     |                    |
| 96421:281b | $0, 0, 0, -e^{12}, a_1 e^{13}, e^{14}, e^{15} + e^{23}, e^{16} + e^{24} + e^{35}, e^{37} + e^{26} + e^{18}$                                                                 | $1/4(1, 2, 2, 3, 3, 4, 4, 5, 6)$             | $\{\emptyset, 13478, 1458, 357\}$     |                    |
| 96421:283  | $0, 0, 0, -e^{12}, -e^{13}, e^{14}, e^{24}, e^{16} + e^{25} + e^{34}, e^{28} + e^{37} + e^{46}$                                                                             | $4/13(1, 1, 2, 2, 3, 3, 3, 4, 5)$            | $\{\emptyset, 125679, 145789, 2468\}$ |                    |
| 96421:285  | $0, 0, 0, a_1 e^{12}, e^{13}(1 + a_1), e^{14} + e^{23}, e^{15}, e^{34} + e^{25} + e^{16}, e^{36} + e^{18} + e^{27}$                                                         | $1/4(1, 2, 2, 3, 3, 4, 4, 5, 6)$             | $\{\emptyset, 12569, 1458, 24689\}$   |                    |
| 96421:291  | $0, 0, 0, e^{12}, e^{13}, e^{24}, e^{34} + e^{25}, e^{14} + e^{26} + e^{35}, e^{28} + e^{37} + e^{16}$                                                                      | $61/503(4, 2, 3, 6, 7, 8, 9, 10, 12)$        | $\{\emptyset, 357\}$                  |                    |
| 96421:294a | $0, 0, 0, -e^{12}, e^{13}, e^{14} + e^{23}, e^{35} + e^{24}, e^{16} + e^{25}, e^{46} + e^{28} + e^{37}$                                                                     | $16/71(1, 2, 2, 3, 3, 4, 5, 5, 7)$           | $\{\emptyset, 125679, 145789, 2468\}$ |                    |
| 96421:294b | $0, 0, 0, -e^{12}, -e^{13}, e^{23} + e^{14}, e^{35} + e^{24}, e^{16} - e^{25}, e^{37} + e^{46} + e^{28}$                                                                    | $16/71(1, 2, 2, 3, 3, 4, 5, 5, 7)$           | $\{\emptyset, 125679, 145789, 2468\}$ |                    |
| 96421:295  | $0, 0, 0, e^{12}, e^{13}(-1 + a_3),$<br>$a_3 e^{14} + e^{23}, e^{24}, (-2 + a_3)e^{16} + e^{25} + e^{34}, e^{18} + e^{45} + e^{36}$                                         | $1/87(23, 37, 46, 60, 69, 83, 97, 106, 129)$ | $\{\emptyset, 125679, 14578, 24689\}$ |                    |
| 96421:298a | $0, 0, 0, -e^{12}, e^{13}, e^{14}, e^{24} + e^{35}, -e^{25} + e^{16} + e^{34}, e^{28} + e^{46} + e^{37}$                                                                    | $16/71(1, 2, 2, 3, 3, 4, 5, 5, 7)$           | $\{\emptyset, 125679, 145789, 2468\}$ |                    |
| 96421:298b | $0, 0, 0, -e^{12}, -e^{13}, e^{14}, e^{35} + e^{24}, e^{34} + e^{25} + e^{16}, e^{46} + e^{28} + e^{37}$                                                                    | $16/71(1, 2, 2, 3, 3, 4, 5, 5, 7)$           | $\{\emptyset, 125679, 145789, 2468\}$ |                    |
| 96421:300a | $0, 0, 0, e^{12}, e^{13}a_2,$<br>$(1 + a_2)e^{14} + e^{23}, e^{35} + e^{24}, (-1 + a_2)e^{16} + e^{34} + e^{25}, e^{18} + e^{45} + e^{36}$                                  | $31/129(1, 2, 2, 3, 3, 4, 5, 5, 6)$          | $\{\emptyset, 125679, 14578, 24689\}$ |                    |
| 96421:300b | $0, 0, 0, e^{12}, e^{13}a_2,$<br>$(1 + a_2)e^{14} + e^{23}, e^{35} - e^{24}, (-1 + a_2)e^{16} + e^{34} + e^{25}, e^{36} + e^{45} + e^{18}$                                  | $31/129(1, 2, 2, 3, 3, 4, 5, 5, 6)$          | $\{\emptyset, 125679, 14578, 24689\}$ |                    |
| 96421:303  | $0, 0, 0, a_1 e^{12}, e^{13}, e^{23} + e^{14}, -(-1 + a_1)e^{15}, e^{25} + e^{16}, e^{27} + e^{36} + e^{45} + e^{18}$                                                       | $1/4(1, 2, 2, 3, 3, 4, 4, 5, 6)$             | $\{\emptyset, 12569, 1458, 24689\}$   |                    |
| 96421:307  | $0, 0, 0, -e^{12}, e^{13}a_2, (1 + a_2)e^{14} + e^{23}, e^{15}, e^{16} + e^{34}, e^{45} + e^{18} + e^{27} + e^{36}$                                                         | $1/4(1, 2, 2, 3, 3, 4, 4, 5, 6)$             | $\{\emptyset, 12569, 1458, 24689\}$   |                    |
| 96421:308  | $0, 0, 0, e^{12}, e^{13}, e^{14}, e^{24} + e^{15}, e^{16} + e^{34} + e^{25}, e^{18} + e^{27} + e^{36}$                                                                      | $11/81(2, 3, 4, 5, 6, 7, 8, 9, 11)$          | $\{\emptyset, 24689\}$                |                    |
| 96421:313  | $0, 0, 0, -e^{12}, e^{13}a_2,$<br>$(1 + a_2)e^{23} + e^{14}, e^{24}(2 + a_2), e^{25} + e^{34} + e^{16}, e^{37} + e^{28} + e^{46}$                                           | $4/13(1, 1, 2, 2, 3, 3, 3, 4, 5)$            | $\{\emptyset, 125679, 145789, 2468\}$ |                    |
| 96421:318a | $0, 0, 0, -e^{12}, e^{13},$<br>$e^{23}(-1 + a_3) + e^{14}, a_3 e^{24} + e^{35}, (-2 + a_3)e^{25} + e^{34} + e^{16}, e^{28} + e^{46} + e^{37}$                               | $16/71(1, 2, 2, 3, 3, 4, 5, 5, 7)$           | $\{\emptyset, 125679, 145789, 2468\}$ |                    |
| 96421:318b | $0, 0, 0, -e^{12}, -e^{13},$<br>$e^{23}(-1 + a_3) + e^{14}, a_3 e^{24} + e^{35}, -(-2 + a_3)e^{25} + e^{16} + e^{34}, e^{37} + e^{46} + e^{28}$                             | $16/71(1, 2, 2, 3, 3, 4, 5, 5, 7)$           | $\{\emptyset, 125679, 145789, 2468\}$ |                    |
| 96421:320  | $0, 0, 0, e^{12}, e^{13}, e^{23} + e^{14}, e^{24}, e^{16} + e^{25}, e^{27} + e^{18} + e^{36} + e^{45}$                                                                      | $11/81(2, 3, 4, 5, 6, 7, 8, 9, 11)$          | $\{\emptyset, 24689\}$                |                    |
| 96421:322  | $0, 0, 0, e^{12}, e^{13}, 2e^{14}, e^{24}, e^{25} + e^{16} + e^{34}, e^{18} + e^{27} + e^{45} + e^{36}$                                                                     | $11/81(2, 3, 4, 5, 6, 7, 8, 9, 11)$          | $\{\emptyset, 24689\}$                |                    |
| 96421:326  | $0, 0, 0, (-1 + a_2)e^{12}, e^{13}a_2,$<br>$e^{14} + e^{23}, e^{15} + e^{24}, e^{34} + e^{16} + e^{25}, e^{27} + e^{36} + e^{18}$                                           | $11/81(2, 3, 4, 5, 6, 7, 8, 9, 11)$          | $\{\emptyset, 24689\}$                |                    |
| 96421:328  | $0, 0, 0,$<br>$(-1 + a_3 - a_5)e^{12}, e^{13}(-1 + a_3), a_3 e^{14} + e^{23},$<br>$-e^{15}(-2 + a_3 - a_5), e^{25} + e^{34} + e^{16}a_5, e^{18} + e^{27} + e^{45} + e^{36}$ | $1/4(1, 2, 2, 3, 3, 4, 4, 5, 6)$             | $\{\emptyset, 12569, 1458, 24689\}$   |                    |
| 96421:332  | $0, 0, 0, a_1 e^{12}, e^{13},$<br>$e^{14} + e^{23}, -(-1 + a_1)e^{15} + e^{24}, e^{16} + e^{25}, e^{36} + e^{18} + e^{27} + e^{45}$                                         | $11/81(2, 3, 4, 5, 6, 7, 8, 9, 11)$          | $\{\emptyset, 24689\}$                |                    |
| 96421:333  | $0, 0, 0, -e^{12}, e^{13}(-1 + a_3),$<br>$a_3 e^{14} + e^{23}, e^{15} + e^{24}, e^{34} + e^{16}, e^{45} + e^{36} + e^{18} + e^{27}$                                         | $11/81(2, 3, 4, 5, 6, 7, 8, 9, 11)$          | $\{\emptyset, 24689\}$                |                    |
| 96421:334  | $0, 0, 0, e^{12}a_2, e^{13}a_2,$<br>$(1 + a_2)e^{14}, -(-1 + a_2)e^{15} + e^{24}, e^{16} + e^{34} + e^{25}, e^{18} + e^{27} + e^{36} + e^{45}$                              | $11/81(2, 3, 4, 5, 6, 7, 8, 9, 11)$          | $\{\emptyset, 24689\}$                |                    |
| 96421:336  | $0, 0, 0, e^{12}, e^{13}(1 + a_4),$<br>$e^{23} + (2 + a_4)e^{14}, e^{24}, a_4 e^{16} + e^{25} + e^{34}, e^{36} + e^{27} + e^{18} + e^{45}$                                  | $11/81(2, 3, 4, 5, 6, 7, 8, 9, 11)$          | $\{\emptyset, 24689\}$                |                    |

Table A.4 – Continued to next page

Table A.4 – Continued from previous page

| Name       | g                                                                                                                                                                             | N                                                  | S <sub>0</sub>                                        | S = S <sub>0</sub> |
|------------|-------------------------------------------------------------------------------------------------------------------------------------------------------------------------------|----------------------------------------------------|-------------------------------------------------------|--------------------|
| 96421:338  | 0, 0, 0,<br>$a_1 e^{12}, e^{13}(-1 + a_3), a_3 e^{14} + e^{23},$<br>$-(-1 + a_1)e^{15} + e^{24}, (-1 + a_3 - a_1)e^{16} + e^{25} + e^{34}, e^{27} + e^{18} + e^{36} + e^{45}$ | 11/81(2, 3, 4, 5, 6, 7, 8, 9, 11)                  | {0, 24689}                                            |                    |
| 96421:339  | 0, 0, 0, $e^{12}, e^{13}, e^{14}, e^{24}, e^{17} + e^{26}, e^{46} + e^{18}$                                                                                                   | 1/55(10, 23, 50, 33, 60, 43, 56, 66, 76)           | {0, 123679, 125679, 13479, 14579, 23456, 246, 35}     |                    |
| 96421:340a | 0, 0, 0, $-e^{12}, e^{13}, e^{14}, e^{24}, e^{27} + e^{16}, e^{46} + e^{28}$                                                                                                  | 2/131(19, 19, 56, 38, 75, 57, 57, 76, 95)          | {0, 123679, 125679, 134789, 145789, 234568, 2468, 35} |                    |
| 96421:340b | 0, 0, 0, $-e^{12}, e^{13}, -e^{14}, e^{24}, e^{16} + e^{27}, e^{46} + e^{28}$                                                                                                 | 2/131(19, 19, 56, 38, 75, 57, 57, 76, 95)          | {0, 123679, 125679, 134789, 145789, 234568, 2468, 35} |                    |
| 96421:341a | 0, 0, 0, $e^{12}, e^{13}, e^{24}, e^{14}, e^{17} + e^{26}, e^{46} + e^{18}$                                                                                                   | 2/131(19, 19, 56, 38, 75, 57, 57, 76, 95)          | {0, 123679, 125679, 13468, 14568, 2345789, 24789, 35} |                    |
| 96421:341b | 0, 0, 0, $e^{12}, e^{13}, e^{24}, -e^{14}, e^{26} + e^{17}, e^{46} + e^{18}$                                                                                                  | 2/131(19, 19, 56, 38, 75, 57, 57, 76, 95)          | {0, 123679, 125679, 13468, 14568, 2345789, 24789, 35} |                    |
| 96421:342  | 0, 0, 0, $-e^{12}, e^{13}, e^{24}, e^{14}, e^{16} + e^{27}, e^{46} + e^{28}$                                                                                                  | 2/17(3, 2, 7, 5, 10, 7, 8, 10, 12)                 | {0, 123679, 125679, 1346, 1456, 234579, 2479, 35}     |                    |
| 96421:343a | 0, 0, 0, $e^{12}, e^{13}, e^{14}, e^{24}, e^{17} + e^{26}, e^{18} + e^{46} + e^{35}$                                                                                          | 1/101(23, 41, 64, 64, 87, 87, 105, 128, 151)       | {0, 123679, 125679, 13479, 14579, 23456, 246, 35}     |                    |
| 96421:343b | 0, 0, 0, $e^{12}, -e^{13}, e^{14}, e^{24}, e^{17} + e^{26}, e^{18} + e^{35} + e^{46}$                                                                                         | 1/101(23, 41, 64, 64, 87, 87, 105, 128, 151)       | {0, 123679, 125679, 13479, 14579, 23456, 246, 35}     |                    |
| 96421:344a | 0, 0, 0, $-e^{12}, e^{13}, e^{14}, e^{24}, e^{16} + e^{27}, e^{28} + e^{35} + e^{46}$                                                                                         | 4/13(1, 1, 2, 2, 3, 3, 3, 4, 5)                    | {0, 123679, 125679, 134789, 145789, 234568, 2468, 35} | ✓                  |
| 96421:344b | 0, 0, 0, $-e^{12}, e^{13}, -e^{14}, e^{24}, e^{27} + e^{16}, e^{28} + e^{46} + e^{35}$                                                                                        | 4/13(1, 1, 2, 2, 3, 3, 3, 4, 5)                    | {0, 123679, 125679, 134789, 145789, 234568, 2468, 35} | ✓                  |
| 96421:344c | 0, 0, 0, $-e^{12}, -e^{13}, e^{14}, e^{24}, e^{27} + e^{16}, e^{46} + e^{35} + e^{28}$                                                                                        | 4/13(1, 1, 2, 2, 3, 3, 3, 4, 5)                    | {0, 123679, 125679, 134789, 145789, 234568, 2468, 35} | ✓                  |
| 96421:344d | 0, 0, 0, $-e^{12}, -e^{13}, -e^{14}, e^{24}, e^{27} + e^{16}, e^{35} + e^{46} + e^{28}$                                                                                       | 4/13(1, 1, 2, 2, 3, 3, 3, 4, 5)                    | {0, 123679, 125679, 134789, 145789, 234568, 2468, 35} | ✓                  |
| 96421:345a | 0, 0, 0, $e^{12}, e^{13}, e^{24}, e^{14}, e^{26} + e^{17}, e^{35} + e^{18} + e^{46}$                                                                                          | 4/13(1, 1, 2, 2, 3, 3, 3, 4, 5)                    | {0, 123679, 125679, 35}                               |                    |
| 96421:345b | 0, 0, 0, $e^{12}, e^{13}, e^{24}, -e^{14}, e^{17} + e^{26}, e^{18} + e^{46} + e^{35}$                                                                                         | 4/13(1, 1, 2, 2, 3, 3, 3, 4, 5)                    | {0, 123679, 125679, 35}                               |                    |
| 96421:346  | 0, 0, 0, $-e^{12}, e^{13}, e^{24}, e^{14}, e^{27} + e^{16}, e^{28} + e^{46} + e^{35}$                                                                                         | 2/419(71, 59, 124, 130, 195, 189, 201, 260, 319)   | {0, 123679, 125679, 35}                               |                    |
| 96421:350  | 0, 0, 0, $-e^{12}, e^{13}, e^{24}, e^{14}, e^{27} + e^{16}, e^{28} + e^{46} + e^{15}$                                                                                         | 1/71(23, 19, 57, 42, 80, 61, 65, 84, 103)          | {0, 123679, 1456, 234579}                             |                    |
| 96421:352  | 0, 0, 0, $e^{12}, e^{13}, e^{14}, e^{24}, e^{17} + e^{26}, e^{18} + e^{27} + e^{46}$                                                                                          | 1/281(56, 112, 253, 168, 309, 224, 280, 336, 392)  | {0, 13479, 14579, 35}                                 |                    |
| 96421:353  | 0, 0, 0, $-e^{12}, e^{13}, e^{24}, e^{23} + e^{14}, e^{27} + e^{16}, e^{28} + e^{46}$                                                                                         | 2/67(13, 7, 26, 20, 39, 27, 33, 40, 47)            | {0, 125679, 1456, 2479}                               |                    |
| 96421:358  | 0, 0, 0, $-e^{12}, e^{13}, e^{24}, e^{14} + e^{23}, e^{27} + e^{16}, e^{15} + e^{28} + e^{46}$                                                                                | 31/256(3, 2, 6, 5, 9, 7, 8, 10, 12)                | {0, 1456}                                             |                    |
| 96421:414  | 0, 0, 0, $e^{12}, e^{13}, e^{24}, e^{15}, e^{26} + e^{17}, e^{18} + e^{46}$                                                                                                   | 1/327(48, 119, 261, 167, 309, 286, 357, 405, 453)  | {0, 123679, 14568, 2345789}                           |                    |
| 96421:415  | 0, 0, 0, $e^{12}, e^{13}, e^{14}, e^{15} + e^{24}, e^{26} + e^{17}, e^{18} + e^{46}$                                                                                          | 1/157(19, 78, 137, 97, 156, 116, 175, 194, 213)    | {0, 123679, 13479, 246}                               |                    |
| 96421:417  | 0, 0, 0, $e^{12}, e^{13}, e^{24}, e^{15}, e^{17} + e^{26}, e^{18} + e^{35} + e^{46}$                                                                                          | 4/57(3, 5, 9, 8, 12, 13, 15, 18, 21)               | {0, 123679}                                           |                    |
| 96421:418  | 0, 0, 0, $e^{12}, e^{13}, e^{24}, e^{35}, e^{37} + e^{26}, e^{18} + e^{57} + e^{46}$                                                                                          | 2/15(3, 2, 2, 5, 5, 7, 7, 9, 12)                   | {0, 123679, 145678, 234589}                           |                    |
| 96421:421  | 0, 0, 0, $e^{12}, -e^{13}, e^{25} - e^{34}, -2e^{14}, e^{16} + e^{45} + e^{37}, e^{38} + e^{56}$                                                                              | 1/4(1, 2, 1, 3, 2, 4, 4, 5, 6)                     | {0, 123679, 125789, 1348, 1456, 234579, 246789, 3568} |                    |
| 96421:422  | 0, 0, 0, $e^{12}, e^{13}, e^{14}, e^{15} + e^{24}, e^{17} + e^{26}, e^{18} + e^{46} + e^{23}$                                                                                 | 61/493(1, 4, 7, 5, 8, 6, 9, 10, 11)                | {0, 13479}                                            |                    |
| 96421:423a | 0, 0, 0, $e^{12}, e^{13}, e^{14}, e^{24} + e^{15}, e^{17} + e^{26}, e^{35} + e^{46} + e^{18}$                                                                                 | 7/33(1, 2, 3, 3, 4, 4, 5, 6, 7)                    | {0, 123679, 13479, 246}                               |                    |
| 96421:423b | 0, 0, 0, $e^{12}, -e^{13}, e^{14}, e^{24} + e^{15}, e^{26} + e^{17}, e^{35} + e^{18} + e^{46}$                                                                                | 7/33(1, 2, 3, 3, 4, 4, 5, 6, 7)                    | {0, 123679, 13479, 246}                               |                    |
| 96421:424  | 0, 0, 0, $e^{12}, e^{13}, e^{14}, e^{35}, e^{37} + e^{16} + e^{24}, e^{18} + e^{57} + e^{26}$                                                                                 | 17/201(3, 6, 4, 9, 7, 12, 11, 15, 18)              | {0, 14578}                                            |                    |
| 96421:426  | 0, 0, 0, $e^{12}, e^{13}, e^{24}, e^{25} + e^{34}, e^{27} + e^{36}, e^{56} + e^{18} + e^{47}$                                                                                 | 1/5(2, 1, 2, 3, 4, 4, 5, 6, 8)                     | {0, 123679, 12568, 13469, 145678, 234589, 247, 35789} |                    |
| 96421:440a | 0, 0, 0, $e^{12}, e^{13}, e^{25} + e^{34}, e^{35} + e^{24}, e^{26} + e^{37}, e^{18} + e^{46} + e^{57}$                                                                        | 2/15(3, 2, 2, 5, 5, 7, 7, 9, 12)                   | {0, 123679, 12578, 13479, 145678, 234589, 246, 35689} |                    |
| 96421:440b | 0, 0, 0, $e^{12}, e^{13}, -e^{25} - e^{34}, -e^{24} + e^{35}, e^{37} + e^{26}, e^{18} + e^{57} + e^{46}$                                                                      | 2/15(3, 2, 2, 5, 5, 7, 7, 9, 12)                   | {0, 123679, 12578, 13479, 145678, 234589, 246, 35689} |                    |
| 96421:447  | 0, 0, 0, $e^{12}, e^{13}, e^{14} + e^{23}, e^{24} + e^{15}, e^{26} + e^{35} + e^{17}, e^{37} + e^{18} + e^{46}$                                                               | 19/149(2, 3, 4, 5, 6, 7, 8, 10, 12)                | {0, 246}                                              |                    |
| 9642:3     | 0, 0, 0, $e^{12}, e^{13}, e^{14}, e^{24}, e^{16}, e^{26} + e^{17}$                                                                                                            | 1/51(12, 22, 45, 34, 57, 46, 56, 58, 68)           | {0, 12367, 12567, 13478, 14578, 234568, 2468, 35}     |                    |
| 9642:4     | 0, 0, 0, $e^{12}, e^{13}, e^{24}, e^{14}, e^{26}, e^{27} + e^{16}$                                                                                                            | 1/106(40, 29, 86, 69, 126, 98, 109, 127, 138)      | {0, 12367, 12567, 13468, 14568, 234578, 2478, 35}     |                    |
| 9642:8     | 0, 0, 0, $e^{12}, e^{13}, e^{14}, e^{24}, e^{23} + e^{16}, e^{26} + e^{17}$                                                                                                   | 1/33(9, 13, 27, 22, 36, 31, 35, 40, 44)            | {0, 12367, 13478, 2468}                               |                    |
| 9642:9     | 0, 0, 0, $-e^{12}, e^{13}, e^{24}, e^{23} + e^{14}, e^{26}, e^{17} + e^{34}$                                                                                                  | 1/389(139, 116, 278, 255, 417, 371, 394, 487, 533) | {0, 12567, 145689, 24789}                             |                    |
| 9642:11a   | 0, 0, 0, $e^{12}, e^{13}, e^{14}, e^{24}, e^{17} + e^{26}, e^{16} + e^{27}$                                                                                                   | 1/113(36, 36, 95, 72, 131, 108, 108, 144, 144)     | {0, 12367, 12567, 13479, 14579, 234569, 2469, 35}     | ✓                  |
| 9642:11b   | 0, 0, 0, $e^{12}, e^{13}, -e^{14}, e^{24}, -e^{17} + e^{26}, e^{27} + e^{16}$                                                                                                 | 1/113(36, 36, 95, 72, 131, 108, 108, 144, 144)     | {0, 12367, 12567, 13479, 14579, 234569, 2469, 35}     | ✓                  |
| 9642:12    | 0, 0, 0, $e^{12}, e^{13}, e^{24}, e^{23} + e^{14}, e^{26}, e^{25} + e^{17}$                                                                                                   | 1/389(139, 116, 278, 255, 417, 371, 394, 487, 533) | {0, 12567, 145689, 24789}                             |                    |
| 9642:14    | 0, 0, 0, $e^{12}, e^{13}, e^{24}, e^{23} + e^{14}, e^{26}, e^{27} + e^{16}$                                                                                                   | 1/178(70, 47, 140, 117, 210, 164, 187, 211, 234)   | {0, 12567, 14568, 2478}                               |                    |
| 9642:16    | 0, 0, 0, $e^{12}, e^{13}, e^{24}, e^{14}, e^{26}, e^{25} + e^{34} + e^{17}$                                                                                                   | 1/389(139, 116, 278, 255, 417, 371, 394, 487, 533) | {0, 12567, 145689, 24789}                             |                    |
| 9642:17    | 0, 0, 0, $e^{12}, e^{13}, e^{14}, e^{24}, e^{16}, e^{26} + e^{17} + e^{35}$                                                                                                   | 1/119(28, 57, 71, 85, 99, 113, 142, 141, 170)      | {0, 234568, 2468, 35}                                 |                    |
| 9642:18    | 0, 0, 0, $e^{12}, e^{13}, e^{24}, e^{14}, e^{26}, e^{16} + e^{27} + e^{35}$                                                                                                   | 2/123(26, 17, 30, 43, 56, 60, 69, 77, 86)          | {0, 234578, 2478, 35}                                 |                    |
| 9642:20    | 0, 0, 0, $e^{12}, e^{13}, e^{24}, e^{14}, e^{26} + e^{35}, e^{16} + e^{27}$                                                                                                   | 1/109(36, 38, 57, 74, 93, 112, 110, 150, 148)      | {0, 13468, 14568, 35}                                 |                    |

Table A.4 – Continued to next page

Table A.4 – Continued from previous page

| Name      | g                                                                                                                   | N                                                    | S <sub>0</sub>                                                    | S = S <sub>0</sub> |
|-----------|---------------------------------------------------------------------------------------------------------------------|------------------------------------------------------|-------------------------------------------------------------------|--------------------|
| 9642:21   | $0, 0, 0, e^{12}, e^{13}, e^{24}, e^{14} + e^{23}, e^{35} + e^{26}, e^{17} + e^{25}$                                | $3/31(3, 4, 6, 7, 9, 11, 10, 15, 13)$                | $\{\emptyset, 145689\}$                                           |                    |
| 9642:22   | $0, 0, 0, -e^{12}, e^{13}, e^{14} + e^{23}, e^{24}, e^{16} + e^{34}, e^{35} + e^{27}$                               | $3/31(3, 4, 6, 7, 9, 10, 11, 13, 15)$                | $\{\emptyset, 145789\}$                                           |                    |
| 9642:23   | $0, 0, 0, e^{12}, e^{13}, e^{24}, e^{14}, e^{15} + e^{26}, e^{27} + e^{16}$                                         | $1/413(122, 145, 313, 267, 435, 412, 389, 557, 534)$ | $\{\emptyset, 12567, 13468, 234578\}$                             |                    |
| 9642:25   | $0, 0, 0, (-1 + a_2)e^{12}, a_2e^{13}, e^{24}, e^{14} + e^{23}, e^{26}, e^{17} + e^{34} + e^{25}$                   | $1/389(139, 116, 278, 255, 417, 371, 394, 487, 533)$ | $\{\emptyset, 12567, 145689, 24789\}$                             |                    |
| 9642:26   | $0, 0, 0, -e^{12}, e^{13}, e^{14} + e^{23}, e^{24}, e^{34} + e^{16}, e^{15} + e^{27}$                               | $1/3(1, 1, 2, 2, 3, 3, 3, 4, 4)$                     | $\{\emptyset, 12567\}$                                            |                    |
| 9642:27   | $0, 0, 0, e^{12}, e^{13}, e^{24}, e^{14}, e^{26} + e^{35}, e^{17} + e^{25} + e^{34}$                                | $3/31(3, 4, 6, 7, 9, 11, 10, 15, 13)$                | $\{\emptyset, 145689\}$                                           |                    |
| 9642:32   | $0, 0, 0, e^{12}, e^{13}, e^{24}, e^{14}, e^{26} + e^{15}, e^{25} + e^{34} + e^{17}$                                | $1/3(1, 1, 2, 2, 3, 3, 3, 4, 4)$                     | $\{\emptyset, 12567\}$                                            |                    |
| 9642:34   | $0, 0, 0, e^{12}, e^{13}, e^{24}, e^{14}, e^{26} + e^{15}, e^{16} + e^{27} + e^{35}$                                | $38/383(4, 3, 5, 7, 9, 10, 11, 13, 14)$              | $\{\emptyset, 234578\}$                                           |                    |
| 9642:36   | $0, 0, 0, e^{12}a_1, (1 + a_1)e^{13}, e^{24}, e^{23} + e^{14}, e^{26} + e^{35}, e^{17} + e^{25} + e^{34}$           | $3/31(3, 4, 6, 7, 9, 11, 10, 15, 13)$                | $\{\emptyset, 145689\}$                                           |                    |
| 9642:38a  | $0, 0, 0, e^{12}, e^{13}, e^{14}, e^{24}, e^{16} + e^{27}, e^{17} + e^{35} + e^{26}$                                | $22/129(2, 2, 3, 4, 5, 6, 6, 8, 8)$                  | $\{\emptyset, 234568, 2468, 35\}$                                 | ✓                  |
| 9642:38b  | $0, 0, 0, e^{12}, e^{13}, e^{14}, e^{24}, e^{27} - e^{16}, e^{35} + e^{17} + e^{26}$                                | $22/129(2, 2, 3, 4, 5, 6, 6, 8, 8)$                  | $\{\emptyset, 234568, 2468, 35\}$                                 | ✓                  |
| 9642:40   | $0, 0, 0, (-1 + a_2)e^{12}, a_2e^{13}, e^{24}, e^{14} + e^{23}, e^{26} + e^{15}, e^{34} + e^{17} + e^{25}$          | $1/3(1, 1, 2, 2, 3, 3, 3, 4, 4)$                     | $\{\emptyset, 12567\}$                                            |                    |
| 9642:42   | $0, 0, 0, e^{12}, e^{13}, e^{14} + e^{23}, e^{24}, e^{16} + e^{25}, e^{17} + e^{26} + e^{35}$                       | $9/64(2, 3, 4, 5, 6, 7, 8, 9, 10)$                   | $\{\emptyset, 2468\}$                                             |                    |
| 9642:43   | $0, 0, 0, -e^{12}, e^{13}, e^{14} + e^{23}, e^{24}, e^{16} + e^{34}, e^{17} + e^{26} + e^{35}$                      | $9/64(2, 3, 4, 5, 6, 7, 8, 9, 10)$                   | $\{\emptyset, 2468\}$                                             |                    |
| 9642:44   | $0, 0, 0, e^{12}, e^{13}, e^{14}, e^{24}, e^{34} + e^{25} + e^{16}, e^{35} + e^{26} + e^{17}$                       | $9/64(2, 3, 4, 5, 6, 7, 8, 9, 10)$                   | $\{\emptyset, 2468\}$                                             |                    |
| 9642:45   | $0, 0, 0, e^{12}a_1, (1 + a_1)e^{13}, e^{23} + e^{14}, e^{24}, e^{16} + e^{25} + e^{34}, e^{17} + e^{26}$           | $1/3(1, 1, 2, 2, 3, 3, 3, 4, 4)$                     | $\{\emptyset, 12567, 14578, 2468\}$                               |                    |
| 9642:47   | $0, 0, 0, (-1 + a_2)e^{12}, a_2e^{13}, e^{23} + e^{14}, e^{24}, e^{34} + e^{25} + e^{16}, e^{35} + e^{17} + e^{26}$ | $9/64(2, 3, 4, 5, 6, 7, 8, 9, 10)$                   | $\{\emptyset, 2468\}$                                             |                    |
| 9642:65   | $0, 0, 0, e^{12}, e^{13}, e^{14}, e^{15} + e^{24}, e^{16}, e^{17} + e^{26}$                                         | $3/160(10, 27, 44, 37, 54, 47, 64, 57, 74)$          | $\{\emptyset, 12367, 13478, 2468\}$                               |                    |
| 9642:66   | $0, 0, 0, e^{12}, e^{13}, e^{24}, e^{34} + e^{25}, e^{26}, e^{27} + e^{36}$                                         | $1/31(19, 5, 13, 24, 32, 29, 37, 34, 42)$            | $\{\emptyset, 12367, 12569, 13468, 1456789, 234589, 2478, 3579\}$ |                    |
| 9642:82   | $0, 0, 0, -e^{12}, e^{13}, e^{14}, e^{15}, e^{16}, e^{45} + e^{36} + e^{27}$                                        | $1/31(5, 19, 20, 24, 25, 29, 30, 34, 49)$            | $\{\emptyset, 12367, 12569, 134789, 1458, 2345678, 24689, 3579\}$ |                    |
| 9642:83a  | $0, 0, 0, e^{12}, e^{13}, e^{14}, e^{15} + e^{24}, e^{16} + e^{23}, e^{17} + e^{26}$                                | $11/47(1, 2, 3, 3, 4, 4, 5, 5, 6)$                   | $\{\emptyset, 12367, 13478, 2468\}$                               | ✓                  |
| 9642:83b  | $0, 0, 0, -e^{12}, e^{13}, e^{14}, e^{24} + e^{15}, e^{23} + e^{16}, e^{17} + e^{26}$                               | $11/47(1, 2, 3, 3, 4, 4, 5, 5, 6)$                   | $\{\emptyset, 12367, 13478, 2468\}$                               | ✓                  |
| 9642:86   | $0, 0, 0, -e^{12}, a_2e^{13}, e^{14}, e^{23} + e^{15}, e^{16} + e^{24}, e^{17} + e^{34}$                            | $1/8(2, 4, 5, 6, 7, 8, 9, 10, 11)$                   | $\{\emptyset, 13478, 14589, 3579\}$                               |                    |
| 9642:97   | $0, 0, 0, e^{12}, e^{13}, e^{24}, e^{34} + e^{25}, e^{26}, e^{27} + e^{36} + e^{14}$                                | $1/281(168, 47, 121, 215, 289, 262, 336, 309, 383)$  | $\{\emptyset, 12569, 13468, 234589\}$                             |                    |
| 9642:99   | $0, 0, 0, e^{12}, e^{13}, e^{24}, e^{25} + e^{34}, e^{26}, e^{36} + e^{27} + e^{15}$                                | $4/17(2, 1, 2, 3, 4, 4, 5, 5, 6)$                    | $\{\emptyset, 234589, 2478, 3579\}$                               |                    |
| 9642:102  | $0, 0, 0, e^{12}, e^{13}, e^{24}, e^{25} + e^{34}, e^{15} + e^{26}, e^{27} + e^{36}$                                | $1/361(156, 101, 147, 257, 303, 358, 404, 459, 505)$ | $\{\emptyset, 12569, 13468, 234589\}$                             |                    |
| 9642:103  | $0, 0, 0, e^{12}, e^{13}, e^{24}, e^{25} + e^{34}, e^{26} + e^{35}, e^{36} + e^{27}$                                | $1/67(40, 14, 21, 54, 61, 68, 75, 82, 89)$           | $\{\emptyset, 13468, 1456789, 3579\}$                             |                    |
| 9642:104  | $0, 0, 0, -e^{12}, e^{13}, e^{14}, e^{15} + e^{23}, e^{16}, e^{45} + e^{36} + e^{27}$                               | $2/17(2, 4, 5, 6, 7, 8, 9, 10, 13)$                  | $\{\emptyset, 134789, 1458, 3579\}$                               |                    |
| 9642:110  | $0, 0, 0, -e^{12}, e^{13}, e^{14}, e^{15} + e^{24}, e^{16}, e^{27} + e^{36} + e^{45}$                               | $1/369(83, 162, 241, 245, 324, 328, 407, 411, 569)$  | $\{\emptyset, 12367, 134789, 24689\}$                             |                    |
| 9642:111  | $0, 0, 0, e^{12}, e^{13}, 2e^{14}, e^{25} + e^{34}, e^{16}, e^{36} + e^{45} + e^{17}$                               | $1/72(14, 38, 39, 52, 53, 66, 91, 80, 105)$          | $\{\emptyset, 12367, 12569, 13489, 14578, 234568, 246789, 3579\}$ |                    |
| 9642:116  | $0, 0, 0, e^{12}, e^{13}, a_2e^{14}, e^{15}, e^{16} + e^{24}, e^{17} + e^{34} + e^{25}$                             | $1/8(2, 4, 5, 6, 7, 8, 9, 10, 11)$                   | $\{\emptyset, 13478, 14589, 3579\}$                               |                    |
| 9642:120  | $0, 0, 0, -e^{12}, e^{13}, e^{14}, e^{15}, e^{23} + e^{16}, e^{36} + e^{45} + e^{27}$                               | $1/329(65, 186, 195, 251, 260, 316, 325, 381, 511)$  | $\{\emptyset, 12367, 134789, 24689\}$                             |                    |
| 9642:122  | $0, 0, 0, -e^{12}, e^{13}, e^{14}, e^{15}, e^{16} + e^{35}, e^{45} + e^{27} + e^{36}$                               | $2/67(7, 20, 17, 27, 24, 34, 31, 41, 51)$            | $\{\emptyset, 134789, 1458, 3579\}$                               |                    |
| 9642:123  | $0, 0, 0, -e^{12}, e^{13}, e^{23} + e^{14}, e^{24} + e^{15}, e^{16} + e^{34}, e^{17} + e^{26}$                      | $9/64(2, 3, 4, 5, 6, 7, 8, 9, 10)$                   | $\{\emptyset, 2468\}$                                             |                    |
| 9642:126a | $0, 0, 0, e^{12}, e^{13}, e^{25} + e^{34}, e^{24} + e^{35}, e^{36} + e^{27}, e^{37} + e^{26}$                       | $7/33(3, 1, 1, 4, 4, 5, 5, 6, 6)$                    | $\{\emptyset, 12367, 12579, 13478, 1456789, 234589, 2468, 3569\}$ |                    |
| 9642:126b | $0, 0, 0, -e^{12}, e^{13}, -e^{25} + e^{34}, e^{24} + e^{35}, -e^{27} + e^{36}, e^{26} + e^{37}$                    | $7/33(3, 1, 1, 4, 4, 5, 5, 6, 6)$                    | $\{\emptyset, 12367, 12579, 13478, 1456789, 234589, 2468, 3569\}$ |                    |
| 9642:128  | $0, 0, 0, (-1 + a_2)e^{12}, a_2e^{13}, a_3e^{14}, e^{15} + e^{23}, e^{24} + e^{16}, e^{25} + e^{34} + e^{17}$       | $1/8(2, 4, 5, 6, 7, 8, 9, 10, 11)$                   | $\{\emptyset, 13478, 14589, 3579\}$                               |                    |
| 9642:130a | $0, 0, 0, -e^{12}, e^{13}, a_2e^{14} + e^{23}, e^{15}, e^{34} + e^{16}, e^{35} + e^{24} + e^{17}$                   | $29/109(1, 2, 2, 3, 3, 4, 4, 5, 5)$                  | $\{\emptyset, 12569, 14589, 2468\}$                               |                    |
| 9642:130b | $0, 0, 0, -e^{12}, -e^{13}, a_2e^{14} + e^{23}, e^{15}, e^{34} + e^{16}, e^{24} + e^{17} + e^{35}$                  | $29/109(1, 2, 2, 3, 3, 4, 4, 5, 5)$                  | $\{\emptyset, 12569, 14589, 2468\}$                               |                    |
| 9642:132a | $0, 0, 0, -e^{12}, e^{13}, a_2e^{14}, e^{23} + e^{15}, e^{35} + e^{24} + e^{16}, e^{34} + e^{17}$                   | $29/109(1, 2, 2, 3, 3, 4, 4, 5, 5)$                  | $\{\emptyset, 13478, 14589, 3579\}$                               |                    |
| 9642:132b | $0, 0, 0, -e^{12}, -e^{13}, a_2e^{14}, e^{23} + e^{15}, e^{35} + e^{24} + e^{16}, e^{17} + e^{34}$                  | $29/109(1, 2, 2, 3, 3, 4, 4, 5, 5)$                  | $\{\emptyset, 13478, 14589, 3579\}$                               |                    |
| 9642:143  | $0, 0, 0, e^{12}, e^{13}, e^{24}, e^{34} + e^{25}, a_2e^{14} + e^{26}, e^{36} + e^{15} + e^{27}$                    | $4/17(2, 1, 2, 3, 4, 4, 5, 5, 6)$                    | $\{\emptyset, 234589, 2478, 3579\}$                               |                    |
| 9642:145  | $0, 0, 0, e^{12}, e^{13}, e^{24}, e^{25} + e^{34}, e^{26} + e^{35}, e^{14} + e^{36} + e^{27}$                       | $67/597(5, 2, 3, 7, 8, 9, 10, 11, 12)$               | $\{\emptyset, 13468\}$                                            |                    |
| 9642:148  | $0, 0, 0, e^{12}, e^{13}, e^{24}, e^{25} + e^{34}, e^{35} + e^{26}, e^{36} + e^{15} + e^{27}$                       | $1/8(4, 2, 3, 6, 7, 8, 9, 10, 11)$                   | $\{\emptyset, 3579\}$                                             |                    |
| 9642:149  | $0, 0, 0, -e^{12}a_1, e^{13}, e^{14}, e^{15}a_1 + e^{23}, e^{24} + e^{16}, e^{45} + e^{36} + e^{27}$                | $2/17(2, 4, 5, 6, 7, 8, 9, 10, 13)$                  | $\{\emptyset, 134789, 1458, 3579\}$                               |                    |
| 9642:150a | $0, 0, 0, -e^{12}, e^{13}, e^{14}, e^{15} + e^{23}, e^{16} + e^{35}, e^{45} + e^{27} + e^{36}$                      | $1/4(1, 2, 2, 3, 3, 4, 4, 5, 6)$                     | $\{\emptyset, 134789, 1458, 3579\}$                               |                    |
| 9642:150b | $0, 0, 0, -e^{12}, -e^{13}, -e^{14}, e^{23} + e^{15}, e^{16} + e^{35}, e^{27} + e^{36} + e^{45}$                    | $1/4(1, 2, 2, 3, 3, 4, 4, 5, 6)$                     | $\{\emptyset, 134789, 1458, 3579\}$                               |                    |

Table A.4 – Continued to next page

Table A.4 – Continued from previous page

| Name      | g                                                                                                                                          | N                                                  | S <sub>0</sub>                                                    | S = S <sub>0</sub> |
|-----------|--------------------------------------------------------------------------------------------------------------------------------------------|----------------------------------------------------|-------------------------------------------------------------------|--------------------|
| 9642:153  | $0, 0, 0, e^{12}, e^{13}, 2e^{14}, e^{25} + e^{34}, e^{16} + e^{24}, e^{17} + e^{36} + e^{45}$                                             | $1/13(3, 6, 7, 9, 10, 12, 16, 15, 19)$             | $\{\emptyset, 13489, 14578, 3579\}$                               |                    |
| 9642:154  | $0, 0, 0, -e^{12}, e^{13}, e^{14}, e^{15} + e^{24}, e^{16} + e^{35}, e^{45} + e^{36} + e^{27}$                                             | $38/389(3, 4, 5, 7, 8, 10, 11, 13, 15)$            | $\{\emptyset, 134789\}$                                           |                    |
| 9642:155  | $0, 0, 0, e^{12}, e^{13}, 2e^{14}, e^{25} + e^{34}, e^{16} + e^{35}, e^{17} + e^{45} + e^{36}$                                             | $1/48(10, 26, 23, 36, 33, 46, 59, 56, 69)$         | $\{\emptyset, 13489, 14578, 3579\}$                               |                    |
| 9642:157  | $0, 0, 0, -e^{12}, e^{13}, e^{23} + e^{14}, e^{15}, e^{34} + e^{16}, e^{27} + e^{36} + e^{45}$                                             | $1/4(1, 2, 2, 3, 3, 4, 4, 5, 6)$                   | $\{\emptyset, 12569, 1458, 24689\}$                               |                    |
| 9642:158  | $0, 0, 0, -e^{12}, e^{13}, e^{23} + e^{14}, e^{15}, e^{16} + e^{25}, e^{36} + e^{45} + e^{27}$                                             | $1/4(1, 2, 2, 3, 3, 4, 4, 5, 6)$                   | $\{\emptyset, 12569, 1458, 24689\}$                               |                    |
| 9642:161  | $0, 0, 0, -e^{12}, e^{13}, e^{14}, e^{24} + e^{15}, e^{26} + e^{17}, e^{36} + e^{27} + e^{45}$                                             | $7/33(1, 2, 3, 3, 4, 4, 5, 6, 7)$                  | $\{\emptyset, 12367, 13479, 2469\}$                               |                    |
| 9642:163a | $0, 0, 0, e^{12}, e^{13}, e^{14}a_1, e^{15}, e^{34} + e^{25} + e^{16}, e^{17} + e^{35} + e^{24}$                                           | $29/109(1, 2, 2, 3, 3, 4, 4, 5, 5)$                | $\{\emptyset, 12569, 14589, 2468\}$                               |                    |
| 9642:163b | $0, 0, 0, -e^{12}, e^{13}, e^{14}a_1, e^{15}, e^{34} + e^{16} - e^{25}, e^{35} + e^{24} + e^{17}$                                          | $29/109(1, 2, 2, 3, 3, 4, 4, 5, 5)$                | $\{\emptyset, 12569, 14589, 2468\}$                               |                    |
| 9642:167  | $0, 0, 0, -e^{12}, e^{13}, e^{14} + e^{23}, e^{24} + a_3e^{15}, e^{34} + e^{16}, e^{26} + e^{35} + e^{17}$                                 | $9/64(2, 3, 4, 5, 6, 7, 8, 9, 10)$                 | $\{\emptyset, 2468\}$                                             |                    |
| 9642:168  | $0, 0, 0, (-1 + a_2)e^{12}, a_2e^{13}, e^{14} + e^{23}, e^{15} + e^{24}, e^{25} + e^{16} + e^{34}, e^{26} + e^{17}$                        | $9/64(2, 3, 4, 5, 6, 7, 8, 9, 10)$                 | $\{\emptyset, 2468\}$                                             |                    |
| 9642:169  | $0, 0, 0, e^{12}a_1, e^{13}, e^{23} + e^{14}, e^{24} + e^{15}, e^{16} + e^{25}, e^{17} + e^{26} + e^{35}$                                  | $9/64(2, 3, 4, 5, 6, 7, 8, 9, 10)$                 | $\{\emptyset, 2468\}$                                             |                    |
| 9642:171  | $0, 0, 0, -e^{12}, e^{13}, e^{23} + e^{14}, e^{15} + e^{24}, e^{16} + e^{34}, e^{27} + e^{36} + e^{45}$                                    | $11/81(2, 3, 4, 5, 6, 7, 8, 9, 11)$                | $\{\emptyset, 24689\}$                                            |                    |
| 9642:172  | $0, 0, 0, -e^{12}, e^{13}, e^{14} + e^{23}, e^{15} + e^{24}, e^{16} + e^{25}, e^{45} + e^{36} + e^{27}$                                    | $11/81(2, 3, 4, 5, 6, 7, 8, 9, 11)$                | $\{\emptyset, 24689\}$                                            |                    |
| 9642:175a | $0, 0, 0, e^{12}, e^{13}, e^{34} + e^{25}, e^{35} + e^{24}, e^{37} + e^{26}, e^{36} + e^{27} + e^{14}$                                     | $14/53(2, 1, 1, 3, 3, 4, 4, 5, 5)$                 | $\{\emptyset, 234589, 2469, 3568\}$                               |                    |
| 9642:175b | $0, 0, 0, e^{12}, e^{13}, e^{34} + e^{25}, e^{35} - e^{24}, -e^{26} + e^{37}, e^{14} + e^{27} + e^{36}$                                    | $14/53(2, 1, 1, 3, 3, 4, 4, 5, 5)$                 | $\{\emptyset, 234589, 2469, 3568\}$                               |                    |
| 9642:176a | $0, 0, 0, e^{12}, e^{13}, e^{35} + e^{24}, e^{25} + e^{34}, e^{37} + e^{26}, e^{36} + e^{14} + e^{27}$                                     | $14/53(2, 1, 1, 3, 3, 4, 4, 5, 5)$                 | $\{\emptyset, 12569, 13468, 234589\}$                             |                    |
| 9642:176b | $0, 0, 0, -e^{12}, e^{13}, e^{24} + e^{35}, -e^{25} + e^{34}, e^{37} - e^{26}, e^{37} + e^{27} + e^{14}$                                   | $14/53(2, 1, 1, 3, 3, 4, 4, 5, 5)$                 | $\{\emptyset, 12569, 13468, 234589\}$                             |                    |
| 9642:177  | $0, 0, 0, -e^{12}, e^{13}, e^{14} + e^{23}, e^{15} + e^{24}, e^{17} + e^{26}, e^{27} + e^{45} + e^{36}$                                    | $7/53(2, 3, 4, 5, 6, 7, 8, 10, 11)$                | $\{\emptyset, 2469\}$                                             |                    |
| 9642:178a | $0, 0, 0, (-1 + a_2)e^{12}, a_2e^{13}, e^{14}, e^{15} + e^{23}, e^{35} + e^{16} + a_3e^{24}, e^{34} + e^{17} + e^{25}$                     | $29/109(1, 2, 2, 3, 3, 4, 4, 5, 5)$                | $\{\emptyset, 13478, 14589, 3579\}$                               |                    |
| 9642:178b | $0, 0, 0, (-1 + a_2)e^{12}, a_2e^{13}, -e^{14}, e^{15} + e^{23}, e^{16} + e^{35} + a_3e^{24}, e^{17} + e^{25} + e^{34}$                    | $29/109(1, 2, 2, 3, 3, 4, 4, 5, 5)$                | $\{\emptyset, 13478, 14589, 3579\}$                               |                    |
| 9642:182  | $0, 0, 0, e^{12}, e^{13}, e^{14}, e^{24} + a_3e^{15}, e^{16} + e^{34} + e^{25}, e^{17} + e^{35} + e^{26}$                                  | $9/64(2, 3, 4, 5, 6, 7, 8, 9, 10)$                 | $\{\emptyset, 2468\}$                                             |                    |
| 9642:183  | $0, 0, 0, e^{12}, e^{13}, e^{24}, e^{25} + e^{34}, a_2e^{14} + e^{35} + e^{26}, e^{36} + e^{15} + e^{27}$                                  | $1/8(4, 2, 3, 6, 7, 8, 9, 10, 11)$                 | $\{\emptyset, 3579\}$                                             |                    |
| 9642:184a | $0, 0, 0, -e^{12}a_1, e^{13}, e^{14}, e^{15}a_1 + e^{23}, e^{24} + e^{35} + e^{16}, e^{45} + e^{36} + e^{27}$                              | $1/4(1, 2, 2, 3, 3, 4, 4, 5, 6)$                   | $\{\emptyset, 134789, 1458, 3579\}$                               |                    |
| 9642:184b | $0, 0, 0, -e^{12}a_1, -e^{13}, -e^{14}, e^{15}a_1 + e^{23}, e^{16} + e^{24} + e^{35}, e^{45} + e^{27} + e^{36}$                            | $1/4(1, 2, 2, 3, 3, 4, 4, 5, 6)$                   | $\{\emptyset, 134789, 1458, 3579\}$                               |                    |
| 9642:186  | $0, 0, 0, -e^{12}, -e^{13}, -e^{14}, e^{15} + e^{24}, e^{16} + e^{25} + e^{34}, e^{27} + e^{36} + e^{45}$                                  | $11/81(2, 3, 4, 5, 6, 7, 8, 9, 11)$                | $\{\emptyset, 24689\}$                                            |                    |
| 9642:187a | $0, 0, 0, e^{12}, e^{13}, 2e^{14}, e^{25} + e^{34}, e^{16} + e^{24} + e^{35}, e^{45} + e^{17} + e^{36}$                                    | $31/129(1, 2, 2, 3, 3, 4, 4, 5, 6)$                | $\{\emptyset, 13489, 14578, 3579\}$                               |                    |
| 9642:187b | $0, 0, 0, -e^{12}, e^{13}, 2e^{14}, -e^{25} + e^{34}, e^{16} + e^{24} + e^{35}, e^{17} + e^{45} + e^{36}$                                  | $31/129(1, 2, 2, 3, 3, 4, 4, 5, 6)$                | $\{\emptyset, 13489, 14578, 3579\}$                               |                    |
| 9642:190  | $0, 0, 0, -e^{12}a_1, -(-1 + a_1)e^{13}, -(-1 + a_1)e^{14} + e^{23}, e^{15}a_1, e^{16} + e^{34} + e^{25}, e^{27} + e^{36} + e^{45}$        | $1/4(1, 2, 2, 3, 3, 4, 4, 5, 6)$                   | $\{\emptyset, 12569, 1458, 24689\}$                               |                    |
| 9642:192  | $0, 0, 0, -e^{12}, e^{13}, e^{14}, e^{24} + e^{15}, e^{35} + e^{17} + e^{26}, e^{36} + e^{45} + e^{27}$                                    | $7/53(2, 3, 4, 5, 6, 7, 8, 10, 11)$                | $\{\emptyset, 2469\}$                                             |                    |
| 9642:194  | $0, 0, 0, (-1 + a_2)e^{12}, a_2e^{13}, e^{14} + e^{23}, e^{15}a_4 + e^{24}, e^{25} + e^{34} + e^{16}, e^{26} + e^{35} + e^{17}$            | $9/64(2, 3, 4, 5, 6, 7, 8, 9, 10)$                 | $\{\emptyset, 2468\}$                                             |                    |
| 9642:197  | $0, 0, 0, (-1 + a_2)e^{12}, a_2e^{13}, a_2e^{14} + e^{23}, -(-1 + a_2)e^{15} + e^{24}, e^{34} + e^{25} + e^{16}, e^{27} + e^{45} + e^{36}$ | $11/81(2, 3, 4, 5, 6, 7, 8, 9, 11)$                | $\{\emptyset, 24689\}$                                            |                    |
| 9642:198a | $0, 0, 0, e^{12}, e^{13}, e^{34} + e^{25}, e^{35} + e^{24}, e^{14}a_1 + e^{27} + e^{36}, e^{26} + e^{15} + e^{37}$                         | $14/53(2, 1, 1, 3, 3, 4, 4, 5, 5)$                 | $\{\emptyset, 234589, 2468, 3569\}$                               |                    |
| 9642:198b | $0, 0, 0, -e^{12}, e^{13}, -e^{25} + e^{34}, e^{35} + e^{24}, e^{14}a_1 - e^{27} + e^{36}, e^{15} + e^{26} + e^{37}$                       | $14/53(2, 1, 1, 3, 3, 4, 4, 5, 5)$                 | $\{\emptyset, 234589, 2468, 3569\}$                               |                    |
| 9642:199a | $0, 0, 0, e^{12}, e^{13}, e^{25} + e^{34}, e^{24}a_4 + e^{35}, e^{26}a_4 + e^{14} + e^{37}, e^{15} + e^{36} + e^{27}$                      | $14/53(2, 1, 1, 3, 3, 4, 4, 5, 5)$                 | $\{\emptyset, 12578, 13479, 234589\}$                             |                    |
| 9642:199b | $0, 0, 0, e^{12}, e^{13}, e^{25} + e^{34}, e^{24}a_4 + e^{35}, e^{26}a_4 - e^{14} + e^{37}, e^{15} + e^{36} + e^{27}$                      | $14/53(2, 1, 1, 3, 3, 4, 4, 5, 5)$                 | $\{\emptyset, 12578, 13479, 234589\}$                             |                    |
| 9642:200  | $0, 0, 0, -e^{12}, e^{13}, e^{23}a_4 + e^{14}, e^{24} + e^{15}, e^{35} + e^{26} + e^{17}, e^{27} + e^{36} + e^{45}$                        | $7/53(2, 3, 4, 5, 6, 7, 8, 10, 11)$                | $\{\emptyset, 2469\}$                                             |                    |
| 96321:6   | $0, 0, 0, -e^{12}, e^{13}, e^{23}, e^{14}, e^{17}, e^{47} + e^{28}$                                                                        | $1/233(50, 94, 185, 144, 235, 279, 194, 244, 338)$ | $\{\emptyset, 12379, 125679, 134689, 14589, 234578, 24678, 356\}$ |                    |
| 96321:9   | $0, 0, 0, e^{12}, e^{13}, e^{23}, e^{14}, e^{17}, e^{18} + e^{25} + e^{34}$                                                                | $3/221(16, 39, 48, 55, 64, 87, 71, 87, 103)$       | $\{\emptyset, 12379, 13468, 246789\}$                             |                    |
| 96321:11a | $0, 0, 0, -e^{12}, e^{13}, e^{23}, e^{14}, e^{17}, e^{47} + e^{35} + e^{28}$                                                               | $2/131(13, 31, 44, 44, 57, 75, 57, 70, 101)$       | $\{\emptyset, 12379, 125679, 134689, 14589, 234578, 24678, 356\}$ |                    |
| 96321:11b | $0, 0, 0, -e^{12}, -e^{13}, e^{23}, e^{14}, e^{17}, e^{35} + e^{28} + e^{47}$                                                              | $2/131(13, 31, 44, 44, 57, 75, 57, 70, 101)$       | $\{\emptyset, 12379, 125679, 134689, 14589, 234578, 24678, 356\}$ |                    |
| 96321:17  | $0, 0, 0, e^{12}, e^{13}, e^{23}, e^{14}, e^{24} + e^{17}, e^{27} + e^{35} + e^{18}$                                                       | $21/173(2, 4, 5, 6, 7, 9, 8, 10, 12)$              | $\{\emptyset, 356\}$                                              |                    |
| 96321:19a | $0, 0, 0, -e^{12}, e^{13}, e^{23}, e^{14}, e^{17} + e^{24}, e^{28} + e^{35} + e^{47}$                                                      | $17/77(1, 2, 3, 3, 4, 5, 4, 5, 7)$                 | $\{\emptyset, 134689, 14589, 356\}$                               |                    |
| 96321:19b | $0, 0, 0, -e^{12}, -e^{13}, e^{23}, e^{14}, e^{17} + e^{24}, e^{47} + e^{28} + e^{35}$                                                     | $17/77(1, 2, 3, 3, 4, 5, 4, 5, 7)$                 | $\{\emptyset, 134689, 14589, 356\}$                               |                    |
| 96321:23  | $0, 0, 0, e^{12}, e^{13}, e^{23}, e^{24}, e^{27} + e^{15}, e^{47} + e^{18}$                                                                | $4/185(11, 15, 34, 26, 45, 49, 41, 56, 67)$        | $\{\emptyset, 125679, 134678, 234589\}$                           |                    |

Table A.4 – Continued to next page

Table A.4 – Continued from previous page

| Name      | g                                                                                                              | N                                                    | S <sub>0</sub>                                                    | S = S <sub>0</sub> |
|-----------|----------------------------------------------------------------------------------------------------------------|------------------------------------------------------|-------------------------------------------------------------------|--------------------|
| 96321:26a | $0, 0, 0, e^{12}, e^{13}, e^{23}, e^{24}, e^{27} + e^{15}, e^{18} + e^{36} + e^{47}$                           | $4/13(1, 1, 2, 2, 3, 3, 3, 4, 5)$                    | $\{\emptyset, 125679, 134678, 234589\}$                           |                    |
| 96321:26b | $0, 0, 0, e^{12}, e^{13}, -e^{23}, e^{24}, e^{15} + e^{27}, e^{18} + e^{47} + e^{36}$                          | $4/13(1, 1, 2, 2, 3, 3, 3, 4, 5)$                    | $\{\emptyset, 125679, 134678, 234589\}$                           |                    |
| 9653:2    | $0, 0, 0, e^{12}, e^{14}, e^{24}, e^{15}, e^{13} + e^{26}, e^{25} + e^{16}$                                    | $1/135(40, 43, 129, 83, 123, 126, 163, 169, 166)$    | $\{\emptyset, 12356, 14678, 234578\}$                             |                    |
| 9653:3    | $0, 0, 0, e^{12}, e^{14}, e^{24}, e^{15} + e^{23}, e^{13} + e^{26}, e^{25} + e^{16}$                           | $25/81(1, 1, 3, 2, 3, 3, 4, 4, 4)$                   | $\{\emptyset, 12356\}$                                            |                    |
| 9653:4    | $0, 0, 0, e^{12}, e^{14}, e^{13} + e^{24}, e^{15}, e^{26} + e^{34}, e^{16} + e^{25}$                           | $1/75(20, 27, 54, 47, 67, 74, 87, 101, 94)$          | $\{\emptyset, 1256, 14678, 24578\}$                               |                    |
| 9641:7    | $0, 0, 0, e^{12}, e^{13}, e^{14}, e^{35}, e^{25} + e^{34}, e^{16}$                                             | $5/49(2, 6, 5, 8, 7, 10, 12, 13, 12)$                | $\{\emptyset, 123678, 12567, 13479, 145789, 234569, 24689, 358\}$ |                    |
| 9641:8    | $0, 0, 0, e^{12}, e^{13}, e^{24}, e^{35}, e^{34} + e^{25}, e^{26}$                                             | $1/39(22, 9, 14, 31, 36, 40, 50, 45, 49)$            | $\{\emptyset, 123678, 12567, 134679, 1456789, 23459, 2489, 358\}$ |                    |
| 9641:14   | $0, 0, 0, e^{12}, e^{13}, e^{14}, e^{15}, e^{34} + e^{25}, e^{16}$                                             | $1/179(37, 104, 116, 141, 153, 178, 190, 257, 215)$  | $\{\emptyset, 123678, 1256, 13479, 14589, 2345679, 24689, 3578\}$ |                    |
| 9641:16   | $0, 0, 0, e^{12}, e^{13}, e^{24}, e^{15}, e^{25} + e^{34}, e^{26}$                                             | $2/39(7, 6, 11, 13, 18, 19, 25, 24, 25)$             | $\{\emptyset, 123678, 1256, 134679, 145689, 234579, 2489, 3578\}$ |                    |
| 9641:22   | $0, 0, 0, e^{12}, e^{13}, e^{14}, e^{24}, e^{25} + e^{34}, e^{16}$                                             | $1/225(58, 100, 153, 158, 211, 216, 258, 311, 274)$  | $\{\emptyset, 123678, 12567, 13479, 145789, 234569, 24689, 358\}$ |                    |
| 9641:23   | $0, 0, 0, e^{12}, e^{13}, e^{24}, e^{14}, e^{25} + e^{34}, e^{26}$                                             | $1/225(100, 58, 139, 158, 239, 216, 258, 297, 274)$  | $\{\emptyset, 123678, 12567, 13469, 145689, 234579, 24789, 358\}$ |                    |
| 9641:35a  | $0, 0, 0, e^{12}, e^{13}, e^{14}, e^{34} + e^{25}, e^{35} + e^{24}, e^{16}$                                    | $10/131(3, 7, 7, 10, 10, 13, 17, 17, 16)$            | $\{\emptyset, 123678, 12568, 13489, 145789, 234569, 24679, 357\}$ | ✓                  |
| 9641:35b  | $0, 0, 0, -e^{12}, e^{13}, e^{14}, -e^{25} + e^{34}, e^{35} + e^{24}, e^{16}$                                  | $10/131(3, 7, 7, 10, 10, 13, 17, 17, 16)$            | $\{\emptyset, 123678, 12568, 13489, 145789, 234569, 24679, 357\}$ | ✓                  |
| 9641:36   | $0, 0, 0, e^{12}, e^{13}, e^{24}, e^{35} + e^{14}, e^{25} + e^{34}, e^{26}$                                    | $1/75(40, 18, 29, 58, 69, 76, 98, 87, 94)$           | $\{\emptyset, 123678, 12567, 358\}$                               |                    |
| 9641:37   | $0, 0, 0, e^{12}, e^{13}, e^{14}, e^{15}, e^{34} + e^{25}, e^{35} + e^{16}$                                    | $1/58(14, 34, 31, 48, 45, 62, 59, 79, 76)$           | $\{\emptyset, 13479, 14589, 3578\}$                               |                    |
| 9641:38   | $0, 0, 0, e^{12}, e^{13}, e^{24}, e^{15}, e^{34} + e^{25}, e^{26} + e^{35}$                                    | $2/37(7, 6, 9, 13, 16, 19, 23, 22, 25)$              | $\{\emptyset, 134679, 145689, 3578\}$                             |                    |
| 9641:39   | $0, 0, 0, e^{12}, e^{13}, e^{24}, e^{35}, e^{25} + e^{34}, e^{15} + e^{26}$                                    | $1/501(239, 144, 193, 383, 432, 527, 625, 576, 671)$ | $\{\emptyset, 12567, 134679, 23459\}$                             |                    |
| 9641:43   | $0, 0, 0, e^{12}, e^{13}, e^{14}, e^{15}, e^{34} + e^{25}, e^{23} + e^{16}$                                    | $1/61(13, 35, 39, 48, 52, 61, 65, 87, 74)$           | $\{\emptyset, 123678, 13479, 24689\}$                             |                    |
| 9641:50   | $0, 0, 0, e^{12}, a_1 e^{13}, e^{14}, e^{35}, e^{23} + e^{15}, e^{24} + e^{16}$                                | $1/67(18, 36, 35, 54, 53, 72, 88, 71, 90)$           | $\{\emptyset, 134789, 14579, 358\}$                               |                    |
| 9641:52   | $0, 0, 0, e^{12}, e^{13}, e^{14}, e^{24} + e^{15}, e^{25} + e^{34}, e^{16}$                                    | $1/389(97, 179, 261, 276, 358, 373, 455, 537, 470)$  | $\{\emptyset, 123678, 13479, 24689\}$                             |                    |
| 9641:53   | $0, 0, 0, e^{12}, e^{13}, e^{14} + e^{23}, e^{24}, e^{35}, e^{25} + e^{16}$                                    | $3/92(8, 15, 16, 23, 24, 31, 38, 40, 39)$            | $\{\emptyset, 125678, 145789, 2469\}$                             |                    |
| 9641:55   | $0, 0, 0, e^{12}, e^{13}, e^{14}, e^{24}, e^{25} + e^{34}, e^{16} + e^{35}$                                    | $1/225(67, 100, 117, 167, 184, 234, 267, 284, 301)$  | $\{\emptyset, 13479, 145789, 358\}$                               |                    |
| 9641:56   | $0, 0, 0, e^{12}, e^{13}, e^{24}, e^{14}, e^{25} + e^{34}, e^{26} + e^{35}$                                    | $1/19(8, 6, 9, 14, 17, 20, 22, 23, 26)$              | $\{\emptyset, 13469, 145689, 358\}$                               |                    |
| 9641:57   | $0, 0, 0, e^{12}, e^{13}, e^{14}, e^{35}, e^{25} + e^{34}, e^{16} + e^{24}$                                    | $5/213(11, 22, 21, 33, 32, 44, 53, 54, 55)$          | $\{\emptyset, 13479, 145789, 358\}$                               |                    |
| 9641:58   | $0, 0, 0, e^{12}, e^{13}, e^{24}, e^{35}, e^{34} + e^{25}, e^{14} + e^{26}$                                    | $1/423(218, 109, 162, 327, 380, 436, 542, 489, 545)$ | $\{\emptyset, 23459, 2489, 358\}$                                 |                    |
| 9641:59   | $0, 0, 0, -e^{12}, e^{13}, e^{23} + e^{14}, e^{24}, e^{35}, e^{16} + e^{34}$                                   | $3/92(8, 15, 16, 23, 24, 31, 38, 40, 39)$            | $\{\emptyset, 125678, 145789, 2469\}$                             |                    |
| 9641:63   | $0, 0, 0, e^{12}, e^{13}, e^{14} + e^{23}, e^{24}, e^{15}, e^{25} + e^{16}$                                    | $1/148(44, 67, 88, 111, 132, 155, 178, 176, 199)$    | $\{\emptyset, 12567, 14579, 2469\}$                               |                    |
| 9641:64   | $0, 0, 0, e^{12}, e^{13}, e^{24}, e^{14}, e^{34} + e^{25}, e^{26} + e^{15}$                                    | $1/425(160, 137, 251, 297, 411, 434, 457, 548, 571)$ | $\{\emptyset, 12567, 13469, 234579\}$                             |                    |
| 9641:65   | $0, 0, 0, e^{12}, e^{13}, e^{14}, e^{15}, e^{25} + e^{34}, e^{24} + e^{16}$                                    | $1/8(2, 4, 5, 6, 7, 8, 9, 11, 10)$                   | $\{\emptyset, 13479, 14589, 3578\}$                               |                    |
| 9641:67   | $0, 0, 0, -e^{12}, e^{13}, e^{14} + e^{23}, e^{24}, e^{15}, e^{16} + e^{34}$                                   | $1/148(44, 67, 88, 111, 132, 155, 178, 176, 199)$    | $\{\emptyset, 12567, 14579, 2469\}$                               |                    |
| 9641:68   | $0, 0, 0, e^{12}, e^{13}, e^{14}, e^{24}, e^{35}, e^{16} + e^{34} + e^{25}$                                    | $3/92(8, 15, 16, 23, 24, 31, 38, 40, 39)$            | $\{\emptyset, 125678, 145789, 2469\}$                             |                    |
| 9641:72a  | $0, 0, 0, e^{12}, e^{13}, e^{23} + e^{14}, e^{15}, e^{35} + e^{24}, e^{16} + e^{25}$                           | $29/109(1, 2, 2, 3, 3, 4, 4, 5, 5)$                  | $\{\emptyset, 12568, 14589, 2469\}$                               |                    |
| 9641:72b  | $0, 0, 0, -e^{12}, e^{13}, e^{14} + e^{23}, e^{15}, e^{24} + e^{35}, e^{25} + e^{16}$                          | $29/109(1, 2, 2, 3, 3, 4, 4, 5, 5)$                  | $\{\emptyset, 12568, 14589, 2469\}$                               |                    |
| 9641:77a  | $0, 0, 0, -e^{12}, e^{13}, e^{14} + e^{23}, e^{15}, e^{24} + e^{35}, e^{16} + e^{34}$                          | $29/109(1, 2, 2, 3, 3, 4, 4, 5, 5)$                  | $\{\emptyset, 12568, 14589, 2469\}$                               |                    |
| 9641:77b  | $0, 0, 0, -e^{12}, -e^{13}, e^{14} + e^{23}, e^{15}, e^{35} + e^{24}, e^{16} + e^{34}$                         | $29/109(1, 2, 2, 3, 3, 4, 4, 5, 5)$                  | $\{\emptyset, 12568, 14589, 2469\}$                               |                    |
| 9641:79   | $0, 0, 0, e^{12}, e^{13}, e^{14}, e^{24}, e^{15}, e^{25} + e^{34} + e^{16}$                                    | $1/148(44, 67, 88, 111, 132, 155, 178, 176, 199)$    | $\{\emptyset, 12567, 14579, 2469\}$                               |                    |
| 9641:82   | $0, 0, 0, a_2 e^{12}, a_2 e^{13}, e^{14}, e^{15} + e^{23}, e^{25} + e^{34}, e^{16} + e^{24}$                   | $1/8(2, 4, 5, 6, 7, 8, 9, 11, 10)$                   | $\{\emptyset, 13479, 14589, 3578\}$                               |                    |
| 9641:84a  | $0, 0, 0, e^{12}, e^{13}, e^{14}, e^{15}, e^{35} + e^{24}, e^{34} + e^{25} + e^{16}$                           | $29/109(1, 2, 2, 3, 3, 4, 4, 5, 5)$                  | $\{\emptyset, 12568, 14589, 2469\}$                               | ✓                  |
| 9641:84b  | $0, 0, 0, e^{12}, e^{13}, e^{14}, e^{15}, e^{35} - e^{24}, e^{16} + e^{25} + e^{34}$                           | $29/109(1, 2, 2, 3, 3, 4, 4, 5, 5)$                  | $\{\emptyset, 12568, 14589, 2469\}$                               | ✓                  |
| 9641:85a  | $0, 0, 0, e^{12}, e^{13}, e^{14}, e^{15}, e^{25} + e^{34}, e^{24} + e^{35} + e^{16}$                           | $29/109(1, 2, 2, 3, 3, 4, 4, 5, 5)$                  | $\{\emptyset, 13479, 14589, 3578\}$                               | ✓                  |
| 9641:85b  | $0, 0, 0, -e^{12}, e^{13}, e^{14}, e^{15}, e^{34} - e^{25}, e^{35} + e^{16} + e^{24}$                          | $29/109(1, 2, 2, 3, 3, 4, 4, 5, 5)$                  | $\{\emptyset, 13479, 14589, 3578\}$                               | ✓                  |
| 9641:88   | $0, 0, 0, (-1 + a_2) e^{12}, a_2 e^{13}, e^{14} + e^{23}, e^{24}, e^{35}, e^{16} + e^{25} + e^{34}$            | $3/92(8, 15, 16, 23, 24, 31, 38, 40, 39)$            | $\{\emptyset, 125678, 145789, 2469\}$                             |                    |
| 9641:90   | $0, 0, 0, (-1 + a_2) e^{12}, a_2 e^{13}, e^{23} + e^{14}, e^{24}, e^{15}, e^{34} + e^{25} + e^{16}$            | $1/148(44, 67, 88, 111, 132, 155, 178, 176, 199)$    | $\{\emptyset, 12567, 14579, 2469\}$                               |                    |
| 9641:91   | $0, 0, 0, e^{12}, e^{13}, e^{14}, e^{23} + e^{15}, a_2 e^{24} + e^{35}, e^{16} + e^{25} + e^{34}$              | $29/109(1, 2, 2, 3, 3, 4, 4, 5, 5)$                  | $\{\emptyset, 14589\}$                                            |                    |
| 9641:92a  | $0, 0, 0, e^{12}, a_1 e^{13}, e^{14}, e^{15} + e^{23}, e^{34} + \frac{e^{25}}{a_1}, e^{24} + e^{35} + e^{16}$  | $29/109(1, 2, 2, 3, 3, 4, 4, 5, 5)$                  | $\{\emptyset, 13479, 14589, 3578\}$                               |                    |
| 9641:92b  | $0, 0, 0, -e^{12}, a_1 e^{13}, e^{14}, e^{15} + e^{23}, e^{34} - \frac{e^{25}}{a_1}, e^{16} + e^{24} + e^{35}$ | $29/109(1, 2, 2, 3, 3, 4, 4, 5, 5)$                  | $\{\emptyset, 13479, 14589, 3578\}$                               |                    |

Table A.4 – Continued to next page

Table A.4 – Continued from previous page

| Name      | $g$                                                                                                            | $N$                                                | $S_0$                                                             | $S = S_0$ |
|-----------|----------------------------------------------------------------------------------------------------------------|----------------------------------------------------|-------------------------------------------------------------------|-----------|
| 9641:94a  | $0, 0, 0, a_1 e^{12}, (1 + a_1) e^{13}, e^{14} + e^{23}, e^{15}, e^{24} + e^{35}, e^{16} + e^{25} + e^{34}$    | $29/109(1, 2, 2, 3, 3, 4, 4, 5, 5)$                | $\{\emptyset, 12568, 14589, 2469\}$                               |           |
| 9641:94b  | $0, 0, 0, a_1 e^{12}, (1 + a_1) e^{13}, e^{14} + e^{23}, e^{15}, e^{35} - e^{24}, e^{34} + e^{25} + e^{16}$    | $29/109(1, 2, 2, 3, 3, 4, 4, 5, 5)$                | $\{\emptyset, 12568, 14589, 2469\}$                               |           |
| 9641:97   | $0, 0, 0, e^{12}, e^{13}, e^{14}, e^{24}, e^{35}, e^{17} + e^{26}$                                             | $1/39(12, 15, 20, 27, 32, 39, 42, 52, 54)$         | $\{\emptyset, 123678, 125678, 13478, 14578, 23456, 246, 35\}$     |           |
| 9641:99   | $0, 0, 0, e^{12}, e^{13}, e^{14}, e^{24}, e^{15}, e^{26} + e^{17}$                                             | $1/31(7, 14, 24, 21, 31, 28, 35, 38, 42)$          | $\{\emptyset, 123678, 12567, 13478, 1457, 234568, 246, 358\}$     |           |
| 9641:105  | $0, 0, 0, e^{12}, e^{13}, e^{14}, e^{24}, e^{15}, e^{17} + e^{26} + e^{35}$                                    | $1/29(8, 13, 17, 21, 25, 29, 34, 33, 42)$          | $\{\emptyset, 234568, 246, 358\}$                                 |           |
| 9641:106a | $0, 0, 0, e^{12}, e^{13}, e^{14}, e^{24}, e^{25} + e^{34}, e^{27} + e^{16}$                                    | $1/3(1, 1, 2, 2, 3, 3, 3, 4, 4)$                   | $\{\emptyset, 123678, 12567, 13479, 145789, 234569, 24689, 358\}$ |           |
| 9641:106b | $0, 0, 0, e^{12}, e^{13}, -e^{14}, e^{24}, e^{34} + e^{25}, e^{16} + e^{27}$                                   | $1/3(1, 1, 2, 2, 3, 3, 3, 4, 4)$                   | $\{\emptyset, 123678, 12567, 13479, 145789, 234569, 24689, 358\}$ |           |
| 9641:107  | $0, 0, 0, e^{12}, e^{13}, e^{14}, e^{24}, e^{25} + e^{34}, e^{17} + e^{26}$                                    | $1/3(1, 1, 2, 2, 3, 3, 3, 4, 4)$                   | $\{\emptyset, 123678, 12567, 1347, 14578, 23456, 2468, 358\}$     |           |
| 9641:110  | $0, 0, 0, e^{12}, e^{13}, e^{24}, e^{14} + e^{23}, e^{15}, e^{16} + e^{27} + e^{35}$                           | $53/367(2, 3, 4, 5, 6, 8, 7, 8, 10)$               | $\{\emptyset, 247\}$                                              |           |
| 9641:112a | $0, 0, 0, e^{12}, e^{13}, e^{14}, e^{24}, e^{25} + e^{34}, e^{27} + e^{16} + e^{35}$                           | $43/243(2, 2, 3, 4, 5, 6, 6, 7, 8)$                | $\{\emptyset, 13479, 145789, 358\}$                               |           |
| 9641:112b | $0, 0, 0, e^{12}, e^{13}, -e^{14}, e^{24}, e^{25} + e^{34}, e^{16} + e^{27} + e^{35}$                          | $43/243(2, 2, 3, 4, 5, 6, 6, 7, 8)$                | $\{\emptyset, 13479, 145789, 358\}$                               |           |
| 9641:113  | $0, 0, 0, e^{12}, e^{13}, e^{14}, e^{24}, e^{25} + e^{34}, e^{17} + e^{26} + e^{35}$                           | $1/41(14, 15, 22, 29, 36, 43, 44, 51, 58)$         | $\{\emptyset, 23456, 2468, 358\}$                                 |           |
| 9641:144  | $0, 0, 0, e^{12}, e^{13}, e^{24}, e^{15}, e^{25} + e^{34}, e^{17} + e^{26}$                                    | $20/531(7, 10, 16, 17, 23, 27, 30, 33, 37)$        | $\{\emptyset, 123678, 125689, 13468, 145689, 234579\}$            |           |
| 9641:145  | $0, 0, 0, e^{12}, e^{13}, e^{24}, e^{35}, e^{25} + e^{34}, e^{37} + e^{26}$                                    | $1/27(16, 7, 7, 23, 23, 30, 30, 30, 37)$           | $\{\emptyset, 123678, 1456789, 23459\}$                           |           |
| 9641:146  | $0, 0, 0, e^{12}, e^{13}, e^{24}, e^{25} + e^{34}, e^{14}, e^{27} + e^{36}$                                    | $4/17(2, 1, 2, 3, 4, 4, 5, 5, 6)$                  | $\{\emptyset, 123678, 125689, 1346, 145679, 234589, 2478, 3579\}$ |           |
| 9641:147  | $0, 0, 0, e^{12}, e^{13}, e^{14}, e^{24} + e^{15}, e^{35}, e^{26} + e^{17}$                                    | $5/223(13, 18, 23, 31, 36, 44, 49, 59, 62)$        | $\{\emptyset, 123678, 13478, 246\}$                               |           |
| 9641:148  | $0, 0, 0, e^{12}, e^{13}, e^{24}, e^{25} + e^{34}, e^{15}, e^{36} + e^{27}$                                    | $1/185(78, 55, 74, 133, 152, 188, 207, 230, 262)$  | $\{\emptyset, 123678, 12569, 13468, 145679, 234589, 247, 35789\}$ |           |
| 9641:149  | $0, 0, 0, e^{12}, e^{13}, e^{24}, e^{25} + e^{34}, e^{35}, e^{36} + e^{27}$                                    | $1/17(10, 4, 5, 14, 15, 18, 19, 20, 23)$           | $\{\emptyset, 123678, 125689, 13468, 1456789, 23459, 247, 3579\}$ |           |
| 9641:152  | $0, 0, 0, -e^{12}, e^{13}, e^{14}, e^{15}, e^{24}, e^{45} + e^{27} + e^{36}$                                   | $2/17(2, 4, 5, 6, 7, 8, 9, 10, 13)$                | $\{\emptyset, 123678, 125689, 134789, 1458, 234567, 2469, 3579\}$ |           |
| 9641:155  | $0, 0, 0, e^{12}, e^{13}, e^{14}, e^{15} + e^{24}, e^{25} + e^{34}, e^{17} + e^{26}$                           | $2/41(5, 9, 13, 14, 18, 19, 23, 27, 28)$           | $\{\emptyset, 123678, 1347, 2468\}$                               |           |
| 9641:156  | $0, 0, 0, e^{12}, e^{13}, e^{24}, e^{34} + e^{25}, e^{35} + e^{14}, e^{36} + e^{27}$                           | $1/8(4, 2, 3, 6, 7, 8, 9, 10, 11)$                 | $\{\emptyset, 123678, 125689, 3579\}$                             |           |
| 9641:158a | $0, 0, 0, e^{12}, e^{13}, e^{25} + e^{34}, e^{35} + e^{24}, e^{14}, e^{37} + e^{26}$                           | $4/99(11, 8, 8, 19, 19, 27, 27, 30, 35)$           | $\{\emptyset, 123678, 125789, 1347, 145679, 234589, 2468, 3569\}$ |           |
| 9641:158b | $0, 0, 0, -e^{12}, e^{13}, -e^{25} + e^{34}, e^{24} + e^{35}, e^{14}, e^{37} + e^{26}$                         | $4/99(11, 8, 8, 19, 19, 27, 27, 30, 35)$           | $\{\emptyset, 123678, 125789, 1347, 145679, 234589, 2468, 3569\}$ |           |
| 9641:159a | $0, 0, 0, e^{12}, e^{13}, e^{35} + e^{24}, e^{34} + e^{25}, e^{14}, e^{37} + e^{26}$                           | $4/99(11, 8, 8, 19, 19, 27, 27, 30, 35)$           | $\{\emptyset, 123678, 12568, 13469, 145679, 234589, 24789, 357\}$ |           |
| 9641:159b | $0, 0, 0, e^{12}, e^{13}, e^{35} - e^{24}, e^{34} + e^{25}, e^{14}, e^{26} + e^{37}$                           | $4/99(11, 8, 8, 19, 19, 27, 27, 30, 35)$           | $\{\emptyset, 123678, 12568, 13469, 145679, 234589, 24789, 357\}$ |           |
| 9641:162  | $0, 0, 0, e^{12}, e^{13}, e^{14}, e^{35}, e^{25} + e^{34}, e^{16} + e^{24} + e^{37}$                           | $8/85(3, 6, 4, 9, 7, 12, 11, 13, 15)$              | $\{\emptyset, 145789\}$                                           |           |
| 9641:163  | $0, 0, 0, e^{12}, e^{13}, e^{24}, e^{35}, e^{34} + e^{25}, e^{37} + e^{14} + e^{26}$                           | $27/97(2, 1, 1, 3, 3, 4, 4, 4, 5)$                 | $\{\emptyset, 23459\}$                                            |           |
| 9641:166a | $0, 0, 0, -e^{12}, e^{13}, e^{14}, e^{15}, e^{24} + e^{35}, e^{45} + e^{36} + e^{27}$                          | $1/4(1, 2, 2, 3, 3, 4, 4, 5, 6)$                   | $\{\emptyset, 123678, 125689, 134789, 1458, 234567, 2469, 3579\}$ |           |
| 9641:166b | $0, 0, 0, -e^{12}, -e^{13}, -e^{14}, e^{15}, e^{24} + e^{35}, e^{45} + e^{27} + e^{36}$                        | $1/4(1, 2, 2, 3, 3, 4, 4, 5, 6)$                   | $\{\emptyset, 123678, 125689, 134789, 1458, 234567, 2469, 3579\}$ |           |
| 9641:167  | $0, 0, 0, -e^{12}, -e^{13}, -e^{14}, e^{15}, e^{34} + e^{25}, e^{27} + e^{36} + e^{45}$                        | $1/4(1, 2, 2, 3, 3, 4, 4, 5, 6)$                   | $\{\emptyset, 123678, 12569, 13479, 1458, 234567, 24689, 35789\}$ |           |
| 9641:170  | $0, 0, 0, e^{12}, e^{13}, e^{24}, e^{25} + e^{34}, e^{35}, e^{27} + e^{14} + e^{36}$                           | $1/309(173, 77, 96, 250, 269, 327, 346, 365, 423)$ | $\{\emptyset, 125689, 13468, 23459\}$                             |           |
| 9641:171  | $0, 0, 0, e^{12}, e^{13}, e^{24}, e^{34} + e^{25}, e^{35}, e^{27} + e^{36} + e^{15}$                           | $3/67(12, 6, 7, 18, 19, 24, 25, 26, 31)$           | $\{\emptyset, 23459, 247, 3579\}$                                 |           |
| 9641:173  | $0, 0, 0, -e^{12}, e^{13}, e^{14} + e^{23}, e^{15}, e^{24}, e^{36} + e^{27} + e^{45}$                          | $6/67(3, 5, 6, 8, 9, 11, 12, 13, 17)$              | $\{\emptyset, 125689, 1458, 2469\}$                               |           |
| 9641:175  | $0, 0, 0, e^{12}, e^{13}, 2e^{14}, e^{34} + e^{25}, e^{24}, e^{17} + e^{45} + e^{36}$                          | $1/72(20, 30, 37, 50, 57, 70, 87, 80, 107)$        | $\{\emptyset, 123678, 125689, 13489, 14578, 23456, 24679, 3579\}$ |           |
| 9641:176  | $0, 0, 0, -e^{12}, e^{13}, e^{14}, e^{15} + e^{24}, e^{35}, e^{27} + e^{36} + e^{45}$                          | $2/99(16, 19, 22, 35, 38, 51, 54, 60, 73)$         | $\{\emptyset, 123678, 134789, 2469\}$                             |           |
| 9641:180  | $0, 0, 0, e^{12}, e^{13}, 2e^{14}, e^{25} + e^{34}, e^{35}, e^{17} + e^{36} + e^{45}$                          | $1/72(18, 38, 31, 56, 49, 74, 87, 80, 105)$        | $\{\emptyset, 123678, 125689, 13489, 14578, 23456, 24679, 3579\}$ |           |
| 9641:181  | $0, 0, 0, e^{12}, e^{13}, e^{14} + e^{23}, e^{15} + e^{24}, e^{34} + e^{25}, e^{17} + e^{26}$                  | $9/64(2, 3, 4, 5, 6, 7, 8, 9, 10)$                 | $\{\emptyset, 2468\}$                                             |           |
| 9641:187  | $0, 0, 0, e^{12}, e^{13}, e^{14}, e^{15} + e^{24}, e^{34} + e^{25}, e^{35} + e^{17} + e^{26}$                  | $9/64(2, 3, 4, 5, 6, 7, 8, 9, 10)$                 | $\{\emptyset, 2468\}$                                             |           |
| 9641:194  | $0, 0, 0, -e^{12}, -e^{13}, -e^{14}, e^{15} + e^{24}, e^{25} + e^{34}, e^{27} + e^{36} + e^{45}$               | $5/87(5, 7, 9, 12, 14, 17, 19, 21, 26)$            | $\{\emptyset, 123678, 13479, 24689\}$                             |           |
| 9641:197a | $0, 0, 0, e^{12}, e^{13}, 2e^{14}, e^{34} + e^{25}, e^{35} + e^{24}, e^{45} + e^{36} + e^{17}$                 | $1/11(3, 5, 5, 8, 8, 11, 13, 13, 16)$              | $\{\emptyset, 123678, 125689, 13489, 14578, 23456, 24679, 3579\}$ |           |
| 9641:197b | $0, 0, 0, -e^{12}, e^{13}, 2e^{14}, e^{34} - e^{25}, e^{35} + e^{24}, e^{17} + e^{36} + e^{45}$                | $1/11(3, 5, 5, 8, 8, 11, 13, 13, 16)$              | $\{\emptyset, 123678, 125689, 13489, 14578, 23456, 24679, 3579\}$ |           |
| 9641:205  | $0, 0, 0, e^{12}, e^{13}, e^{35} + 2e^{14}, e^{25} + e^{34}, e^{24}, e^{36} + e^{17} + e^{45}$                 | $1/24(8, 10, 9, 18, 17, 26, 27, 28, 35)$           | $\{\emptyset, 123678, 125689, 3579\}$                             |           |
| 9641:206  | $0, 0, 0, a_1 e^{12}, a_1 e^{13}, e^{14} + e^{23}, e^{15} + e^{24}, e^{34} + e^{25}, e^{17} + e^{35} + e^{26}$ | $9/64(2, 3, 4, 5, 6, 7, 8, 9, 10)$                 | $\{\emptyset, 2468\}$                                             |           |
| 9641:214  | $0, 0, 0, e^{12}, e^{13}, -e^{15} + e^{24}, e^{14} + e^{35}, e^{25} + e^{34}, e^{37} + e^{26} + e^{45}$        | $10/27(1, 1, 1, 2, 2, 3, 3, 3, 4)$                 | $\{\emptyset, 123678\}$                                           |           |
| 9641:216  | $0, 0, 0, e^{12}, e^{13}, e^{14}, e^{24}, e^{35}, e^{38} + e^{17} + e^{26}$                                    | $1/93(33, 36, 35, 69, 68, 102, 105, 103, 138)$     | $\{\emptyset, 123678, 13478, 246\}$                               |           |
| 9641:218  | $0, 0, 0, e^{12}, e^{13}, e^{14}, e^{24}, e^{25} + e^{34}, e^{37} + e^{16} + e^{28}$                           | $4/371(37, 26, 48, 63, 85, 100, 89, 111, 137)$     | $\{\emptyset, 123678, 145789, 234569\}$                           |           |
| 9641:219a | $0, 0, 0, e^{12}, e^{13}, e^{14}, e^{15}, e^{24} + e^{35}, e^{37} + e^{26} + e^{18}$                           | $1/4(1, 2, 2, 3, 3, 4, 4, 5, 6)$                   | $\{\emptyset, 123678, 12568, 13478, 1458, 234567, 246, 357\}$     |           |

Table A.4 – Continued to next page



Table A.4 – Continued from previous page

| Name      | g                                                                                                                                              | N                                                    | S <sub>0</sub>                                                    | S = S <sub>0</sub> |
|-----------|------------------------------------------------------------------------------------------------------------------------------------------------|------------------------------------------------------|-------------------------------------------------------------------|--------------------|
| 9641:219b | $0, 0, 0, -e^{12}, e^{13}, e^{14}, e^{15}, e^{35} + e^{24}, e^{18} + e^{37} + e^{26}$                                                          | $1/4(1, 2, 2, 3, 3, 4, 4, 5, 6)$                     | $\{\emptyset, 123678, 12568, 13478, 1458, 234567, 246, 357\}$     |                    |
| 9641:220  | $0, 0, 0, e^{12}, e^{13}, e^{14}, e^{15}, e^{34} + e^{25}, e^{27} + e^{36} + e^{18}$                                                           | $1/4(1, 2, 2, 3, 3, 4, 4, 5, 6)$                     | $\{\emptyset, 123678, 12569, 13479, 1458, 234567, 24689, 35789\}$ |                    |
| 9641:222a | $0, 0, 0, e^{12}, e^{13}, e^{24}, e^{15}, e^{25} + e^{34}, e^{17} + e^{28} + e^{36}$                                                           | $5/101(7, 7, 9, 14, 16, 21, 23, 23, 30)$             | $\{\emptyset, 123678, 12569, 13467, 145689, 234579, 248, 35789\}$ |                    |
| 9641:222b | $0, 0, 0, e^{12}, e^{13}, e^{24}, -e^{15}, e^{34} + e^{25}, e^{17} + e^{28} + e^{36}$                                                          | $5/101(7, 7, 9, 14, 16, 21, 23, 23, 30)$             | $\{\emptyset, 123678, 12569, 13467, 145689, 234579, 248, 35789\}$ |                    |
| 9641:226  | $0, 0, 0, e^{12}, e^{13}, e^{14}, e^{15} + e^{24}, e^{25} + e^{34}, e^{36} + e^{18} + e^{27}$                                                  | $5/87(5, 7, 9, 12, 14, 17, 19, 21, 26)$              | $\{\emptyset, 123678, 13479, 24689\}$                             |                    |
| 9641:227a | $0, 0, 0, e^{12}, e^{13}, e^{14}, e^{25} + e^{34}, e^{24} + e^{35}, e^{27} + e^{16} + e^{38}$                                                  | $10/27(1, 1, 1, 2, 2, 3, 3, 3, 4)$                   | $\{\emptyset, 123678, 145789, 234569\}$                           |                    |
| 9641:227b | $0, 0, 0, -e^{12}, e^{13}, e^{14}, e^{34} - e^{25}, e^{35} + e^{24}, e^{38} + e^{27} + e^{16}$                                                 | $10/27(1, 1, 1, 2, 2, 3, 3, 3, 4)$                   | $\{\emptyset, 123678, 145789, 234569\}$                           |                    |
| 9641:228a | $0, 0, 0, e^{12}, e^{13}, e^{14}, e^{25} + e^{34}, e^{35} + e^{24}, e^{37} + e^{16} + e^{28}$                                                  | $10/27(1, 1, 1, 2, 2, 3, 3, 3, 4)$                   | $\{\emptyset, 123678, 12568, 13489, 145789, 234569, 24679, 357\}$ |                    |
| 9641:228b | $0, 0, 0, e^{12}, e^{13}, e^{14}, e^{25} + e^{34}, -e^{24} + e^{35}, e^{37} + e^{16} + e^{28}$                                                 | $10/27(1, 1, 1, 2, 2, 3, 3, 3, 4)$                   | $\{\emptyset, 123678, 12568, 13489, 145789, 234569, 24679, 357\}$ |                    |
| 9641:228c | $0, 0, 0, e^{12}, e^{13}, -e^{14}, e^{34} + e^{25}, e^{35} + e^{24}, e^{28} + e^{37} + e^{16}$                                                 | $10/27(1, 1, 1, 2, 2, 3, 3, 3, 4)$                   | $\{\emptyset, 123678, 12568, 13489, 145789, 234569, 24679, 357\}$ |                    |
| 9641:228d | $0, 0, 0, e^{12}, e^{13}, -e^{14}, e^{34} + e^{25}, e^{35} - e^{24}, e^{28} + e^{37} + e^{16}$                                                 | $10/27(1, 1, 1, 2, 2, 3, 3, 3, 4)$                   | $\{\emptyset, 123678, 12568, 13489, 145789, 234569, 24679, 357\}$ |                    |
| 9641:229  | $0, 0, 0, e^{12}, e^{13}, e^{24}, e^{35} + e^{14}, e^{25} + e^{34}, e^{27} + e^{16} + e^{38}$                                                  | $1/19(8, 6, 7, 14, 15, 20, 22, 21, 28)$              | $\{\emptyset, 123678, 12567, 358\}$                               |                    |
| 9641:230  | $0, 0, 0, e^{12}, e^{13}, 2e^{14}, e^{24}, e^{25} + e^{34}, e^{36} + e^{18} + e^{27} + e^{45}$                                                 | $5/87(5, 7, 9, 12, 14, 17, 19, 21, 26)$              | $\{\emptyset, 123678, 13479, 24689\}$                             |                    |
| 9641:231  | $0, 0, 0, e^{12}(-1 + a_3), e^{13}(-1 + a_3),$<br>$e^{14}a_3, -(-2 + a_3)e^{15}, e^{34} + e^{25}, e^{45} + e^{36} + e^{18} + e^{27}$           | $1/4(1, 2, 2, 3, 3, 4, 4, 5, 6)$                     | $\{\emptyset, 123678, 12569, 13479, 1458, 234567, 24689, 35789\}$ |                    |
| 9641:234  | $0, 0, 0, e^{12}, e^{13}, e^{24} + e^{15}, e^{35} + e^{14}, e^{25} + e^{34}, e^{38} + e^{27} + e^{16}$                                         | $10/27(1, 1, 1, 2, 2, 3, 3, 3, 4)$                   | $\{\emptyset, 123678\}$                                           |                    |
| 9641:235  | $0, 0, 0, e^{12}, e^{13}, e^{24} + e^{15}, e^{35} + e^{14}, e^{25} + e^{34}, e^{18} + e^{37} + e^{26}$                                         | $10/27(1, 1, 1, 2, 2, 3, 3, 3, 4)$                   | $\{\emptyset, 123678\}$                                           |                    |
| 9641:238  | $0, 0, 0, e^{12}(-1 + a_3), e^{13}(-1 + a_3),$<br>$e^{14}a_3, -(-2 + a_3)e^{15} + e^{24}, e^{25} + e^{34}, e^{27} + e^{18} + e^{36} + e^{45}$  | $5/87(5, 7, 9, 12, 14, 17, 19, 21, 26)$              | $\{\emptyset, 123678, 13479, 24689\}$                             |                    |
| 9641:239  | $0, 0, 0, e^{12}, e^{13}, e^{24}, 2e^{14} + e^{35}, e^{25} + e^{34}, e^{45} + e^{37} + e^{18} + e^{26}$                                        | $10/27(1, 1, 1, 2, 2, 3, 3, 3, 4)$                   | $\{\emptyset, 123678\}$                                           |                    |
| 9641:241  | $0, 0, 0, a_2e^{12}, a_2e^{13},$<br>$-(-1 + a_2)e^{15} + e^{24}, e^{14}(1 + a_2) + e^{35}, e^{34} + e^{25}, e^{18} + e^{26} + e^{37} + e^{45}$ | $10/27(1, 1, 1, 2, 2, 3, 3, 3, 4)$                   | $\{\emptyset, 123678\}$                                           |                    |
| 9631:7    | $0, 0, 0, e^{12}, e^{13}, e^{23}, e^{14}, e^{25} + e^{34}, e^{17}$                                                                             | $1/8(2, 4, 5, 6, 7, 9, 8, 11, 10)$                   | $\{\emptyset, 12378, 12567, 13469, 14589, 234579, 246789, 3568\}$ |                    |
| 9631:27   | $0, 0, 0, e^{12}, e^{13}, e^{23}, e^{14}, e^{34} + e^{25}, e^{35} + e^{17}$                                                                    | $1/81(21, 44, 43, 65, 64, 87, 86, 108, 107)$         | $\{\emptyset, 13469, 14589, 3568\}$                               |                    |
| 9631:39   | $0, 0, 0, (-1 + a_2)e^{12}, e^{13}a_2, e^{23}, e^{14}, e^{34} + e^{25} + e^{16}, e^{17}$                                                       | $1/8(2, 4, 5, 6, 7, 9, 8, 11, 10)$                   | $\{\emptyset, 12378, 12567, 13469, 14589, 234579, 246789, 3568\}$ |                    |
| 9631:41   | $0, 0, 0, e^{12}, e^{13}, e^{23}, e^{14}, e^{16} + e^{25}, e^{17} + e^{35}$                                                                    | $1/81(21, 44, 43, 65, 64, 87, 86, 108, 107)$         | $\{\emptyset, 13469, 14589, 3568\}$                               |                    |
| 9631:43   | $0, 0, 0, e^{12}, e^{13}, e^{23}, e^{24}, e^{16} + e^{25}, e^{35} + e^{27}$                                                                    | $3/92(14, 10, 15, 24, 29, 25, 34, 39, 44)$           | $\{\emptyset, 134679, 145789, 3568\}$                             |                    |
| 9631:45   | $0, 0, 0, e^{12}, e^{13}, e^{23}, e^{14}, e^{35}, e^{25} + e^{34} + e^{17}$                                                                    | $1/221(55, 133, 110, 188, 165, 243, 243, 275, 298)$  | $\{\emptyset, 125678, 14589, 24679\}$                             |                    |
| 9631:48   | $0, 0, 0, e^{12}, e^{13}, e^{23}, e^{14}, e^{25} + e^{34}, e^{17} + e^{36}$                                                                    | $3/92(10, 14, 15, 24, 25, 29, 34, 39, 44)$           | $\{\emptyset, 234579, 246789, 3568\}$                             |                    |
| 9631:53   | $0, 0, 0, e^{12}, e^{13}, e^{23}, e^{14}, e^{15}, e^{17} + e^{25} + e^{34}$                                                                    | $1/88(25, 48, 50, 73, 75, 98, 98, 100, 123)$         | $\{\emptyset, 12567, 1459, 24679\}$                               |                    |
| 9631:60   | $0, 0, 0, e^{12}, e^{13}, e^{23}, e^{14}, e^{25} + e^{34}, e^{17} + e^{26}$                                                                    | $1/389(128, 151, 233, 279, 361, 384, 407, 512, 535)$ | $\{\emptyset, 12567, 13469, 234579\}$                             |                    |
| 9631:68   | $0, 0, 0, (-1 + a_2)e^{12}, e^{13}a_2, e^{23}, e^{14}, e^{34} + e^{25} + e^{16}, e^{17} + e^{35}$                                              | $1/81(21, 44, 43, 65, 64, 87, 86, 108, 107)$         | $\{\emptyset, 13469, 14589, 3568\}$                               |                    |
| 9631:69   | $0, 0, 0, (-1 + a_2)e^{12}, e^{13}a_2, e^{23}, e^{24}, e^{34} + e^{16} + e^{25}, e^{27} + e^{35}$                                              | $3/92(14, 10, 15, 24, 29, 25, 34, 39, 44)$           | $\{\emptyset, 134679, 145789, 3568\}$                             |                    |
| 9631:73   | $0, 0, 0, e^{12}, e^{13}, e^{23}, e^{14}, e^{24}, e^{17} + e^{25} + e^{34}$                                                                    | $1/197(65, 81, 130, 146, 195, 211, 211, 227, 276)$   | $\{\emptyset, 125678, 14589, 24679\}$                             |                    |
| 9631:78   | $0, 0, 0, e^{12}, e^{13}, e^{23}, e^{14}, e^{25} + e^{16}, e^{35} + e^{26} + e^{17}$                                                           | $71/657(3, 4, 5, 7, 8, 9, 10, 12, 13)$               | $\{\emptyset, 13469\}$                                            |                    |
| 9631:80   | $0, 0, 0, (-1 + a_2)e^{12}, e^{13}a_2, e^{23}, e^{24}, e^{16} + e^{25} + e^{34}, e^{15} + e^{27}$                                              | $1/389(151, 128, 233, 279, 384, 361, 407, 512, 535)$ | $\{\emptyset, 12567, 134679, 23459\}$                             |                    |
| 9631:81a  | $0, 0, 0, e^{12}, e^{13}, e^{23}, e^{14}, e^{24} + e^{35}, e^{25} + e^{34} + e^{17}$                                                           | $29/109(1, 2, 2, 3, 3, 4, 4, 5, 5)$                  | $\{\emptyset, 125678, 14589, 24679\}$                             | ✓                  |
| 9631:81b  | $0, 0, 0, e^{12}, e^{13}, e^{23}, e^{14}, -e^{24} + e^{35}, e^{25} + e^{17} + e^{34}$                                                          | $29/109(1, 2, 2, 3, 3, 4, 4, 5, 5)$                  | $\{\emptyset, 125678, 14589, 24679\}$                             | ✓                  |
| 9631:82a  | $0, 0, 0, e^{12}, e^{13}, e^{23}, e^{14}, e^{34} + e^{25}, e^{17} + e^{35} + e^{24}$                                                           | $29/109(1, 2, 2, 3, 3, 4, 4, 5, 5)$                  | $\{\emptyset, 13469, 14589, 3568\}$                               | ✓                  |
| 9631:82b  | $0, 0, 0, -e^{12}, e^{13}, e^{23}, e^{14}, -e^{25} + e^{34}, e^{17} + e^{35} + e^{24}$                                                         | $29/109(1, 2, 2, 3, 3, 4, 4, 5, 5)$                  | $\{\emptyset, 13469, 14589, 3568\}$                               | ✓                  |
| 9631:84   | $0, 0, 0, e^{12}, e^{13}, e^{23}, e^{14}, e^{34} + e^{25}, e^{35} + e^{17} + e^{26}$                                                           | $71/657(3, 4, 5, 7, 8, 9, 10, 12, 13)$               | $\{\emptyset, 13469\}$                                            |                    |
| 9631:91   | $0, 0, 0, e^{12}, e^{13}, e^{23}, e^{14}, e^{15} + e^{24}, e^{17} + e^{34} + e^{25}$                                                           | $17/111(2, 3, 4, 5, 6, 7, 7, 8, 9)$                  | $\{\emptyset, 24679\}$                                            |                    |
| 9631:92   | $0, 0, 0, a_1e^{12}, e^{13}, e^{23}, e^{14}, e^{15} + e^{24}, e^{26} + e^{35} + e^{17}$                                                        | $35/317(3, 4, 5, 7, 8, 9, 10, 11, 13)$               | $\{\emptyset, 134689\}$                                           |                    |
| 9631:95a  | $0, 0, 0, e^{12}, e^{13}, e^{23}, e^{14}, e^{25} + e^{16}, e^{35} + e^{17} + e^{24}$                                                           | $29/109(1, 2, 2, 3, 3, 4, 4, 5, 5)$                  | $\{\emptyset, 13469, 14589, 3568\}$                               |                    |
| 9631:95b  | $0, 0, 0, -e^{12}, e^{13}, e^{23}, e^{14}, e^{16} + e^{25}, e^{17} + e^{35} + e^{24}$                                                          | $29/109(1, 2, 2, 3, 3, 4, 4, 5, 5)$                  | $\{\emptyset, 13469, 14589, 3568\}$                               |                    |
| 9631:103  | $0, 0, 0, (-1 + a_2)e^{12}, e^{13}a_2, e^{23}, e^{14}, e^{34} + e^{25} + e^{16}, e^{35} + e^{26} + e^{17}$                                     | $71/657(3, 4, 5, 7, 8, 9, 10, 12, 13)$               | $\{\emptyset, 13469\}$                                            |                    |
| 9631:104a | $0, 0, 0, a_1e^{12}, e^{13}, e^{23}, e^{14}, (1 + a_1)e^{25} + e^{16} + e^{34}, e^{35} + e^{24} + e^{17}$                                      | $29/109(1, 2, 2, 3, 3, 4, 4, 5, 5)$                  | $\{\emptyset, 13469, 14589, 3568\}$                               |                    |

Table A.4 – Continued to next page

Table A.4 – Continued from previous page

| Name      | g                                                                                                                                         | N                                             | S <sub>0</sub>                                        | S = S <sub>0</sub> |
|-----------|-------------------------------------------------------------------------------------------------------------------------------------------|-----------------------------------------------|-------------------------------------------------------|--------------------|
| 9631:104b | $0, 0, 0, -a_1 e^{12}, -e^{13}, e^{23}, e^{14}, e^{25}(-1 + a_1) + e^{34} + e^{16}, e^{24} + e^{35} + e^{17}$                             | 29/109(1, 2, 2, 3, 3, 4, 4, 5, 5)             | {0, 13469, 14589, 3568}                               |                    |
| 9631:108  | $0, 0, 0, e^{12}, e^{13}, e^{23}, e^{14}, e^{24}, e^{27} + e^{18}$                                                                        | 1/61(21, 21, 47, 42, 68, 68, 63, 63, 84)      | {0, 12378, 125678, 13468, 1458, 23457, 2467, 356}     |                    |
| 9631:134  | $0, 0, 0, e^{12}, e^{13}, e^{23}, e^{14}, e^{15} + e^{24}, e^{18} + e^{27}$                                                               | 1/58(14, 27, 40, 41, 54, 67, 55, 68, 82)      | {0, 12378, 13468, 2467}                               |                    |
| 9631:139  | $0, 0, 0, -e^{12}, e^{13}, e^{23}, e^{14}, e^{15}, e^{37} + e^{45} + e^{28}$                                                              | 1/55(13, 30, 30, 43, 43, 60, 56, 56, 86)      | {0, 12378, 125679, 134689, 145, 234578, 24679, 35689} |                    |
| 9631:142  | $0, 0, 0, e^{12}, e^{13}, e^{23}, e^{14}, e^{15} + e^{24}, e^{27} + e^{18} + e^{35}$                                                      | 13/88(2, 3, 4, 5, 6, 7, 7, 8, 10)             | {0, 2467}                                             |                    |
| 9631:144  | $0, 0, 0, e^{12}, e^{13}, e^{23}, e^{14}, e^{15} + e^{24}, e^{36} + e^{18} + e^{27}$                                                      | 71/661(3, 4, 5, 7, 8, 9, 10, 11, 14)          | {0, 13468}                                            |                    |
| 9631:145  | $0, 0, 0, -e^{12}, e^{13}, e^{23}, e^{14}, e^{24} + e^{15}, e^{28} + e^{37} + e^{45}$                                                     | 1/107(29, 46, 63, 75, 92, 109, 104, 121, 167) | {0, 12378, 134689, 24679}                             |                    |
| 9631:156  | $0, 0, 0, e^{12}, -e^{13}, e^{23}, e^{25} - 2e^{16} + e^{34}, e^{24}, e^{17} + e^{45}$                                                    | 1/72(18, 31, 39, 49, 57, 70, 88, 80, 106)     | {0, 12378, 125689, 134689, 14578, 2345, 24679, 35679} |                    |
| 9631:157  | $0, 0, 0, -2e^{12}, -e^{13}, e^{23}, e^{16} + e^{34} + e^{25}, e^{14}, e^{37} + e^{56}$                                                   | 1/76(28, 36, 25, 64, 53, 61, 89, 92, 114)     | {0, 12378, 12568, 13469, 14579, 234589, 246789, 3567} |                    |
| 9631:159a | $0, 0, 0, e^{12}, -e^{13}, e^{23}, -2e^{16} + e^{25} + e^{34}, e^{24} + e^{35}, e^{17} + e^{45}$                                          | 1/40(10, 19, 19, 29, 29, 38, 48, 48, 58)      | {0, 12378, 125689, 134689, 14578, 2345, 24679, 35679} |                    |
| 9631:159b | $0, 0, 0, -e^{12}, -e^{13}, e^{23}, -2e^{16} + 2e^{16} + e^{34}, e^{24} + e^{35}, e^{17} + e^{45}$                                        | 1/40(10, 19, 19, 29, 29, 38, 48, 48, 58)      | {0, 12378, 125689, 134689, 14578, 2345, 24679, 35679} |                    |
| 9631:161  | $0, 0, 0, -e^{12}, -2e^{13}, -e^{23}, e^{16} + e^{25} + e^{34}, e^{35} + e^{14}, e^{46} + e^{27}$                                         | 19/293(7, 5, 6, 12, 13, 11, 18, 19, 23)       | {0, 12378, 125689, 35679}                             |                    |
| 9631:167  | $0, 0, 0, -e^{12}, -2e^{13}, -e^{23}, e^{34} + e^{25} + e^{16}, e^{14}, e^{46} + e^{35} + e^{27}$                                         | 1/87(37, 23, 46, 60, 83, 69, 106, 97, 129)    | {0, 125689, 14579, 24678}                             |                    |
| 9631:178  | $0, 0, 0, e^{12}, e^{13}, e^{23}, e^{14}, e^{16} + e^{25}, e^{18} + e^{37} + e^{45}$                                                      | 1/4(1, 2, 2, 3, 3, 4, 4, 5, 6)                | {0, 12378, 125679, 13469, 1458, 23457, 246789, 35689} |                    |
| 9631:179a | $0, 0, 0, -e^{12}, e^{13}, e^{23}, e^{14}, e^{15} + e^{26}, e^{45} + e^{28} + e^{37}$                                                     | 1/101(35, 35, 52, 70, 87, 87, 105, 122, 157)  | {0, 12378, 125679, 134689, 145, 234578, 24679, 35689} |                    |
| 9631:179b | $0, 0, 0, -e^{12}, -e^{13}, e^{23}, -e^{14}, e^{26} + e^{15}, e^{28} + e^{45} + e^{37}$                                                   | 1/101(35, 35, 52, 70, 87, 87, 105, 122, 157)  | {0, 12378, 125679, 134689, 145, 234578, 24679, 35689} |                    |
| 9631:184  | $0, 0, 0, e^{12}, -e^{13}, e^{23}, e^{25} - 2e^{16} + e^{34}, e^{45} + e^{18} + e^{27}$                                                   | 1/49(13, 20, 27, 33, 40, 47, 53, 60, 73)      | {0, 12378, 134679, 24689}                             |                    |
| 9631:185  | $0, 0, 0, e^{12}, e^{13}(-1 + a_3), e^{23}, a_3 e^{14}, (-2 + a_3)e^{16} + e^{34} + e^{25}, e^{18} + e^{37} + e^{45}$                     | 1/4(1, 2, 2, 3, 3, 4, 4, 5, 6)                | {0, 12378, 125679, 13469, 1458, 23457, 246789, 35689} |                    |
| 9631:186a | $0, 0, 0, -2e^{12}, -e^{13}, e^{23}, e^{14}, e^{16} + e^{25} + e^{34}, e^{56} + e^{17} + e^{38}$                                          | 1/23(8, 11, 8, 19, 16, 19, 27, 27, 35)        | {0, 12378, 12567, 13469, 14589, 234579, 246789, 3568} |                    |
| 9631:186b | $0, 0, 0, -2e^{12}, -e^{13}, e^{23}, -e^{14}, e^{16} + e^{25} + e^{34}, e^{56} + e^{17} + e^{38}$                                         | 1/23(8, 11, 8, 19, 16, 19, 27, 27, 35)        | {0, 12378, 12567, 13469, 14589, 234579, 246789, 3568} |                    |
| 9631:187  | $0, 0, 0, -e^{12}, -e^{13}, e^{23}, e^{15} + e^{24}, e^{16} + e^{34}, e^{18} + e^{27} + e^{45}$                                           | 1/49(13, 20, 27, 33, 40, 47, 53, 60, 73)      | {0, 12378, 134679, 24689}                             |                    |
| 9631:188a | $0, 0, 0, e^{12}, e^{13}, e^{23}, e^{24} - e^{15}, e^{36} + e^{14}, e^{38} + e^{27} + e^{45}$                                             | 19/49(1, 1, 1, 2, 2, 2, 3, 3, 4)              | {0, 12378, 134679, 24689}                             |                    |
| 9631:188b | $0, 0, 0, -e^{12}, e^{13}, e^{23}, e^{24} + e^{15}, e^{36} + e^{14}, e^{45} + e^{38} + e^{27}$                                            | 19/49(1, 1, 1, 2, 2, 2, 3, 3, 4)              | {0, 12378, 134679, 24689}                             |                    |
| 9631:189a | $0, 0, 0, e^{12}, e^{13}, e^{23}, e^{25} + e^{34}, e^{36} + 2e^{14}, e^{17} + e^{45} + e^{38}$                                            | 1/23(8, 11, 8, 19, 16, 19, 27, 27, 35)        | {0, 12378, 125689, 13469, 1457, 23458, 246789, 35679} |                    |
| 9631:189b | $0, 0, 0, e^{12}, e^{13}, -e^{23}, e^{34} + e^{25}, e^{36} + 2e^{14}, e^{17} + e^{38} + e^{45}$                                           | 1/23(8, 11, 8, 19, 16, 19, 27, 27, 35)        | {0, 12378, 125689, 13469, 1457, 23458, 246789, 35679} |                    |
| 9631:190  | $0, 0, 0, e^{12}, e^{13}, -e^{23}, e^{14} + e^{35}, e^{36} + e^{24}, e^{27} + e^{56} + e^{18}$                                            | 19/49(1, 1, 1, 2, 2, 2, 3, 3, 4)              | {0, 12378, 125678, 356}                               |                    |
| 9631:191a | $0, 0, 0, e^{12}, e^{13}, -e^{23}, e^{35} + e^{24}, e^{36} + e^{14}, e^{27} + e^{18} + e^{56}$                                            | 19/49(1, 1, 1, 2, 2, 2, 3, 3, 4)              | {0, 12378, 125678, 134679, 14579, 234589, 24689, 356} |                    |
| 9631:191b | $0, 0, 0, e^{12}, e^{13}, -e^{23}, e^{24} + e^{35}, -e^{14} + e^{36}, e^{18} + e^{27} + e^{56}$                                           | 19/49(1, 1, 1, 2, 2, 2, 3, 3, 4)              | {0, 12378, 125678, 134679, 14579, 234589, 24689, 356} |                    |
| 9631:191c | $0, 0, 0, -e^{12}, e^{13}, -e^{23}, e^{35} + e^{24}, e^{36} + e^{14}, e^{56} + e^{18} + e^{27}$                                           | 19/49(1, 1, 1, 2, 2, 2, 3, 3, 4)              | {0, 12378, 125678, 134679, 14579, 234589, 24689, 356} |                    |
| 9631:192a | $0, 0, 0, e^{12}, e^{13}, e^{23}, e^{34} + e^{25}, e^{36} + e^{14}, e^{56} + e^{37} + e^{18}$                                             | 1/23(8, 11, 8, 19, 16, 19, 27, 27, 35)        | {0, 12378, 12568, 13469, 14579, 234589, 246789, 3567} |                    |
| 9631:192b | $0, 0, 0, e^{12}, e^{13}, e^{23}, e^{25} + e^{34}, e^{36} - e^{14}, e^{37} + e^{18} + e^{56}$                                             | 1/23(8, 11, 8, 19, 16, 19, 27, 27, 35)        | {0, 12378, 12568, 13469, 14579, 234589, 246789, 3567} |                    |
| 9631:195  | $0, 0, 0, -a_1 e^{12}, -e^{13}, e^{23}, (1 + a_1)e^{15} + e^{24}, e^{16}(-1 + a_1) + e^{25} + e^{34}, e^{45} + e^{18} + e^{27}$           | 1/49(13, 20, 27, 33, 40, 47, 53, 60, 73)      | {0, 12378, 134679, 24689}                             |                    |
| 9631:197a | $0, 0, 0, -e^{12}, e^{13}, e^{23} a_2, e^{35} + (1 + a_2)e^{24}, e^{16} + e^{34} + (-1 + a_2)e^{25}, e^{28} + e^{37} + e^{46}$            | 1/23(11, 8, 8, 19, 19, 16, 27, 27, 35)        | {0, 12378, 125679, 13467, 145789, 23459, 2468, 35689} |                    |
| 9631:197b | $0, 0, 0, -e^{12}, -e^{13}, e^{23} a_2, e^{35} + (1 + a_2)e^{24}, e^{16} + e^{34} - (-1 + a_2)e^{25}, e^{46} + e^{28} + e^{37}$           | 1/23(11, 8, 8, 19, 19, 16, 27, 27, 35)        | {0, 12378, 125679, 13467, 145789, 23459, 2468, 35689} |                    |
| 9631:199  | $0, 0, 0, -e^{12}, -2e^{13}, -e^{23}, e^{14}, e^{16} + e^{25} + e^{34}, e^{35} + e^{46} + e^{28} + e^{17}$                                | 11/81(3, 2, 4, 5, 7, 6, 8, 9, 11)             | {0, 14589}                                            |                    |
| 9631:201  | $0, 0, 0, -e^{12}, -e^{13}, e^{23}, e^{15} + e^{24}, e^{34} + e^{16}, e^{18} + e^{27} + e^{45} + e^{36}$                                  | 11/81(2, 3, 4, 5, 6, 7, 8, 9, 11)             | {0, 24689}                                            |                    |
| 9631:204  | $0, 0, 0, -e^{12}, e^{13}, a_3 e^{23}, e^{15} + e^{24} + e^{36}, e^{14} + e^{35} + e^{26}, e^{38} + e^{27} + e^{45}$                      | 19/49(1, 1, 1, 2, 2, 2, 3, 3, 4)              | {0, 12378}                                            |                    |
| 9631:205  | $0, 0, 0, -e^{12}(-1 + a_3), -e^{13}, e^{23}, a_3 e^{15} + e^{24}, (-2 + a_3)e^{16} + e^{25} + e^{34}, e^{36} + e^{45} + e^{27} + e^{18}$ | 11/81(2, 3, 4, 5, 6, 7, 8, 9, 11)             | {0, 24689}                                            |                    |
| 963:5     | $0, 0, 0, e^{12}, e^{13}, e^{23}, e^{14}, e^{15}, e^{25} + e^{34}$                                                                        | 1/13(4, 7, 7, 11, 11, 14, 15, 15, 18)         | {0, 123789, 12567, 13468, 1459, 234578, 24679, 35689} |                    |
| 963:9     | $0, 0, 0, e^{12}, e^{13}, e^{23}, e^{14}, e^{15} + e^{24}, e^{34} + e^{25}$                                                               | 1/33(11, 15, 19, 26, 30, 34, 37, 41, 45)      | {0, 123789, 13468, 24679}                             |                    |
| 963:16    | $0, 0, 0, e^{12}, e^{13}, e^{23}, e^{14}, e^{24}, e^{16} + e^{25}$                                                                        | 1/13(5, 5, 8, 10, 13, 13, 15, 15, 18)         | {0, 123789, 125678, 13468, 14589, 23457, 24679, 3569} |                    |
| 963:22    | $0, 0, 0, -e^{12}, e^{13}, e^{23}, e^{24}, e^{15}, e^{16} + e^{34}$                                                                       | 1/9(3, 4, 5, 7, 8, 9, 11, 11, 12)             | {0, 123789, 12567, 134678, 14579, 23458, 2469, 35689} |                    |
| 963:27    | $0, 0, 0, -e^{12}, e^{13}, e^{23}, e^{24}, e^{35}, e^{16} + e^{34}$                                                                       | 3/7(1, 1, 1, 2, 2, 2, 3, 3, 3)                | {0, 123789, 125678, 134678, 145789, 2345, 2469, 3569} |                    |

Table A.4 – Continued to next page

Table A.4 – Continued from previous page

| Name    | g                                                                                                                                      | N                                                 | S <sub>0</sub>                                            | S = S <sub>0</sub> |
|---------|----------------------------------------------------------------------------------------------------------------------------------------|---------------------------------------------------|-----------------------------------------------------------|--------------------|
| 963:28  | $0, 0, 0, a_1 e^{12}, e^{13}(1 + a_1), e^{23}, e^{14}, e^{24}, e^{25} + e^{34} + e^{16}$                                               | $1/13(5, 5, 8, 10, 13, 13, 15, 15, 18)$           | $\{0, 123789, 125678, 13468, 14589, 23457, 24679, 3569\}$ |                    |
| 963:29  | $0, 0, 0, (-1 + a_2)e^{12}, e^{13}a_2, e^{23}, e^{14}, e^{15}, e^{25} + e^{16} + e^{34}$                                               | $1/13(4, 7, 7, 11, 11, 14, 15, 15, 18)$           | $\{0, 123789, 12567, 13468, 1459, 234578, 24679, 35689\}$ |                    |
| 963:31  | $0, 0, 0, (-1 + a_2)e^{12}, e^{13}a_2, e^{23}, e^{24}, e^{15}, e^{34} + e^{25} + e^{16}$                                               | $1/9(3, 4, 5, 7, 8, 9, 11, 11, 12)$               | $\{0, 123789, 12567, 134678, 14579, 23458, 2469, 35689\}$ |                    |
| 963:32  | $0, 0, 0, a_1 e^{12}, e^{13}(1 + a_1), e^{23}, e^{24}, e^{35}, e^{16} + e^{25} + e^{34}$                                               | $3/7(1, 1, 1, 2, 2, 2, 3, 3, 3)$                  | $\{0, 123789, 125678, 134678, 145789, 2345, 2469, 3569\}$ |                    |
| 963:33  | $0, 0, 0, -e^{12}, e^{13}, e^{23}, e^{14}, e^{15} + e^{24}, e^{16} + e^{34}$                                                           | $1/33(11, 15, 19, 26, 30, 34, 37, 41, 45)$        | $\{0, 123789, 13468, 24679\}$                             |                    |
| 963:34a | $0, 0, 0, -e^{12}, e^{13}, e^{23}, e^{14}, e^{35} + e^{24}, e^{34} + e^{16}$                                                           | $1/89(31, 43, 43, 74, 74, 86, 105, 117, 117)$     | $\{0, 123789, 125678, 13468, 14589, 23457, 24679, 3569\}$ |                    |
| 963:34b | $0, 0, 0, -e^{12}, -e^{13}, e^{23}, e^{14}, e^{35} + e^{24}, e^{16} + e^{34}$                                                          | $1/89(31, 43, 43, 74, 74, 86, 105, 117, 117)$     | $\{0, 123789, 125678, 13468, 14589, 23457, 24679, 3569\}$ |                    |
| 963:36  | $0, 0, 0, e^{12}, e^{13}, e^{23}, e^{14}, e^{24} + e^{15}, e^{25} + e^{16}$                                                            | $1/33(11, 15, 19, 26, 30, 34, 37, 41, 45)$        | $\{0, 123789, 13468, 24679\}$                             |                    |
| 963:37  | $0, 0, 0, a_1 e^{12}, e^{13}, e^{23}, e^{14}, e^{15} + e^{24}, e^{35} + e^{26}$                                                        | $1/16(6, 7, 8, 13, 14, 15, 19, 20, 22)$           | $\{0, 123789, 134689, 2467\}$                             |                    |
| 963:39a | $0, 0, 0, e^{12}, e^{13}, e^{23}, e^{14}, e^{34} + e^{25}, e^{26} + e^{15}$                                                            | $1/89(35, 35, 47, 70, 82, 82, 105, 117, 117)$     | $\{0, 123789, 12567, 13469, 1458, 234579, 24678, 35689\}$ |                    |
| 963:39b | $0, 0, 0, -e^{12}, -e^{13}, e^{23}, e^{14}, e^{25} + e^{34}, e^{15} + e^{26}$                                                          | $1/89(35, 35, 47, 70, 82, 82, 105, 117, 117)$     | $\{0, 123789, 12567, 13469, 1458, 234579, 24678, 35689\}$ |                    |
| 963:40a | $0, 0, 0, e^{12}, e^{13}, e^{23}, e^{14}, e^{24} + e^{35}, e^{16} + e^{25}$                                                            | $1/89(31, 43, 43, 74, 74, 86, 105, 117, 117)$     | $\{0, 123789, 125678, 13468, 14589, 23457, 24679, 3569\}$ |                    |
| 963:40b | $0, 0, 0, -e^{12}, e^{13}, e^{23}, e^{14}, e^{35} + e^{24}, e^{25} + e^{16}$                                                           | $1/89(31, 43, 43, 74, 74, 86, 105, 117, 117)$     | $\{0, 123789, 125678, 13468, 14589, 23457, 24679, 3569\}$ |                    |
| 963:43a | $0, 0, 0, e^{12}, e^{13}, e^{23}, e^{24}, e^{25} + e^{34}, e^{15} + e^{26}$                                                            | $1/89(35, 35, 47, 70, 82, 82, 105, 117, 117)$     | $\{0, 123789, 12567, 134679, 14578, 23459, 2468, 35689\}$ |                    |
| 963:43b | $0, 0, 0, -e^{12}, -e^{13}, e^{23}, e^{24}, e^{25} + e^{34}, e^{26} + e^{15}$                                                          | $1/89(35, 35, 47, 70, 82, 82, 105, 117, 117)$     | $\{0, 123789, 12567, 134679, 14578, 23459, 2468, 35689\}$ |                    |
| 963:46  | $0, 0, 0, e^{12}, e^{13}, e^{23}, e^{14}, e^{34} + e^{25}, e^{26} + e^{35}$                                                            | $1/123(49, 53, 57, 102, 106, 110, 151, 159, 163)$ | $\{0, 123789, 13469, 24678\}$                             |                    |
| 963:48  | $0, 0, 0, e^{12}, e^{13}, e^{23}, e^{24}, e^{25} + e^{34}, e^{15} + e^{36}$                                                            | $1/123(53, 49, 57, 102, 110, 106, 151, 159, 163)$ | $\{0, 123789, 14578, 23459\}$                             |                    |
| 963:52  | $0, 0, 0, e^{12}, e^{13}, e^{23}, e^{24} + e^{15}, e^{34} + e^{25}, e^{36}$                                                            | $1/123(57, 53, 49, 110, 106, 102, 163, 159, 151)$ | $\{0, 123789, 13467, 24689\}$                             |                    |
| 963:54  | $0, 0, 0, (-1 + a_2)e^{12}, e^{13}a_2, e^{23}, e^{14}, e^{15} + e^{24}, e^{34} + e^{25} + e^{16}$                                      | $1/33(11, 15, 19, 26, 30, 34, 37, 41, 45)$        | $\{0, 123789, 13468, 24679\}$                             |                    |
| 963:55a | $0, 0, 0, (-1 + a_2)e^{12}, e^{13}a_2, e^{23}, e^{14}, e^{35} + e^{24}, e^{34} + e^{16} + e^{25}$                                      | $1/89(31, 43, 43, 74, 74, 86, 105, 117, 117)$     | $\{0, 123789, 125678, 13468, 14589, 23457, 24679, 3569\}$ |                    |
| 963:55b | $0, 0, 0, (-1 + a_2)e^{12}, e^{13}a_2, e^{23}, e^{14}, e^{35} - e^{24}, e^{16} + e^{25} + e^{34}$                                      | $1/89(31, 43, 43, 74, 74, 86, 105, 117, 117)$     | $\{0, 123789, 125678, 13468, 14589, 23457, 24679, 3569\}$ |                    |
| 963:59a | $0, 0, 0, (-1 + a_2)e^{12}, e^{13}a_2, e^{23}, e^{14}, e^{15} + e^{26}, e^{16} + e^{25} + e^{34}$                                      | $1/89(35, 35, 47, 70, 82, 82, 105, 117, 117)$     | $\{0, 123789, 12567, 13468, 1459, 234578, 24679, 35689\}$ |                    |
| 963:59b | $0, 0, 0, (-1 + a_2)e^{12}, e^{13}a_2, e^{23}, e^{14}, e^{26} - e^{15}, e^{25} + e^{34} + e^{16}$                                      | $1/89(35, 35, 47, 70, 82, 82, 105, 117, 117)$     | $\{0, 123789, 12567, 13468, 1459, 234578, 24679, 35689\}$ |                    |
| 963:62  | $0, 0, 0, a_1 e^{12}, e^{13}, e^{23}, e^{14}, e^{26} + e^{35}, e^{15} + e^{36} + e^{24}$                                               | $3/7(1, 1, 1, 2, 2, 2, 3, 3, 3)$                  | $\{0, 123789\}$                                           |                    |
| 963:63  | $0, 0, 0, (-1 + a_2)e^{12}, e^{13}a_2, e^{23}, e^{14}, e^{26} + e^{35}, e^{16} + e^{25} + e^{34}$                                      | $1/123(49, 53, 57, 102, 106, 110, 151, 163, 159)$ | $\{0, 123789, 13468, 24679\}$                             |                    |
| 963:66a | $0, 0, 0, e^{12}, e^{13}, e^{23}, e^{24} + e^{15}, e^{25} + e^{34}, e^{36} + e^{14}$                                                   | $3/7(1, 1, 1, 2, 2, 2, 3, 3, 3)$                  | $\{0, 123789, 13467, 24689\}$                             |                    |
| 963:66b | $0, 0, 0, -e^{12}, -e^{13}, e^{23}, e^{24} + e^{15}, e^{25} + e^{34}, e^{36} + e^{14}$                                                 | $3/7(1, 1, 1, 2, 2, 2, 3, 3, 3)$                  | $\{0, 123789, 13467, 24689\}$                             |                    |
| 963:68  | $0, 0, 0, e^{12}a_2, e^{13}a_2, e^{23}, e^{35} + e^{14}, e^{25} + e^{34}, e^{36} + e^{24}$                                             | $3/7(1, 1, 1, 2, 2, 2, 3, 3, 3)$                  | $\{0, 123789, 125679, 3568\}$                             |                    |
| 963:71a | $0, 0, 0, e^{12}, e^{13}, e^{23}, e^{15} + e^{24}, e^{14} + e^{36}, e^{25} + e^{16}$                                                   | $3/7(1, 1, 1, 2, 2, 2, 3, 3, 3)$                  | $\{0, 123789, 13467, 24689\}$                             |                    |
| 963:71b | $0, 0, 0, -e^{12}, e^{13}, e^{23}, e^{24} + e^{15}, e^{36} + e^{14}, e^{16} + e^{25}$                                                  | $3/7(1, 1, 1, 2, 2, 2, 3, 3, 3)$                  | $\{0, 123789, 13467, 24689\}$                             |                    |
| 963:72a | $0, 0, 0, e^{12}, e^{13}, e^{23}, e^{24} + a_1 e^{15}, e^{36} + e^{14}, e^{26} + e^{35}$                                               | $3/7(1, 1, 1, 2, 2, 2, 3, 3, 3)$                  | $\{0, 123789, 134679, 2468\}$                             | ✓                  |
| 963:72b | $0, 0, 0, -e^{12}, e^{13}, e^{23}, e^{24} + a_1 e^{15}, e^{14} + e^{36}, e^{26} + e^{35}$                                              | $3/7(1, 1, 1, 2, 2, 2, 3, 3, 3)$                  | $\{0, 123789, 134679, 2468\}$                             | ✓                  |
| 963:73  | $0, 0, 0, -e^{12}, e^{13}, e^{23}, e^{15}a_2 + e^{24}, e^{16} + e^{34}, e^{26} + e^{35}$                                               | $3/7(1, 1, 1, 2, 2, 2, 3, 3, 3)$                  | $\{0, 123789, 134679, 2468\}$                             |                    |
| 963:74a | $0, 0, 0, e^{12}, e^{13}, e^{23}, e^{35} + e^{24}, e^{36} + a_1 e^{14}, e^{15} + e^{26}$                                               | $3/7(1, 1, 1, 2, 2, 2, 3, 3, 3)$                  | $\{0, 123789, 125678, 134679, 1457, 234589, 2468, 3569\}$ | ✓                  |
| 963:74b | $0, 0, 0, e^{12}, -e^{13}, e^{23}, e^{35} + e^{24}, e^{36} + a_1 e^{14}, e^{15} + e^{26}$                                              | $3/7(1, 1, 1, 2, 2, 2, 3, 3, 3)$                  | $\{0, 123789, 125678, 134679, 1457, 234589, 2468, 3569\}$ | ✓                  |
| 963:75a | $0, 0, 0, e^{12}, e^{13}, e^{23}, e^{25} + e^{34}, e^{36} + e^{14}, e^{26} + e^{15}$                                                   | $3/7(1, 1, 1, 2, 2, 2, 3, 3, 3)$                  | $\{0, 123789, 12568, 13469, 1457, 234589, 24678, 35679\}$ | ✓                  |
| 963:75b | $0, 0, 0, e^{12}, e^{13}, e^{23}, e^{34} + e^{25}, e^{36} - e^{14}, e^{26} + e^{15}$                                                   | $3/7(1, 1, 1, 2, 2, 2, 3, 3, 3)$                  | $\{0, 123789, 12568, 13469, 1457, 234589, 24678, 35679\}$ | ✓                  |
| 963:75c | $0, 0, 0, -e^{12}, -e^{13}, e^{23}, e^{34} + e^{25}, -e^{14} + e^{36}, e^{26} + e^{15}$                                                | $3/7(1, 1, 1, 2, 2, 2, 3, 3, 3)$                  | $\{0, 123789, 12568, 13469, 1457, 234589, 24678, 35679\}$ | ✓                  |
| 963:80a | $0, 0, 0, (-1 + a_2)e^{12}, e^{13}a_2, e^{23}, e^{24} + e^{15}, e^{36} + e^{14}, e^{16} + e^{25} + e^{34}$                             | $3/7(1, 1, 1, 2, 2, 2, 3, 3, 3)$                  | $\{0, 123789, 13467, 24689\}$                             |                    |
| 963:80b | $0, 0, 0, (-1 + a_2)e^{12}, e^{13}a_2, e^{23}, e^{24} + e^{15}, e^{36} - e^{14}, e^{25} + e^{34} + e^{16}$                             | $3/7(1, 1, 1, 2, 2, 2, 3, 3, 3)$                  | $\{0, 123789, 13467, 24689\}$                             |                    |
| 963:83  | $0, 0, 0, (-1 + a_2)e^{12}, e^{13}a_2, e^{23}, a_3 e^{14} + e^{35}, e^{36} + e^{24}, e^{16} + e^{25} + e^{34}$                         | $3/7(1, 1, 1, 2, 2, 2, 3, 3, 3)$                  | $\{0, 123789, 125678, 3569\}$                             |                    |
| 963:84a | $0, 0, 0, (-1 + a_2)e^{12}, e^{13}a_2, e^{23}, e^{24} + e^{35}, e^{14} + e^{36}, e^{16} + e^{25} + e^{34}$                             | $3/7(1, 1, 1, 2, 2, 2, 3, 3, 3)$                  | $\{0, 123789, 125678, 13467, 14579, 23458, 24689, 3569\}$ | ✓                  |
| 963:84b | $0, 0, 0, (-1 + a_2)e^{12}, e^{13}a_2, e^{23}, e^{35} - e^{24}, e^{36} + e^{14}, e^{34} + e^{25} + e^{16}$                             | $3/7(1, 1, 1, 2, 2, 2, 3, 3, 3)$                  | $\{0, 123789, 125678, 13467, 14579, 23458, 24689, 3569\}$ | ✓                  |
| 963:84c | $0, 0, 0, (-1 + a_2)e^{12}, e^{13}a_2, e^{23}, e^{35} - e^{24}, e^{36} - e^{14}, e^{34} + e^{25} + e^{16}$                             | $3/7(1, 1, 1, 2, 2, 2, 3, 3, 3)$                  | $\{0, 123789, 125678, 13467, 14579, 23458, 24689, 3569\}$ | ✓                  |
| 963:86  | $0, 0, 0, e^{12}a_2, e^{13}a_2, e^{23}, e^{25} + e^{34}, a_3 e^{14} + e^{26} + e^{35}, e^{24} + e^{36} + e^{15}$                       | $3/7(1, 1, 1, 2, 2, 2, 3, 3, 3)$                  | $\{0, 123789\}$                                           |                    |
| 963:87  | $0, 0, 0, a_1 e^{12}, e^{13}(a_3 + a_1), e^{23}, a_3 e^{16} + e^{34} + e^{25}, a_4 e^{14} + e^{35} + e^{26}, e^{36} + e^{15} + e^{24}$ | $3/7(1, 1, 1, 2, 2, 2, 3, 3, 3)$                  | $\{0, 123789\}$                                           |                    |

Table A.4 – Continued to next page

Table A.4 – Continued from previous page

| Name      | g                                                                                                                                        | N                                                 | S <sub>0</sub>                                        | S = S <sub>0</sub> |
|-----------|------------------------------------------------------------------------------------------------------------------------------------------|---------------------------------------------------|-------------------------------------------------------|--------------------|
| 954321:8  | $0, 0, 0, 0, -e^{12}, e^{15}, e^{16}, e^{23} + e^{17}, e^{18} + e^{35} + e^{24}$                                                         | 1/119(20, 69, 80, 100, 89, 109, 129, 149, 169)    | {0, 12468, 14579, 256789}                             |                    |
| 954321:12 | $0, 0, 0, 0, e^{12}, e^{15}, e^{16}, e^{17} + e^{25}, e^{18} + e^{26} + e^{34}$                                                          | 21/116(1, 3, 4, 4, 5, 6, 7, 8)                    | {0, 123468, 1268, 34}                                 |                    |
| 954321:13 | $0, 0, 0, 0, -e^{12}, e^{15}, e^{16} + e^{23}, e^{17} + e^{35}, e^{24} + e^{36} + e^{18}$                                                | 2/35(3, 10, 9, 15, 13, 16, 19, 22, 25)            | {0, 123468, 134579, 256789}                           |                    |
| 954321:22 | $0, 0, 0, 0, -e^{12}, e^{15}, e^{16} + e^{23}, e^{17} + e^{35} + e^{24}, e^{18} + e^{36} + e^{45}$                                       | 1/87(16, 47, 48, 64, 63, 79, 95, 111, 127)        | {0, 12368, 13579, 256789}                             |                    |
| 954321:24 | $0, 0, 0, 0, e^{12}, e^{15}, e^{16} + e^{25}, e^{17} + e^{26}, e^{18} + e^{34} + e^{56}$                                                 | 5/47(2, 4, 7, 7, 6, 8, 10, 12, 14)                | {0, 13579, 14579, 34}                                 |                    |
| 954321:25 | $0, 0, 0, 0, e^{12}, e^{15}, e^{25} + e^{16}, e^{26} + e^{17}, e^{18} + e^{34} + e^{27}$                                                 | 5/47(2, 4, 7, 7, 6, 8, 10, 12, 14)                | {0, 13579, 14579, 34}                                 |                    |
| 954321:37 | $0, 0, 0, 0, -e^{12}, e^{15} + e^{23}, e^{16} + e^{35}, e^{17} + e^{36}, e^{37} + e^{24} + e^{18}$                                       | 1/95(16, 55, 32, 80, 71, 87, 103, 119, 135)       | {0, 12468, 14579, 256789}                             |                    |
| 954321:38 | $0, 0, 0, 0, a_1 e^{12}, e^{25} - (-1 + a_1) e^{16}, e^{17} + e^{26}, e^{18} + e^{27} + e^{56} + e^{34}$                                 | 5/47(2, 4, 7, 7, 6, 8, 10, 12, 14)                | {0, 13579, 14579, 34}                                 |                    |
| 954321:42 | $0, 0, 0, 0, -e^{12}, e^{15} + e^{23}, e^{16} + e^{35}, e^{17} + e^{36} + e^{24}, e^{18} + e^{37} + e^{45}$                              | 2/11(1, 3, 2, 4, 4, 5, 6, 7, 8)                   | {0, 1268, 1579, 256789}                               |                    |
| 954321:48 | $0, 0, 0, 0, -e^{12}, e^{15} + e^{23}, e^{16} + e^{24} + e^{35}, e^{45} + e^{17} + e^{36}, e^{46} + e^{37} + e^{18}$                     | 1/21(4, 11, 8, 12, 15, 19, 23, 27, 31)            | {0, 12468, 14579, 256789}                             |                    |
| 95432:2   | $0, 0, 0, 0, -e^{12}, e^{15}, e^{16}, e^{17}, e^{34} + e^{56} + e^{27}$                                                                  | 1/257(32, 155, 203, 203, 187, 219, 251, 283, 406) | {0, 123689, 124689, 13579, 14579, 2345678, 25678, 34} |                    |
| 95432:6   | $0, 0, 0, 0, -e^{12}, e^{15}, e^{16}, e^{17} + e^{23}, e^{34} + e^{27} + e^{56}$                                                         | 1/109(19, 55, 76, 91, 74, 93, 112, 131, 167)      | {0, 124689, 14579, 25678}                             |                    |
| 95432:12  | $0, 0, 0, 0, -e^{12}, e^{15}, e^{16}, e^{17} + e^{25}, e^{27} + e^{34} + e^{56}$                                                         | 44/515(2, 6, 9, 9, 8, 10, 12, 14, 18)             | {0, 123689, 124689, 34}                               |                    |
| 95432:14  | $0, 0, 0, 0, -e^{12}, e^{15}, e^{23} + e^{16}, e^{35} + e^{17}, e^{34} + e^{56} + e^{27}$                                                | 1/381(77, 169, 231, 338, 246, 323, 400, 477, 569) | {0, 123689, 13579, 25678}                             |                    |
| 95432:18  | $0, 0, 0, 0, -e^{12}, e^{15}, e^{23} + e^{16}, e^{35} + e^{24} + e^{17}, e^{27} + e^{56}$                                                | 1/47(11, 17, 33, 44, 28, 39, 50, 61, 67)          | {0, 123689, 13579, 25678}                             |                    |
| 95432:21a | $0, 0, 0, 0, -e^{12}, e^{15}, e^{23} + e^{16}, e^{24} + e^{17} + e^{35}, e^{56} + e^{34} + e^{27}$                                       | 7/33(1, 2, 3, 4, 3, 4, 5, 6, 7)                   | {0, 123689, 13579, 25678}                             |                    |
| 95432:21b | $0, 0, 0, 0, -e^{12}, -e^{15}, e^{16} + e^{23}, e^{17} + e^{35} + e^{24}, e^{27} + e^{56} + e^{34}$                                      | 7/33(1, 2, 3, 4, 3, 4, 5, 6, 7)                   | {0, 123689, 13579, 25678}                             |                    |
| 95432:22  | $0, 0, 0, 0, -e^{12}, e^{15}, e^{16} + e^{25}, e^{17} + e^{26}, e^{27} + e^{34} + e^{56}$                                                | 5/47(2, 4, 7, 7, 6, 8, 10, 12, 14)                | {0, 13579, 14579, 34}                                 |                    |
| 95421:14  | $0, 0, 0, 0, -e^{12}, e^{15}, e^{34} + e^{25}, e^{23} + e^{16}, e^{18} + e^{35}$                                                         | 1/521(97, 301, 291, 408, 398, 495, 699, 592, 689) | {0, 123679, 13578, 25689}                             |                    |
| 95421:17  | $0, 0, 0, 0, -e^{12}, e^{15}, e^{25}, e^{16}, e^{56} + e^{28} + e^{34}$                                                                  | 1/124(26, 57, 96, 96, 83, 109, 140, 135, 192)     | {0, 123679, 124679, 135789, 145789, 234568, 2568, 34} |                    |
| 95421:19  | $0, 0, 0, 0, -e^{12}, e^{15}, e^{25} + e^{13}, e^{16} + e^{24}, e^{45} + e^{18}$                                                         | 3/389(29, 63, 126, 87, 92, 121, 155, 150, 179)    | {0, 124679, 14578, 25689}                             |                    |
| 95421:25  | $0, 0, 0, 0, -e^{12}, e^{15}, e^{25}, e^{16} + e^{23}, e^{18} + e^{24} + e^{35}$                                                         | 1/123(29, 57, 87, 116, 86, 115, 143, 144, 173)    | {0, 123679, 13578, 25689}                             |                    |
| 95421:26a | $0, 0, 0, 0, -e^{12}, e^{15}, e^{25} + e^{34}, e^{23} + e^{16}, e^{24} + e^{18} + e^{35}$                                                | 4/21(1, 3, 3, 4, 4, 5, 7, 6, 7)                   | {0, 123679, 13578, 25689}                             |                    |
| 95421:26b | $0, 0, 0, 0, -e^{12}, e^{15}, e^{34} - e^{25}, e^{16} + e^{23}, e^{18} + e^{35} + e^{24}$                                                | 4/21(1, 3, 3, 4, 4, 5, 7, 6, 7)                   | {0, 123679, 13578, 25689}                             |                    |
| 95421:29  | $0, 0, 0, 0, -e^{12}, e^{15}, e^{25}, e^{16} + e^{23}, e^{56} + e^{28} + e^{34}$                                                         | 1/29(7, 12, 21, 24, 19, 26, 31, 33, 45)           | {0, 123679, 135789, 2568}                             |                    |
| 95421:32a | $0, 0, 0, 0, -e^{12}, e^{15}, e^{13} + e^{25}, e^{16} + e^{24}, e^{18} + e^{23} + e^{45}$                                                | 11/47(1, 2, 4, 3, 3, 4, 5, 5, 6)                  | {0, 124679, 14578, 25689}                             |                    |
| 95421:32b | $0, 0, 0, 0, -e^{12}, -e^{15}, e^{13} + e^{25}, e^{24} + e^{16}, e^{23} + e^{45} + e^{18}$                                               | 11/47(1, 2, 4, 3, 3, 4, 5, 5, 6)                  | {0, 124679, 14578, 25689}                             |                    |
| 95421:37  | $0, 0, 0, 0, -e^{12}, e^{15}, e^{25} + a_2 e^{13}, e^{16} + e^{24}, e^{28} + e^{56} + e^{34}$                                            | 1/29(7, 12, 24, 21, 19, 26, 31, 33, 45)           | {0, 124679, 145789, 2568}                             |                    |
| 95421:47  | $0, 0, 0, 0, e^{12}, e^{25} + e^{13}, e^{34} + e^{15}, e^{35} + e^{26}, e^{28} + e^{36}$                                                 | 1/381(203, 79, 158, 327, 282, 361, 485, 440, 519) | {0, 124679, 15689, 24578}                             |                    |
| 95421:48  | $0, 0, 0, 0, -e^{12}, e^{15} + e^{23}, e^{25} + e^{14}, e^{16} + e^{35}, e^{18} + e^{36}$                                                | 1/162(37, 78, 74, 156, 115, 152, 193, 189, 226)   | {0, 12679, 1578, 25689}                               |                    |
| 95421:52  | $0, 0, 0, 0, e^{12}, e^{25} + e^{13}, e^{15}, e^{26} + e^{35}, e^{28} + e^{14} + e^{36}$                                                 | 1/162(74, 39, 78, 156, 113, 152, 187, 191, 230)   | {0, 12679, 15689, 2578}                               |                    |
| 95421:53  | $0, 0, 0, 0, e^{12}, e^{13} + e^{25}, e^{34} + e^{15}, e^{35} + e^{26}, e^{36} + e^{28} + e^{14}$                                        | 71/673(5, 2, 4, 8, 7, 9, 12, 11, 13)              | {0, 15689}                                            |                    |
| 95421:59a | $0, 0, 0, 0, -e^{12}, e^{15} + e^{23}, e^{14} + e^{25}, e^{16} + e^{35}, e^{18} + e^{24} + e^{36}$                                       | 4/17(1, 2, 2, 4, 3, 4, 5, 5, 6)                   | {0, 12679, 1578, 25689}                               |                    |
| 95421:59b | $0, 0, 0, 0, -e^{12}, e^{23} + e^{15}, -e^{14} + e^{25}, e^{35} + e^{16}, e^{24} + e^{36} + e^{18}$                                      | 4/17(1, 2, 2, 4, 3, 4, 5, 5, 6)                   | {0, 12679, 1578, 25689}                               |                    |
| 95421:72  | $0, 0, 0, 0, e^{12}, e^{13} + e^{25}, e^{15}, e^{14} + e^{26} + e^{35}, e^{28} + e^{36} + e^{45}$                                        | 1/87(37, 23, 46, 69, 60, 83, 97, 106, 129)        | {0, 124679, 15689, 24578}                             |                    |
| 95421:73a | $0, 0, 0, 0, e^{12}, e^{25} + e^{13}, e^{15} + e^{34}, e^{26} + e^{35} + e^{14}, e^{28} + e^{36} + e^{45}$                               | 31/129(2, 1, 2, 3, 3, 4, 5, 5, 6)                 | {0, 124679, 15689, 24578}                             |                    |
| 95421:73b | $0, 0, 0, 0, e^{12}, e^{25} + e^{13}, -e^{15} + e^{34}, e^{14} + e^{26} + e^{35}, e^{45} + e^{28} + e^{36}$                              | 31/129(2, 1, 2, 3, 3, 4, 5, 5, 6)                 | {0, 124679, 15689, 24578}                             |                    |
| 95421:74  | $0, 0, 0, 0, e^{12}, e^{13} + e^{25}, e^{34} + 2e^{15}, e^{35} + e^{26}, e^{37} + e^{56} + e^{18}$                                       | 1/28(13, 6, 12, 20, 19, 25, 32, 31, 44)           | {0, 124679, 1568, 245789}                             |                    |
| 95421:86  | $0, 0, 0, 0, e^{12}, e^{13} + e^{25}, 2e^{15}, e^{14} + e^{26} + e^{35}, e^{37} + e^{56} + e^{18}$                                       | 4/13(1, 1, 2, 3, 2, 3, 3, 4, 5)                   | {0, 124679, 1568, 245789}                             |                    |
| 95421:87a | $0, 0, 0, 0, e^{12}, e^{25} + e^{13}, e^{34} + 2e^{15}, e^{26} + e^{35} + e^{14}, e^{18} + e^{37} + e^{56}$                              | 16/71(2, 1, 2, 3, 3, 4, 5, 5, 7)                  | {0, 124679, 1568, 245789}                             |                    |
| 95421:87b | $0, 0, 0, 0, e^{12}, e^{25} + e^{13}, 2e^{15} + e^{34}, e^{26} + e^{35} - e^{14}, e^{56} + e^{18} + e^{37}$                              | 16/71(2, 1, 2, 3, 3, 4, 5, 5, 7)                  | {0, 124679, 1568, 245789}                             |                    |
| 95421:91  | $0, 0, 0, 0, -e^{12}, e^{15} + e^{23}, e^{25} + e^{14}, e^{16} + e^{24} + e^{35}, e^{18} + e^{27} + e^{36}$                              | 11/81(2, 3, 4, 6, 5, 7, 8, 9, 11)                 | {0, 25689}                                            |                    |
| 95421:95  | $0, 0, 0, 0, -e^{12}, e^{15} + e^{23}, e^{25} - e^{14}, e^{16} + e^{35}, e^{27} + e^{18} + e^{36} + e^{45}$                              | 11/81(2, 3, 4, 6, 5, 7, 8, 9, 11)                 | {0, 25689}                                            |                    |
| 95421:96  | $0, 0, 0, 0, e^{12}, e^{25} + e^{13}, e^{15}, e^{14} + e^{26} + e^{35}, e^{28} + e^{17} + e^{36} + e^{45}$                               | 11/81(3, 2, 4, 6, 5, 7, 8, 9, 11)                 | {0, 15689}                                            |                    |
| 95421:99  | $0, 0, 0, 0, -e^{12} a_1, e^{15} + e^{23}, -(-1 + a_1) e^{14} + e^{25}, e^{16} a_1 + e^{24} + e^{35}, e^{18} + e^{45} + e^{36} + e^{27}$ | 11/81(2, 3, 4, 6, 5, 7, 8, 9, 11)                 | {0, 25689}                                            |                    |
| 95421:103 | $0, 0, 0, 0, e^{12}, e^{15}, e^{25}, e^{17} + e^{26}, e^{18} + e^{34} + e^{56}$                                                          | 1/185(46, 71, 140, 140, 117, 163, 188, 234, 280)  | {0, 123679, 124679, 13579, 14579, 23456, 256, 34}     |                    |

Table A.4 – Continued to next page

Table A.4 – Continued from previous page

| Name       | g                                                                                                          | N                                                   | S <sub>0</sub>                                            | S = S <sub>0</sub> |
|------------|------------------------------------------------------------------------------------------------------------|-----------------------------------------------------|-----------------------------------------------------------|--------------------|
| 95421:104a | $0, 0, 0, 0, -e^{12}, e^{15}, e^{25}, e^{16} + e^{27}, e^{56} + e^{28} + e^{34}$                           | $24/155(2, 2, 5, 5, 4, 6, 6, 8, 10)$                | $\{0, 123679, 124679, 135789, 145789, 234568, 2568, 34\}$ |                    |
| 95421:104b | $0, 0, 0, 0, -e^{12}, -e^{15}, e^{25}, e^{27} + e^{16}, e^{34} + e^{56} + e^{28}$                          | $24/155(2, 2, 5, 5, 4, 6, 6, 8, 10)$                | $\{0, 123679, 124679, 135789, 145789, 234568, 2568, 34\}$ |                    |
| 95421:112  | $0, 0, 0, 0, e^{12}, e^{15}, e^{13} + e^{25}, e^{26} + e^{17}, e^{24} + e^{18} + e^{56}$                   | $1/128(22, 57, 114, 123, 79, 101, 136, 158, 180)$   | $\{0, 12679, 14579, 2456\}$                               |                    |
| 95421:131  | $0, 0, 0, 0, e^{12}, e^{15} + e^{23}, e^{14} + e^{25}, e^{17} + e^{34} + e^{26}, e^{18} + e^{56} + e^{37}$ | $1/11(3, 4, 6, 8, 7, 10, 11, 14, 17)$               | $\{0, 12679, 1579, 256\}$                                 |                    |
| 95321:11   | $0, 0, 0, 0, e^{12}, -e^{13}, e^{15}, e^{34} + e^{17}, e^{46} + e^{18}$                                    | $1/109(16, 87, 76, 59, 103, 92, 119, 135, 151)$     | $\{0, 123479, 12679, 1358, 14568, 2356789, 245789, 346\}$ |                    |
| 95321:20   | $0, 0, 0, 0, -e^{12}, e^{34}, e^{15}, e^{23} + e^{17}, e^{18} + e^{35}$                                    | $1/49(8, 33, 24, 37, 41, 61, 49, 57, 65)$           | $\{0, 123479, 123679, 13458, 13568, 2456789, 25789, 46\}$ |                    |
| 95321:21a  | $0, 0, 0, 0, e^{12}, e^{14} + e^{23}, e^{15}, e^{17} + e^{34}, e^{36} + e^{18}$                            | $1/37(7, 24, 14, 31, 31, 38, 38, 45, 52)$           | $\{0, 123479, 12679, 13568, 1458, 235789, 2456789, 346\}$ | ✓                  |
| 95321:21b  | $0, 0, 0, 0, -e^{12}, e^{14} + e^{23}, e^{15}, e^{17} + e^{34}, e^{18} + e^{36}$                           | $1/37(7, 24, 14, 31, 31, 38, 38, 45, 52)$           | $\{0, 123479, 12679, 13568, 1458, 235789, 2456789, 346\}$ | ✓                  |
| 95321:32   | $0, 0, 0, 0, -e^{12}, e^{13}, e^{15}, e^{24} + e^{17}, e^{45} + e^{18}$                                    | $1/41(8, 25, 37, 24, 33, 45, 41, 49, 57)$           | $\{0, 123479, 124679, 13458, 14568, 2356789, 25789, 36\}$ |                    |
| 95321:33   | $0, 0, 0, 0, e^{12}, e^{13}, e^{25}, e^{14} + e^{27}, e^{45} + e^{28}$                                     | $1/40(20, 9, 30, 27, 29, 50, 38, 47, 56)$           | $\{0, 123479, 124679, 135789, 156789, 234568, 2458, 36\}$ |                    |
| 95321:35   | $0, 0, 0, 0, e^{12}, -e^{13}, e^{15}, e^{34} + e^{17}, e^{18} + e^{46} + e^{23}$                           | $1/119(20, 89, 80, 69, 109, 100, 129, 149, 169)$    | $\{0, 12679, 14568, 245789\}$                             |                    |
| 95321:36   | $0, 0, 0, 0, -e^{12}, e^{34}, e^{15}, e^{23} + e^{17}, e^{57} + e^{28}$                                    | $1/156(32, 69, 96, 108, 101, 204, 133, 165, 234)$   | $\{0, 123479, 123679, 134589, 135689, 245678, 2578, 46\}$ |                    |
| 95321:37   | $0, 0, 0, 0, -e^{12}, e^{34}, e^{15}, e^{17} + e^{23}, e^{18} + e^{46} + e^{35}$                           | $12/193(3, 11, 9, 7, 14, 16, 17, 20, 23)$           | $\{0, 123479, 123679, 46\}$                               |                    |
| 95321:38   | $0, 0, 0, 0, -e^{12}, e^{34}, e^{15}, e^{17}, e^{28} + e^{36} + e^{57}$                                    | $1/60(10, 33, 28, 40, 43, 68, 53, 63, 96)$          | $\{0, 123479, 124679, 134589, 145689, 235678, 2578, 36\}$ |                    |
| 95321:43   | $0, 0, 0, 0, e^{12}, e^{13}, e^{25}, e^{27}, e^{57} + e^{34} + e^{18}$                                     | $1/39(18, 8, 27, 33, 26, 45, 34, 42, 60)$           | $\{0, 12379, 124679, 134578, 15678, 235689, 24589, 346\}$ |                    |
| 95321:44   | $0, 0, 0, 0, -e^{12}, e^{24} + e^{13}, e^{15}, e^{17}, e^{57} + e^{28}$                                    | $1/233(50, 94, 231, 187, 144, 281, 194, 244, 338)$  | $\{0, 123479, 12679, 13589, 145689, 235678, 24578, 346\}$ |                    |
| 95321:50   | $0, 0, 0, 0, -e^{12}, e^{34}, e^{15}, e^{23} + e^{17}, e^{35} + e^{24} + e^{18}$                           | $1/17(3, 11, 9, 12, 14, 21, 17, 20, 23)$            | $\{0, 123679, 13568, 25789\}$                             |                    |
| 95321:51   | $0, 0, 0, 0, e^{12}, e^{13}, e^{15}, e^{23} + e^{17}, e^{26} + e^{18} + e^{34}$                            | $1/221(48, 133, 144, 181, 181, 192, 229, 277, 325)$ | $\{0, 12379, 13458, 245789\}$                             |                    |
| 95321:54   | $0, 0, 0, 0, -e^{12}, e^{13}, e^{15}, e^{17} + e^{24}, e^{28} + e^{57}$                                    | $1/124(32, 45, 108, 96, 77, 140, 109, 141, 186)$    | $\{0, 123479, 124679, 134589, 145689, 235678, 2578, 36\}$ |                    |
| 95321:55   | $0, 0, 0, 0, e^{12}, e^{13}, e^{25}, e^{14} + e^{27}, e^{57} + e^{18}$                                     | $1/39(12, 11, 33, 33, 23, 45, 34, 45, 57)$          | $\{0, 123479, 124679, 13578, 15678, 2345689, 24589, 36\}$ |                    |
| 95321:58a  | $0, 0, 0, 0, e^{12}, -e^{13} + e^{24}, e^{15}, e^{17} + e^{34}, e^{18} + e^{23} + e^{46}$                  | $37/181(1, 3, 4, 2, 4, 5, 5, 6, 7)$                 | $\{0, 12679, 14568, 245789\}$                             | ✓                  |
| 95321:58b  | $0, 0, 0, 0, -e^{12}, -e^{13} + e^{24}, e^{15}, e^{17} + e^{34}, e^{18} + e^{46} + e^{23}$                 | $37/181(1, 3, 4, 2, 4, 5, 5, 6, 7)$                 | $\{0, 12679, 14568, 245789\}$                             | ✓                  |
| 95321:60   | $0, 0, 0, 0, e^{12}, -e^{13}, e^{15}, e^{34} + e^{17}, e^{18} + e^{46} + e^{25}$                           | $1/19(4, 12, 13, 11, 16, 17, 20, 24, 28)$           | $\{0, 123479, 12679, 346\}$                               |                    |
| 95321:62   | $0, 0, 0, 0, -e^{12}, e^{13}, e^{15}, e^{24} + e^{17}, e^{45} + e^{18} + e^{36}$                           | $12/491(9, 25, 26, 27, 34, 35, 43, 52, 61)$         | $\{0, 123479, 124679, 36\}$                               |                    |
| 95321:63a  | $0, 0, 0, 0, e^{12}, e^{13}, e^{25}, e^{27} + e^{14}, e^{28} + e^{36} + e^{45}$                            | $1/4(2, 1, 2, 3, 3, 4, 4, 5, 6)$                    | $\{0, 123479, 124679, 135789, 156789, 234568, 2458, 36\}$ | ✓                  |
| 95321:63b  | $0, 0, 0, 0, e^{12}, -e^{13}, e^{25}, e^{27} + e^{14}, e^{28} + e^{36} + e^{45}$                           | $1/4(2, 1, 2, 3, 3, 4, 4, 5, 6)$                    | $\{0, 123479, 124679, 135789, 156789, 234568, 2458, 36\}$ | ✓                  |
| 95321:64   | $0, 0, 0, 0, e^{12}, -e^{13}, e^{25}, e^{34} + e^{27}, e^{57} + e^{46} + e^{18}$                           | $1/15(6, 4, 9, 9, 10, 15, 14, 18, 24)$              | $\{0, 123479, 12679, 13578, 145678, 235689, 24589, 346\}$ |                    |
| 95321:66a  | $0, 0, 0, 0, -e^{12}, e^{34}, e^{15}, e^{23} + e^{17}, e^{46} + e^{57} + e^{28}$                           | $8/195(5, 12, 15, 12, 17, 27, 22, 27, 39)$          | $\{0, 123479, 123679, 134589, 135689, 245678, 2578, 46\}$ |                    |
| 95321:66b  | $0, 0, 0, 0, -e^{12}, e^{34}, e^{15}, -e^{23} + e^{17}, e^{57} + e^{46} + e^{28}$                          | $8/195(5, 12, 15, 12, 17, 27, 22, 27, 39)$          | $\{0, 123479, 123679, 134589, 135689, 245678, 2578, 46\}$ |                    |
| 95321:72   | $0, 0, 0, 0, -e^{12}, e^{13}, e^{15}, e^{17} + e^{24}, e^{18} + e^{45} + e^{23}$                           | $1/61(13, 35, 52, 39, 48, 65, 61, 74, 87)$          | $\{0, 124679, 14568, 25789\}$                             |                    |
| 95321:78   | $0, 0, 0, 0, -e^{12}, e^{13}, e^{15}, e^{17} + e^{24}, e^{57} + e^{34} + e^{28}$                           | $1/29(7, 12, 24, 21, 19, 31, 26, 33, 45)$           | $\{0, 124679, 145689, 2578\}$                             |                    |
| 95321:79   | $0, 0, 0, 0, e^{12}, e^{13}, e^{25}, e^{27} + e^{14}, e^{34} + e^{57} + e^{18}$                            | $1/183(69, 47, 138, 141, 116, 207, 163, 210, 279)$  | $\{0, 124679, 15678, 24589\}$                             |                    |
| 95321:84   | $0, 0, 0, 0, e^{12}, e^{24} + e^{13}, e^{15}, e^{17}, e^{18} + e^{26} + e^{35}$                            | $1/33(9, 13, 27, 23, 22, 36, 31, 40, 49)$           | $\{0, 123479, 1358, 245789\}$                             |                    |
| 95321:89   | $0, 0, 0, 0, e^{12}, e^{13}, e^{25}, e^{27} + e^{14}, e^{28} + e^{45} + e^{16}$                            | $1/33(13, 9, 23, 27, 22, 36, 31, 40, 49)$           | $\{0, 123479, 135789, 2458\}$                             |                    |
| 95321:90a  | $0, 0, 0, 0, e^{12}, e^{23} + e^{14}, e^{15}, e^{17} + e^{34}, e^{36} + e^{25} + e^{18}$                   | $37/181(1, 3, 2, 4, 4, 5, 5, 6, 7)$                 | $\{0, 123479, 12679, 346\}$                               | ✓                  |
| 95321:90b  | $0, 0, 0, 0, -e^{12}, e^{14} + e^{23}, e^{15}, e^{34} + e^{17}, e^{36} + e^{25} + e^{18}$                  | $37/181(1, 3, 2, 4, 4, 5, 5, 6, 7)$                 | $\{0, 123479, 12679, 346\}$                               | ✓                  |
| 95321:92   | $0, 0, 0, 0, e^{12}, e^{34}, e^{15}, e^{17} + e^{25}, e^{18} + e^{27} + e^{36}$                            | $1/327(81, 162, 134, 218, 243, 352, 324, 405, 486)$ | $\{0, 13568, 158, 36\}$                                   |                    |
| 95321:93a  | $0, 0, 0, 0, -e^{12}, e^{13}, e^{15}, e^{24} + e^{17}, e^{28} + e^{36} + e^{57}$                           | $8/155(5, 8, 13, 15, 13, 18, 18, 23, 31)$           | $\{0, 123479, 124679, 134589, 145689, 235678, 2578, 36\}$ |                    |
| 95321:93b  | $0, 0, 0, 0, -e^{12}, -e^{13}, e^{15}, e^{17} + e^{24}, e^{57} + e^{28} + e^{36}$                          | $8/155(5, 8, 13, 15, 13, 18, 18, 23, 31)$           | $\{0, 123479, 124679, 134589, 145689, 235678, 2578, 36\}$ |                    |
| 95321:94   | $0, 0, 0, 0, e^{12}, e^{13}, e^{25}, e^{14} + e^{27}, e^{57} + e^{36} + e^{18}$                            | $8/225(10, 8, 17, 24, 18, 27, 26, 34, 44)$          | $\{0, 123479, 124679, 36\}$                               |                    |
| 95321:96   | $0, 0, 0, 0, -e^{12}, e^{34}, e^{15}, e^{17} + e^{25}, e^{36} + e^{28} + e^{57}$                           | $2/771(87, 174, 176, 257, 261, 433, 348, 435, 609)$ | $\{0, 134589, 145689, 36\}$                               |                    |
| 95321:99   | $0, 0, 0, 0, e^{12}, e^{13}, e^{25}, e^{27} + e^{15}, e^{17} + e^{28} + e^{34}$                            | $1/29(14, 7, 19, 23, 21, 33, 28, 35, 42)$           | $\{0, 234568, 258, 346\}$                                 |                    |
| 95321:109  | $0, 0, 0, 0, -e^{12}, e^{13}, e^{15}, e^{17} + e^{25}, e^{28} + e^{57} + e^{34}$                           | $1/213(48, 96, 167, 169, 144, 215, 192, 240, 336)$  | $\{0, 13589, 145689, 346\}$                               |                    |
| 95321:110  | $0, 0, 0, 0, e^{12}, e^{13}, e^{25}, e^{27} + e^{15}, e^{34} + e^{57} + e^{18}$                            | $1/223(98, 49, 156, 187, 147, 254, 196, 245, 343)$  | $\{0, 235689, 24589, 346\}$                               |                    |
| 95321:116  | $0, 0, 0, 0, (-1 + a_2)e^{12}, e^{24} + a_2e^{13}, e^{15}, e^{23} + e^{17}, e^{26} + e^{18} + e^{35}$      | $1/33(9, 13, 27, 23, 22, 36, 31, 40, 49)$           | $\{0, 123479, 1358, 245789\}$                             |                    |
| 95321:120  | $0, 0, 0, 0, -e^{12}, e^{34}, e^{15} + e^{23}, e^{17} + e^{35}, e^{18} + e^{37}$                           | $1/17(3, 11, 6, 14, 14, 20, 17, 20, 23)$            | $\{0, 124679, 1279, 14568, 158, 2456789, 25789, 46\}$     |                    |
| 95321:124  | $0, 0, 0, 0, e^{12}, -e^{13}, e^{15}, e^{25} + e^{34} + e^{17}, e^{27} + e^{18} + e^{46}$                  | $1/67(17, 34, 45, 40, 51, 62, 68, 85, 102)$         | $\{0, 1358, 14568, 346\}$                                 |                    |

Table A.4 – Continued to next page

Table A.4 – Continued from previous page

| Name       | g                                                                                                                            | N                                                    | S <sub>0</sub>                                                    | S = S <sub>0</sub> |
|------------|------------------------------------------------------------------------------------------------------------------------------|------------------------------------------------------|-------------------------------------------------------------------|--------------------|
| 95321:134  | $0, 0, 0, 0, -e^{12}, e^{13}, e^{15} + e^{24}, e^{17} + e^{45}, e^{18} + e^{47}$                                             | $1/31(6, 19, 28, 12, 25, 34, 31, 37, 43)$            | $\{\emptyset, 12379, 12679, 1358, 1568, 2356789, 25789, 36\}$     |                    |
| 95321:135  | $0, 0, 0, 0, e^{12}, e^{13}, e^{25} + e^{14}, e^{27} + e^{45}, e^{28} + e^{47}$                                              | $1/185(90, 43, 140, 86, 133, 230, 176, 219, 262)$    | $\{\emptyset, 12379, 12679, 135789, 156789, 23568, 258, 36\}$     |                    |
| 95321:144  | $0, 0, 0, 0, -e^{12}, e^{34}, e^{15} + e^{23}, e^{35} + e^{17}, e^{46} + e^{37} + e^{18}$                                    | $1/207(43, 132, 86, 109, 175, 195, 218, 261, 304)$   | $\{\emptyset, 14568, 158, 46\}$                                   |                    |
| 95321:145a | $0, 0, 0, 0, e^{12}, e^{23} + e^{14}, e^{15}, e^{34} + e^{25} + e^{17}, e^{27} + e^{36} + e^{18}$                            | $1/4(1, 2, 2, 3, 3, 4, 4, 5, 6)$                     | $\{\emptyset, 13568, 1458, 346\}$                                 |                    |
| 95321:145b | $0, 0, 0, 0, -e^{12}, e^{23} + e^{14}, e^{15}, e^{17} + e^{25} + e^{34}, e^{36} + e^{27} + e^{18}$                           | $1/4(1, 2, 2, 3, 3, 4, 4, 5, 6)$                     | $\{\emptyset, 13568, 1458, 346\}$                                 |                    |
| 95321:149  | $0, 0, 0, 0, -e^{12}, e^{34}, e^{15} + e^{23}, e^{17} + e^{35}, e^{24} + e^{37} + e^{18}$                                    | $1/67(13, 41, 26, 52, 54, 78, 67, 80, 93)$           | $\{\emptyset, 1279, 158, 25789\}$                                 |                    |
| 95321:156  | $0, 0, 0, 0, -e^{12}, e^{13}, e^{15} + e^{24}, e^{17} + e^{45}, e^{18} + e^{47} + e^{36}$                                    | $1/381(86, 228, 243, 172, 314, 329, 400, 486, 572)$  | $\{\emptyset, 12379, 12679, 36\}$                                 |                    |
| 95321:157a | $0, 0, 0, 0, e^{12}, e^{13}, e^{14} + e^{25}, e^{27} + e^{45}, e^{28} + e^{36} + e^{47}$                                     | $1/19(9, 5, 10, 10, 14, 19, 19, 24, 29)$             | $\{\emptyset, 12379, 12679, 135789, 156789, 23568, 258, 36\}$     |                    |
| 95321:157b | $0, 0, 0, 0, e^{12}, -e^{13}, e^{25} + e^{14}, e^{27} + e^{45}, e^{28} + e^{47} + e^{36}$                                    | $1/19(9, 5, 10, 10, 14, 19, 19, 24, 29)$             | $\{\emptyset, 12379, 12679, 135789, 156789, 23568, 258, 36\}$     |                    |
| 95321:163  | $0, 0, 0, 0, -e^{12}, e^{13}, e^{15} + e^{24}, e^{17} + e^{45}, e^{18} + e^{23} + e^{47}$                                    | $1/14(3, 8, 12, 6, 11, 15, 14, 17, 20)$              | $\{\emptyset, 12679, 1568, 25789\}$                               |                    |
| 95321:172  | $0, 0, 0, 0, -e^{12}, e^{34}, e^{23} + e^{15}, e^{35} + e^{17}, e^{37} + e^{25} + e^{18}$                                    | $1/71(14, 42, 28, 57, 56, 85, 70, 84, 98)$           | $\{\emptyset, 124679, 1279, 46\}$                                 |                    |
| 95321:173  | $0, 0, 0, 0, e^{12}, e^{13}, e^{25} + e^{14}, e^{45} + e^{27}, e^{28} + e^{47} + e^{16}$                                     | $1/183(71, 51, 133, 102, 122, 204, 173, 224, 275)$   | $\{\emptyset, 12379, 135789, 258\}$                               |                    |
| 95321:180  | $0, 0, 0, 0, -e^{12}, e^{34}, e^{15} + e^{23}, e^{17} + e^{35} + e^{24}, e^{18} + e^{37} + e^{45}$                           | $1/49(11, 27, 22, 33, 38, 55, 49, 60, 71)$           | $\{\emptyset, 124679, 14568, 25789\}$                             |                    |
| 95321:183  | $0, 0, 0, 0, e^{12}, e^{13}, e^{25}, e^{16} + e^{27}, e^{57} + e^{18} + e^{34}$                                              | $8/225(8, 9, 19, 24, 17, 27, 26, 35, 43)$            | $\{\emptyset, 124679, 134578, 235689\}$                           |                    |
| 95321:188  | $0, 0, 0, 0, -e^{12}, e^{13}, e^{15} + e^{24}, e^{17} + e^{45}, e^{18} + e^{25} + e^{47}$                                    | $1/281(56, 168, 253, 112, 224, 309, 280, 336, 392)$  | $\{\emptyset, 12379, 12679, 36\}$                                 |                    |
| 95321:194  | $0, 0, 0, 0, e^{12}, -e^{13}, e^{25}, e^{27} + e^{16} + e^{34}, e^{57} + e^{46} + e^{18}$                                    | $1/93(30, 29, 57, 60, 59, 87, 88, 117, 147)$         | $\{\emptyset, 12679, 13578, 235689\}$                             |                    |
| 95321:201  | $0, 0, 0, 0, -e^{12}, e^{13}, e^{15} + e^{24}, e^{17} + e^{45} + e^{23}, e^{18} + e^{47} + e^{26}$                           | $1/4(1, 2, 3, 2, 3, 4, 4, 5, 6)$                     | $\{\emptyset, 12379, 1358, 25789\}$                               |                    |
| 95321:204  | $0, 0, 0, 0, -e^{12}, e^{34}, e^{15} + e^{23}, e^{35} + e^{17}, e^{37} + e^{46} + e^{18} + e^{25}$                           | $35/333(2, 6, 4, 5, 8, 9, 10, 12, 14)$               | $\{\emptyset, 46\}$                                               |                    |
| 95321:226  | $0, 0, 0, 0, -e^{12}, -e^{13}, e^{15} + e^{24}, e^{17} + e^{45}, e^{26} + e^{47} + e^{18} + e^{35}$                          | $1/4(1, 2, 3, 2, 3, 4, 4, 5, 6)$                     | $\{\emptyset, 12379, 1358, 25789\}$                               |                    |
| 95321:237  | $0, 0, 0, 0, -e^{12}, -2e^{13}, -e^{23} + e^{15}, e^{35} + e^{17} + e^{26}, e^{57} + e^{28} + e^{34}$                        | $4/13(1, 1, 2, 3, 2, 3, 3, 4, 5)$                    | $\{\emptyset, 124679, 145689, 2578\}$                             |                    |
| 95321:240  | $0, 0, 0, 0, -a_4e^{12}, -e^{13}(-1 + a_4), e^{24} + e^{15}, a_4e^{17} + e^{23} + e^{45}, e^{26} + e^{35} + e^{18} + e^{47}$ | $1/4(1, 2, 3, 2, 3, 4, 4, 5, 6)$                     | $\{\emptyset, 12379, 1358, 25789\}$                               |                    |
| 95321:254  | $0, 0, 0, 0, e^{12}, e^{14} + e^{23}, -e^{13} + e^{25}, e^{27} + e^{35} - 2e^{16}, e^{18} + e^{57}$                          | $1/333(68, 117, 234, 283, 185, 351, 302, 419, 487)$  | $\{\emptyset, 12679, 14578, 245689\}$                             |                    |
| 95321:258  | $0, 0, 0, 0, e^{12}, e^{14} + e^{23}, -e^{13} + e^{25}, -2e^{16} + e^{27} + e^{35}, e^{57} + e^{18} + e^{34}$                | $32/279(2, 3, 6, 7, 5, 9, 8, 11, 13)$                | $\{\emptyset, 245689\}$                                           |                    |
| 9542:8     | $0, 0, 0, 0, e^{12}, e^{15}, e^{25}, e^{16}, e^{17} + e^{26} + e^{34}$                                                       | $1/28(7, 13, 20, 20, 20, 27, 33, 34, 40)$            | $\{\emptyset, 123467, 1267, 134578, 1578, 234568, 2568, 34\}$     |                    |
| 9542:9     | $0, 0, 0, 0, e^{12}, e^{15}, e^{25}, e^{16} + e^{34}, e^{17} + e^{26}$                                                       | $1/124(41, 45, 84, 84, 86, 127, 131, 168, 172)$      | $\{\emptyset, 123467, 1267, 13578, 14578, 23568, 24568, 34\}$     |                    |
| 9542:15    | $0, 0, 0, 0, e^{12}, e^{15}, e^{25} + e^{13}, e^{34} + e^{16}, e^{35} + e^{27}$                                              | $1/127(46, 41, 82, 97, 87, 133, 128, 179, 169)$      | $\{\emptyset, 1267, 145789, 245689\}$                             |                    |
| 9542:16a   | $0, 0, 0, 0, e^{12}, e^{15}, e^{25}, e^{27} + e^{16}, e^{17} + e^{26} + e^{34}$                                              | $11/32(1, 1, 2, 2, 2, 3, 3, 4, 4)$                   | $\{\emptyset, 123467, 1267, 134578, 1578, 234568, 2568, 34\}$     | ✓                  |
| 9542:16b   | $0, 0, 0, 0, e^{12}, e^{15}, e^{25}, e^{27} - e^{16}, e^{26} + e^{34} + e^{17}$                                              | $11/32(1, 1, 2, 2, 2, 3, 3, 4, 4)$                   | $\{\emptyset, 123467, 1267, 134578, 1578, 234568, 2568, 34\}$     | ✓                  |
| 9542:17a   | $0, 0, 0, 0, e^{12}, e^{15}, e^{25}, e^{17} + e^{26}, e^{27} + e^{34} + e^{16}$                                              | $11/32(1, 1, 2, 2, 2, 3, 3, 4, 4)$                   | $\{\emptyset, 123467, 1267, 13579, 14579, 23569, 24569, 34\}$     | ✓                  |
| 9542:17b   | $0, 0, 0, 0, e^{12}, -e^{15}, e^{25}, e^{26} - e^{17}, e^{27} + e^{34} + e^{16}$                                             | $11/32(1, 1, 2, 2, 2, 3, 3, 4, 4)$                   | $\{\emptyset, 123467, 1267, 13579, 14579, 23569, 24569, 34\}$     | ✓                  |
| 9542:20    | $0, 0, 0, 0, e^{12}, e^{15}, e^{25} + e^{13}, e^{16} + e^{24}, e^{27} + e^{35}$                                              | $1/425(131, 154, 308, 393, 285, 416, 439, 547, 593)$ | $\{\emptyset, 12467, 145789, 25689\}$                             |                    |
| 9542:24    | $0, 0, 0, 0, e^{12}, e^{15}, e^{13} + e^{25}, e^{24} + e^{16}, e^{17} + e^{26}$                                              | $1/160(44, 67, 134, 132, 111, 155, 178, 199, 222)$   | $\{\emptyset, 12467, 14578, 2568\}$                               |                    |
| 9542:31    | $0, 0, 0, 0, e^{12}, e^{13} + e^{25}, e^{15}, e^{35} + e^{26}, e^{34} + e^{27} + e^{16}$                                     | $1/10(4, 3, 6, 8, 7, 10, 11, 13, 14)$                | $\{\emptyset, 1267, 1568, 2578\}$                                 |                    |
| 9542:34    | $0, 0, 0, 0, -e^{12}, e^{23} + e^{15}, -e^{14} + e^{25}, e^{35} + e^{16}, e^{45} + e^{27}$                                   | $11/32(1, 1, 2, 2, 2, 3, 3, 4, 4)$                   | $\{\emptyset, 1267, 15789, 25689\}$                               |                    |
| 9542:39    | $0, 0, 0, 0, -e^{12}, e^{15} + e^{23}, e^{25} + e^{14}, e^{16} + e^{35}, e^{17} + e^{26}$                                    | $1/10(3, 4, 6, 8, 7, 10, 11, 13, 14)$                | $\{\emptyset, 1267, 1578, 2568\}$                                 |                    |
| 9542:45    | $0, 0, 0, 0, -e^{12}, e^{15} + e^{23}, a_3e^{14} + e^{25}, e^{16} + e^{35}, e^{17} + e^{26} + e^{34}$                        | $1/10(3, 4, 6, 8, 7, 10, 11, 13, 14)$                | $\{\emptyset, 1267, 1578, 2568\}$                                 |                    |
| 9531:99    | $0, 0, 0, 0, e^{12}, e^{13}, e^{15}, e^{26} + e^{35}, e^{17} + e^{34}$                                                       | $1/109(30, 59, 62, 87, 89, 92, 119, 151, 149)$       | $\{\emptyset, 123478, 1267, 1359, 145689, 235679, 245789, 3468\}$ |                    |
| 9531:101   | $0, 0, 0, 0, e^{12}, e^{13}, e^{25}, e^{35} + e^{26}, e^{34} + e^{27}$                                                       | $1/69(40, 17, 33, 58, 57, 73, 74, 90, 91)$           | $\{\emptyset, 123478, 1267, 13579, 1456789, 23569, 24589, 3468\}$ |                    |
| 9531:106   | $0, 0, 0, 0, e^{12}, e^{13}, e^{25}, e^{26} + e^{35} + e^{14}, e^{27}$                                                       | $1/8(4, 2, 5, 7, 6, 9, 8, 11, 10)$                   | $\{\emptyset, 12378, 12467, 134579, 156789, 23569, 24589, 3468\}$ |                    |
| 9531:119   | $0, 0, 0, 0, e^{12}, e^{34}, e^{13} + e^{25}, e^{15}, e^{27} + e^{35}$                                                       | $1/28(13, 8, 16, 20, 21, 36, 29, 34, 37)$            | $\{\emptyset, 124678, 1278, 145679, 1579, 245689, 2589, 46\}$     |                    |
| 9531:121   | $0, 0, 0, 0, e^{12}, -e^{13}, e^{34} + e^{15}, e^{36}, e^{17} + e^{46}$                                                      | $1/49(10, 38, 25, 33, 48, 35, 58, 60, 68)$           | $\{\emptyset, 12378, 124678, 134589, 15689, 235679, 24579, 346\}$ |                    |
| 9531:138   | $0, 0, 0, 0, e^{12}, e^{13}, e^{15}, e^{26} + e^{35}, e^{17} + e^{24}$                                                       | $1/225(64, 106, 147, 192, 170, 211, 234, 317, 298)$  | $\{\emptyset, 123478, 12467, 13459, 145689, 235679, 25789, 368\}$ |                    |
| 9531:140   | $0, 0, 0, 0, e^{12}, e^{13}, e^{25}, e^{26} + e^{35}, e^{14} + e^{27}$                                                       | $1/225(106, 64, 133, 192, 170, 239, 234, 303, 298)$  | $\{\emptyset, 123478, 12467, 13579, 156789, 234569, 24589, 368\}$ |                    |
| 9531:164   | $0, 0, 0, 0, e^{12}, e^{13}, e^{25}, e^{14} + e^{35} + e^{26}, e^{34} + e^{27}$                                              | $1/81(44, 21, 43, 64, 65, 87, 86, 108, 107)$         | $\{\emptyset, 23569, 24589, 3468\}$                               |                    |
| 9531:171   | $0, 0, 0, 0, e^{12}, e^{13}, e^{14} + e^{25}, e^{15}, e^{45} + e^{27}$                                                       | $1/106(40, 37, 86, 74, 77, 126, 114, 117, 151)$      | $\{\emptyset, 12378, 12678, 13579, 15679, 235689, 2589, 36\}$     |                    |
| 9531:172   | $0, 0, 0, 0, -e^{12}, e^{13}, e^{24} + e^{15}, e^{25}, e^{17} + e^{45}$                                                      | $1/100(32, 43, 84, 64, 75, 116, 107, 118, 139)$      | $\{\emptyset, 12378, 12678, 13589, 15689, 235679, 2579, 36\}$     |                    |

Table A.4 – Continued to next page

Table A.4 – Continued from previous page

| Name      | g                                                                                        | N                                                  | S <sub>0</sub>                                        | S = S <sub>0</sub> |
|-----------|------------------------------------------------------------------------------------------|----------------------------------------------------|-------------------------------------------------------|--------------------|
| 9531:175  | $0, 0, 0, 0, e^{12}, -e^{13}, e^{34} + e^{15}, e^{16}, e^{17} + e^{46}$                  | 1/179(37, 143, 116, 101, 180, 153, 217, 190, 254)  | {0, 12378, 12467, 134589, 1569, 2356789, 24579, 3468} |                    |
| 9531:177  | $0, 0, 0, 0, -e^{12}, e^{34}, e^{15} + e^{23}, e^{46}, e^{17} + e^{35}$                  | 1/24(6, 15, 12, 10, 21, 22, 27, 32, 33)            | {0, 12467, 127, 14569, 159, 245679, 2579, 46}         |                    |
| 9531:178  | $0, 0, 0, 0, e^{12}, e^{13}, e^{14} + e^{25}, e^{15} + e^{34}, e^{45} + e^{27}$          | 1/453(218, 135, 301, 270, 353, 519, 488, 571, 623) | {0, 12378, 15679, 235689}                             |                    |
| 9531:179  | $0, 0, 0, 0, -e^{12}, e^{13}, e^{15} + e^{24}, e^{34} + e^{25}, e^{45} + e^{17}$         | 1/25(7, 13, 19, 14, 20, 26, 27, 33, 34)            | {0, 12378, 13589, 2579}                               |                    |
| 9531:181  | $0, 0, 0, 0, e^{12}, e^{13}, e^{23} + e^{15}, e^{36}, e^{17} + e^{26} + e^{34}$          | 1/221(55, 144, 110, 199, 199, 165, 254, 275, 309)  | {0, 12678, 145689, 24579}                             |                    |
| 9531:184  | $0, 0, 0, 0, e^{12}, e^{13}, e^{23} + e^{15}, e^{36} + e^{24}, e^{17} + e^{26}$          | 1/389(107, 212, 214, 323, 319, 321, 426, 535, 533) | {0, 12678, 145689, 24579}                             |                    |
| 9531:187  | $0, 0, 0, 0, e^{12}, e^{13}, e^{25}, e^{14} + e^{26} + e^{35}, e^{36} + e^{27}$          | 3/92(14, 10, 15, 25, 24, 29, 34, 39, 44)           | {0, 134579, 156789, 3468}                             |                    |
| 9531:192  | $0, 0, 0, 0, -e^{12}, e^{13}, e^{15} + e^{23}, e^{36} + e^{24}, e^{35} + e^{17}$         | 1/389(107, 212, 214, 323, 319, 321, 426, 535, 533) | {0, 12678, 145689, 24579}                             |                    |
| 9531:194  | $0, 0, 0, 0, e^{12}, -e^{13}, e^{15} + e^{34}, e^{24} + e^{36}, e^{17} + e^{46}$         | 1/489(109, 346, 267, 297, 455, 376, 564, 643, 673) | {0, 12378, 134589, 24579}                             |                    |
| 9531:219  | $0, 0, 0, 0, -e^{12}, e^{23} + e^{14}, e^{15}, e^{35} + e^{16}, e^{17}$                  | 1/179(37, 104, 101, 168, 141, 205, 178, 242, 215)  | {0, 123478, 1267, 13569, 14589, 23579, 2456789, 3468} |                    |
| 9531:220  | $0, 0, 0, 0, e^{12}, e^{24} + e^{13}, e^{15}, e^{35} + e^{26}, e^{17}$                   | 2/39(6, 7, 15, 14, 13, 21, 19, 28, 25)             | {0, 123478, 1267, 1359, 145689, 235679, 245789, 3468} |                    |
| 9531:241  | $0, 0, 0, 0, e^{12}, -e^{13}, e^{15} + e^{34}, e^{25}, e^{17} + e^{46}$                  | 1/257(82, 126, 155, 135, 208, 237, 290, 334, 372)  | {0, 12378, 124678, 134589, 15689, 235679, 24579, 346} |                    |
| 9531:242  | $0, 0, 0, 0, -e^{12}, e^{13}, e^{24} + e^{15}, e^{36}, e^{17} + e^{45}$                  | 1/21(6, 12, 11, 12, 18, 17, 24, 28, 30)            | {0, 12378, 12678, 13589, 15689, 235679, 2579, 36}     |                    |
| 9531:243  | $0, 0, 0, 0, e^{12}, e^{13}, e^{25} + e^{14}, e^{36}, e^{27} + e^{45}$                   | 1/9(4, 3, 4, 6, 7, 8, 10, 12, 13)                  | {0, 12378, 12678, 135789, 156789, 23569, 259, 36}     |                    |
| 9531:244  | $0, 0, 0, 0, e^{12}, e^{13}, e^{14} + e^{25}, e^{15} + e^{23}, e^{45} + e^{27}$          | 1/178(70, 61, 140, 122, 131, 210, 192, 201, 253)   | {0, 12678, 15679, 2589}                               |                    |
| 9531:247  | $0, 0, 0, 0, e^{12}, e^{13}, e^{23} + e^{15}, e^{16}, e^{17} + e^{26} + e^{34}$          | 1/88(25, 53, 50, 78, 78, 75, 103, 100, 128)        | {0, 1267, 14569, 24579}                               |                    |
| 9531:249  | $0, 0, 0, 0, e^{12}, e^{13}, e^{15}, e^{35} + e^{26}, e^{17} + e^{36} + e^{24}$          | 1/75(22, 38, 41, 66, 60, 63, 82, 101, 104)         | {0, 13459, 145689, 368}                               |                    |
| 9531:251  | $0, 0, 0, 0, e^{12}, e^{13}, e^{25}, e^{26} + e^{35}, e^{14} + e^{27} + e^{36}$          | 1/217(107, 66, 99, 198, 173, 206, 239, 272, 305)   | {0, 13579, 156789, 368}                               |                    |
| 9531:252  | $0, 0, 0, 0, e^{12}, e^{13}, e^{25}, e^{26} + e^{35}, e^{27} + e^{16} + e^{34}$          | 1/216(97, 69, 110, 194, 166, 207, 235, 276, 304)   | {0, 1267, 13579, 23569}                               |                    |
| 9531:254  | $0, 0, 0, 0, e^{12}, e^{13}, e^{25}, e^{14} + e^{26} + e^{35}, e^{16} + e^{27}$          | 1/389(151, 128, 233, 361, 279, 384, 407, 512, 535) | {0, 12467, 134579, 23569}                             |                    |
| 9531:259  | $0, 0, 0, 0, e^{12}, e^{13}, e^{23} + e^{15}, e^{34} + e^{25}, e^{17} + e^{26}$          | 2/27(4, 7, 8, 10, 11, 12, 15, 18, 19)              | {0, 124678, 145689, 2579}                             |                    |
| 9531:260  | $0, 0, 0, 0, -e^{12}, e^{13}, e^{15} + e^{23}, e^{36}, e^{17} + e^{35} + e^{24}$         | 2/53(7, 16, 14, 21, 23, 21, 30, 35, 37)            | {0, 124678, 145689, 2579}                             |                    |
| 9531:261  | $0, 0, 0, 0, -e^{12}, e^{13}, e^{15} + e^{23}, e^{16} + e^{24}, e^{17} + e^{35}$         | 1/148(47, 70, 94, 118, 117, 141, 164, 188, 211)    | {0, 12467, 1569, 24579}                               |                    |
| 9531:265  | $0, 0, 0, 0, e^{12}, e^{13}, e^{15}, e^{24} + e^{36}, e^{35} + e^{17} + e^{26}$          | 1/389(107, 212, 214, 323, 319, 321, 426, 535, 533) | {0, 12678, 145689, 24579}                             |                    |
| 9531:269a | $0, 0, 0, 0, e^{12}, -e^{13}, e^{15} + e^{34}, e^{16} + e^{24}, e^{46} + e^{17}$         | 1/29(7, 20, 20, 14, 27, 27, 34, 34, 41)            | {0, 12378, 12467, 134589, 1569, 2356789, 24579, 3468} | ✓                  |
| 9531:269b | $0, 0, 0, 0, -e^{12}, -e^{13}, e^{15} + e^{34}, e^{16} + e^{24}, e^{17} + e^{46}$        | 1/29(7, 20, 20, 14, 27, 27, 34, 34, 41)            | {0, 12378, 12467, 134589, 1569, 2356789, 24579, 3468} | ✓                  |
| 9531:272  | $0, 0, 0, 0, e^{12}, e^{34}, e^{25} + e^{13}, e^{36} + e^{14}, e^{35} + e^{27}$          | 1/139(100, 25, 50, 89, 125, 139, 150, 189, 175)    | {0, 245689, 259, 468}                                 |                    |
| 9531:276a | $0, 0, 0, 0, e^{12}, e^{13}, e^{15} + e^{23}, e^{24} + e^{36}, e^{26} + e^{17} + e^{34}$ | 14/51(1, 2, 2, 3, 3, 3, 4, 5, 5)                   | {0, 12678, 145689, 24579}                             |                    |
| 9531:276b | $0, 0, 0, 0, e^{12}, e^{13}, e^{23} + e^{15}, e^{36} - e^{24}, e^{17} + e^{26} + e^{34}$ | 14/51(1, 2, 2, 3, 3, 3, 4, 5, 5)                   | {0, 12678, 145689, 24579}                             |                    |
| 9531:280a | $0, 0, 0, 0, e^{12}, -e^{13}, e^{15} + e^{34}, e^{36} + e^{25}, e^{17} + e^{46}$         | 1/129(38, 69, 69, 76, 107, 107, 145, 176, 183)     | {0, 12378, 124678, 134589, 15689, 235679, 24579, 346} |                    |
| 9531:280b | $0, 0, 0, 0, -e^{12}, -e^{13}, e^{34} + e^{15}, e^{36} + e^{25}, e^{46} + e^{17}$        | 1/129(38, 69, 69, 76, 107, 107, 145, 176, 183)     | {0, 12378, 124678, 134589, 15689, 235679, 24579, 346} |                    |
| 9531:281  | $0, 0, 0, 0, -e^{12}, -e^{13}, e^{34} + e^{15}, e^{35} + e^{26}, e^{46} + e^{17}$        | 1/30(8, 18, 15, 19, 26, 23, 34, 41, 42)            | {0, 12378, 12467, 13459, 15689, 235679, 245789, 3468} |                    |
| 9531:285  | $0, 0, 0, 0, a_1 e^{12}, e^{13}, e^{25}, e^{24} + e^{15}, e^{27} + e^{16} + e^{34}$      | 7/139(8, 7, 13, 16, 15, 21, 22, 23, 29)            | {0, 12678, 13579, 235689}                             |                    |
| 9531:291  | $0, 0, 0, 0, e^{12}, a_1 e^{13}, e^{15}, e^{16} + e^{23}, e^{25} + e^{34} + e^{17}$      | 1/14(4, 8, 9, 11, 12, 13, 16, 17, 20)              | {0, 13589, 14569, 3468}                               |                    |
| 9531:296  | $0, 0, 0, 0, e^{12}, e^{13}, e^{14} + e^{25}, e^{16}, e^{27} + e^{45}$                   | 1/39(11, 15, 28, 30, 26, 39, 41, 50, 56)           | {0, 12378, 1267, 135789, 15679, 235689, 259, 368}     |                    |
| 9531:299a | $0, 0, 0, 0, -e^{12}, e^{14} + e^{23}, e^{15}, e^{16} + e^{35}, e^{17} + e^{34}$         | 1/29(7, 17, 14, 24, 24, 31, 31, 38, 38)            | {0, 123478, 1267, 13569, 14589, 23579, 2456789, 3468} | ✓                  |
| 9531:299b | $0, 0, 0, 0, -e^{12}, -e^{14} + e^{23}, e^{15}, e^{16} + e^{35}, e^{17} + e^{34}$        | 1/29(7, 17, 14, 24, 24, 31, 31, 38, 38)            | {0, 123478, 1267, 13569, 14589, 23579, 2456789, 3468} | ✓                  |
| 9531:300a | $0, 0, 0, 0, e^{12}, e^{13} + e^{24}, e^{15}, e^{35} + e^{26}, e^{17} + e^{34}$          | 2/37(6, 7, 13, 12, 13, 19, 19, 26, 25)             | {0, 123478, 1267, 1359, 145689, 235679, 245789, 3468} | ✓                  |
| 9531:300b | $0, 0, 0, 0, e^{12}, e^{24} + e^{13}, -e^{15}, e^{35} + e^{26}, e^{17} + e^{34}$         | 2/37(6, 7, 13, 12, 13, 19, 19, 26, 25)             | {0, 123478, 1267, 1359, 145689, 235679, 245789, 3468} | ✓                  |
| 9531:308  | $0, 0, 0, 0, e^{12}, e^{13}, e^{15} + e^{23}, e^{25}, e^{17} + e^{26} + e^{34}$          | 1/9(3, 4, 6, 7, 9, 10, 11, 13)                     | {0, 12678, 145689, 24579}                             |                    |
| 9531:309  | $0, 0, 0, 0, e^{12}, e^{13}, e^{15} + e^{23}, e^{14} + e^{25}, e^{17} + e^{26}$          | 1/71(23, 32, 46, 64, 55, 69, 78, 87, 101)          | {0, 12678, 15689, 2579}                               |                    |
| 9531:310  | $0, 0, 0, 0, -e^{12}, e^{13}, e^{15} + e^{23}, e^{16}, e^{17} + e^{24} + e^{35}$         | 1/88(26, 49, 52, 78, 75, 78, 101, 104, 127)        | {0, 12467, 14569, 2579}                               |                    |
| 9531:312  | $0, 0, 0, 0, e^{12}, e^{13}, e^{15}, e^{24} + e^{16}, e^{35} + e^{26} + e^{17}$          | 1/148(47, 70, 94, 118, 117, 141, 164, 188, 211)    | {0, 12467, 1569, 24579}                               |                    |
| 9531:315  | $0, 0, 0, 0, e^{12}, e^{13}, e^{25}, e^{26} + e^{35}, e^{34} + e^{27} + e^{15}$          | 1/186(100, 50, 93, 157, 150, 193, 200, 243, 250)   | {0, 23569, 24589, 3468}                               |                    |
| 9531:318  | $0, 0, 0, 0, e^{12}, -e^{13}, e^{15} + e^{34}, e^{16}, e^{17} + e^{46} + e^{23}$         | 1/61(13, 48, 39, 35, 61, 52, 74, 65, 87)           | {0, 12378, 134589, 24579}                             |                    |
| 9531:321  | $0, 0, 0, 0, e^{12}, e^{13}, e^{15}, e^{25} + e^{34}, e^{17} + e^{26} + e^{35}$          | 2/27(4, 7, 8, 10, 11, 12, 15, 18, 19)              | {0, 124678, 145689, 2579}                             |                    |
| 9531:333  | $0, 0, 0, 0, e^{12}, e^{13}, e^{25}, e^{35} + e^{14} + e^{26}, e^{27} + e^{16} + e^{34}$ | 71/657(4, 3, 5, 8, 7, 9, 10, 12, 13)               | {0, 23569}                                            |                    |

Table A.4 – Continued to next page

Table A.4 – Continued from previous page

| Name      | g                                                                                                     | N                                                    | S <sub>0</sub>                                                | S = S <sub>0</sub> |
|-----------|-------------------------------------------------------------------------------------------------------|------------------------------------------------------|---------------------------------------------------------------|--------------------|
| 9531:335  | $0, 0, 0, 0, -e^{12}, e^{13}a_2, e^{15} + e^{24}, e^{34} + e^{16}, e^{45} + e^{17}$                   | $1/8(2, 5, 6, 4, 7, 8, 9, 10, 11)$                   | $\{\emptyset, 12378, 1267, 13589, 1569, 2356789, 2579, 368\}$ |                    |
| 9531:336a | $0, 0, 0, 0, e^{12}, e^{13}, e^{25} + e^{14}, e^{16} + e^{34}, e^{27} + e^{45}$                       | $1/37(13, 13, 24, 26, 26, 37, 39, 50, 52)$           | $\{\emptyset, 12378, 1267, 135789, 15679, 235689, 259, 368\}$ | ✓                  |
| 9531:336b | $0, 0, 0, 0, e^{12}, -e^{13}, e^{14} + e^{25}, e^{16} + e^{34}, e^{45} + e^{27}$                      | $1/37(13, 13, 24, 26, 26, 37, 39, 50, 52)$           | $\{\emptyset, 12378, 1267, 135789, 15679, 235689, 259, 368\}$ | ✓                  |
| 9531:347  | $0, 0, 0, 0, e^{12}, e^{14} + e^{23}, e^{15} + e^{34}, e^{25}, e^{17} + e^{36}$                       | $1/215(70, 102, 105, 137, 172, 207, 242, 274, 312)$  | $\{\emptyset, 23579, 245679, 346\}$                           |                    |
| 9531:351  | $0, 0, 0, 0, e^{12}, -e^{13}, e^{34} + e^{15}, e^{36}, e^{17} + e^{46} + e^{25}$                      | $1/17(5, 10, 8, 12, 15, 13, 20, 21, 25)$             | $\{\emptyset, 134589, 15689, 346\}$                           |                    |
| 9531:353  | $0, 0, 0, 0, e^{12}, e^{34}, e^{25} + e^{13}, e^{15} + e^{46}, e^{27} + e^{35}$                       | $1/144(81, 38, 76, 62, 119, 138, 157, 200, 195)$     | $\{\emptyset, 145679, 1579, 46\}$                             |                    |
| 9531:354a | $0, 0, 0, 0, e^{12}, e^{13}, e^{15} + e^{23}, e^{36} + e^{25}, e^{17} + e^{26} + e^{34}$              | $14/51(1, 2, 2, 3, 3, 3, 4, 5, 5)$                   | $\{\emptyset, 12678, 145689, 24579\}$                         |                    |
| 9531:354b | $0, 0, 0, 0, -e^{12}, e^{13}, e^{15} + e^{23}, e^{25} + e^{36}, e^{17} + e^{26} + e^{34}$             | $14/51(1, 2, 2, 3, 3, 3, 4, 5, 5)$                   | $\{\emptyset, 12678, 145689, 24579\}$                         |                    |
| 9531:359  | $0, 0, 0, 0, a_1e^{12}, e^{13}(1 + a_1), e^{15} + e^{23}, e^{36} + e^{24}, e^{17} + e^{26} + e^{35}$  | $1/389(107, 212, 214, 323, 319, 321, 426, 535, 533)$ | $\{\emptyset, 12678, 145689, 24579\}$                         |                    |
| 9531:366  | $0, 0, 0, 0, -e^{12}, e^{14} + e^{23}, e^{34} + e^{15}, e^{35} + e^{16}, e^{36} + e^{17}$             | $1/41(10, 26, 15, 31, 36, 41, 46, 51, 56)$           | $\{\emptyset, 23579, 2456789, 3468\}$                         |                    |
| 9531:367  | $0, 0, 0, 0, -e^{12}, -e^{13} + e^{24}, e^{15} + e^{34}, e^{35} + e^{26}, e^{17} + e^{46}$            | $4/99(8, 11, 15, 12, 19, 23, 27, 34, 35)$            | $\{\emptyset, 235679, 245789, 3468\}$                         |                    |
| 9531:371  | $0, 0, 0, 0, -e^{12}, e^{14} + e^{23}, e^{15}, e^{35} + e^{16}, e^{24} + e^{17}$                      | $1/401(109, 197, 239, 327, 306, 436, 415, 545, 524)$ | $\{\emptyset, 123478, 14589, 23579\}$                         |                    |
| 9531:372  | $0, 0, 0, 0, e^{12}, e^{13}, e^{15}, e^{25} + e^{14}, e^{26} + e^{17} + e^{35}$                       | $1/71(23, 32, 46, 64, 55, 69, 78, 87, 101)$          | $\{\emptyset, 12678, 15689, 2579\}$                           |                    |
| 9531:374  | $0, 0, 0, 0, -e^{12}, e^{13}, e^{15} + e^{24}, e^{16} + e^{23}, e^{17} + e^{45}$                      | $1/61(17, 34, 44, 34, 51, 61, 68, 78, 85)$           | $\{\emptyset, 13589, 1569, 368\}$                             |                    |
| 9531:383a | $0, 0, 0, 0, e^{12}, e^{13}, e^{25}, e^{14} + e^{26} + e^{35}, e^{15} + e^{34} + e^{27}$              | $29/109(2, 1, 2, 3, 3, 4, 4, 5, 5)$                  | $\{\emptyset, 23569, 24589, 3468\}$                           |                    |
| 9531:383b | $0, 0, 0, 0, e^{12}, e^{13}, e^{25}, e^{35} - e^{14} + e^{26}, e^{34} + e^{27} + e^{15}$              | $29/109(2, 1, 2, 3, 3, 4, 4, 5, 5)$                  | $\{\emptyset, 23569, 24589, 3468\}$                           |                    |
| 9531:389  | $0, 0, 0, 0, e^{12}, -e^{13}, e^{15} + e^{34}, e^{16}, e^{46} + e^{17} + e^{25}$                      | $2/101(15, 30, 29, 31, 45, 44, 60, 59, 75)$          | $\{\emptyset, 134589, 1569, 3468\}$                           |                    |
| 9531:392  | $0, 0, 0, 0, -e^{12}, e^{13}, e^{24} + e^{15}, e^{16}, e^{36} + e^{45} + e^{17}$                      | $1/101(29, 62, 60, 58, 91, 89, 120, 118, 149)$       | $\{\emptyset, 13589, 1569, 368\}$                             |                    |
| 9531:393  | $0, 0, 0, 0, e^{12}, e^{13}, e^{25} + e^{14}, e^{16}, e^{36} + e^{27} + e^{45}$                       | $1/243(77, 96, 144, 192, 173, 221, 269, 298, 365)$   | $\{\emptyset, 135789, 15679, 368\}$                           |                    |
| 9531:395  | $0, 0, 0, 0, e^{12}, e^{34}, e^{13} + e^{25}, e^{15}, e^{27} + e^{46} + e^{35}$                       | $1/135(62, 44, 88, 53, 106, 141, 150, 168, 194)$     | $\{\emptyset, 124678, 1278, 46\}$                             |                    |
| 9531:397a | $0, 0, 0, 0, -e^{12}, e^{13}, e^{15} + e^{24}, e^{36} + e^{25}, e^{45} + e^{17}$                      | $1/129(38, 69, 69, 76, 107, 107, 145, 176, 183)$     | $\{\emptyset, 12378, 12678, 13589, 15689, 235679, 2579, 36\}$ |                    |
| 9531:397b | $0, 0, 0, 0, -e^{12}, -e^{13}, e^{15} + e^{24}, e^{36} + e^{25}, e^{45} + e^{17}$                     | $1/129(38, 69, 69, 76, 107, 107, 145, 176, 183)$     | $\{\emptyset, 12378, 12678, 13589, 15689, 235679, 2579, 36\}$ |                    |
| 9531:398  | $0, 0, 0, 0, -e^{12}, -e^{13}, e^{15} + e^{24}, e^{35} + e^{26}, e^{17} + e^{45}$                     | $1/31(10, 13, 20, 20, 23, 30, 33, 43, 43)$           | $\{\emptyset, 12378, 1267, 1359, 15689, 235679, 25789, 368\}$ |                    |
| 9531:399  | $0, 0, 0, 0, e^{12}, e^{13}, e^{14} + e^{25}, e^{35} + e^{26}, e^{45} + e^{27}$                       | $1/31(13, 10, 19, 20, 23, 32, 33, 42, 43)$           | $\{\emptyset, 12378, 1267, 13579, 156789, 23569, 2589, 368\}$ |                    |
| 9531:400  | $0, 0, 0, 0, e^{12}, e^{13}, e^{15} + e^{23}, e^{25} + e^{16}, e^{26} + e^{34} + e^{17}$              | $49/309(2, 3, 4, 5, 5, 6, 7, 8, 9)$                  | $\{\emptyset, 24579\}$                                        |                    |
| 9531:401  | $0, 0, 0, 0, a_1e^{12}, e^{13}(1 + a_1), e^{15} + e^{23}, e^{16} + e^{24}, e^{26} + e^{17} + e^{35}$  | $1/148(47, 70, 94, 118, 117, 141, 164, 188, 211)$    | $\{\emptyset, 12467, 1569, 24579\}$                           |                    |
| 9531:402a | $0, 0, 0, 0, -e^{12}, e^{13}, e^{23} + e^{15}, e^{36} + e^{25}, e^{17} + e^{35} + e^{24}$             | $14/51(1, 2, 2, 3, 3, 3, 4, 5, 5)$                   | $\{\emptyset, 124678, 145689, 2579\}$                         |                    |
| 9531:402b | $0, 0, 0, 0, -e^{12}, -e^{13}, e^{15} + e^{23}, e^{25} + e^{36}, e^{17} + e^{35} + e^{24}$            | $14/51(1, 2, 2, 3, 3, 3, 4, 5, 5)$                   | $\{\emptyset, 124678, 145689, 2579\}$                         |                    |
| 9531:410  | $0, 0, 0, 0, (-1 + a_2)e^{12}, e^{13}a_2, e^{23} + e^{15}, e^{34} + e^{25}, e^{35} + e^{26} + e^{17}$ | $2/27(4, 7, 8, 10, 11, 12, 15, 18, 19)$              | $\{\emptyset, 124678, 145689, 2579\}$                         |                    |
| 9531:412  | $0, 0, 0, 0, e^{12}, -e^{13}, e^{34} + e^{15}, e^{24} + e^{36}, e^{46} + e^{25} + e^{17}$             | $39/401(3, 6, 5, 7, 9, 8, 12, 13, 15)$               | $\{\emptyset, 134589\}$                                       |                    |
| 9531:416  | $0, 0, 0, 0, -e^{12}, e^{13}a_2, e^{24} + e^{15}, e^{34} + e^{16}, e^{36} + e^{45} + e^{17}$          | $1/101(29, 62, 60, 58, 91, 89, 120, 118, 149)$       | $\{\emptyset, 13589, 1569, 368\}$                             |                    |
| 9531:417a | $0, 0, 0, 0, e^{12}, e^{13}, e^{14} + e^{25}, e^{16} + e^{34}, e^{36} + e^{45} + e^{27}$              | $41/223(2, 2, 3, 4, 4, 5, 6, 7, 8)$                  | $\{\emptyset, 135789, 15679, 368\}$                           | ✓                  |
| 9531:417b | $0, 0, 0, 0, e^{12}, -e^{13}, e^{25} + e^{14}, e^{34} + e^{16}, e^{36} + e^{27} + e^{45}$             | $41/223(2, 2, 3, 4, 4, 5, 6, 7, 8)$                  | $\{\emptyset, 135789, 15679, 368\}$                           | ✓                  |
| 9531:421  | $0, 0, 0, 0, -e^{12}, e^{14} + e^{23}, e^{15} + e^{34}, e^{16} + e^{24} + e^{35}, e^{17} + e^{36}$    | $9/64(2, 4, 3, 5, 6, 7, 8, 9, 10)$                   | $\{\emptyset, 3468\}$                                         |                    |
| 9531:424  | $0, 0, 0, 0, -e^{12}, e^{23} + e^{14}, e^{15}, e^{35} + e^{16}, e^{17} + e^{25}$                      | $1/8(2, 4, 5, 7, 6, 9, 8, 11, 10)$                   | $\{\emptyset, 13569, 14589, 3468\}$                           |                    |
| 9531:426  | $0, 0, 0, 0, e^{12}, e^{14} + e^{23}, e^{13} + e^{25}, e^{15}, e^{16} + e^{27}$                       | $1/317(110, 119, 238, 247, 229, 357, 348, 339, 467)$ | $\{\emptyset, 12678, 14579, 245689\}$                         |                    |
| 9531:431  | $0, 0, 0, 0, e^{12}, e^{13}, e^{14} + e^{25}, e^{15}, e^{36} + e^{45} + e^{27}$                       | $1/521(192, 202, 303, 404, 394, 495, 596, 586, 798)$ | $\{\emptyset, 13579, 15679, 36\}$                             |                    |
| 9531:432  | $0, 0, 0, 0, -e^{12}, e^{13}, e^{24} + e^{15}, e^{25}, e^{36} + e^{17} + e^{45}$                      | $1/489(176, 206, 279, 352, 382, 455, 558, 588, 734)$ | $\{\emptyset, 134589, 15689, 36\}$                            |                    |
| 9531:433  | $0, 0, 0, 0, -e^{12}, e^{13}, e^{15} + e^{23}, e^{25} + e^{16}, e^{17} + e^{35} + e^{24}$             | $5/32(2, 3, 4, 6, 5, 6, 7, 8, 9)$                    | $\{\emptyset, 2579\}$                                         |                    |
| 9531:436  | $0, 0, 0, 0, a_1e^{12}, e^{13}(1 + a_1), e^{15} + e^{23}, e^{25} + e^{14}, e^{35} + e^{17} + e^{26}$  | $1/71(23, 32, 46, 64, 55, 69, 78, 87, 101)$          | $\{\emptyset, 12678, 15689, 2579\}$                           |                    |
| 9531:438  | $0, 0, 0, 0, e^{12}, -e^{13}, e^{15}a_2 + e^{34}, e^{23} + e^{16}, e^{46} + e^{17} + e^{25}$          | $2/101(15, 30, 29, 31, 45, 44, 60, 59, 75)$          | $\{\emptyset, 134589, 1569, 3468\}$                           |                    |
| 9531:439a | $0, 0, 0, 0, e^{12}, -e^{13}, e^{34} + e^{15}, e^{24} + e^{16}, e^{46} + e^{25} + e^{17}$             | $13/44(1, 2, 2, 2, 3, 3, 4, 4, 5)$                   | $\{\emptyset, 134589, 1569, 3468\}$                           | ✓                  |
| 9531:439b | $0, 0, 0, 0, -e^{12}, -e^{13}, e^{15} + e^{34}, e^{16} + e^{24}, e^{25} + e^{17} + e^{46}$            | $13/44(1, 2, 2, 2, 3, 3, 4, 4, 5)$                   | $\{\emptyset, 134589, 1569, 3468\}$                           | ✓                  |
| 9531:442a | $0, 0, 0, 0, -e^{12}, e^{13}, e^{15} + e^{24}, e^{23} + e^{16}, e^{45} + e^{36} + e^{17}$             | $13/44(1, 2, 2, 2, 3, 3, 4, 4, 5)$                   | $\{\emptyset, 13589, 1569, 368\}$                             | ✓                  |
| 9531:442b | $0, 0, 0, 0, -e^{12}, e^{13}, -e^{15} + e^{24}, e^{16} + e^{23}, e^{17} + e^{36} + e^{45}$            | $13/44(1, 2, 2, 2, 3, 3, 4, 4, 5)$                   | $\{\emptyset, 13589, 1569, 368\}$                             | ✓                  |
| 9531:450  | $0, 0, 0, 0, -e^{12}, e^{13}a_2, e^{15} + e^{24}, e^{16} + e^{25} + e^{34}, e^{17} + e^{45}$          | $1/25(7, 13, 19, 14, 20, 26, 27, 33, 34)$            | $\{\emptyset, 12378, 13589, 2579\}$                           |                    |
| 9531:456  | $0, 0, 0, 0, e^{12}, e^{13}, e^{25} + e^{14}, e^{15} + e^{34}, e^{27} + e^{36} + e^{45}$              | $87/997(5, 4, 6, 8, 9, 11, 13, 14, 17)$              | $\{\emptyset, 15679\}$                                        |                    |

Table A.4 – Continued to next page



Table A.4 – Continued from previous page

| Name      | g                                                                                                                   | N                                                  | S <sub>0</sub>                                    | S = S <sub>0</sub> |
|-----------|---------------------------------------------------------------------------------------------------------------------|----------------------------------------------------|---------------------------------------------------|--------------------|
| 9531:457  | $0, 0, 0, 0, -e^{12}, e^{13}, e^{15} + e^{24}, e^{25} + e^{34}, e^{17} + e^{36} + e^{45}$                           | 67/589(3, 4, 5, 6, 7, 8, 10, 11, 13)               | {0, 13589}                                        |                    |
| 9531:460  | $0, 0, 0, 0, -e^{12}, -e^{13}, e^{15} + e^{34}, e^{26} + e^{35}, e^{25} + e^{17} + e^{46}$                          | 1/162(46, 92, 81, 103, 138, 127, 184, 219, 230)    | {0, 13459, 15689, 3468}                           |                    |
| 9531:461  | $0, 0, 0, 0, -e^{12}, e^{24} + e^{13}, e^{23} + e^{15}, e^{45} + e^{16}, e^{17} + e^{26}$                           | 1/128(43, 51, 86, 78, 94, 129, 137, 172, 180)      | {0, 1267, 14569, 24579}                           |                    |
| 9531:462  | $0, 0, 0, 0, -e^{12}, -e^{13}, e^{15} + e^{24}, e^{26} + e^{35}, e^{17} + e^{36} + e^{45}$                          | 1/9(3, 4, 5, 6, 7, 8, 10, 12, 13)                  | {0, 1359, 15689, 368}                             |                    |
| 9531:463  | $0, 0, 0, 0, e^{12}, e^{13}, e^{14} + e^{25}, e^{26} + e^{35}, e^{36} + e^{27} + e^{45}$                            | 1/157(67, 54, 81, 108, 121, 148, 175, 202, 229)    | {0, 13579, 156789, 368}                           |                    |
| 9531:467  | $0, 0, 0, 0, -e^{12}, e^{14} + e^{23}, e^{34} + e^{15}, e^{35} + e^{16}, e^{17} + e^{36} + e^{24}$                  | 61/489(2, 5, 3, 6, 7, 8, 9, 10, 11)                | {0, 23579}                                        |                    |
| 9531:469  | $0, 0, 0, 0, e^{12}, e^{24} + e^{13}, e^{15}, e^{25}, e^{17} + e^{26} + e^{35}$                                     | 1/317(119, 110, 238, 247, 229, 357, 348, 339, 467) | {0, 12678, 145689, 24579}                         |                    |
| 9531:470  | $0, 0, 0, 0, e^{12}, e^{13}, e^{14} + e^{25}, e^{15}, e^{45} + e^{16} + e^{27}$                                     | 1/317(110, 119, 247, 238, 229, 357, 348, 339, 467) | {0, 12678, 13579, 235689}                         |                    |
| 9531:471a | $0, 0, 0, 0, -e^{12}, e^{14} + e^{23}, e^{15}, e^{35} + e^{16}, e^{34} + e^{17} + e^{25}$                           | 29/109(1, 2, 2, 3, 3, 4, 4, 5, 5)                  | {0, 13569, 14589, 3468}                           | ✓                  |
| 9531:471b | $0, 0, 0, 0, -e^{12}, -e^{14} + e^{23}, e^{15}, e^{16} + e^{35}, e^{17} + e^{34} + e^{25}$                          | 29/109(1, 2, 2, 3, 3, 4, 4, 5, 5)                  | {0, 13569, 14589, 3468}                           | ✓                  |
| 9531:474  | $0, 0, 0, 0, -e^{12}, e^{13}a_2 + e^{24}, e^{15}, e^{16} + e^{45} + e^{23}, e^{17} + e^{25}$                        | 1/8(2, 4, 7, 5, 6, 9, 8, 11, 10)                   | {0, 13589, 14569, 3468}                           |                    |
| 9531:475a | $0, 0, 0, 0, e^{12}, e^{23} + e^{14}, e^{25} + e^{13}, e^{15}, e^{27} + e^{16} + e^{34}$                            | 7/19(1, 1, 2, 2, 2, 3, 3, 4)                       | {0, 12678, 14579, 245689}                         | ✓                  |
| 9531:475b | $0, 0, 0, 0, -e^{12}, e^{14} + e^{23}, e^{25} + e^{13}, e^{15}, e^{16} + e^{34} + e^{27}$                           | 7/19(1, 1, 2, 2, 2, 3, 3, 4)                       | {0, 12678, 14579, 245689}                         | ✓                  |
| 9531:482a | $0, 0, 0, 0, e^{12}, e^{13}, e^{25} + e^{14}, e^{15} + e^{24}, e^{45} + e^{36} + e^{27}$                            | 4/21(2, 2, 3, 4, 4, 5, 6, 6, 8)                    | {0, 13579, 15679, 36}                             |                    |
| 9531:482b | $0, 0, 0, 0, -e^{12}, e^{13}, e^{25} - e^{14}, e^{24} + e^{15}, e^{27} + e^{36} + e^{45}$                           | 4/21(2, 2, 3, 4, 4, 5, 6, 6, 8)                    | {0, 13579, 15679, 36}                             |                    |
| 9531:487  | $0, 0, 0, 0, -e^{12}, e^{13}, e^{15} + e^{24}, e^{25} + e^{16}, e^{45} + e^{36} + e^{17}$                           | 67/589(3, 4, 5, 6, 7, 8, 10, 11, 13)               | {0, 13589}                                        |                    |
| 9531:489  | $0, 0, 0, 0, e^{12}, e^{13}, e^{14} + e^{25}, e^{35} + e^{26}, e^{45} + e^{27} + e^{16}$                            | 1/128(51, 43, 78, 86, 94, 129, 137, 172, 180)      | {0, 1267, 13579, 23569}                           |                    |
| 9531:490  | $0, 0, 0, 0, -e^{12}, -e^{14} + e^{23}, e^{15}, e^{35} + e^{16}, e^{26} + e^{17} + e^{45}$                          | 1/128(43, 51, 78, 86, 94, 129, 137, 172, 180)      | {0, 1267, 13569, 23579}                           |                    |
| 9531:494  | $0, 0, 0, 0, -e^{12}, e^{13}a_2, e^{15} + e^{24}, e^{16} + e^{34} + e^{25}, e^{17} + e^{36} + e^{45}$               | 67/589(3, 4, 5, 6, 7, 8, 10, 11, 13)               | {0, 13589}                                        |                    |
| 9531:496  | $0, 0, 0, 0, -e^{12}, e^{14} + e^{23}, e^{15} + e^{34}, e^{16} + e^{35}, e^{25} + e^{17} + e^{36}$                  | 9/64(2, 4, 3, 5, 6, 7, 8, 9, 10)                   | {0, 3468}                                         |                    |
| 9531:498  | $0, 0, 0, 0, e^{12}, e^{23} + e^{14}, e^{15}, e^{25} + e^{13}, e^{17} + e^{26} + e^{45}$                            | 7/19(1, 1, 2, 2, 2, 3, 3, 4)                       | {0, 12678}                                        |                    |
| 9531:500  | $0, 0, 0, 0, e^{12}, e^{13}, e^{14} + e^{25}, e^{15} + e^{23}, e^{16} + e^{27} + e^{45}$                            | 7/19(1, 1, 2, 2, 2, 3, 3, 4)                       | {0, 12678}                                        |                    |
| 9531:501a | $0, 0, 0, 0, e^{12}, e^{13}, e^{14} + e^{25}, e^{24} + e^{15}, e^{45} + e^{27} + e^{16}$                            | 7/19(1, 1, 2, 2, 2, 3, 3, 4)                       | {0, 12678, 13579, 235689}                         |                    |
| 9531:501b | $0, 0, 0, 0, -e^{12}, e^{13}, e^{25} - e^{14}, e^{24} + e^{15}, e^{27} + e^{16} + e^{45}$                           | 7/19(1, 1, 2, 2, 2, 3, 3, 4)                       | {0, 12678, 13579, 235689}                         |                    |
| 9531:503a | $0, 0, 0, 0, -e^{12}, e^{24} + e^{13}, e^{15}, e^{23}a_2 + e^{16} + e^{45}, e^{34} + e^{17} + e^{25}$               | 29/109(1, 2, 3, 2, 3, 4, 4, 5, 5)                  | {0, 13589, 14569, 3468}                           |                    |
| 9531:503b | $0, 0, 0, 0, -e^{12}, e^{24} - e^{13}, e^{15}, e^{23}a_2 + e^{16} + e^{45}, e^{17} + e^{25} + e^{34}$               | 29/109(1, 2, 3, 2, 3, 4, 4, 5, 5)                  | {0, 13589, 14569, 3468}                           |                    |
| 9531:504  | $0, 0, 0, 0, a_1e^{12}, e^{13} + e^{24}, e^{15} + e^{23}, e^{25} + e^{14}, e^{17} + e^{26} + e^{34}$                | 7/19(1, 1, 2, 2, 2, 3, 3, 4)                       | {0, 12678}                                        |                    |
| 9531:505  | $0, 0, 0, 0, a_1e^{12}, e^{23} + e^{14}, e^{13}(1 + a_1) + e^{25}, e^{15}, e^{35} + e^{27} + e^{16}$                | 1/317(110, 119, 238, 247, 229, 357, 348, 339, 467) | {0, 12678, 14579, 245689}                         |                    |
| 9531:512  | $0, 0, 0, 0, -a_3e^{12}, -e^{13}(-1 + a_3) + e^{24}, e^{15} + e^{23}, a_3e^{16} + e^{45}, e^{26} + e^{35} + e^{17}$ | 1/128(43, 51, 86, 78, 94, 129, 137, 172, 180)      | {0, 1267, 14569, 24579}                           |                    |
| 9531:514  | $0, 0, 0, 0, -e^{12}, e^{14} + e^{23}, a_3e^{15} + e^{34}, e^{16} + e^{24} + e^{35}, e^{17} + e^{25} + e^{36}$      | 9/64(2, 4, 3, 5, 6, 7, 8, 9, 10)                   | {0, 3468}                                         |                    |
| 9531:515  | $0, 0, 0, 0, (-1 + a_2)e^{12}, e^{13}a_2 + e^{24}, e^{15} + e^{23}, e^{14} + e^{25}, e^{17} + e^{35} + e^{26}$      | 7/19(1, 1, 2, 2, 2, 3, 3, 4)                       | {0, 12678}                                        |                    |
| 9531:521  | $0, 0, 0, 0, e^{12}, e^{13}, e^{15}, e^{25}, e^{27} + e^{18} + e^{34}$                                              | 1/31(11, 12, 22, 24, 23, 33, 34, 35, 46)           | {0, 123478, 12678, 13458, 1568, 234567, 257, 346} |                    |
| 9531:523  | $0, 0, 0, 0, e^{12}, e^{24} + e^{13}, e^{15}, e^{25}, e^{18} + e^{27}$                                              | 3/61(7, 7, 18, 18, 14, 25, 21, 21, 28)             | {0, 123478, 12678, 1358, 14568, 23567, 2457, 346} |                    |
| 9531:525  | $0, 0, 0, 0, e^{12}, e^{13} + e^{24}, e^{15}, e^{25}, e^{18} + e^{34} + e^{27}$                                     | 7/19(1, 1, 2, 2, 2, 3, 3, 4)                       | {0, 123478, 12678, 346}                           |                    |
| 9531:528  | $0, 0, 0, 0, e^{12}, e^{13}, e^{15}, e^{25} + e^{14}, e^{27} + e^{18}$                                              | 1/61(16, 27, 53, 54, 43, 69, 59, 70, 86)           | {0, 12378, 12678, 1358, 1568, 23567, 257, 36}     |                    |
| 9531:529  | $0, 0, 0, 0, e^{12}, e^{13}, e^{25}, e^{15} + e^{24}, e^{28} + e^{17}$                                              | 1/179(72, 55, 143, 144, 127, 215, 182, 199, 254)   | {0, 12378, 12678, 1357, 1567, 23568, 258, 36}     |                    |
| 9531:535  | $0, 0, 0, 0, e^{12}, e^{13}, e^{25}, e^{15} + e^{24}, e^{28} + e^{34} + e^{17}$                                     | 1/61(23, 22, 44, 46, 45, 67, 67, 68, 90)           | {0, 12678, 1567, 258}                             |                    |
| 9531:536  | $0, 0, 0, 0, e^{12}, e^{23} + e^{14}, e^{15}, e^{25} + e^{13}, e^{27} + e^{18}$                                     | 1/10(3, 4, 8, 9, 7, 12, 10, 11, 14)                | {0, 12678, 1458, 24567}                           |                    |
| 9531:538a | $0, 0, 0, 0, e^{12}, e^{13}, e^{15} + e^{24}, e^{25} + e^{14}, e^{17} + e^{28}$                                     | 1/89(32, 32, 73, 64, 64, 105, 96, 96, 128)         | {0, 12378, 12678, 13589, 15689, 235679, 2579, 36} | ✓                  |
| 9531:538b | $0, 0, 0, 0, e^{12}, e^{13}, e^{24} - e^{15}, e^{25} + e^{14}, e^{28} + e^{17}$                                     | 1/89(32, 32, 73, 64, 64, 105, 96, 96, 128)         | {0, 12378, 12678, 13589, 15689, 235679, 2579, 36} | ✓                  |
| 9531:539a | $0, 0, 0, 0, e^{12}, e^{13}, e^{14} + e^{25}, e^{24} + e^{15}, e^{28} + e^{17}$                                     | 1/89(32, 32, 73, 64, 64, 105, 96, 96, 128)         | {0, 12378, 12678, 1357, 1567, 23568, 258, 36}     | ✓                  |
| 9531:539b | $0, 0, 0, 0, e^{12}, e^{13}, e^{25} - e^{14}, e^{24} + e^{15}, e^{28} + e^{17}$                                     | 1/89(32, 32, 73, 64, 64, 105, 96, 96, 128)         | {0, 12378, 12678, 1357, 1567, 23568, 258, 36}     | ✓                  |
| 9531:542  | $0, 0, 0, 0, e^{12}, e^{34}, e^{15}, e^{25}, e^{27} + e^{18} + e^{36}$                                              | 1/24(9, 9, 10, 16, 18, 26, 27, 27, 36)             | {0, 123678, 1278, 13568, 158, 23567, 257, 36}     |                    |
| 9531:545a | $0, 0, 0, 0, e^{12}, e^{13}, e^{15}, e^{25} + e^{14}, e^{45} + e^{17} + e^{28}$                                     | 1/89(32, 32, 73, 64, 64, 105, 96, 96, 128)         | {0, 12378, 12678, 13589, 15689, 235679, 2579, 36} |                    |
| 9531:545b | $0, 0, 0, 0, e^{12}, e^{13}, -e^{15}, e^{25} + e^{14}, e^{28} + e^{45} + e^{17}$                                    | 1/89(32, 32, 73, 64, 64, 105, 96, 96, 128)         | {0, 12378, 12678, 13589, 15689, 235679, 2579, 36} |                    |
| 9531:546a | $0, 0, 0, 0, -e^{12}, e^{13}, e^{25}, e^{24} + e^{15}, e^{45} + e^{27} + e^{18}$                                    | 1/89(32, 32, 73, 64, 64, 105, 96, 96, 128)         | {0, 12378, 12678, 13579, 15679, 235689, 2589, 36} |                    |
| 9531:546b | $0, 0, 0, 0, -e^{12}, e^{13}, e^{25}, e^{24} - e^{15}, e^{27} + e^{18} + e^{45}$                                    | 1/89(32, 32, 73, 64, 64, 105, 96, 96, 128)         | {0, 12378, 12678, 13579, 15679, 235689, 2589, 36} |                    |

Table A.4 – Continued to next page

Table A.4 – Continued from previous page

| Name      | $g$                                                                                                              | $N$                                                  | $S_0$                                                     | $S = S_0$ |
|-----------|------------------------------------------------------------------------------------------------------------------|------------------------------------------------------|-----------------------------------------------------------|-----------|
| 9531:549a | $0, 0, 0, 0, e^{12}, e^{13}, e^{15} + e^{24}, e^{14} + e^{25}, e^{28} + e^{34} + e^{17}$                         | $7/19(1, 1, 2, 2, 2, 3, 3, 3, 4)$                    | $\{0, 12678, 13589, 235679\}$                             | ✓         |
| 9531:549b | $0, 0, 0, 0, e^{12}, e^{13}, -e^{15} + e^{24}, e^{25} + e^{14}, e^{28} + e^{17} + e^{34}$                        | $7/19(1, 1, 2, 2, 2, 3, 3, 3, 4)$                    | $\{0, 12678, 13589, 235679\}$                             | ✓         |
| 9531:550a | $0, 0, 0, 0, e^{12}, e^{13}, e^{15} + e^{24}, e^{14} + e^{25}, e^{18} + e^{34} + e^{27}$                         | $7/19(1, 1, 2, 2, 2, 3, 3, 3, 4)$                    | $\{0, 12678, 1568, 257\}$                                 | ✓         |
| 9531:550b | $0, 0, 0, 0, e^{12}, e^{13}, e^{15} + e^{24}, e^{25} - e^{14}, e^{18} + e^{27} + e^{34}$                         | $7/19(1, 1, 2, 2, 2, 3, 3, 3, 4)$                    | $\{0, 12678, 1568, 257\}$                                 | ✓         |
| 9531:553  | $0, 0, 0, 0, e^{12}, -e^{13}, e^{15}, e^{25} + e^{34}, e^{18} + e^{46} + e^{27}$                                 | $1/17(5, 8, 11, 10, 13, 16, 18, 21, 26)$             | $\{0, 12378, 124678, 1358, 14568, 234567, 257, 346\}$     |           |
| 9531:554a | $0, 0, 0, 0, e^{12}, -e^{13}, e^{25}, e^{34} + e^{15}, e^{18} + e^{27} + e^{46}$                                 | $1/73(28, 28, 43, 41, 56, 71, 84, 84, 112)$          | $\{0, 12378, 124678, 134579, 15679, 235689, 24589, 346\}$ |           |
| 9531:554b | $0, 0, 0, 0, e^{12}, -e^{13}, e^{25}, -e^{15} + e^{34}, e^{27} + e^{18} + e^{46}$                                | $1/73(28, 28, 43, 41, 56, 71, 84, 84, 112)$          | $\{0, 12378, 124678, 134579, 15679, 235689, 24589, 346\}$ |           |
| 9531:558a | $0, 0, 0, 0, a_1 e^{12}, e^{13}, e^{15} + e^{24}, e^{14}(1 + a_1) + e^{25}, e^{17} + e^{28} + e^{45}$            | $1/89(32, 32, 73, 64, 64, 105, 96, 96, 128)$         | $\{0, 12378, 12678, 13589, 15689, 235679, 2579, 36\}$     |           |
| 9531:558b | $0, 0, 0, 0, a_1 e^{12}, e^{13}, -e^{15} + e^{24}, e^{14}(1 + a_1) + e^{25}, e^{28} + e^{45} + e^{17}$           | $1/89(32, 32, 73, 64, 64, 105, 96, 96, 128)$         | $\{0, 12378, 12678, 13589, 15689, 235679, 2579, 36\}$     |           |
| 9531:559  | $0, 0, 0, 0, e^{12}, e^{13}, e^{15}, e^{25} + e^{14}, e^{27} + e^{18} + e^{36}$                                  | $1/217(64, 99, 131, 198, 163, 195, 227, 262, 326)$   | $\{0, 23567, 257, 36\}$                                   |           |
| 9531:560  | $0, 0, 0, 0, e^{12}, e^{13}, e^{25}, e^{15} + e^{24}, e^{28} + e^{17} + e^{36}$                                  | $1/213(88, 73, 117, 176, 161, 205, 234, 249, 322)$   | $\{0, 23568, 258, 36\}$                                   |           |
| 9531:562  | $0, 0, 0, 0, a_1 e^{12}, e^{13}, e^{23} + e^{15}, e^{25} + e^{14}, e^{34} + e^{27} + e^{18}$                     | $1/31(11, 12, 22, 24, 23, 33, 34, 35, 46)$           | $\{0, 12678, 1568, 257\}$                                 |           |
| 9531:564  | $0, 0, 0, 0, e^{12}, e^{14} + e^{23}, e^{15}, e^{25} + e^{34}, e^{18} + e^{27} + e^{36}$                         | $3/67(7, 10, 12, 15, 17, 22, 24, 27, 34)$            | $\{0, 13568, 1458, 346\}$                                 |           |
| 9531:565  | $0, 0, 0, 0, e^{12}, -e^{13}, e^{23} + e^{15}, e^{34} + e^{25}, e^{18} + e^{27} + e^{46}$                        | $1/163(51, 74, 102, 97, 125, 153, 176, 199, 250)$    | $\{0, 124678, 14568, 257\}$                               |           |
| 9531:572  | $0, 0, 0, 0, a_1 e^{12}, e^{24} + e^{13}, e^{23} + e^{15}, e^{14} + e^{25}, e^{27} + e^{18} + e^{34}$            | $7/19(1, 1, 2, 2, 2, 3, 3, 3, 4)$                    | $\{0, 12678\}$                                            |           |
| 9531:573  | $0, 0, 0, 0, e^{12}, e^{13}, e^{15} + e^{23}, e^{25} + e^{14}, e^{18} + e^{36} + e^{27}$                         | $17/113(2, 3, 4, 6, 5, 6, 7, 8, 10)$                 | $\{0, 257\}$                                              |           |
| 9531:574a | $0, 0, 0, 0, e^{12}, e^{13}, e^{15} + e^{24}, e^{25} + e^{14}, e^{17} + e^{28} + e^{36}$                         | $4/21(2, 2, 3, 4, 4, 5, 6, 6, 8)$                    | $\{0, 13589, 15689, 36\}$                                 | ✓         |
| 9531:574b | $0, 0, 0, 0, e^{12}, e^{13}, e^{24} - e^{15}, e^{25} + e^{14}, e^{17} + e^{28} + e^{36}$                         | $4/21(2, 2, 3, 4, 4, 5, 6, 6, 8)$                    | $\{0, 13589, 15689, 36\}$                                 | ✓         |
| 9531:575a | $0, 0, 0, 0, e^{12}, e^{13}, e^{15} + e^{24}, e^{25} + e^{14}, e^{27} + e^{18} + e^{36}$                         | $4/21(2, 2, 3, 4, 4, 5, 6, 6, 8)$                    | $\{0, 23567, 257, 36\}$                                   | ✓         |
| 9531:575b | $0, 0, 0, 0, e^{12}, e^{13}, e^{15} + e^{24}, -e^{14} + e^{25}, e^{36} + e^{18} + e^{27}$                        | $4/21(2, 2, 3, 4, 4, 5, 6, 6, 8)$                    | $\{0, 23567, 257, 36\}$                                   | ✓         |
| 9531:577  | $0, 0, 0, 0, e^{12}, -e^{23} + e^{14}, e^{13} + e^{25}, e^{15} + e^{34}, e^{46} + e^{28} + e^{17}$               | $23/211(4, 3, 6, 5, 7, 9, 10, 11, 14)$               | $\{0, 24568\}$                                            |           |
| 9531:579a | $0, 0, 0, 0, -e^{12}, e^{13}, e^{25}, e^{15} + e^{24}, e^{27} + e^{36} + e^{45} + e^{18}$                        | $4/21(2, 2, 3, 4, 4, 5, 6, 6, 8)$                    | $\{0, 13579, 15679, 36\}$                                 |           |
| 9531:579b | $0, 0, 0, 0, -e^{12}, e^{13}, e^{25}, -e^{15} + e^{24}, e^{27} + e^{18} + e^{36} + e^{45}$                       | $4/21(2, 2, 3, 4, 4, 5, 6, 6, 8)$                    | $\{0, 13579, 15679, 36\}$                                 |           |
| 9531:581a | $0, 0, 0, 0, (-1 + a_2) e^{12}, e^{13}, e^{24} + e^{15}, e^{14} a_2 + e^{25}, e^{28} + e^{36} + e^{45} + e^{17}$ | $4/21(2, 2, 3, 4, 4, 5, 6, 6, 8)$                    | $\{0, 13589, 15689, 36\}$                                 |           |
| 9531:581b | $0, 0, 0, 0, (-1 + a_2) e^{12}, e^{13}, e^{24} - e^{15}, e^{14} a_2 + e^{25}, e^{36} + e^{45} + e^{28} + e^{17}$ | $4/21(2, 2, 3, 4, 4, 5, 6, 6, 8)$                    | $\{0, 13589, 15689, 36\}$                                 |           |
| 9531:658  | $0, 0, 0, 0, e^{12}, e^{13}, e^{15}, e^{25} + e^{16}, e^{18} + e^{34} + e^{27}$                                  | $1/175(47, 84, 121, 141, 131, 168, 178, 215, 262)$   | $\{0, 123478, 13458, 257\}$                               |           |
| 9531:659  | $0, 0, 0, 0, e^{12}, e^{13}, e^{25}, e^{26} + e^{35}, e^{37} + e^{14} + e^{28}$                                  | $1/55(30, 13, 24, 50, 43, 54, 56, 67, 80)$           | $\{0, 123478, 12679, 13457, 156789, 234569, 258, 34689\}$ |           |
| 9531:661  | $0, 0, 0, 0, e^{12}, e^{13}, e^{25} + e^{34}, e^{36} + e^{24}, e^{27} + e^{38}$                                  | $1/27(17, 7, 7, 24, 24, 24, 31, 31, 38)$             | $\{0, 12378, 1456789, 234569\}$                           |           |
| 9531:666  | $0, 0, 0, 0, -e^{12}, e^{13}, e^{25}, e^{16} + e^{24}, e^{45} + e^{18} + e^{27}$                                 | $1/81(20, 33, 59, 66, 53, 79, 86, 99, 119)$          | $\{0, 12378, 15679, 235689\}$                             |           |
| 9531:667  | $0, 0, 0, 0, e^{12}, e^{13}, e^{14} + e^{25}, e^{16}, e^{18} + e^{27} + e^{45}$                                  | $1/81(20, 33, 59, 66, 53, 79, 86, 99, 119)$          | $\{0, 12378, 15679, 235689\}$                             |           |
| 9531:668  | $0, 0, 0, 0, -e^{12}, e^{13}, e^{24} + e^{15}, e^{36}, e^{45} + e^{38} + e^{17}$                                 | $1/537(174, 303, 217, 348, 477, 391, 651, 608, 825)$ | $\{0, 12378, 15689, 235679\}$                             |           |
| 9531:669  | $0, 0, 0, 0, e^{12}, e^{13}, e^{25} + e^{14}, e^{36}, e^{27} + e^{45} + e^{38}$                                  | $1/23(11, 8, 8, 16, 19, 19, 27, 27, 35)$             | $\{0, 12378, 156789, 23569\}$                             |           |
| 9531:675  | $0, 0, 0, 0, e^{12}, e^{13}, e^{34} + e^{25}, e^{26} + e^{35}, e^{28} + e^{37}$                                  | $1/17(11, 4, 5, 14, 15, 16, 19, 20, 24)$             | $\{0, 12378, 124679, 1357, 1456789, 234569, 258, 34689\}$ |           |
| 9531:680  | $0, 0, 0, 0, e^{12}, e^{13}, e^{25} + e^{34}, e^{24} + e^{36}, e^{14} + e^{38} + e^{27}$                         | $13/45(2, 1, 1, 3, 3, 3, 4, 4, 5)$                   | $\{0, 234569\}$                                           |           |
| 9531:681  | $0, 0, 0, 0, -e^{12}, e^{13}, e^{15}, e^{16} + e^{24}, e^{37} + e^{56} + e^{28}$                                 | $1/185(55, 78, 108, 140, 133, 163, 188, 218, 296)$   | $\{0, 12378, 124679, 134589, 156, 235678, 24579, 34689\}$ |           |
| 9531:682  | $0, 0, 0, 0, e^{12}, e^{13}, e^{15} + e^{23}, e^{16} + e^{25}, e^{18} + e^{34} + e^{27}$                         | $17/113(2, 3, 4, 6, 5, 6, 7, 8, 10)$                 | $\{0, 257\}$                                              |           |
| 9531:683  | $0, 0, 0, 0, (-1 + a_2) e^{12}, e^{13}, e^{14} a_2 + e^{25}, e^{24} + e^{16}, e^{45} + e^{27} + e^{18}$          | $1/81(20, 33, 59, 66, 53, 79, 86, 99, 119)$          | $\{0, 12378, 15679, 235689\}$                             |           |
| 9531:684a | $0, 0, 0, 0, e^{12}, e^{13}, e^{26} + e^{35}, e^{36} + e^{25}, e^{38} + e^{27} + e^{14}$                         | $2/33(9, 5, 5, 15, 14, 14, 19, 19, 24)$              | $\{0, 123478, 12689, 13458, 156789, 234569, 257, 34679\}$ |           |
| 9531:684b | $0, 0, 0, 0, -e^{12}, e^{13}, -e^{26} + e^{35}, e^{25} + e^{36}, e^{14} + e^{38} + e^{27}$                       | $2/33(9, 5, 5, 15, 14, 14, 19, 19, 24)$              | $\{0, 123478, 12689, 13458, 156789, 234569, 257, 34679\}$ |           |
| 9531:687  | $0, 0, 0, 0, e^{12}, e^{13}, e^{25} + e^{34}, e^{24} + e^{36}, e^{38} + e^{15} + e^{27}$                         | $13/45(2, 1, 1, 3, 3, 3, 4, 4, 5)$                   | $\{0, 234569\}$                                           |           |
| 9531:689  | $0, 0, 0, 0, e^{12}, e^{13}, e^{34} + e^{25}, e^{35} + e^{26}, e^{14} + e^{28} + e^{37}$                         | $1/163(102, 40, 51, 131, 142, 153, 182, 193, 233)$   | $\{0, 234569, 258, 34689\}$                               |           |
| 9531:694  | $0, 0, 0, 0, -e^{12}, e^{13}, e^{15} + e^{24}, e^{34} + e^{16}, e^{28} + e^{37} + e^{56}$                        | $1/15(5, 7, 7, 10, 12, 12, 17, 17, 24)$              | $\{0, 12378, 12679, 13589, 156, 235678, 2579, 3689\}$     |           |
| 9531:695a | $0, 0, 0, 0, -e^{12}, e^{13}, e^{15} + e^{34}, e^{16} + e^{24}, e^{28} + e^{37} + e^{56}$                        | $1/15(5, 7, 7, 10, 12, 12, 17, 17, 24)$              | $\{0, 12378, 124679, 134589, 156, 235678, 24579, 34689\}$ |           |
| 9531:695b | $0, 0, 0, 0, -e^{12}, e^{13}, e^{34} + e^{15}, -e^{24} + e^{16}, e^{28} + e^{37} + e^{56}$                       | $1/15(5, 7, 7, 10, 12, 12, 17, 17, 24)$              | $\{0, 12378, 124679, 134589, 156, 235678, 24579, 34689\}$ |           |
| 9531:696  | $0, 0, 0, 0, e^{12}, e^{13}, e^{25}, e^{14} + e^{26} + e^{35}, e^{28} + e^{37} + e^{45}$                         | $1/4(2, 1, 2, 3, 3, 4, 4, 5, 6)$                     | $\{0, 12378, 124679, 13457, 156789, 23569, 2458, 34689\}$ |           |
| 9531:698  | $0, 0, 0, 0, e^{12}, e^{13}, e^{25} + e^{14}, e^{35} + e^{26}, e^{46} + e^{28} + e^{37}$                         | $1/15(7, 5, 6, 10, 12, 13, 17, 18, 23)$              | $\{0, 12378, 12679, 1357, 156789, 23569, 258, 3689\}$     |           |
| 9531:706  | $0, 0, 0, 0, -e^{12}, e^{13}, e^{25}, e^{24} + e^{16}, e^{18} + e^{45} + e^{36} + e^{27}$                        | $15/149(3, 4, 6, 8, 7, 9, 11, 12, 15)$               | $\{0, 15679\}$                                            |           |

Table A.4 – Continued to next page

Table A.4 – Continued from previous page

| Name      | g                                                                                                                                                           | N                                                    | S <sub>0</sub>                                                    | S = S <sub>0</sub> |
|-----------|-------------------------------------------------------------------------------------------------------------------------------------------------------------|------------------------------------------------------|-------------------------------------------------------------------|--------------------|
| 9531:707  | $0, 0, 0, 0, e^{12}, e^{13}, e^{15}, e^{14} + e^{36}, e^{25} + e^{38} + e^{17} + e^{46}$                                                                    | $15/149(3, 6, 4, 8, 9, 7, 12, 11, 15)$               | $\{\emptyset, 15689\}$                                            |                    |
| 9531:709  | $0, 0, 0, 0, e^{12}, e^{13}, e^{25} + e^{34}, e^{26} + e^{35}, e^{15} + e^{28} + e^{37}$                                                                    | $1/71(42, 19, 23, 57, 61, 65, 80, 84, 103)$          | $\{\emptyset, 124679, 1357, 234569\}$                             |                    |
| 9531:711  | $0, 0, 0, 0, e^{12}, e^{13}, e^{34} + e^{25}, e^{35} + e^{26}, e^{37} + e^{28} + e^{16}$                                                                    | $1/35(20, 10, 11, 29, 30, 31, 40, 41, 51)$           | $\{\emptyset, 234569, 258, 34689\}$                               |                    |
| 9531:715  | $0, 0, 0, 0, -e^{12}, e^{13}, e^{34} + e^{15}, e^{25} + e^{16}, e^{37} + e^{28} + e^{56}$                                                                   | $1/441(167, 174, 181, 327, 341, 348, 508, 515, 689)$ | $\{\emptyset, 12378, 134589, 24579\}$                             |                    |
| 9531:716  | $0, 0, 0, 0, e^{12}, e^{13}, e^{34} + 2e^{15}, e^{35} + e^{26}, e^{56} + e^{18} + e^{37}$                                                                   | $1/76(25, 38, 28, 60, 63, 53, 88, 91, 116)$          | $\{\emptyset, 12378, 124679, 13459, 1568, 23567, 245789, 34689\}$ |                    |
| 9531:717  | $0, 0, 0, 0, e^{12}, e^{13}, e^{34} + e^{25}, e^{14} + e^{26} + e^{35}, e^{28} + e^{37} + e^{45}$                                                           | $1/49(27, 13, 20, 33, 40, 47, 53, 60, 73)$           | $\{\emptyset, 12378, 124679, 34689\}$                             |                    |
| 9531:718  | $0, 0, 0, 0, a_1 e^{12}, -e^{13}, e^{15} + e^{24}, e^{16} + e^{25} + e^{34}, e^{27} + e^{18} + e^{46}$                                                      | $1/17(5, 8, 11, 10, 13, 16, 18, 21, 26)$             | $\{\emptyset, 12378, 1358, 257\}$                                 |                    |
| 9531:719  | $0, 0, 0, 0, a_1 e^{12}, e^{13}, e^{14}(1 + a_1) + e^{25}, e^{16} + e^{24}, e^{45} + e^{36} + e^{18} + e^{27}$                                              | $15/149(3, 4, 6, 8, 7, 9, 11, 12, 15)$               | $\{\emptyset, 15679\}$                                            |                    |
| 9531:724  | $0, 0, 0, 0, e^{12}, -e^{13}, e^{23} + e^{15}, e^{16} + e^{34} + e^{25}, e^{18} + e^{27} + e^{46}$                                                          | $49/319(2, 3, 4, 4, 5, 6, 7, 8, 10)$                 | $\{\emptyset, 257\}$                                              |                    |
| 9531:726  | $0, 0, 0, 0, -e^{12}, -e^{13}, 2e^{16} + e^{25}, e^{26} + e^{35}, e^{56} + e^{18} + e^{34} + e^{27}$                                                        | $5/87(5, 7, 9, 17, 12, 14, 19, 21, 26)$              | $\{\emptyset, 123478, 13579, 24589\}$                             |                    |
| 9531:727  | $0, 0, 0, 0, -e^{12}, e^{13}, e^{15} + e^{24}, e^{25} + e^{16} + e^{34}, e^{28} + e^{37} + e^{56}$                                                          | $1/46(16, 19, 22, 32, 35, 38, 51, 54, 73)$           | $\{\emptyset, 12378, 13589, 2579\}$                               |                    |
| 9531:729a | $0, 0, 0, 0, e^{12}, e^{13}, e^{36} + e^{25}, e^{26} + e^{35} + e^{14}, e^{37} + e^{28} + e^{45}$                                                           | $1/23(11, 8, 8, 16, 19, 19, 27, 27, 35)$             | $\{\emptyset, 12378, 124679, 13457, 156789, 23569, 2458, 34689\}$ |                    |
| 9531:729b | $0, 0, 0, 0, e^{12}, -e^{13}, e^{36} + e^{25}, e^{35} + e^{14} - e^{26}, e^{28} + e^{37} + e^{45}$                                                          | $1/23(11, 8, 8, 16, 19, 19, 27, 27, 35)$             | $\{\emptyset, 12378, 124679, 13457, 156789, 23569, 2458, 34689\}$ |                    |
| 9531:730a | $0, 0, 0, 0, e^{12}, e^{13}, e^{26} + e^{35}, e^{14} + e^{36} + e^{25}, e^{28} + e^{37} + e^{45}$                                                           | $1/23(11, 8, 8, 16, 19, 19, 27, 27, 35)$             | $\{\emptyset, 12378, 1268, 13589, 156789, 23569, 2579, 367\}$     |                    |
| 9531:730b | $0, 0, 0, 0, e^{12}, e^{13}, e^{26} + e^{35}, -e^{25} + e^{36} + e^{14}, e^{28} + e^{37} + e^{45}$                                                          | $1/23(11, 8, 8, 16, 19, 19, 27, 27, 35)$             | $\{\emptyset, 12378, 1268, 13589, 156789, 23569, 2579, 367\}$     |                    |
| 9531:739  | $0, 0, 0, 0, -e^{12}, -e^{13}, 2e^{16} + e^{25}, e^{26} + e^{35} + e^{14}, e^{27} + e^{18} + e^{56}$                                                        | $1/49(13, 20, 27, 47, 33, 40, 53, 60, 73)$           | $\{\emptyset, 12378, 134579, 24589\}$                             |                    |
| 9531:742  | $0, 0, 0, 0, e^{12}, e^{13}, e^{25} + e^{34}, e^{35} + e^{14} + e^{26}, e^{37} + e^{45} + e^{16} + e^{28}$                                                  | $11/81(4, 2, 3, 5, 6, 7, 8, 9, 11)$                  | $\{\emptyset, 34689\}$                                            |                    |
| 9531:743  | $0, 0, 0, 0, -e^{12}, e^{13}, e^{25} + e^{34} + e^{16}, e^{24} + e^{36} + e^{15}, e^{27} + e^{56} + e^{38}$                                                 | $19/49(1, 1, 1, 2, 2, 2, 3, 4)$                      | $\{\emptyset, 12378\}$                                            |                    |
| 9531:745  | $0, 0, 0, 0, -e^{12}, -e^{13}, 2e^{16} + e^{25}, e^{14} + e^{26} + e^{35}, e^{27} + e^{56} + e^{18} + e^{34}$                                               | $11/81(2, 3, 4, 7, 5, 6, 8, 9, 11)$                  | $\{\emptyset, 24589\}$                                            |                    |
| 9531:752  | $0, 0, 0, 0, -e^{12}, e^{14} + e^{23}, e^{15}, e^{35} + e^{16}, e^{18} + e^{37}$                                                                            | $1/31(5, 20, 13, 28, 25, 33, 30, 38, 43)$            | $\{\emptyset, 123478, 12679, 13569, 1458, 2357, 2456789, 34689\}$ |                    |
| 9531:753  | $0, 0, 0, 0, -e^{12}, e^{34}, e^{15} + e^{23}, e^{46}, e^{48} + e^{17} + e^{35}$                                                                            | $1/327(93, 201, 186, 98, 294, 284, 387, 382, 480)$   | $\{\emptyset, 127, 14569, 245679\}$                               |                    |
| 9531:755  | $0, 0, 0, 0, -e^{12}, e^{23} + e^{14}, e^{34} + e^{15}, e^{16} + e^{35}, e^{18} + e^{37}$                                                                   | $1/67(14, 45, 21, 52, 59, 66, 73, 80, 94)$           | $\{\emptyset, 2357, 2456789, 34689\}$                             |                    |
| 9531:756  | $0, 0, 0, 0, -e^{12}, e^{23} + e^{14}, e^{15}, e^{16} + e^{35}, e^{18} + e^{37} + e^{24}$                                                                   | $1/329(65, 195, 147, 277, 260, 342, 325, 407, 472)$  | $\{\emptyset, 123478, 12679, 34689\}$                             |                    |
| 9531:757  | $0, 0, 0, 0, -e^{12}, e^{23} + e^{14}, e^{15}, e^{16} + e^{35}, e^{25} + e^{37} + e^{18}$                                                                   | $1/128(22, 79, 57, 114, 101, 136, 123, 158, 180)$    | $\{\emptyset, 12679, 13569, 2357\}$                               |                    |
| 9531:759a | $0, 0, 0, 0, e^{14} + e^{23}, e^{13} + e^{24}, e^{25} + e^{16}, e^{26} + e^{15}, e^{17} + e^{28}$                                                           | $1/33(7, 7, 24, 24, 31, 31, 38, 38, 45)$             | $\{\emptyset, 123478, 12569, 1357, 14689, 23679, 2458, 3456789\}$ |                    |
| 9531:759b | $0, 0, 0, 0, -e^{14} + e^{23}, e^{13} + e^{24}, -e^{16} + e^{25}, e^{15} + e^{26}, e^{17} + e^{28}$                                                         | $1/33(7, 7, 24, 24, 31, 31, 38, 38, 45)$             | $\{\emptyset, 123478, 12569, 1357, 14689, 23679, 2458, 3456789\}$ |                    |
| 9531:760  | $0, 0, 0, 0, -e^{12}, e^{23} + e^{14}, e^{15} + e^{34}, e^{35} + e^{16}, e^{24} + e^{37} + e^{18}$                                                          | $23/211(2, 6, 3, 7, 8, 9, 10, 11, 13)$               | $\{\emptyset, 34689\}$                                            |                    |
| 9531:762  | $0, 0, 0, 0, -e^{12}, e^{14} + e^{23}, e^{34} + e^{15}, e^{35} + e^{16}, e^{18} + e^{37} + e^{25}$                                                          | $31/256(2, 5, 3, 6, 7, 8, 9, 10, 12)$                | $\{\emptyset, 2357\}$                                             |                    |
| 9531:763  | $0, 0, 0, 0, -e^{12}, e^{14} + e^{23}, e^{15}, e^{35} + e^{16} + e^{24}, e^{26} + e^{37} + e^{18}$                                                          | $1/4(1, 2, 2, 3, 3, 4, 4, 5, 6)$                     | $\{\emptyset, 13569, 1458, 34689\}$                               |                    |
| 9531:764  | $0, 0, 0, 0, -e^{12}, e^{24} + e^{13}, e^{15} + e^{23}, e^{16} + e^{45}, e^{18} + e^{47} + e^{36}$                                                          | $1/46(14, 23, 28, 19, 37, 42, 51, 56, 70)$           | $\{\emptyset, 12679, 14569, 2457\}$                               |                    |
| 9531:770  | $0, 0, 0, 0, -e^{12}, -e^{14} + e^{23}, e^{15}, e^{16} + e^{35}, e^{37} + e^{18} + e^{26} + e^{45}$                                                         | $1/4(1, 2, 2, 3, 3, 4, 4, 5, 6)$                     | $\{\emptyset, 13569, 1458, 34689\}$                               |                    |
| 9531:772a | $0, 0, 0, 0, e^{23} + e^{14}, e^{24} + e^{13}, e^{25} + e^{16}, e^{26} + e^{15}, e^{34} + e^{28} + e^{17}$                                                  | $16/69(1, 1, 3, 3, 4, 4, 5, 5, 6)$                   | $\{\emptyset, 123478, 14689, 23679\}$                             |                    |
| 9531:772b | $0, 0, 0, 0, e^{23} - e^{14}, e^{24} + e^{13}, -e^{16} + e^{25}, e^{15} + e^{26}, e^{28} + e^{17} + e^{34}$                                                 | $16/69(1, 1, 3, 3, 4, 4, 5, 5, 6)$                   | $\{\emptyset, 123478, 14689, 23679\}$                             |                    |
| 9531:773  | $0, 0, 0, 0, -e^{12}, e^{14} + e^{23}, e^{34} + e^{15}, e^{24} + e^{35} + e^{16}, e^{18} + e^{37} + e^{26}$                                                 | $11/81(2, 4, 3, 5, 6, 7, 8, 9, 11)$                  | $\{\emptyset, 34689\}$                                            |                    |
| 9531:778  | $0, 0, 0, 0, (-1 + a_2)e^{12}, e^{13}a_2 + e^{24}, e^{15}, -(-1 + a_2)e^{16} + e^{23} + e^{45}, e^{26} + e^{47} + e^{18} + e^{35}$                          | $1/4(1, 2, 3, 2, 3, 4, 4, 5, 6)$                     | $\{\emptyset, 1358, 14569, 34689\}$                               |                    |
| 9531:782  | $0, 0, 0, 0, -e^{12}, -e^{14} + e^{23}, e^{15} + e^{34}, e^{16} + e^{35}, e^{37} + e^{18} + e^{26} + e^{45}$                                                | $11/81(2, 4, 3, 5, 6, 7, 8, 9, 11)$                  | $\{\emptyset, 34689\}$                                            |                    |
| 9531:784a | $0, 0, 0, 0, e^{14} + e^{23}, e^{13} + e^{24}, e^{26} + e^{15}, e^{34} + e^{25} + e^{16}, e^{35} + e^{18} + e^{27}$                                         | $5/17(1, 1, 2, 2, 3, 3, 4, 4, 5)$                    | $\{\emptyset, 12569, 1358, 23689\}$                               |                    |
| 9531:784b | $0, 0, 0, 0, e^{14} + e^{23}, e^{13} - e^{24}, e^{15} + e^{26}, -e^{16} + e^{34} + e^{25}, e^{18} + e^{35} + e^{27}$                                        | $5/17(1, 1, 2, 2, 3, 3, 4, 4, 5)$                    | $\{\emptyset, 12569, 1358, 23689\}$                               |                    |
| 9531:785a | $0, 0, 0, 0, e^{24} + e^{13}, e^{23} + e^{14}, e^{15} + e^{26}, e^{16} + e^{25} + e^{34}, e^{35} + e^{28} + e^{17}$                                         | $5/17(1, 1, 2, 2, 3, 3, 4, 4, 5)$                    | $\{\emptyset, 12569, 14589, 2468\}$                               |                    |
| 9531:785b | $0, 0, 0, 0, e^{24} + e^{13}, -e^{14} + e^{23}, e^{26} - e^{15}, e^{25} + e^{34} + e^{16}, e^{35} + e^{17} + e^{28}$                                        | $5/17(1, 1, 2, 2, 3, 3, 4, 4, 5)$                    | $\{\emptyset, 12569, 14589, 2468\}$                               |                    |
| 9531:789  | $0, 0, 0, 0, (-1 + a_2)e^{12}, e^{13}a_2 + e^{24}, e^{34} + e^{15}, -(-1 + a_2)e^{16} + e^{45} + e^{23}, e^{18} + e^{47} + e^{35} + e^{26}$                 | $11/81(2, 4, 5, 3, 6, 7, 8, 9, 11)$                  | $\{\emptyset, 34689\}$                                            |                    |
| 9531:792a | $0, 0, 0, 0, e^{14} + e^{23}, e^{13} + e^{24}, e^{16} + e^{25}, e^{26} + e^{15}, e^{28} + e^{46} + e^{35} + e^{17}$                                         | $5/17(1, 1, 2, 2, 3, 3, 4, 4, 5)$                    | $\{\emptyset, 12569, 1357, 23679\}$                               |                    |
| 9531:792b | $0, 0, 0, 0, -e^{23} - e^{14}, e^{24} - e^{13}, -e^{16} + e^{25}, e^{15} + e^{26}, e^{28} + e^{17} + e^{35} + e^{46}$                                       | $5/17(1, 1, 2, 2, 3, 3, 4, 4, 5)$                    | $\{\emptyset, 12569, 1357, 23679\}$                               |                    |
| 9531:795a | $0, 0, 0, 0, e^{23}(-1 + a_5) + e^{14}a_5, e^{13} + e^{24}a_5, \frac{e^{15}}{-1+a_5} + e^{26}, e^{16} + e^{25} + e^{34}, e^{45} + e^{28} + e^{17} + e^{36}$ | $5/17(1, 1, 2, 2, 3, 3, 4, 4, 5)$                    | $\{\emptyset, 12569, 13589, 2368\}$                               |                    |

Table A.4 – Continued to next page

Table A.4 – Continued from previous page

| Name      | g                                                                                                                                                                  | N                                                  | S <sub>0</sub>                                        | S = S <sub>0</sub> |
|-----------|--------------------------------------------------------------------------------------------------------------------------------------------------------------------|----------------------------------------------------|-------------------------------------------------------|--------------------|
| 9531:795b | $0, 0, 0, 0, e^{23}(-1 + a_5) + e^{14}a_5,$<br>$-e^{13} + e^{24}a_5, -\frac{e^{15}}{-1+a_5} + e^{26}, e^{34} + e^{25} + e^{16}, e^{45} + e^{36} + e^{17} + e^{28}$ | 5/17(1, 1, 2, 2, 3, 3, 4, 4, 5)                    | {0, 12569, 13589, 2368}                               |                    |
| 9521:49   | $0, 0, 0, 0, e^{12}, e^{13}, e^{34}, e^{14} + e^{25}, e^{45} + e^{28}$                                                                                             | 1/109(58, 31, 69, 62, 89, 127, 131, 120, 151)      | {0, 12378, 1268, 135789, 15689, 235679, 259, 367}     |                    |
| 9521:65   | $0, 0, 0, 0, -e^{12}, e^{13}, e^{23}, e^{15} + e^{24}, e^{45} + e^{18}$                                                                                            | 1/179(58, 83, 132, 116, 141, 190, 215, 199, 257)   | {0, 1238, 12678, 13579, 1569, 235689, 25789, 367}     |                    |
| 9521:68   | $0, 0, 0, 0, e^{12}, e^{13}, e^{34}, e^{15} + e^{23}, e^{18} + e^{26}$                                                                                             | 1/7(2, 4, 4, 5, 6, 6, 9, 8, 10)                    | {0, 124678, 1268, 145679, 1569, 245789, 2589, 47}     |                    |
| 9521:84   | $0, 0, 0, 0, e^{12}, e^{13}, e^{34}, e^{15}, e^{26} + e^{35} + e^{18}$                                                                                             | 1/7(2, 4, 4, 5, 6, 6, 9, 8, 10)                    | {0, 124678, 1268, 145679, 1569, 245789, 2589, 47}     |                    |
| 9521:86   | $0, 0, 0, 0, e^{12}, -e^{13}, e^{23}, e^{34} + e^{15}, e^{18} + e^{46}$                                                                                            | 1/109(30, 69, 62, 67, 99, 92, 131, 129, 159)       | {0, 1238, 124678, 134579, 1569, 235689, 245789, 3467} |                    |
| 9521:88   | $0, 0, 0, 0, e^{12}, -e^{13}, e^{24}, e^{15} + e^{34}, e^{18} + e^{46}$                                                                                            | 1/69(17, 47, 48, 33, 64, 65, 80, 81, 98)           | {0, 12378, 12468, 134579, 1569, 2356789, 24589, 3467} |                    |
| 9521:104  | $0, 0, 0, 0, e^{12}, e^{13}, e^{24}, e^{15}, e^{18} + e^{26} + e^{35}$                                                                                             | 1/9(3, 4, 6, 7, 9, 11, 10, 13)                     | {0, 12468, 12678, 145679, 1569, 24589, 25789, 47}     |                    |
| 9521:114  | $0, 0, 0, 0, e^{12}, -e^{23} + e^{14}, e^{13}, e^{34} + e^{25}, e^{46} + e^{28}$                                                                                   | 1/119(61, 38, 80, 57, 99, 118, 141, 137, 175)      | {0, 135689, 145789, 3467}                             |                    |
| 9521:115  | $0, 0, 0, 0, e^{12}(-1 + a_2), a_2e^{13}, e^{34}, e^{23} + e^{15}, e^{35} + e^{18} + e^{26}$                                                                       | 1/7(2, 4, 4, 5, 6, 6, 9, 8, 10)                    | {0, 124678, 1268, 145679, 1569, 245789, 2589, 47}     |                    |
| 9521:123  | $0, 0, 0, 0, e^{12}, -e^{13}, e^{34}, e^{25}, e^{17} + e^{28} + e^{46}$                                                                                            | 1/39(18, 14, 21, 21, 32, 39, 42, 46, 60)           | {0, 12378, 124678, 134589, 15689, 235679, 24579, 346} |                    |
| 9521:127  | $0, 0, 0, 0, e^{12}, e^{13}, e^{14}, e^{25}, e^{28} + e^{37} + e^{46}$                                                                                             | 1/21(9, 8, 12, 12, 17, 21, 21, 25, 33)             | {0, 12378, 12468, 134589, 156789, 23569, 24579, 3467} |                    |
| 9521:134  | $0, 0, 0, 0, e^{12}(-1 + a_2), a_2e^{13}, e^{14}, e^{15} + e^{23}, e^{18} + e^{35} + e^{26}$                                                                       | 1/13(4, 7, 8, 11, 11, 12, 15, 15, 19)              | {0, 12468, 12678, 14569, 15679, 245789, 2589, 47}     |                    |
| 9521:135  | $0, 0, 0, 0, e^{12}(-1 + a_2), a_2e^{13}, e^{24}, e^{23} + e^{15}, e^{35} + e^{18} + e^{26}$                                                                       | 1/9(3, 4, 6, 7, 7, 9, 11, 10, 13)                  | {0, 12468, 12678, 145679, 1569, 24589, 25789, 47}     |                    |
| 9521:136  | $0, 0, 0, 0, e^{12}, e^{14} + e^{23}, e^{34}, e^{13} + e^{25}, e^{28} + e^{16}$                                                                                    | 1/92(41, 31, 62, 52, 72, 93, 114, 103, 134)        | {0, 1268, 145789, 245679}                             |                    |
| 9521:139  | $0, 0, 0, 0, e^{12}, e^{34}, e^{13}, e^{25} + e^{14}, e^{28} + e^{36} + e^{45}$                                                                                    | 1/423(257, 123, 190, 246, 380, 436, 447, 503, 626) | {0, 12368, 1278, 367}                                 |                    |
| 9521:140  | $0, 0, 0, 0, e^{12}, -e^{13}, e^{23}, e^{15} + e^{34}, e^{37} + e^{18} + e^{46}$                                                                                   | 1/92(30, 52, 45, 67, 82, 75, 97, 112, 142)         | {0, 235689, 245789, 3467}                             |                    |
| 9521:141  | $0, 0, 0, 0, e^{12}, e^{13}(-1 + a_2), a_2e^{14}, e^{15} + e^{34}, e^{18} + e^{46} + e^{37}$                                                                       | 1/8(2, 6, 5, 5, 8, 7, 7, 10, 12)                   | {0, 12378, 12468, 13459, 15679, 235689, 245789, 3467} |                    |
| 9521:143  | $0, 0, 0, 0, -e^{12}, e^{13}, e^{34}, e^{24} + e^{15}, e^{36} + e^{18} + e^{45}$                                                                                   | 1/101(29, 62, 60, 58, 91, 89, 118, 120, 149)       | {0, 13579, 1569, 367}                                 |                    |
| 9521:144  | $0, 0, 0, 0, e^{12}, e^{13}, e^{34}, e^{25} + e^{14}, e^{28} + e^{45} + e^{36}$                                                                                    | 1/49(25, 16, 24, 32, 41, 49, 56, 57, 73)           | {0, 135789, 15689, 367}                               |                    |
| 9521:151  | $0, 0, 0, 0, e^{12}, -e^{13}, e^{23}, e^{15} + e^{34}, e^{25} + e^{18} + e^{46}$                                                                                   | 2/101(15, 30, 29, 31, 45, 44, 59, 60, 75)          | {0, 134579, 1569, 3467}                               |                    |
| 9521:153  | $0, 0, 0, 0, e^{12}, -e^{13}, e^{24}, e^{34} + e^{15}, e^{46} + e^{25} + e^{18}$                                                                                   | 2/27(4, 8, 9, 7, 12, 13, 15, 16, 20)               | {0, 134579, 1569, 3467}                               |                    |
| 9521:154  | $0, 0, 0, 0, e^{12}, e^{24} + e^{13}, e^{34}, e^{15}, e^{35} + e^{18} + e^{26}$                                                                                    | 1/92(31, 41, 62, 52, 72, 93, 114, 103, 134)        | {0, 1268, 145679, 245789}                             |                    |
| 9521:155  | $0, 0, 0, 0, e^{12}, -e^{13}, e^{23}, e^{34} + e^{15}, e^{18} + e^{46} + e^{27}$                                                                                   | 4/491(43, 62, 67, 81, 105, 110, 129, 148, 191)     | {0, 124678, 134579, 235689}                           |                    |
| 9521:157  | $0, 0, 0, 0, e^{12}, e^{13}, e^{23} + e^{14}, e^{15}, e^{18} + e^{37} + e^{46}$                                                                                    | 1/92(30, 52, 45, 67, 82, 75, 97, 112, 142)         | {0, 235689, 245789, 3467}                             |                    |
| 9521:159  | $0, 0, 0, 0, e^{12}, e^{13}, e^{34}, e^{15} + e^{23}, e^{18} + e^{26} + e^{47}$                                                                                    | 5/33(2, 4, 4, 3, 6, 6, 7, 8, 10)                   | {0, 124678, 1268, 47}                                 |                    |
| 9521:160  | $0, 0, 0, 0, e^{12}, e^{13}, e^{24}, e^{34} + e^{25}, e^{37} + e^{28} + e^{16}$                                                                                    | 1/441(226, 149, 221, 303, 375, 447, 452, 524, 673) | {0, 12468, 13589, 234569}                             |                    |
| 9521:161  | $0, 0, 0, 0, -e^{12}, e^{13}, e^{23}, e^{24} + e^{15}, e^{36} + e^{45} + e^{18}$                                                                                   | 1/27(9, 14, 16, 18, 23, 25, 30, 32, 41)            | {0, 13579, 1569, 367}                                 |                    |
| 9521:164  | $0, 0, 0, 0, e^{12}, e^{13}, e^{24}, e^{25} + e^{14}, e^{45} + e^{36} + e^{28}$                                                                                    | 1/17(8, 6, 9, 12, 14, 17, 18, 20, 26)              | {0, 13589, 15689, 36}                                 |                    |
| 9521:165  | $0, 0, 0, 0, e^{12}, e^{13}, e^{34}, e^{14} + e^{25}, e^{28} + e^{45} + e^{16}$                                                                                    | 1/92(41, 31, 52, 62, 72, 93, 114, 103, 134)        | {0, 1268, 135789, 235679}                             |                    |
| 9521:168  | $0, 0, 0, 0, e^{12}, a_1e^{13}, e^{23} + (1 + a_1)e^{14}, e^{15} + e^{34}, e^{18} + e^{46} + e^{37}$                                                               | 1/92(30, 52, 45, 67, 82, 75, 97, 112, 142)         | {0, 235689, 245789, 3467}                             |                    |
| 9521:170  | $0, 0, 0, 0, -e^{12}, e^{14} + e^{23}, e^{13}, e^{25}, e^{28} + e^{35} + e^{16}$                                                                                   | 1/221(79, 82, 164, 167, 161, 246, 243, 243, 325)   | {0, 12678, 145789, 24569}                             |                    |
| 9521:171  | $0, 0, 0, 0, e^{12}, e^{14} + e^{23}, e^{13}, e^{15}, e^{26} + e^{45} + e^{18}$                                                                                    | 1/317(116, 125, 223, 232, 241, 348, 339, 357, 473) | {0, 12678, 13569, 235789}                             |                    |
| 9521:172  | $0, 0, 0, 0, e^{12}, e^{13}, e^{23}, e^{25} + e^{14}, e^{16} + e^{28} + e^{45}$                                                                                    | 1/317(125, 116, 223, 232, 241, 348, 339, 357, 473) | {0, 12678, 135789, 23569}                             |                    |
| 9521:173  | $0, 0, 0, 0, e^{12}, e^{13}, e^{24}, e^{25} + e^{14}, e^{16} + e^{28} + e^{45}$                                                                                    | 3/221(28, 27, 53, 54, 55, 81, 81, 82, 109)         | {0, 12678, 13589, 235679}                             |                    |
| 9521:174  | $0, 0, 0, 0, e^{12}, e^{13}, e^{14}, e^{15} + e^{23}, e^{47} + e^{18} + e^{26}$                                                                                    | 5/123(8, 14, 16, 15, 22, 24, 23, 30, 38)           | {0, 14569, 15679, 47}                                 |                    |
| 9521:175  | $0, 0, 0, 0, e^{12}, e^{13}, e^{24}, e^{15} + e^{23}, e^{18} + e^{26} + e^{47}$                                                                                    | 1/17(6, 8, 12, 9, 14, 18, 17, 20, 26)              | {0, 24589, 25789, 47}                                 |                    |
| 9521:177  | $0, 0, 0, 0, e^{12}, e^{13}, e^{34}, e^{15}, e^{35} + e^{47} + e^{26} + e^{18}$                                                                                    | 5/33(2, 4, 4, 3, 6, 6, 7, 8, 10)                   | {0, 124678, 1268, 47}                                 |                    |
| 9521:184  | $0, 0, 0, 0, e^{12}, e^{13}, e^{14} - e^{23}, e^{34} + e^{25}, e^{47} + e^{28} + e^{16}$                                                                           | 14/155(5, 4, 7, 6, 9, 12, 11, 13, 17)              | {0, 135789}                                           |                    |
| 9521:188  | $0, 0, 0, 0, e^{12}, e^{34}, e^{14} + e^{23}, e^{25} + e^{13}, e^{46} + e^{28} + e^{17}$                                                                           | 35/324(5, 3, 6, 4, 8, 10, 9, 11, 14)               | {0, 1278}                                             |                    |
| 9521:189  | $0, 0, 0, 0, e^{12}(-1 + a_2), e^{14} + e^{23}, e^{34}, a_2e^{13} + e^{25}, e^{35} + e^{28} + e^{16}$                                                              | 1/92(41, 31, 62, 52, 72, 93, 114, 103, 134)        | {0, 1268, 145789, 245679}                             |                    |
| 9521:197  | $0, 0, 0, 0, e^{12}, e^{13}, e^{24}, e^{15}, e^{18} + e^{26} + e^{35} + e^{47}$                                                                                    | 1/17(6, 8, 12, 9, 14, 18, 17, 20, 26)              | {0, 24589, 25789, 47}                                 |                    |
| 9521:198a | $0, 0, 0, 0, e^{12}, e^{24} + e^{13}, e^{14} + e^{23}, e^{15}, e^{18} + e^{26} + e^{35}$                                                                           | 7/19(1, 1, 2, 2, 2, 3, 3, 4)                       | {0, 12678, 14569, 245789}                             |                    |
| 9521:198b | $0, 0, 0, 0, -e^{12}, -e^{13} + e^{24}, e^{14} + e^{23}, e^{15}, e^{18} + e^{26} + e^{35}$                                                                         | 7/19(1, 1, 2, 2, 2, 3, 3, 4)                       | {0, 12678, 14569, 245789}                             |                    |
| 9521:199  | $0, 0, 0, 0, a_1e^{12}, e^{23} + (1 + a_1)e^{14}, e^{13}, e^{15} + e^{24}, e^{18} + e^{26} + e^{45}$                                                               | 1/317(116, 125, 223, 232, 241, 348, 339, 357, 473) | {0, 12678, 13569, 235789}                             |                    |

Table A.4 – Continued to next page

Table A.4 – Continued from previous page

| Name     | g                                                                                                               | N                                                    | S <sub>0</sub>                                            | S = S <sub>0</sub> |
|----------|-----------------------------------------------------------------------------------------------------------------|------------------------------------------------------|-----------------------------------------------------------|--------------------|
| 9521:200 | $0, 0, 0, 0, e^{12}, e^{13}, e^{23} + e^{14}, e^{24} + e^{15}, e^{36} + e^{27} + e^{18}$                        | $65/549(3, 4, 5, 6, 7, 8, 9, 10, 13)$                | $\{0, 13579\}$                                            |                    |
| 9521:201 | $0, 0, 0, 0, e^{12}, e^{34}, e^{24} + e^{13}, e^{15}, e^{18} + e^{46} + e^{27} + e^{35}$                        | $35/324(3, 5, 6, 4, 8, 10, 9, 11, 14)$               | $\{0, 1278\}$                                             |                    |
| 9521:203 | $0, 0, 0, 0, e^{12}(-1 + a_2), a_2 e^{13}, e^{34}, e^{23} + e^{15}, e^{18} + e^{26} + e^{47} + e^{35}$          | $5/33(2, 4, 4, 3, 6, 6, 7, 8, 10)$                   | $\{0, 124678, 1268, 47\}$                                 |                    |
| 9521:204 | $0, 0, 0, 0, e^{12}, e^{13}(-1 + a_2), a_2 e^{14}, e^{15} + e^{34}, e^{25} + e^{18} + e^{37} + e^{46}$          | $25/81(1, 2, 2, 2, 3, 3, 4, 5)$                      | $\{0, 13459, 15679, 3467\}$                               |                    |
| 9521:205 | $0, 0, 0, 0, e^{12}, e^{13}, e^{34}, e^{14} + e^{25}, e^{45} + e^{16} + e^{28} + e^{37}$                        | $35/324(5, 3, 4, 6, 8, 9, 10, 11, 14)$               | $\{0, 1268\}$                                             |                    |
| 9521:208 | $0, 0, 0, 0, e^{12}, e^{13}, e^{14} + e^{23}, e^{15}, e^{36} + e^{27} + e^{18} + e^{45}$                        | $65/549(3, 4, 5, 6, 7, 8, 9, 10, 13)$                | $\{0, 13579\}$                                            |                    |
| 9521:210 | $0, 0, 0, 0, e^{12}, e^{13}, e^{23}, e^{25} + e^{14}, e^{16} + e^{28} + e^{37} + e^{45}$                        | $65/549(4, 3, 5, 6, 7, 9, 8, 10, 13)$                | $\{0, 23569\}$                                            |                    |
| 9521:211 | $0, 0, 0, 0, e^{12}(-1 + a_2), a_2 e^{13}, e^{14}, e^{15} + e^{23}, e^{18} + e^{26} + e^{35} + e^{47}$          | $5/123(8, 14, 16, 15, 22, 24, 23, 30, 38)$           | $\{0, 14569, 15679, 47\}$                                 |                    |
| 9521:212 | $0, 0, 0, 0, a_1 e^{12}, (1 + a_1) e^{13}, e^{24}, e^{15} + e^{23}, e^{18} + e^{26} + e^{35} + e^{47}$          | $1/17(6, 8, 12, 9, 14, 18, 17, 20, 26)$              | $\{0, 24589, 25789, 47\}$                                 |                    |
| 9521:215 | $0, 0, 0, 0, e^{12}(-1 + a_2), e^{34}, e^{14} + e^{23}, a_2 e^{13} + e^{25}, e^{17} + e^{46} + e^{35} + e^{28}$ | $35/324(5, 3, 6, 4, 8, 10, 9, 11, 14)$               | $\{0, 1278\}$                                             |                    |
| 9521:218 | $0, 0, 0, 0, a_1 e^{12}, e^{13}, e^{23} + (1 + a_1) e^{14}, e^{24} + e^{15}, e^{36} + e^{45} + e^{27} + e^{18}$ | $65/549(3, 4, 5, 6, 7, 8, 9, 10, 13)$                | $\{0, 13579\}$                                            |                    |
| 9521:254 | $0, 0, 0, 0, e^{12}, -e^{13}, e^{14} + e^{23}, -2e^{17} + e^{26} + e^{35}, e^{56} + e^{18}$                     | $1/72(14, 39, 39, 64, 53, 53, 78, 92, 106)$          | $\{0, 12348, 12679, 13579, 14568, 2356, 245789, 346789\}$ |                    |
| 964:3    | $0, 0, 0, e^{12}, e^{13}, e^{14}, e^{24}, e^{15}, e^{34} + e^{25}$                                              | $1/179(55, 80, 104, 135, 159, 190, 215, 214, 239)$   | $\{0, 1236789, 12567, 13478, 14579, 234568, 2469, 3589\}$ |                    |
| 964:4    | $0, 0, 0, e^{12}, e^{13}, e^{14}, e^{24}, e^{35}, e^{25} + e^{34}$                                              | $1/109(41, 45, 48, 86, 89, 127, 131, 137, 134)$      | $\{0, 1236789, 125678, 13478, 145789, 23456, 2469, 359\}$ |                    |
| 964:8a   | $0, 0, 0, e^{12}, e^{13}, e^{14}, e^{15}, e^{25} + e^{34}, e^{35} + e^{24}$                                     | $1/41(13, 20, 20, 33, 33, 46, 46, 53, 53)$           | $\{0, 1236789, 12569, 13479, 14589, 234567, 2468, 3578\}$ | ✓                  |
| 964:8b   | $0, 0, 0, -e^{12}, e^{13}, e^{14}, e^{15}, -e^{25} + e^{34}, e^{24} + e^{35}$                                   | $1/41(13, 20, 20, 33, 33, 46, 46, 53, 53)$           | $\{0, 1236789, 12569, 13479, 14589, 234567, 2468, 3578\}$ | ✓                  |
| 953:28   | $0, 0, 0, 0, e^{12} a_1, e^{13}, e^{25}, e^{15} + e^{24}, e^{34} + e^{16}$                                      | $1/11(4, 5, 7, 8, 9, 11, 14, 13, 15)$                | $\{0, 123789, 12678, 13579, 1567, 235689, 258, 369\}$     | ✓                  |
| 953:59   | $0, 0, 0, 0, e^{12}, e^{13}, e^{15}, e^{25} + e^{14}, e^{26} + e^{35}$                                          | $1/61(21, 27, 38, 54, 48, 59, 69, 75, 86)$           | $\{0, 123789, 12678, 1358, 15689, 23567, 2579, 369\}$     |                    |
| 953:60   | $0, 0, 0, 0, e^{12}, e^{13}, e^{25}, e^{15} + e^{24}, e^{26} + e^{35}$                                          | $3/61(9, 7, 12, 18, 16, 21, 23, 25, 28)$             | $\{0, 123789, 12678, 1357, 15679, 23568, 2589, 369\}$     |                    |
| 953:61   | $0, 0, 0, 0, e^{12}, e^{13}, e^{15}, e^{34} + e^{25}, e^{35} + e^{26}$                                          | $2/31(6, 7, 8, 12, 13, 14, 19, 20, 21)$              | $\{0, 123789, 124678, 1358, 145689, 234567, 2579, 3469\}$ |                    |
| 953:62   | $0, 0, 0, 0, e^{12}, e^{13}, e^{25}, e^{34} + e^{15}, e^{35} + e^{26}$                                          | $1/106(50, 38, 53, 85, 88, 103, 126, 138, 141)$      | $\{0, 123789, 124678, 13457, 15679, 23568, 24589, 3469\}$ |                    |
| 953:67   | $0, 0, 0, 0, e^{12}, e^{13}, e^{25}, e^{36}, e^{14} + e^{26} + e^{35}$                                          | $3/7(1, 1, 1, 2, 2, 2, 3, 3)$                        | $\{0, 123789, 124678, 134578, 156789, 2356, 2459, 3469\}$ |                    |
| 953:69   | $0, 0, 0, 0, e^{12}, e^{13}, e^{15}, e^{16} + e^{24}, e^{26} + e^{35}$                                          | $1/100(35, 46, 58, 82, 81, 93, 116, 128, 139)$       | $\{0, 123789, 12467, 13458, 1569, 235678, 24579, 34689\}$ |                    |
| 953:71   | $0, 0, 0, 0, e^{12}, e^{13}, e^{25}, e^{16} + e^{24}, e^{26} + e^{35}$                                          | $1/106(40, 43, 58, 95, 83, 98, 126, 138, 141)$       | $\{0, 123789, 12467, 134578, 15679, 23568, 2459, 34689\}$ |                    |
| 953:75   | $0, 0, 0, 0, e^{12}, e^{13}, e^{15}, e^{14} + e^{36}, e^{26} + e^{35}$                                          | $1/179(57, 101, 84, 168, 158, 141, 215, 225, 242)$   | $\{0, 123789, 12678, 1358, 15689, 23567, 2579, 369\}$     |                    |
| 953:77   | $0, 0, 0, 0, e^{12}, e^{13}, e^{15}, e^{24} + e^{36}, e^{35} + e^{26}$                                          | $1/225(84, 106, 107, 192, 190, 191, 274, 298, 297)$  | $\{0, 123789, 12678, 13458, 145689, 234567, 24579, 369\}$ |                    |
| 953:79   | $0, 0, 0, 0, e^{12}, e^{13}, e^{25}, e^{36} + e^{14}, e^{35} + e^{26}$                                          | $1/25(11, 10, 11, 22, 21, 22, 31, 33, 32)$           | $\{0, 123789, 12678, 13578, 156789, 2356, 259, 369\}$     |                    |
| 953:80   | $0, 0, 0, 0, e^{12}, e^{13}, e^{25}, e^{34} + e^{16}, e^{26} + e^{35}$                                          | $1/69(29, 28, 33, 58, 57, 62, 85, 91, 90)$           | $\{0, 123789, 1267, 13578, 15679, 23568, 259, 3689\}$     |                    |
| 953:81   | $0, 0, 0, 0, e^{12}, e^{13}, e^{25}, e^{36} + e^{24}, e^{35} + e^{26}$                                          | $1/31(16, 11, 12, 29, 27, 28, 38, 40, 39)$           | $\{0, 123789, 12678, 134578, 1456789, 23456, 2459, 369\}$ |                    |
| 953:101a | $0, 0, 0, 0, e^{12}, e^{13}, e^{24} + e^{15}, e^{25} + e^{14}, e^{26} + e^{35}$                                 | $1/5(2, 2, 3, 4, 4, 5, 6, 6, 7)$                     | $\{0, 123789, 12678, 1358, 15689, 23567, 2579, 369\}$     |                    |
| 953:101b | $0, 0, 0, 0, e^{12}, e^{13}, -e^{15} + e^{24}, e^{25} + e^{14}, e^{26} + e^{35}$                                | $1/5(2, 2, 3, 4, 4, 5, 6, 6, 7)$                     | $\{0, 123789, 12678, 1358, 15689, 23567, 2579, 369\}$     |                    |
| 953:102  | $0, 0, 0, 0, e^{12}, e^{13}, e^{25} + e^{14}, e^{34} + e^{15}, e^{26} + e^{35}$                                 | $1/377(169, 145, 193, 290, 314, 362, 459, 483, 507)$ | $\{0, 123789, 15679, 23568\}$                             |                    |
| 953:112  | $0, 0, 0, 0, e^{12} a_1, e^{13}, e^{25}, e^{34} + e^{16}, e^{15} + e^{36} + e^{24}$                             | $1/67(28, 30, 29, 56, 58, 57, 88, 85, 86)$           | $\{0, 123789, 12679, 368\}$                               |                    |
| 953:116  | $0, 0, 0, 0, e^{12}, e^{13}, e^{25} + e^{14}, e^{16} + e^{24}, e^{26} + e^{35}$                                 | $1/377(137, 161, 209, 322, 298, 346, 459, 483, 507)$ | $\{0, 123789, 15679, 23568\}$                             |                    |
| 953:118a | $0, 0, 0, 0, e^{12}, e^{13}, e^{15} a_1 + e^{24}, e^{34} + e^{16}, e^{25} + e^{36}$                             | $1/8(3, 4, 4, 6, 7, 7, 10, 10, 11)$                  | $\{0, 123789, 12679, 13589, 1569, 235678, 257, 368\}$     |                    |
| 953:118b | $0, 0, 0, 0, -e^{12}, e^{13}, e^{15} a_1 + e^{24}, e^{16} + e^{34}, e^{36} + e^{25}$                            | $1/8(3, 4, 4, 6, 7, 7, 10, 10, 11)$                  | $\{0, 123789, 12679, 13589, 1569, 235678, 257, 368\}$     |                    |
| 953:119a | $0, 0, 0, 0, e^{12}, e^{13}, e^{24} + e^{15}, e^{36} + e^{14}, e^{26} + e^{35}$                                 | $2/29(6, 7, 6, 12, 13, 12, 19, 18, 19)$              | $\{0, 123789, 12678, 1358, 15689, 23567, 2579, 369\}$     | ✓                  |
| 953:119b | $0, 0, 0, 0, e^{12}, e^{13}, -e^{15} + e^{24}, e^{14} + e^{36}, e^{26} + e^{35}$                                | $2/29(6, 7, 6, 12, 13, 12, 19, 18, 19)$              | $\{0, 123789, 12678, 1358, 15689, 23567, 2579, 369\}$     | ✓                  |
| 953:120  | $0, 0, 0, 0, e^{12}, e^{13}, a_2 e^{15} + e^{24}, e^{16} + e^{34}, e^{26} + e^{35}$                             | $1/8(3, 4, 4, 6, 7, 7, 10, 10, 11)$                  | $\{0, 123789, 1267, 1358, 1569, 235678, 2579, 3689\}$     |                    |
| 953:121  | $0, 0, 0, 0, e^{12}, e^{13}, e^{25} + e^{14}, e^{36} + e^{24}, e^{26} + e^{35}$                                 | $1/187(85, 79, 76, 158, 164, 161, 243, 237, 240)$    | $\{0, 123789, 12678, 369\}$                               |                    |
| 953:122a | $0, 0, 0, 0, e^{12}, e^{13}, e^{15} a_1 + e^{34}, e^{16} + e^{24}, e^{36} + e^{25}$                             | $1/8(3, 4, 4, 6, 7, 7, 10, 10, 11)$                  | $\{0, 123789, 124679, 134589, 1569, 235678, 2457, 3468\}$ |                    |
| 953:122b | $0, 0, 0, 0, -e^{12}, e^{13}, e^{15} a_1 + e^{34}, e^{16} + e^{24}, e^{36} + e^{25}$                            | $1/8(3, 4, 4, 6, 7, 7, 10, 10, 11)$                  | $\{0, 123789, 124679, 134589, 1569, 235678, 2457, 3468\}$ |                    |
| 953:123a | $0, 0, 0, 0, e^{12}, e^{13}, e^{34} + e^{15}, e^{24} + e^{16}, e^{35} + e^{26}$                                 | $1/8(3, 4, 4, 6, 7, 7, 10, 10, 11)$                  | $\{0, 123789, 12467, 13458, 1569, 235678, 24579, 34689\}$ | ✓                  |
| 953:123b | $0, 0, 0, 0, e^{12}, e^{13}, -e^{15} + e^{34}, e^{24} + e^{16}, e^{35} + e^{26}$                                | $1/8(3, 4, 4, 6, 7, 7, 10, 10, 11)$                  | $\{0, 123789, 12467, 13458, 1569, 235678, 24579, 34689\}$ | ✓                  |
| 953:125  | $0, 0, 0, 0, e^{12}, e^{13}, e^{25} + e^{34}, e^{24} + e^{16}, e^{26} + e^{35}$                                 | $1/425(167, 191, 203, 346, 358, 370, 549, 537, 561)$ | $\{0, 123789, 12467, 34689\}$                             |                    |
| 953:126  | $0, 0, 0, 0, e^{12}, e^{13}, e^{34} + e^{25}, e^{36} + e^{24}, e^{35} + e^{26}$                                 | $1/19(10, 7, 7, 17, 17, 17, 24, 24, 24)$             | $\{0, 123789, 1456789, 23456\}$                           |                    |
| 953:145a | $0, 0, 0, 0, e^{12}, e^{13}, e^{15}, e^{36} + e^{25}, e^{14} + e^{26} + e^{35}$                                 | $1/89(31, 43, 43, 86, 74, 74, 105, 117, 117)$        | $\{0, 123789, 124678, 13458, 15689, 23567, 24579, 3469\}$ | ✓                  |

Table A.4 – Continued to next page

Table A.4 – Continued from previous page

| Name     | g                                                                                                                  | N                                                    | S <sub>0</sub>                                                                                                | S = S <sub>0</sub> |
|----------|--------------------------------------------------------------------------------------------------------------------|------------------------------------------------------|---------------------------------------------------------------------------------------------------------------|--------------------|
| 953:145b | $0, 0, 0, 0, e^{12}, e^{13}, e^{15}, -e^{25} + e^{36}, e^{14} + e^{26} + e^{35}$                                   | $1/89(31, 43, 43, 86, 74, 74, 105, 117, 117)$        | $\{0, 123789, 124678, 13458, 15689, 23567, 24579, 3469\}$                                                     | ✓                  |
| 953:146a | $0, 0, 0, 0, e^{12}, e^{13}, e^{15}, e^{35} + e^{26}, e^{25} + e^{36} + e^{14}$                                    | $1/89(31, 43, 43, 86, 74, 74, 105, 117, 117)$        | $\{0, 123789, 12679, 1359, 15689, 23567, 2578, 368\}$                                                         | ✓                  |
| 953:146b | $0, 0, 0, 0, -e^{12}, e^{13}, e^{15}, e^{35} - e^{26}, e^{36} + e^{14} + e^{25}$                                   | $1/89(31, 43, 43, 86, 74, 74, 105, 117, 117)$        | $\{0, 123789, 12679, 1359, 15689, 23567, 2578, 368\}$                                                         | ✓                  |
| 953:149  | $0, 0, 0, 0, e^{12}, e^{13}, e^{25}, e^{26} + e^{35}, e^{15} + e^{36} + e^{24}$                                    | $1/19(9, 7, 8, 18, 16, 17, 23, 24, 25)$              | $\{0, 123789, 12679, 368\}$                                                                                   |                    |
| 953:151  | $0, 0, 0, 0, e^{12}, e^{13}, e^{14} + e^{25}, e^{15} + e^{36}, e^{26} + e^{35}$                                    | $1/187(77, 83, 80, 166, 160, 157, 243, 237, 240)$    | $\{0, 123789, 12678, 369\}$                                                                                   |                    |
| 953:152a | $0, 0, 0, 0, e^{12}, e^{13}, e^{15} + e^{24}, e^{35} + e^{26}, e^{36} + e^{25}$                                    | $3/7(1, 1, 1, 2, 2, 2, 3, 3, 3)$                     | $\{0, 123789, 12679, 1359, 15689, 23567, 2578, 368\}$                                                         | ✓                  |
| 953:152b | $0, 0, 0, 0, -e^{12}, e^{13}, e^{24} + e^{15}, e^{35} - e^{26}, e^{25} + e^{36}$                                   | $3/7(1, 1, 1, 2, 2, 2, 3, 3, 3)$                     | $\{0, 123789, 12679, 1359, 15689, 23567, 2578, 368\}$                                                         | ✓                  |
| 953:153  | $0, 0, 0, 0, e^{12}, e^{13}, e^{15} + e^{34}, e^{16} + e^{25}, e^{35} + e^{26}$                                    | $1/425(175, 187, 199, 338, 362, 374, 537, 549, 561)$ | $\{0, 123789, 13458, 24579\}$                                                                                 |                    |
| 953:154a | $0, 0, 0, 0, e^{12}, e^{13}, e^{34} + e^{15}, e^{26} + e^{35}, e^{36} + e^{25}$                                    | $3/7(1, 1, 1, 2, 2, 2, 3, 3, 3)$                     | $\{0, 123789, 124679, 13459, 15689, 23567, 24578, 3468\}$                                                     | ✓                  |
| 953:154b | $0, 0, 0, 0, -e^{12}, e^{13}, e^{15} + e^{34}, -e^{26} + e^{35}, e^{25} + e^{36}$                                  | $3/7(1, 1, 1, 2, 2, 2, 3, 3, 3)$                     | $\{0, 123789, 124679, 13459, 15689, 23567, 24578, 3468\}$                                                     | ✓                  |
| 953:155  | $0, 0, 0, 0, e^{12}, e^{13}, e^{34} + e^{25}, e^{36} + e^{15}, e^{26} + e^{35}$                                    | $3/7(1, 1, 1, 2, 2, 2, 3, 3, 3)$                     | $\{0, 123789, 124678, 3469\}$                                                                                 |                    |
| 953:177a | $0, 0, 0, 0, e^{12}, e^{13}, e^{25} + e^{14}, e^{26} + e^{35}, e^{15} + e^{24} + e^{36}$                           | $3/7(1, 1, 1, 2, 2, 2, 3, 3, 3)$                     | $\{0, 123789, 12679, 368\}$                                                                                   |                    |
| 953:177b | $0, 0, 0, 0, e^{12}, e^{13}, e^{25} - e^{14}, e^{35} + e^{26}, e^{24} + e^{36} + e^{15}$                           | $3/7(1, 1, 1, 2, 2, 2, 3, 3, 3)$                     | $\{0, 123789, 12679, 368\}$                                                                                   |                    |
| 953:179  | $0, 0, 0, 0, e^{12}, e^{13}, a_2 e^{15} + e^{24}, e^{26} + e^{35}, e^{16} + e^{25} + e^{34}$                       | $2/31(6, 7, 8, 12, 13, 14, 19, 21, 20)$              | $\{0, 123789, 1359, 2578\}$                                                                                   |                    |
| 953:183  | $0, 0, 0, 0, e^{12}, e^{13}, e^{25} + e^{34}, a_2 e^{15} + e^{36}, e^{14} + e^{26} + e^{35}$                       | $3/7(1, 1, 1, 2, 2, 2, 3, 3, 3)$                     | $\{0, 123789, 124678, 3469\}$                                                                                 |                    |
| 953:195  | $0, 0, 0, 0, e^{12}, e^{13}, e^{26} + e^{35}, a_2 e^{16} + e^{34} + e^{25}, e^{15} + e^{36} + e^{24}$              | $3/7(1, 1, 1, 2, 2, 2, 3, 3, 3)$                     | $\{0, 123789\}$                                                                                               |                    |
| 953:196  | $0, 0, 0, 0, e^{12}, e^{13}, a_2 e^{16} + e^{25} + e^{34}, e^{26} + e^{35} + a_3 e^{14}, e^{15} + e^{36} + e^{24}$ | $3/7(1, 1, 1, 2, 2, 2, 3, 3, 3)$                     | $\{0, 123789\}$                                                                                               |                    |
| 953:202  | $0, 0, 0, 0, -e^{12}, e^{14} + e^{23}, e^{15}, e^{25}, e^{16} + e^{35}$                                            | $1/179(55, 80, 119, 144, 135, 199, 190, 215, 254)$   | $\{0, 1234789, 12678, 13568, 14589, 2357, 245679, 3469\}$                                                     |                    |
| 953:214  | $0, 0, 0, 0, e^{12}, e^{23} + e^{14}, e^{15}, e^{13} + e^{25}, e^{45} + e^{26}$                                    | $1/178(73, 64, 128, 119, 137, 192, 210, 201, 256)$   | $\{0, 12678, 1458, 24567\}$                                                                                   |                    |
| 953:215  | $0, 0, 0, 0, -e^{12}, e^{14} + e^{23}, e^{15}, e^{25} + e^{34}, e^{35} + e^{16}$                                   | $1/41(13, 20, 23, 30, 33, 43, 46, 53, 56)$           | $\{0, 13568, 14589, 3469\}$                                                                                   |                    |
| 953:217  | $0, 0, 0, 0, -e^{12}, e^{23} - e^{14}, e^{15}, e^{16} + e^{35}, e^{26} + e^{45}$                                   | $1/31(11, 12, 19, 20, 23, 31, 34, 42, 43)$           | $\{0, 1234789, 1267, 13569, 1458, 23579, 245678, 34689\}$                                                     |                    |
| 953:229  | $0, 0, 0, 0, e^{12}, e^{14} + e^{23}, e^{13} + e^{25}, e^{34} + e^{15}, e^{45} + e^{26}$                           | $67/581(4, 3, 6, 5, 7, 9, 10, 11, 12)$               | $\{0, 24568\}$                                                                                                |                    |
| 953:233  | $0, 0, 0, 0, -e^{12}, -e^{14} + e^{23}, e^{34} + e^{15}, e^{35} + e^{16}, e^{45} + e^{26}$                         | $1/329(124, 133, 186, 195, 257, 319, 381, 443, 452)$ | $\{0, 23579, 245678, 34689\}$                                                                                 |                    |
| 953:241a | $0, 0, 0, 0, e^{14} + e^{23}, e^{24} + e^{13}, e^{16} + e^{25}, e^{15} + e^{26}, e^{35} + e^{46}$                  | $1/33(13, 13, 16, 16, 29, 29, 42, 42, 45)$           | $\{0, 1234789, 12569, 1357, 1468, 23679, 24589, 345678\}$                                                     |                    |
| 953:241b | $0, 0, 0, 0, -e^{14} - e^{23}, -e^{13} + e^{24}, e^{25} - e^{16}, e^{26} + e^{15}, e^{46} + e^{35}$                | $1/33(13, 13, 16, 16, 29, 29, 42, 42, 45)$           | $\{0, 1234789, 12569, 1357, 1468, 23679, 24589, 345678\}$                                                     |                    |
| 952:83   | $0, 0, 0, 0, e^{12}, e^{13}, e^{14}, e^{15}, e^{35} + e^{26}$                                                      | $1/13(4, 7, 8, 11, 11, 12, 15, 15, 19)$              | $\{0, 123489, 123789, 12468, 12678, 1345, 1357, 14569, 15679, 2345678, 23568, 245789, 2589, 34679, 369, 47\}$ |                    |
| 952:85   | $0, 0, 0, 0, e^{12}, e^{13}, e^{14}, e^{25}, e^{35} + e^{26}$                                                      | $1/5(2, 2, 3, 4, 4, 5, 6, 6, 7)$                     | $\{0, 123489, 123789, 12468, 12678, 13458, 13578, 145689, 156789, 234567, 2356, 24579, 259, 34679, 369, 47\}$ |                    |
| 952:87   | $0, 0, 0, 0, e^{12}, e^{13}, e^{24}, e^{15}, e^{26} + e^{35}$                                                      | $1/5(2, 2, 3, 4, 4, 5, 6, 6, 7)$                     | $\{0, 123489, 123789, 12468, 12678, 13457, 135, 145679, 1569, 234568, 235678, 24589, 25789, 34679, 369, 47\}$ |                    |
| 952:89   | $0, 0, 0, 0, e^{12}, e^{13}, e^{24}, e^{25}, e^{26} + e^{35}$                                                      | $1/13(7, 4, 7, 11, 11, 14, 15, 15, 18)$              | $\{0, 123489, 123789, 12468, 12678, 134578, 1358, 1456789, 15689, 23456, 23567, 2459, 2579, 34679, 369, 47\}$ |                    |
| 952:92   | $0, 0, 0, 0, e^{12}, e^{13}, e^{34}, e^{15}, e^{26} + e^{35}$                                                      | $1/8(3, 4, 4, 6, 7, 7, 10, 10, 11)$                  | $\{0, 123489, 123789, 124678, 1268, 1345, 1357, 145679, 1569, 234568, 235678, 245789, 2589, 3469, 3679, 47\}$ |                    |
| 952:94   | $0, 0, 0, 0, e^{12}, e^{13}, e^{34}, e^{25}, e^{26} + e^{35}$                                                      | $1/9(5, 3, 4, 7, 8, 9, 11, 11, 12)$                  | $\{0, 123489, 123789, 124678, 1268, 13458, 13578, 1456789, 15689, 23456, 23567, 24579, 259, 3469, 3679, 47\}$ |                    |
| 952:110  | $0, 0, 0, 0, e^{12} a_1, e^{13}, e^{23}, e^{15} + e^{24}, e^{34} + e^{16}$                                         | $1/19(7, 11, 11, 14, 18, 18, 22, 25, 25)$            | $\{0, 12389, 12678, 13579, 156, 235689, 2578, 3679\}$                                                         |                    |
| 952:140  | $0, 0, 0, 0, e^{12}, e^{13}, e^{14}, e^{15} + e^{24}, e^{26} + e^{35}$                                             | $1/61(23, 29, 36, 46, 52, 59, 69, 75, 88)$           | $\{0, 123789, 12678, 1357, 15679, 23568, 2589, 369\}$                                                         |                    |
| 952:142  | $0, 0, 0, 0, e^{12}, e^{13}, e^{24}, e^{25} + e^{14}, e^{26} + e^{35}$                                             | $1/61(29, 23, 34, 46, 52, 63, 69, 75, 86)$           | $\{0, 123789, 12678, 1358, 15689, 23567, 2579, 369\}$                                                         |                    |
| 952:146  | $0, 0, 0, 0, e^{12}, e^{13}, e^{14}, e^{15} + e^{34}, e^{35} + e^{26}$                                             | $1/51(19, 27, 27, 38, 46, 46, 57, 65, 73)$           | $\{0, 123789, 12468, 1345, 15679, 23568, 245789, 34679\}$                                                     |                    |
| 952:148  | $0, 0, 0, 0, e^{12}, e^{13}, e^{14}, e^{25} + e^{34}, e^{35} + e^{26}$                                             | $1/41(18, 17, 22, 30, 35, 40, 48, 52, 57)$           | $\{0, 123789, 12468, 13578, 145689, 234567, 259, 34679\}$                                                     |                    |
| 952:150  | $0, 0, 0, 0, e^{12}, e^{13}, e^{24}, e^{34} + e^{15}, e^{26} + e^{35}$                                             | $1/100(43, 42, 54, 74, 85, 97, 116, 128, 139)$       | $\{0, 123789, 12468, 13457, 1569, 235678, 24589, 34679\}$                                                     |                    |
| 952:152  | $0, 0, 0, 0, e^{12}, e^{13}, e^{24}, e^{25} + e^{34}, e^{26} + e^{35}$                                             | $1/61(34, 21, 29, 47, 55, 63, 68, 76, 84)$           | $\{0, 123789, 12468, 1358, 1456789, 23456, 2579, 34679\}$                                                     |                    |
| 952:156  | $0, 0, 0, 0, e^{12}, e^{13}, e^{34}, e^{25} + e^{14}, e^{26} + e^{35}$                                             | $1/179(93, 66, 83, 132, 159, 176, 215, 225, 242)$    | $\{0, 123789, 1268, 13578, 15689, 23567, 259, 3679\}$                                                         |                    |
| 952:190  | $0, 0, 0, 0, e^{12}, e^{13}, e^{14}, e^{25} + e^{16}, e^{35} + e^{26}$                                             | $1/41(14, 19, 24, 34, 33, 38, 48, 52, 57)$           | $\{0, 123489, 123789, 13458, 13578, 24579, 259, 47\}$                                                         |                    |
| 952:192  | $0, 0, 0, 0, e^{12}, e^{13}, e^{24}, e^{16} + e^{25}, e^{35} + e^{26}$                                             | $2/31(6, 7, 8, 12, 13, 14, 19, 20, 21)$              | $\{0, 123489, 123789, 134578, 1358, 2459, 2579, 47\}$                                                         |                    |

Table A.4 – Continued to next page

Table A.4 – Continued from previous page

| Name     | g                                                                                                      | N                                                | S <sub>0</sub>                                                                                            | S = S <sub>0</sub> |
|----------|--------------------------------------------------------------------------------------------------------|--------------------------------------------------|-----------------------------------------------------------------------------------------------------------|--------------------|
| 952:193a | $0, 0, 0, 0, e^{12}, e^{13}, e^{14}, e^{26} + e^{35}, e^{36} + e^{25}$                                 | 1/15(6, 7, 7, 12, 13, 13, 18, 20, 20)            | {0, 123489, 123789, 12469, 12679, 13459, 13579, 145689, 156789, 234567, 2356, 24578, 258, 34678, 368, 47} | ✓                  |
| 952:193b | $0, 0, 0, 0, -e^{12}, e^{13}, e^{14}, -e^{26} + e^{35}, e^{25} + e^{36}$                               | 1/15(6, 7, 7, 12, 13, 13, 18, 20, 20)            | {0, 123489, 123789, 12469, 12679, 13459, 13579, 145689, 156789, 234567, 2356, 24578, 258, 34678, 368, 47} | ✓                  |
| 952:194  | $0, 0, 0, 0, e^{12}, e^{13}, e^{24}, e^{36} + e^{15}, e^{26} + e^{35}$                                 | 1/225(100, 98, 99, 176, 198, 199, 274, 298, 297) | {0, 123489, 123789, 12468, 12678, 34679, 369, 47}                                                         |                    |
| 952:195a | $0, 0, 0, 0, e^{12}, e^{13}, e^{24}, e^{26} + e^{35}, e^{25} + e^{36}$                                 | 1/53(29, 20, 20, 43, 49, 49, 63, 69, 69)         | {0, 123489, 123789, 12469, 12679, 134579, 1359, 1456789, 15689, 23456, 23567, 2458, 2578, 34678, 368, 47} | ✓                  |
| 952:195b | $0, 0, 0, 0, -e^{12}, e^{13}, e^{24}, -e^{26} + e^{35}, e^{36} + e^{25}$                               | 1/53(29, 20, 20, 43, 49, 49, 63, 69, 69)         | {0, 123489, 123789, 12469, 12679, 134579, 1359, 1456789, 15689, 23456, 23567, 2458, 2578, 34678, 368, 47} | ✓                  |
| 952:206  | $0, 0, 0, 0, e^{12}a_1, e^{13}, e^{14}, e^{24} + e^{15}, e^{25} + e^{34} + e^{16}$                     | 3/17(2, 3, 4, 4, 5, 6, 6, 7, 8)                  | {0, 123789, 13579, 258}                                                                                   |                    |
| 952:217  | $0, 0, 0, 0, e^{12}a_1, e^{13}, e^{23}, e^{15} + e^{24}, e^{16} + e^{34} + e^{25}$                     | 1/26(10, 13, 16, 20, 23, 26, 29, 33, 36)         | {0, 12389, 13579, 2578}                                                                                   | ✓                  |
| 952:233  | $0, 0, 0, 0, e^{12}, e^{13}, e^{14}, e^{26} + e^{35}, e^{24} + e^{36} + e^{15}$                        | 1/13(5, 7, 6, 10, 12, 11, 15, 18, 17)            | {0, 123789, 12679, 368}                                                                                   |                    |
| 952:236a | $0, 0, 0, 0, e^{12}, e^{13}, e^{24}, e^{36} + e^{25}, e^{14} + e^{26} + e^{35}$                        | 1/89(47, 35, 35, 70, 82, 82, 105, 117, 117)      | {0, 123789, 12468, 134578, 15689, 23567, 2459, 34679}                                                     | ✓                  |
| 952:236b | $0, 0, 0, 0, e^{12}, e^{13}, e^{24}, -e^{25} + e^{36}, e^{26} + e^{35} + e^{14}$                       | 1/89(47, 35, 35, 70, 82, 82, 105, 117, 117)      | {0, 123789, 12468, 134578, 15689, 23567, 2459, 34679}                                                     | ✓                  |
| 952:237a | $0, 0, 0, 0, e^{12}, e^{13}, e^{24}, e^{26} + e^{35}, e^{14} + e^{36} + e^{25}$                        | 1/89(47, 35, 35, 70, 82, 82, 105, 117, 117)      | {0, 123789, 12679, 1359, 15689, 23567, 2578, 368}                                                         | ✓                  |
| 952:237b | $0, 0, 0, 0, -e^{12}, e^{13}, e^{24}, -e^{26} + e^{35}, e^{25} + e^{14} + e^{36}$                      | 1/89(47, 35, 35, 70, 82, 82, 105, 117, 117)      | {0, 123789, 12679, 1359, 15689, 23567, 2578, 368}                                                         | ✓                  |
| 952:239  | $0, 0, 0, 0, e^{12}a_1, e^{13}, e^{23} + e^{14}, e^{24} + e^{15}, e^{16} + e^{25} + e^{34}$            | 21/167(3, 4, 5, 6, 7, 8, 9, 10, 11)              | {0, 13579}                                                                                                |                    |
| 952:260  | $0, 0, 0, 0, e^{12}, e^{13}, e^{23}, e^{15}, e^{17} + e^{26} + e^{34}$                                 | 1/16(6, 8, 9, 14, 14, 15, 17, 20, 23)            | {0, 12389, 12678, 13457, 14569, 234568, 245789, 3679}                                                     |                    |
| 952:266  | $0, 0, 0, 0, e^{12}, e^{13}, e^{23}, e^{15} + e^{34}, e^{17} + e^{26}$                                 | 1/12(5, 6, 6, 10, 11, 11, 12, 16, 17)            | {0, 12389, 124678, 13457, 1569, 23568, 245789, 34679}                                                     |                    |
| 952:279a | $0, 0, 0, 0, e^{12}a_1, e^{13}, e^{23}, e^{14} + e^{25}, e^{27} + e^{16} + e^{34}$                     | 1/7(3, 3, 4, 6, 6, 7, 7, 9, 10)                  | {0, 12389, 12678, 135789, 1568, 23569, 257, 3679}                                                         |                    |
| 952:279b | $0, 0, 0, 0, e^{12}a_1, -e^{13}, e^{23}, e^{25} + e^{14}, e^{34} + e^{27} + e^{16}$                    | 1/7(3, 3, 4, 6, 6, 7, 7, 9, 10)                  | {0, 12389, 12678, 135789, 1568, 23569, 257, 3679}                                                         |                    |
| 952:284  | $0, 0, 0, 0, (-1 + a_2)e^{12}, a_2e^{13}, e^{23}, e^{25} + e^{14}, e^{17} + e^{26} + e^{35}$           | 1/7(3, 3, 4, 6, 6, 7, 7, 9, 10)                  | {0, 12389, 12678, 13578, 15689, 2356, 2579, 3679}                                                         |                    |
| 952:286  | $0, 0, 0, 0, e^{12}a_1, (1 + a_1)e^{13}, e^{23}, e^{15} + e^{34}, e^{17} + e^{26} + e^{35}$            | 1/12(5, 6, 6, 10, 11, 11, 12, 16, 17)            | {0, 12389, 124678, 13457, 1569, 23568, 245789, 34679}                                                     |                    |
| 952:289  | $0, 0, 0, 0, -e^{12}, e^{13}, e^{23}, e^{16} + e^{25}, e^{17} + e^{24} + e^{35}$                       | 1/88(34, 41, 48, 82, 75, 82, 89, 116, 123)       | {0, 12389, 13578, 2579}                                                                                   |                    |
| 952:290  | $0, 0, 0, 0, e^{12}, e^{13}a_1, e^{23}, e^{15} + e^{36}, e^{25} + e^{14} + e^{37}$                     | 1/59(26, 28, 27, 56, 54, 53, 55, 80, 82)         | {0, 12389, 126789, 367}                                                                                   |                    |
| 952:291  | $0, 0, 0, 0, -e^{12}, e^{13}, e^{23}, e^{36} + e^{15}, e^{35} + e^{24} + e^{17}$                       | 1/197(81, 103, 92, 173, 184, 173, 195, 265, 276) | {0, 12389, 124678, 34679}                                                                                 |                    |
| 952:294a | $0, 0, 0, 0, -e^{12}, e^{13}, e^{23}, e^{36} + e^{25}, e^{35} + e^{24} + e^{17}$                       | 1/53(25, 24, 24, 49, 49, 49, 48, 73, 73)         | {0, 12389, 124678, 13578, 145689, 23456, 2579, 34679}                                                     |                    |
| 952:294b | $0, 0, 0, 0, -e^{12}, -e^{13}, e^{23}, e^{36} + e^{25}, e^{24} + e^{35} + e^{17}$                      | 1/53(25, 24, 24, 49, 49, 49, 48, 73, 73)         | {0, 12389, 124678, 13578, 145689, 23456, 2579, 34679}                                                     |                    |
| 952:295  | $0, 0, 0, 0, e^{12}, e^{13}, e^{23}, e^{35} + e^{26}, e^{37} + e^{25} + e^{14}$                        | 1/71(35, 31, 33, 62, 66, 68, 64, 99, 97)         | {0, 12389, 12679, 3678}                                                                                   |                    |
| 952:296a | $0, 0, 0, 0, e^{12}, e^{13}, e^{23}, e^{26} + e^{35}, e^{15} + e^{37} + e^{24}$                        | 1/32(15, 14, 15, 30, 29, 30, 29, 44, 44)         | {0, 12389, 12679, 1357, 1568, 23569, 25789, 3678}                                                         |                    |
| 952:296b | $0, 0, 0, 0, -e^{12}, -e^{13}, e^{23}, e^{26} + e^{35}, e^{15} + e^{37} + e^{24}$                      | 1/32(15, 14, 15, 30, 29, 30, 29, 44, 44)         | {0, 12389, 12679, 1357, 1568, 23569, 25789, 3678}                                                         |                    |
| 952:297  | $0, 0, 0, 0, e^{12}, e^{13}, e^{23}, e^{26} + e^{35}, e^{15} + e^{34} + e^{27}$                        | 1/71(33, 31, 35, 62, 64, 68, 66, 99, 97)         | {0, 12389, 1568, 23569}                                                                                   |                    |
| 952:302a | $0, 0, 0, 0, e^{12}, e^{13}, e^{23}, e^{15}a_1 + e^{36} + e^{24}, e^{37} + e^{25} + e^{14}$            | 17/37(1, 1, 1, 2, 2, 2, 2, 3, 3)                 | {0, 12389, 126789, 367}                                                                                   | ✓                  |
| 952:302b | $0, 0, 0, 0, e^{12}, -e^{13}, e^{23}, e^{15}a_1 + e^{24} + e^{36}, e^{25} + e^{37} + e^{14}$           | 17/37(1, 1, 1, 2, 2, 2, 2, 3, 3)                 | {0, 12389, 126789, 367}                                                                                   | ✓                  |
| 952:303a | $0, 0, 0, 0, e^{12}, e^{13}, e^{23}, e^{14}a_1 + e^{36} + e^{25}, e^{24} + e^{37} + e^{15}$            | 17/37(1, 1, 1, 2, 2, 2, 2, 3, 3)                 | {0, 12389, 126789, 13578, 1568, 23569, 2579, 367}                                                         | ✓                  |
| 952:303b | $0, 0, 0, 0, e^{12}, -e^{13}, e^{23}, e^{14}a_1 + e^{36} + e^{25}, e^{24} + e^{37} + e^{15}$           | 17/37(1, 1, 1, 2, 2, 2, 2, 3, 3)                 | {0, 12389, 126789, 13578, 1568, 23569, 2579, 367}                                                         | ✓                  |
| 952:303c | $0, 0, 0, 0, -e^{12}, -e^{13}, e^{23}, e^{14}a_1 + e^{25} + e^{36}, e^{37} + e^{15} + e^{24}$          | 17/37(1, 1, 1, 2, 2, 2, 2, 3, 3)                 | {0, 12389, 126789, 13578, 1568, 23569, 2579, 367}                                                         | ✓                  |
| 952:304a | $0, 0, 0, 0, e^{12}, e^{13}, e^{23}, e^{26} + e^{35} + e^{14}, e^{37} + e^{24} + e^{15}$               | 17/37(1, 1, 1, 2, 2, 2, 2, 3, 3)                 | {0, 12389, 1568, 23569}                                                                                   |                    |
| 952:304b | $0, 0, 0, 0, -e^{12}, -e^{13}, e^{23}, e^{26} + e^{35} + e^{14}, e^{15} + e^{37} + e^{24}$             | 17/37(1, 1, 1, 2, 2, 2, 2, 3, 3)                 | {0, 12389, 1568, 23569}                                                                                   |                    |
| 952:305a | $0, 0, 0, 0, e^{12}, e^{13}a_1, e^{23}, e^{16} + e^{25} + e^{34}, e^{15} + e^{24} + e^{37}$            | 17/37(1, 1, 1, 2, 2, 2, 2, 3, 3)                 | {0, 12389, 13578, 2579}                                                                                   |                    |
| 952:305b | $0, 0, 0, 0, -e^{12}, e^{13}a_1, e^{23}, e^{34} + e^{25} + e^{16}, e^{37} + e^{15} + e^{24}$           | 17/37(1, 1, 1, 2, 2, 2, 2, 3, 3)                 | {0, 12389, 13578, 2579}                                                                                   |                    |
| 952:307  | $0, 0, 0, 0, e^{12}, e^{13}a_1, e^{23}, e^{24} + e^{36} + e^{15}, e^{25} + e^{37} + e^{16}$            | 17/37(1, 1, 1, 2, 2, 2, 2, 3, 3)                 | {0, 12389}                                                                                                |                    |
| 952:308  | $0, 0, 0, 0, e^{12}, e^{13}, e^{23}, e^{35} + e^{14} + e^{26}, e^{37} + e^{25} + e^{16}$               | 17/37(1, 1, 1, 2, 2, 2, 2, 3, 3)                 | {0, 12389}                                                                                                |                    |
| 952:309a | $0, 0, 0, 0, (-1 + a_2)e^{12}, a_2e^{13}, e^{23}, e^{14} + e^{36} + e^{25}, e^{26} + e^{35} + e^{17}$  | 1/32(14, 15, 15, 30, 29, 29, 30, 44, 44)         | {0, 12389, 12678, 13578, 15689, 2356, 2579, 3679}                                                         |                    |
| 952:309b | $0, 0, 0, 0, (-1 + a_2)e^{12}, a_2e^{13}, e^{23}, -e^{25} + e^{36} + e^{14}, e^{17} + e^{26} + e^{35}$ | 1/32(14, 15, 15, 30, 29, 29, 30, 44, 44)         | {0, 12389, 12678, 13578, 15689, 2356, 2579, 3679}                                                         |                    |
| 952:310  | $0, 0, 0, 0, e^{12}a_1, (1 + a_1)e^{13}, e^{23}, e^{15} + e^{24} + e^{36}, e^{17} + e^{26} + e^{35}$   | 1/71(31, 35, 33, 62, 66, 64, 68, 97, 99)         | {0, 12389, 12678, 3679}                                                                                   |                    |
| 952:334  | $0, 0, 0, 0, e^{12}, e^{23} + e^{14}, e^{13}, e^{15}, e^{45} + e^{26}$                                 | 1/106(43, 40, 74, 71, 83, 114, 117, 126, 154)    | {0, 123489, 12678, 13569, 1457, 235789, 24568, 34679}                                                     |                    |

Table A.4 – Continued to next page

Table A.4 – Continued from previous page

| Name     | g                                                                                        | N                                                  | S <sub>0</sub>                                                                                            | S = S <sub>0</sub> |
|----------|------------------------------------------------------------------------------------------|----------------------------------------------------|-----------------------------------------------------------------------------------------------------------|--------------------|
| 952:335  | $0, 0, 0, 0, e^{12}, e^{14} + e^{23}, e^{13}, e^{25}, e^{45} + e^{26}$                   | 1/100(46, 35, 72, 61, 81, 107, 118, 116, 142)      | {0, 123489, 12678, 135689, 14578, 23579, 2456, 34679}                                                     |                    |
| 952:336  | $0, 0, 0, 0, -e^{12}, e^{14} + e^{23}, e^{34}, e^{15}, e^{16} + e^{35}$                  | 1/179(55, 104, 83, 132, 159, 187, 215, 214, 242)   | {0, 123489, 1268, 13567, 14579, 23578, 2456789, 3469}                                                     |                    |
| 952:337  | $0, 0, 0, 0, e^{12}, e^{24} + e^{13}, e^{34}, e^{15}, e^{26} + e^{35}$                   | 1/109(48, 41, 62, 69, 89, 110, 131, 137, 151)      | {0, 123489, 1268, 1357, 145679, 235678, 245789, 3469}                                                     |                    |
| 952:365  | $0, 0, 0, 0, e^{12}, e^{14} + e^{23}, e^{13}, e^{15} + e^{34}, e^{26} + e^{45}$          | 1/23(10, 9, 15, 14, 19, 24, 25, 29, 33)            | {0, 235789, 24568, 34679}                                                                                 |                    |
| 952:366  | $0, 0, 0, 0, e^{12}, e^{23} + e^{14}, e^{13}, e^{34} + e^{25}, e^{26} + e^{45}$          | 1/401(195, 148, 269, 222, 343, 417, 464, 491, 565) | {0, 135689, 14578, 34679}                                                                                 |                    |
| 952:370  | $0, 0, 0, 0, -e^{12}, e^{24} + e^{13}, e^{34}, e^{23} + e^{15}, e^{16} + e^{45}$         | 1/160(55, 87, 110, 78, 142, 165, 188, 197, 220)    | {0, 1268, 14567, 24578}                                                                                   |                    |
| 952:374  | $0, 0, 0, 0, -e^{12}, -e^{14} + e^{23}, e^{34}, e^{35} + e^{16}, e^{45} + e^{26}$        | 1/55(23, 23, 30, 30, 46, 53, 60, 76, 76)           | {0, 123489, 126, 135679, 14578, 23579, 245678, 34689}                                                     |                    |
| 952:387a | $0, 0, 0, 0, e^{14} + e^{23}, e^{24} + e^{13}, e^{12}, e^{45} + e^{36}, e^{46} + e^{35}$ | 4/21(3, 3, 2, 2, 5, 5, 6, 7, 7)                    | {0, 123489, 125689, 13578, 14678, 23679, 24579, 3456}                                                     |                    |
| 952:387b | $0, 0, 0, 0, e^{14} - e^{23}, e^{13} + e^{24}, e^{12}, e^{45} - e^{36}, e^{46} + e^{35}$ | 4/21(3, 3, 2, 2, 5, 5, 6, 7, 7)                    | {0, 123489, 125689, 13578, 14678, 23679, 24579, 3456}                                                     |                    |
| 952:409  | $0, 0, 0, 0, e^{12}, e^{13}, e^{14}, e^{15}, e^{46} + e^{37}$                            | 1/8(2, 6, 5, 5, 8, 7, 7, 10, 12)                   | {0, 123489, 12378, 12468, 126789, 13459, 1357, 1456, 15679, 2345678, 235689, 245789, 258, 3467, 369, 479} |                    |
| 952:411  | $0, 0, 0, 0, e^{12}, e^{13}, e^{14}, e^{25}, e^{37} + e^{46}$                            | 1/60(24, 28, 33, 33, 52, 57, 57, 80, 90)           | {0, 123489, 12378, 12468, 126789, 134589, 13578, 14568, 156789, 234567, 23569, 24579, 25, 3467, 369, 479} |                    |
| 952:414  | $0, 0, 0, 0, e^{12}, -e^{13}, e^{34}, e^{15}, e^{17} + e^{46}$                           | 1/8(2, 6, 5, 4, 8, 7, 9, 10, 11)                   | {0, 123489, 12378, 124678, 12689, 13459, 1357, 14567, 1569, 234568, 2356789, 245789, 258, 346, 3679, 479} |                    |
| 952:416  | $0, 0, 0, 0, e^{12}, -e^{13}, e^{34}, e^{25}, e^{17} + e^{46}$                           | 1/60(24, 28, 33, 30, 52, 57, 63, 80, 87)           | {0, 123489, 12378, 124678, 12689, 134589, 13578, 145678, 15689, 23456, 235679, 24579, 25, 346, 3679, 479} |                    |
| 952:421  | $0, 0, 0, 0, e^{12}, e^{13}, e^{14} + e^{23}, e^{15}, e^{46} + e^{37}$                   | 1/28(10, 16, 13, 19, 26, 23, 29, 36, 42)           | {0, 123489, 126789, 1357, 1456, 235689, 245789, 3467}                                                     |                    |
| 952:422  | $0, 0, 0, 0, e^{12}, e^{13}, e^{14} + e^{23}, e^{25}, e^{46} + e^{37}$                   | 1/124(52, 56, 65, 69, 108, 117, 121, 164, 186)     | {0, 123489, 126789, 13578, 14568, 23569, 24579, 3467}                                                     |                    |
| 952:423  | $0, 0, 0, 0, e^{12}, e^{34}, e^{14} + e^{23}, e^{15}, e^{16} + e^{37}$                   | 1/109(34, 69, 41, 76, 103, 117, 110, 137, 151)     | {0, 123489, 12789, 13567, 1456, 235689, 2456789, 347}                                                     |                    |
| 952:424  | $0, 0, 0, 0, e^{12}, e^{34}, e^{24} + e^{13}, e^{15}, e^{37} + e^{26}$                   | 1/233(108, 94, 115, 129, 202, 244, 223, 310, 338)  | {0, 123489, 12789, 13569, 145679, 235678, 24568, 347}                                                     |                    |
| 952:437  | $0, 0, 0, 0, e^{12}, e^{13}, e^{14}, e^{15} + e^{23}, e^{46} + e^{37}$                   | 1/31(9, 22, 18, 19, 31, 27, 28, 40, 46)            | {0, 12468, 126789, 1456, 15679, 245789, 258, 479}                                                         |                    |
| 952:446  | $0, 0, 0, 0, e^{12}, -e^{13}, e^{34}, e^{15} + e^{23}, e^{17} + e^{46}$                  | 1/31(9, 22, 18, 16, 31, 27, 34, 40, 43)            | {0, 124678, 12689, 14567, 1569, 245789, 258, 479}                                                         |                    |
| 952:468  | $0, 0, 0, 0, e^{12}, e^{13}, e^{14}, e^{25}, e^{17} + e^{35} + e^{26}$                   | 1/9(3, 4, 6, 7, 7, 9, 10, 11, 13)                  | {0, 123489, 12678, 13578, 145689, 2356, 24579, 34679}                                                     |                    |
| 952:472  | $0, 0, 0, 0, e^{12}, e^{13}, e^{14}, e^{15}, e^{26} + e^{47} + e^{35}$                   | 1/225(66, 133, 153, 143, 199, 219, 209, 265, 352)  | {0, 123489, 123789, 14569, 15679, 2345678, 23568, 47}                                                     |                    |
| 952:473  | $0, 0, 0, 0, e^{12}, e^{13}, e^{14}, e^{15}, e^{25} + e^{37} + e^{46}$                   | 1/25(7, 16, 16, 16, 23, 23, 23, 30, 39)            | {0, 123489, 126789, 13459, 15679, 2345678, 258, 3467}                                                     |                    |
| 952:476  | $0, 0, 0, 0, e^{12}, e^{13}, e^{14}, e^{25}, e^{26} + e^{35} + e^{47}$                   | 1/40(16, 17, 27, 22, 33, 43, 38, 50, 60)           | {0, 123489, 123789, 145689, 156789, 234567, 2356, 47}                                                     |                    |
| 952:477  | $0, 0, 0, 0, -e^{12}, e^{13}, e^{24}, e^{15}, e^{36} + e^{45} + e^{17}$                  | 1/109(36, 59, 63, 67, 95, 99, 126, 131, 162)       | {0, 123489, 124689, 1359, 1569, 234568, 2458, 36}                                                         |                    |
| 952:479  | $0, 0, 0, 0, e^{12}, e^{13}, e^{24}, e^{15}, e^{35} + e^{47} + e^{26}$                   | 1/49(19, 22, 33, 26, 41, 52, 48, 60, 74)           | {0, 123489, 123789, 13457, 135, 24589, 25789, 47}                                                         |                    |
| 952:481  | $0, 0, 0, 0, e^{12}, -e^{13}, e^{34}, e^{15}, e^{46} + e^{25} + e^{17}$                  | 1/109(34, 63, 67, 59, 97, 101, 126, 131, 160)      | {0, 123489, 12689, 13459, 1569, 234568, 258, 346}                                                         |                    |
| 952:483  | $0, 0, 0, 0, e^{12}, e^{13}, e^{34}, e^{15}, e^{26} + e^{47} + e^{35}$                   | 2/39(7, 11, 11, 9, 18, 18, 20, 25, 29)             | {0, 123489, 123789, 124678, 1268, 3469, 3679, 47}                                                         |                    |
| 952:485  | $0, 0, 0, 0, e^{12}, e^{13}, e^{34}, e^{25}, e^{26} + e^{47} + e^{35}$                   | 2/39(11, 7, 10, 9, 18, 21, 19, 25, 28)             | {0, 123489, 123789, 124678, 1268, 3469, 3679, 47}                                                         |                    |
| 952:488  | $0, 0, 0, 0, e^{12}, e^{13}, e^{14}, e^{26} + e^{35}, e^{17} + e^{25}$                   | 1/25(7, 13, 16, 19, 20, 23, 26, 36, 33)            | {0, 123489, 12469, 13459, 145689, 2356, 258, 368}                                                         |                    |
| 952:490  | $0, 0, 0, 0, e^{12}, e^{13}, e^{24}, e^{26} + e^{35}, e^{15} + e^{27}$                   | 1/25(13, 7, 14, 19, 20, 27, 26, 34, 33)            | {0, 123489, 12469, 135, 1568, 234569, 24589, 368}                                                         |                    |
| 952:494  | $0, 0, 0, 0, e^{12}, e^{13}, e^{34}, e^{35} + e^{26}, e^{37} + e^{15}$                   | 1/28(13, 14, 10, 20, 27, 23, 30, 37, 40)           | {0, 123489, 124679, 1357, 1568, 234569, 245789, 3678}                                                     |                    |
| 952:495  | $0, 0, 0, 0, e^{12}, e^{13}, e^{34}, e^{35} + e^{26}, e^{25} + e^{37}$                   | 1/109(67, 41, 34, 81, 108, 101, 115, 142, 149)     | {0, 123489, 124679, 13459, 1456789, 23567, 258, 3678}                                                     |                    |
| 952:497  | $0, 0, 0, 0, e^{12}, e^{13}, e^{14}, e^{36} + e^{15}, e^{45} + e^{27}$                   | 1/233(92, 128, 110, 129, 220, 202, 221, 312, 349)  | {0, 123489, 12378, 124689, 12678, 34679, 36, 479}                                                         |                    |
| 952:498a | $0, 0, 0, 0, e^{12}, e^{13}, e^{14}, e^{26} + e^{35}, e^{25} + e^{47}$                   | 1/65(26, 32, 37, 32, 58, 63, 58, 95, 90)           | {0, 123489, 123789, 12469, 12679, 13459, 13579, 145689, 156789, 234567, 2356, 24578, 258, 34678, 368, 47} |                    |
| 952:498b | $0, 0, 0, 0, -e^{12}, -e^{13}, e^{14}, e^{35} + e^{26}, e^{47} + e^{25}$                 | 1/65(26, 32, 37, 32, 58, 63, 58, 95, 90)           | {0, 123489, 123789, 12469, 12679, 13459, 13579, 145689, 156789, 234567, 2356, 24578, 258, 34678, 368, 47} |                    |
| 952:499  | $0, 0, 0, 0, e^{12}, e^{13}, e^{14}, e^{26} + e^{35}, e^{27} + e^{45}$                   | 1/5(2, 2, 3, 3, 4, 5, 5, 7, 7)                     | {0, 123489, 12378, 12469, 1267, 1345, 13579, 14568, 156789, 234567, 23569, 24578, 2589, 346789, 368, 479} |                    |
| 952:500  | $0, 0, 0, 0, -e^{12}, e^{13}, e^{24}, e^{15} + e^{36}, e^{17} + e^{45}$                  | 1/233(92, 128, 110, 117, 220, 202, 245, 312, 337)  | {0, 123489, 12378, 124689, 12678, 34679, 36, 479}                                                         |                    |
| 952:503a | $0, 0, 0, 0, e^{12}, e^{13}, e^{24}, e^{26} + e^{35}, e^{47} + e^{15}$                   | 1/65(32, 26, 35, 32, 58, 67, 58, 93, 90)           | {0, 123489, 123789, 12469, 12679, 13457, 135, 145678, 1568, 234569, 235679, 24589, 25789, 34678, 368, 47} |                    |

Table A.4 – Continued to next page



Table A.4 – Continued from previous page

| Name     | g                                                                                           | N                                                    | S <sub>0</sub>                                                                                                | S = S <sub>0</sub> |
|----------|---------------------------------------------------------------------------------------------|------------------------------------------------------|---------------------------------------------------------------------------------------------------------------|--------------------|
| 952:503b | $0, 0, 0, 0, -e^{12}, -e^{13}, e^{24}, e^{35} + e^{26}, e^{47} + e^{15}$                    | $1/65(32, 26, 35, 32, 58, 67, 58, 93, 90)$           | $\{0, 123489, 123789, 12469, 12679, 13457, 135, 145678, 1568, 234569, 235679, 24589, 25789, 34678, 368, 47\}$ |                    |
| 952:504  | $0, 0, 0, 0, -e^{12}, -e^{13}, e^{24}, e^{35} + e^{26}, e^{17} + e^{45}$                    | $1/5(2, 2, 3, 3, 4, 5, 5, 7, 7)$                     | $\{0, 123489, 12378, 12469, 1267, 13457, 1359, 145678, 15689, 23456, 235679, 2458, 25789, 346789, 368, 479\}$ |                    |
| 952:508  | $0, 0, 0, 0, e^{12}, e^{13}, e^{34}, e^{35} + e^{26}, e^{47} + e^{15}$                      | $1/124(57, 62, 56, 60, 119, 113, 116, 175, 176)$     | $\{0, 123489, 123789, 145678, 1568, 234569, 235679, 47\}$                                                     |                    |
| 952:509  | $0, 0, 0, 0, e^{12}, e^{13}, e^{34}, e^{26} + e^{35}, e^{47} + e^{25}$                      | $1/257(142, 109, 108, 126, 251, 250, 234, 359, 360)$ | $\{0, 123489, 123789, 13459, 13579, 24578, 258, 47\}$                                                         |                    |
| 952:511a | $0, 0, 0, 0, e^{12}, e^{23} + e^{14}, e^{24} + e^{13}, e^{15}, e^{47} + e^{36}$             | $1/32(14, 14, 17, 17, 28, 31, 31, 42, 48)$           | $\{0, 123489, 126789, 1356, 1457, 235789, 245689, 3467\}$                                                     | ✓                  |
| 952:511b | $0, 0, 0, 0, e^{12}, e^{14} - e^{23}, e^{24} + e^{13}, e^{15}, e^{36} + e^{47}$             | $1/32(14, 14, 17, 17, 28, 31, 31, 42, 48)$           | $\{0, 123489, 126789, 1356, 1457, 235789, 245689, 3467\}$                                                     | ✓                  |
| 952:512a | $0, 0, 0, 0, e^{12}, e^{13} + e^{24}, e^{14} + e^{23}, e^{15}, e^{36} + e^{47}$             | $1/32(14, 14, 17, 17, 28, 31, 31, 42, 48)$           | $\{0, 123489, 126789, 13579, 14569, 23568, 24578, 3467\}$                                                     | ✓                  |
| 952:512b | $0, 0, 0, 0, e^{12}, e^{24} - e^{13}, e^{23} + e^{14}, e^{15}, e^{47} + e^{36}$             | $1/32(14, 14, 17, 17, 28, 31, 31, 42, 48)$           | $\{0, 123489, 126789, 13579, 14569, 23568, 24578, 3467\}$                                                     | ✓                  |
| 952:516  | $0, 0, 0, 0, e^{12}, e^{13}, e^{14} + e^{23}, e^{15} + e^{34}, e^{26} + e^{17}$             | $1/111(40, 61, 60, 81, 101, 100, 121, 141, 161)$     | $\{0, 23568, 245789, 34679\}$                                                                                 |                    |
| 952:517  | $0, 0, 0, 0, e^{12}, e^{13}, e^{23} + e^{14}, e^{25} + e^{34}, e^{17} + e^{26}$             | $1/73(27, 34, 44, 51, 61, 71, 78, 95, 105)$          | $\{0, 13578, 145689, 34679\}$                                                                                 |                    |
| 952:524  | $0, 0, 0, 0, e^{12}, e^{34}, e^{24} - e^{13}, e^{23} + e^{15}, e^{16} + e^{47}$             | $23/413(6, 11, 12, 7, 17, 19, 18, 23, 25)$           | $\{0, 12789, 14567, 245689\}$                                                                                 |                    |
| 952:525  | $0, 0, 0, 0, e^{12}a_1, (1 + a_1)e^{13}, e^{23} + e^{14}, e^{15}, e^{17} + e^{26} + e^{35}$ | $1/13(4, 7, 8, 11, 11, 12, 15, 15, 19)$              | $\{0, 123489, 12678, 1357, 14569, 23568, 245789, 34679\}$                                                     |                    |
| 952:526  | $0, 0, 0, 0, e^{12}a_1, (1 + a_1)e^{13}, e^{14} + e^{23}, e^{25}, e^{17} + e^{26} + e^{35}$ | $1/9(3, 4, 6, 7, 7, 9, 10, 11, 13)$                  | $\{0, 123489, 12678, 13578, 145689, 2356, 24579, 34679\}$                                                     |                    |
| 952:527a | $0, 0, 0, 0, e^{12}, e^{13}, e^{14} + e^{23}, e^{15}, e^{45} + e^{27} + e^{16}$             | $1/89(35, 35, 61, 61, 70, 96, 96, 105, 131)$         | $\{0, 123489, 12678, 13579, 1456, 235689, 24578, 34679\}$                                                     |                    |
| 952:527b | $0, 0, 0, 0, e^{12}, -e^{13}, e^{23} + e^{14}, e^{15}, e^{27} + e^{45} + e^{16}$            | $1/89(35, 35, 61, 61, 70, 96, 96, 105, 131)$         | $\{0, 123489, 12678, 13579, 1456, 235689, 24578, 34679\}$                                                     |                    |
| 952:528a | $0, 0, 0, 0, e^{12}, e^{13}, e^{23} + e^{14}, e^{25}, e^{45} + e^{27} + e^{16}$             | $1/89(35, 35, 61, 61, 70, 96, 96, 105, 131)$         | $\{0, 123489, 12678, 135789, 14568, 23569, 2457, 34679\}$                                                     |                    |
| 952:528b | $0, 0, 0, 0, e^{12}, -e^{13}, e^{14} + e^{23}, e^{25}, e^{27} + e^{16} + e^{45}$            | $1/89(35, 35, 61, 61, 70, 96, 96, 105, 131)$         | $\{0, 123489, 12678, 135789, 14568, 23569, 2457, 34679\}$                                                     |                    |
| 952:530  | $0, 0, 0, 0, e^{12}, e^{13}, e^{14} + e^{23}, e^{15}, e^{27} + e^{36} + e^{45}$             | $1/441(159, 209, 259, 309, 368, 418, 468, 527, 677)$ | $\{0, 123489, 13579, 24578\}$                                                                                 |                    |
| 952:533  | $0, 0, 0, 0, e^{12}, e^{34}, e^{14} + e^{23}, e^{15}, e^{16} + e^{25} + e^{37}$             | $1/9(3, 5, 4, 6, 8, 10, 9, 11, 13)$                  | $\{0, 123489, 12789, 347\}$                                                                                   |                    |
| 952:535  | $0, 0, 0, 0, e^{12}, e^{34}, e^{24} + e^{13}, e^{15}, e^{46} + e^{27} + e^{35}$             | $2/423(81, 109, 123, 95, 190, 218, 204, 271, 313)$   | $\{0, 123489, 1278, 3479\}$                                                                                   |                    |
| 952:536  | $0, 0, 0, 0, -e^{12}, e^{13}, e^{14} + e^{23}, e^{25} + e^{16}, e^{17} + e^{35}$            | $1/61(19, 29, 39, 49, 48, 58, 68, 77, 87)$           | $\{0, 123489, 13578, 24579\}$                                                                                 |                    |
| 952:538a | $0, 0, 0, 0, -e^{12}, e^{13}, e^{23} + e^{14}, e^{25} + e^{36}, e^{17} + e^{35}$            | $1/13(4, 7, 7, 10, 11, 11, 14, 18, 18)$              | $\{0, 123489, 12678, 13578, 145689, 2356, 24579, 34679\}$                                                     |                    |
| 952:538b | $0, 0, 0, 0, -e^{12}, -e^{13}, e^{14} + e^{23}, e^{36} + e^{25}, e^{17} + e^{35}$           | $1/13(4, 7, 7, 10, 11, 11, 14, 18, 18)$              | $\{0, 123489, 12678, 13578, 145689, 2356, 24579, 34679\}$                                                     |                    |
| 952:540  | $0, 0, 0, 0, e^{12}, e^{13}, e^{14} + e^{23}, e^{15} + e^{36}, e^{27} + e^{45}$             | $1/417(171, 215, 193, 237, 386, 364, 408, 557, 623)$ | $\{0, 123489, 12678, 34679\}$                                                                                 |                    |
| 952:541a | $0, 0, 0, 0, e^{12}, e^{13}, e^{23} + e^{14}, e^{36} + e^{25}, e^{45} + e^{27}$             | $1/121(49, 59, 59, 69, 108, 108, 118, 167, 177)$     | $\{0, 123489, 12678, 135789, 14568, 23569, 2457, 34679\}$                                                     |                    |
| 952:541b | $0, 0, 0, 0, e^{12}, -e^{13}, e^{14} + e^{23}, e^{36} + e^{25}, e^{27} + e^{45}$            | $1/121(49, 59, 59, 69, 108, 108, 118, 167, 177)$     | $\{0, 123489, 12678, 135789, 14568, 23569, 2457, 34679\}$                                                     |                    |
| 952:543  | $0, 0, 0, 0, -e^{12}, e^{34}, e^{14} + e^{23}, e^{15} + e^{36}, e^{35} + e^{17}$            | $1/3(1, 2, 1, 2, 3, 3, 3, 4, 4)$                     | $\{0, 123489, 13567, 2456789\}$                                                                               |                    |
| 952:544  | $0, 0, 0, 0, e^{12}, e^{34}, e^{24} + e^{13}, e^{15} + e^{36}, e^{27} + e^{35}$             | $1/127(68, 47, 54, 75, 115, 129, 122, 183, 169)$     | $\{0, 123489, 1356, 245689\}$                                                                                 |                    |
| 952:546  | $0, 0, 0, 0, e^{12}, e^{34}, e^{14} + e^{23}, e^{15} + e^{36}, e^{27} + e^{45}$             | $8/17(1, 1, 1, 1, 2, 2, 2, 3, 3)$                    | $\{0, 123489, 135679, 245678\}$                                                                               |                    |
| 952:547  | $0, 0, 0, 0, e^{23} + e^{14}, -e^{12}, e^{13}, e^{36} + e^{15}, e^{35} + e^{47}$            | $1/5(2, 3, 2, 3, 5, 4, 7, 7)$                        | $\{0, 123489, 12579, 1356, 14678, 23679, 245689, 34578\}$                                                     |                    |
| 952:548  | $0, 0, 0, 0, e^{23} + e^{14}, e^{12}, e^{13}, e^{46} + e^{25}, e^{35} + e^{47}$             | $1/30(15, 14, 14, 13, 28, 29, 29, 42, 42)$           | $\{0, 123489, 12579, 13568, 1467, 236789, 24569, 34578\}$                                                     |                    |
| 952:549  | $0, 0, 0, 0, e^{14} + e^{23}, -e^{12}, e^{34}, e^{36} + e^{15}, e^{35} + e^{17}$            | $1/3(1, 2, 1, 2, 3, 3, 3, 4, 4)$                     | $\{0, 123489, 1259, 13567, 14678, 23679, 2456789, 3458\}$                                                     |                    |
| 952:550  | $0, 0, 0, 0, e^{14} - e^{23}, e^{12}, e^{34}, e^{15} + e^{36}, e^{45} + e^{27}$             | $8/17(1, 1, 1, 1, 2, 2, 2, 3, 3)$                    | $\{0, 123489, 1259, 135679, 146789, 2367, 245678, 3458\}$                                                     |                    |
| 952:568  | $0, 0, 0, 0, e^{12}, e^{13}, e^{14}, e^{15} + e^{23}, e^{45} + e^{27} + e^{16}$             | $1/71(26, 35, 52, 43, 61, 78, 69, 87, 104)$          | $\{0, 12678, 1456, 24578\}$                                                                                   |                    |
| 952:571  | $0, 0, 0, 0, e^{12}, e^{13}, e^{14}, e^{23} + e^{15}, e^{35} + e^{47} + e^{26}$             | $5/123(8, 14, 16, 15, 22, 24, 23, 30, 38)$           | $\{0, 14569, 15679, 47\}$                                                                                     |                    |
| 952:572  | $0, 0, 0, 0, e^{12}, e^{13}, e^{14}, e^{23} + e^{15}, e^{37} + e^{46} + e^{25}$             | $1/187(57, 116, 114, 118, 173, 171, 175, 230, 289)$  | $\{0, 126789, 15679, 258\}$                                                                                   |                    |
| 952:573  | $0, 0, 0, 0, e^{12}, e^{13}, e^{14}, e^{15} + e^{23}, e^{36} + e^{27} + e^{45}$             | $1/389(121, 223, 242, 261, 344, 363, 382, 465, 605)$ | $\{0, 124689, 15679, 24578\}$                                                                                 |                    |
| 952:582  | $0, 0, 0, 0, e^{12}, e^{13}, e^{14}, e^{15} + e^{34}, e^{17} + e^{26} + e^{35}$             | $1/111(40, 61, 60, 81, 101, 100, 121, 141, 161)$     | $\{0, 23568, 245789, 34679\}$                                                                                 |                    |
| 952:583  | $0, 0, 0, 0, e^{12}, e^{13}, e^{14}, e^{34} + e^{25}, e^{17} + e^{35} + e^{26}$             | $1/73(27, 34, 44, 51, 61, 71, 78, 95, 105)$          | $\{0, 13578, 145689, 34679\}$                                                                                 |                    |
| 952:587  | $0, 0, 0, 0, e^{12}, e^{13}, e^{14}, e^{15} + e^{34}, e^{35} + e^{47} + e^{26}$             | $1/449(147, 261, 283, 272, 408, 430, 419, 555, 691)$ | $\{0, 123789, 15679, 23568\}$                                                                                 |                    |
| 952:588  | $0, 0, 0, 0, e^{12}, e^{13}, e^{14}, e^{34} + e^{15}, e^{46} + e^{25} + e^{37}$             | $25/81(1, 2, 2, 2, 3, 3, 3, 4, 5)$                   | $\{0, 13459, 15679, 3467\}$                                                                                   |                    |
| 952:608  | $0, 0, 0, 0, e^{12}, e^{13}, e^{14}, e^{26} + e^{35}, e^{34} + e^{17} + e^{25}$             | $1/187(57, 97, 114, 137, 154, 171, 194, 268, 251)$   | $\{0, 12469, 145689, 258\}$                                                                                   |                    |
| 952:627  | $0, 0, 0, 0, e^{12}, e^{13}, e^{34}, e^{14} + e^{35} + e^{26}, e^{25} + e^{37}$             | $1/389(233, 151, 128, 279, 384, 361, 407, 512, 535)$ | $\{0, 124679, 13459, 23567\}$                                                                                 |                    |
| 952:632  | $0, 0, 0, 0, e^{12}, e^{13}, e^{14}, e^{25} + e^{16}, e^{17} + e^{35} + e^{26}$             | $1/61(19, 29, 39, 49, 48, 58, 68, 77, 87)$           | $\{0, 123489, 13578, 24579\}$                                                                                 |                    |
| 952:634a | $0, 0, 0, 0, e^{12}, e^{13}, e^{14}, e^{36} + e^{25}, e^{26} + e^{35} + e^{17}$             | $1/13(4, 7, 7, 10, 11, 11, 14, 18, 18)$              | $\{0, 123489, 12678, 13578, 145689, 2356, 24579, 34679\}$                                                     | ✓                  |

Table A.4 – Continued to next page

Table A.4 – Continued from previous page

| Name     | g                                                                                                           | N                                                    | S <sub>0</sub>                                                                                                        | S = S <sub>0</sub> |
|----------|-------------------------------------------------------------------------------------------------------------|------------------------------------------------------|-----------------------------------------------------------------------------------------------------------------------|--------------------|
| 952:634b | $0, 0, 0, 0, e^{12}, e^{13}, e^{14}, -e^{25} + e^{36}, e^{17} + e^{26} + e^{35}$                            | $1/13(4, 7, 7, 10, 11, 11, 14, 18, 18)$              | $\{\emptyset, 123489, 12678, 13578, 145689, 2356, 24579, 34679\}$                                                     | ✓                  |
| 952:635a | $0, 0, 0, 0, e^{12}, e^{13}, e^{14}, e^{26} + e^{35}, e^{17} + e^{36} + e^{25}$                             | $1/13(4, 7, 7, 10, 11, 11, 14, 18, 18)$              | $\{\emptyset, 123489, 12469, 13459, 145689, 2356, 258, 368\}$                                                         | ✓                  |
| 952:635b | $0, 0, 0, 0, -e^{12}, e^{13}, e^{14}, -e^{26} + e^{35}, e^{17} + e^{25} + e^{36}$                           | $1/13(4, 7, 7, 10, 11, 11, 14, 18, 18)$              | $\{\emptyset, 123489, 12469, 13459, 145689, 2356, 258, 368\}$                                                         | ✓                  |
| 952:636  | $0, 0, 0, 0, e^{12}, e^{13}, e^{24}, e^{35} + e^{26}, e^{15} + e^{27} + e^{36}$                             | $1/217(117, 71, 94, 163, 188, 211, 234, 282, 305)$   | $\{\emptyset, 123489, 12469, 368\}$                                                                                   |                    |
| 952:639  | $0, 0, 0, 0, e^{12}, e^{13}, e^{14}, e^{25} + e^{16}, e^{47} + e^{26} + e^{35}$                             | $4/491(41, 61, 81, 71, 102, 122, 112, 163, 183)$     | $\{\emptyset, 123489, 123789, 47\}$                                                                                   |                    |
| 952:640  | $0, 0, 0, 0, e^{12}, e^{13}, e^{14}, e^{25} + e^{16}, e^{45} + e^{27} + e^{36}$                             | $1/28(10, 13, 16, 19, 23, 26, 29, 36, 42)$           | $\{\emptyset, 123489, 135789, 2457\}$                                                                                 |                    |
| 952:642  | $0, 0, 0, 0, -e^{12}, e^{13}, e^{24}, e^{16} + e^{25}, e^{17} + e^{36} + e^{45}$                            | $1/213(79, 98, 117, 136, 177, 196, 234, 275, 313)$   | $\{\emptyset, 123489, 13589, 245\}$                                                                                   |                    |
| 952:643a | $0, 0, 0, 0, e^{12}, e^{13}, e^{24}, e^{16} + e^{25}, e^{26} + e^{35} + e^{47}$                             | $2/37(7, 9, 11, 9, 16, 18, 18, 25, 27)$              | $\{\emptyset, 123489, 123789, 134578, 1358, 2459, 2579, 47\}$                                                         | ✓                  |
| 952:643b | $0, 0, 0, 0, -e^{12}, -e^{13}, e^{24}, e^{16} + e^{25}, e^{26} + e^{35} + e^{47}$                           | $2/37(7, 9, 11, 9, 16, 18, 18, 25, 27)$              | $\{\emptyset, 123489, 123789, 134578, 1358, 2459, 2579, 47\}$                                                         | ✓                  |
| 952:649a | $0, 0, 0, 0, e^{12}, e^{13}, e^{14}, e^{25} + e^{36}, e^{26} + e^{35} + e^{47}$                             | $2/35(7, 9, 9, 9, 16, 16, 16, 25, 25)$               | $\{\emptyset, 123489, 123789, 145689, 156789, 234567, 2356, 47\}$                                                     | ✓                  |
| 952:649b | $0, 0, 0, 0, e^{12}, e^{13}, e^{14}, e^{36} - e^{25}, e^{26} + e^{35} + e^{47}$                             | $2/35(7, 9, 9, 9, 16, 16, 16, 25, 25)$               | $\{\emptyset, 123489, 123789, 145689, 156789, 234567, 2356, 47\}$                                                     | ✓                  |
| 952:650a | $0, 0, 0, 0, e^{12}, e^{13}, e^{14}, e^{26} + e^{35}, e^{25} + e^{36} + e^{47}$                             | $2/35(7, 9, 9, 9, 16, 16, 16, 25, 25)$               | $\{\emptyset, 123489, 123789, 12469, 12679, 13459, 13579, 145689, 156789, 234567, 2356, 24578, 258, 34678, 368, 47\}$ | ✓                  |
| 952:650b | $0, 0, 0, 0, e^{12}, -e^{13}, e^{14}, e^{35} - e^{26}, e^{47} + e^{25} + e^{36}$                            | $2/35(7, 9, 9, 9, 16, 16, 16, 25, 25)$               | $\{\emptyset, 123489, 123789, 12469, 12679, 13459, 13579, 145689, 156789, 234567, 2356, 24578, 258, 34678, 368, 47\}$ | ✓                  |
| 952:650c | $0, 0, 0, 0, -e^{12}, -e^{13}, e^{14}, e^{35} + e^{26}, e^{47} + e^{36} + e^{25}$                           | $2/35(7, 9, 9, 9, 16, 16, 16, 25, 25)$               | $\{\emptyset, 123489, 123789, 12469, 12679, 13459, 13579, 145689, 156789, 234567, 2356, 24578, 258, 34678, 368, 47\}$ | ✓                  |
| 952:651  | $0, 0, 0, 0, e^{12}, e^{13}, e^{14}, e^{26} + e^{35}, e^{46} + e^{25} + e^{37}$                             | $1/55(22, 29, 24, 34, 51, 46, 56, 75, 80)$           | $\{\emptyset, 123489, 12679, 13459, 156789, 234567, 258, 34678\}$                                                     |                    |
| 952:652  | $0, 0, 0, 0, e^{12}, e^{13}, e^{24}, e^{15} + e^{36}, e^{26} + e^{47} + e^{35}$                             | $4/531(59, 67, 63, 61, 126, 122, 128, 185, 189)$     | $\{\emptyset, 123489, 123789, 47\}$                                                                                   |                    |
| 952:653a | $0, 0, 0, 0, e^{12}, e^{13}, e^{24}, e^{35} + e^{26}, e^{15} + e^{36} + e^{47}$                             | $1/67(34, 28, 31, 34, 62, 65, 62, 93, 96)$           | $\{\emptyset, 123489, 123789, 12469, 12679, 34678, 368, 47\}$                                                         |                    |
| 952:653b | $0, 0, 0, 0, -e^{12}, -e^{13}, e^{24}, e^{26} + e^{35}, e^{15} + e^{47} + e^{36}$                           | $1/67(34, 28, 31, 34, 62, 65, 62, 93, 96)$           | $\{\emptyset, 123489, 123789, 12469, 12679, 34678, 368, 47\}$                                                         |                    |
| 952:654  | $0, 0, 0, 0, -e^{12}, -e^{13}, e^{24}, e^{26} + e^{35}, e^{17} + e^{36} + e^{45}$                           | $1/31(13, 13, 16, 19, 26, 29, 32, 42, 45)$           | $\{\emptyset, 123489, 12469, 1359, 15689, 23456, 2458, 368\}$                                                         |                    |
| 952:655a | $0, 0, 0, 0, e^{12}, e^{13}, e^{24}, e^{36} + e^{25}, e^{35} + e^{47} + e^{26}$                             | $4/123(17, 13, 13, 15, 30, 30, 28, 43, 43)$          | $\{\emptyset, 123489, 123789, 134578, 1358, 2459, 2579, 47\}$                                                         | ✓                  |
| 952:655b | $0, 0, 0, 0, e^{12}, e^{13}, e^{24}, -e^{25} + e^{36}, e^{35} + e^{47} + e^{26}$                            | $4/123(17, 13, 13, 15, 30, 30, 28, 43, 43)$          | $\{\emptyset, 123489, 123789, 134578, 1358, 2459, 2579, 47\}$                                                         | ✓                  |
| 952:657  | $0, 0, 0, 0, e^{12}, e^{34}, -e^{13}, e^{36} + e^{15}, e^{47} + e^{25} + e^{16}$                            | $4/123(14, 15, 13, 17, 29, 30, 27, 43, 44)$          | $\{\emptyset, 123489, 1579, 234578\}$                                                                                 |                    |
| 952:660  | $0, 0, 0, 0, e^{12}, e^{34}, e^{13}, e^{36} + e^{25}, e^{27} + e^{46} + e^{35}$                             | $2/37(11, 7, 8, 9, 18, 17, 19, 25, 26)$              | $\{\emptyset, 123489, 124678, 3679\}$                                                                                 |                    |
| 952:665a | $0, 0, 0, 0, (-1 + a_2)e^{12}, e^{23} + e^{14}, a_2e^{13} + e^{24}, e^{15}, e^{27} + e^{16} + e^{35}$       | $1/89(35, 35, 61, 61, 70, 96, 96, 105, 131)$         | $\{\emptyset, 123489, 12678, 1356, 14579, 23578, 245689, 34679\}$                                                     |                    |
| 952:665b | $0, 0, 0, 0, (-1 + a_2)e^{12}, -e^{14} + e^{23}, a_2e^{13} + e^{24}, e^{15}, e^{16} + e^{27} + e^{35}$      | $1/89(35, 35, 61, 61, 70, 96, 96, 105, 131)$         | $\{\emptyset, 123489, 12678, 1356, 14579, 23578, 245689, 34679\}$                                                     |                    |
| 952:670a | $0, 0, 0, 0, -e^{23} + e^{14}, e^{12}, e^{24} + e^{13}, e^{36} + e^{15}, e^{35} + e^{47}$                   | $1/81(39, 39, 37, 37, 76, 78, 76, 115, 113)$         | $\{\emptyset, 123489, 12579, 1356, 14678, 23679, 245689, 34578\}$                                                     |                    |
| 952:670b | $0, 0, 0, 0, e^{23} + e^{14}, -e^{12}, e^{24} + e^{13}, e^{36} + e^{15}, e^{35} + e^{47}$                   | $1/81(39, 39, 37, 37, 76, 78, 76, 115, 113)$         | $\{\emptyset, 123489, 12579, 1356, 14678, 23679, 245689, 34578\}$                                                     |                    |
| 952:674  | $0, 0, 0, 0, (-1 + a_2)e^{12}, a_2e^{13}, e^{14} + e^{23}, e^{15} + e^{24}, e^{17} + e^{26} + e^{35}$       | $1/71(26, 35, 43, 52, 61, 69, 78, 87, 104)$          | $\{\emptyset, 12678, 1357, 23568\}$                                                                                   |                    |
| 952:675  | $0, 0, 0, 0, (-1 + a_2)e^{12}, a_2e^{13}, e^{14} + e^{23}, e^{34} + e^{15}, e^{35} + e^{17} + e^{26}$       | $1/111(40, 61, 60, 81, 101, 100, 121, 141, 161)$     | $\{\emptyset, 23568, 245789, 34679\}$                                                                                 |                    |
| 952:676  | $0, 0, 0, 0, (-1 + a_2)e^{12}, a_2e^{13}, e^{14} + e^{23}, e^{34} + e^{25}, e^{17} + e^{35} + e^{26}$       | $1/73(27, 34, 44, 51, 61, 71, 78, 95, 105)$          | $\{\emptyset, 13578, 145689, 34679\}$                                                                                 |                    |
| 952:680a | $0, 0, 0, 0, e^{12}, e^{13}, e^{23} + e^{14}, e^{15} + e^{34}, e^{27} + e^{16} + e^{45}$                    | $37/177(2, 2, 3, 3, 4, 5, 5, 6, 7)$                  | $\{\emptyset, 235689, 24578, 34679\}$                                                                                 |                    |
| 952:680b | $0, 0, 0, 0, e^{12}, -e^{13}, e^{14} + e^{23}, e^{15} + e^{34}, e^{45} + e^{16} + e^{27}$                   | $37/177(2, 2, 3, 3, 4, 5, 5, 6, 7)$                  | $\{\emptyset, 235689, 24578, 34679\}$                                                                                 |                    |
| 952:681a | $0, 0, 0, 0, e^{12}, e^{13}, e^{14} + e^{23}, e^{25} + e^{34}, e^{27} + e^{16} + e^{45}$                    | $37/177(2, 2, 3, 3, 4, 5, 5, 6, 7)$                  | $\{\emptyset, 135789, 14568, 34679\}$                                                                                 |                    |
| 952:681b | $0, 0, 0, 0, e^{12}, -e^{13}, e^{14} + e^{23}, e^{34} + e^{25}, e^{16} + e^{27} + e^{45}$                   | $37/177(2, 2, 3, 3, 4, 5, 5, 6, 7)$                  | $\{\emptyset, 135789, 14568, 34679\}$                                                                                 |                    |
| 952:683  | $0, 0, 0, 0, e^{12}, e^{13}, e^{14} + e^{23}, e^{34} + e^{15}, e^{45} + e^{36} + e^{27}$                    | $81/853(4, 5, 6, 7, 9, 10, 11, 13, 16)$              | $\{\emptyset, 24578\}$                                                                                                |                    |
| 952:692  | $0, 0, 0, 0, -e^{12}, e^{13}, e^{23} + e^{14}, e^{24} + e^{15} + e^{36}, e^{17} + e^{35}$                   | $13/109(3, 5, 4, 6, 8, 7, 9, 11, 12)$                | $\{\emptyset, 12678\}$                                                                                                |                    |
| 952:705  | $0, 0, 0, 0, (-1 + a_2)e^{12}, a_2e^{13}, e^{14} + e^{23}, e^{25} + e^{16}, e^{26} + e^{35} + e^{17}$       | $1/61(19, 29, 39, 49, 48, 58, 68, 77, 87)$           | $\{\emptyset, 123489, 13578, 24579\}$                                                                                 |                    |
| 952:706a | $0, 0, 0, 0, (-1 + a_2)e^{12}, a_2e^{13}, e^{14} + e^{23}, e^{36} + e^{25}, e^{35} + e^{26} + e^{17}$       | $1/13(4, 7, 7, 10, 11, 11, 14, 18, 18)$              | $\{\emptyset, 123489, 12678, 13578, 145689, 2356, 24579, 34679\}$                                                     |                    |
| 952:706b | $0, 0, 0, 0, (-1 + a_2)e^{12}, a_2e^{13}, e^{14} + e^{23}, e^{36} - e^{25}, e^{26} + e^{35} + e^{17}$       | $1/13(4, 7, 7, 10, 11, 11, 14, 18, 18)$              | $\{\emptyset, 123489, 12678, 13578, 145689, 2356, 24579, 34679\}$                                                     |                    |
| 952:708  | $0, 0, 0, 0, e^{12}, e^{13}, e^{14} + e^{23}, e^{25} + e^{16}, e^{27} + e^{45} + e^{36}$                    | $1/28(10, 13, 16, 19, 23, 26, 29, 36, 42)$           | $\{\emptyset, 123489, 135789, 2457\}$                                                                                 |                    |
| 952:713  | $0, 0, 0, 0, e^{12}, e^{34}, e^{24} - e^{13}, e^{36} + e^{15}, e^{47} + e^{25} + e^{16}$                    | $8/17(1, 1, 1, 1, 2, 2, 2, 3, 3)$                    | $\{\emptyset, 123489\}$                                                                                               |                    |
| 952:716  | $0, 0, 0, 0, -e^{12}, e^{23} + e^{14}, e^{13}, e^{16} + e^{35}, e^{25} + e^{47} + e^{36}$                   | $1/281(107, 151, 129, 173, 258, 280, 236, 387, 409)$ | $\{\emptyset, 123489, 12679, 34678\}$                                                                                 |                    |
| 952:717  | $0, 0, 0, 0, -e^{12}, -e^{14} + e^{23}, e^{13}, e^{16} + e^{35}, e^{37} + e^{26} + e^{45}$                  | $1/281(107, 129, 151, 173, 236, 280, 258, 387, 409)$ | $\{\emptyset, 123489, 13569, 24568\}$                                                                                 |                    |
| 952:718  | $0, 0, 0, 0, e^{12}, a_1, e^{14}, a_1 + e^{23}, (1 + a_1)e^{13}, e^{45} + e^{26}, e^{35} + e^{27} + e^{16}$ | $1/5(2, 2, 3, 3, 4, 5, 5, 7, 7)$                     | $\{\emptyset, 123489, 1267, 13568, 14579, 23578, 24569, 346789\}$                                                     |                    |

Table A.4 – Continued to next page

Table A.4 – Continued from previous page

| Name     | g                                                                                                                                      | N                                                    | S <sub>0</sub>                                                    | S = S <sub>0</sub> |
|----------|----------------------------------------------------------------------------------------------------------------------------------------|------------------------------------------------------|-------------------------------------------------------------------|--------------------|
| 952:719a | $0, 0, 0, 0, e^{12}, e^{23} + e^{14}, e^{13}, e^{26} + e^{45}, e^{47} + e^{36} + e^{15}$                                               | $1/81(39, 37, 39, 37, 76, 76, 78, 113, 115)$         | $\{\emptyset, 123489, 12679, 13568, 1457, 235789, 24569, 34678\}$ |                    |
| 952:719b | $0, 0, 0, 0, -e^{12}, e^{23} - e^{14}, -e^{13}, e^{45} + e^{26}, e^{47} + e^{36} + e^{15}$                                             | $1/81(39, 37, 39, 37, 76, 76, 78, 113, 115)$         | $\{\emptyset, 123489, 12679, 13568, 1457, 235789, 24569, 34678\}$ |                    |
| 952:720  | $0, 0, 0, 0, e^{12}, e^{14} + e^{23}, e^{13}, e^{45} + e^{26}, e^{47} + e^{36} + e^{25}$                                               | $1/107(53, 49, 51, 47, 102, 100, 104, 149, 151)$     | $\{\emptyset, 123489, 12679, 34678\}$                             |                    |
| 952:721  | $0, 0, 0, 0, -e^{12}, e^{14} + e^{23}, e^{34}, e^{16} + e^{35}, e^{25} + e^{17} + e^{36}$                                              | $2/41(7, 11, 9, 13, 18, 20, 22, 27, 29)$             | $\{\emptyset, 123489, 1269, 3468\}$                               |                    |
| 952:723  | $0, 0, 0, 0, -e^{12}, e^{23} - e^{14}, e^{34}, e^{16} + e^{35}, e^{26} + e^{37} + e^{45}$                                              | $1/157(64, 78, 71, 85, 142, 149, 156, 213, 227)$     | $\{\emptyset, 123489, 126, 34689\}$                               |                    |
| 952:735  | $0, 0, 0, 0, e^{12}, e^{13}, e^{14}, e^{15} + e^{36} + e^{24}, e^{17} + e^{26} + e^{35}$                                               | $13/109(3, 5, 4, 6, 8, 7, 9, 11, 12)$                | $\{\emptyset, 12678\}$                                            |                    |
| 952:756  | $0, 0, 0, 0, e^{12}, e^{13}, a_1, e^{24}, e^{15} + e^{27} + e^{36}, e^{25} + e^{47} + e^{16}$                                          | $8/17(1, 1, 1, 1, 2, 2, 2, 3, 3)$                    | $\{\emptyset, 123489\}$                                           |                    |
| 952:759  | $0, 0, 0, 0, e^{12}, e^{13}, e^{14}, e^{35} + e^{17} + e^{26}, e^{37} + e^{46} + e^{25}$                                               | $1/281(107, 151, 129, 173, 258, 236, 280, 387, 409)$ | $\{\emptyset, 123489, 12679, 34678\}$                             |                    |
| 952:760  | $0, 0, 0, 0, e^{12}, e^{13}, e^{24}, e^{36} + e^{27} + e^{15}, e^{26} + e^{35} + e^{47}$                                               | $8/17(1, 1, 1, 1, 2, 2, 2, 3, 3)$                    | $\{\emptyset, 123489\}$                                           |                    |
| 952:761  | $0, 0, 0, 0, e^{12}, e^{13}, e^{14}, e^{37} + e^{46} + e^{25}, e^{47} + e^{35} + e^{26}$                                               | $2/35(7, 9, 9, 9, 16, 16, 16, 25, 25)$               | $\{\emptyset, 123489, 156789, 234567\}$                           |                    |
| 952:762  | $0, 0, 0, 0, -e^{12}, -e^{13}, e^{24}, e^{36} + e^{45} + e^{17}, e^{26} + e^{47} + e^{35}$                                             | $8/17(1, 1, 1, 1, 2, 2, 2, 3, 3)$                    | $\{\emptyset, 123489, 1358, 2459\}$                               |                    |
| 952:765a | $0, 0, 0, 0, (-1 + a_2)e^{12}, e^{23} + e^{14}, a_2e^{13} + e^{24}, e^{34} + e^{15}, e^{16} + e^{27} + e^{35}$                         | $37/177(2, 2, 3, 3, 4, 5, 5, 6, 7)$                  | $\{\emptyset, 23578, 245689, 34679\}$                             |                    |
| 952:765b | $0, 0, 0, 0, (-1 + a_2)e^{12}, e^{23} - e^{14}, a_2e^{13} + e^{24}, e^{15} + e^{34}, e^{27} + e^{16} + e^{35}$                         | $37/177(2, 2, 3, 3, 4, 5, 5, 6, 7)$                  | $\{\emptyset, 23578, 245689, 34679\}$                             |                    |
| 952:770a | $0, 0, 0, 0, e^{12}, e^{14} - e^{23}, e^{13} + e^{24}, e^{35} + e^{16}, e^{36} + e^{47} + e^{15}$                                      | $8/17(1, 1, 1, 1, 2, 2, 2, 3, 3)$                    | $\{\emptyset, 123489, 12679, 1356, 14578, 23579, 245689, 34678\}$ |                    |
| 952:770b | $0, 0, 0, 0, e^{12}, e^{23} + e^{14}, e^{24} + e^{13}, e^{35} - e^{16}, e^{47} + e^{36} + e^{15}$                                      | $8/17(1, 1, 1, 1, 2, 2, 2, 3, 3)$                    | $\{\emptyset, 123489, 12679, 1356, 14578, 23579, 245689, 34678\}$ |                    |
| 952:770c | $0, 0, 0, 0, -e^{12}, e^{23} + e^{14}, e^{24} + e^{13}, e^{35} + e^{16}, e^{47} + e^{36} + e^{15}$                                     | $8/17(1, 1, 1, 1, 2, 2, 2, 3, 3)$                    | $\{\emptyset, 123489, 12679, 1356, 14578, 23579, 245689, 34678\}$ |                    |
| 952:770d | $0, 0, 0, 0, -e^{12}, e^{14} - e^{23}, e^{24} + e^{13}, e^{35} - e^{16}, e^{47} + e^{36} + e^{15}$                                     | $8/17(1, 1, 1, 1, 2, 2, 2, 3, 3)$                    | $\{\emptyset, 123489, 12679, 1356, 14578, 23579, 245689, 34678\}$ |                    |
| 952:772a | $0, 0, 0, 0, e^{12}, -e^{23} + e^{14}, e^{24} + e^{13}, e^{16} + e^{35}, e^{25} + e^{47} + e^{36}$                                     | $8/17(1, 1, 1, 1, 2, 2, 2, 3, 3)$                    | $\{\emptyset, 123489, 12679, 34678\}$                             |                    |
| 952:772b | $0, 0, 0, 0, -e^{12}, e^{14} + e^{23}, e^{24} + e^{13}, e^{16} + e^{35}, e^{47} + e^{36} + e^{25}$                                     | $8/17(1, 1, 1, 1, 2, 2, 2, 3, 3)$                    | $\{\emptyset, 123489, 12679, 34678\}$                             |                    |
| 952:774a | $0, 0, 0, 0, e^{13}, a_1 + e^{24}, e^{14} + e^{23}, (-1 + a_1)e^{12}, e^{26} + e^{15}, e^{37} + e^{25} + e^{16}$                       | $1/5(2, 2, 3, 3, 5, 5, 4, 7, 7)$                     | $\{\emptyset, 123489, 1256, 13678, 14579, 23578, 24679, 345689\}$ |                    |
| 952:774b | $0, 0, 0, 0, e^{13}, a_1 + e^{24}, -e^{14} + e^{23}, (-1 + a_1)e^{12}, e^{26} - e^{15}, e^{37} + e^{16} + e^{25}$                      | $1/5(2, 2, 3, 3, 5, 5, 4, 7, 7)$                     | $\{\emptyset, 123489, 1256, 13678, 14579, 23578, 24679, 345689\}$ |                    |
| 952:777a | $0, 0, 0, 0, e^{14} + a_3e^{23}, e^{13} + e^{24}, -(-1 + a_3)e^{12}, e^{46} + e^{35}, e^{37} + e^{26} + e^{15}$                        | $1/81(39, 39, 37, 37, 76, 76, 78, 113, 115)$         | $\{\emptyset, 123489, 12568, 1357, 14679, 23678, 245789, 34569\}$ |                    |
| 952:777b | $0, 0, 0, 0, -e^{14} + a_3e^{23}, e^{24} - e^{13}, -e^{12}(1 + a_3), e^{46} + e^{35}, e^{26} + e^{37} + e^{15}$                        | $1/81(39, 39, 37, 37, 76, 76, 78, 113, 115)$         | $\{\emptyset, 123489, 12568, 1357, 14679, 23678, 245789, 34569\}$ |                    |
| 952:778a | $0, 0, 0, 0, e^{23} + e^{14}, e^{24} + e^{13}, e^{12}, e^{35} + e^{46}, e^{17} + e^{36} + e^{45}$                                      | $8/17(1, 1, 1, 1, 2, 2, 2, 3, 3)$                    | $\{\emptyset, 123489, 125689, 3456\}$                             |                    |
| 952:778b | $0, 0, 0, 0, -e^{14} + e^{23}, e^{24} + e^{13}, e^{12}, -e^{35} + e^{46}, e^{17} + e^{36} + e^{45}$                                    | $8/17(1, 1, 1, 1, 2, 2, 2, 3, 3)$                    | $\{\emptyset, 123489, 125689, 3456\}$                             |                    |
| 952:779a | $0, 0, 0, 0, e^{13} + e^{24}, e^{14} + e^{23}, e^{12}, e^{46} + e^{35}, e^{17} + e^{45} + e^{36}$                                      | $8/17(1, 1, 1, 1, 2, 2, 2, 3, 3)$                    | $\{\emptyset, 123489, 125689, 13678, 14578, 23579, 24679, 3456\}$ |                    |
| 952:779b | $0, 0, 0, 0, e^{13} - e^{24}, e^{14} + e^{23}, e^{12}, e^{46} - e^{35}, e^{17} + e^{36} + e^{45}$                                      | $8/17(1, 1, 1, 1, 2, 2, 2, 3, 3)$                    | $\{\emptyset, 123489, 125689, 13678, 14578, 23579, 24679, 3456\}$ |                    |
| 952:779c | $0, 0, 0, 0, e^{24} + e^{13}, e^{23} + e^{14}, -e^{12}, e^{35} + e^{46}, e^{36} + e^{45} + e^{17}$                                     | $8/17(1, 1, 1, 1, 2, 2, 2, 3, 3)$                    | $\{\emptyset, 123489, 125689, 13678, 14578, 23579, 24679, 3456\}$ |                    |
| 952:783  | $0, 0, 0, 0, (-1 + a_2)e^{12}, a_2e^{13}, e^{14} + e^{23}, e^{15} + e^{24} + e^{36}, e^{17} + e^{26} + e^{35}$                         | $13/109(3, 5, 4, 6, 8, 7, 9, 11, 12)$                | $\{\emptyset, 12678\}$                                            |                    |
| 952:795  | $0, 0, 0, 0, (-1 + a_3)e^{12}, a_3e^{13}, e^{23} + a_3e^{14}, e^{17} + e^{26} + e^{35}, e^{46} + e^{25} + e^{37}$                      | $1/281(107, 151, 129, 173, 258, 236, 280, 387, 409)$ | $\{\emptyset, 123489, 12679, 34678\}$                             |                    |
| 952:796a | $0, 0, 0, 0, e^{12}, e^{13}, e^{14} + e^{23}, e^{27} + e^{16} + e^{45}, e^{15} + e^{46} + e^{37}$                                      | $8/17(1, 1, 1, 1, 2, 2, 2, 3, 3)$                    | $\{\emptyset, 123489, 12679, 13578, 1456, 235689, 24579, 34678\}$ |                    |
| 952:796b | $0, 0, 0, 0, e^{12}, e^{13}, e^{14} + e^{23}, -e^{16} + e^{27} + e^{45}, e^{15} + e^{46} + e^{37}$                                     | $8/17(1, 1, 1, 1, 2, 2, 2, 3, 3)$                    | $\{\emptyset, 123489, 12679, 13578, 1456, 235689, 24579, 34678\}$ |                    |
| 952:796c | $0, 0, 0, 0, -e^{12}, -e^{13}, e^{23} - e^{14}, e^{45} + e^{27} - e^{16}, e^{37} + e^{46} + e^{15}$                                    | $8/17(1, 1, 1, 1, 2, 2, 2, 3, 3)$                    | $\{\emptyset, 123489, 12679, 13578, 1456, 235689, 24579, 34678\}$ |                    |
| 952:797a | $0, 0, 0, 0, e^{12}, e^{13}, e^{14} + e^{23}, e^{45} + e^{27} + e^{16}, e^{46} + e^{25} + e^{37}$                                      | $8/17(1, 1, 1, 1, 2, 2, 2, 3, 3)$                    | $\{\emptyset, 123489, 12679, 34678\}$                             |                    |
| 952:797b | $0, 0, 0, 0, -e^{12}, -e^{13}, -e^{14} + e^{23}, e^{16} + e^{45} + e^{27}, e^{25} + e^{37} + e^{46}$                                   | $8/17(1, 1, 1, 1, 2, 2, 2, 3, 3)$                    | $\{\emptyset, 123489, 12679, 34678\}$                             |                    |
| 952:798  | $0, 0, 0, 0, e^{12}, e^{13}, e^{23} + e^{14}, e^{27} + e^{36} + e^{45}, e^{37} + e^{46} + e^{25}$                                      | $8/17(1, 1, 1, 1, 2, 2, 2, 3, 3)$                    | $\{\emptyset, 123489\}$                                           |                    |
| 952:799a | $0, 0, 0, 0, e^{12}, e^{34}, e^{24} - e^{13}, e^{15} + e^{26} + e^{37}, e^{16} + e^{25} + e^{47}$                                      | $8/17(1, 1, 1, 1, 2, 2, 2, 3, 3)$                    | $\{\emptyset, 123489, 12789, 347\}$                               |                    |
| 952:799b | $0, 0, 0, 0, e^{12}, e^{34}, e^{24} - e^{13}, -e^{15} + e^{37} + e^{26}, e^{47} + e^{16} + e^{25}$                                     | $8/17(1, 1, 1, 1, 2, 2, 2, 3, 3)$                    | $\{\emptyset, 123489, 12789, 347\}$                               |                    |
| 952:800  | $0, 0, 0, 0, -e^{12}, e^{34}, a_2e^{13} + e^{24}, e^{26} + e^{15} + e^{37}, e^{17} + e^{45} + e^{36}$                                  | $8/17(1, 1, 1, 1, 2, 2, 2, 3, 3)$                    | $\{\emptyset, 123489, 1278, 3479\}$                               |                    |
| 952:801a | $0, 0, 0, 0, e^{12}, e^{34}, -e^{23} + e^{14}, e^{25} + e^{37} + e^{16}, e^{46} + e^{35} + e^{17}$                                     | $8/17(1, 1, 1, 1, 2, 2, 2, 3, 3)$                    | $\{\emptyset, 123489, 1278, 3479\}$                               |                    |
| 952:801b | $0, 0, 0, 0, -e^{12}, e^{34}, e^{23} + e^{14}, e^{37} + e^{16} + e^{25}, e^{35} + e^{46} + e^{17}$                                     | $8/17(1, 1, 1, 1, 2, 2, 2, 3, 3)$                    | $\{\emptyset, 123489, 1278, 3479\}$                               |                    |
| 952:802a | $0, 0, 0, 0, (1 + a_2)e^{13} + e^{24}, e^{14} + e^{23}, a_2e^{12} + e^{34}, e^{26} + e^{15}, e^{37} + e^{25} + e^{16}$                 | $8/17(1, 1, 1, 1, 2, 2, 2, 3, 3)$                    | $\{\emptyset, 123489, 1256, 13678, 14579, 23578, 24679, 345689\}$ |                    |
| 952:802b | $0, 0, 0, 0, (1 + a_2)e^{13} - e^{24}, e^{14} + e^{23}, a_2e^{12} + e^{34}, e^{26} - e^{15}, e^{37} + e^{25} + e^{16}$                 | $8/17(1, 1, 1, 1, 2, 2, 2, 3, 3)$                    | $\{\emptyset, 123489, 1256, 13678, 14579, 23578, 24679, 345689\}$ |                    |
| 952:802c | $0, 0, 0, 0, (1 + a_2)e^{13} - e^{24}, -e^{14} + e^{23}, a_2e^{12} + e^{34}, e^{26} + e^{15}, e^{37} + e^{16} + e^{25}$                | $8/17(1, 1, 1, 1, 2, 2, 2, 3, 3)$                    | $\{\emptyset, 123489, 1256, 13678, 14579, 23578, 24679, 345689\}$ |                    |
| 952:807a | $0, 0, 0, 0, e^{12}, a_1, (a_3 - a_1)e^{23} + (1 + a_1)e^{14}, e^{24} + a_3e^{13}, e^{35} + e^{27} + e^{16}, e^{45} + e^{17} + e^{26}$ | $1/5(2, 2, 3, 3, 4, 5, 5, 7, 7)$                     | $\{\emptyset, 123489, 1267, 13569, 14578, 23579, 24568, 346789\}$ |                    |

Table A.4 – Continued to next page

Table A.4 – Continued from previous page

| Name     | g                                                                                                                                                         | N                                               | S <sub>0</sub>                                                                                            | S = S <sub>0</sub> |
|----------|-----------------------------------------------------------------------------------------------------------------------------------------------------------|-------------------------------------------------|-----------------------------------------------------------------------------------------------------------|--------------------|
| 952:807b | $0, 0, 0, 0, e^{12}a_1,$<br>$-(a_3 - a_1)e^{23} + (1 + a_1)e^{14}, e^{24} + a_3e^{13}, e^{27} + e^{35} - e^{16}, e^{26} + e^{17} + e^{45}$                | 1/5(2, 2, 3, 3, 4, 5, 5, 7, 7)                  | {0, 123489, 1267, 13569, 14578, 23579, 24568, 346789}                                                     |                    |
| 952:808a | $0, 0, 0, 0, e^{12},$<br>$(-1 + a_2)e^{23} + a_2e^{14}, a_2e^{13} + e^{24}, e^{27} + e^{35} + e^{16}, e^{47} + e^{36} + e^{15}$                           | 8/17(1, 1, 1, 1, 2, 2, 2, 3, 3)                 | {0, 123489, 12679, 1356, 14578, 23579, 245689, 34678}                                                     |                    |
| 952:808b | $0, 0, 0, 0, e^{12},$<br>$-(-1 + a_2)e^{23} + a_2e^{14}, a_2e^{13} + e^{24}, e^{27} + e^{35} - e^{16}, e^{15} + e^{36} + e^{47}$                          | 8/17(1, 1, 1, 1, 2, 2, 2, 3, 3)                 | {0, 123489, 12679, 1356, 14578, 23579, 245689, 34678}                                                     |                    |
| 952:808c | $0, 0, 0, 0, -e^{12},$<br>$(1 + a_2)e^{23} + a_2e^{14}, a_2e^{13} + e^{24}, e^{27} + e^{16} + e^{35}, e^{15} + e^{47} + e^{36}$                           | 8/17(1, 1, 1, 1, 2, 2, 2, 3, 3)                 | {0, 123489, 12679, 1356, 14578, 23579, 245689, 34678}                                                     |                    |
| 952:808d | $0, 0, 0, 0, -e^{12},$<br>$(-1 + a_2)e^{23} - a_2e^{14}, -a_2e^{13} + e^{24}, -e^{16} + e^{27} + e^{35}, e^{47} + e^{15} + e^{36}$                        | 8/17(1, 1, 1, 1, 2, 2, 2, 3, 3)                 | {0, 123489, 12679, 1356, 14578, 23579, 245689, 34678}                                                     |                    |
| 952:809a | $0, 0, 0, 0, (-1 + a_2)e^{12}, e^{14} + e^{23}, a_2e^{13} + e^{24}, e^{27} + e^{16} + e^{35}, e^{15} + e^{46} + e^{37}$                                   | 8/17(1, 1, 1, 1, 2, 2, 2, 3, 3)                 | {0, 123489, 12679, 34678}                                                                                 |                    |
| 952:809b | $0, 0, 0, 0, (-1 + a_2)e^{12},$<br>$-e^{14} + e^{23}, a_2e^{13} + e^{24}, e^{16} + e^{35} + e^{27}, e^{15} + e^{46} + e^{37}$                             | 8/17(1, 1, 1, 1, 2, 2, 2, 3, 3)                 | {0, 123489, 12679, 34678}                                                                                 |                    |
| 952:810a | $0, 0, 0, 0, e^{12}, a_2e^{14} + e^{23}, a_2e^{13} + e^{24}, e^{37} + e^{46} + e^{15}, e^{47} + e^{36} + e^{25}$                                          | 8/17(1, 1, 1, 1, 2, 2, 2, 3, 3)                 | {0, 123489, 126789, 3467}                                                                                 |                    |
| 952:810b | $0, 0, 0, 0, e^{12}, a_2e^{14} - e^{23}, a_2e^{13} + e^{24}, e^{46} - e^{37} + e^{15}, e^{47} + e^{36} + e^{25}$                                          | 8/17(1, 1, 1, 1, 2, 2, 2, 3, 3)                 | {0, 123489, 126789, 3467}                                                                                 |                    |
| 952:811a | $0, 0, 0, 0, e^{12}, e^{14} + e^{23}, e^{13}a_1 + e^{24}, e^{36}a_1 + e^{15} + e^{47}, e^{25} + e^{37} + e^{46}$                                          | 8/17(1, 1, 1, 1, 2, 2, 2, 3, 3)                 | {0, 123489, 126789, 13569, 14579, 23578, 24568, 3467}                                                     |                    |
| 952:811b | $0, 0, 0, 0, e^{12}, e^{23} - e^{14}, -e^{13}a_1 + e^{24}, e^{36}a_1 + e^{47} + e^{15}, e^{37} + e^{46} + e^{25}$                                         | 8/17(1, 1, 1, 1, 2, 2, 2, 3, 3)                 | {0, 123489, 126789, 13569, 14579, 23578, 24568, 3467}                                                     |                    |
| 952:811c | $0, 0, 0, 0, -e^{12}, e^{23} - e^{14}, -e^{13}a_1 + e^{24}, e^{36}a_1 + e^{15} + e^{47}, e^{25} + e^{37} + e^{46}$                                        | 8/17(1, 1, 1, 1, 2, 2, 2, 3, 3)                 | {0, 123489, 126789, 13569, 14579, 23578, 24568, 3467}                                                     |                    |
| 952:812a | $0, 0, 0, 0, (-1 + a_4 + a_1)e^{23} + e^{14},$<br>$e^{24}a_4 + e^{13}a_1, -(-1 + a_4)e^{12} + e^{34}, e^{15} + e^{37} + e^{26}, e^{16} + e^{25} + e^{47}$ | 8/17(1, 1, 1, 1, 2, 2, 2, 3, 3)                 | {0, 123489, 1256, 13579, 14678, 23679, 24578, 345689}                                                     |                    |
| 952:812b | $0, 0, 0, 0, (-1 + a_4 + a_1)e^{23} + e^{14},$<br>$e^{24}a_4 + e^{13}a_1, -(-1 + a_4)e^{12} + e^{34}, e^{26} - e^{15} + e^{37}, e^{25} + e^{16} + e^{47}$ | 8/17(1, 1, 1, 1, 2, 2, 2, 3, 3)                 | {0, 123489, 1256, 13579, 14678, 23679, 24578, 345689}                                                     |                    |
| 952:812c | $0, 0, 0, 0, (-1 + a_4 - a_1)e^{23} - e^{14},$<br>$-e^{24}a_4 + e^{13}a_1, (-1 + a_4)e^{12} + e^{34}, e^{15} + e^{26} + e^{37}, e^{16} + e^{47} + e^{25}$ | 8/17(1, 1, 1, 1, 2, 2, 2, 3, 3)                 | {0, 123489, 1256, 13579, 14678, 23679, 24578, 345689}                                                     |                    |
| 952:812d | $0, 0, 0, 0, (-1 + a_4 - a_1)e^{23} - e^{14},$<br>$e^{24}a_4 - e^{13}a_1, (-1 + a_4)e^{12} + e^{34}, e^{37} - e^{15} + e^{26}, e^{47} + e^{16} + e^{25}$  | 8/17(1, 1, 1, 1, 2, 2, 2, 3, 3)                 | {0, 123489, 1256, 13579, 14678, 23679, 24578, 345689}                                                     |                    |
| 951:22   | $0, 0, 0, 0, e^{12}, e^{13}, e^{14}, e^{24}, e^{26} + e^{35}$                                                                                             | 1/13(6, 6, 7, 9, 12, 13, 15, 15, 19)            | {0, 12349, 123789, 1246, 12678, 13458, 1357, 145689, 15679, 234567, 23568, 24579, 2589, 346789, 369, 478} |                    |
| 951:25   | $0, 0, 0, 0, e^{12}, e^{13}, e^{24}, e^{34}, e^{35} + e^{26}$                                                                                             | 1/7(4, 3, 3, 5, 7, 7, 8, 8, 10)                 | {0, 12349, 123789, 12468, 1267, 13457, 1358, 1456789, 1569, 23456, 235678, 24589, 2579, 34679, 3689, 478} |                    |
| 951:29   | $0, 0, 0, 0, e^{12}, e^{13}, e^{23}, e^{14}, e^{26} + e^{35}$                                                                                             | 1/19(8, 10, 10, 15, 18, 18, 20, 23, 28)         | {0, 12349, 12389, 12467, 12678, 13457, 13578, 14569, 15689, 234568, 2356, 245789, 2579, 346789, 3679, 48} |                    |
| 951:46   | $0, 0, 0, 0, e^{12}(-1 + a_2), a_2e^{13}, e^{23}, e^{14}, e^{35} + e^{17} + e^{26}$                                                                       | 1/19(8, 10, 10, 15, 18, 18, 20, 23, 28)         | {0, 12349, 12389, 12467, 12678, 13457, 13578, 14569, 15689, 234568, 2356, 245789, 2579, 346789, 3679, 48} |                    |
| 951:56   | $0, 0, 0, 0, e^{12}, e^{23} + e^{14}, e^{13}, e^{34}, e^{45} + e^{26}$                                                                                    | 1/51(27, 22, 31, 26, 49, 53, 58, 57, 75)        | {0, 12349, 1267, 135689, 14578, 235789, 24568, 34679}                                                     |                    |
| 951:65   | $0, 0, 0, 0, e^{12}, e^{13}, e^{14}, e^{23}, e^{26} + e^{35} + e^{17}$                                                                                    | 3/16(2, 3, 3, 4, 5, 5, 6, 6, 8)                 | {0, 12349, 12678, 13578, 14569, 2356, 245789, 346789}                                                     |                    |
| 951:68   | $0, 0, 0, 0, e^{12}, e^{13}, e^{14}, e^{23}, e^{27} + e^{45} + e^{16}$                                                                                    | 1/12(5, 6, 8, 7, 11, 13, 12, 14, 18)            | {0, 12349, 12678, 135789, 1456, 23569, 24578, 346789}                                                     |                    |
| 951:71   | $0, 0, 0, 0, e^{12}, e^{13}, e^{14}, e^{23}, e^{26} + e^{47} + e^{35}$                                                                                    | 1/9(4, 5, 5, 5, 9, 9, 9, 10, 14)                | {0, 12349, 12379, 14569, 15679, 234567, 2356, 47}                                                         |                    |
| 951:72   | $0, 0, 0, 0, e^{12}, e^{13}, e^{14}, e^{23}, e^{25} + e^{37} + e^{46}$                                                                                    | 1/41(18, 23, 22, 24, 41, 40, 42, 45, 64)        | {0, 12349, 126789, 134589, 15679, 234567, 258, 34678}                                                     |                    |
| 951:74   | $0, 0, 0, 0, -e^{12}, e^{13}, e^{24}, e^{23}, e^{45} + e^{17} + e^{36}$                                                                                   | 1/179(83, 93, 97, 101, 176, 180, 194, 190, 277) | {0, 12349, 124689, 13589, 1569, 23456, 2458, 368}                                                         |                    |
| 951:79   | $0, 0, 0, 0, -e^{12}, e^{13}, e^{24}, e^{34}, e^{17} + e^{36} + e^{45}$                                                                                   | 1/179(81, 101, 97, 93, 182, 178, 194, 190, 275) | {0, 12349, 124689, 13589, 1569, 23456, 2458, 368}                                                         |                    |
| 951:83   | $0, 0, 0, 0, e^{12}(-1 + a_2), a_2e^{13}, e^{14} + e^{23}, e^{24}, e^{26} + e^{35} + e^{17}$                                                              | 1/12(5, 6, 7, 8, 11, 12, 13, 14, 18)            | {0, 12349, 12678, 1357, 145689, 23568, 24579, 346789}                                                     |                    |
| 951:84a  | $0, 0, 0, 0, e^{12}, e^{13}, e^{14} + e^{23}, e^{24}, e^{16} + e^{45} + e^{27}$                                                                           | 3/53(8, 8, 11, 11, 16, 19, 19, 19, 27)          | {0, 12349, 12678, 13579, 14568, 235689, 2457, 346789}                                                     |                    |
| 951:84b  | $0, 0, 0, 0, e^{12}, -e^{13}, e^{23} + e^{14}, e^{24}, e^{16} + e^{27} + e^{45}$                                                                          | 3/53(8, 8, 11, 11, 16, 19, 19, 19, 27)          | {0, 12349, 12678, 13579, 14568, 235689, 2457, 346789}                                                     |                    |
| 951:85a  | $0, 0, 0, 0, e^{12}, e^{13}, e^{23} + e^{14}, e^{24}, e^{15} + e^{37} + e^{46}$                                                                           | 1/23(11, 13, 11, 13, 24, 22, 24, 26, 35)        | {0, 12349, 126789, 1357, 14568, 235689, 24579, 34678}                                                     |                    |
| 951:85b  | $0, 0, 0, 0, -e^{12}, e^{13}, e^{14} + e^{23}, e^{24}, e^{15} + e^{37} + e^{46}$                                                                          | 1/23(11, 13, 11, 13, 24, 22, 24, 26, 35)        | {0, 12349, 126789, 1357, 14568, 235689, 24579, 34678}                                                     |                    |
| 951:86   | $0, 0, 0, 0, e^{12}, e^{13}, e^{14} + e^{23}, e^{24}, e^{25} + e^{46} + e^{37}$                                                                           | 3/401(65, 71, 68, 74, 136, 133, 139, 145, 207)  | {0, 12349, 126789, 34678}                                                                                 |                    |

Table A.4 – Continued to next page

Table A.4 – Continued from previous page

| Name     | g                                                                                                              | N                                                  | S <sub>0</sub>                                        | S = S <sub>0</sub> |
|----------|----------------------------------------------------------------------------------------------------------------|----------------------------------------------------|-------------------------------------------------------|--------------------|
| 951:87   | $0, 0, 0, 0, e^{12}, e^{13}, e^{23} + e^{14}, e^{24}, e^{27} + e^{36} + e^{45}$                                | 5/148(14, 15, 16, 17, 29, 30, 31, 32, 46)          | {0, 12349, 13579, 2457}                               |                    |
| 951:89   | $0, 0, 0, 0, e^{12}, e^{34}, e^{14} - e^{23}, e^{13}, e^{26} + e^{15} + e^{47}$                                | 3/160(28, 26, 29, 27, 54, 56, 55, 57, 82)          | {0, 12349, 12789, 3478}                               |                    |
| 951:91a  | $0, 0, 0, 0, a_1 e^{12}, e^{23} + e^{14}, e^{24} + e^{13}(1 + a_1), e^{34}, e^{27} + e^{16} + e^{35}$          | 1/23(11, 11, 13, 13, 22, 24, 24, 26, 35)           | {0, 12349, 1267, 13568, 145789, 23578, 245689, 34679} |                    |
| 951:91b  | $0, 0, 0, 0, a_1 e^{12}, -e^{14} + e^{23}, e^{24} + e^{13}(1 + a_1), e^{34}, e^{16} + e^{27} + e^{35}$         | 1/23(11, 11, 13, 13, 22, 24, 24, 26, 35)           | {0, 12349, 1267, 13568, 145789, 23578, 245689, 34679} |                    |
| 951:92a  | $0, 0, 0, 0, e^{12}, e^{14} + e^{23}, e^{13} + e^{24}, e^{34}, e^{36} + e^{47} + e^{15}$                       | 15/29(1, 1, 1, 1, 2, 2, 2, 3)                      | {0, 12349, 12679, 13568, 14578, 235789, 245689, 3467} | ✓                  |
| 951:92b  | $0, 0, 0, 0, e^{12}, -e^{23} + e^{14}, e^{24} + e^{13}, e^{34}, e^{47} + e^{36} + e^{15}$                      | 15/29(1, 1, 1, 1, 2, 2, 2, 3)                      | {0, 12349, 12679, 13568, 14578, 235789, 245689, 3467} | ✓                  |
| 951:92c  | $0, 0, 0, 0, -e^{12}, e^{23} + e^{14}, e^{24} + e^{13}, e^{34}, e^{47} + e^{36} + e^{15}$                      | 15/29(1, 1, 1, 1, 2, 2, 2, 3)                      | {0, 12349, 12679, 13568, 14578, 235789, 245689, 3467} | ✓                  |
| 951:93a  | $0, 0, 0, 0, e^{12}, e^{14} + e^{23}, e^{24} + e^{13}, e^{34}, e^{46} + e^{37} + e^{15}$                       | 15/29(1, 1, 1, 1, 2, 2, 2, 3)                      | {0, 12349, 12679, 3467}                               | ✓                  |
| 951:93b  | $0, 0, 0, 0, e^{12}, -e^{14} + e^{23}, e^{13} + e^{24}, e^{34}, e^{37} + e^{15} + e^{46}$                      | 15/29(1, 1, 1, 1, 2, 2, 2, 3)                      | {0, 12349, 12679, 3467}                               | ✓                  |
| 951:95   | $0, 0, 0, 0, e^{12}(-1 + a_2), a_2 e^{13}, e^{23}, e^{14}, e^{17} + e^{26} + e^{48} + e^{35}$                  | 1/9(4, 5, 5, 5, 9, 9, 10, 9, 14)                   | {0, 12349, 12389, 14569, 15689, 234568, 2356, 48}     |                    |
| 951:96   | $0, 0, 0, 0, e^{12}, e^{13}, e^{23}, e^{14}, e^{15} + e^{27} + e^{38} + e^{46}$                                | 5/148(15, 16, 14, 17, 31, 29, 30, 32, 46)          | {0, 12349, 1456, 23569}                               |                    |
| 951:98a  | $0, 0, 0, 0, e^{12}, e^{13}, e^{24}, e^{14} + e^{23}, e^{48} + e^{16} + e^{25} + e^{37}$                       | 15/29(1, 1, 1, 1, 2, 2, 2, 3)                      | {0, 12349, 13589, 2458}                               |                    |
| 951:98b  | $0, 0, 0, 0, -e^{12}, e^{13}, e^{24}, e^{14} + e^{23}, e^{37} + e^{48} + e^{25} + e^{16}$                      | 15/29(1, 1, 1, 1, 2, 2, 2, 3)                      | {0, 12349, 13589, 2458}                               |                    |
| 951:99   | $0, 0, 0, 0, e^{12}(-1 + a_2), e^{13}, e^{24}, a_2 e^{14} + e^{23}, e^{17} + e^{28} + e^{36} + e^{45}$         | 5/148(14, 15, 16, 17, 29, 30, 32, 31, 46)          | {0, 12349, 13589, 2458}                               |                    |
| 951:100a | $0, 0, 0, 0, e^{12}, e^{34}, (1 + a_2)e^{14} + e^{23}, a_2 e^{13} + e^{24}, e^{48} + e^{37} + e^{16} + e^{25}$ | 15/29(1, 1, 1, 1, 2, 2, 2, 3)                      | {0, 12349, 12789, 3478}                               |                    |
| 951:100b | $0, 0, 0, 0, e^{12}, e^{34}, (1 + a_2)e^{14} - e^{23}, a_2 e^{13} + e^{24}, e^{48} + e^{25} + e^{37} + e^{16}$ | 15/29(1, 1, 1, 1, 2, 2, 2, 3)                      | {0, 12349, 12789, 3478}                               |                    |
| 94321:10 | $0, 0, 0, 0, 0, -e^{12}, e^{16}, e^{17} + e^{23}, e^{18} + e^{45} + e^{36}$                                    | 3/40(3, 8, 9, 10, 10, 11, 14, 17, 20)              | {0, 123479, 123579, 134568, 1368, 246789, 256789, 45} |                    |
| 94321:16 | $0, 0, 0, 0, 0, -e^{12}, e^{16}, e^{23} + e^{17}, e^{28} + e^{45} + e^{67}$                                    | 2/15(2, 3, 6, 6, 6, 5, 7, 9, 12)                   | {0, 123479, 123579, 134689, 135689, 245678, 2678, 45} |                    |
| 94321:28 | $0, 0, 0, 0, 0, -e^{12}, e^{23} + e^{16}, e^{36} + e^{17}, e^{37} + e^{45} + e^{18}$                           | 1/185(43, 108, 86, 140, 140, 151, 194, 237, 280)   | {0, 12479, 12579, 14568, 168, 246789, 256789, 45}     |                    |
| 9431:24  | $0, 0, 0, 0, 0, e^{12}, e^{26} + e^{13}, e^{16} + e^{45}, e^{27} + e^{36}$                                     | 1/124(65, 38, 76, 84, 84, 103, 141, 168, 179)      | {0, 12478, 12578, 145679, 1679, 24689, 25689, 45}     |                    |
| 9431:27  | $0, 0, 0, 0, 0, e^{12}, e^{26} + e^{13}, e^{16}, e^{27} + e^{36} + e^{45}$                                     | 1/59(24, 22, 44, 45, 45, 46, 68, 70, 90)           | {0, 124578, 1278, 14679, 15679, 24689, 25689, 45}     |                    |
| 9431:28  | $0, 0, 0, 0, 0, e^{12}, e^{26} + e^{13}, e^{16} + e^{34}, e^{45} + e^{36} + e^{27}$                            | 1/477(233, 155, 310, 311, 387, 388, 543, 621, 698) | {0, 124578, 15679, 24689}                             |                    |
| 9431:36  | $0, 0, 0, 0, 0, e^{12}, e^{26} + e^{13}, e^{16} + e^{34}, e^{15} + e^{36} + e^{27}$                            | 2/27(7, 4, 8, 10, 12, 11, 15, 18, 19)              | {0, 124578, 1679, 245689}                             |                    |
| 9431:40  | $0, 0, 0, 0, 0, -e^{12}, e^{23} + e^{16}, e^{26} + e^{14}, e^{25} + e^{36} + e^{17}$                           | 1/71(23, 32, 46, 64, 69, 55, 78, 87, 101)          | {0, 12578, 15689, 2679}                               |                    |
| 9431:50  | $0, 0, 0, 0, 0, e^{12}, e^{16}, e^{26} + e^{13}, e^{18} + e^{27} + e^{45}$                                     | 1/25(8, 11, 22, 19, 19, 19, 27, 30, 38)            | {0, 124578, 1278, 14568, 168, 24567, 267, 45}         |                    |
| 9431:56a | $0, 0, 0, 0, 0, e^{12}, e^{23} + e^{16}, e^{13} + e^{26}, e^{45} + e^{17} + e^{28}$                            | 5/13(1, 1, 2, 2, 2, 2, 3, 3, 4)                    | {0, 124578, 1278, 14689, 15689, 24679, 25679, 45}     | ✓                  |
| 9431:56b | $0, 0, 0, 0, 0, e^{12}, e^{23} - e^{16}, e^{26} + e^{13}, e^{28} + e^{45} + e^{17}$                            | 5/13(1, 1, 2, 2, 2, 2, 3, 3, 4)                    | {0, 124578, 1278, 14689, 15689, 24679, 25679, 45}     | ✓                  |
| 9431:57a | $0, 0, 0, 0, 0, e^{12}, e^{23} + e^{16}, e^{13} + e^{26}, e^{45} + e^{27} + e^{18}$                            | 5/13(1, 1, 2, 2, 2, 2, 3, 3, 4)                    | {0, 124578, 1278, 14568, 168, 24567, 267, 45}         | ✓                  |
| 9431:57b | $0, 0, 0, 0, 0, e^{12}, e^{16} + e^{23}, -e^{13} + e^{26}, e^{27} + e^{18} + e^{45}$                           | 5/13(1, 1, 2, 2, 2, 2, 3, 3, 4)                    | {0, 124578, 1278, 14568, 168, 24567, 267, 45}         | ✓                  |
| 9431:59a | $0, 0, 0, 0, 0, e^{12}, e^{16}, e^{13} + e^{26}, e^{17} + e^{28} + e^{45} + e^{36}$                            | 5/13(1, 1, 2, 2, 2, 2, 3, 3, 4)                    | {0, 124578, 1278, 14689, 15689, 24679, 25679, 45}     |                    |
| 9431:59b | $0, 0, 0, 0, 0, e^{12}, -e^{16}, e^{26} + e^{13}, e^{28} + e^{36} + e^{45} + e^{17}$                           | 5/13(1, 1, 2, 2, 2, 2, 3, 3, 4)                    | {0, 124578, 1278, 14689, 15689, 24679, 25679, 45}     |                    |
| 9431:62  | $0, 0, 0, 0, 0, e^{12}, e^{16} + e^{23}, e^{26} + e^{14}, e^{27} + e^{18} + e^{35}$                            | 1/17(6, 7, 12, 14, 14, 13, 19, 20, 26)             | {0, 1278, 168, 267}                                   |                    |
| 9431:63a | $0, 0, 0, 0, 0, (-1 + a_2)e^{12}, e^{16} + e^{23}, e^{13}a_2 + e^{26}, e^{45} + e^{28} + e^{17} + e^{36}$      | 5/13(1, 1, 2, 2, 2, 2, 3, 3, 4)                    | {0, 124578, 1278, 14689, 15689, 24679, 25679, 45}     |                    |
| 9431:63b | $0, 0, 0, 0, 0, (-1 + a_2)e^{12}, e^{23} - e^{16}, e^{13}a_2 + e^{26}, e^{17} + e^{28} + e^{45} + e^{36}$      | 5/13(1, 1, 2, 2, 2, 2, 3, 3, 4)                    | {0, 124578, 1278, 14689, 15689, 24679, 25679, 45}     |                    |
| 9421:62  | $0, 0, 0, 0, 0, -e^{12}, e^{34}, e^{16} + e^{23}, e^{18} + e^{36} + e^{45}$                                    | 1/109(31, 67, 62, 69, 91, 98, 131, 129, 160)       | {0, 124578, 128, 14679, 1569, 246789, 25689, 457}     |                    |
| 9421:65  | $0, 0, 0, 0, 0, e^{12}, e^{14} + e^{35}, e^{13} + e^{26}, e^{28} + e^{36}$                                     | 1/109(58, 31, 62, 91, 87, 89, 149, 120, 151)       | {0, 1248, 12578, 14689, 156789, 245679, 269, 457}     |                    |
| 9421:75  | $0, 0, 0, 0, 0, -e^{12}, e^{13}, e^{16} + e^{24}, e^{18} + e^{46} + e^{35}$                                    | 1/179(58, 101, 132, 116, 143, 159, 190, 217, 275)  | {0, 12358, 1278, 1369, 15679, 236789, 25689, 357}     |                    |
| 9421:76  | $0, 0, 0, 0, 0, e^{12}, e^{13}, e^{26} + e^{14}, e^{28} + e^{35} + e^{46}$                                     | 1/69(33, 24, 47, 48, 58, 57, 80, 81, 105)          | {0, 12358, 1278, 13689, 156789, 23679, 2569, 357}     |                    |
| 9421:77  | $0, 0, 0, 0, 0, -e^{12}, e^{24} + e^{13}, e^{16} + e^{25}, e^{56} + e^{18}$                                    | 1/179(58, 83, 168, 143, 116, 141, 226, 199, 257)   | {0, 12348, 1278, 1369, 14679, 236789, 24689, 347}     |                    |
| 9421:80  | $0, 0, 0, 0, 0, e^{12}, e^{34}, e^{13} + e^{26}, e^{36} + e^{15} + e^{28}$                                     | 1/7(4, 2, 4, 5, 6, 6, 9, 8, 10)                    | {0, 124578, 1258, 146789, 1689, 245679, 2569, 47}     |                    |
| 9421:82  | $0, 0, 0, 0, 0, e^{12}, e^{35} + e^{14}, e^{13} + e^{26}, e^{28} + e^{45} + e^{36}$                            | 1/73(40, 22, 44, 55, 51, 62, 95, 84, 106)          | {0, 14689, 156789, 457}                               |                    |
| 9421:91  | $0, 0, 0, 0, 0, -e^{12}, e^{13}, e^{16} + e^{24}, e^{25} + e^{18} + e^{46}$                                    | 1/13(4, 7, 11, 8, 12, 11, 15, 15, 19)              | {0, 12358, 12578, 13569, 15679, 236789, 2689, 37}     |                    |
| 9421:93  | $0, 0, 0, 0, 0, e^{12}, e^{13}, e^{16} + e^{23}, e^{18} + e^{27} + e^{45}$                                     | 1/9(3, 5, 6, 7, 7, 8, 9, 11, 14)                   | {0, 124578, 1278, 14679, 15679, 24689, 25689, 45}     |                    |
| 9421:94a | $0, 0, 0, 0, 0, -e^{12}, e^{13} + e^{24}, e^{25} + e^{16}, e^{34} + e^{56} + e^{18}$                           | 2/29(5, 7, 12, 10, 10, 12, 17, 17, 22)             | {0, 12348, 1278, 1369, 14679, 236789, 24689, 347}     | ✓                  |
| 9421:94b | $0, 0, 0, 0, 0, -e^{12}, e^{24} - e^{13}, e^{25} + e^{16}, e^{34} + e^{56} + e^{18}$                           | 2/29(5, 7, 12, 10, 10, 12, 17, 17, 22)             | {0, 12348, 1278, 1369, 14679, 236789, 24689, 347}     | ✓                  |
| 9421:95  | $0, 0, 0, 0, 0, e^{12}, -e^{13}, e^{16} + e^{34}, e^{35} + e^{47} + e^{18}$                                    | 1/8(2, 6, 5, 5, 7, 8, 7, 10, 12)                   | {0, 12358, 12478, 13469, 15679, 236789, 245689, 3457} |                    |
| 9421:107 | $0, 0, 0, 0, 0, e^{12}, -e^{13}, e^{16} + e^{34}, e^{18} + e^{47} + e^{25}$                                    | 1/225(64, 152, 147, 133, 192, 216, 211, 280, 344)  | {0, 12358, 124578, 134569, 15679, 236789, 24689, 347} |                    |

Table A.4 – Continued to next page

Table A.4 – Continued from previous page

| Name     | g                                                                                                         | N                                                  | S <sub>0</sub>                                                                                                        | S = S <sub>0</sub> |
|----------|-----------------------------------------------------------------------------------------------------------|----------------------------------------------------|-----------------------------------------------------------------------------------------------------------------------|--------------------|
| 9421:111 | $0, 0, 0, 0, 0, e^{12}, e^{35} + e^{14}, e^{34} + e^{16}, e^{18} + e^{37}$                                | $1/39(9, 29, 14, 33, 28, 38, 42, 47, 56)$          | $\{\emptyset, 12378, 1248, 134569, 15679, 235689, 2456789, 347\}$                                                     |                    |
| 9421:113 | $0, 0, 0, 0, 0, e^{12}, -e^{13} + e^{24}, e^{34} + e^{16}, e^{47} + e^{18} + e^{35}$                      | $1/92(30, 52, 67, 45, 75, 82, 97, 112, 142)$       | $\{\emptyset, 236789, 245689, 3457\}$                                                                                 |                    |
| 9421:120 | $0, 0, 0, 0, 0, e^{12}, e^{23} + e^{14}, e^{16} + e^{34}, e^{25} + e^{18} + e^{37}$                       | $3/217(22, 43, 33, 54, 66, 65, 76, 87, 109)$       | $\{\emptyset, 23689, 246789, 347\}$                                                                                   |                    |
| 9421:121 | $0, 0, 0, 0, 0, (-1 + a_2)e^{12}, e^{13}a_2, e^{16} + e^{23}, e^{45} + e^{36} + e^{18} + e^{27}$          | $1/9(3, 5, 6, 7, 7, 8, 9, 11, 14)$                 | $\{\emptyset, 124578, 1278, 14679, 15679, 24689, 25689, 45\}$                                                         |                    |
| 9421:122 | $0, 0, 0, 0, 0, e^{12}, e^{45} - e^{13}, e^{34} + e^{16}, e^{35} + e^{47} + e^{18}$                       | $1/81(20, 59, 66, 33, 53, 79, 86, 99, 119)$        | $\{\emptyset, 12478, 15679, 245689\}$                                                                                 |                    |
| 9421:125 | $0, 0, 0, 0, 0, -e^{12}, e^{34}, e^{16} + e^{25}, e^{18} + e^{56} + e^{37}$                               | $1/9(3, 5, 4, 6, 6, 8, 10, 11, 14)$                | $\{\emptyset, 12378, 128, 13469, 14679, 234689, 246789, 37\}$                                                         |                    |
| 9421:127 | $0, 0, 0, 0, 0, e^{12}, e^{23} + e^{14}, e^{13} + e^{26}, e^{35} + e^{28} + e^{17}$                       | $2/53(11, 10, 20, 19, 21, 21, 30, 31, 41)$         | $\{\emptyset, 1278, 145689, 245679\}$                                                                                 |                    |
| 9421:128 | $0, 0, 0, 0, 0, e^{12}, e^{14} + e^{23}, e^{13} + e^{26}, e^{28} + e^{45} + e^{17}$                       | $5/81(7, 6, 12, 11, 14, 13, 18, 19, 25)$           | $\{\emptyset, 1278, 14689, 24679\}$                                                                                   |                    |
| 9421:129 | $0, 0, 0, 0, 0, e^{12}, -e^{13} + e^{45}, e^{16} + e^{34}, e^{23} + e^{47} + e^{18}$                      | $1/33(9, 22, 27, 13, 23, 31, 36, 40, 49)$          | $\{\emptyset, 1238, 134569, 245689\}$                                                                                 |                    |
| 9421:130 | $0, 0, 0, 0, 0, e^{12}, e^{35} + e^{14}, e^{16} + e^{34}, e^{18} + e^{37} + e^{25}$                       | $1/207(49, 152, 76, 174, 147, 201, 223, 250, 299)$ | $\{\emptyset, 134569, 15679, 347\}$                                                                                   |                    |
| 9421:131 | $0, 0, 0, 0, 0, e^{12}, -e^{13}, e^{16} + e^{34}, e^{18} + e^{26} + e^{35} + e^{47}$                      | $25/81(1, 2, 2, 2, 3, 3, 3, 4, 5)$                 | $\{\emptyset, 13469, 15679, 3457\}$                                                                                   |                    |
| 9421:132 | $0, 0, 0, 0, 0, e^{12}, e^{34}, e^{13} + e^{26}, e^{28} + e^{15} + e^{36} + e^{47}$                       | $5/33(4, 2, 4, 3, 6, 6, 7, 8, 10)$                 | $\{\emptyset, 124578, 1258, 47\}$                                                                                     |                    |
| 9421:134 | $0, 0, 0, 0, 0, e^{12}, e^{13} + e^{24}, e^{16}, e^{18} + e^{27} + e^{45} + e^{36}$                       | $5/81(6, 7, 12, 11, 14, 13, 18, 19, 25)$           | $\{\emptyset, 1278, 14679, 24689\}$                                                                                   |                    |
| 9421:136 | $0, 0, 0, 0, 0, e^{12}, e^{13}, e^{14} + e^{26}, e^{35} + e^{46} + e^{28} + e^{17}$                       | $5/81(7, 6, 11, 12, 14, 13, 18, 19, 25)$           | $\{\emptyset, 1278, 13689, 23679\}$                                                                                   |                    |
| 9421:137 | $0, 0, 0, 0, 0, -e^{12}, e^{13}, e^{24} + e^{16}, e^{25} + e^{37} + e^{18} + e^{46}$                      | $5/123(8, 14, 15, 16, 24, 22, 23, 30, 38)$         | $\{\emptyset, 13569, 15679, 37\}$                                                                                     |                    |
| 9421:139 | $0, 0, 0, 0, 0, e^{12}, e^{35} + e^{14}, e^{34} + e^{16}, e^{18} + e^{37} + e^{26}$                       | $1/243(73, 146, 94, 198, 177, 219, 271, 292, 365)$ | $\{\emptyset, 134569, 15679, 347\}$                                                                                   |                    |
| 9421:140 | $0, 0, 0, 0, 0, -e^{12}, -e^{13}, e^{35} + e^{16} + e^{24}, e^{46} + e^{57} + e^{18}$                     | $1/31(10, 19, 20, 20, 19, 29, 30, 39, 49)$         | $\{\emptyset, 1238, 12578, 13569, 1679, 236789, 25689, 357\}$                                                         |                    |
| 9421:142 | $0, 0, 0, 0, 0, -e^{12}, e^{15} + e^{34}, e^{16} + e^{23} + e^{45}, e^{36} + e^{18} + e^{47}$             | $1/17(5, 11, 10, 8, 13, 16, 18, 21, 26)$           | $\{\emptyset, 12478, 1258, 457\}$                                                                                     |                    |
| 9421:144 | $0, 0, 0, 0, 0, (-1 + a_2)e^{12}, e^{23} + e^{14}, e^{26} + e^{13}a_2, e^{28} + e^{36} + e^{45} + e^{17}$ | $5/81(7, 6, 12, 11, 14, 13, 18, 19, 25)$           | $\{\emptyset, 1278, 14689, 24679\}$                                                                                   |                    |
| 9421:145 | $0, 0, 0, 0, 0, e^{12}, -e^{13} + e^{45}, e^{16} + e^{34}, e^{35} + e^{47} + e^{18} + e^{26}$             | $15/149(3, 6, 8, 4, 7, 9, 11, 12, 15)$             | $\{\emptyset, 15679\}$                                                                                                |                    |
| 9421:146 | $0, 0, 0, 0, 0, -e^{12}, e^{14} + e^{23}, e^{25} + e^{34} + e^{16}, e^{18} + e^{56} + e^{37}$             | $1/157(54, 85, 81, 112, 108, 139, 166, 193, 247)$  | $\{\emptyset, 23689, 246789, 347\}$                                                                                   |                    |
| 942:55   | $0, 0, 0, 0, 0, e^{12}, a_1e^{14} + e^{23}, e^{16} + e^{35}, e^{26} + e^{45}$                             | $1/11(5, 5, 8, 8, 7, 10, 13, 15, 15)$              | $\{\emptyset, 123489, 125789, 135679, 1469, 2368, 245678, 3457\}$                                                     | ✓                  |
| 942:192  | $0, 0, 0, 0, 0, e^{12}, e^{13}, e^{16}, e^{36} + e^{45} + e^{27}$                                         | $1/9(3, 5, 6, 7, 7, 8, 9, 11, 14)$                 | $\{\emptyset, 123489, 123589, 124578, 1278, 13456, 136, 14679, 15679, 2345678, 23678, 24689, 25689, 3479, 3579, 45\}$ |                    |
| 942:194  | $0, 0, 0, 0, 0, e^{12}, e^{13}, e^{26}, e^{36} + e^{27} + e^{45}$                                         | $1/8(4, 3, 5, 6, 6, 7, 9, 10, 12)$                 | $\{\emptyset, 123489, 123589, 124578, 1278, 134568, 1368, 146789, 156789, 234567, 2367, 2469, 2569, 3479, 3579, 45\}$ |                    |
| 942:197  | $0, 0, 0, 0, 0, e^{12}, e^{13}, e^{45} + e^{16}, e^{27} + e^{36}$                                         | $1/52(23, 26, 28, 36, 36, 49, 51, 72, 77)$         | $\{\emptyset, 123489, 123589, 12478, 12578, 13456, 136, 145679, 1679, 234678, 235678, 24689, 25689, 34579, 379, 45\}$ |                    |
| 942:199  | $0, 0, 0, 0, 0, e^{12}, e^{13}, e^{26} + e^{45}, e^{27} + e^{36}$                                         | $1/52(26, 23, 27, 36, 36, 49, 53, 72, 76)$         | $\{\emptyset, 123489, 123589, 12478, 12578, 13468, 13568, 146789, 156789, 234567, 2367, 24569, 269, 34579, 379, 45\}$ |                    |
| 942:213  | $0, 0, 0, 0, 0, a_1e^{12}, e^{13}, e^{16} + e^{24}, e^{17} + e^{25} + e^{34}$                             | $1/19(7, 11, 13, 14, 16, 18, 20, 25, 27)$          | $\{\emptyset, 12389, 12578, 13569, 167, 236789, 2568, 3579\}$                                                         |                    |
| 942:234  | $0, 0, 0, 0, 0, e^{12}, e^{13}, e^{16} + e^{24}, e^{45} + e^{36} + e^{27}$                                | $1/179(66, 93, 116, 132, 143, 159, 182, 225, 275)$ | $\{\emptyset, 123589, 1278, 136, 15679, 23678, 25689, 3579\}$                                                         |                    |
| 942:237  | $0, 0, 0, 0, 0, e^{12}, e^{13}, e^{16} + e^{34}, e^{27} + e^{36} + e^{45}$                                | $1/106(40, 58, 63, 75, 86, 98, 103, 138, 161)$     | $\{\emptyset, 123589, 124578, 13456, 15679, 23678, 24689, 3479\}$                                                     |                    |
| 942:239  | $0, 0, 0, 0, 0, e^{12}, e^{13}, e^{26} + e^{34}, e^{36} + e^{45} + e^{27}$                                | $2/31(8, 6, 9, 11, 12, 14, 17, 20, 23)$            | $\{\emptyset, 123589, 124578, 1368, 146789, 234567, 2569, 3479\}$                                                     |                    |
| 942:262  | $0, 0, 0, 0, 0, e^{12}, e^{13}, e^{34} + e^{26}, e^{27} + e^{36} + e^{15}$                                | $1/12(6, 5, 6, 10, 11, 11, 12, 16, 17)$            | $\{\emptyset, 12389, 124578, 13568, 146789, 23467, 2569, 34579\}$                                                     |                    |
| 942:268  | $0, 0, 0, 0, 0, e^{12}, e^{13}, e^{35} + e^{14} + e^{26}, e^{36} + e^{27}$                                | $1/61(29, 27, 30, 54, 53, 56, 59, 83, 86)$         | $\{\emptyset, 12389, 12578, 1368, 156789, 23567, 269, 3579\}$                                                         |                    |
| 942:270  | $0, 0, 0, 0, 0, e^{12}, e^{13}, e^{35} + e^{16} + e^{24}, e^{27} + e^{36}$                                | $1/22(10, 10, 11, 20, 19, 20, 21, 30, 31)$         | $\{\emptyset, 12389, 12578, 1356, 1679, 23678, 25689, 3579\}$                                                         |                    |
| 942:277  | $0, 0, 0, 0, 0, e^{12}, e^{13}, e^{26} + e^{17}, e^{27} + e^{36} + e^{45}$                                | $1/109(41, 54, 67, 81, 81, 95, 108, 149, 162)$     | $\{\emptyset, 123489, 123589, 134568, 1368, 2469, 2569, 45\}$                                                         |                    |
| 942:278  | $0, 0, 0, 0, 0, e^{12}, e^{13}, e^{27} + e^{36}, e^{17} + e^{26} + e^{45}$                                | $1/31(14, 15, 16, 22, 22, 29, 30, 45, 44)$         | $\{\emptyset, 123489, 123589, 13469, 13569, 24568, 268, 45\}$                                                         |                    |
| 942:279a | $0, 0, 0, 0, 0, e^{12}, e^{13}, e^{37} + e^{26}, e^{36} + e^{27} + e^{45}$                                | $1/28(14, 13, 13, 20, 20, 27, 27, 40, 40)$         | $\{\emptyset, 123489, 123589, 124578, 1278, 134568, 1368, 146789, 156789, 234567, 2367, 2469, 2569, 3479, 3579, 45\}$ | ✓                  |
| 942:279b | $0, 0, 0, 0, 0, e^{12}, e^{13}, e^{37} - e^{26}, e^{45} + e^{36} + e^{27}$                                | $1/28(14, 13, 13, 20, 20, 27, 27, 40, 40)$         | $\{\emptyset, 123489, 123589, 124578, 1278, 134568, 1368, 146789, 156789, 234567, 2367, 2469, 2569, 3479, 3579, 45\}$ | ✓                  |
| 942:280a | $0, 0, 0, 0, 0, e^{12}, e^{13}, e^{27} + e^{36}, e^{26} + e^{37} + e^{45}$                                | $1/28(14, 13, 13, 20, 20, 27, 27, 40, 40)$         | $\{\emptyset, 123489, 123589, 12479, 12579, 13469, 13569, 146789, 156789, 234567, 2367, 24568, 268, 34578, 378, 45\}$ | ✓                  |
| 942:280b | $0, 0, 0, 0, 0, -e^{12}, e^{13}, e^{36} - e^{27}, e^{37} + e^{45} + e^{26}$                               | $1/28(14, 13, 13, 20, 20, 27, 27, 40, 40)$         | $\{\emptyset, 123489, 123589, 12479, 12579, 13469, 13569, 146789, 156789, 234567, 2367, 24568, 268, 34578, 378, 45\}$ | ✓                  |

Table A.4 – Continued to next page

Table A.4 – Continued from previous page

| Name     | g                                                                                                       | N                                                    | S <sub>0</sub>                                            | S = S <sub>0</sub> |
|----------|---------------------------------------------------------------------------------------------------------|------------------------------------------------------|-----------------------------------------------------------|--------------------|
| 942:285a | $0, 0, 0, 0, 0, e^{12}, e^{13}, a_1 e^{25} + e^{34} + e^{16}, e^{24} + e^{35} + e^{17}$                 | $1/13(5, 8, 8, 10, 10, 13, 13, 18, 18)$              | $\{0, 12389, 12478, 13469, 167, 236789, 2468, 3479\}$     | ✓                  |
| 942:285b | $0, 0, 0, 0, 0, -e^{12}, e^{13}, a_1 e^{25} + e^{16} + e^{34}, e^{24} + e^{17} + e^{35}$                | $1/13(5, 8, 8, 10, 10, 13, 13, 18, 18)$              | $\{0, 12389, 12478, 13469, 167, 236789, 2468, 3479\}$     | ✓                  |
| 942:290  | $0, 0, 0, 0, 0, e^{12}, e^{13}, e^{16} + e^{35} + e^{24}, e^{27} + e^{36} + e^{45}$                     | $1/178(70, 94, 105, 140, 129, 164, 175, 234, 269)$   | $\{0, 23678, 25689, 3579\}$                               |                    |
| 942:301  | $0, 0, 0, 0, 0, a_1 e^{12}, e^{13}, e^{35} + e^{16} + e^{24}, e^{17} + e^{34} + e^{26}$                 | $1/14(6, 7, 8, 12, 11, 13, 14, 19, 20)$              | $\{0, 12389, 13569, 2568\}$                               |                    |
| 942:309a | $0, 0, 0, 0, 0, e^{12}, e^{13}, e^{36} + e^{27} + e^{14}, e^{37} + e^{26} + e^{15}$                     | $1/32(14, 15, 15, 30, 30, 29, 29, 44, 44)$           | $\{0, 12389, 12479, 13469, 16789, 2367, 2468, 3478\}$     | ✓                  |
| 942:309b | $0, 0, 0, 0, 0, -e^{12}, e^{13}, e^{14} - e^{27} + e^{36}, e^{37} + e^{26} + e^{15}$                    | $1/32(14, 15, 15, 30, 30, 29, 29, 44, 44)$           | $\{0, 12389, 12479, 13469, 16789, 2367, 2468, 3478\}$     | ✓                  |
| 942:310  | $0, 0, 0, 0, 0, e^{12}, e^{13}, e^{27} + e^{36} + e^{14}, e^{16} + e^{37} + e^{25}$                     | $1/71(31, 35, 33, 68, 62, 66, 64, 99, 97)$           | $\{0, 12389, 12479, 3478\}$                               |                    |
| 942:362  | $0, 0, 0, 0, 0, -e^{12}, e^{14} + e^{23}, e^{16}, e^{17} + e^{36} + e^{25}$                             | $1/13(4, 7, 8, 11, 12, 11, 15, 15, 19)$              | $\{0, 123489, 12578, 1367, 14569, 23568, 246789, 34579\}$ |                    |
| 942:364  | $0, 0, 0, 0, 0, e^{12}, e^{13} + e^{24}, e^{16}, e^{27} + e^{36} + e^{45}$                              | $1/69(28, 29, 48, 47, 58, 57, 76, 85, 105)$          | $\{0, 123489, 1278, 136, 14679, 23678, 24689, 3479\}$     |                    |
| 942:365  | $0, 0, 0, 0, 0, -e^{12}, e^{23} + e^{14}, e^{15} + e^{26}, e^{36} + e^{17}$                             | $1/179(57, 84, 116, 143, 168, 141, 200, 225, 257)$   | $\{0, 123489, 1278, 13678, 14689, 236, 24679, 3479\}$     |                    |
| 942:367  | $0, 0, 0, 0, 0, -e^{12}, e^{14} + e^{23}, e^{35} + e^{16}, e^{17} + e^{36}$                             | $1/179(55, 116, 83, 144, 143, 171, 199, 226, 254)$   | $\{0, 123489, 12578, 13567, 1469, 2368, 2456789, 34579\}$ |                    |
| 942:368  | $0, 0, 0, 0, 0, e^{12}, e^{13} + e^{24}, e^{35} + e^{16}, e^{27} + e^{36}$                              | $1/59(31, 19, 33, 45, 48, 50, 64, 81, 83)$           | $\{0, 123489, 12578, 1356, 14679, 23678, 245689, 34579\}$ |                    |
| 942:369  | $0, 0, 0, 0, 0, -e^{12}, e^{24} + e^{13}, e^{16} + e^{35}, e^{17} + e^{46}$                             | $1/17(7, 9, 11, 9, 12, 16, 18, 23, 25)$              | $\{0, 123489, 12578, 13569, 1467, 236789, 24568, 34579\}$ |                    |
| 942:370  | $0, 0, 0, 0, 0, e^{12}, e^{14} + e^{23}, e^{16} + e^{35}, e^{27} + e^{46}$                              | $1/19(9, 8, 12, 11, 14, 17, 20, 26, 28)$             | $\{0, 123489, 12578, 135679, 146, 23689, 245678, 34579\}$ |                    |
| 942:390  | $0, 0, 0, 0, 0, -e^{12}, e^{14} + e^{23}, e^{35} + e^{16}, e^{36} + e^{25} + e^{17}$                    | $1/61(19, 39, 29, 49, 48, 58, 68, 77, 87)$           | $\{0, 123489, 12578, 34579\}$                             |                    |
| 942:391a | $0, 0, 0, 0, 0, -e^{12}, e^{13} + e^{24}, e^{26} + e^{15}, e^{17} + e^{46} + e^{35}$                    | $4/29(3, 3, 5, 5, 6, 6, 8, 9, 11)$                   | $\{0, 123489, 1278, 13689, 14678, 23679, 246, 3479\}$     | ✓                  |
| 942:391b | $0, 0, 0, 0, 0, -e^{12}, e^{24} - e^{13}, e^{26} + e^{15}, e^{17} + e^{46} + e^{35}$                    | $4/29(3, 3, 5, 5, 6, 6, 8, 9, 11)$                   | $\{0, 123489, 1278, 13689, 14678, 23679, 246, 3479\}$     | ✓                  |
| 942:392  | $0, 0, 0, 0, 0, -e^{12}, e^{13} a_2 + e^{24}, e^{16} + e^{25}, e^{17} + e^{35} + e^{46}$                | $1/8(3, 4, 6, 5, 6, 7, 9, 10, 12)$                   | $\{0, 123489, 1278, 1369, 1467, 236789, 2468, 3479\}$     |                    |
| 942:395  | $0, 0, 0, 0, 0, -e^{12}, e^{23} + e^{14}, e^{35} + e^{16}, e^{36} + e^{45} + e^{17}$                    | $2/61(11, 17, 17, 23, 22, 28, 34, 39, 45)$           | $\{0, 123489, 1469, 2368\}$                               |                    |
| 942:396  | $0, 0, 0, 0, 0, e^{12}, e^{24} + e^{13}, e^{35} + e^{16}, e^{36} + e^{27} + e^{45}$                     | $1/417(203, 157, 249, 295, 314, 360, 452, 563, 609)$ | $\{0, 123489, 14679, 23678\}$                             |                    |
| 942:408  | $0, 0, 0, 0, 0, e^{12}, e^{14} + e^{23}, e^{26} + e^{13}, e^{15} + e^{27} + e^{46}$                     | $1/71(35, 26, 52, 43, 69, 61, 78, 87, 104)$          | $\{0, 12578, 14568, 2467\}$                               |                    |
| 942:411  | $0, 0, 0, 0, 0, e^{12}, e^{13} + e^{24}, e^{16} + e^{34}, e^{27} + e^{15} + e^{36}$                     | $1/73(34, 27, 44, 51, 71, 61, 78, 95, 105)$          | $\{0, 23678, 245689, 34579\}$                             |                    |
| 942:412  | $0, 0, 0, 0, 0, -e^{12}, e^{14} + e^{23}, e^{16} + e^{34}, e^{17} + e^{25} + e^{36}$                    | $1/111(40, 61, 60, 81, 100, 101, 121, 141, 161)$     | $\{0, 23568, 246789, 34579\}$                             |                    |
| 942:414  | $0, 0, 0, 0, 0, e^{12}, e^{24} + e^{13}, e^{34} + e^{16}, e^{45} + e^{36} + e^{27}$                     | $3/14(2, 2, 3, 3, 4, 4, 5, 6, 7)$                    | $\{0, 23678, 24689, 3479\}$                               |                    |
| 942:420  | $0, 0, 0, 0, 0, -e^{12}, e^{23} + e^{14}, e^{35} + e^{16}, e^{24} + e^{36} + e^{17}$                    | $1/148(47, 94, 70, 117, 118, 141, 164, 188, 211)$    | $\{0, 13567, 1469, 34579\}$                               |                    |
| 942:422  | $0, 0, 0, 0, 0, -e^{12}, e^{14} + e^{23}, e^{26} + e^{34} + e^{15}, e^{36} + e^{17}$                    | $1/178(62, 86, 105, 129, 172, 148, 191, 234, 253)$   | $\{0, 13678, 14689, 3479\}$                               |                    |
| 942:423  | $0, 0, 0, 0, 0, -e^{12}, e^{14} + e^{23}, e^{35} + e^{16} + e^{24}, e^{17} + e^{36}$                    | $1/178(64, 105, 87, 128, 146, 169, 192, 233, 256)$   | $\{0, 12578, 13567, 2368\}$                               |                    |
| 942:429  | $0, 0, 0, 0, 0, -e^{12}, -e^{14} + e^{23}, e^{17} + e^{36}, e^{27} + e^{35} + e^{46}$                   | $1/31(12, 14, 17, 19, 28, 26, 31, 43, 45)$           | $\{0, 123489, 127, 13679, 1468, 2369, 24678, 34789\}$     |                    |
| 942:436  | $0, 0, 0, 0, 0, e^{12}, e^{24} + e^{13}, e^{16} + e^{25} + e^{34}, e^{36} + e^{15} + e^{27}$            | $13/109(4, 3, 5, 6, 8, 7, 9, 11, 12)$                | $\{0, 23678\}$                                            |                    |
| 942:438  | $0, 0, 0, 0, 0, -e^{12}, e^{24} + e^{13}, e^{16} + e^{45} + e^{23}, e^{17} + e^{46} + e^{35}$           | $7/38(2, 3, 4, 3, 4, 5, 6, 7, 8)$                    | $\{0, 2468\}$                                             |                    |
| 942:439  | $0, 0, 0, 0, 0, -e^{12}, e^{13} a_2 + e^{24}, e^{16} + e^{25} + e^{34}, e^{17} + e^{35} + e^{46}$       | $2/31(6, 8, 11, 9, 12, 14, 17, 20, 23)$              | $\{0, 236789, 2468, 3479\}$                               |                    |
| 942:442a | $0, 0, 0, 0, 0, -e^{12}, e^{24} - e^{13}, e^{35} + e^{46} + e^{17}, e^{36} + e^{45} + e^{27}$           | $1/7(3, 3, 4, 4, 6, 6, 7, 10, 10)$                   | $\{0, 123489, 127, 1368, 14679, 23678, 2469, 34789\}$     |                    |
| 942:442b | $0, 0, 0, 0, 0, -e^{12}, e^{24} - e^{13}, -e^{35} + e^{17} + e^{46}, e^{36} + e^{27} + e^{45}$          | $1/7(3, 3, 4, 4, 6, 6, 7, 10, 10)$                   | $\{0, 123489, 127, 1368, 14679, 23678, 2469, 34789\}$     |                    |
| 942:445a | $0, 0, 0, 0, 0, e^{14} + e^{23}, e^{13} + e^{24}, e^{27} + e^{16}, e^{17} + e^{35} + e^{26}$            | $1/5(2, 2, 3, 3, 4, 5, 5, 7, 7)$                     | $\{0, 123489, 1267, 1369, 1478, 2379, 2468, 346789\}$     |                    |
| 942:445b | $0, 0, 0, 0, 0, e^{14} + e^{23}, -e^{13} + e^{24}, e^{27} - e^{16}, e^{26} + e^{35} + e^{17}$           | $1/5(2, 2, 3, 3, 4, 5, 5, 7, 7)$                     | $\{0, 123489, 1267, 1369, 1478, 2379, 2468, 346789\}$     |                    |
| 942:446a | $0, 0, 0, 0, 0, e^{24} + e^{13}, e^{23} + e^{14}, e^{27} + e^{16}, e^{17} + e^{26} + e^{35}$            | $1/5(2, 2, 3, 3, 4, 5, 5, 7, 7)$                     | $\{0, 123489, 1267, 13578, 14569, 23568, 24579, 346789\}$ |                    |
| 942:446b | $0, 0, 0, 0, 0, e^{24} + e^{13}, -e^{14} + e^{23}, -e^{16} + e^{27}, e^{17} + e^{26} + e^{35}$          | $1/5(2, 2, 3, 3, 4, 5, 5, 7, 7)$                     | $\{0, 123489, 1267, 13578, 14569, 23568, 24579, 346789\}$ |                    |
| 942:447a | $0, 0, 0, 0, 0, e^{14} + e^{23}, e^{13} + e^{24}, e^{27} + e^{16}, e^{15} + e^{36} + e^{47}$            | $1/81(37, 37, 39, 39, 78, 76, 76, 113, 115)$         | $\{0, 123489, 12679, 1356, 14578, 23579, 245689, 34678\}$ |                    |
| 942:447b | $0, 0, 0, 0, 0, -e^{14} - e^{23}, -e^{13} + e^{24}, e^{16} + e^{27}, e^{15} + e^{47} + e^{36}$          | $1/81(37, 37, 39, 39, 78, 76, 76, 113, 115)$         | $\{0, 123489, 12679, 1356, 14578, 23579, 245689, 34678\}$ |                    |
| 942:448a | $0, 0, 0, 0, 0, e^{23} + e^{14}, e^{24} + e^{13}, e^{27} + e^{16}, e^{37} + e^{46} + e^{15}$            | $1/81(37, 37, 39, 39, 78, 76, 76, 113, 115)$         | $\{0, 123489, 12679, 1369, 14789, 237, 2468, 34678\}$     |                    |
| 942:448b | $0, 0, 0, 0, 0, -e^{14} + e^{23}, e^{24} + e^{13}, e^{27} + e^{16}, e^{46} + e^{37} + e^{15}$           | $1/81(37, 37, 39, 39, 78, 76, 76, 113, 115)$         | $\{0, 123489, 12679, 1369, 14789, 237, 2468, 34678\}$     |                    |
| 942:455a | $0, 0, 0, 0, 0, -e^{24} + e^{13}, e^{12} + e^{34}, e^{37} + e^{15} + e^{26}, e^{47} + e^{16} + e^{25}$  | $8/17(1, 1, 1, 1, 2, 2, 2, 3, 3)$                    | $\{0, 123489, 1256, 13579, 14678, 23679, 24578, 345689\}$ |                    |
| 942:455b | $0, 0, 0, 0, 0, -e^{24} + e^{13}, e^{12} + e^{34}, e^{37} + e^{26} + e^{15}, e^{25} + e^{16} + e^{47}$  | $8/17(1, 1, 1, 1, 2, 2, 2, 3, 3)$                    | $\{0, 123489, 1256, 13579, 14678, 23679, 24578, 345689\}$ |                    |
| 942:455c | $0, 0, 0, 0, 0, -e^{13} + e^{24}, e^{34} - e^{12}, e^{37} + e^{26} + e^{15}, e^{47} + e^{25} + e^{16}$  | $8/17(1, 1, 1, 1, 2, 2, 2, 3, 3)$                    | $\{0, 123489, 1256, 13579, 14678, 23679, 24578, 345689\}$ |                    |
| 942:455d | $0, 0, 0, 0, 0, -e^{13} + e^{24}, -e^{12} + e^{34}, e^{26} - e^{15} + e^{37}, e^{47} + e^{16} + e^{25}$ | $8/17(1, 1, 1, 1, 2, 2, 2, 3, 3)$                    | $\{0, 123489, 1256, 13579, 14678, 23679, 24578, 345689\}$ |                    |
| 942:456a | $0, 0, 0, 0, 0, e^{24} + e^{13}, e^{34} - e^{12}, e^{15} + e^{27} + e^{36}, e^{16} + e^{25} + e^{47}$   | $8/17(1, 1, 1, 1, 2, 2, 2, 3, 3)$                    | $\{0, 123489, 14678, 23679\}$                             |                    |
| 942:456b | $0, 0, 0, 0, 0, e^{24} - e^{13}, e^{34} - e^{12}, e^{15} + e^{36} + e^{27}, e^{16} + e^{25} + e^{47}$   | $8/17(1, 1, 1, 1, 2, 2, 2, 3, 3)$                    | $\{0, 123489, 14678, 23679\}$                             |                    |

Table A.4 – Continued to next page

Table A.4 – Continued from previous page

| Name     | g                                                                                                               | N                                                  | S <sub>0</sub>                                                                                                        | S = S <sub>0</sub> |
|----------|-----------------------------------------------------------------------------------------------------------------|----------------------------------------------------|-----------------------------------------------------------------------------------------------------------------------|--------------------|
| 942:457a | $0, 0, 0, 0, 0, -e^{13} + e^{24}, e^{12} + e^{34}, e^{27} + e^{15} + e^{36}, e^{17} + e^{25} + e^{46}$          | $8/17(1, 1, 1, 1, 2, 2, 2, 3, 3)$                  | $\{\emptyset, 123489, 12689, 1378, 14678, 23679, 2479, 346\}$                                                         |                    |
| 942:457b | $0, 0, 0, 0, 0, e^{24} - e^{13}, e^{34} + e^{12}, e^{27} + e^{36} - e^{15}, e^{46} + e^{25} + e^{17}$           | $8/17(1, 1, 1, 1, 2, 2, 2, 3, 3)$                  | $\{\emptyset, 123489, 12689, 1378, 14678, 23679, 2479, 346\}$                                                         |                    |
| 942:457c | $0, 0, 0, 0, 0, e^{24} - e^{13}, -e^{12} + e^{34}, e^{36} + e^{15} + e^{27}, e^{46} + e^{17} + e^{25}$          | $8/17(1, 1, 1, 1, 2, 2, 2, 3, 3)$                  | $\{\emptyset, 123489, 12689, 1378, 14678, 23679, 2479, 346\}$                                                         |                    |
| 942:457d | $0, 0, 0, 0, 0, e^{24} - e^{13}, -e^{12} + e^{34}, e^{36} + e^{27} - e^{15}, e^{46} + e^{25} + e^{17}$          | $8/17(1, 1, 1, 1, 2, 2, 2, 3, 3)$                  | $\{\emptyset, 123489, 12689, 1378, 14678, 23679, 2479, 346\}$                                                         |                    |
| 942:458a | $0, 0, 0, 0, 0, a_1 e^{23} + e^{14}, a_1 e^{13} + e^{24}, e^{26} + e^{17} + e^{35}, e^{16} + e^{45} + e^{27}$   | $1/5(2, 2, 3, 3, 4, 5, 5, 7, 7)$                   | $\{\emptyset, 123489, 1267, 1368, 1479, 2378, 2469, 346789\}$                                                         |                    |
| 942:458b | $0, 0, 0, 0, 0, a_1 e^{23} - e^{14}, a_1 e^{13} + e^{24}, e^{35} - e^{17} + e^{26}, e^{45} + e^{16} + e^{27}$   | $1/5(2, 2, 3, 3, 4, 5, 5, 7, 7)$                   | $\{\emptyset, 123489, 1267, 1368, 1479, 2378, 2469, 346789\}$                                                         |                    |
| 942:459a | $0, 0, 0, 0, 0, a_3 e^{23} + e^{14}, a_3 e^{13} + e^{24}, e^{27} + e^{16} + e^{35}, e^{17} + e^{26} + e^{45}$   | $1/5(2, 2, 3, 3, 4, 5, 5, 7, 7)$                   | $\{\emptyset, 123489, 1267, 13569, 14578, 23579, 24568, 346789\}$                                                     |                    |
| 942:459b | $0, 0, 0, 0, 0, a_3 e^{23} + e^{14}, -a_3 e^{13} + e^{24}, -e^{16} + e^{27} + e^{35}, e^{17} + e^{26} + e^{45}$ | $1/5(2, 2, 3, 3, 4, 5, 5, 7, 7)$                   | $\{\emptyset, 123489, 1267, 13569, 14578, 23579, 24568, 346789\}$                                                     |                    |
| 941:217  | $0, 0, 0, 0, 0, e^{12}, e^{13}, e^{14}, e^{45} + e^{36} + e^{27}$                                               | $1/7(3, 4, 4, 5, 6, 7, 7, 8, 11)$                  | $\{\emptyset, 12349, 123589, 12457, 1278, 13456, 1368, 14679, 156789, 2345678, 2367, 24689, 2569, 34789, 3579, 458\}$ |                    |
| 941:220  | $0, 0, 0, 0, 0, e^{12}, e^{13}, e^{24}, e^{27} + e^{36} + e^{45}$                                               | $1/13(7, 6, 7, 9, 11, 13, 14, 15, 20)$             | $\{\emptyset, 12349, 123589, 12457, 1278, 134568, 136, 146789, 15679, 234567, 23678, 2469, 25689, 34789, 3579, 458\}$ |                    |
| 941:224  | $0, 0, 0, 0, 0, e^{12}, e^{13}, e^{14} + e^{25}, e^{36} + e^{27}$                                               | $1/13(6, 6, 7, 11, 11, 12, 13, 17, 19)$            | $\{\emptyset, 123459, 12389, 12457, 1278, 1346, 13568, 14679, 156789, 234678, 23567, 24689, 2569, 345789, 379, 458\}$ |                    |
| 941:230  | $0, 0, 0, 0, 0, e^{12}, e^{13}, e^{24} + e^{35}, e^{27} + e^{36}$                                               | $1/7(4, 3, 3, 6, 6, 7, 7, 9, 10)$                  | $\{\emptyset, 123459, 12389, 1247, 12578, 13468, 1356, 1456789, 1679, 234567, 23678, 2469, 25689, 34789, 3579, 458\}$ |                    |
| 941:239  | $0, 0, 0, 0, 0, e^{12}, e^{13}, e^{23}, e^{27} + e^{36} + e^{45}$                                               | $5/19(2, 2, 2, 3, 3, 4, 4, 4, 6)$                  | $\{\emptyset, 12349, 12359, 124578, 1278, 134568, 1368, 14679, 15679, 234567, 2367, 24689, 25689, 34789, 35789, 45\}$ |                    |
| 941:245  | $0, 0, 0, 0, 0, e^{12}, e^{13}, e^{24}, e^{27} + e^{15} + e^{36}$                                               | $1/19(10, 8, 10, 15, 18, 18, 20, 23, 28)$          | $\{\emptyset, 12349, 12389, 12457, 12578, 134568, 1356, 146789, 1679, 23467, 23678, 24569, 25689, 345789, 3579, 48\}$ |                    |
| 941:250  | $0, 0, 0, 0, 0, e^{12}, e^{13}, e^{25} + e^{14}, e^{27} + e^{36} + e^{45}$                                      | $1/61(29, 30, 34, 47, 46, 59, 63, 76, 93)$         | $\{\emptyset, 12457, 1278, 14679, 156789, 24689, 2569, 458\}$                                                         |                    |
| 941:253  | $0, 0, 0, 0, 0, e^{12}, e^{13}, e^{35} + e^{24}, e^{36} + e^{45} + e^{27}$                                      | $1/61(34, 29, 29, 46, 46, 63, 63, 75, 92)$         | $\{\emptyset, 234567, 23678, 2469, 25689, 34789, 3579, 458\}$                                                         |                    |
| 941:275  | $0, 0, 0, 0, 0, (-1 + a_2)e^{12}, a_2 e^{13}, e^{23}, e^{45} + e^{36} + e^{18} + e^{27}$                        | $5/19(2, 2, 2, 3, 3, 4, 4, 4, 6)$                  | $\{\emptyset, 12349, 12359, 124578, 1278, 134568, 1368, 14679, 15679, 234567, 2367, 24689, 25689, 34789, 35789, 45\}$ |                    |
| 941:293  | $0, 0, 0, 0, 0, -e^{12}, e^{23} + e^{14}, e^{15}, e^{36} + e^{17}$                                              | $1/13(4, 8, 7, 11, 11, 12, 15, 15, 19)$            | $\{\emptyset, 123459, 123489, 1257, 1278, 13567, 13678, 14569, 14689, 23568, 236, 2456789, 24679, 345789, 3479, 58\}$ |                    |
| 941:294  | $0, 0, 0, 0, 0, e^{12}, e^{24} + e^{13}, e^{15}, e^{36} + e^{27}$                                               | $1/8(4, 3, 5, 6, 6, 7, 9, 10, 12)$                 | $\{\emptyset, 123459, 123489, 1257, 1278, 1356, 1368, 145679, 146789, 235678, 2367, 245689, 2469, 345789, 3479, 58\}$ |                    |
| 941:295  | $0, 0, 0, 0, 0, -e^{12}, e^{14} + e^{23}, e^{35}, e^{36} + e^{17}$                                              | $1/9(3, 6, 4, 7, 7, 9, 10, 11, 13)$                | $\{\emptyset, 123459, 123489, 12578, 127, 13567, 13678, 145689, 1469, 2356, 2368, 2456789, 24679, 34579, 34789, 58\}$ |                    |
| 941:296  | $0, 0, 0, 0, 0, -e^{12}, e^{13} + e^{24}, e^{35}, e^{17} + e^{46}$                                              | $1/52(23, 28, 32, 27, 36, 51, 55, 68, 78)$         | $\{\emptyset, 123459, 123489, 12578, 127, 13569, 13689, 145678, 1467, 235679, 236789, 24568, 246, 34579, 34789, 58\}$ |                    |
| 941:313  | $0, 0, 0, 0, 0, -e^{12}, e^{24} + e^{13}, e^{15} + e^{23}, e^{17} + e^{46}$                                     | $1/51(19, 27, 37, 29, 45, 46, 56, 64, 75)$         | $\{\emptyset, 123459, 1278, 13689, 14567, 23679, 24568, 345789\}$                                                     |                    |
| 941:315  | $0, 0, 0, 0, 0, -e^{12}, e^{14} + e^{23}, e^{34} + e^{15}, e^{36} + e^{17}$                                     | $1/61(21, 38, 29, 46, 54, 59, 67, 75, 88)$         | $\{\emptyset, 123459, 1257, 13678, 14689, 23568, 2456789, 3479\}$                                                     |                    |
| 941:316  | $0, 0, 0, 0, 0, e^{12}, e^{13} + e^{24}, e^{14} + e^{35}, e^{27} + e^{36}$                                      | $1/106(63, 40, 51, 74, 86, 103, 114, 137, 154)$    | $\{\emptyset, 123459, 12578, 1368, 14679, 23567, 245689, 34789\}$                                                     |                    |
| 941:317  | $0, 0, 0, 0, 0, e^{12}, e^{24} + e^{13}, e^{15} + e^{34}, e^{36} + e^{27}$                                      | $2/31(8, 6, 9, 11, 12, 14, 17, 20, 23)$            | $\{\emptyset, 123459, 1257, 1368, 146789, 235678, 245689, 3479\}$                                                     |                    |
| 941:320  | $0, 0, 0, 0, 0, -e^{12}, e^{13} + e^{24}, e^{15}, e^{46} + e^{35} + e^{17}$                                     | $1/61(23, 36, 47, 34, 46, 59, 70, 69, 93)$         | $\{\emptyset, 123489, 1278, 13689, 14678, 23679, 246, 3479\}$                                                         |                    |
| 941:323  | $0, 0, 0, 0, 0, -e^{12}, e^{14} + e^{23}, e^{35}, e^{45} + e^{36} + e^{17}$                                     | $1/179(66, 116, 83, 133, 132, 182, 199, 215, 265)$ | $\{\emptyset, 123489, 127, 13678, 1469, 2368, 24679, 34789\}$                                                         |                    |
| 941:326a | $0, 0, 0, 0, 0, e^{14} + e^{23}, e^{13} + e^{24}, e^{15}, e^{16} + e^{27}$                                      | $1/53(20, 20, 37, 37, 43, 57, 57, 63, 77)$         | $\{\emptyset, 123459, 123489, 12567, 12678, 1356, 1368, 14579, 14789, 23578, 237, 245689, 2469, 3456789, 34679, 58\}$ | ✓                  |
| 941:326b | $0, 0, 0, 0, 0, e^{23} - e^{14}, e^{24} + e^{13}, e^{15}, e^{27} + e^{16}$                                      | $1/53(20, 20, 37, 37, 43, 57, 57, 63, 77)$         | $\{\emptyset, 123459, 123489, 12567, 12678, 1356, 1368, 14579, 14789, 23578, 237, 245689, 2469, 3456789, 34679, 58\}$ | ✓                  |
| 941:327a | $0, 0, 0, 0, 0, e^{24} + e^{13}, e^{12} + e^{34}, e^{15}, e^{37} + e^{26}$                                      | $1/28(16, 13, 13, 16, 20, 29, 29, 36, 42)$         | $\{\emptyset, 123459, 123489, 1256, 1268, 1357, 1378, 145679, 146789, 235678, 2367, 245789, 2479, 345689, 3469, 58\}$ | ✓                  |
| 941:327b | $0, 0, 0, 0, 0, e^{13} - e^{24}, e^{12} + e^{34}, e^{15}, e^{37} + e^{26}$                                      | $1/28(16, 13, 13, 16, 20, 29, 29, 36, 42)$         | $\{\emptyset, 123459, 123489, 1256, 1268, 1357, 1378, 145679, 146789, 235678, 2367, 245789, 2479, 345689, 3469, 58\}$ | ✓                  |

Table A.4 – Continued to next page



Table A.4 – Continued from previous page

| Name     | g                                                                                                           | N                                                  | S <sub>0</sub>                                                                                            | S = S <sub>0</sub> |
|----------|-------------------------------------------------------------------------------------------------------------|----------------------------------------------------|-----------------------------------------------------------------------------------------------------------|--------------------|
| 941:328a | $0, 0, 0, 0, 0, e^{34} + e^{12}, e^{24} + e^{13}, e^{15}, e^{26} + e^{37}$                                  | 1/28(16, 13, 13, 16, 20, 29, 29, 36, 42)           | {0, 123459, 123489, 12579, 12789, 13569, 13689, 145679, 146789, 235678, 2367, 24568, 246, 34578, 347, 58} | ✓                  |
| 941:328b | $0, 0, 0, 0, 0, e^{34} - e^{12}, e^{24} + e^{13}, e^{15}, e^{26} + e^{37}$                                  | 1/28(16, 13, 13, 16, 20, 29, 29, 36, 42)           | {0, 123459, 123489, 12579, 12789, 13569, 13689, 145679, 146789, 235678, 2367, 24568, 246, 34578, 347, 58} | ✓                  |
| 941:340  | $0, 0, 0, 0, 0, e^{12}, e^{23} + e^{14}, e^{13}, e^{35} + e^{46} + e^{27}$                                  | 1/22(11, 10, 14, 13, 20, 21, 24, 25, 34)           | {0, 12349, 1278, 13679, 1468, 23689, 2467, 34789}                                                         |                    |
| 941:341  | $0, 0, 0, 0, 0, e^{12}, e^{24} + e^{13}, e^{34}, e^{36} + e^{27} + e^{15}$                                  | 1/12(7, 5, 6, 8, 11, 12, 13, 14, 18)               | {0, 12349, 1257, 13568, 146789, 23678, 245689, 34579}                                                     |                    |
| 941:342  | $0, 0, 0, 0, 0, -e^{12}, e^{13} + e^{24}, e^{34}, e^{17} + e^{46} + e^{35}$                                 | 3/61(9, 12, 13, 10, 18, 21, 22, 23, 31)            | {0, 12349, 127, 13689, 14678, 236789, 2468, 3479}                                                         |                    |
| 941:349  | $0, 0, 0, 0, 0, -e^{12}, e^{24} + e^{13}, e^{15} + e^{23}, e^{46} + e^{35} + e^{17}$                        | 1/184(75, 97, 128, 106, 150, 172, 203, 225, 278)   | {0, 1278, 13689, 23679}                                                                                   |                    |
| 941:352  | $0, 0, 0, 0, 0, -e^{12}, e^{23} + e^{14}, e^{15} + e^{34}, e^{17} + e^{25} + e^{36}$                        | 1/71(26, 43, 35, 52, 61, 69, 78, 87, 104)          | {0, 1257, 13678, 23568}                                                                                   |                    |
| 941:353  | $0, 0, 0, 0, 0, -e^{12}, e^{24} + e^{13}, e^{15} + e^{34}, e^{17} + e^{35} + e^{46}$                        | 1/10(4, 6, 7, 5, 8, 10, 11, 12, 15)                | {0, 13689, 14678, 3479}                                                                                   |                    |
| 941:354  | $0, 0, 0, 0, 0, e^{12}, e^{14} + e^{23}, e^{45} + e^{13}, e^{46} + e^{35} + e^{27}$                         | 1/178(105, 70, 122, 87, 140, 175, 192, 227, 262)   | {0, 13679, 1468, 34789}                                                                                   |                    |
| 941:359a | $0, 0, 0, 0, 0, e^{24} + e^{13}, e^{34} - e^{12}, e^{15} + e^{23}, e^{16} + e^{47}$                         | 1/113(47, 71, 71, 47, 95, 118, 118, 142, 165)      | {0, 123459, 1268, 13789, 14567, 23679, 24578, 345689}                                                     | ✓                  |
| 941:359b | $0, 0, 0, 0, 0, e^{24} - e^{13}, e^{34} - e^{12}, e^{15} + e^{23}, e^{47} + e^{16}$                         | 1/113(47, 71, 71, 47, 95, 118, 118, 142, 165)      | {0, 123459, 1268, 13789, 14567, 23679, 24578, 345689}                                                     | ✓                  |
| 941:360a | $0, 0, 0, 0, 0, e^{14} + e^{23}, -e^{12} + e^{34}, e^{15}, e^{25} + e^{16} + e^{37}$                        | 1/89(35, 61, 35, 61, 70, 96, 96, 105, 131)         | {0, 123489, 1256, 13678, 14579, 23578, 24679, 345689}                                                     | ✓                  |
| 941:360b | $0, 0, 0, 0, 0, -e^{14} + e^{23}, -e^{12} + e^{34}, e^{15}, e^{16} + e^{25} + e^{37}$                       | 1/89(35, 61, 35, 61, 70, 96, 96, 105, 131)         | {0, 123489, 1256, 13678, 14579, 23578, 24679, 345689}                                                     | ✓                  |
| 941:361a | $0, 0, 0, 0, 0, e^{23} + e^{14}, e^{12} + e^{34}, e^{15}, e^{36} + e^{17} + e^{25}$                         | 1/89(35, 61, 35, 61, 70, 96, 96, 105, 131)         | {0, 123489, 12689, 13678, 1478, 2379, 24679, 346}                                                         | ✓                  |
| 941:361b | $0, 0, 0, 0, 0, e^{14} + e^{23}, -e^{12} + e^{34}, e^{15}, e^{36} + e^{25} + e^{17}$                        | 1/89(35, 61, 35, 61, 70, 96, 96, 105, 131)         | {0, 123489, 12689, 13678, 1478, 2379, 24679, 346}                                                         | ✓                  |
| 941:373a | $0, 0, 0, 0, 0, e^{14} + e^{23}, e^{13} + e^{24}, e^{12}, e^{15} + e^{47} + e^{36}$                         | 1/23(13, 13, 11, 11, 22, 24, 24, 26, 35)           | {0, 12349, 12679, 13568, 14578, 235789, 245689, 3467}                                                     | ✓                  |
| 941:373b | $0, 0, 0, 0, 0, -e^{23} + e^{14}, e^{24} + e^{13}, e^{12}, e^{36} + e^{47} + e^{15}$                        | 1/23(13, 13, 11, 11, 22, 24, 24, 26, 35)           | {0, 12349, 12679, 13568, 14578, 235789, 245689, 3467}                                                     | ✓                  |
| 941:374a | $0, 0, 0, 0, 0, e^{23} + e^{14}, e^{24} + e^{13}, e^{12}, e^{15} + e^{37} + e^{46}$                         | 1/23(13, 13, 11, 11, 22, 24, 24, 26, 35)           | {0, 12349, 12679, 13689, 14789, 2378, 2468, 3467}                                                         | ✓                  |
| 941:374b | $0, 0, 0, 0, 0, -e^{14} + e^{23}, e^{24} + e^{13}, e^{12}, e^{46} + e^{15} + e^{37}$                        | 1/23(13, 13, 11, 11, 22, 24, 24, 26, 35)           | {0, 12349, 12679, 13689, 14789, 2378, 2468, 3467}                                                         | ✓                  |
| 941:380a | $0, 0, 0, 0, 0, e^{23} + e^{14}, e^{12} + e^{34}, e^{13} + e^{25}, e^{47} + e^{15} + e^{26}$                | 37/177(3, 2, 3, 2, 4, 5, 5, 6, 7)                  | {0, 13679, 14578, 345689}                                                                                 | ✓                  |
| 941:380b | $0, 0, 0, 0, 0, e^{14} - e^{23}, e^{12} + e^{34}, e^{13} + e^{25}, e^{47} + e^{26} + e^{15}$                | 37/177(3, 2, 3, 2, 4, 5, 5, 6, 7)                  | {0, 13679, 14578, 345689}                                                                                 | ✓                  |
| 941:381a | $0, 0, 0, 0, 0, e^{14} - e^{23}, e^{12} + e^{34}, e^{13} + e^{25}, e^{15} + e^{46} + e^{27}$                | 37/177(3, 2, 3, 2, 4, 5, 5, 6, 7)                  | {0, 12689, 13679, 2378}                                                                                   | ✓                  |
| 941:381b | $0, 0, 0, 0, 0, -e^{23} - e^{14}, e^{34} + e^{12}, e^{25} + e^{13}, e^{27} + e^{46} + e^{15}$               | 37/177(3, 2, 3, 2, 4, 5, 5, 6, 7)                  | {0, 12689, 13679, 2378}                                                                                   | ✓                  |
| 941:408a | $0, 0, 0, 0, 0, e^{12}, e^{13}, e^{14} + e^{23}, e^{25} + e^{38} + e^{47} + e^{16}$                         | 5/32(3, 4, 3, 4, 6, 7, 6, 7, 10)                   | {0, 12349, 12789, 1368, 1467, 23679, 24689, 3478}                                                         |                    |
| 941:408b | $0, 0, 0, 0, 0, -e^{12}, e^{13}, e^{23} + e^{14}, e^{25} + e^{16} + e^{38} + e^{47}$                        | 5/32(3, 4, 3, 4, 6, 7, 6, 7, 10)                   | {0, 12349, 12789, 1368, 1467, 23679, 24689, 3478}                                                         |                    |
| 941:409  | $0, 0, 0, 0, 0, a_1 e^{12}, (1 + a_1) e^{13}, e^{23} + e^{14}, e^{27} + e^{18} + e^{36} + e^{45}$           | 1/7(3, 4, 4, 5, 6, 7, 7, 8, 11)                    | {0, 12349, 1278, 1368, 14679, 2367, 24689, 34789}                                                         |                    |
| 941:410  | $0, 0, 0, 0, 0, e^{12}, e^{34}, e^{24} - e^{13}, e^{17} + e^{26} + e^{35} + e^{48}$                         | 5/148(14, 16, 17, 15, 29, 30, 32, 31, 46)          | {0, 12349, 12589, 3458}                                                                                   |                    |
| 941:414a | $0, 0, 0, 0, 0, (-1 + a_2) e^{12}, e^{14} + e^{23}, a_2 e^{13} + e^{24}, e^{28} + e^{36} + e^{45} + e^{17}$ | 5/32(3, 3, 4, 4, 6, 6, 7, 7, 10)                   | {0, 12349, 1278, 1367, 14689, 2368, 24679, 34789}                                                         |                    |
| 941:414b | $0, 0, 0, 0, 0, (-1 + a_2) e^{12}, e^{23} - e^{14}, a_2 e^{13} + e^{24}, e^{28} + e^{17} + e^{36} + e^{45}$ | 5/32(3, 3, 4, 4, 6, 6, 7, 7, 10)                   | {0, 12349, 1278, 1367, 14689, 2368, 24679, 34789}                                                         |                    |
| 941:417  | $0, 0, 0, 0, 0, e^{24} + e^{13}, e^{23} + e^{15}, e^{14}, e^{17} + e^{26}$                                  | 1/31(11, 12, 23, 22, 24, 34, 35, 33, 46)           | {0, 123459, 12678, 1378, 14569, 236, 245789, 3456789}                                                     |                    |
| 941:418  | $0, 0, 0, 0, 0, e^{24} + e^{13}, e^{12} + e^{35}, e^{14}, e^{37} + e^{26}$                                  | 1/28(18, 13, 11, 16, 20, 29, 31, 34, 42)           | {0, 123459, 1268, 1378, 145679, 2367, 245789, 345689}                                                     |                    |
| 941:419  | $0, 0, 0, 0, 0, e^{14} + e^{23}, e^{13} + e^{25}, e^{45}, e^{16} + e^{27}$                                  | 1/16(7, 7, 10, 10, 10, 17, 17, 20, 24)             | {0, 123459, 1267, 136, 14579, 237, 24569, 345679}                                                         |                    |
| 941:422  | $0, 0, 0, 0, 0, e^{14} + e^{23}, e^{13} + e^{25}, e^{15} + e^{24}, e^{27} + e^{16}$                         | 7/19(1, 1, 2, 2, 2, 3, 3, 3, 4)                    | {0, 123459, 12678, 3456789}                                                                               |                    |
| 941:428  | $0, 0, 0, 0, 0, e^{34} - e^{12}, e^{15} + e^{23}, e^{14}, e^{17} + e^{25} + e^{36}$                         | 1/317(116, 232, 125, 223, 241, 348, 357, 339, 473) | {0, 13678, 14569, 345789}                                                                                 |                    |
| 941:441  | $0, 0, 0, 0, 0, e^{12}, e^{13}, e^{45}, e^{36} + e^{48} + e^{27}$                                           | 1/60(30, 33, 33, 28, 40, 63, 63, 68, 96)           | {0, 123459, 123589, 12478, 127, 13468, 136, 145679, 156789, 234678, 2367, 24569, 25689, 34579, 35789, 48} |                    |
| 941:442  | $0, 0, 0, 0, 0, e^{12}, e^{13}, e^{25} + e^{14}, e^{17} + e^{28} + e^{46}$                                  | 1/7(3, 3, 5, 5, 5, 6, 8, 8, 11)                    | {0, 123459, 1278, 135689, 1467, 235679, 2468, 345789}                                                     |                    |
| 941:443  | $0, 0, 0, 0, 0, -e^{12}, e^{13}, e^{15} + e^{24}, e^{37} + e^{46} + e^{18}$                                 | 1/225(80, 139, 136, 133, 192, 219, 216, 272, 352)  | {0, 123459, 124579, 13569, 15679, 23467, 246, 37}                                                         |                    |
| 941:444  | $0, 0, 0, 0, 0, e^{12}, e^{13}, e^{25} + e^{14}, e^{28} + e^{37} + e^{46}$                                  | 1/40(20, 17, 22, 27, 30, 37, 42, 47, 64)           | {0, 123459, 124579, 135689, 156789, 234678, 2468, 37}                                                     |                    |
| 941:445  | $0, 0, 0, 0, 0, -e^{12}, e^{34}, e^{15} + e^{23}, e^{47} + e^{36} + e^{18}$                                 | 1/49(19, 33, 24, 26, 38, 52, 50, 57, 76)           | {0, 123459, 123579, 12478, 128, 34589, 35789, 47}                                                         |                    |
| 941:447  | $0, 0, 0, 0, 0, -e^{12}, -e^{13}, e^{35} + e^{24}, e^{18} + e^{46} + e^{57}$                                | 1/5(2, 3, 3, 3, 3, 5, 5, 6, 8)                     | {0, 123459, 1238, 12479, 12578, 13468, 13569, 145678, 1679, 234567, 236789, 246, 25689, 34789, 357, 4589} |                    |
| 941:448a | $0, 0, 0, 0, 0, -e^{12}, e^{34}, e^{13} + e^{25}, e^{47} + e^{18} + e^{56}$                                 | 1/65(32, 35, 40, 32, 37, 67, 72, 72, 104)          | {0, 123459, 123579, 12478, 128, 13469, 13679, 145678, 1568, 234689, 236789, 24567, 256, 34589, 35789, 47} |                    |

Table A.4 – Continued to next page

Table A.4 – Continued from previous page

| Name     | g                                                                                                      | N                                                    | S <sub>0</sub>                                                                                                        | S = S <sub>0</sub> |
|----------|--------------------------------------------------------------------------------------------------------|------------------------------------------------------|-----------------------------------------------------------------------------------------------------------------------|--------------------|
| 941:448b | $0, 0, 0, 0, 0, -e^{12}, e^{34}, -e^{13} + e^{25}, e^{18} + e^{56} + e^{47}$                           | $1/65(32, 35, 40, 32, 37, 67, 72, 72, 104)$          | $\{\emptyset, 123459, 123579, 12478, 128, 13469, 13679, 145678, 1568, 234689, 236789, 24567, 256, 34589, 35789, 47\}$ |                    |
| 941:452  | $0, 0, 0, 0, 0, (-1 + a_2)e^{12}, e^{23} + e^{14}, a_2e^{13} + e^{25}, e^{17} + e^{28} + e^{36}$       | $1/7(3, 3, 5, 5, 5, 6, 8, 8, 11)$                    | $\{\emptyset, 123459, 1278, 1367, 145689, 2368, 245679, 345789\}$                                                     |                    |
| 941:453  | $0, 0, 0, 0, 0, e^{12}, e^{23} + e^{14}, e^{15} + e^{34}, e^{18} + e^{26} + e^{37}$                    | $1/175(65, 103, 84, 122, 141, 168, 187, 206, 271)$   | $\{\emptyset, 123459, 12579, 347\}$                                                                                   |                    |
| 941:455  | $0, 0, 0, 0, 0, e^{12}, e^{14} + e^{23}, e^{13} + e^{45}, e^{48} + e^{26} + e^{37}$                    | $7/116(10, 8, 9, 7, 12, 18, 17, 19, 26)$             | $\{\emptyset, 123459, 125789, 3478\}$                                                                                 |                    |
| 941:458  | $0, 0, 0, 0, 0, e^{12}, e^{24} + e^{13}, e^{34} + e^{15}, e^{28} + e^{37} + e^{56}$                    | $1/55(30, 24, 29, 35, 34, 54, 59, 64, 88)$           | $\{\emptyset, 123459, 12579, 13689, 146789, 235678, 24568, 347\}$                                                     |                    |
| 941:459a | $0, 0, 0, 0, 0, e^{14} + e^{23}, e^{24} + e^{13}, e^{15}, e^{16} + e^{27} + e^{58}$                    | $2/131(28, 28, 46, 46, 37, 74, 74, 65, 102)$         | $\{\emptyset, 123459, 123489, 14579, 14789, 23578, 237, 58\}$                                                         | ✓                  |
| 941:459b | $0, 0, 0, 0, 0, -e^{14} + e^{23}, e^{13} + e^{24}, e^{15}, e^{27} + e^{16} + e^{58}$                   | $2/131(28, 28, 46, 46, 37, 74, 74, 65, 102)$         | $\{\emptyset, 123459, 123489, 14579, 14789, 23578, 237, 58\}$                                                         | ✓                  |
| 941:460a | $0, 0, 0, 0, 0, e^{24} + e^{13}, e^{34} + e^{12}, e^{15}, e^{58} + e^{26} + e^{37}$                    | $2/35(10, 9, 9, 10, 9, 19, 19, 19, 28)$              | $\{\emptyset, 123459, 123489, 145679, 146789, 235678, 2367, 58\}$                                                     | ✓                  |
| 941:460b | $0, 0, 0, 0, 0, -e^{24} + e^{13}, e^{12} + e^{34}, e^{15}, e^{37} + e^{26} + e^{58}$                   | $2/35(10, 9, 9, 10, 9, 19, 19, 19, 28)$              | $\{\emptyset, 123459, 123489, 145679, 146789, 235678, 2367, 58\}$                                                     | ✓                  |
| 941:461a | $0, 0, 0, 0, 0, e^{24} + e^{13}, e^{12} + e^{34}, e^{15}, e^{58} + e^{36} + e^{27}$                    | $2/35(10, 9, 9, 10, 9, 19, 19, 19, 28)$              | $\{\emptyset, 123459, 123489, 12569, 12689, 13579, 13789, 145679, 146789, 235678, 2367, 24578, 247, 34568, 346, 58\}$ | ✓                  |
| 941:461b | $0, 0, 0, 0, 0, e^{13} + e^{24}, -e^{12} + e^{34}, e^{15}, e^{58} + e^{27} + e^{36}$                   | $2/35(10, 9, 9, 10, 9, 19, 19, 19, 28)$              | $\{\emptyset, 123459, 123489, 12569, 12689, 13579, 13789, 145679, 146789, 235678, 2367, 24578, 247, 34568, 346, 58\}$ | ✓                  |
| 941:461c | $0, 0, 0, 0, 0, e^{24} - e^{13}, e^{34} - e^{12}, e^{15}, e^{27} + e^{36} + e^{58}$                    | $2/35(10, 9, 9, 10, 9, 19, 19, 19, 28)$              | $\{\emptyset, 123459, 123489, 12569, 12689, 13579, 13789, 145679, 146789, 235678, 2367, 24578, 247, 34568, 346, 58\}$ | ✓                  |
| 941:462a | $0, 0, 0, 0, 0, e^{12}, e^{35} + e^{14}, e^{45} + e^{23}, e^{16} + e^{47} + e^{38}$                    | $1/47(23, 29, 23, 26, 26, 52, 49, 52, 75)$           | $\{\emptyset, 123459, 12379, 12489, 125789, 3478, 358, 457\}$                                                         |                    |
| 941:462b | $0, 0, 0, 0, 0, -e^{12}, e^{14} + e^{35}, e^{23} + e^{45}, e^{16} + e^{38} + e^{47}$                   | $1/47(23, 29, 23, 26, 26, 52, 49, 52, 75)$           | $\{\emptyset, 123459, 12379, 12489, 125789, 3478, 358, 457\}$                                                         |                    |
| 941:463  | $0, 0, 0, 0, 0, -e^{12}, e^{34} + e^{15}, e^{45} + e^{23}, e^{36} + e^{47} + e^{18}$                   | $1/31(13, 19, 17, 16, 20, 32, 33, 36, 49)$           | $\{\emptyset, 123459, 12379, 12478, 1258, 3489, 35789, 457\}$                                                         |                    |
| 941:472  | $0, 0, 0, 0, 0, e^{24} + e^{13}, e^{15} + e^{23}, e^{45} + e^{12}, e^{18} + e^{47} + e^{36}$           | $1/329(163, 195, 179, 147, 211, 342, 374, 358, 521)$ | $\{\emptyset, 123459, 12679, 34567\}$                                                                                 |                    |
| 941:473  | $0, 0, 0, 0, 0, e^{13} + e^{24}, e^{15} + e^{23}, e^{25} + e^{14}, e^{47} + e^{58} + e^{36}$           | $2/35(10, 10, 9, 9, 9, 19, 19, 19, 28)$              | $\{\emptyset, 123459, 126789, 345678\}$                                                                               |                    |
| 931:101  | $0, 0, 0, 0, 0, 0, -e^{12}, e^{14} + e^{23}, e^{56} + e^{37} + e^{18}$                                 | $1/5(2, 3, 3, 4, 4, 4, 5, 6, 8)$                     | $\{\emptyset, 123459, 123469, 12568, 128, 135678, 1378, 14579, 14679, 23567, 237, 245789, 246789, 34589, 34689, 56\}$ |                    |
| 931:107a | $0, 0, 0, 0, 0, 0, e^{14} + e^{23}, e^{13} + e^{24}, e^{17} + e^{28} + e^{56}$                         | $1/15(7, 7, 10, 10, 12, 12, 17, 17, 24)$             | $\{\emptyset, 123459, 123469, 125678, 1278, 13567, 137, 14589, 14689, 23568, 238, 24579, 24679, 345789, 346789, 56\}$ | ✓                  |
| 931:107b | $0, 0, 0, 0, 0, 0, -e^{14} + e^{23}, e^{13} + e^{24}, e^{17} + e^{56} + e^{28}$                        | $1/15(7, 7, 10, 10, 12, 12, 17, 17, 24)$             | $\{\emptyset, 123459, 123469, 125678, 1278, 13567, 137, 14589, 14689, 23568, 238, 24579, 24679, 345789, 346789, 56\}$ | ✓                  |
| 931:111a | $0, 0, 0, 0, 0, 0, e^{24} + e^{13}, e^{34} - e^{12}, e^{17} + e^{25} + e^{36} + e^{48}$                | $5/32(3, 4, 4, 3, 6, 6, 7, 7, 10)$                   | $\{\emptyset, 12349, 1257, 13589, 1478, 23789, 2458, 34579\}$                                                         | ✓                  |
| 931:111b | $0, 0, 0, 0, 0, 0, -e^{13} + e^{24}, -e^{12} + e^{34}, e^{48} + e^{17} + e^{36} + e^{25}$              | $5/32(3, 4, 4, 3, 6, 6, 7, 7, 10)$                   | $\{\emptyset, 12349, 1257, 13589, 1478, 23789, 2458, 34579\}$                                                         | ✓                  |
| 931:115  | $0, 0, 0, 0, 0, 0, e^{13} + e^{24}, e^{12} + e^{35}, e^{27} + e^{16} + e^{38}$                         | $1/7(5, 3, 3, 5, 5, 6, 8, 8, 11)$                    | $\{\emptyset, 123459, 1267, 1368, 145789, 2378, 245689, 345679\}$                                                     |                    |
| 931:116  | $0, 0, 0, 0, 0, 0, e^{14} + e^{23}, e^{13} + e^{25}, e^{17} + e^{46} + e^{28}$                         | $1/25(11, 10, 18, 17, 19, 22, 28, 29, 39)$           | $\{\emptyset, 123459, 1278, 137, 14589, 238, 24579, 345789\}$                                                         |                    |
| 93:66    | $0, 0, 0, 0, 0, 0, a_1e^{14} + e^{23}, e^{26} + e^{15}, e^{46} + e^{35}$                               | $2/3(1, 1, 1, 1, 1, 1, 2, 2, 2)$                     | $\{\emptyset, 123456, 123489, 125679, 1278, 1357, 136789, 1459, 1468, 2358, 2369, 245789, 2467, 345678, 3479, 5689\}$ | ✓                  |
| 93:86    | $0, 0, 0, 0, 0, 0, a_1e^{15} + e^{24} + e^{36}, e^{25} + e^{13} + e^{46}, e^{34} + e^{12} + e^{56}$    | $2/3(1, 1, 1, 1, 1, 1, 2, 2, 2)$                     | $\{\emptyset, 123456\}$                                                                                               |                    |
| 93:87    | $0, 0, 0, 0, 0, 0, a_1e^{16} + e^{24} + e^{35}, a_2e^{13} + e^{25} + e^{46}, e^{12} + e^{34} + e^{56}$ | $2/3(1, 1, 1, 1, 1, 1, 2, 2, 2)$                     | $\{\emptyset, 123456, 145789, 236789\}$                                                                               | ✓                  |

End of Table A.4
